# Supplementary material for: N=4 conformal supergravity: the complete actions
Source: arXiv:1910.11874 ancillary file (2019-10-31)
Supplement: Supplementary file 1 [file FullComps.pdf]

# Full component expressions for the $4D \mathcal{N} = 4$ conformal supergravity action

Collected below are results for the various components needed to construct the full actions discussed in the main body of the paper. Each block is grouped by the number of fermions with a subscript.

## The $F$ block

The zero fermion terms are:

$$\begin{aligned}
F_0 = & \left( \frac{1}{2} \mathcal{D}^\dagger \bar{\mathcal{H}} + \mathcal{D} \bar{\mathcal{I}} \right) \nabla_a \nabla_a \nabla_b P_b + \left( \mathcal{D}^\dagger \mathcal{I} + \frac{1}{2} \mathcal{D} \mathcal{H} \right) \nabla_a \nabla_a \nabla_b \bar{P}_b - 4 \bar{\mathcal{I}} P_a \nabla_a \nabla_b P_b - 4 \bar{\mathcal{I}} P_a \nabla_b \nabla_a P_a - 2 \bar{\mathcal{I}} \nabla_a P_a \nabla_b P_b - 4 \bar{\mathcal{I}} \nabla_a P_b \nabla_a P_b \\
& - 4 \mathcal{I} \bar{P}_a \nabla_a \nabla_b \bar{P}_b - 4 \mathcal{I} \bar{P}_a \nabla_b \nabla_a \bar{P}_a - 2 \mathcal{I} \nabla_a \bar{P}_a \nabla_b \bar{P}_b - 4 \mathcal{I} \nabla_a \bar{P}_b \nabla_a \bar{P}_b + \left( -\frac{1}{18} \bar{\mathcal{H}} + \frac{1}{18} \mathcal{H} \right) \nabla_a T_{abij} \nabla_c T_{bc}{}^{ij} + \left( -\frac{1}{18} \bar{\mathcal{H}} + \frac{1}{18} \mathcal{H} \right) \nabla_a T_{bcij} \nabla_b T_{ac}{}^{ij} \\
& + \left( \frac{1}{36} \bar{\mathcal{H}} - \frac{1}{36} \mathcal{H} \right) \nabla_a T_{bcij} \nabla_a T_{bc}{}^{ij} + \left( \frac{1}{8} \bar{\mathcal{H}} + \frac{1}{8} \mathcal{H} \right) D^{ij}{}_{kl} D^{kl}{}_{ij} + \left( \frac{1}{8} \bar{\mathcal{H}} + \frac{1}{8} \mathcal{H} \right) E_{ij} \nabla_a \nabla_a E^{ij} + \left( \frac{1}{8} \bar{\mathcal{H}} + \frac{1}{8} \mathcal{H} \right) E^{ij} \nabla_a \nabla_a E_{ij} \\
& + \left( \frac{1}{4} \bar{\mathcal{H}} + \frac{1}{4} \mathcal{H} \right) R(M)_{abcd} R(M)_{abcd} + \left( \frac{1}{2} \bar{\mathcal{H}} + \frac{1}{2} \mathcal{H} \right) R(V)_{ab}{}^i{}_j R(V)_{ab}{}^j{}_i + (2 \bar{\mathcal{H}} + 2 \mathcal{H}) T_{abij} \nabla_a \nabla_c T_{bc}{}^{ij} + (2 \bar{\mathcal{H}} + 2 \mathcal{H}) T_{ab}{}^{ij} \nabla_a \nabla_c T_{bcij} \\
& + E_{ij} T_{ab}{}^{ik} \mathcal{D} \mathcal{H} R(V)_{ab}{}^j{}_k - E^{ij} T_{abik} \mathcal{D}^\dagger \bar{\mathcal{H}} R(V)_{ab}{}^k{}_j - 4 \mathcal{D}^\dagger \bar{\mathcal{I}} P_a P_a \nabla_b P_b - 8 \mathcal{D}^\dagger \bar{\mathcal{I}} P_a P_b \nabla_a P_b - 4 \mathcal{D} \mathcal{I} \bar{P}_a \bar{P}_a \nabla_b \bar{P}_b - 8 \mathcal{D} \mathcal{I} \bar{P}_a \bar{P}_b \nabla_a \bar{P}_b \\
& + (-6 \mathcal{D}^\dagger \mathcal{I} - 3 \mathcal{D} \mathcal{H}) P_a \bar{P}_b \nabla_a \bar{P}_b + \left( -\frac{9}{2} \mathcal{D}^\dagger \bar{\mathcal{H}} - 3 \mathcal{D} \bar{\mathcal{I}} \right) P_a T_{bc}{}^{ij} \nabla_b T_{acij} + (-3 \mathcal{D}^\dagger \bar{\mathcal{H}} - 6 \mathcal{D} \bar{\mathcal{I}}) P_a \bar{P}_b \nabla_b P_a + \left( -\frac{8}{3} \mathcal{D}^\dagger \mathcal{I} - \frac{4}{3} \mathcal{D} \mathcal{H} \right) P_a \bar{P}_a \nabla_b \bar{P}_b \\
& + (-2 \mathcal{D}^\dagger \bar{\mathcal{H}} - 2 \mathcal{D} \bar{\mathcal{I}}) T_{abij} T_{ac}{}^{ij} \nabla_b P_c + (-2 \mathcal{D}^\dagger \bar{\mathcal{H}} - 2 \mathcal{D} \bar{\mathcal{I}}) T_{abij} T_{ac}{}^{ij} \nabla_c P_b + (-2 \mathcal{D}^\dagger \mathcal{I} - 2 \mathcal{D} \mathcal{H}) T_{abij} T_{ac}{}^{ij} \nabla_b \bar{P}_c \\
& + (-2 \mathcal{D}^\dagger \mathcal{I} - 2 \mathcal{D} \mathcal{H}) T_{abij} T_{ac}{}^{ij} \nabla_c \bar{P}_b + \left( -\frac{4}{3} \mathcal{D}^\dagger \bar{\mathcal{H}} - \frac{8}{3} \mathcal{D} \bar{\mathcal{I}} \right) P_a \bar{P}_a \nabla_b P_b + \left( -\mathcal{D}^\dagger \mathcal{I} - \frac{1}{2} \mathcal{D} \mathcal{H} \right) T_{ab}{}^{ij} \nabla_c \nabla_c T_{ab}{}^{kl} \varepsilon_{ijkl} \\
& + \left( -\mathcal{D}^\dagger \mathcal{I} - \frac{1}{2} \mathcal{D} \mathcal{H} \right) \nabla_a T_{bc}{}^{ij} \nabla_a T_{bc}{}^{kl} \varepsilon_{ijkl} + \left( -\frac{2}{3} \mathcal{D}^\dagger \mathcal{I} - \frac{1}{3} \mathcal{D} \mathcal{H} \right) \bar{P}_a \bar{P}_b \nabla_a P_b + \left( -\frac{1}{2} \mathcal{D}^\dagger \bar{\mathcal{H}} - \mathcal{D} \bar{\mathcal{I}} \right) P_a T_{bcij} \nabla_b T_{ac}{}^{ij} \\
& + \left( -\frac{1}{2} \mathcal{D}^\dagger \bar{\mathcal{H}} - \mathcal{D} \bar{\mathcal{I}} \right) T_{abij} \nabla_c \nabla_c T_{abkl} \varepsilon^{ijkl} + \left( -\frac{1}{2} \mathcal{D}^\dagger \bar{\mathcal{H}} - \mathcal{D} \bar{\mathcal{I}} \right) \nabla_a T_{bcij} \nabla_a T_{bckl} \varepsilon^{ijkl} + \left( -\frac{1}{3} \mathcal{D}^\dagger \bar{\mathcal{H}} - \frac{2}{3} \mathcal{D} \bar{\mathcal{I}} \right) P_a P_b \nabla_a \bar{P}_b \\
& + \left( -\frac{1}{12} \mathcal{D}^\dagger \mathcal{I} - \frac{1}{24} \mathcal{D} \mathcal{H} \right) E_{ij} \bar{P}_a \nabla_a E^{ij} + \left( -\frac{1}{12} \mathcal{D}^\dagger \mathcal{I} + \frac{1}{12} \mathcal{D} \mathcal{H} \right) E_{ij} E^{ij} \nabla_a \bar{P}_a + \left( -\frac{1}{12} \mathcal{D}^\dagger \mathcal{I} + \frac{5}{24} \mathcal{D} \mathcal{H} \right) E^{ij} \bar{P}_a \nabla_a E_{ij} \\
& + \left( -\frac{1}{24} \mathcal{D}^\dagger \bar{\mathcal{H}} - \frac{1}{12} \mathcal{D} \bar{\mathcal{I}} \right) E^{ij} P_a \nabla_a E_{ij} + \left( \frac{1}{12} \mathcal{D}^\dagger \bar{\mathcal{H}} - \frac{1}{12} \mathcal{D} \bar{\mathcal{I}} \right) E_{ij} E^{ij} \nabla_a P_a + \left( \frac{1}{8} \bar{\mathcal{H}} - \frac{1}{8} \mathcal{H} \right) R(M)_{abcd} R(M)_{abef} \varepsilon_{cdef} \\
& + \left( \frac{5}{24} \mathcal{D}^\dagger \bar{\mathcal{H}} - \frac{1}{12} \mathcal{D} \bar{\mathcal{I}} \right) E_{ij} P_a \nabla_a E^{ij} + \left( \frac{1}{4} \bar{\mathcal{H}} - \frac{1}{4} \mathcal{H} \right) R(V)_{ab}{}^i{}_j R(V)_{cd}{}^j{}_i \varepsilon_{abcd} + \left( \frac{1}{4} \mathcal{D}^\dagger \bar{\mathcal{H}} + \frac{1}{2} \mathcal{D} \bar{\mathcal{I}} \right) P_a T_{bcij} \nabla_a T_{bc}{}^{ij} \\
& + \left( \frac{1}{2} \mathcal{D}^\dagger \bar{\mathcal{H}} + \mathcal{D} \bar{\mathcal{I}} \right) \nabla_a T_{abij} \nabla_c T_{bckl} \varepsilon^{ijkl} + \left( \frac{1}{2} \mathcal{D}^\dagger \bar{\mathcal{H}} + \mathcal{D} \bar{\mathcal{I}} \right) \nabla_a T_{bcij} \nabla_b T_{ackl} \varepsilon^{ijkl} + \left( \frac{1}{2} \mathcal{D}^\dagger \mathcal{I} + \frac{1}{4} \mathcal{D} \mathcal{H} \right) T_{ab}{}^{ij} \bar{P}_c \nabla_c T_{abij} \\
& + \left( \frac{1}{2} \mathcal{D}^\dagger \mathcal{I} + \frac{3}{4} \mathcal{D} \mathcal{H} \right) T_{abij} \bar{P}_c \nabla_c T_{ab}{}^{ij} + \left( \frac{2}{3} \mathcal{D}^\dagger \bar{\mathcal{H}} + \frac{4}{3} \mathcal{D} \bar{\mathcal{I}} \right) P_a \bar{P}_b \nabla_a P_b + \left( \frac{3}{4} \mathcal{D}^\dagger \bar{\mathcal{H}} + \frac{1}{2} \mathcal{D} \bar{\mathcal{I}} \right) P_a T_{bc}{}^{ij} \nabla_a T_{bcij} + \left( \mathcal{D}^\dagger \mathcal{I} + \frac{1}{2} \mathcal{D} \mathcal{H} \right) T_{ab}{}^{ij} \bar{P}_a \nabla_c T_{bcij} \\
& + \left( \mathcal{D}^\dagger \mathcal{I} + \frac{1}{2} \mathcal{D} \mathcal{H} \right) \nabla_a T_{ab}{}^{ij} \nabla_c T_{bc}{}^{kl} \varepsilon_{ijkl} + \left( \mathcal{D}^\dagger \mathcal{I} + \frac{1}{2} \mathcal{D} \mathcal{H} \right) \nabla_a T_{bc}{}^{ij} \nabla_b T_{ac}{}^{kl} \varepsilon_{ijkl} + \left( \mathcal{D}^\dagger \mathcal{I} + \frac{3}{2} \mathcal{D} \mathcal{H} \right) T_{abij} \bar{P}_c \nabla_a T_{bc}{}^{ij} \\
& + \left( \frac{4}{3} \mathcal{D}^\dagger \mathcal{I} + \frac{2}{3} \mathcal{D} \mathcal{H} \right) P_a \bar{P}_b \nabla_b \bar{P}_a + \left( \frac{3}{2} \mathcal{D}^\dagger \bar{\mathcal{H}} + \mathcal{D} \bar{\mathcal{I}} \right) P_a T_{ab}{}^{ij} \nabla_c T_{bcij} + \left( \frac{3}{2} \mathcal{D}^\dagger \bar{\mathcal{H}} + 3 \mathcal{D} \bar{\mathcal{I}} \right) P_a T_{abij} \nabla_c T_{bc}{}^{ij} + \left( 3 \mathcal{D}^\dagger \mathcal{I} + \frac{3}{2} \mathcal{D} \mathcal{H} \right) T_{ab}{}^{ij} \bar{P}_c \nabla_a T_{bcij} \\
& + \left( 3 \mathcal{D}^\dagger \mathcal{I} + \frac{9}{2} \mathcal{D} \mathcal{H} \right) T_{abij} \bar{P}_a \nabla_c T_{bc}{}^{ij} + \frac{1}{16} D^{ij}{}_{kl} E_{im} E_{jn} \mathcal{D} \mathcal{H} \varepsilon^{klmn} + \frac{1}{16} D^{ij}{}_{kl} E^{km} E^{ln} \mathcal{D}^\dagger \bar{\mathcal{H}} \varepsilon_{ijmn} - \frac{1}{8} D^{ij}{}_{kl} T_{abmn} T_{abij} \mathcal{D}^\dagger \bar{\mathcal{H}} \varepsilon^{klmn} \\
& - \frac{1}{8} D^{ij}{}_{kl} T_{ab}{}^{mn} T_{ab}{}^{kl} \mathcal{D} \mathcal{H} \varepsilon_{ijmn} - \frac{1}{8} E_{ij} E_{kl} T_{ab}{}^{ik} T_{ab}{}^{jl} \mathcal{D} \mathcal{D} \mathcal{H} - \frac{1}{8} E^{ij} E^{kl} T_{abik} T_{abjl} \mathcal{D}^\dagger \mathcal{D}^\dagger \bar{\mathcal{H}} - \frac{1}{3} T_{abij} \bar{\mathcal{H}} \bar{P}_c \nabla_c T_{abkl} \varepsilon^{ijkl} + \frac{40}{3} \bar{\mathcal{I}} P_a P_a P_b \bar{P}_b \\
& - 2 \bar{\mathcal{I}} P_a T_{abij} \nabla_c T_{bckl} \varepsilon^{ijkl} + \frac{14}{3} \bar{\mathcal{I}} P_a T_{bcij} \nabla_a T_{bckl} \varepsilon^{ijkl} - 2 \bar{\mathcal{I}} P_a T_{bcij} \nabla_b T_{ackl} \varepsilon^{ijkl} + \frac{4}{3} \bar{\mathcal{I}} T_{abij} T_{abkl} \nabla_c P_c \varepsilon^{ijkl} - \bar{\mathcal{H}} P_a T_{ab}{}^{ij} \nabla_c T_{bc}{}^{kl} \varepsilon_{ijkl} + \dots
\end{aligned}$$

$$\begin{aligned}
F_{0,cont} = & -\bar{\mathcal{H}}P_aT_{bc}{}^{ij}\nabla_bT_{ac}{}^{kl}\varepsilon_{ijkl}-2\mathcal{D}^\dagger\mathcal{D}^\dagger\bar{\mathcal{L}}P_aP_aP_bP_b-2\mathcal{D}^\dagger\mathcal{I}T_{ab}{}^{ij}T_{ac}{}^{kl}R(V)_{bc}{}^m{}_k\varepsilon_{ijlm}-2\mathcal{D}\bar{\mathcal{L}}T_{abij}T_{ackl}R(V)_{bc}{}^i{}_m\varepsilon^{ijklm} \\
& -2\mathcal{D}\mathcal{D}\bar{\mathcal{L}}\bar{P}_a\bar{P}_a\bar{P}_b\bar{P}_b+\frac{40}{3}\mathcal{I}P_a\bar{P}_a\bar{P}_b\bar{P}_b+\frac{4}{3}\mathcal{I}T_{ab}{}^{ij}T_{ab}{}^{kl}\nabla_c\bar{P}_c\varepsilon_{ijkl}-2\mathcal{I}T_{ab}{}^{ij}\bar{P}_a\nabla_cT_{bc}{}^{kl}\varepsilon_{ijkl}+2\mathcal{I}T_{ab}{}^{ij}\bar{P}_c\nabla_aT_{bc}{}^{kl}\varepsilon_{ijkl} \\
& +\frac{14}{3}\mathcal{I}T_{ab}{}^{ij}\bar{P}_c\nabla_cT_{ab}{}^{kl}\varepsilon_{ijkl}-\frac{1}{3}\mathcal{H}P_aT_{bc}{}^{ij}\nabla_aT_{bc}{}^{kl}\varepsilon_{ijkl}-\mathcal{H}T_{abij}\bar{P}_a\nabla_cT_{bckl}\varepsilon^{ijkl}+\mathcal{H}T_{abij}\bar{P}_c\nabla_aT_{bckl}\varepsilon^{ijkl}+(-3\bar{\mathcal{H}}-3\mathcal{H})P_aT_{abij}T_{bc}{}^{ij}\bar{P}_c \\
& +(-2\mathcal{D}\mathcal{D}\mathcal{H}+8\mathcal{I})T_{abij}T_{ac}{}^{ij}\bar{P}_b\bar{P}_c+(-\bar{\mathcal{L}}+\frac{1}{4}\mathcal{D}^\dagger\mathcal{D}^\dagger\bar{\mathcal{H}})P_aP_aT_{bcij}T_{bc}{}^{ij}+(-\bar{\mathcal{H}}-\mathcal{H})P_aT_{bcij}T_{ab}{}^{ij}\bar{P}_c+(-\bar{\mathcal{H}}-\mathcal{H})T_{abij}T_{cdkl}T_{ac}{}^{ik}T_{bd}{}^{jl} \\
& +(-\frac{3}{4}\bar{\mathcal{H}}-\frac{3}{4}\mathcal{H})T_{abij}T_{abkl}T_{cd}{}^{ik}T_{cd}{}^{jl}+(-\frac{1}{2}\bar{\mathcal{H}}-\frac{1}{2}\mathcal{H})E^{ij}T_{ab}{}^{kl}R(V)_{ab}{}^m{}_i\varepsilon_{ijklm}+(-\frac{1}{2}\bar{\mathcal{H}}-\frac{1}{2}\mathcal{H})P_aT_{bcij}T_{bc}{}^{ij}\bar{P}_a \\
& +(-\frac{1}{2}\bar{\mathcal{H}}-\frac{1}{6}\mathcal{H})T_{ab}{}^{ij}T_{ab}{}^{kl}\nabla_cP_c\varepsilon_{ijkl}+(-\frac{1}{3}\bar{\mathcal{H}}-\frac{1}{3}\mathcal{H})P_aP_b\bar{P}_a\bar{P}_b+(-\frac{1}{4}\bar{\mathcal{H}}-\frac{1}{4}\mathcal{H})E_{ij}E^{ij}P_a\bar{P}_a+(-\frac{1}{4}\bar{\mathcal{H}}-\frac{1}{4}\mathcal{H})T_{abij}T_{cdkl}T_{ab}{}^{ij}T_{cd}{}^{kl} \\
& +(-\frac{1}{4}\bar{\mathcal{H}}-\frac{1}{4}\mathcal{H})T_{abij}T_{cdkl}T_{ab}{}^{kl}T_{cd}{}^{ij}+(-\frac{1}{6}\bar{\mathcal{H}}-\frac{1}{2}\mathcal{H})T_{abij}T_{abkl}\nabla_c\bar{P}_c\varepsilon^{ijkl}+(-\frac{1}{16}\bar{\mathcal{H}}-\frac{1}{16}\mathcal{H})E_{ij}E_{kl}E^{ik}E^{jl} \\
& +(\frac{1}{48}\bar{\mathcal{H}}+\frac{1}{48}\mathcal{H})E_{ij}E_{kl}E^{ij}E^{kl}+(\frac{1}{8}\mathcal{D}\mathcal{D}\mathcal{H}+\frac{1}{6}\mathcal{I})E_{ij}E^{ij}\bar{P}_a\bar{P}_a+(\frac{1}{6}\bar{\mathcal{L}}+\frac{1}{8}\mathcal{D}^\dagger\mathcal{D}^\dagger\bar{\mathcal{H}})E_{ij}E^{ij}P_aP_a+(\frac{1}{4}\mathcal{D}\mathcal{D}\mathcal{H}-\mathcal{I})T_{abij}T_{ab}{}^{ij}\bar{P}_c\bar{P}_c \\
& +(\frac{1}{2}\bar{\mathcal{H}}+\frac{1}{2}\mathcal{H})E_{ij}T_{abkl}R(V)_{ab}{}^i{}_m\varepsilon^{ijklm}+(\frac{1}{2}\bar{\mathcal{H}}+\frac{1}{2}\mathcal{H})T_{abij}T_{cdkl}T_{ab}{}^{ik}T_{cd}{}^{jl}+(\frac{1}{2}\mathcal{D}^\dagger\bar{\mathcal{H}}+\frac{1}{2}\mathcal{D}\bar{\mathcal{L}})T_{abij}T_{cdkl}R(M)_{abcd}\varepsilon^{ijkl} \\
& +(\frac{1}{2}\mathcal{D}^\dagger\mathcal{I}+\frac{1}{2}\mathcal{D}\mathcal{H})T_{ab}{}^{ij}T_{cd}{}^{kl}R(M)_{abcd}\varepsilon_{ijkl}+(\frac{3}{4}\bar{\mathcal{H}}+\frac{3}{4}\mathcal{H})T_{abij}T_{abkl}T_{cd}{}^{ij}T_{cd}{}^{kl}+(\bar{\mathcal{H}}+\mathcal{H})P_aP_a\bar{P}_b\bar{P}_b+(\bar{\mathcal{H}}+\mathcal{H})T_{abij}T_{cdkl}T_{ac}{}^{ij}T_{bd}{}^{kl} \\
& +(8\bar{\mathcal{L}}-2\mathcal{D}^\dagger\mathcal{D}^\dagger\bar{\mathcal{H}})P_aP_bT_{acij}T_{bc}{}^{ij}-\frac{1}{24}E_{ij}E^{ij}T_{abkl}T_{abmn}\mathcal{D}^\dagger\bar{\mathcal{H}}\varepsilon^{klmn}-\frac{1}{24}E_{ij}E^{ij}T_{ab}{}^{kl}T_{ab}{}^{mn}\mathcal{D}\mathcal{H}\varepsilon_{klmn} \\
& -\frac{1}{6}E_{ij}T_{ab}{}^{ik}T_{ac}{}^{lm}T_{bc}{}^{jn}\mathcal{D}\mathcal{D}\mathcal{H}\varepsilon_{klmn}-\frac{1}{6}E^{ij}T_{abik}T_{aclm}T_{bcjn}\mathcal{D}^\dagger\mathcal{D}^\dagger\bar{\mathcal{H}}\varepsilon^{klmn}+\frac{4}{3}\mathcal{D}^\dagger\bar{\mathcal{L}}P_aP_aT_{bcij}T_{bckl}\varepsilon^{ijkl} \\
& -\frac{1}{2}\mathcal{D}^\dagger\bar{\mathcal{H}}P_aP_aT_{bc}{}^{ij}T_{bc}{}^{kl}\varepsilon_{ijkl}+\frac{4}{3}\mathcal{D}\mathcal{I}T_{ab}{}^{ij}T_{ab}{}^{kl}\bar{P}_c\bar{P}_c\varepsilon_{ijkl}-\frac{1}{2}\mathcal{D}\mathcal{H}T_{abij}T_{abkl}\bar{P}_c\bar{P}_c\varepsilon^{ijkl}+(\frac{1}{2}\mathcal{D}^\dagger\bar{\mathcal{H}}+\frac{4}{3}\mathcal{D}\bar{\mathcal{L}})P_aT_{bcij}T_{bckl}\bar{P}_a\varepsilon^{ijkl} \\
& +(\frac{4}{3}\mathcal{D}^\dagger\mathcal{I}+\frac{1}{2}\mathcal{D}\mathcal{H})P_aT_{bc}{}^{ij}T_{bc}{}^{kl}\bar{P}_a\varepsilon_{ijkl}+\frac{1}{384}E_{ij}E_{kl}E_{mn}E_{pq}\mathcal{D}\mathcal{D}\mathcal{H}\varepsilon^{ikmp}\varepsilon^{jlnq}-\frac{1}{6}E_{ij}T_{abkl}T_{acmn}T_{bcpq}\mathcal{D}^\dagger\bar{\mathcal{H}}\varepsilon^{iklm}\varepsilon^{jnpq} \\
& +\frac{1}{384}E^{ij}E^{kl}E^{mn}E^{pq}\mathcal{D}^\dagger\mathcal{D}^\dagger\bar{\mathcal{H}}\varepsilon_{ikmp}\varepsilon_{jlnq}-\frac{1}{6}E^{ij}T_{ab}{}^{kl}T_{ac}{}^{mn}T_{bc}{}^{pq}\mathcal{D}\mathcal{H}\varepsilon_{iklm}\varepsilon_{jnpq}-\frac{1}{64}T_{abij}T_{abkl}T_{cdmn}T_{cdpq}\mathcal{D}^\dagger\mathcal{D}^\dagger\bar{\mathcal{H}}\varepsilon^{ijkl}\varepsilon^{mnpq} \\
& +\frac{1}{32}T_{abij}T_{abkl}T_{cdmn}T_{cdpq}\mathcal{D}^\dagger\mathcal{D}^\dagger\bar{\mathcal{H}}\varepsilon^{ijmn}\varepsilon^{klpq}-\frac{1}{64}T_{ab}{}^{ij}T_{ab}{}^{kl}T_{cd}{}^{mn}T_{cd}{}^{pq}\mathcal{D}\mathcal{D}\mathcal{H}\varepsilon_{ijkl}\varepsilon_{mnpq}+\frac{1}{32}T_{ab}{}^{ij}T_{ab}{}^{kl}T_{cd}{}^{mn}T_{cd}{}^{pq}\mathcal{D}\mathcal{D}\mathcal{H}\varepsilon_{ijmn}\varepsilon_{klpq} \\
& +(-\frac{1}{16}\bar{\mathcal{H}}-\frac{1}{16}\mathcal{H})E_{ij}E_{kl}T_{abmn}T_{abpq}\varepsilon^{ikmn}\varepsilon^{jlpq}+(-\frac{1}{16}\bar{\mathcal{H}}-\frac{1}{16}\mathcal{H})E^{ij}E^{kl}T_{ab}{}^{mn}T_{ab}{}^{pq}\varepsilon_{ikmn}\varepsilon_{jlpq}
\end{aligned}$$

$$\begin{aligned}
F_2 = & -R(Q)_{ab}{}^{\dot{\alpha}}{}_i R(S)_{ab}{}^{\dot{\beta}i} \bar{\mathcal{H}} \epsilon_{\dot{\alpha}\dot{\beta}} - \mathcal{H} R(Q)_{ab\alpha}{}^i R(S)_{ab\beta i} \epsilon^{\alpha\beta} + \left(\frac{1}{8} \bar{\mathcal{H}} + \frac{3}{8} \mathcal{H}\right) \Lambda^{\dot{\alpha}i} \gamma_a{}^{\alpha}{}_{\dot{\alpha}} \nabla_a \nabla_b \nabla_b \Lambda_{\alpha i} + \left(\frac{1}{4} \bar{\mathcal{H}} + \frac{3}{4} \mathcal{H}\right) \chi_{\alpha}{}^{ik} \gamma_a{}^{\alpha}{}_{\dot{\alpha}} \nabla_a \chi^{\dot{\alpha}}{}_{ij}{}^k \\
& + \left(\frac{3}{8} \bar{\mathcal{H}} + \frac{1}{8} \mathcal{H}\right) \Lambda_{\alpha i} \gamma_a{}^{\alpha}{}_{\dot{\alpha}} \nabla_a \nabla_b \nabla_b \Lambda^{\dot{\alpha}i} + \left(\frac{3}{4} \bar{\mathcal{H}} + \frac{1}{4} \mathcal{H}\right) \chi^{\dot{\alpha}}{}_{ij}{}^k \gamma_a{}^{\alpha}{}_{\dot{\alpha}} \nabla_a \chi_{\alpha}{}^{ij}{}_k + (\mathcal{D}^{\dagger} \bar{\mathcal{H}} + 2 \mathcal{D} \bar{\mathcal{L}}) \epsilon_{\dot{\alpha}\dot{\beta}} \nabla_a \Lambda^{\dot{\alpha}i} \nabla_b R(Q)_{ab}{}^{\dot{\beta}}{}_i \\
& + (2 \mathcal{D}^{\dagger} \mathcal{I} + \mathcal{D} \mathcal{H}) \epsilon^{\alpha\beta} \nabla_a \Lambda_{\alpha i} \nabla_b R(Q)_{ab\beta}{}^i + \frac{1}{2} D^{ij}{}_{kl} \mathcal{D}^{\dagger} \bar{\mathcal{H}} \Lambda^{\dot{\alpha}k} \chi^{\dot{\beta}}{}_{ij}{}^l \epsilon_{\dot{\alpha}\dot{\beta}} + \frac{1}{2} D^{ij}{}_{kl} \mathcal{D} \mathcal{H} \Lambda_{\alpha i} \chi_{\beta}{}^{kl}{}_j \epsilon^{\alpha\beta} + \frac{1}{2} E_{ij} \mathcal{D} \mathcal{H} \chi_{\alpha}{}^{ik}{}_l \chi_{\beta}{}^{jl}{}_k \epsilon^{\alpha\beta} \\
& + \frac{1}{2} E^{ij} \mathcal{D}^{\dagger} \bar{\mathcal{H}} \chi^{\dot{\alpha}}{}_{ik}{}^l \chi^{\dot{\beta}}{}_{jl}{}^k \epsilon_{\dot{\alpha}\dot{\beta}} + R(Q)_{ab}{}^{\dot{\alpha}}{}_i \bar{\mathcal{H}} \bar{P}_a \epsilon_{\dot{\alpha}\dot{\beta}} \nabla_b \Lambda^{\dot{\beta}i} - 2 \bar{\mathcal{L}} P_a \Lambda^{\dot{\alpha}i} \epsilon_{\dot{\alpha}\dot{\beta}} \nabla_b R(Q)_{ab}{}^{\dot{\beta}}{}_i + 2 \bar{\mathcal{L}} P_a R(Q)_{ab}{}^{\dot{\alpha}}{}_i \epsilon_{\dot{\alpha}\dot{\beta}} \nabla_b \Lambda^{\dot{\beta}i} \\
& - \frac{2}{3} \bar{\mathcal{L}} T_{abij} \Lambda^{\dot{\alpha}i} \gamma_{ab\dot{\alpha}\dot{\beta}} \nabla_c \nabla_c \Lambda^{\dot{\beta}j} - \frac{4}{3} \bar{\mathcal{L}} T_{abij} \epsilon_{\dot{\alpha}\dot{\beta}} \nabla_a \Lambda^{\dot{\alpha}i} \nabla_b \Lambda^{\dot{\beta}j} - \frac{2}{3} \bar{\mathcal{L}} T_{abij} \gamma_{ab\dot{\alpha}\dot{\beta}} \nabla_c \Lambda^{\dot{\alpha}i} \nabla_c \Lambda^{\dot{\beta}j} - \frac{1}{6} \bar{\mathcal{L}} \Lambda^{\dot{\alpha}i} \Lambda^{\dot{\beta}j} \gamma_{ab\dot{\alpha}\dot{\beta}} \nabla_c \nabla_c T_{abij} \\
& - \frac{4}{3} \bar{\mathcal{L}} \Lambda^{\dot{\alpha}i} \epsilon_{\dot{\alpha}\dot{\beta}} \nabla_a T_{abij} \nabla_b \Lambda^{\dot{\beta}j} - \frac{4}{3} \bar{\mathcal{L}} \Lambda^{\dot{\alpha}i} \gamma_{ab\dot{\alpha}\dot{\beta}} \nabla_a T_{bcij} \nabla_c \Lambda^{\dot{\beta}j} - \bar{\mathcal{L}} \Lambda^{\dot{\alpha}i} \gamma_{ab\dot{\alpha}\dot{\beta}} \nabla_c T_{abij} \nabla_c \Lambda^{\dot{\beta}j} - \frac{4}{3} \bar{\mathcal{L}} \Lambda^{\dot{\alpha}i} \gamma_{ab\dot{\alpha}\dot{\beta}} \nabla_c T_{acij} \nabla_b \Lambda^{\dot{\beta}j} \\
& + \frac{3}{8} \mathcal{D}^{\dagger} \bar{\mathcal{H}} P_a \Lambda_{\alpha i} \gamma_a{}^{\alpha}{}_{\dot{\alpha}} \nabla_b \nabla_b \Lambda^{\dot{\alpha}i} + \frac{1}{4} \mathcal{D}^{\dagger} \bar{\mathcal{H}} P_a \chi_{\alpha}{}^{ij}{}_k \chi^{\dot{\alpha}}{}_{ij}{}^k \gamma_a{}^{\alpha}{}_{\dot{\alpha}} - \frac{1}{2} \mathcal{D}^{\dagger} \bar{\mathcal{H}} \Lambda^{\dot{\alpha}i} R(V)_{ab}{}^j{}_k \chi^{\dot{\beta}}{}_{ij}{}^k \gamma_{ab\dot{\alpha}\dot{\beta}} \\
& + \frac{3}{2} \mathcal{D}^{\dagger} \mathcal{I} T_{ab}{}^{ij} \Lambda_{\alpha k} \gamma_a{}^{\alpha}{}_{\dot{\alpha}} \nabla_b \chi^{\dot{\alpha}}{}_{ij}{}^k + \frac{7}{24} \mathcal{D}^{\dagger} \mathcal{I} \Lambda_{\alpha i} \Lambda^{\dot{\alpha}i} \gamma_a{}^{\alpha}{}_{\dot{\alpha}} \nabla_b \nabla_b \bar{P}_a + \frac{3}{2} \mathcal{D} \bar{\mathcal{L}} T_{abij} \Lambda^{\dot{\alpha}k} \gamma_a{}^{\alpha}{}_{\dot{\alpha}} \nabla_b \chi_{\alpha}{}^{ij}{}_k \\
& - \frac{7}{24} \mathcal{D} \bar{\mathcal{L}} \Lambda_{\alpha i} \Lambda^{\dot{\alpha}i} \gamma_a{}^{\alpha}{}_{\dot{\alpha}} \nabla_b \nabla_b P_a + \frac{1}{2} \mathcal{D} \mathcal{H} \Lambda_{\alpha i} R(V)_{ab}{}^j{}_k \chi_{\beta}{}^{ik}{}_j \gamma_{ab}{}^{\alpha\beta} + \frac{3}{8} \mathcal{D} \mathcal{H} \Lambda^{\dot{\alpha}i} \bar{P}_a \gamma_a{}^{\alpha}{}_{\dot{\alpha}} \nabla_b \nabla_b \Lambda_{\alpha i} - \frac{1}{4} \mathcal{D} \mathcal{H} \bar{P}_a \chi_{\alpha}{}^{ij}{}_k \chi^{\dot{\alpha}}{}_{ij}{}^k \gamma_a{}^{\alpha}{}_{\dot{\alpha}} \\
& - \frac{2}{3} \mathcal{I} T_{ab}{}^{ij} \Lambda_{\alpha i} \gamma_{ab}{}^{\alpha\beta} \nabla_c \nabla_c \Lambda_{\beta j} - \frac{4}{3} \mathcal{I} T_{ab}{}^{ij} \epsilon^{\alpha\beta} \nabla_a \Lambda_{\alpha i} \nabla_b \Lambda_{\beta j} - \frac{2}{3} \mathcal{I} T_{ab}{}^{ij} \gamma_{ab}{}^{\alpha\beta} \nabla_c \Lambda_{\alpha i} \nabla_c \Lambda_{\beta j} - \frac{1}{6} \mathcal{I} \Lambda_{\alpha i} \Lambda_{\beta j} \gamma_{ab}{}^{\alpha\beta} \nabla_c \nabla_c T_{ab}{}^{ij} \\
& - 2 \mathcal{I} \Lambda_{\alpha i} \bar{P}_a \epsilon^{\alpha\beta} \nabla_b R(Q)_{ab\beta}{}^i - \frac{4}{3} \mathcal{I} \Lambda_{\alpha i} \epsilon^{\alpha\beta} \nabla_a T_{ab}{}^{ij} \nabla_b \Lambda_{\beta j} - \frac{4}{3} \mathcal{I} \Lambda_{\alpha i} \gamma_{ab}{}^{\alpha\beta} \nabla_a T_{bc}{}^{ij} \nabla_c \Lambda_{\beta j} - \mathcal{I} \Lambda_{\alpha i} \gamma_{ab}{}^{\alpha\beta} \nabla_c T_{ab}{}^{ij} \nabla_c \Lambda_{\beta j} \\
& - \frac{4}{3} \mathcal{I} \Lambda_{\alpha i} \gamma_{ab}{}^{\alpha\beta} \nabla_c T_{ac}{}^{ij} \nabla_b \Lambda_{\beta j} + 2 \mathcal{I} R(Q)_{ab\alpha}{}^i \bar{P}_a \epsilon^{\alpha\beta} \nabla_b \Lambda_{\beta i} + \mathcal{H} P_a R(Q)_{ab\alpha}{}^i \epsilon^{\alpha\beta} \nabla_b \Lambda_{\beta i} + \left(-\frac{3}{2} \bar{\mathcal{H}} + \frac{1}{2} \mathcal{H}\right) P_a \Lambda_{\alpha i} \epsilon^{\alpha\beta} \nabla_b R(Q)_{ab\beta}{}^i \\
& + \left(-\frac{3}{2} \mathcal{D}^{\dagger} \mathcal{I} - \mathcal{D} \mathcal{H}\right) T_{ab}{}^{ij} \chi^{\dot{\alpha}}{}_{ij}{}^k \gamma_a{}^{\alpha}{}_{\dot{\alpha}} \nabla_b \Lambda_{\alpha k} + \left(-\mathcal{D}^{\dagger} \bar{\mathcal{H}} - \frac{3}{2} \mathcal{D} \bar{\mathcal{L}}\right) T_{abij} \chi_{\alpha}{}^{ij}{}_k \gamma_a{}^{\alpha}{}_{\dot{\alpha}} \nabla_b \Lambda^{\dot{\alpha}k} + \left(-\frac{5}{6} \mathcal{D}^{\dagger} \bar{\mathcal{H}} + \frac{5}{6} \mathcal{D} \bar{\mathcal{L}}\right) \Lambda^{\dot{\alpha}i} R(Q)_{ab}{}^{\dot{\beta}}{}_j R(V)_{ab}{}^j{}_i \epsilon_{\dot{\alpha}\dot{\beta}} \\
& + \left(-\frac{5}{6} \mathcal{D}^{\dagger} \mathcal{I} + \frac{5}{6} \mathcal{D} \mathcal{H}\right) \Lambda_{\alpha i} R(Q)_{ab\beta}{}^j R(V)_{ab}{}^i{}_j \epsilon^{\alpha\beta} + \left(-\frac{1}{2} \mathcal{D}^{\dagger} \mathcal{I} - \frac{1}{4} \mathcal{D} \mathcal{H}\right) \Lambda_{\alpha i} \epsilon^{\alpha\beta} \nabla_a E^{ij} \nabla_a \Lambda_{\beta j} + \left(-\frac{5}{12} \mathcal{D}^{\dagger} \mathcal{I} - \frac{1}{3} \mathcal{D} \mathcal{H}\right) E^{ij} \Lambda_{\alpha i} \epsilon^{\alpha\beta} \nabla_a \nabla_a \Lambda_{\beta j} \\
& + \left(-\frac{5}{12} \mathcal{D}^{\dagger} \mathcal{I} - \frac{1}{3} \mathcal{D} \mathcal{H}\right) E^{ij} \epsilon^{\alpha\beta} \nabla_a \Lambda_{\alpha i} \nabla_a \Lambda_{\beta j} + \left(-\frac{1}{3} \mathcal{D}^{\dagger} \bar{\mathcal{H}} - \frac{5}{12} \mathcal{D} \bar{\mathcal{L}}\right) E_{ij} \Lambda^{\dot{\alpha}i} \epsilon_{\dot{\alpha}\dot{\beta}} \nabla_a \nabla_a \Lambda^{\dot{\beta}j} + \left(-\frac{1}{3} \mathcal{D}^{\dagger} \bar{\mathcal{H}} - \frac{5}{12} \mathcal{D} \bar{\mathcal{L}}\right) E_{ij} \epsilon_{\dot{\alpha}\dot{\beta}} \nabla_a \Lambda^{\dot{\alpha}i} \nabla_a \Lambda^{\dot{\beta}j} \\
& + \left(-\frac{1}{3} \mathcal{D}^{\dagger} \mathcal{I} + \frac{7}{12} \mathcal{D} \mathcal{H}\right) \Lambda^{\dot{\alpha}i} \bar{P}_a \gamma_b{}^{\alpha}{}_{\dot{\alpha}} \nabla_a \nabla_b \Lambda_{\alpha i} + \left(-\frac{1}{4} \mathcal{D}^{\dagger} \bar{\mathcal{H}} - \frac{1}{2} \mathcal{D} \bar{\mathcal{L}}\right) \Lambda^{\dot{\alpha}i} \epsilon_{\dot{\alpha}\dot{\beta}} \nabla_a E_{ij} \nabla_a \Lambda^{\dot{\beta}j} + \left(-\frac{1}{4} \mathcal{D}^{\dagger} \bar{\mathcal{H}} + \frac{1}{8} \mathcal{D} \bar{\mathcal{L}}\right) \Lambda^{\dot{\alpha}i} R(M)_{abcd} R(Q)_{ab}{}^{\dot{\beta}}{}_i \gamma_{cd\dot{\alpha}\dot{\beta}} \\
& + \left(-\frac{1}{4} \mathcal{D}^{\dagger} \mathcal{I} + \frac{1$$

$$\begin{aligned}
F_{2,cont} = & + \frac{1}{16} D^{ij}{}_{kl} T_{abij} \mathcal{D}^\dagger \mathcal{D}^\dagger \bar{\mathcal{H}} \Lambda^{\dot{\alpha}k} \Lambda^{\dot{\beta}l} \gamma_{ab\dot{\alpha}\dot{\beta}} + \frac{1}{16} D^{ij}{}_{kl} T_{ab}{}^{kl} \mathcal{D} \mathcal{D} \mathcal{H} \Lambda_{\alpha i} \Lambda_{\beta j} \gamma_{ab}{}^{\alpha\beta} + \frac{1}{4} E_{ij} E^{ik} \mathcal{D}^\dagger \bar{\mathcal{H}} \Lambda^{\dot{\alpha}l} \chi^{\dot{\beta}}{}_{kl}{}^j \epsilon_{\dot{\alpha}\dot{\beta}} \\
& + \frac{1}{4} E_{ij} E^{ik} \mathcal{D} \mathcal{H} \Lambda_{\alpha l} \chi_{\beta}{}^{jl}{}_{\dot{k}} \epsilon^{\alpha\beta} - \frac{1}{4} E_{ij} T_{ab}{}^{ik} \mathcal{D} \mathcal{D} \mathcal{H} \Lambda_{\alpha l} \chi_{\beta}{}^{jl}{}_{\dot{k}} \gamma_{ab}{}^{\alpha\beta} - \frac{1}{4} E^{ij} T_{abik} \mathcal{D}^\dagger \mathcal{D}^\dagger \bar{\mathcal{H}} \Lambda^{\dot{\alpha}l} \chi^{\dot{\beta}}{}_{jl}{}^k \gamma_{ab\dot{\alpha}\dot{\beta}} \\
& - \frac{1}{4} T_{abij} \mathcal{D}^\dagger \bar{\mathcal{H}} \chi^{\dot{\alpha}}{}_{kl}{}^m \chi^{\dot{\beta}}{}_{mn}{}^k \gamma_{ab\dot{\alpha}\dot{\beta}} \varepsilon^{ijln} - \frac{1}{4} T_{ab}{}^{ij} \mathcal{D} \mathcal{H} \chi_{\alpha}{}^{kl}{}_{\dot{m}} \chi_{\beta}{}^{mn}{}_{\dot{k}} \gamma_{ab}{}^{\alpha\beta} \varepsilon_{ijln} + \frac{1}{3} \bar{\mathcal{I}} E_{ij} P_a \Lambda^{\dot{\alpha}i} \gamma_{ab\dot{\alpha}\dot{\beta}} \nabla_b \Lambda^{\dot{\beta}j} \\
& - \frac{11}{6} \bar{\mathcal{I}} P_a P_a \Lambda^{\dot{\alpha}i} \gamma_b{}^{\alpha}{}_{\dot{\alpha}} \nabla_b \Lambda_{\alpha i} - \frac{1}{3} \bar{\mathcal{I}} P_a P_b \Lambda^{\dot{\alpha}i} \gamma_a{}^{\alpha}{}_{\dot{\alpha}} \nabla_b \Lambda_{\alpha i} + \frac{7}{12} \bar{\mathcal{I}} P_a \Lambda^{\dot{\alpha}i} \Lambda^{\dot{\beta}j} \epsilon_{\dot{\alpha}\dot{\beta}} \nabla_a E_{ij} - \frac{1}{6} \bar{\mathcal{H}} E_{ij} \Lambda_{\alpha k} \Lambda^{\dot{\alpha}i} \gamma_a{}^{\alpha}{}_{\dot{\alpha}} \nabla_a E^{jk} \\
& + \frac{1}{6} \bar{\mathcal{H}} E^{ij} P_a \Lambda_{\alpha i} \gamma_{ab}{}^{\alpha\beta} \nabla_b \Lambda_{\beta j} - \frac{4}{3} \mathcal{D}^\dagger \bar{\mathcal{I}} P_a T_{abij} \Lambda^{\dot{\alpha}i} \epsilon_{\dot{\alpha}\dot{\beta}} \nabla_b \Lambda^{\dot{\beta}j} + \frac{1}{3} \mathcal{D}^\dagger \bar{\mathcal{I}} P_a T_{abij} \Lambda^{\dot{\alpha}i} \gamma_{bc\dot{\alpha}\dot{\beta}} \nabla_c \Lambda^{\dot{\beta}j} - \frac{1}{3} \mathcal{D}^\dagger \bar{\mathcal{I}} P_a T_{bcij} \Lambda^{\dot{\alpha}i} \gamma_{ab\dot{\alpha}\dot{\beta}} \nabla_c \Lambda^{\dot{\beta}j} \\
& - \frac{4}{3} \mathcal{D}^\dagger \bar{\mathcal{I}} P_a T_{bcij} \Lambda^{\dot{\alpha}i} \gamma_{bc\dot{\alpha}\dot{\beta}} \nabla_a \Lambda^{\dot{\beta}j} + \frac{1}{2} \mathcal{D}^\dagger \bar{\mathcal{I}} P_a \Lambda^{\dot{\alpha}i} \Lambda^{\dot{\beta}j} \gamma_{ab\dot{\alpha}\dot{\beta}} \nabla_c T_{bcij} - \frac{1}{2} \mathcal{D}^\dagger \bar{\mathcal{I}} P_a \Lambda^{\dot{\alpha}i} \Lambda^{\dot{\beta}j} \gamma_{bc\dot{\alpha}\dot{\beta}} \nabla_a T_{bcij} \\
& + \frac{1}{2} \mathcal{D}^\dagger \bar{\mathcal{I}} P_a \Lambda^{\dot{\alpha}i} \Lambda^{\dot{\beta}j} \gamma_{bc\dot{\alpha}\dot{\beta}} \nabla_b T_{acij} - \frac{1}{3} \mathcal{D}^\dagger \bar{\mathcal{I}} T_{abij} \Lambda^{\dot{\alpha}i} \Lambda^{\dot{\beta}j} \gamma_{ab\dot{\alpha}\dot{\beta}} \nabla_c P_c - \frac{1}{4} \mathcal{D}^\dagger \bar{\mathcal{I}} T_{abij} \Lambda^{\dot{\alpha}i} \Lambda^{\dot{\beta}j} \gamma_{ac\dot{\alpha}\dot{\beta}} \nabla_b P_c + \frac{1}{4} \mathcal{D}^\dagger \bar{\mathcal{I}} T_{abij} \Lambda^{\dot{\alpha}i} \Lambda^{\dot{\beta}j} \gamma_{ac\dot{\alpha}\dot{\beta}} \nabla_c P_b \\
& - \frac{1}{12} \mathcal{D}^\dagger \bar{\mathcal{I}} E^{ij} \Lambda_{\alpha i} \Lambda_{\beta k} R(V)_{ab}{}^k{}_j \gamma_{ab}{}^{\alpha\beta} - \frac{1}{12} \mathcal{D}^\dagger \bar{\mathcal{I}} T_{ab}{}^{ij} \Lambda_{\alpha i} \Lambda_{\beta j} \gamma_{ab}{}^{\alpha\beta} \nabla_c P_c + \frac{3}{8} \mathcal{D}^\dagger \bar{\mathcal{I}} T_{ab}{}^{ij} R(Q)_{cd\alpha}{}^k R(Q)_{cd\beta}{}^l \gamma_{ab}{}^{\alpha\beta} \varepsilon_{ijkl} \\
& + \frac{1}{12} \mathcal{D} \bar{\mathcal{I}} E_{ij} \Lambda^{\dot{\alpha}i} \Lambda^{\dot{\beta}k} R(V)_{ab}{}^j{}_k \gamma_{ab\dot{\alpha}\dot{\beta}} - \frac{1}{12} \mathcal{D} \bar{\mathcal{I}} T_{abij} \Lambda^{\dot{\alpha}i} \Lambda^{\dot{\beta}j} \gamma_{ab\dot{\alpha}\dot{\beta}} \nabla_c \bar{P}_c + \frac{3}{8} \mathcal{D} \bar{\mathcal{I}} T_{abij} R(Q)_{cd}{}^{\dot{\alpha}}{}_k R(Q)_{cd}{}^{\dot{\beta}}{}_l \gamma_{ab\dot{\alpha}\dot{\beta}} \varepsilon^{ijkl} \\
& - \frac{1}{3} \mathcal{D} \bar{\mathcal{I}} T_{ab}{}^{ij} \Lambda_{\alpha i} \Lambda_{\beta j} \gamma_{ab}{}^{\alpha\beta} \nabla_c \bar{P}_c - \frac{1}{4} \mathcal{D} \bar{\mathcal{I}} T_{ab}{}^{ij} \Lambda_{\alpha i} \Lambda_{\beta j} \gamma_{ac}{}^{\alpha\beta} \nabla_b \bar{P}_c + \frac{1}{4} \mathcal{D} \bar{\mathcal{I}} T_{ab}{}^{ij} \Lambda_{\alpha i} \Lambda_{\beta j} \gamma_{ac}{}^{\alpha\beta} \nabla_c \bar{P}_b - \frac{4}{3} \mathcal{D} \bar{\mathcal{I}} T_{ab}{}^{ij} \Lambda_{\alpha i} \bar{P}_a \epsilon^{\alpha\beta} \nabla_b \Lambda_{\beta j} \\
& + \frac{1}{3} \mathcal{D} \bar{\mathcal{I}} T_{ab}{}^{ij} \Lambda_{\alpha i} \bar{P}_a \gamma_{bc}{}^{\alpha\beta} \nabla_c \Lambda_{\beta j} - \frac{4}{3} \mathcal{D} \bar{\mathcal{I}} T_{ab}{}^{ij} \Lambda_{\alpha i} \bar{P}_c \gamma_{ab}{}^{\alpha\beta} \nabla_c \Lambda_{\beta j} + \frac{1}{3} \mathcal{D} \bar{\mathcal{I}} T_{ab}{}^{ij} \Lambda_{\alpha i} \bar{P}_c \gamma_{ac}{}^{\alpha\beta} \nabla_b \Lambda_{\beta j} + \frac{1}{2} \mathcal{D} \bar{\mathcal{I}} \Lambda_{\alpha i} \Lambda_{\beta j} \bar{P}_a \gamma_{ab}{}^{\alpha\beta} \nabla_c T_{bc}{}^{ij} \\
& - \frac{1}{2} \mathcal{D} \bar{\mathcal{I}} \Lambda_{\alpha i} \Lambda_{\beta j} \bar{P}_a \gamma_{bc}{}^{\alpha\beta} \nabla_a T_{bc}{}^{ij} + \frac{1}{2} \mathcal{D} \bar{\mathcal{I}} \Lambda_{\alpha i} \Lambda_{\beta j} \bar{P}_a \gamma_{bc}{}^{\alpha\beta} \nabla_b T_{ac}{}^{ij} + \frac{1}{3} \mathcal{I} E^{ij} \Lambda_{\alpha i} \bar{P}_a \gamma_{ab}{}^{\alpha\beta} \nabla_b \Lambda_{\beta j} + \frac{7}{12} \mathcal{I} \Lambda_{\alpha i} \Lambda_{\beta j} \bar{P}_a \epsilon^{\alpha\beta} \nabla_a E^{ij} \\
& - \frac{11}{6} \mathcal{I} \Lambda_{\alpha i} \bar{P}_a \bar{P}_b \gamma_b{}^{\alpha}{}_{\dot{\alpha}} \nabla_b \Lambda^{\dot{\alpha}i} - \frac{1}{3} \mathcal{I} \Lambda_{\alpha i} \bar{P}_a \bar{P}_b \gamma_a{}^{\alpha}{}_{\dot{\alpha}} \nabla_b \Lambda^{\dot{\alpha}i} + \frac{1}{6} \mathcal{H} E_{ij} \Lambda^{\dot{\alpha}i} \bar{P}_a \gamma_{ab\dot{\alpha}\dot{\beta}} \nabla_b \Lambda^{\dot{\beta}j} + \frac{1}{6} \mathcal{H} E^{ij} \Lambda_{\alpha i} \Lambda^{\dot{\alpha}k} \gamma_a{}^{\alpha}{}_{\dot{\alpha}} \nabla_a E_{jk} \\
& + (-\frac{5}{2} \mathcal{D}^\dagger \bar{\mathcal{I}} - \frac{1}{2} \mathcal{D} \mathcal{H}) P_a \Lambda_{\alpha i} R(Q)_{ab\beta}{}^i \bar{P}_b \epsilon^{\alpha\beta} + (-\frac{25}{16} \bar{\mathcal{H}} - \frac{29}{48} \mathcal{H}) P_a \Lambda_{\alpha i} \bar{P}_b \gamma_b{}^{\alpha}{}_{\dot{\alpha}} \nabla_a \Lambda^{\dot{\alpha}i} + (-\frac{4}{3} \bar{\mathcal{I}} - \frac{1}{2} \mathcal{D}^\dagger \mathcal{D}^\dagger \bar{\mathcal{H}}) T_{abij} \Lambda^{\dot{\alpha}i} \Lambda^{\dot{\beta}k} R(V)_{ac}{}^j{}_k \gamma_{bc\dot{\alpha}\dot{\beta}} \\
& + (-\frac{4}{3} \mathcal{D}^\dagger \bar{\mathcal{I}} - \frac{2}{3} \mathcal{D} \mathcal{H}) P_a T_{ab}{}^{ij} \Lambda_{\alpha i} \epsilon^{\alpha\beta} \nabla_b \Lambda_{\beta j} + (-\frac{9}{8} \bar{\mathcal{H}} - \frac{3}{8} \mathcal{H}) T_{abij} T_{ac}{}^{ij} \Lambda^{\dot{\alpha}k} \gamma_b{}^{\alpha}{}_{\dot{\alpha}} \nabla_c \Lambda_{\alpha k} + (-\frac{9}{8} \bar{\mathcal{H}} - \frac{3}{8} \mathcal{H}) T_{ab}{}^{ij} \Lambda_{\alpha i} \Lambda^{\dot{\alpha}k} \gamma_c{}^{\alpha}{}_{\dot{\alpha}} \nabla_a T_{bcjk} \\
& + (-\frac{9}{8} \bar{\mathcal{H}} - \frac{3}{8} \mathcal{H}) T_{ab}{}^{ij} \Lambda_{\alpha k} \Lambda^{\dot{\alpha}k} \gamma_c{}^{\alpha}{}_{\dot{\alpha}} \nabla_a T_{bcij} + (-\bar{\mathcal{H}} - \frac{5}{12} \mathcal{H}) \Lambda_{\alpha i} \Lambda^{\dot{\alpha}i} \bar{P}_a \gamma_a{}^{\alpha}{}_{\dot{\alpha}} \nabla_b P_b + (-\frac{5}{6} \mathcal{D}^\dagger \bar{\mathcal{I}} - \frac{1}{3} \mathcal{D} \mathcal{H}) P_a T_{bc}{}^{ij} \Lambda_{\alpha i} \gamma_{bc}{}^{\alpha\beta} \nabla_a \Lambda_{\beta j} \\
& + (-\frac{19}{24} \bar{\mathcal{H}} - \frac{3}{8} \mathcal{H}) \Lambda_{\alpha i} \chi^{\dot{\alpha}}{}_{jk}{}^i \gamma_a{}^{\alpha}{}_{\dot{\alpha}} \nabla_b T_{ablm} \varepsilon^{jklm} + (-\frac{2}{3} \bar{\mathcal{I}} + \frac{5}{8} \mathcal{D}^\dagger \mathcal{D}^\dagger \bar{\mathcal{H}}) E^{ij} T_{abik} \Lambda^{\dot{\alpha}k} R(Q)_{ab}{}^{\dot{\beta}}{}_j \epsilon_{\dot{\alpha}\dot{\beta}} \\
& + (-\frac{2}{3} \mathcal{D}^\dagger \bar{\mathcal{H}} - \frac{4}{3} \mathcal{D} \bar{\mathcal{I}}) T_{abij} \Lambda^{\dot{\alpha}i} \bar{P}_a \epsilon_{\dot{\alpha}\dot{\beta}} \nabla_b \Lambda^{\dot{\beta}j} + (-\frac{5}{8} \bar{\mathcal{H}} - \frac{5}{24} \mathcal{H}) T_{ab}{}^{ij} \chi_{\alpha}{}^{kl}{}_{\dot{m}} \gamma_a{}^{\alpha}{}_{\dot{\alpha}} \nabla_b \Lambda^{\dot{\alpha}m} \varepsilon_{ijkl} + (-\frac{29}{48} \bar{\mathcal{H}} - \frac{25}{16} \mathcal{H}) P_a \Lambda^{\dot{\alpha}i} \bar{P}_b \gamma_a{}^{\alpha}{}_{\dot{\alpha}} \nabla_b \Lambda_{\alpha i} \\
& + (-\frac{7}{12} \mathcal{D}^\dagger \bar{\mathcal{I}} - \frac{7}{24} \mathcal{D} \mathcal{H}) \bar{P}_a \gamma_b{}^{\alpha}{}_{\dot{\alpha}} \nabla_c \Lambda_{\alpha i} \nabla_d \Lambda^{\dot{\alpha}i} \varepsilon_{abcd} + (-\frac{1}{2} \mathcal{D} \mathcal{D} \mathcal{H} - \frac{2}{3} \mathcal{I}) T_{ab}{}^{ij} \Lambda_{\alpha i} \Lambda_{\beta k} R(V)_{ab}{}^k{}_j \epsilon^{\alpha\beta} \\
& + (-\frac{11}{24} \bar{\mathcal{H}} - \frac{1}{8} \mathcal{H}) T_{abij} R(Q)_{ab}{}^{\dot{\alpha}}{}_k \gamma_c{}^{\alpha}{}_{\dot{\alpha}} \nabla_c \Lambda_{\alpha l} \varepsilon^{ijkl} + (-\frac{5}{12} \bar{\mathcal{H}} - \frac{1}{3} \mathcal{H}) P_a \Lambda^{\dot{\alpha}i} \bar{P}_a \gamma_b{}^{\alpha}{}_{\dot{\alpha}} \nabla_b \Lambda_{\alpha i} + (-\frac{3}{8} \bar{\mathcal{H}} - \frac{9}{8} \mathcal{H}) T_{abij} T_{ac}{}^{ij} \Lambda_{\alpha k} \gamma_b{}^{\alpha}{}_{\dot{\alpha}} \nabla_c \Lambda^{\dot{\alpha}k} \\
& + (-\frac{3}{8} \bar{\mathcal{H}} - \frac{19}{24} \mathcal{H}) \Lambda^{\dot{\alpha}i} \chi_{\alpha}{}^{jk}{}_{\dot{i}} \gamma_a{}^{\alpha}{}_{\dot{\alpha}} \nabla_b T_{ab}{}^{lm} \varepsilon_{jklm} + (-\frac{3}{8} \bar{\mathcal{H}} - \frac{1}{8} \mathcal{H}) T_{abij} T_{ac}{}^{ij} \Lambda^{\dot{\alpha}k} \gamma_c{}^{\alpha}{}_{\dot{\alpha}} \nabla_b \Lambda_{\alpha k} + (-\frac{3}{8} \bar{\mathcal{H}} - \frac{1}{8} \mathcal{H}) T_{ab}{}^{ij} \Lambda_{\alpha i} \Lambda^{\dot{\alpha}k} \gamma_a{}^{\alpha}{}_{\dot{\alpha}} \nabla_c T_{bcjk} \\
& + (-\frac{3}{8} \bar{\mathcal{H}} - \frac{1}{8} \mathcal{H}) T_{ab}{}^{ij} \Lambda_{\alpha k} \Lambda^{\dot{\alpha}k} \gamma_a{}^{\alpha}{}_{\dot{\alpha}} \nabla_c T_{bcij} + (-\frac{3}{8} \mathcal{D} \mathcal{D} \mathcal{H} - \frac{25}{6} \mathcal{I}) \Lambda_{\alpha i} \Lambda^{\dot{\alpha}i} \bar{P}_a \gamma_b{}^{\alpha}{}_{\dot{\alpha}} \nabla_a \bar{P}_b + (-\frac{3}{8} \mathcal{D} \mathcal{D} \mathcal{H} - \frac{25}{6} \mathcal{I}) \Lambda_{\alpha i} \Lambda^{\dot{\alpha}i} \bar{P}_a \gamma_b{}^{\alpha}{}_{\dot{\alpha}} \nabla_b \bar{P}_a \\
& + (-\frac{3}{8} \mathcal{D} \mathcal{D} \mathcal{H} - \frac{5}{2} \mathcal{I}) \Lambda_{\alpha i} \Lambda^{\dot{\alpha}i} \bar{P}_a \gamma_a{}^{\alpha}{}_{\dot{\alpha}} \nabla_b \bar{P}_b + (-\frac{17}{48} \bar{\mathcal{H}} + \frac{5}{48} \mathcal{H}) \Lambda_{\alpha i} R(V)_{ab}{}^i{}_j \gamma_c{}^{\alpha}{}_{\dot{\alpha}} \nabla_d \Lambda^{\dot{\alpha}j} \varepsilon_{abcd} + (-\frac{1}{3} \bar{\mathcal{H}} - \frac{5}{12} \mathcal{H}) P_a \Lambda_{\alpha i} \bar{P}_a \gamma_b{}^{\alpha}{}_{\dot{\alpha}} \nabla_b \Lambda^{\dot{\alpha}i} \\
& + (-\frac{1}{3} \mathcal{D}^\dagger \bar{\mathcal{H}} - \frac{5}{6} \mathcal{D} \bar{\mathcal{I}}) T_{abij} \Lambda^{\dot{\alpha}i} \bar{P}_c \gamma_{ab\dot{\alpha}\dot{\beta}} \nabla_c \Lambda^{\dot{\beta}j} + (-\frac{1}{3} \mathcal{D}^\dagger \bar{\mathcal{H}} - \frac{1}{12} \mathcal{D} \bar{\mathcal{I}}) E^{ij} T_{abik} \Lambda^{\dot{\alpha}k} \gamma_a{}^{\alpha}{}_{\dot{\alpha}} \nabla_b \Lambda_{\alpha j} \\
& + (-\frac{1}{3} \mathcal{D}^\dagger \bar{\mathcal{H}} + \frac{1}{12} \mathcal{D} \bar{\mathcal{I}}) E^{ij} \Lambda_{\alpha i} \Lambda^{\dot{\alpha}k} \gamma_a{}^{\alpha}{}_{\dot{\alpha}} \nabla_b T_{abjk} + (-\frac{1}{3} \mathcal{D}^\dagger \bar{\mathcal{I}} - \frac{1}{6} \mathcal{D} \mathcal{H}) P_a T_{bc}{}^{ij} \Lambda_{\alpha i} \gamma_{ab}{}^{\alpha\beta} \nabla_c \Lambda_{\beta j} + (-\frac{7}{24} \bar{\mathcal{H}} - \frac{1}{12} \mathcal{H}) P_a \Lambda_{\alpha i} \Lambda_{\beta j} \epsilon^{\alpha\beta} \nabla_a E^{ij} \\
& + (-\frac{7}{24} \bar{\mathcal{H}} - \frac{1}{24} \mathcal{H}) P_a \Lambda_{\alpha i} \Lambda^{\dot{\alpha}i} \gamma_b{}^{\alpha}{}_{\dot{\alpha}} \nabla_a \bar{P}_b + (-\frac{7}{24} \bar{\mathcal{H}} - \frac{1}{24} \mathcal{H}) P_a \Lambda_{\alpha i} \Lambda^{\dot{\alpha}i} \gamma_b{}^{\alpha}{}_{\dot{\alpha}} \nabla_b \bar{P}_a + (-\frac{7}{24} \bar{\mathcal{H}} + \frac{1}{8} \mathcal{H}) T_{abij} \Lambda_{\alpha k} \gamma_a{}^{\alpha}{}_{\dot{\alpha}} \nabla_b \chi^{\dot{\alpha}}{}_{lm}{}^k \varepsilon^{ijlm} \\
& + (-\frac{1}{4} \bar{\mathcal{H}} - \frac{1}{12} \mathcal{H}) E_{ij} E^{ik} \Lambda_{\alpha k} \gamma_a{}^{\alpha}{}_{\dot{\alpha}} \nabla_a \Lambda^{\dot{\alpha}j} + (-\frac{1}{4} \mathcal{D}^\dagger \bar{\mathcal{I}} - \frac{1}{12} \mathcal{D} \mathcal{H}) P_a \Lambda_{\alpha i} \Lambda_{\beta j} \gamma_{bc}{}^{\alpha\beta} \nabla_a T_{bc}{}^{ij} + (-\frac{1}{4} \mathcal{D} \mathcal{D} \mathcal{H} + \frac{11}{6} \mathcal{I}) E^{ij} \Lambda_{\alpha i} \bar{P}_a \epsilon^{\alpha\beta} \nabla_a \Lambda_{\beta j} \\
& + (-\frac{1}{4} \mathcal{D} \mathcal{D} \mathcal{H} + 3 \mathcal{I}) T_{ab}{}^{ij} \Lambda_{\alpha k} \bar{P}_a \chi^{\dot{\alpha}}{}_{ij}{}^k \gamma_b{}^{\alpha}{}_{\dot{\alpha}} \nabla_c \Lambda^{\dot{\alpha}k} + (-\frac{5}{24} \bar{\mathcal{H}} - \frac{5}{8} \mathcal{H}) T_{abij} \chi^{\dot{\alpha}}{}_{kl}{}^m \gamma_a{}^{\alpha}{}_{\dot{\alpha}} \nabla_b \Lambda_{\alpha m} \varepsilon^{ijkl} + (-\frac{5}{24} \bar{\mathcal{H}} + \frac{1}{24} \mathcal{H}) E^{ij} \Lambda_{\alpha i} \Lambda_{\beta j} \epsilon^{\alpha\beta} \nabla_a P_a \\
& + (-\frac{3}{16} \bar{\mathcal{H}} - \frac{1}{16} \mathcal{H}) T_{abij} T_{ab}{}^{ik} \Lambda^{\dot{\alpha}j} \gamma_c{}^{\alpha}{}_{\dot{\alpha}} \nabla_c \Lambda_{\alpha k} + (-\frac{3}{16} \bar{\mathcal{H}} - \frac{1}{16} \mathcal{H}) T_{ab}{}^{ij} \Lambda_{\alpha i} \Lambda^{\dot{\alpha}k} \gamma_c{}^{\alpha}{}_{\dot{\alpha}} \nabla_c T_{abjk} + (-\frac{3}{16} \bar{\mathcal{H}} - \frac{1}{16} \mathcal{H}) T_{ab}{}^{ij} \Lambda_{\alpha k} \Lambda^{\dot{\alpha}k} \gamma_c{}^{\alpha}{}_{\dot{\alpha}} \nabla_c T_{abij} \\
& + (-\frac{1}{6} \mathcal{D}^\dagger \bar{\mathcal{H}} - \frac{1}{12} \mathcal{D} \bar{\mathcal{I}}) \Lambda^{\dot{\alpha}i} \Lambda^{\dot{\beta}j} \gamma_{ab\dot{\alpha}\dot{\beta}} \nabla_a \nabla_c T_{bc}{}^{kl} \varepsilon_{ijkl} + (-\frac{1}{6} \mathcal{D}^\dagger \bar{\mathcal{I}} - \frac{1}{12} \mathcal{D} \mathcal{H}) \Lambda_{\alpha i} \gamma_{ab}{}^{\alpha\beta} \nabla_a T_{bcjk} \nabla_c \Lambda_{\beta l} \varepsilon^{ijkl} \\
& + (-\frac{7}{48} \mathcal{D}^\dagger \bar{\mathcal{H}} - \frac{5}{36} \mathcal{D} \bar{\mathcal{I}}) T_{abij} \Lambda^{\dot{\alpha}i} \Lambda^{\dot{\beta}j} \gamma_{ac\dot{\alpha}\dot{\beta}} \nabla_b \bar{P}_c + (-\frac{5}{36} \mathcal{D}^\dagger \bar{\mathcal{I}} - \frac{7}{48} \mathcal{D} \mathcal{H}) T_{ab}{}^{ij} \Lambda_{\alpha i} \Lambda_{\beta j} \gamma_{ac}{}^{\alpha\beta} \nabla_b P_c \\
& + (-\frac{1}{8} \bar{\mathcal{H}} - \frac{11}{24} \mathcal{H}) T_{ab}{}^{ij} R(Q)_{ab\alpha}{}^k \gamma_c{}^{\alpha}{}_{\dot{\alpha}} \nabla_c \Lambda^{\dot{\alpha}l} \varepsilon_{ijkl} + (-\frac{1}{8} \bar{\mathcal{H}} - \frac{3}{8} \mathcal{H}) T_{abij} T_{ac}{}^{ij} \Lambda_{\alpha k} \gamma_c{}^{\alpha}{}_{\dot{\alpha}} \nabla_b \Lambda^{\dot{\alpha}k} \\
& + (-\frac{1}{8} \mathcal{D} \mathcal{D} \mathcal{H} + \frac{1}{2} \mathcal{I}) T_{ab}{}^{ij} \Lambda_{\alpha i} \Lambda_{\beta j} R(M)_{abcd} \gamma_{cd}{}^{\alpha\beta} + (-\frac{1}{12} \bar{\mathcal{H}} - \frac{7}{24} \mathcal{H}) \Lambda^{\dot{\alpha}i} \Lambda^{\dot{\beta}j} \bar{P}_a \epsilon_{\dot{\alpha}\dot{\beta}} \nabla_a E_{ij} + (-\frac{1}{12} \bar{\mathcal{H}} - \frac{1}{4} \mathcal{H}) E_{ij} E^{ik} \Lambda^{\dot{\alpha}j} \gamma_a{}^{\alpha}{}_{\dot{\alpha}} \nabla_a \Lambda_{\alpha k} + 2 \dots
\end{aligned}$$

$$\begin{aligned}
F_{2,cont} = & +(-\frac{1}{12} \mathcal{D}^\dagger \bar{\mathcal{H}} - \frac{1}{4} \mathcal{D} \bar{\mathcal{L}}) \Lambda^{\dot{\alpha}i} \Lambda^{\dot{\beta}j} \bar{P}_a \gamma_{bc\dot{\alpha}\dot{\beta}} \nabla_a T_{bcij} + (-\frac{1}{12} \mathcal{D}^\dagger \bar{\mathcal{H}} - \frac{1}{6} \mathcal{D} \bar{\mathcal{L}}) \Lambda^{\dot{\alpha}i} \gamma_{ab\dot{\alpha}\dot{\beta}} \nabla_a T_{bc}{}^{jk} \nabla_c \Lambda^{\dot{\beta}l} \varepsilon_{ijkl} \\
& + (-\frac{1}{12} \mathcal{D}^\dagger \mathcal{I} - \frac{1}{3} \mathcal{D} \mathcal{H}) E_{ij} T_{ab}{}^{ik} \Lambda_{\alpha k} \gamma_a{}^\alpha{}_{\dot{\alpha}} \nabla_b \Lambda^{\dot{\alpha}j} + (-\frac{1}{12} \mathcal{D}^\dagger \mathcal{I} - \frac{1}{6} \mathcal{D} \mathcal{H}) \Lambda_{\alpha i} \Lambda_{\beta j} \gamma_{ab}{}^{\alpha\beta} \nabla_a \nabla_c T_{bckl} \varepsilon^{ijkl} \\
& + (-\frac{1}{12} \mathcal{D}^\dagger \mathcal{I} + \frac{1}{3} \mathcal{D} \mathcal{H}) E_{ij} \Lambda_{\alpha k} \Lambda^{\dot{\alpha}i} \gamma_a{}^\alpha{}_{\dot{\alpha}} \nabla_b T_{ab}{}^{jk} + (-\frac{1}{12} \mathcal{D}^\dagger \mathcal{I} + \frac{1}{3} \mathcal{D} \mathcal{H}) \Lambda_{\alpha i} \Lambda^{\dot{\alpha}j} R(V)_{ab}{}^i{}_j \bar{P}_a \gamma_b{}^\alpha{}_{\dot{\alpha}} \\
& + (-\frac{1}{16} \bar{\mathcal{H}} - \frac{3}{16} \mathcal{H}) T_{abij} T_{ab}{}^{ik} \Lambda_{\alpha k} \gamma_c{}^\alpha{}_{\dot{\alpha}} \nabla_c \Lambda^{\dot{\alpha}j} + (-\frac{1}{16} \mathcal{D} \mathcal{D} \mathcal{H} + \frac{1}{2} \mathcal{I}) E^{ij} \Lambda_{\alpha i} \Lambda_{\beta j} \epsilon^{\alpha\beta} \nabla_a \bar{P}_a \\
& + (-\frac{1}{24} \mathcal{D}^\dagger \mathcal{I} + \frac{1}{6} \mathcal{D} \mathcal{H}) E_{ij} \Lambda_{\alpha k} \gamma_a{}^\alpha{}_{\dot{\alpha}} \nabla_a \chi^{\dot{\alpha}lm}{}_i \varepsilon^{jklm} + (-\frac{1}{48} \bar{\mathcal{H}} + \frac{1}{48} \mathcal{H}) E_{ij} \Lambda_{\alpha k} \Lambda^{\dot{\alpha}k} \gamma_a{}^\alpha{}_{\dot{\alpha}} \nabla_a E^{ij} + (-\frac{1}{48} \bar{\mathcal{H}} + \frac{1}{48} \mathcal{H}) E^{ij} \Lambda_{\alpha k} \Lambda^{\dot{\alpha}k} \gamma_a{}^\alpha{}_{\dot{\alpha}} \nabla_a E_{ij} \\
& + (\frac{1}{48} \bar{\mathcal{H}} + \frac{1}{16} \mathcal{H}) E_{ij} E^{ij} \Lambda_{\alpha k} \gamma_a{}^\alpha{}_{\dot{\alpha}} \nabla_a \Lambda^{\dot{\alpha}k} + (\frac{1}{24} \bar{\mathcal{H}} - \frac{5}{24} \mathcal{H}) E_{ij} \Lambda^{\dot{\alpha}i} \Lambda^{\dot{\beta}j} \epsilon_{\dot{\alpha}\dot{\beta}} \nabla_a \bar{P}_a + (\frac{1}{24} \bar{\mathcal{H}} + \frac{1}{8} \mathcal{H}) \Lambda_{\alpha i} R(Q)_{ab}{}^{\dot{\alpha}}{}_j \gamma_c{}^\alpha{}_{\dot{\alpha}} \nabla_c T_{abkl} \varepsilon^{ijkl} \\
& + (\frac{1}{24} \bar{\mathcal{H}} + \frac{7}{24} \mathcal{H}) \Lambda_{\alpha i} \Lambda^{\dot{\alpha}i} \bar{P}_a \gamma_b{}^\alpha{}_{\dot{\alpha}} \nabla_a P_b + (\frac{1}{24} \bar{\mathcal{H}} + \frac{7}{24} \mathcal{H}) \Lambda_{\alpha i} \Lambda^{\dot{\alpha}i} \bar{P}_a \gamma_b{}^\alpha{}_{\dot{\alpha}} \nabla_b P_a + (\frac{1}{24} \mathcal{D}^\dagger \mathcal{I} + \frac{1}{12} \mathcal{D} \mathcal{H}) E_{ij} \chi^{\dot{\alpha}kl}{}_i \gamma_a{}^\alpha{}_{\dot{\alpha}} \nabla_a \Lambda_{\alpha m} \varepsilon^{jklm} \\
& + (\frac{1}{24} \mathcal{D}^\dagger \mathcal{I} + \frac{1}{12} \mathcal{D} \mathcal{H}) \Lambda_{\alpha i} \chi^{\dot{\alpha}jk}{}_i \gamma_a{}^\alpha{}_{\dot{\alpha}} \nabla_a E_{lm} \varepsilon^{ijklm} + (\frac{1}{16} \bar{\mathcal{H}} + \frac{1}{48} \mathcal{H}) E_{ij} E^{ij} \Lambda^{\dot{\alpha}k} \gamma_a{}^\alpha{}_{\dot{\alpha}} \nabla_a \Lambda_{\alpha k} \\
& + (\frac{1}{16} \bar{\mathcal{H}} + \frac{3}{16} \mathcal{H}) T_{abij} T_{ab}{}^{ij} \Lambda_{\alpha k} \gamma_c{}^\alpha{}_{\dot{\alpha}} \nabla_c \Lambda^{\dot{\alpha}k} + (\frac{1}{16} \bar{\mathcal{H}} + \frac{3}{16} \mathcal{H}) T_{abij} \Lambda_{\alpha k} \Lambda^{\dot{\alpha}i} \gamma_c{}^\alpha{}_{\dot{\alpha}} \nabla_c T_{ab}{}^{jk} + (\frac{1}{16} \bar{\mathcal{H}} + \frac{3}{16} \mathcal{H}) T_{abij} \Lambda_{\alpha k} \Lambda^{\dot{\alpha}k} \gamma_c{}^\alpha{}_{\dot{\alpha}} \nabla_c T_{ab}{}^{ij} \\
& + (\frac{1}{12} \mathcal{D}^\dagger \bar{\mathcal{H}} + \frac{1}{24} \mathcal{D} \bar{\mathcal{L}}) E^{ij} \chi_{\alpha}{}^{kl}{}_i \gamma_a{}^\alpha{}_{\dot{\alpha}} \nabla_a \Lambda^{\dot{\alpha}m} \varepsilon_{jklm} + (\frac{1}{12} \mathcal{D}^\dagger \bar{\mathcal{H}} + \frac{1}{24} \mathcal{D} \bar{\mathcal{L}}) \Lambda^{\dot{\alpha}i} \chi_{\alpha}{}^{jk}{}_i \gamma_a{}^\alpha{}_{\dot{\alpha}} \nabla_a E^{lm} \varepsilon_{ijklm} \\
& + (\frac{1}{12} \mathcal{D}^\dagger \bar{\mathcal{H}} + \frac{1}{6} \mathcal{D} \bar{\mathcal{L}}) \Lambda^{\dot{\alpha}i} \gamma_{ab\dot{\alpha}\dot{\beta}} \nabla_c T_{ac}{}^{jk} \nabla_b \Lambda^{\dot{\beta}l} \varepsilon_{ijkl} + (\frac{1}{12} \mathcal{D}^\dagger \mathcal{I} - \frac{1}{6} \mathcal{D} \mathcal{H}) T_{ab}{}^{ij} \Lambda_{\alpha i} \Lambda^{\dot{\alpha}k} \gamma_a{}^\alpha{}_{\dot{\alpha}} \nabla_b E_{jk} \\
& + (\frac{1}{12} \mathcal{D}^\dagger \mathcal{I} + \frac{1}{6} \mathcal{D} \mathcal{H}) E_{ij} T_{ab}{}^{ik} \Lambda^{\dot{\alpha}j} \gamma_a{}^\alpha{}_{\dot{\alpha}} \nabla_b \Lambda_{\alpha k} + (\frac{1}{12} \mathcal{D}^\dagger \mathcal{I} + \frac{1}{6} \mathcal{D} \mathcal{H}) T_{abij} \Lambda_{\alpha k} \gamma_{ac}{}^{\alpha\beta} \nabla_b \nabla_c \Lambda_{\beta l} \varepsilon^{ijkl} \\
& + (\frac{1}{12} \mathcal{D}^\dagger \mathcal{I} + \frac{1}{6} \mathcal{D} \mathcal{H}) T_{abij} \Lambda_{\alpha k} \gamma_{ac}{}^{\alpha\beta} \nabla_c \nabla_b \Lambda_{\beta l} \varepsilon^{ijkl} + (\frac{5}{48} \bar{\mathcal{H}} - \frac{17}{48} \mathcal{H}) \Lambda^{\dot{\alpha}i} R(V)_{ab}{}^j{}_i \gamma_c{}^\alpha{}_{\dot{\alpha}} \nabla_d \Lambda_{\alpha j} \varepsilon_{abcd} \\
& + (\frac{1}{8} \bar{\mathcal{H}} - \frac{7}{24} \mathcal{H}) T_{ab}{}^{ij} \Lambda^{\dot{\alpha}k} \gamma_a{}^\alpha{}_{\dot{\alpha}} \nabla_b \chi_{\alpha}{}^{lm}{}_k \varepsilon_{ijlm} + (\frac{1}{8} \bar{\mathcal{H}} + \frac{1}{24} \mathcal{H}) \Lambda^{\dot{\alpha}i} R(Q)_{ab\alpha}{}^j \gamma_c{}^\alpha{}_{\dot{\alpha}} \nabla_c T_{ab}{}^{kl} \varepsilon_{ijkl} + (\frac{1}{8} \bar{\mathcal{H}} + \frac{3}{8} \mathcal{H}) T_{abij} T_{ac}{}^{ik} \Lambda_{\alpha k} \gamma_c{}^\alpha{}_{\dot{\alpha}} \nabla_b \Lambda^{\dot{\alpha}j} \\
& + (\frac{1}{8} \bar{\mathcal{H}} + \frac{3}{8} \mathcal{H}) T_{abij} \Lambda_{\alpha k} \Lambda^{\dot{\alpha}i} \gamma_c{}^\alpha{}_{\dot{\alpha}} \nabla_a T_{bc}{}^{jk} + (\frac{1}{8} \bar{\mathcal{H}} + \frac{3}{8} \mathcal{H}) T_{abij} \Lambda_{\alpha k} \Lambda^{\dot{\alpha}k} \gamma_c{}^\alpha{}_{\dot{\alpha}} \nabla_a T_{bc}{}^{ij} + (\frac{5}{36} \mathcal{D}^\dagger \mathcal{I} + \frac{7}{48} \mathcal{D} \mathcal{H}) T_{ab}{}^{ij} \Lambda_{\alpha i} \Lambda_{\beta j} \gamma_{ac}{}^{\alpha\beta} \nabla_c P_b \\
& + (\frac{7}{48} \mathcal{D}^\dagger \bar{\mathcal{H}} + \frac{5}{36} \mathcal{D} \bar{\mathcal{L}}) T_{abij} \Lambda^{\dot{\alpha}i} \Lambda^{\dot{\beta}j} \gamma_{ac\dot{\alpha}\dot{\beta}} \nabla_c \bar{P}_b + (\frac{1}{6} \mathcal{D}^\dagger \bar{\mathcal{H}} - \frac{1}{12} \mathcal{D} \bar{\mathcal{L}}) T_{abij} \Lambda_{\alpha k} \Lambda^{\dot{\alpha}i} \gamma_a{}^\alpha{}_{\dot{\alpha}} \nabla_b E^{jk} \\
& + (\frac{1}{6} \mathcal{D}^\dagger \bar{\mathcal{H}} - \frac{1}{24} \mathcal{D} \bar{\mathcal{L}}) E^{ij} \Lambda^{\dot{\alpha}k} \gamma_a{}^\alpha{}_{\dot{\alpha}} \nabla_a \chi_{\alpha}{}^{lm}{}_i \varepsilon_{jklm} + (\frac{1}{6} \mathcal{D}^\dagger \bar{\mathcal{H}} + \frac{1}{12} \mathcal{D} \bar{\mathcal{L}}) E^{ij} T_{abik} \Lambda_{\alpha j} \gamma_a{}^\alpha{}_{\dot{\alpha}} \nabla_b \Lambda^{\dot{\alpha}k} \\
& + (\frac{1}{6} \mathcal{D}^\dagger \bar{\mathcal{H}} + \frac{1}{12} \mathcal{D} \bar{\mathcal{L}}) T_{ab}{}^{ij} \Lambda^{\dot{\alpha}k} \gamma_{ac\dot{\alpha}\dot{\beta}} \nabla_b \nabla_c \Lambda^{\dot{\beta}l} \varepsilon_{ijkl} + (\frac{1}{6} \mathcal{D}^\dagger \bar{\mathcal{H}} + \frac{1}{12} \mathcal{D} \bar{\mathcal{L}}) T_{ab}{}^{ij} \Lambda^{\dot{\alpha}k} \gamma_{ac\dot{\alpha}\dot{\beta}} \nabla_c \nabla_b \Lambda^{\dot{\beta}l} \varepsilon_{ijkl} \\
& + (\frac{1}{6} \mathcal{D}^\dagger \bar{\mathcal{H}} + \frac{1}{3} \mathcal{D} \bar{\mathcal{L}}) T_{abij} \Lambda^{\dot{\alpha}i} \bar{P}_a \gamma_{bc\dot{\alpha}\dot{\beta}} \nabla_c \Lambda^{\dot{\beta}j} + (\frac{1}{6} \mathcal{D}^\dagger \bar{\mathcal{H}} + \frac{1}{3} \mathcal{D} \bar{\mathcal{L}}) T_{abij} \Lambda^{\dot{\alpha}i} \bar{P}_c \gamma_{ac\dot{\alpha}\dot{\beta}} \nabla_b \Lambda^{\dot{\beta}j} + (\frac{1}{6} \mathcal{D}^\dagger \bar{\mathcal{H}} + \frac{1}{3} \mathcal{D} \bar{\mathcal{L}}) T_{ab}{}^{ij} \epsilon_{\dot{\alpha}\dot{\beta}} \nabla_a \Lambda^{\dot{\alpha}k} \nabla_b \Lambda^{\dot{\beta}l} \varepsilon_{ijkl} \\
& + (\frac{1}{6} \mathcal{D}^\dagger \bar{\mathcal{H}} + \frac{1}{3} \mathcal{D} \bar{\mathcal{L}}) \Lambda^{\dot{\alpha}i} \epsilon_{\dot{\alpha}\dot{\beta}} \nabla_a T_{ab}{}^{jk} \nabla_b \Lambda^{\dot{\beta}l} \varepsilon_{ijkl} + (\frac{1}{6} \mathcal{D}^\dagger \mathcal{I} + \frac{1}{12} \mathcal{D} \mathcal{H}) \Lambda_{\alpha i} \gamma_{ab}{}^{\alpha\beta} \nabla_c T_{acjk} \nabla_b \Lambda_{\beta l} \varepsilon^{ijkl} \\
& + (\frac{1}{6} \mathcal{D}^\dagger \mathcal{I} + \frac{1}{3} \mathcal{D} \mathcal{H}) T_{abij} \gamma_{ac}{}^{\alpha\beta} \nabla_b \Lambda_{\alpha k} \nabla_c \Lambda_{\beta l} \varepsilon^{ijkl} + (\frac{3}{16} \bar{\mathcal{H}} + \frac{1}{16} \mathcal{H}) T_{abij} T_{ab}{}^{ij} \Lambda^{\dot{\alpha}k} \gamma_c{}^\alpha{}_{\dot{\alpha}} \nabla_c \Lambda_{\alpha k} \\
& + (\frac{11}{48} \bar{\mathcal{H}} + \frac{7}{16} \mathcal{H}) P_a \Lambda_{\alpha i} \bar{P}_b \gamma_a{}^\alpha{}_{\dot{\alpha}} \nabla_b \Lambda^{\dot{\alpha}i} + (\frac{1}{4} \bar{\mathcal{H}} + \frac{1}{4} \mathcal{H}) E_{ij} \chi^{\dot{\alpha}kl}{}_i \chi^{\dot{\beta}mn}{}_j \epsilon_{\dot{\alpha}\dot{\beta}} \varepsilon^{klmn} + (\frac{1}{4} \bar{\mathcal{H}} + \frac{1}{4} \mathcal{H}) E^{ij} \chi_{\alpha}{}^{kl}{}_i \chi_{\beta}{}^{mn}{}_j \epsilon^{\alpha\beta} \varepsilon_{klmn} \\
& + (\frac{1}{4} \bar{\mathcal{H}} + \frac{1}{3} \mathcal{H}) E^{ij} P_a \Lambda_{\alpha i} \epsilon^{\alpha\beta} \nabla_a \Lambda_{\beta j} + (\frac{1}{4} \mathcal{D}^\dagger \bar{\mathcal{H}} + \frac{1}{2} \mathcal{D} \bar{\mathcal{L}}) \Lambda^{\dot{\alpha}i} \Lambda^{\dot{\beta}j} \bar{P}_a \gamma_{ab\dot{\alpha}\dot{\beta}} \nabla_c T_{bcij} + (\frac{1}{4} \mathcal{D}^\dagger \bar{\mathcal{H}} + \frac{1}{2} \mathcal{D} \bar{\mathcal{L}}) \Lambda^{\dot{\alpha}i} \Lambda^{\dot{\beta}j} \bar{P}_a \gamma_{bc\dot{\alpha}\dot{\beta}} \nabla_b T_{acij} \\
& + (\frac{1}{4} \mathcal{D}^\dagger \mathcal{I} + \frac{3}{4} \mathcal{D} \mathcal{H}) T_{ab}{}^{ij} R(Q)_{ab\alpha}{}^k \chi_{\beta}{}^{lm}{}_k \epsilon^{\alpha\beta} \varepsilon_{ijlm} + (\frac{7}{24} \mathcal{D}^\dagger \bar{\mathcal{H}} + \frac{7}{12} \mathcal{D} \bar{\mathcal{L}}) P_a \gamma_b{}^\alpha{}_{\dot{\alpha}} \nabla_c \Lambda_{\alpha i} \nabla_d \Lambda^{\dot{\alpha}i} \varepsilon_{abcd} \\
& + (\frac{1}{3} \bar{\mathcal{H}} + \frac{1}{4} \mathcal{H}) E_{ij} \Lambda^{\dot{\alpha}i} \bar{P}_a \epsilon_{\dot{\alpha}\dot{\beta}} \nabla_a \Lambda^{\dot{\beta}j} + (\frac{1}{3} \mathcal{D}^\dagger \bar{\mathcal{H}} - \frac{1}{12} \mathcal{D} \bar{\mathcal{L}}) P_a \Lambda_{\alpha i} \Lambda^{\dot{\alpha}j} R(V)_{ab}{}^i{}_j \gamma_b{}^\alpha{}_{\dot{\alpha}} + (\frac{1}{3} \mathcal{D}^\dagger \bar{\mathcal{H}} + \frac{1}{6} \mathcal{D} \bar{\mathcal{L}}) T_{ab}{}^{ij} \gamma_{ac\dot{\alpha}\dot{\beta}} \nabla_b \Lambda^{\dot{\alpha}k} \nabla_c \Lambda^{\dot{\beta}l} \varepsilon_{ijkl} \\
& + (\frac{1}{3} \mathcal{D}^\dagger \mathcal{I} + \frac{1}{6} \mathcal{D} \mathcal{H}) P_a T_{ab}{}^{ij} \Lambda_{\alpha i} \gamma_{bc}{}^{\alpha\beta} \nabla_c \Lambda_{\beta j} + (\frac{1}{3} \mathcal{D}^\dagger \mathcal{I} + \frac{1}{6} \mathcal{D} \mathcal{H}) T_{abij} \epsilon^{\alpha\beta} \nabla_a \Lambda_{\alpha k} \nabla_b \Lambda_{\beta l} \varepsilon^{ijkl} + (\frac{1}{3} \mathcal{D}^\dagger \mathcal{I} + \frac{1}{6} \mathcal{D} \mathcal{H}) \Lambda_{\alpha i} \epsilon^{\alpha\beta} \nabla_a T_{abjk} \nabla_b \Lambda_{\beta l} \varepsilon^{ijkl} \\
& + (\frac{3}{8} \bar{\mathcal{H}} + \frac{1}{8} \mathcal{H}) T_{abij} T_{ac}{}^{ik} \Lambda^{\dot{\alpha}j} \gamma_c{}^\alpha{}_{\dot{\alpha}} \nabla_b \Lambda_{\alpha k} + (\frac{3}{8} \bar{\mathcal{H}} + \frac{13}{24} \mathcal{H}) T_{ab}{}^{ij} \Lambda^{\dot{\alpha}k} \gamma_c{}^\alpha{}_{\dot{\alpha}} \nabla_c R(Q)_{ab\alpha}{}^l \varepsilon_{ijkl} + (\frac{3}{8} \bar{\mathcal{H}} + \frac{9}{8} \mathcal{H}) T_{abij} T_{ac}{}^{ik} \Lambda_{\alpha k} \gamma_b{}^\alpha{}_{\dot{\alpha}} \nabla_c \Lambda^{\dot{\alpha}j} \\
& + (\frac{3}{8} \bar{\mathcal{H}} + \frac{9}{8} \mathcal{H}) T_{abij} \Lambda_{\alpha k} \Lambda^{\dot{\alpha}i} \gamma_a{}^\alpha{}_{\dot{\alpha}} \nabla_c T_{bc}{}^{jk} + (\frac{3}{8} \bar{\mathcal{H}} + \frac{9}{8} \mathcal{H}) T_{abij} \Lambda_{\alpha k} \Lambda^{\dot{\alpha}k} \gamma_a{}^\alpha{}_{\dot{\alpha}} \nabla_c T_{bc}{}^{ij} + (\frac{3}{8} \mathcal{D} \mathcal{D} \mathcal{H} + 2 \mathcal{I}) \Lambda^{\dot{\alpha}i} \bar{P}_a \bar{P}_a \gamma_b{}^\alpha{}_{\dot{\alpha}} \nabla_b \Lambda_{\alpha i} \\
& + (\frac{5}{12} \bar{\mathcal{H}} + \mathcal{H}) P_a \Lambda_{\alpha i} \Lambda^{\dot{\alpha}i} \gamma_a{}^\alpha{}_{\dot{\alpha}} \nabla_b \bar{P}_b + (\frac{7}{16} \bar{\mathcal{H}} + \frac{11}{48} \mathcal{H}) P_a \Lambda^{\dot{\alpha}i} \bar{P}_b \gamma_b{}^\alpha{}_{\dot{\alpha}} \nabla_a \Lambda_{\alpha i} + (\frac{1}{2} \bar{\mathcal{L}} - \frac{1}{8} \mathcal{D}^\dagger \mathcal{D}^\dagger \bar{\mathcal{H}}) T_{abij} \Lambda^{\dot{\alpha}i} \Lambda^{\dot{\beta}j} R(M)_{abcd} \gamma_{cd\dot{\alpha}\dot{\beta}} \\
& + (\frac{1}{2} \bar{\mathcal{L}} - \frac{1}{16} \mathcal{D}^\dagger \mathcal{D}^\dagger \bar{\mathcal{H}}) E_{ij} \Lambda^{\dot{\alpha}i} \Lambda^{\dot{\beta}j} \epsilon_{\dot{\alpha}\dot{\beta}} \nabla_a P_a + (\frac{1}{2} \bar{\mathcal{H}} + 2 \mathcal{H}) T_{abij} \Lambda^{\dot{\alpha}k} \bar{P}_a \chi_{\alpha}{}^{ij}{}_k \gamma_b{}^\alpha{}_{\dot{\alpha}} + (\frac{1}{2} \mathcal{D}^\dagger \bar{\mathcal{H}} + \frac{5}{2} \mathcal{D} \bar{\mathcal{L}}) P_a \Lambda^{\dot{\alpha}i} R(Q)_{ab}{}^{\dot{\beta}}{}_i \bar{P}_b \epsilon_{\dot{\alpha}\dot{\beta}} \\
& + (\frac{1}{2} \mathcal{D}^\dagger \mathcal{I} + \frac{1}{4} \mathcal{D} \mathcal{H}) P_a \Lambda_{\alpha i} \Lambda_{\beta j} \gamma_{ab}{}^{\alpha\beta} \nabla_c T_{bc}{}^{ij} + (\frac{1}{2} \mathcal{D}^\dagger \mathcal{I} + \frac{1}{4} \mathcal{D} \mathcal{H}) P_a \Lambda_{\alpha i} \Lambda_{\beta j} \gamma_{bc}{}^{\alpha\beta} \nabla_b T_{ac}{}^{ij} + (\frac{1}{2} \mathcal{D} \mathcal{D} \mathcal{H} + \frac{4}{3} \mathcal{I}) T_{ab}{}^{ij} \Lambda_{\alpha i} \Lambda_{\beta k} R(V)_{ac}{}^k{}_j \gamma_{bc}{}^{\alpha\beta} \\
& + (\frac{13}{24} \bar{\mathcal{H}} + \frac{3}{8} \mathcal{H}) T_{abij} \Lambda_{\alpha k} \gamma_c{}^\alpha{}_{\dot{\alpha}} \nabla_c R(Q)_{ab}{}^{\dot{\alpha}}{}_l \varepsilon^{ijkl} + (\frac{5}{8} \mathcal{D} \mathcal{D} \mathcal{H} - \frac{2}{3} \mathcal{I}) E_{ij} T_{ab}{}^{ik} \Lambda_{\alpha k} R(Q)_{ab\beta}{}^j \epsilon^{\alpha\beta} + 3 \dots
\end{aligned}$$

$$\begin{aligned}
F_{2,cont} = & + \left( \frac{2}{3} \bar{\mathcal{I}} + \frac{1}{2} \mathcal{D}^\dagger \mathcal{D}^\dagger \bar{\mathcal{H}} \right) T_{abij} \Lambda^{\dot{\alpha}i} \Lambda^{\dot{\beta}k} R(V)_{ab}{}^j{}_k \epsilon_{\dot{\alpha}\dot{\beta}} + \left( \frac{2}{3} \bar{\mathcal{I}} + \frac{3}{4} \mathcal{D}^\dagger \mathcal{D}^\dagger \bar{\mathcal{H}} \right) P_a P_b \Lambda_{\alpha i} \gamma_a{}^\alpha{}_{\dot{\alpha}} \nabla_b \Lambda^{\dot{\alpha}i} + \left( \frac{3}{4} \mathcal{D}^\dagger \bar{\mathcal{H}} + \frac{1}{4} \mathcal{D} \bar{\mathcal{I}} \right) T_{abij} R(Q)_{ab}{}^{\dot{\alpha}}{}_k \chi^{\dot{\beta}}{}_{lm}{}^k \epsilon_{\dot{\alpha}\dot{\beta}} \epsilon^{ijlm} \\
& + \left( \frac{3}{4} \mathcal{D} \mathcal{D} \mathcal{H} + \frac{2}{3} \mathcal{I} \right) \Lambda^{\dot{\alpha}i} \bar{P}_a \bar{P}_b \gamma_a{}^\alpha{}_{\dot{\alpha}} \nabla_b \Lambda_{\alpha i} + \left( \frac{9}{8} \bar{\mathcal{H}} + \frac{3}{8} \mathcal{H} \right) T_{abij} T_{ac}{}^{ik} \Lambda^{\dot{\alpha}j} \gamma_b{}^\alpha{}_{\dot{\alpha}} \nabla_c \Lambda_{\alpha k} + \left( \frac{11}{6} \bar{\mathcal{I}} - \frac{1}{4} \mathcal{D}^\dagger \mathcal{D}^\dagger \bar{\mathcal{H}} \right) E_{ij} P_a \Lambda^{\dot{\alpha}i} \epsilon_{\dot{\alpha}\dot{\beta}} \nabla_a \Lambda^{\dot{\beta}j} \\
& + \left( 2 \bar{\mathcal{I}} + \frac{3}{8} \mathcal{D}^\dagger \mathcal{D}^\dagger \bar{\mathcal{H}} \right) P_a P_a \Lambda_{\alpha i} \gamma_b{}^\alpha{}_{\dot{\alpha}} \nabla_b \Lambda^{\dot{\alpha}i} + \left( 2 \bar{\mathcal{H}} + \frac{1}{2} \mathcal{H} \right) P_a T_{ab}{}^{ij} \Lambda_{\alpha k} \chi^{\dot{\beta}}{}_{ij}{}^k \gamma_b{}^\alpha{}_{\dot{\alpha}} + \left( \frac{5}{2} \bar{\mathcal{I}} + \frac{3}{8} \mathcal{D}^\dagger \mathcal{D}^\dagger \bar{\mathcal{H}} \right) P_a \Lambda_{\alpha i} \Lambda^{\dot{\alpha}i} \gamma_a{}^\alpha{}_{\dot{\alpha}} \nabla_b P_b \\
& + \left( 3 \bar{\mathcal{I}} - \frac{1}{4} \mathcal{D}^\dagger \mathcal{D}^\dagger \bar{\mathcal{H}} \right) P_a T_{abij} \Lambda^{\dot{\alpha}k} \chi_{\alpha}{}^{ij}{}_k \gamma_b{}^\alpha{}_{\dot{\alpha}} + \left( \frac{25}{6} \bar{\mathcal{I}} + \frac{3}{8} \mathcal{D}^\dagger \mathcal{D}^\dagger \bar{\mathcal{H}} \right) P_a \Lambda_{\alpha i} \Lambda^{\dot{\alpha}i} \gamma_b{}^\alpha{}_{\dot{\alpha}} \nabla_a P_b + \left( \frac{25}{6} \bar{\mathcal{I}} + \frac{3}{8} \mathcal{D}^\dagger \mathcal{D}^\dagger \bar{\mathcal{H}} \right) P_a \Lambda_{\alpha i} \Lambda^{\dot{\alpha}i} \gamma_b{}^\alpha{}_{\dot{\alpha}} \nabla_b P_a \\
& - \frac{1}{16} D^{ij}{}_{kl} E_{im} \mathcal{D} \mathcal{D} \mathcal{H} \Lambda_{\alpha j} \Lambda_{\beta n} \epsilon^{\alpha\beta} \epsilon^{klmn} - \frac{1}{16} D^{ij}{}_{kl} E^{km} \mathcal{D}^\dagger \mathcal{D}^\dagger \bar{\mathcal{H}} \Lambda^{\dot{\alpha}l} \Lambda^{\dot{\beta}n} \epsilon_{\dot{\alpha}\dot{\beta}} \epsilon_{ijmn} - \frac{1}{24} E_{ij} E_{kl} E^{ij} \mathcal{D}^\dagger \bar{\mathcal{H}} \Lambda^{\dot{\alpha}k} \Lambda^{\dot{\beta}l} \epsilon_{\dot{\alpha}\dot{\beta}} \\
& + \frac{1}{16} E_{ij} E_{kl} E^{ik} \mathcal{D}^\dagger \bar{\mathcal{H}} \Lambda^{\dot{\alpha}j} \Lambda^{\dot{\beta}l} \epsilon_{\dot{\alpha}\dot{\beta}} + \frac{1}{8} E_{ij} E_{kl} \mathcal{D} \mathcal{D} \mathcal{H} \Lambda_{\alpha m} \chi_{\beta}{}^{ik}{}_n \epsilon^{\alpha\beta} \epsilon^{jlmn} - \frac{1}{24} E_{ij} E^{ij} E^{kl} \mathcal{D} \mathcal{H} \Lambda_{\alpha k} \Lambda_{\beta l} \epsilon^{\alpha\beta} + \frac{1}{16} E_{ij} E^{ik} E^{jl} \mathcal{D} \mathcal{H} \Lambda_{\alpha k} \Lambda_{\beta l} \epsilon^{\alpha\beta} \\
& + \frac{1}{48} E_{ij} E^{ij} T_{abkl} \mathcal{D}^\dagger \mathcal{D}^\dagger \bar{\mathcal{H}} \Lambda^{\dot{\alpha}k} \Lambda^{\dot{\beta}l} \gamma_{ab\dot{\alpha}\dot{\beta}} - \frac{1}{24} E_{ij} E^{ik} T_{abkl} \mathcal{D}^\dagger \mathcal{D}^\dagger \bar{\mathcal{H}} \Lambda^{\dot{\alpha}j} \Lambda^{\dot{\beta}l} \gamma_{ab\dot{\alpha}\dot{\beta}} + \frac{1}{48} E_{ij} E^{ij} T_{ab}{}^{kl} \mathcal{D} \mathcal{D} \mathcal{H} \Lambda_{\alpha k} \Lambda_{\beta l} \gamma_{ab}{}^{\alpha\beta} \\
& - \frac{1}{24} E_{ij} E^{ik} T_{ab}{}^{jl} \mathcal{D} \mathcal{D} \mathcal{H} \Lambda_{\alpha k} \Lambda_{\beta l} \gamma_{ab}{}^{\alpha\beta} - \frac{1}{24} E_{ij} T_{abkl} \mathcal{D}^\dagger \bar{\mathcal{H}} \Lambda^{\dot{\alpha}i} \chi^{\dot{\beta}}{}_{mn}{}^j \gamma_{ab\dot{\alpha}\dot{\beta}} \epsilon^{klmn} - \frac{1}{8} E_{ij} T_{abkl} \mathcal{D}^\dagger \bar{\mathcal{H}} \Lambda^{\dot{\alpha}m} \chi^{\dot{\beta}}{}_{mn}{}^i \gamma_{ab\dot{\alpha}\dot{\beta}} \epsilon^{jklm} \\
& + \frac{1}{8} E_{ij} T_{ab}{}^{ik} T_{ab}{}^{jl} \mathcal{D} \mathcal{D} \mathcal{D} \mathcal{H} \Lambda_{\alpha k} \Lambda_{\beta l} \epsilon^{\alpha\beta} - \frac{1}{8} E_{ij} T_{ab}{}^{ik} T_{ac}{}^{jl} \mathcal{D} \mathcal{D} \mathcal{D} \mathcal{H} \Lambda_{\alpha k} \Lambda_{\beta l} \gamma_{bc}{}^{\alpha\beta} - \frac{1}{16} E_{ij} \mathcal{D} \mathcal{D} \mathcal{H} \Lambda_{\alpha k} \Lambda_{\beta l} R(V)_{ab}{}^i{}_m \gamma_{ab}{}^{\alpha\beta} \epsilon^{jklm} \\
& + \frac{1}{8} E^{ij} E^{kl} \mathcal{D}^\dagger \mathcal{D}^\dagger \bar{\mathcal{H}} \Lambda^{\dot{\alpha}m} \chi^{\dot{\beta}}{}_{ik}{}_n \epsilon_{\dot{\alpha}\dot{\beta}} \epsilon_{jlmn} + \frac{1}{8} E^{ij} T_{abik} T_{abjl} \mathcal{D}^\dagger \mathcal{D}^\dagger \bar{\mathcal{H}} \Lambda^{\dot{\alpha}k} \Lambda^{\dot{\beta}l} \epsilon_{\dot{\alpha}\dot{\beta}} - \frac{1}{8} E^{ij} T_{abik} T_{acjl} \mathcal{D}^\dagger \mathcal{D}^\dagger \bar{\mathcal{H}} \Lambda^{\dot{\alpha}k} \Lambda^{\dot{\beta}l} \gamma_{bc\dot{\alpha}\dot{\beta}} \\
& - \frac{1}{24} E^{ij} T_{ab}{}^{kl} \mathcal{D} \mathcal{H} \Lambda_{\alpha i} \chi_{\beta}{}^{mn}{}^j \gamma_{ab}{}^{\alpha\beta} \epsilon_{klmn} - \frac{1}{8} E^{ij} T_{ab}{}^{kl} \mathcal{D} \mathcal{H} \Lambda_{\alpha m} \chi_{\beta}{}^{mn}{}^i \gamma_{ab}{}^{\alpha\beta} \epsilon_{jklm} + \frac{1}{16} E^{ij} \mathcal{D}^\dagger \mathcal{D}^\dagger \bar{\mathcal{H}} \Lambda^{\dot{\alpha}k} \Lambda^{\dot{\beta}l} R(V)_{ab}{}^m{}_i \gamma_{ab\dot{\alpha}\dot{\beta}} \epsilon_{jklm} \\
& - \frac{1}{4} T_{abij} T_{abkl} \mathcal{D}^\dagger \mathcal{D}^\dagger \bar{\mathcal{H}} \Lambda^{\dot{\alpha}i} \chi^{\dot{\beta}}{}_{mn}{}^j \epsilon_{\dot{\alpha}\dot{\beta}} \epsilon^{klmn} - \frac{1}{8} T_{abij} T_{ackl} \mathcal{D}^\dagger \mathcal{D}^\dagger \bar{\mathcal{H}} \Lambda^{\dot{\alpha}m} \chi^{\dot{\beta}}{}_{mn}{}^i \gamma_{bc\dot{\alpha}\dot{\beta}} \epsilon^{jklm} + \frac{1}{8} T_{abij} T_{ackl} \mathcal{D}^\dagger \mathcal{D}^\dagger \bar{\mathcal{H}} \Lambda^{\dot{\alpha}m} \chi^{\dot{\beta}}{}_{mn}{}^k \gamma_{bc\dot{\alpha}\dot{\beta}} \epsilon^{ijlm} \\
& - \frac{1}{8} T_{abij} \mathcal{D}^\dagger \bar{\mathcal{H}} \Lambda_{\alpha k} \Lambda^{\dot{\alpha}i} \gamma_c{}^\alpha{}_{\dot{\alpha}} \nabla_c T_{ablm} \epsilon^{jklm} - \frac{1}{4} T_{ab}{}^{ij} T_{ab}{}^{kl} \mathcal{D} \mathcal{D} \mathcal{H} \Lambda_{\alpha i} \chi_{\beta}{}^{mn}{}^j \epsilon^{\alpha\beta} \epsilon_{klmn} - \frac{1}{8} T_{ab}{}^{ij} T_{ac}{}^{kl} \mathcal{D} \mathcal{D} \mathcal{H} \Lambda_{\alpha m} \chi_{\beta}{}^{mn}{}^i \gamma_{bc}{}^{\alpha\beta} \epsilon_{jklm} \\
& + \frac{1}{8} T_{ab}{}^{ij} T_{ac}{}^{kl} \mathcal{D} \mathcal{D} \mathcal{H} \Lambda_{\alpha m} \chi_{\beta}{}^{mn}{}^k \gamma_{bc}{}^{\alpha\beta} \epsilon_{ijlm} + \frac{1}{8} T_{ab}{}^{ij} \mathcal{D} \mathcal{H} \Lambda_{\alpha k} \Lambda^{\dot{\alpha}l} \gamma_c{}^\alpha{}_{\dot{\alpha}} \nabla_c T_{ab}{}^{km} \epsilon_{ijlm} - \frac{2}{3} \bar{\mathcal{I}} P_a T_{ab}{}^{ij} \Lambda^{\dot{\alpha}k} \epsilon_{\dot{\alpha}\dot{\beta}} \nabla_b \Lambda^{\dot{\beta}l} \epsilon_{ijkl} \\
& + \frac{1}{2} \bar{\mathcal{I}} P_a \Lambda^{\dot{\alpha}i} \Lambda^{\dot{\beta}j} \gamma_{ab\dot{\alpha}\dot{\beta}} \nabla_c T_{bc}{}^{kl} \epsilon_{ijkl} - \frac{1}{3} \bar{\mathcal{H}} P_a T_{abij} \Lambda_{\alpha k} \epsilon^{\alpha\beta} \nabla_b \Lambda_{\beta l} \epsilon^{ijkl} - \frac{1}{3} \mathcal{D}^\dagger \bar{\mathcal{H}} E_{ij} E^{ik} P_a \Lambda_{\alpha k} \Lambda^{\dot{\alpha}j} \gamma_a{}^\alpha{}_{\dot{\alpha}} - \frac{3}{8} \mathcal{D}^\dagger \bar{\mathcal{H}} E^{ij} P_a P_a \Lambda_{\alpha i} \Lambda_{\beta j} \epsilon^{\alpha\beta} \\
& - \frac{1}{8} \mathcal{D}^\dagger \bar{\mathcal{H}} P_a T_{abij} T_{bc}{}^{ik} \Lambda_{\alpha k} \Lambda^{\dot{\alpha}j} \gamma_c{}^\alpha{}_{\dot{\alpha}} - \frac{3}{8} \mathcal{D}^\dagger \bar{\mathcal{H}} P_a T_{bcij} T_{ab}{}^{ik} \Lambda_{\alpha k} \Lambda^{\dot{\alpha}j} \gamma_c{}^\alpha{}_{\dot{\alpha}} - \frac{1}{16} \mathcal{D}^\dagger \bar{\mathcal{H}} P_a T_{bcij} T_{bc}{}^{ik} \Lambda_{\alpha k} \Lambda^{\dot{\alpha}j} \gamma_a{}^\alpha{}_{\dot{\alpha}} \\
& + \frac{5}{8} \mathcal{D}^\dagger \bar{\mathcal{H}} P_a T_{abij} \Lambda_{\alpha k} \chi^{\dot{\alpha}}{}_{lm}{}^k \gamma_b{}^\alpha{}_{\dot{\alpha}} \epsilon^{ijlm} - \frac{5}{8} \mathcal{D}^\dagger \bar{\mathcal{H}} P_a T_{ab}{}^{ij} \Lambda^{\dot{\alpha}k} \chi_{\alpha}{}^{lm}{}_k \gamma_b{}^\alpha{}_{\dot{\alpha}} \epsilon_{ijlm} - \frac{1}{3} \mathcal{D}^\dagger \mathcal{D}^\dagger \bar{\mathcal{I}} P_a P_a T_{bcij} \Lambda^{\dot{\alpha}i} \Lambda^{\dot{\beta}j} \gamma_{bc\dot{\alpha}\dot{\beta}} \\
& - \frac{5}{64} \mathcal{D}^\dagger \mathcal{D}^\dagger \bar{\mathcal{H}} T_{abij} T_{cdkl} \Lambda^{\dot{\alpha}m} R(Q)_{ab}{}^{\dot{\beta}}{}_m \gamma_{cd\dot{\alpha}\dot{\beta}} \epsilon^{ijkl} - \frac{1}{3} \mathcal{D} \mathcal{D} \mathcal{I} T_{ab}{}^{ij} \Lambda_{\alpha i} \Lambda_{\beta j} \bar{P}_c \bar{P}_c \gamma_{ab}{}^{\alpha\beta} - \frac{5}{64} \mathcal{D} \mathcal{D} \mathcal{H} T_{ab}{}^{ij} T_{cd}{}^{kl} \Lambda_{\alpha m} R(Q)_{ab\beta}{}^m \gamma_{cd}{}^{\alpha\beta} \epsilon_{ijkl} \\
& + \frac{1}{3} \mathcal{D} \mathcal{H} E_{ij} E^{ik} \Lambda_{\alpha k} \Lambda^{\dot{\alpha}j} \bar{P}_a \gamma_a{}^\alpha{}_{\dot{\alpha}} - \frac{3}{8} \mathcal{D} \mathcal{H} E_{ij} \Lambda^{\dot{\alpha}i} \Lambda^{\dot{\beta}j} \bar{P}_a \bar{P}_a \epsilon_{\dot{\alpha}\dot{\beta}} + \frac{1}{16} \mathcal{D} \mathcal{H} T_{abij} T_{ab}{}^{ik} \Lambda_{\alpha k} \Lambda^{\dot{\alpha}j} \bar{P}_c \gamma_c{}^\alpha{}_{\dot{\alpha}} \\
& - \frac{1}{8} \mathcal{D} \mathcal{H} T_{abij} T_{ac}{}^{ik} \Lambda_{\alpha k} \Lambda^{\dot{\alpha}j} \bar{P}_b \gamma_c{}^\alpha{}_{\dot{\alpha}} - \frac{3}{8} \mathcal{D} \mathcal{H} T_{abij} T_{ac}{}^{ik} \Lambda_{\alpha k} \Lambda^{\dot{\alpha}j} \bar{P}_c \gamma_b{}^\alpha{}_{\dot{\alpha}} - \frac{5}{8} \mathcal{D} \mathcal{H} T_{abij} \Lambda_{\alpha k} \bar{P}_a \chi^{\dot{\alpha}}{}_{lm}{}^k \gamma_b{}^\alpha{}_{\dot{\alpha}} \epsilon^{ijlm} \\
& + \frac{5}{8} \mathcal{D} \mathcal{H} T_{ab}{}^{ij} \Lambda^{\dot{\alpha}k} \bar{P}_a \chi_{\alpha}{}^{lm}{}_k \gamma_b{}^\alpha{}_{\dot{\alpha}} \epsilon_{ijlm} - \frac{2}{3} \mathcal{I} T_{abij} \Lambda_{\alpha k} \bar{P}_a \epsilon^{\alpha\beta} \nabla_b \Lambda_{\beta l} \epsilon^{ijkl} + \frac{1}{2} \mathcal{I} \Lambda_{\alpha i} \Lambda_{\beta j} \bar{P}_a \gamma_{ab}{}^{\alpha\beta} \nabla_c T_{bc}{}^{kl} \epsilon^{ijkl} \\
& - \frac{1}{3} \mathcal{H} T_{ab}{}^{ij} \Lambda^{\dot{\alpha}k} \bar{P}_a \epsilon_{\dot{\alpha}\dot{\beta}} \nabla_b \Lambda^{\dot{\beta}l} \epsilon_{ijkl} + \left( -\frac{21}{8} \mathcal{D}^\dagger \mathcal{I} - \frac{5}{12} \mathcal{D} \mathcal{H} \right) P_a \Lambda_{\alpha i} \Lambda^{\dot{\alpha}i} \bar{P}_b \bar{P}_b \gamma_a{}^\alpha{}_{\dot{\alpha}} + \left( -\frac{5}{3} \mathcal{D}^\dagger \bar{\mathcal{H}} - \frac{7}{24} \mathcal{D} \bar{\mathcal{I}} \right) P_a P_b \Lambda_{\alpha i} \Lambda^{\dot{\alpha}i} \bar{P}_a \gamma_b{}^\alpha{}_{\dot{\alpha}} \\
& + \left( -\frac{3}{2} \mathcal{D}^\dagger \mathcal{I} - \frac{9}{8} \mathcal{D} \mathcal{H} \right) T_{abij} T_{ac}{}^{ij} \Lambda_{\alpha k} \Lambda^{\dot{\alpha}k} \bar{P}_c \gamma_b{}^\alpha{}_{\dot{\alpha}} + \left( -\frac{7}{6} \mathcal{D}^\dagger \mathcal{I} - \frac{5}{12} \mathcal{D} \mathcal{H} \right) T_{ab}{}^{ij} \Lambda_{\alpha k} \Lambda^{\dot{\alpha}l} \gamma_c{}^\alpha{}_{\dot{\alpha}} \nabla_a T_{bc}{}^{km} \epsilon_{ijlm} \\
& + \left( -\frac{9}{8} \mathcal{D}^\dagger \bar{\mathcal{H}} - \frac{3}{2} \mathcal{D} \bar{\mathcal{I}} \right) P_a T_{bcij} T_{ab}{}^{ij} \Lambda_{\alpha k} \Lambda^{\dot{\alpha}k} \gamma_c{}^\alpha{}_{\dot{\alpha}} + \left( -\frac{7}{12} \mathcal{D}^\dagger \mathcal{I} + \frac{1}{6} \mathcal{D} \mathcal{H} \right) T_{ab}{}^{ij} T_{ac}{}^{kl} \Lambda^{\dot{\alpha}m} \gamma_c{}^\alpha{}_{\dot{\alpha}} \nabla_b \Lambda_{\alpha i} \epsilon_{jklm} \\
& + \left( -\frac{49}{96} \mathcal{D}^\dagger \mathcal{I} - \frac{7}{24} \mathcal{D} \mathcal{H} \right) T_{ab}{}^{ij} T_{ac}{}^{kl} \Lambda_{\alpha i} \gamma_b{}^\alpha{}_{\dot{\alpha}} \nabla_c \Lambda^{\dot{\alpha}m} \epsilon_{jklm} + \left( -\frac{1}{2} \bar{\mathcal{H}} - \frac{1}{2} \mathcal{H} \right) T_{abij} T_{abkl} \Lambda_{\alpha m} \chi_{\beta}{}^{ij}{}_n \epsilon^{\alpha\beta} \epsilon^{klmn} \\
& + \left( -\frac{1}{2} \bar{\mathcal{H}} - \frac{1}{2} \mathcal{H} \right) T_{ab}{}^{ij} T_{ab}{}^{kl} \Lambda^{\dot{\alpha}m} \chi^{\dot{\beta}}{}_{ij}{}^n \epsilon_{\dot{\alpha}\dot{\beta}} \epsilon_{klmn} + \left( -\frac{1}{2} \mathcal{D}^\dagger \mathcal{I} - \frac{3}{8} \mathcal{D} \mathcal{H} \right) T_{abij} T_{ac}{}^{ij} \Lambda_{\alpha k} \Lambda^{\dot{\alpha}k} \bar{P}_b \gamma_c{}^\alpha{}_{\dot{\alpha}} \\
& + \left( -\frac{47}{96} \mathcal{D}^\dagger \mathcal{I} - \frac{3}{16} \mathcal{D} \mathcal{H} \right) T_{ab}{}^{ij} \Lambda_{\alpha k} \Lambda^{\dot{\alpha}k} \gamma_c{}^\alpha{}_{\dot{\alpha}} \nabla_c T_{ab}{}^{lm} \epsilon_{ijlm} + \left( -\frac{7}{16} \bar{\mathcal{H}} + \frac{7}{16} \mathcal{H} \right) P_a \Lambda^{\dot{\alpha}i} \bar{P}_b \gamma_c{}^\alpha{}_{\dot{\alpha}} \nabla_d \Lambda_{\alpha i} \epsilon_{abcd} \\
& + \left( -\frac{5}{12} \bar{\mathcal{H}} - \frac{13}{36} \mathcal{H} \right) E^{ij} T_{ab}{}^{kl} \Lambda^{\dot{\alpha}m} \gamma_a{}^\alpha{}_{\dot{\alpha}} \nabla_b \Lambda_{\alpha i} \epsilon_{jklm} + \left( -\frac{5}{12} \bar{\mathcal{H}} - \frac{1}{3} \mathcal{H} \right) E^{ij} T_{abik} \Lambda_{\alpha j} \Lambda^{\dot{\alpha}k} \bar{P}_a \gamma_b{}^\alpha{}_{\dot{\alpha}} + 4 \dots
\end{aligned}$$

$$\begin{aligned}
F_{2,cont} = & +(-\frac{5}{12} \mathcal{D}^\dagger \bar{\mathcal{H}} - \frac{85}{48} \mathcal{D} \bar{\mathcal{L}}) T_{abij} \Lambda_{\alpha k} \Lambda^{\dot{\alpha} k} \gamma_a^\alpha \nabla_c T_{bclm} \varepsilon^{ijlm} + (-\frac{3}{8} \mathcal{D}^\dagger \bar{\mathcal{H}} - \frac{21}{32} \mathcal{D} \bar{\mathcal{L}}) T_{abij} T_{ackl} \Lambda^{\dot{\alpha} k} \gamma_c^\alpha \nabla_b \Lambda_{\alpha m} \varepsilon^{ijlm} \\
& + (-\frac{3}{8} \mathcal{D}^\dagger \bar{\mathcal{H}} - \frac{1}{2} \mathcal{D} \bar{\mathcal{L}}) P_a T_{abij} T_{bc}{}^{ij} \Lambda_{\alpha k} \Lambda^{\dot{\alpha} k} \gamma_c^\alpha \nabla_a + (-\frac{3}{8} \mathcal{D} \mathcal{D} \mathcal{H} - 5 \mathcal{D} \mathcal{I}) \Lambda_{\alpha i} \Lambda^{\dot{\alpha} i} \bar{P}_a \bar{P}_b \bar{P}_c \gamma_b^\alpha \nabla_a \\
& + (-\frac{13}{36} \bar{\mathcal{H}} - \frac{5}{12} \mathcal{H}) E_{ij} T_{abkl} \Lambda_{\alpha m} \gamma_a^\alpha \nabla_b \Lambda^{\dot{\alpha} i} \varepsilon^{jklm} + (-\frac{1}{3} \bar{\mathcal{L}} - \frac{5}{32} \mathcal{D}^\dagger \mathcal{D}^\dagger \bar{\mathcal{H}}) T_{abij} T_{ackl} \Lambda^{\dot{\alpha} i} R(Q)_{bc}{}^{\dot{\beta}}{}_m \epsilon_{\dot{\alpha}\dot{\beta}} \varepsilon^{jklm} \\
& + (-\frac{1}{3} \bar{\mathcal{L}} - \frac{5}{32} \mathcal{D}^\dagger \mathcal{D}^\dagger \bar{\mathcal{H}}) T_{abij} T_{ackl} \Lambda^{\dot{\alpha} i} R(Q)_{bd}{}^{\dot{\beta}}{}_m \gamma_{cd\dot{\alpha}\dot{\beta}} \varepsilon^{jklm} + (-\frac{1}{3} \bar{\mathcal{L}} - \frac{5}{32} \mathcal{D}^\dagger \mathcal{D}^\dagger \bar{\mathcal{H}}) T_{abij} T_{cdkl} \Lambda^{\dot{\alpha} i} R(Q)_{cd}{}^{\dot{\beta}}{}_m \gamma_{ab\dot{\alpha}\dot{\beta}} \varepsilon^{jklm} \\
& + (-\frac{1}{3} \bar{\mathcal{L}} + \frac{1}{8} \mathcal{D}^\dagger \mathcal{D}^\dagger \bar{\mathcal{H}}) T_{ab}{}^{ij} \Lambda^{\dot{\alpha} k} \Lambda^{\dot{\beta} l} \gamma_{ac\dot{\alpha}\dot{\beta}} \nabla_c P_b \varepsilon_{ijkl} + (-\frac{1}{3} \bar{\mathcal{H}} - \frac{7}{18} \mathcal{H}) T_{ab}{}^{ij} \Lambda^{\dot{\alpha} k} \bar{P}_c \gamma_{ac\dot{\alpha}\dot{\beta}} \nabla_b \Lambda^{\dot{\beta} l} \varepsilon_{ijkl} \\
& + (-\frac{1}{3} \bar{\mathcal{H}} - \frac{11}{36} \mathcal{H}) \Lambda^{\dot{\alpha} i} \Lambda^{\dot{\beta} j} \bar{P}_a \gamma_{ab\dot{\alpha}\dot{\beta}} \nabla_c T_{bc}{}^{kl} \varepsilon_{ijkl} + (-\frac{1}{3} \mathcal{D}^\dagger \bar{\mathcal{H}} - \frac{1}{4} \mathcal{D} \bar{\mathcal{L}}) E_{ij} T_{abkl} \Lambda^{\dot{\alpha} i} R(Q)_{ab}{}^{\dot{\beta}}{}_m \epsilon_{\dot{\alpha}\dot{\beta}} \varepsilon^{jklm} \\
& + (-\frac{1}{3} \mathcal{D}^\dagger \mathcal{I} - \frac{7}{24} \mathcal{D} \mathcal{H}) T_{abij} \Lambda_{\alpha k} R(Q)_{ab}{}^{\dot{\alpha}}{}_l \bar{P}_c \gamma_c^\alpha \nabla_a \varepsilon^{ijkl} + (-\frac{11}{36} \bar{\mathcal{H}} - \frac{1}{3} \mathcal{H}) P_a \Lambda_{\alpha i} \Lambda_{\beta j} \gamma_{ab}{}^{\alpha\beta} \nabla_c T_{bckl} \varepsilon^{ijkl} \\
& + (-\frac{7}{24} \mathcal{D}^\dagger \bar{\mathcal{H}} - \frac{1}{3} \mathcal{D} \bar{\mathcal{L}}) P_a T_{bc}{}^{ij} \Lambda^{\dot{\alpha} k} R(Q)_{bc\alpha}{}^l \gamma_a^\alpha \nabla_c \varepsilon_{ijkl} + (-\frac{1}{4} \mathcal{D}^\dagger \mathcal{I} - \frac{1}{3} \mathcal{D} \mathcal{H}) E^{ij} T_{ab}{}^{kl} \Lambda_{\alpha i} R(Q)_{ab\beta}{}^m \epsilon^{\alpha\beta} \varepsilon_{jklm} \\
& + (-\frac{23}{96} \mathcal{D}^\dagger \mathcal{I} - \frac{1}{6} \mathcal{D} \mathcal{H}) T_{ab}{}^{ij} T_{ab}{}^{kl} \Lambda_{\alpha m} \gamma_c^\alpha \nabla_c \Lambda^{\dot{\alpha} m} \varepsilon_{ijkl} + (-\frac{5}{24} \mathcal{D} \mathcal{D} \mathcal{H} - \frac{1}{6} \mathcal{I}) E_{ij} T_{ab}{}^{ik} \Lambda_{\alpha k} \Lambda^{\dot{\alpha} j} \bar{P}_a \gamma_b^\alpha \nabla_a \\
& + (-\frac{7}{36} \bar{\mathcal{H}} - \frac{1}{4} \mathcal{H}) E_{ij} \Lambda_{\alpha k} \Lambda^{\dot{\alpha} i} \gamma_a^\alpha \nabla_b T_{ablm} \varepsilon^{jklm} + (-\frac{3}{16} \mathcal{D}^\dagger \bar{\mathcal{H}} - \frac{1}{4} \mathcal{D} \bar{\mathcal{L}}) P_a T_{bcij} T_{bc}{}^{ij} \Lambda_{\alpha k} \Lambda^{\dot{\alpha} k} \gamma_a^\alpha \nabla_a \\
& + (-\frac{1}{6} \mathcal{D}^\dagger \bar{\mathcal{H}} - \frac{23}{96} \mathcal{D} \bar{\mathcal{L}}) T_{abij} T_{abkl} \Lambda^{\dot{\alpha} m} \gamma_c^\alpha \nabla_c \Lambda_{\alpha m} \varepsilon^{ijkl} + (-\frac{1}{6} \mathcal{D}^\dagger \bar{\mathcal{H}} + \frac{7}{12} \mathcal{D} \bar{\mathcal{L}}) T_{abij} T_{ackl} \Lambda_{\alpha m} \gamma_c^\alpha \nabla_b \Lambda^{\dot{\alpha} k} \varepsilon^{ijlm} \\
& + (-\frac{5}{32} \mathcal{D} \mathcal{D} \mathcal{H} - \frac{1}{3} \mathcal{I}) T_{ab}{}^{ij} T_{ac}{}^{kl} \Lambda_{\alpha i} R(Q)_{bc\beta}{}^m \epsilon^{\alpha\beta} \varepsilon_{jklm} + (-\frac{5}{32} \mathcal{D} \mathcal{D} \mathcal{H} - \frac{1}{3} \mathcal{I}) T_{ab}{}^{ij} T_{ac}{}^{kl} \Lambda_{\alpha i} R(Q)_{bd\beta}{}^m \gamma_{cd}{}^{\alpha\beta} \varepsilon_{jklm} \\
& + (-\frac{5}{32} \mathcal{D} \mathcal{D} \mathcal{H} - \frac{1}{3} \mathcal{I}) T_{ab}{}^{ij} T_{cd}{}^{kl} \Lambda_{\alpha i} R(Q)_{cd\beta}{}^m \gamma_{ab}{}^{\alpha\beta} \varepsilon_{jklm} + (-\frac{7}{48} \mathcal{D}^\dagger \mathcal{I} + \frac{1}{24} \mathcal{D} \mathcal{H}) T_{ab}{}^{ij} T_{ac}{}^{kl} \Lambda^{\dot{\alpha} m} \gamma_c^\alpha \nabla_b \Lambda_{\alpha m} \varepsilon_{ijkl} \\
& + (-\frac{5}{36} \bar{\mathcal{H}} - \frac{1}{12} \mathcal{H}) T_{abij} \Lambda_{\alpha k} \Lambda^{\dot{\alpha} l} \gamma_a^\alpha \nabla_b E_{lm} \varepsilon^{ijkm} + (-\frac{49}{384} \mathcal{D}^\dagger \mathcal{I} - \frac{7}{96} \mathcal{D} \mathcal{H}) T_{ab}{}^{ij} T_{ac}{}^{kl} \Lambda_{\alpha m} \gamma_b^\alpha \nabla_c \Lambda^{\dot{\alpha} m} \varepsilon_{ijkl} \\
& + (-\frac{3}{32} \mathcal{D}^\dagger \bar{\mathcal{H}} - \frac{21}{128} \mathcal{D} \bar{\mathcal{L}}) T_{abij} T_{ackl} \Lambda^{\dot{\alpha} m} \gamma_c^\alpha \nabla_b \Lambda_{\alpha m} \varepsilon^{ijkl} + (-\frac{1}{12} \mathcal{D}^\dagger \bar{\mathcal{H}} - \frac{3}{16} \mathcal{D} \bar{\mathcal{L}}) T_{abij} \Lambda_{\alpha k} \Lambda^{\dot{\alpha} k} \gamma_c^\alpha \nabla_a T_{bclm} \varepsilon^{ijlm} \\
& + (-\frac{1}{16} \mathcal{D} \mathcal{D} \mathcal{D} \mathcal{H} + \frac{1}{2} \mathcal{D} \mathcal{I}) E^{ij} \Lambda_{\alpha i} \Lambda_{\beta j} \bar{P}_a \bar{P}_b \epsilon^{\alpha\beta} + (-\frac{1}{16} \mathcal{D} \mathcal{D} \mathcal{H} + \frac{1}{12} \mathcal{I}) E_{ij} \Lambda_{\alpha k} \bar{P}_a \chi^{\dot{\alpha}}{}_{lm}{}^i \gamma_a^\alpha \nabla_c \varepsilon^{jklm} \\
& + (-\frac{1}{24} \mathcal{D}^\dagger \bar{\mathcal{H}} + \frac{7}{48} \mathcal{D} \bar{\mathcal{L}}) T_{abij} T_{ackl} \Lambda_{\alpha m} \gamma_c^\alpha \nabla_b \Lambda^{\dot{\alpha} m} \varepsilon^{ijkl} + (-\frac{1}{24} \mathcal{D}^\dagger \mathcal{I} - \frac{1}{48} \mathcal{D} \mathcal{H}) E_{ij} E^{ij} \Lambda_{\alpha k} \Lambda^{\dot{\alpha} k} \bar{P}_a \gamma_a^\alpha \nabla_a \\
& + (\frac{1}{48} \mathcal{D}^\dagger \bar{\mathcal{H}} + \frac{1}{24} \mathcal{D} \bar{\mathcal{L}}) E_{ij} E^{ij} P_a \Lambda_{\alpha k} \Lambda^{\dot{\alpha} k} \gamma_a^\alpha \nabla_a + (\frac{1}{36} \bar{\mathcal{H}} + \frac{1}{12} \mathcal{H}) E_{ij} T_{abkl} \Lambda^{\dot{\alpha} i} \gamma_a^\alpha \nabla_b \Lambda_{\alpha m} \varepsilon^{jklm} \\
& + (\frac{1}{32} \mathcal{D}^\dagger \bar{\mathcal{H}} + \frac{13}{64} \mathcal{D} \bar{\mathcal{L}}) T_{abij} T_{abkl} \Lambda_{\alpha m} \gamma_c^\alpha \nabla_c \Lambda^{\dot{\alpha} m} \varepsilon^{ijkl} + (\frac{1}{24} \mathcal{D}^\dagger \bar{\mathcal{H}} - \frac{7}{24} \mathcal{D} \bar{\mathcal{L}}) P_a \Lambda_{\alpha i} \Lambda^{\dot{\alpha} j} R(V)_{bc}{}^i{}_j \gamma_d^\alpha \nabla_c \varepsilon_{abcd} \\
& + (\frac{1}{24} \mathcal{D}^\dagger \bar{\mathcal{H}} - \frac{7}{48} \mathcal{D} \bar{\mathcal{L}}) T_{abij} T_{abkl} \Lambda_{\alpha m} \gamma_c^\alpha \nabla_c \Lambda^{\dot{\alpha} k} \varepsilon^{ijlm} + (\frac{1}{24} \mathcal{D}^\dagger \bar{\mathcal{H}} - \frac{7}{48} \mathcal{D} \bar{\mathcal{L}}) T_{abij} T_{ackl} \Lambda_{\alpha m} \gamma_b^\alpha \nabla_c \Lambda^{\dot{\alpha} m} \varepsilon^{ijkl} \\
& + (\frac{1}{24} \mathcal{D} \mathcal{D} \mathcal{H} + \frac{13}{6} \mathcal{I}) P_a T_{bc}{}^{ij} \Lambda_{\alpha i} \Lambda_{\beta j} \bar{P}_a \gamma_{bc}{}^{\alpha\beta} + (\frac{7}{96} \mathcal{D}^\dagger \bar{\mathcal{H}} + \frac{49}{384} \mathcal{D} \bar{\mathcal{L}}) T_{abij} T_{ackl} \Lambda^{\dot{\alpha} m} \gamma_b^\alpha \nabla_c \Lambda_{\alpha m} \varepsilon^{ijkl} \\
& + (\frac{5}{64} \mathcal{D} \mathcal{D} \mathcal{H} + \frac{1}{6} \mathcal{I}) T_{ab}{}^{ij} T_{cd}{}^{kl} \Lambda_{\alpha i} R(Q)_{ab\beta}{}^m \gamma_{cd}{}^{\alpha\beta} \varepsilon_{jklm} + (\frac{1}{12} \bar{\mathcal{L}} - \frac{1}{16} \mathcal{D}^\dagger \mathcal{D}^\dagger \bar{\mathcal{H}}) E^{ij} P_a \Lambda^{\dot{\alpha} k} \chi_{\alpha}{}^{lm}{}_i \gamma_a^\alpha \nabla_c \varepsilon_{jklm} \\
& + (\frac{1}{12} \bar{\mathcal{H}} + \frac{1}{36} \mathcal{H}) E^{ij} T_{ab}{}^{kl} \Lambda_{\alpha i} \gamma_a^\alpha \nabla_b \Lambda^{\dot{\alpha} m} \varepsilon_{jklm} + (\frac{1}{12} \bar{\mathcal{H}} + \frac{1}{12} \mathcal{H}) E_{ij} E_{kl} \Lambda^{\dot{\alpha} i} \chi^{\dot{\beta}}{}_{mn}{}^k \epsilon_{\dot{\alpha}\dot{\beta}} \varepsilon^{jlmn} + (\frac{1}{12} \bar{\mathcal{H}} + \frac{1}{12} \mathcal{H}) E^{ij} E^{kl} \Lambda_{\alpha i} \chi_{\beta}{}^{mn}{}_k \epsilon^{\alpha\beta} \varepsilon_{jlmn} \\
& + (\frac{1}{12} \bar{\mathcal{H}} + \frac{5}{36} \mathcal{H}) T_{ab}{}^{ij} \Lambda_{\alpha k} \Lambda^{\dot{\alpha} l} \gamma_a^\alpha \nabla_b E^{km} \varepsilon_{ijlm} + (\frac{1}{12} \bar{\mathcal{H}} + \frac{5}{36} \mathcal{H}) T_{ab}{}^{ij} \Lambda^{\dot{\alpha} k} \Lambda^{\dot{\beta} l} \gamma_{ac\dot{\alpha}\dot{\beta}} \nabla_c \bar{P}_b \varepsilon_{ijkl} + (\frac{1}{12} \bar{\mathcal{H}} + \frac{1}{6} \mathcal{H}) T_{abij} \Lambda^{\dot{\alpha} i} \Lambda^{\dot{\beta} j} \bar{P}_c \bar{P}_c \gamma_{ab\dot{\alpha}\dot{\beta}} \\
& + (\frac{1}{12} \mathcal{D}^\dagger \bar{\mathcal{H}} - \frac{7}{6} \mathcal{D} \bar{\mathcal{L}}) T_{abij} \Lambda_{\alpha k} \Lambda^{\dot{\alpha} i} \gamma_a^\alpha \nabla_c T_{bclm} \varepsilon^{jklm} + (\frac{1}{8} \bar{\mathcal{H}} + \frac{1}{6} \mathcal{H}) E^{ij} \Lambda^{\dot{\alpha} k} \bar{P}_a \chi_{\alpha}{}^{lm}{}_i \gamma_a^\alpha \nabla_c \varepsilon_{jklm} \\
& + (\frac{1}{8} \mathcal{D}^\dagger \bar{\mathcal{H}} + \frac{47}{96} \mathcal{D} \bar{\mathcal{L}}) T_{abij} \Lambda_{\alpha k} \Lambda^{\dot{\alpha} k} \gamma_c^\alpha \nabla_c T_{ablm} \varepsilon^{ijlm} + (\frac{1}{8} \mathcal{D} \mathcal{D} \mathcal{H} - \frac{1}{3} \mathcal{I}) T_{abij} \Lambda_{\alpha k} \Lambda_{\beta l} \gamma_{ac}{}^{\alpha\beta} \nabla_c \bar{P}_b \varepsilon^{ijkl} \\
& + (\frac{5}{36} \bar{\mathcal{H}} + \frac{1}{12} \mathcal{H}) T_{abij} \Lambda_{\alpha k} \Lambda_{\beta l} \gamma_{ac}{}^{\alpha\beta} \nabla_c P_b \varepsilon^{ijkl} + (\frac{7}{48} \mathcal{D}^\dagger \mathcal{I} - \frac{1}{24} \mathcal{D} \mathcal{H}) T_{ab}{}^{ij} T_{ab}{}^{kl} \Lambda^{\dot{\alpha} m} \gamma_c^\alpha \nabla_c \Lambda_{\alpha k} \varepsilon_{ijlm} \\
& + (\frac{7}{48} \mathcal{D}^\dagger \mathcal{I} - \frac{1}{24} \mathcal{D} \mathcal{H}) T_{ab}{}^{ij} T_{ac}{}^{kl} \Lambda^{\dot{\alpha} m} \gamma_b^\alpha \nabla_c \Lambda_{\alpha m} \varepsilon_{ijkl} + (\frac{5}{32} \mathcal{D} \mathcal{D} \mathcal{H} + \frac{1}{3} \mathcal{I}) T_{ab}{}^{ij} T_{ac}{}^{kl} \Lambda_{\alpha k} R(Q)_{bc\beta}{}^m \epsilon^{\alpha\beta} \varepsilon_{jklm} \\
& + (\frac{5}{32} \mathcal{D} \mathcal{D} \mathcal{H} + \frac{1}{3} \mathcal{I}) T_{ab}{}^{ij} T_{cd}{}^{kl} \Lambda_{\alpha i} R(Q)_{ac\beta}{}^m \gamma_{bd}{}^{\alpha\beta} \varepsilon_{jklm} + (\frac{21}{128} \mathcal{D}^\dagger \mathcal{I} + \frac{3}{32} \mathcal{D} \mathcal{H}) T_{ab}{}^{ij} T_{ac}{}^{kl} \Lambda_{\alpha m} \gamma_c^\alpha \nabla_b \Lambda^{\dot{\alpha} m} \varepsilon_{ijkl} + 5 \dots
\end{aligned}$$

$$\begin{aligned}
F_{2,cont} = & + \left( \frac{1}{6} \bar{\mathcal{I}} + \frac{5}{64} \mathcal{D}^\dagger \mathcal{D}^\dagger \bar{\mathcal{H}} \right) T_{abij} T_{cdkl} \Lambda^{\dot{\alpha}i} R(Q)_{ab}{}^{\dot{\beta}}{}_m \gamma_{cd\dot{\alpha}\dot{\beta}} \varepsilon^{jklm} + \left( \frac{1}{6} \bar{\mathcal{I}} + \frac{5}{24} \mathcal{D}^\dagger \mathcal{D}^\dagger \bar{\mathcal{H}} \right) E^{ij} P_a T_{abik} \Lambda_{\alpha j} \Lambda^{\dot{\alpha}k} \gamma_b{}^\alpha{}_{\dot{\alpha}} \\
& + \left( \frac{1}{6} \bar{\mathcal{H}} + \frac{1}{12} \mathcal{H} \right) P_a P_a T_{bc}{}^{ij} \Lambda_{\alpha i} \Lambda_{\beta j} \gamma_{bc}{}^{\alpha\beta} + \left( \frac{1}{6} \bar{\mathcal{H}} + \frac{1}{8} \mathcal{H} \right) E_{ij} P_a \Lambda_{\alpha k} \chi^{\dot{\alpha}}{}_{lm}{}^i \gamma_a{}^\alpha{}_{\dot{\alpha}} \varepsilon^{jklm} + \left( \frac{1}{6} \mathcal{D}^\dagger \bar{\mathcal{H}} - \frac{7}{12} \mathcal{D} \bar{\mathcal{I}} \right) T_{abij} T_{ackl} \Lambda_{\alpha m} \gamma_b{}^\alpha{}_{\dot{\alpha}} \nabla_c \Lambda^{\dot{\alpha}k} \varepsilon^{ijlm} \\
& + \left( \frac{1}{6} \mathcal{D}^\dagger \bar{\mathcal{H}} - \frac{1}{6} \mathcal{D} \bar{\mathcal{I}} \right) T_{ab}{}^{ij} \Lambda^{\dot{\alpha}k} \Lambda^{\dot{\beta}l} R(V)_{ab}{}^m{}_k \epsilon_{\dot{\alpha}\dot{\beta}} \varepsilon_{ijlm} + \left( \frac{1}{6} \mathcal{D}^\dagger \mathcal{I} - \frac{1}{6} \mathcal{D} \mathcal{H} \right) T_{abij} \Lambda_{\alpha k} \Lambda_{\beta l} R(V)_{ab}{}^k{}_m \epsilon^{\alpha\beta} \varepsilon^{ijlm} \\
& + \left( \frac{1}{4} \bar{\mathcal{H}} + \frac{7}{36} \mathcal{H} \right) E^{ij} \Lambda_{\alpha i} \Lambda^{\dot{\alpha}k} \gamma_a{}^\alpha{}_{\dot{\alpha}} \nabla_b T_{ab}{}^{lm} \varepsilon_{ijklm} + \left( \frac{1}{4} \mathcal{D}^\dagger \mathcal{I} + \frac{3}{16} \mathcal{D} \mathcal{H} \right) T_{abij} T_{ab}{}^{ij} \Lambda_{\alpha k} \Lambda^{\dot{\alpha}k} \bar{P}_c \gamma_c{}^\alpha{}_{\dot{\alpha}} \\
& + \left( \frac{53}{192} \mathcal{D}^\dagger \mathcal{I} + \frac{1}{96} \mathcal{D} \mathcal{H} \right) T_{ab}{}^{ij} T_{ab}{}^{kl} \Lambda^{\dot{\alpha}m} \gamma_c{}^\alpha{}_{\dot{\alpha}} \nabla_c \Lambda_{\alpha m} \varepsilon_{ijkl} + \left( \frac{7}{24} \mathcal{D}^\dagger \bar{\mathcal{H}} + \frac{5}{12} \mathcal{D} \bar{\mathcal{I}} \right) P_a T_{bcij} \Lambda_{\alpha k} R(Q)_{bc}{}^{\dot{\alpha}}{}_l \gamma_a{}^\alpha{}_{\dot{\alpha}} \varepsilon^{ijkl} \\
& + \left( \frac{7}{24} \mathcal{D}^\dagger \bar{\mathcal{H}} + \frac{49}{96} \mathcal{D} \bar{\mathcal{I}} \right) T_{abij} T_{ackl} \Lambda^{\dot{\alpha}k} \gamma_b{}^\alpha{}_{\dot{\alpha}} \nabla_c \Lambda_{\alpha m} \varepsilon^{ijlm} + \left( \frac{7}{24} \mathcal{D}^\dagger \mathcal{I} - \frac{1}{24} \mathcal{D} \mathcal{H} \right) \Lambda_{\alpha i} \Lambda^{\dot{\alpha}j} R(V)_{ab}{}^i{}_j \bar{P}_c \gamma_d{}^\alpha{}_{\dot{\alpha}} \varepsilon_{abcd} \\
& + \left( \frac{7}{24} \mathcal{D}^\dagger \mathcal{I} + \frac{5}{3} \mathcal{D} \mathcal{H} \right) P_a \Lambda_{\alpha i} \Lambda^{\dot{\alpha}i} \bar{P}_a \bar{P}_b \gamma_b{}^\alpha{}_{\dot{\alpha}} + \left( \frac{1}{3} \bar{\mathcal{I}} + \frac{5}{32} \mathcal{D}^\dagger \mathcal{D}^\dagger \bar{\mathcal{H}} \right) T_{abij} T_{ackl} \Lambda^{\dot{\alpha}k} R(Q)_{bc}{}^{\dot{\beta}}{}_m \epsilon_{\dot{\alpha}\dot{\beta}} \varepsilon^{ijlm} \\
& + \left( \frac{1}{3} \bar{\mathcal{I}} + \frac{5}{32} \mathcal{D}^\dagger \mathcal{D}^\dagger \bar{\mathcal{H}} \right) T_{abij} T_{cdkl} \Lambda^{\dot{\alpha}i} R(Q)_{ac}{}^{\dot{\beta}}{}_m \gamma_{bd\dot{\alpha}\dot{\beta}} \varepsilon^{jklm} + \left( \frac{1}{3} \bar{\mathcal{H}} + \frac{5}{12} \mathcal{H} \right) E_{ij} P_a T_{ab}{}^{ik} \Lambda_{\alpha k} \Lambda^{\dot{\alpha}j} \gamma_b{}^\alpha{}_{\dot{\alpha}} \\
& + \left( \frac{7}{18} \bar{\mathcal{H}} + \frac{1}{3} \mathcal{H} \right) P_a T_{bcij} \Lambda_{\alpha k} \gamma_{ab}{}^{\alpha\beta} \nabla_c \Lambda_{\beta l} \varepsilon^{ijkl} + \left( \frac{5}{12} \mathcal{D}^\dagger \bar{\mathcal{H}} + \frac{7}{6} \mathcal{D} \bar{\mathcal{I}} \right) T_{abij} \Lambda_{\alpha k} \Lambda^{\dot{\alpha}i} \gamma_c{}^\alpha{}_{\dot{\alpha}} \nabla_a T_{bclm} \varepsilon^{jklm} \\
& + \left( \frac{5}{12} \mathcal{D}^\dagger \bar{\mathcal{H}} + \frac{21}{8} \mathcal{D} \bar{\mathcal{I}} \right) P_a P_a \Lambda_{\alpha i} \Lambda^{\dot{\alpha}i} \bar{P}_b \gamma_b{}^\alpha{}_{\dot{\alpha}} + \left( \frac{5}{12} \mathcal{D}^\dagger \mathcal{I} + \frac{7}{24} \mathcal{D} \mathcal{H} \right) T_{ab}{}^{ij} \Lambda^{\dot{\alpha}k} R(Q)_{aba}{}^l \bar{P}_c \gamma_c{}^\alpha{}_{\dot{\alpha}} \varepsilon_{ijkl} \\
& + \left( \frac{7}{16} \bar{\mathcal{H}} - \frac{7}{16} \mathcal{H} \right) P_a \Lambda_{\alpha i} \bar{P}_b \gamma_c{}^\alpha{}_{\dot{\alpha}} \nabla_d \Lambda^{\dot{\alpha}i} \varepsilon_{abcd} + \left( \frac{1}{2} \mathcal{D}^\dagger \bar{\mathcal{I}} - \frac{1}{16} \mathcal{D}^\dagger \mathcal{D}^\dagger \bar{\mathcal{H}} \right) E_{ij} P_a P_a \Lambda^{\dot{\alpha}i} \Lambda^{\dot{\beta}j} \epsilon_{\dot{\alpha}\dot{\beta}} + \left( \frac{1}{2} \mathcal{D}^\dagger \mathcal{I} + \frac{2}{3} \mathcal{D} \mathcal{H} \right) E^{ij} P_a \Lambda_{\alpha i} \Lambda_{\beta j} \bar{P}_a \epsilon^{\alpha\beta} \\
& + \left( \frac{1}{2} \mathcal{D} \mathcal{D} \mathcal{H} - \mathcal{I} \right) T_{abij} \Lambda_{\alpha k} \bar{P}_c \gamma_{ac}{}^{\alpha\beta} \nabla_b \Lambda_{\beta l} \varepsilon^{ijkl} + \left( \frac{7}{12} \mathcal{D}^\dagger \mathcal{I} - \frac{1}{6} \mathcal{D} \mathcal{H} \right) T_{ab}{}^{ij} T_{ac}{}^{kl} \Lambda^{\dot{\alpha}m} \gamma_b{}^\alpha{}_{\dot{\alpha}} \nabla_c \Lambda_{\alpha i} \varepsilon_{jklm} \\
& + \left( \frac{21}{32} \mathcal{D}^\dagger \mathcal{I} + \frac{3}{8} \mathcal{D} \mathcal{H} \right) T_{ab}{}^{ij} T_{ac}{}^{kl} \Lambda_{\alpha i} \gamma_c{}^\alpha{}_{\dot{\alpha}} \nabla_b \Lambda^{\dot{\alpha}m} \varepsilon_{jklm} + \left( \frac{2}{3} \mathcal{D}^\dagger \bar{\mathcal{H}} + \frac{1}{2} \mathcal{D} \bar{\mathcal{I}} \right) E_{ij} P_a \Lambda^{\dot{\alpha}i} \Lambda^{\dot{\beta}j} \bar{P}_a \epsilon_{\dot{\alpha}\dot{\beta}} \\
& + \left( \frac{37}{48} \mathcal{D}^\dagger \mathcal{I} + \frac{7}{24} \mathcal{D} \mathcal{H} \right) T_{ab}{}^{ij} \Lambda_{\alpha k} \Lambda^{\dot{\alpha}k} \gamma_c{}^\alpha{}_{\dot{\alpha}} \nabla_a T_{bc}{}^{lm} \varepsilon_{ijlm} + \left( \bar{\mathcal{I}} - \frac{1}{2} \mathcal{D}^\dagger \mathcal{D}^\dagger \bar{\mathcal{H}} \right) P_a T_{bc}{}^{ij} \Lambda^{\dot{\alpha}k} \gamma_{ab\dot{\alpha}\dot{\beta}} \nabla_c \Lambda^{\dot{\beta}l} \varepsilon_{ijkl} \\
& + \left( \frac{7}{6} \mathcal{D}^\dagger \mathcal{I} - \frac{1}{12} \mathcal{D} \mathcal{H} \right) T_{ab}{}^{ij} \Lambda_{\alpha k} \Lambda^{\dot{\alpha}l} \gamma_a{}^\alpha{}_{\dot{\alpha}} \nabla_c T_{bc}{}^{km} \varepsilon_{ijlm} + \left( \frac{19}{16} \mathcal{D}^\dagger \mathcal{I} + \frac{11}{24} \mathcal{D} \mathcal{H} \right) T_{ab}{}^{ij} \Lambda_{\alpha k} \Lambda^{\dot{\alpha}k} \gamma_a{}^\alpha{}_{\dot{\alpha}} \nabla_c T_{bc}{}^{lm} \varepsilon_{ijlm} \\
& + \left( \frac{13}{6} \bar{\mathcal{I}} + \frac{1}{24} \mathcal{D}^\dagger \mathcal{D}^\dagger \bar{\mathcal{H}} \right) P_a T_{bcij} \Lambda^{\dot{\alpha}i} \Lambda^{\dot{\beta}j} \bar{P}_a \gamma_{bc\dot{\alpha}\dot{\beta}} + \left( 5 \mathcal{D}^\dagger \bar{\mathcal{I}} + \frac{3}{8} \mathcal{D}^\dagger \mathcal{D}^\dagger \bar{\mathcal{H}} \right) P_a P_a P_b \Lambda_{\alpha i} \Lambda^{\dot{\alpha}i} \gamma_b{}^\alpha{}_{\dot{\alpha}} \\
& + \frac{7}{288} E_{ij} E_{kl} T_{abmn} \mathcal{D}^\dagger \bar{\mathcal{H}} \Lambda^{\dot{\alpha}i} \Lambda^{\dot{\beta}k} \gamma_{ab\dot{\alpha}\dot{\beta}} \varepsilon^{jlmn} + \frac{1}{64} E_{ij} E_{kl} T_{ab}{}^{ik} \mathcal{D} \mathcal{D} \mathcal{D} \mathcal{H} \Lambda_{\alpha m} \Lambda_{\beta n} \gamma_{ab}{}^{\alpha\beta} \varepsilon^{jlmn} + \frac{1}{48} E_{ij} T_{abkl} T_{abmn} \mathcal{D}^\dagger \mathcal{D}^\dagger \bar{\mathcal{H}} \Lambda^{\dot{\alpha}i} \Lambda^{\dot{\beta}j} \epsilon_{\dot{\alpha}\dot{\beta}} \varepsilon^{klmn} \\
& - \frac{1}{12} E_{ij} T_{abkl} T_{acmn} \mathcal{D}^\dagger \mathcal{D}^\dagger \bar{\mathcal{H}} \Lambda^{\dot{\alpha}i} \Lambda^{\dot{\beta}m} \gamma_{bc\dot{\alpha}\dot{\beta}} \varepsilon^{jklm} + \frac{1}{64} E^{ij} E^{kl} T_{abik} \mathcal{D}^\dagger \mathcal{D}^\dagger \mathcal{D}^\dagger \bar{\mathcal{H}} \Lambda^{\dot{\alpha}m} \Lambda^{\dot{\beta}n} \gamma_{ab\dot{\alpha}\dot{\beta}} \varepsilon_{jlmn} \\
& + \frac{7}{288} E^{ij} E^{kl} T_{ab}{}^{mn} \mathcal{D} \mathcal{H} \Lambda_{\alpha i} \Lambda_{\beta k} \gamma_{ab}{}^{\alpha\beta} \varepsilon_{jlmn} + \frac{1}{48} E^{ij} T_{ab}{}^{kl} T_{ab}{}^{mn} \mathcal{D} \mathcal{D} \mathcal{H} \Lambda_{\alpha i} \Lambda_{\beta j} \epsilon^{\alpha\beta} \varepsilon_{klmn} \\
& + \frac{1}{12} E^{ij} T_{ab}{}^{kl} T_{ac}{}^{mn} \mathcal{D} \mathcal{D} \mathcal{H} \Lambda_{\alpha i} \Lambda_{\beta k} \gamma_{bc}{}^{\alpha\beta} \varepsilon_{jlmn} + \frac{1}{12} T_{abij} T_{ackl} T_{bcmn} \mathcal{D}^\dagger \mathcal{D}^\dagger \mathcal{D}^\dagger \bar{\mathcal{H}} \Lambda^{\dot{\alpha}i} \Lambda^{\dot{\beta}m} \epsilon_{\dot{\alpha}\dot{\beta}} \varepsilon^{jklm} \\
& - \frac{1}{64} T_{abij} T_{abkl} T_{cdmn} \mathcal{D}^\dagger \mathcal{D}^\dagger \mathcal{D}^\dagger \bar{\mathcal{H}} \Lambda^{\dot{\alpha}k} \Lambda^{\dot{\beta}l} \gamma_{cd\dot{\alpha}\dot{\beta}} \varepsilon^{ijmn} - \frac{1}{32} T_{abij} T_{ackl} T_{cdmn} \mathcal{D}^\dagger \mathcal{D}^\dagger \mathcal{D}^\dagger \bar{\mathcal{H}} \Lambda^{\dot{\alpha}k} \Lambda^{\dot{\beta}l} \gamma_{bd\dot{\alpha}\dot{\beta}} \varepsilon^{ijmn} \\
& + \frac{1}{32} T_{abij} T_{ackl} T_{cdmn} \mathcal{D}^\dagger \mathcal{D}^\dagger \mathcal{D}^\dagger \bar{\mathcal{H}} \Lambda^{\dot{\alpha}m} \Lambda^{\dot{\beta}n} \gamma_{bd\dot{\alpha}\dot{\beta}} \varepsilon^{ijkl} - \frac{1}{8} T_{abij} T_{abkl} T_{cd}{}^{kl} \mathcal{D} \mathcal{H} \Lambda_{\alpha m} \Lambda_{\beta n} \gamma_{cd}{}^{\alpha\beta} \varepsilon^{ijmn} \\
& + \frac{49}{96} T_{abij} T_{ackl} \Lambda_{\alpha m} \Lambda^{\dot{\alpha}k} \bar{\mathcal{H}} \bar{P}_b \gamma_c{}^\alpha{}_{\dot{\alpha}} \varepsilon^{ijlm} - \frac{21}{32} T_{abij} T_{ackl} \Lambda_{\alpha m} \Lambda^{\dot{\alpha}k} \bar{\mathcal{H}} \bar{P}_c \gamma_b{}^\alpha{}_{\dot{\alpha}} \varepsilon^{ijlm} + \frac{49}{384} T_{abij} T_{ackl} \Lambda_{\alpha m} \Lambda^{\dot{\alpha}m} \bar{\mathcal{H}} \bar{P}_b \gamma_c{}^\alpha{}_{\dot{\alpha}} \varepsilon^{ijkl} \\
& - \frac{21}{128} T_{abij} T_{ackl} \Lambda_{\alpha m} \Lambda^{\dot{\alpha}m} \bar{\mathcal{H}} \bar{P}_c \gamma_b{}^\alpha{}_{\dot{\alpha}} \varepsilon^{ijkl} - \frac{1}{8} T_{abij} T_{cd}{}^{kl} T_{cd}{}^{ij} \mathcal{D}^\dagger \bar{\mathcal{H}} \Lambda^{\dot{\alpha}m} \Lambda^{\dot{\beta}n} \gamma_{ab\dot{\alpha}\dot{\beta}} \varepsilon_{klmn} + \frac{1}{12} T_{ab}{}^{ij} T_{ac}{}^{kl} T_{bc}{}^{mn} \mathcal{D} \mathcal{D} \mathcal{D} \mathcal{H} \Lambda_{\alpha i} \Lambda_{\beta m} \epsilon^{\alpha\beta} \varepsilon_{jklm} \\
& - \frac{1}{64} T_{ab}{}^{ij} T_{ab}{}^{kl} T_{cd}{}^{mn} \mathcal{D} \mathcal{D} \mathcal{D} \mathcal{H} \Lambda_{\alpha k} \Lambda_{\beta l} \gamma_{cd}{}^{\alpha\beta} \varepsilon_{ijmn} - \frac{1}{32} T_{ab}{}^{ij} T_{ac}{}^{kl} T_{cd}{}^{mn} \mathcal{D} \mathcal{D} \mathcal{D} \mathcal{H} \Lambda_{\alpha k} \Lambda_{\beta l} \gamma_{bd}{}^{\alpha\beta} \varepsilon_{ijmn} \\
& + \frac{1}{32} T_{ab}{}^{ij} T_{ac}{}^{kl} T_{cd}{}^{mn} \mathcal{D} \mathcal{D} \mathcal{D} \mathcal{H} \Lambda_{\alpha m} \Lambda_{\beta n} \gamma_{bd}{}^{\alpha\beta} \varepsilon_{ijkl} + \frac{5}{12} \mathcal{D}^\dagger \bar{\mathcal{H}} E_{ij} P_a T_{abkl} \Lambda_{\alpha m} \Lambda^{\dot{\alpha}i} \gamma_b{}^\alpha{}_{\dot{\alpha}} \varepsilon^{jklm} \\
& + \frac{5}{12} \mathcal{D}^\dagger \bar{\mathcal{H}} E^{ij} P_a T_{ab}{}^{kl} \Lambda_{\alpha i} \Lambda^{\dot{\alpha}m} \gamma_b{}^\alpha{}_{\dot{\alpha}} \varepsilon_{jklm} + \frac{13}{36} \mathcal{D}^\dagger \bar{\mathcal{H}} P_a P_b T_{acij} \Lambda_{\alpha k} \Lambda_{\beta l} \gamma_{bc}{}^{\alpha\beta} \varepsilon^{ijkl} - \frac{5}{12} \mathcal{D} \mathcal{H} E_{ij} T_{abkl} \Lambda_{\alpha m} \Lambda^{\dot{\alpha}i} \bar{P}_a \gamma_b{}^\alpha{}_{\dot{\alpha}} \varepsilon^{jklm} + 6 \dots
\end{aligned}$$



$$\begin{aligned}
F_{2,cont} = & -\frac{5}{12} \mathcal{D}\mathcal{H} E^{ij} T_{ab}{}^{kl} \Lambda_{\alpha i} \Lambda^{\dot{\alpha} m} \bar{P}_a \gamma_b{}^{\alpha}{}_{\dot{\alpha}} \varepsilon_{jklm} - \frac{13}{36} \mathcal{D}\mathcal{H} T_{ab}{}^{ij} \Lambda^{\dot{\alpha} k} \Lambda^{\dot{\beta} l} \bar{P}_a \bar{P}_c \gamma_{bc\dot{\alpha}\dot{\beta}} \varepsilon_{ijkl} + \frac{7}{6} \mathcal{H} P_a T_{ab}{}^{ij} T_{bc}{}^{kl} \Lambda_{\alpha k} \Lambda^{\dot{\alpha} m} \gamma_c{}^{\alpha}{}_{\dot{\alpha}} \varepsilon_{ijlm} \\
& + \frac{7}{24} \mathcal{H} P_a T_{ab}{}^{ij} T_{bc}{}^{kl} \Lambda_{\alpha m} \Lambda^{\dot{\alpha} m} \gamma_c{}^{\alpha}{}_{\dot{\alpha}} \varepsilon_{ijkl} - \frac{7}{48} \mathcal{H} P_a T_{bc}{}^{ij} T_{bc}{}^{kl} \Lambda_{\alpha k} \Lambda^{\dot{\alpha} m} \gamma_a{}^{\alpha}{}_{\dot{\alpha}} \varepsilon_{ijlm} + (-\frac{7}{3} \bar{\mathcal{I}} - \frac{7}{12} \mathcal{D}^\dagger \mathcal{D}^\dagger \bar{\mathcal{H}}) P_a T_{abij} T_{bckl} \Lambda_{\alpha m} \Lambda^{\dot{\alpha} i} \gamma_c{}^{\alpha}{}_{\dot{\alpha}} \varepsilon^{jklm} \\
& + (-\frac{167}{96} \bar{\mathcal{I}} - \frac{31}{384} \mathcal{D}^\dagger \mathcal{D}^\dagger \bar{\mathcal{H}}) P_a T_{bcij} T_{bckl} \Lambda_{\alpha m} \Lambda^{\dot{\alpha} m} \gamma_a{}^{\alpha}{}_{\dot{\alpha}} \varepsilon^{ijkl} + (-\frac{5}{6} \mathcal{D}^\dagger \bar{\mathcal{H}} - \frac{1}{3} \mathcal{D} \bar{\mathcal{I}}) P_a T_{bc}{}^{ij} \Lambda^{\dot{\alpha} k} \Lambda^{\dot{\beta} l} \bar{P}_b \gamma_{ac\dot{\alpha}\dot{\beta}} \varepsilon_{ijkl} \\
& + (-\frac{7}{12} \bar{\mathcal{I}} - \frac{7}{48} \mathcal{D}^\dagger \mathcal{D}^\dagger \bar{\mathcal{H}}) P_a T_{abij} T_{bckl} \Lambda_{\alpha m} \Lambda^{\dot{\alpha} m} \gamma_c{}^{\alpha}{}_{\dot{\alpha}} \varepsilon^{ijkl} + (-\frac{1}{3} \mathcal{D}^\dagger \bar{\mathcal{I}} + \frac{1}{8} \mathcal{D}^\dagger \mathcal{D}^\dagger \mathcal{D}^\dagger \bar{\mathcal{H}}) P_a P_b T_{ac}{}^{ij} \Lambda^{\dot{\alpha} k} \Lambda^{\dot{\beta} l} \gamma_{bc\dot{\alpha}\dot{\beta}} \varepsilon_{ijkl} \\
& + (-\frac{1}{3} \mathcal{D}^\dagger \mathcal{I} - \frac{5}{6} \mathcal{D}\mathcal{H}) P_a T_{bcij} \Lambda_{\alpha k} \Lambda_{\beta l} \bar{P}_b \gamma_{ac}{}^{\alpha\beta} \varepsilon^{ijkl} + (-\frac{49}{192} \mathcal{D}\mathcal{D}\mathcal{H} - \frac{49}{48} \mathcal{I}) T_{ab}{}^{ij} T_{ac}{}^{kl} \Lambda_{\alpha i} \Lambda^{\dot{\alpha} m} \bar{P}_b \gamma_c{}^{\alpha}{}_{\dot{\alpha}} \varepsilon_{jklm} \\
& + (-\frac{1}{8} \mathcal{D}\mathcal{D}\mathcal{D}\mathcal{H} + \frac{1}{3} \mathcal{D}\mathcal{I}) T_{abij} \Lambda_{\alpha k} \Lambda_{\beta l} \bar{P}_a \bar{P}_c \gamma_{bc}{}^{\alpha\beta} \varepsilon^{ijkl} + (-\frac{49}{768} \mathcal{D}\mathcal{D}\mathcal{H} - \frac{49}{192} \mathcal{I}) T_{ab}{}^{ij} T_{ac}{}^{kl} \Lambda_{\alpha m} \Lambda^{\dot{\alpha} m} \bar{P}_b \gamma_c{}^{\alpha}{}_{\dot{\alpha}} \varepsilon_{ijkl} \\
& + (\frac{1}{24} \bar{\mathcal{H}} - \frac{15}{64} \mathcal{H}) P_a T_{bc}{}^{ij} T_{bc}{}^{kl} \Lambda_{\alpha m} \Lambda^{\dot{\alpha} m} \gamma_a{}^{\alpha}{}_{\dot{\alpha}} \varepsilon_{ijkl} + (\frac{1}{24} \bar{\mathcal{H}} + \frac{1}{24} \mathcal{H}) E_{ij} T_{ab}{}^{kl} T_{ab}{}^{mn} \Lambda^{\dot{\alpha} i} \Lambda^{\dot{\beta} j} \epsilon_{\dot{\alpha}\dot{\beta}} \varepsilon_{klmn} \\
& + (\frac{1}{24} \bar{\mathcal{H}} + \frac{1}{24} \mathcal{H}) E^{ij} T_{abkl} T_{abmn} \Lambda_{\alpha i} \Lambda_{\beta j} \epsilon^{\alpha\beta} \varepsilon^{klmn} + (\frac{21}{256} \mathcal{D}\mathcal{D}\mathcal{H} + \frac{21}{64} \mathcal{I}) T_{ab}{}^{ij} T_{ac}{}^{kl} \Lambda_{\alpha m} \Lambda^{\dot{\alpha} m} \bar{P}_b \gamma_c{}^{\alpha}{}_{\dot{\alpha}} \varepsilon_{ijkl} \\
& + (\frac{19}{192} \mathcal{D}\mathcal{D}\mathcal{H} + \frac{29}{16} \mathcal{I}) T_{ab}{}^{ij} T_{ab}{}^{kl} \Lambda_{\alpha m} \Lambda^{\dot{\alpha} m} \bar{P}_c \gamma_c{}^{\alpha}{}_{\dot{\alpha}} \varepsilon_{ijkl} + (\frac{19}{96} \bar{\mathcal{H}} - \frac{1}{24} \mathcal{H}) T_{abij} T_{abkl} \Lambda_{\alpha m} \Lambda^{\dot{\alpha} m} \bar{P}_c \gamma_c{}^{\alpha}{}_{\dot{\alpha}} \varepsilon^{ijkl} \\
& + (\frac{7}{24} \bar{\mathcal{I}} + \frac{7}{96} \mathcal{D}^\dagger \mathcal{D}^\dagger \bar{\mathcal{H}}) P_a T_{bcij} T_{bckl} \Lambda_{\alpha m} \Lambda^{\dot{\alpha} k} \gamma_a{}^{\alpha}{}_{\dot{\alpha}} \varepsilon^{ijlm} + (\frac{21}{64} \mathcal{D}\mathcal{D}\mathcal{H} + \frac{21}{16} \mathcal{I}) T_{ab}{}^{ij} T_{ac}{}^{kl} \Lambda_{\alpha i} \Lambda^{\dot{\alpha} m} \bar{P}_c \gamma_b{}^{\alpha}{}_{\dot{\alpha}} \varepsilon_{jklm} \\
& - \frac{1}{192} E_{ij} E_{kl} E_{mn} \mathcal{D}\mathcal{D}\mathcal{D}\mathcal{H} \Lambda_{\alpha p} \Lambda_{\beta q} \epsilon^{\alpha\beta} \varepsilon^{ikmp} \varepsilon^{jlnq} + \frac{1}{8} E_{ij} T_{abkl} T_{abmn} \mathcal{D}\mathcal{H} \Lambda_{\alpha p} \Lambda_{\beta q} \epsilon^{\alpha\beta} \varepsilon^{iklp} \varepsilon^{jmnq} \\
& - \frac{1}{192} E^{ij} E^{kl} E^{mn} \mathcal{D}^\dagger \mathcal{D}^\dagger \mathcal{D}^\dagger \bar{\mathcal{H}} \Lambda^{\dot{\alpha} p} \Lambda^{\dot{\beta} q} \epsilon_{\dot{\alpha}\dot{\beta}} \varepsilon_{ikmp} \varepsilon_{jlnq} + \frac{1}{8} E^{ij} T_{ab}{}^{kl} T_{ab}{}^{mn} \mathcal{D}^\dagger \bar{\mathcal{H}} \Lambda^{\dot{\alpha} p} \Lambda^{\dot{\beta} q} \epsilon_{\dot{\alpha}\dot{\beta}} \varepsilon_{iklp} \varepsilon_{jmnq}
\end{aligned}$$

The four fermion terms are:

$$\begin{aligned}
F_4 = & \frac{1}{6} \mathcal{D}^\dagger \bar{\mathcal{H}} \Lambda_{\alpha i} \Lambda^{\dot{\alpha} j} \chi^{\dot{\beta}}_{jk} \epsilon^{\dot{\alpha} \dot{\gamma}} \gamma_a^\alpha \epsilon_{\dot{\beta}} \nabla_a \Lambda^{\dot{\gamma} k} - \frac{1}{12} \mathcal{D}^\dagger \mathcal{I} \Lambda_{\alpha i} \Lambda_{\beta j} \Lambda^{\dot{\alpha} k} \epsilon^{\alpha \gamma} \gamma_a^\beta \epsilon_{\dot{\alpha}} \nabla_a \chi_{\gamma}^{\dot{\gamma} k} \\
& + \frac{1}{12} \mathcal{D}^\dagger \mathcal{I} \Lambda_{\alpha i} \Lambda_{\beta j} \chi_{\gamma}^{\dot{\gamma} ij} \epsilon^{\alpha \gamma} \gamma_a^\beta \epsilon_{\dot{\alpha}} \nabla_a \Lambda^{\dot{\alpha} k} - \frac{1}{3} \mathcal{D}^\dagger \mathcal{I} \Lambda_{\alpha i} \Lambda^{\dot{\alpha} j} R(Q)_{ab\beta} \epsilon^{\alpha \beta} \gamma_a^\gamma \epsilon_{\dot{\alpha}} \nabla_b \Lambda_{\gamma j} \\
& - \frac{1}{12} \mathcal{D} \bar{\mathcal{I}} \Lambda_{\alpha i} \Lambda^{\dot{\alpha} j} \Lambda^{\dot{\beta} k} \epsilon_{\dot{\alpha} \dot{\gamma}} \gamma_a^\alpha \epsilon_{\dot{\beta}} \nabla_a \chi^{\dot{\gamma}}_{jk}{}^i + \frac{1}{12} \mathcal{D} \bar{\mathcal{I}} \Lambda^{\dot{\alpha} i} \Lambda^{\dot{\beta} j} \chi^{\dot{\gamma}}_{ij}{}^k \epsilon_{\dot{\alpha} \dot{\gamma}} \gamma_a^\alpha \epsilon_{\dot{\beta}} \nabla_a \Lambda_{\alpha k} - \frac{1}{6} \mathcal{D} \mathcal{H} \Lambda_{\alpha i} \Lambda^{\dot{\alpha} j} \chi_{\beta}^{\dot{\gamma} ik} \epsilon^{\alpha \gamma} \gamma_a^\beta \epsilon_{\dot{\alpha}} \nabla_a \Lambda_{\gamma k} \\
& + \left(-\frac{1}{2} \bar{\mathcal{I}} - \frac{3}{16} \mathcal{D}^\dagger \mathcal{D}^\dagger \bar{\mathcal{H}}\right) \Lambda^{\dot{\alpha} i} \Lambda^{\dot{\beta} j} R(Q)_{ab}{}^{\dot{\gamma}}{}_i R(Q)_{ab}{}^{\dot{\delta}}{}_j \epsilon_{\dot{\alpha} \dot{\beta}} \epsilon_{\dot{\gamma} \dot{\delta}} + \left(-\frac{47}{96} \bar{\mathcal{H}} - \frac{7}{96} \mathcal{H}\right) \Lambda_{\alpha i} \Lambda_{\beta j} \Lambda^{\dot{\alpha} i} \epsilon^{\alpha \beta} \epsilon_{\dot{\alpha} \dot{\beta}} \nabla_a \nabla_a \Lambda^{\dot{\beta} j} \\
& + \left(-\frac{9}{40} \bar{\mathcal{I}} + \frac{13}{80} \mathcal{D}^\dagger \mathcal{D}^\dagger \bar{\mathcal{H}}\right) \Lambda^{\dot{\alpha} i} \Lambda^{\dot{\beta} j} \chi^{\dot{\gamma}}_{ik}{}^l \chi^{\dot{\delta}}_{jl}{}^k \epsilon_{\dot{\alpha} \dot{\gamma}} \epsilon_{\dot{\beta} \dot{\delta}} + \left(-\frac{3}{16} \mathcal{D} \mathcal{D} \mathcal{H} - \frac{1}{2} \mathcal{I}\right) \Lambda_{\alpha i} \Lambda_{\beta j} R(Q)_{ab\gamma}{}^i R(Q)_{ab\delta}{}^j \epsilon^{\alpha \beta} \epsilon^{\gamma \delta} \\
& + \left(-\frac{67}{384} \bar{\mathcal{H}} + \frac{13}{128} \mathcal{H}\right) \Lambda_{\alpha i} \Lambda_{\beta j} \epsilon^{\alpha \beta} \epsilon_{\dot{\alpha} \dot{\beta}} \nabla_a \Lambda^{\dot{\alpha} i} \nabla_a \Lambda^{\dot{\beta} j} + \left(-\frac{1}{6} \mathcal{D}^\dagger \bar{\mathcal{H}} + \frac{1}{12} \mathcal{D} \bar{\mathcal{I}}\right) \Lambda_{\alpha i} \Lambda^{\dot{\alpha} j} \chi^{\dot{\beta}}_{jk}{}^i \epsilon_{\dot{\alpha} \dot{\beta}} \gamma_a^\alpha \epsilon_{\dot{\gamma}} \nabla_a \Lambda^{\dot{\gamma} k} \\
& + \left(-\frac{13}{80} \mathcal{D} \mathcal{D} \mathcal{H} + \frac{9}{40} \mathcal{I}\right) \Lambda_{\alpha i} \Lambda_{\beta j} \chi_{\gamma}^{\dot{\gamma} ik} \chi_{\delta}^{\dot{\gamma} jl}{}^k \epsilon^{\alpha \beta} \epsilon^{\gamma \delta} + \left(-\frac{7}{48} \mathcal{D}^\dagger \mathcal{I} - \frac{1}{24} \mathcal{D} \mathcal{H}\right) \Lambda_{\alpha i} \Lambda_{\beta j} \Lambda^{\dot{\alpha} i} \epsilon^{\alpha \gamma} \gamma_a^\beta \epsilon_{\dot{\alpha}} \nabla_b R(Q)_{ab\gamma}{}^j \\
& + \left(-\frac{7}{48} \mathcal{D}^\dagger \mathcal{I} - \frac{1}{24} \mathcal{D} \mathcal{H}\right) \Lambda_{\alpha i} \Lambda_{\beta j} \Lambda^{\dot{\alpha} i} \epsilon^{\beta \gamma} \gamma_a^\alpha \epsilon_{\dot{\alpha}} \nabla_b R(Q)_{ab\gamma}{}^j + \left(-\frac{1}{12} \bar{\mathcal{I}} + \frac{5}{32} \mathcal{D}^\dagger \mathcal{D}^\dagger \bar{\mathcal{H}}\right) \Lambda^{\dot{\alpha} i} \Lambda^{\dot{\beta} j} R(Q)_{ab}{}^{\dot{\gamma}}{}_k \chi^{\dot{\delta}}_{ij}{}^k \epsilon_{\dot{\alpha} \dot{\gamma}} \gamma_{ab\dot{\beta}\dot{\delta}} \\
& + \left(-\frac{1}{12} \mathcal{D}^\dagger \bar{\mathcal{H}} + \frac{17}{24} \mathcal{D} \bar{\mathcal{I}}\right) \Lambda_{\alpha i} \Lambda^{\dot{\alpha} i} R(Q)_{ab}{}^{\dot{\beta}}{}_j \epsilon_{\dot{\alpha} \dot{\beta}} \gamma_a^\alpha \epsilon_{\dot{\gamma}} \nabla_b \Lambda^{\dot{\gamma} j} + \left(-\frac{1}{12} \mathcal{D}^\dagger \mathcal{I} + \frac{1}{6} \mathcal{D} \mathcal{H}\right) \Lambda_{\alpha i} \Lambda^{\dot{\alpha} j} \chi_{\beta}^{\dot{\gamma} ik} \epsilon^{\alpha \beta} \gamma_a^\gamma \epsilon_{\dot{\alpha}} \nabla_a \Lambda_{\gamma k} \\
& + \left(-\frac{29}{384} \mathcal{D}^\dagger \bar{\mathcal{H}} + \frac{65}{192} \mathcal{D} \bar{\mathcal{I}}\right) \Lambda^{\dot{\alpha} i} \Lambda^{\dot{\beta} j} R(Q)_{ab}{}^{\dot{\gamma}}{}_i \epsilon_{\dot{\alpha} \dot{\gamma}} \gamma_a^\alpha \epsilon_{\dot{\beta}} \nabla_b \Lambda_{\alpha j} + \left(-\frac{29}{384} \mathcal{D}^\dagger \bar{\mathcal{H}} + \frac{65}{192} \mathcal{D} \bar{\mathcal{I}}\right) \Lambda^{\dot{\alpha} i} \Lambda^{\dot{\beta} j} R(Q)_{ab}{}^{\dot{\gamma}}{}_i \epsilon_{\dot{\beta} \dot{\gamma}} \gamma_a^\alpha \epsilon_{\dot{\alpha}} \nabla_b \Lambda_{\alpha j} \\
& + \left(-\frac{7}{96} \bar{\mathcal{H}} - \frac{47}{96} \mathcal{H}\right) \Lambda_{\alpha i} \Lambda^{\dot{\alpha} i} \Lambda^{\dot{\beta} j} \epsilon^{\alpha \beta} \epsilon_{\dot{\alpha} \dot{\beta}} \nabla_a \nabla_a \Lambda_{\beta j} + \left(-\frac{7}{96} \bar{\mathcal{H}} - \frac{7}{96} \mathcal{H}\right) \Lambda_{\alpha i} \Lambda^{\dot{\alpha} i} \gamma_a^\alpha \epsilon_{\dot{\alpha}} \gamma_b^\beta \epsilon_{\dot{\beta}} \nabla_a \Lambda_{\beta j} \nabla_b \Lambda^{\dot{\beta} j} \\
& + \left(-\frac{7}{96} \bar{\mathcal{H}} - \frac{7}{96} \mathcal{H}\right) \Lambda_{\alpha i} \Lambda^{\dot{\alpha} i} \gamma_a^\alpha \epsilon_{\dot{\alpha}} \gamma_b^\beta \epsilon_{\dot{\beta}} \nabla_b \Lambda_{\beta j} \nabla_a \Lambda^{\dot{\beta} j} + \left(-\frac{7}{96} \bar{\mathcal{H}} - \frac{7}{96} \mathcal{H}\right) \Lambda_{\alpha i} \Lambda^{\dot{\alpha} i} \gamma_a^\alpha \epsilon_{\dot{\alpha}} \gamma_b^\beta \epsilon_{\dot{\beta}} \nabla_a \Lambda_{\beta j} \nabla_b \Lambda^{\dot{\beta} j} \\
& + \left(-\frac{7}{96} \bar{\mathcal{H}} - \frac{7}{96} \mathcal{H}\right) \Lambda_{\alpha i} \Lambda^{\dot{\alpha} i} \gamma_a^\alpha \epsilon_{\dot{\alpha}} \gamma_b^\beta \epsilon_{\dot{\beta}} \nabla_b \Lambda_{\beta j} \nabla_a \Lambda^{\dot{\beta} j} + \left(-\frac{19}{384} \bar{\mathcal{H}} + \frac{13}{128} \mathcal{H}\right) \Lambda_{\alpha i} \Lambda_{\beta j} \epsilon^{\alpha \beta} \gamma_{ab\dot{\alpha}\dot{\beta}} \nabla_a \Lambda^{\dot{\alpha} i} \nabla_b \Lambda^{\dot{\beta} j} \\
& + \left(-\frac{1}{24} \bar{\mathcal{H}} - \frac{3}{16} \mathcal{H}\right) \Lambda_{\alpha i} \Lambda^{\dot{\alpha} j} \epsilon^{\alpha \beta} \gamma_{ab\dot{\alpha}\dot{\beta}} \nabla_a \Lambda_{\beta j} \nabla_b \Lambda^{\dot{\beta} i} + \left(-\frac{1}{24} \mathcal{D}^\dagger \bar{\mathcal{H}} - \frac{7}{48} \mathcal{D} \bar{\mathcal{I}}\right) \Lambda_{\alpha i} \Lambda^{\dot{\alpha} i} \Lambda^{\dot{\beta} j} \epsilon_{\dot{\alpha} \dot{\gamma}} \gamma_a^\alpha \epsilon_{\dot{\beta}} \nabla_b R(Q)_{ab}{}^{\dot{\gamma}}{}_j \\
& + \left(-\frac{1}{24} \mathcal{D}^\dagger \bar{\mathcal{H}} - \frac{7}{48} \mathcal{D} \bar{\mathcal{I}}\right) \Lambda_{\alpha i} \Lambda^{\dot{\alpha} i} \Lambda^{\dot{\beta} j} \epsilon_{\dot{\beta} \dot{\gamma}} \gamma_a^\alpha \epsilon_{\dot{\alpha}} \nabla_b R(Q)_{ab}{}^{\dot{\gamma}}{}_j + \left(-\frac{5}{256} \bar{\mathcal{H}} + \frac{1}{256} \mathcal{H}\right) \Lambda_{\alpha i} \Lambda_{\beta j} \gamma_a^\alpha \epsilon_{\dot{\alpha}} \gamma_b^\beta \epsilon_{\dot{\beta}} \nabla_a \Lambda^{\dot{\alpha} j} \nabla_b \Lambda^{\dot{\beta} i} \\
& + \left(-\frac{5}{256} \bar{\mathcal{H}} + \frac{1}{256} \mathcal{H}\right) \Lambda_{\alpha i} \Lambda_{\beta j} \gamma_a^\alpha \epsilon_{\dot{\alpha}} \gamma_b^\beta \epsilon_{\dot{\beta}} \nabla_a \Lambda^{\dot{\beta} j} \nabla_b \Lambda^{\dot{\alpha} i} + \left(-\frac{1}{64} \mathcal{D}^\dagger \bar{\mathcal{H}} - \frac{37}{96} \mathcal{D} \bar{\mathcal{I}}\right) \Lambda_{\alpha i} \Lambda^{\dot{\alpha} j} R(Q)_{ab}{}^{\dot{\beta}}{}_j \epsilon_{\dot{\alpha} \dot{\beta}} \gamma_a^\alpha \epsilon_{\dot{\gamma}} \nabla_b \Lambda^{\dot{\gamma} i} \\
& + \left(-\frac{1}{256} \bar{\mathcal{H}} + \frac{5}{256} \mathcal{H}\right) \Lambda^{\dot{\alpha} i} \Lambda^{\dot{\beta} j} \gamma_a^\alpha \epsilon_{\dot{\alpha}} \gamma_b^\beta \epsilon_{\dot{\beta}} \nabla_a \Lambda_{\alpha i} \nabla_b \Lambda_{\beta j} + \left(-\frac{1}{256} \bar{\mathcal{H}} + \frac{5}{256} \mathcal{H}\right) \Lambda^{\dot{\alpha} i} \Lambda^{\dot{\beta} j} \gamma_a^\alpha \epsilon_{\dot{\alpha}} \gamma_b^\beta \epsilon_{\dot{\beta}} \nabla_a \Lambda_{\beta i} \nabla_b \Lambda_{\alpha j} \\
& + \left(\frac{1}{384} \bar{\mathcal{H}} + \frac{1}{128} \mathcal{H}\right) \Lambda_{\alpha i} \Lambda_{\beta j} \epsilon_{\dot{\alpha} \dot{\beta}} \gamma_{ab}{}^{\alpha \beta} \nabla_a \Lambda^{\dot{\alpha} i} \nabla_b \Lambda^{\dot{\beta} j} + \left(\frac{1}{256} \bar{\mathcal{H}} - \frac{5}{256} \mathcal{H}\right) \Lambda^{\dot{\alpha} i}$$

$$\begin{aligned}
F_{4,cont} = & + \left( \frac{13}{80} \mathcal{D}\mathcal{D}\mathcal{H} - \frac{9}{40} \mathcal{I} \right) \Lambda_{\alpha i} \Lambda_{\beta j} \chi_{\gamma}{}^{ik} \iota \chi_{\delta}{}^{jl} k \epsilon^{\alpha\gamma} \epsilon^{\beta\delta} + \left( \frac{3}{16} \bar{\mathcal{H}} + \frac{1}{24} \mathcal{H} \right) \Lambda_{\alpha i} \Lambda^{\dot{\alpha} j} \epsilon_{\dot{\alpha}\dot{\beta}} \gamma_{ab}{}^{\alpha\beta} \nabla_a \Lambda_{\beta j} \nabla_b \Lambda^{\dot{\beta} i} \\
& + \left( \frac{3}{16} \mathcal{D}\mathcal{D}\mathcal{H} + \frac{1}{3} \mathcal{I} \right) \Lambda_{\alpha i} \Lambda_{\beta j} R(Q)_{ab\gamma}{}^i R(Q)_{ab\delta}{}^j \epsilon^{\alpha\delta} \epsilon^{\beta\gamma} + \left( \frac{3}{16} \mathcal{D}\mathcal{D}\mathcal{H} + \frac{1}{3} \mathcal{I} \right) \Lambda_{\alpha i} \Lambda_{\beta j} R(Q)_{ab\gamma}{}^i R(Q)_{ab\delta}{}^j \epsilon^{\alpha\gamma} \epsilon^{\beta\delta} \\
& + \left( \frac{5}{24} \bar{\mathcal{H}} - \frac{1}{24} \mathcal{H} \right) \Lambda_{\alpha i} \Lambda^{\dot{\alpha} i} \epsilon_{\dot{\alpha}\dot{\beta}} \gamma_{ab}{}^{\alpha\beta} \nabla_a \Lambda_{\beta j} \nabla_b \Lambda^{\dot{\beta} j} + \left( \frac{9}{40} \bar{\mathcal{I}} - \frac{13}{80} \mathcal{D}^\dagger \mathcal{D}^\dagger \bar{\mathcal{H}} \right) \Lambda^{\dot{\alpha} i} \Lambda^{\dot{\beta} j} \chi_{\gamma}{}^{ik} \chi_{\delta}{}^{jl} k \epsilon_{\dot{\alpha}\dot{\beta}} \epsilon_{\gamma\delta} \\
& + \left( \frac{9}{40} \bar{\mathcal{I}} + \frac{27}{80} \mathcal{D}^\dagger \mathcal{D}^\dagger \bar{\mathcal{H}} \right) \Lambda^{\dot{\alpha} i} \Lambda^{\dot{\beta} j} \chi_{\gamma}{}^{ik} \chi_{\delta}{}^{jl} k \epsilon_{\dot{\alpha}\dot{\beta}} \epsilon_{\beta\gamma} + \left( \frac{23}{96} \bar{\mathcal{H}} + \frac{23}{96} \mathcal{H} \right) \Lambda_{\alpha i} \Lambda^{\dot{\alpha} j} \epsilon^{\alpha\beta} \epsilon_{\dot{\alpha}\dot{\beta}} \nabla_a \Lambda_{\beta j} \nabla_a \Lambda^{\dot{\beta} i} \\
& + \left( \frac{5}{16} \mathcal{D}^\dagger \mathcal{I} - \frac{1}{12} \mathcal{D}\mathcal{H} \right) \Lambda_{\alpha i} \Lambda_{\beta j} R(Q)_{ab\gamma}{}^i \epsilon^{\alpha\gamma} \gamma_a{}^\beta{}_{\dot{\alpha}} \nabla_b \Lambda^{\dot{\alpha} j} + \left( \frac{5}{16} \mathcal{D}^\dagger \mathcal{I} - \frac{1}{12} \mathcal{D}\mathcal{H} \right) \Lambda_{\alpha i} \Lambda_{\beta j} R(Q)_{ab\gamma}{}^i \epsilon^{\beta\gamma} \gamma_a{}^\alpha{}_{\dot{\alpha}} \nabla_b \Lambda^{\dot{\alpha} j} \\
& + \left( \frac{1}{3} \bar{\mathcal{I}} + \frac{3}{16} \mathcal{D}^\dagger \mathcal{D}^\dagger \bar{\mathcal{H}} \right) \Lambda^{\dot{\alpha} i} \Lambda^{\dot{\beta} j} R(Q)_{ab}{}^{\dot{\gamma}}{}_i R(Q)_{ab}{}^{\dot{\delta}}{}_j \epsilon_{\dot{\alpha}\dot{\delta}} \epsilon_{\beta\dot{\gamma}} + \left( \frac{1}{3} \bar{\mathcal{I}} + \frac{3}{16} \mathcal{D}^\dagger \mathcal{D}^\dagger \bar{\mathcal{H}} \right) \Lambda^{\dot{\alpha} i} \Lambda^{\dot{\beta} j} R(Q)_{ab}{}^{\dot{\gamma}}{}_i R(Q)_{ab}{}^{\dot{\delta}}{}_j \epsilon_{\dot{\alpha}\dot{\gamma}} \epsilon_{\beta\dot{\delta}} \\
& + \left( \frac{1}{3} \mathcal{D}^\dagger \bar{\mathcal{H}} - \frac{1}{12} \mathcal{D}\bar{\mathcal{I}} \right) \Lambda_{\alpha i} \Lambda^{\dot{\alpha} j} \chi^{\dot{\beta}}{}_{jk}{}^i \epsilon_{\dot{\beta}\dot{\gamma}} \gamma_a{}^\alpha{}_{\dot{\alpha}} \nabla_a \Lambda^{\dot{\gamma} k} + \left( \frac{27}{80} \mathcal{D}\mathcal{D}\mathcal{H} + \frac{9}{40} \mathcal{I} \right) \Lambda_{\alpha i} \Lambda_{\beta j} \chi_{\gamma}{}^{ik} \iota \chi_{\delta}{}^{jl} k \epsilon^{\alpha\delta} \epsilon^{\beta\gamma} \\
& + \left( \frac{17}{24} \mathcal{D}^\dagger \mathcal{I} - \frac{1}{12} \mathcal{D}\mathcal{H} \right) \Lambda_{\alpha i} \Lambda^{\dot{\alpha} i} R(Q)_{ab\beta}{}^j \epsilon^{\alpha\beta} \gamma_a{}^\gamma{}_{\dot{\alpha}} \nabla_b \Lambda_{\gamma j} + (\bar{\mathcal{H}} + \mathcal{H}) \Lambda_{\alpha i} \Lambda^{\dot{\alpha} j} \chi_{\beta}{}^{kl} j \chi^{\dot{\beta}}{}_{kl}{}^i \epsilon^{\alpha\beta} \epsilon_{\dot{\alpha}\dot{\beta}} - \frac{1}{12} E_{ij} \mathcal{D}^\dagger \mathcal{D}^\dagger \bar{\mathcal{H}} \Lambda^{\dot{\alpha} i} \Lambda^{\dot{\beta} k} \Lambda^{\dot{\gamma} l} \chi^{\dot{\delta}}{}_{kl}{}^j \epsilon_{\dot{\alpha}\dot{\beta}} \epsilon_{\gamma\dot{\delta}} \\
& - \frac{1}{12} E^{ij} \mathcal{D}\mathcal{D}\mathcal{H} \Lambda_{\alpha i} \Lambda_{\beta k} \Lambda_{\gamma l} \chi_{\delta}{}^{kl} j \epsilon^{\alpha\beta} \epsilon^{\gamma\delta} + \frac{1}{4} T_{abij} \mathcal{D}^\dagger \bar{\mathcal{H}} \Lambda_{\alpha k} \Lambda^{\dot{\alpha} i} \Lambda^{\dot{\beta} l} \chi_{\beta}{}^{jk}{}^l \epsilon^{\alpha\beta} \gamma_{ab\dot{\alpha}\dot{\beta}} + \frac{1}{12} T_{abij} \mathcal{D}^\dagger \mathcal{D}^\dagger \mathcal{D}^\dagger \bar{\mathcal{H}} \Lambda^{\dot{\alpha} i} \Lambda^{\dot{\beta} k} \Lambda^{\dot{\gamma} l} \chi^{\dot{\delta}}{}_{kl}{}^j \epsilon_{\dot{\alpha}\dot{\beta}} \gamma_{ab\dot{\gamma}\dot{\delta}} \\
& + \frac{1}{24} T_{abij} \mathcal{D}^\dagger \mathcal{D}^\dagger \mathcal{D}^\dagger \bar{\mathcal{H}} \Lambda^{\dot{\alpha} i} \Lambda^{\dot{\beta} k} \Lambda^{\dot{\gamma} l} \chi^{\dot{\delta}}{}_{kl}{}^j \epsilon_{\dot{\alpha}\dot{\delta}} \gamma_{ab\dot{\beta}\dot{\gamma}} + \frac{1}{12} T_{abij} \mathcal{D}^\dagger \mathcal{D}^\dagger \mathcal{D}^\dagger \bar{\mathcal{H}} \Lambda^{\dot{\alpha} i} \Lambda^{\dot{\beta} k} \Lambda^{\dot{\gamma} l} \chi^{\dot{\delta}}{}_{kl}{}^j \epsilon_{\dot{\beta}\dot{\delta}} \gamma_{ab\dot{\alpha}\dot{\gamma}} \\
& + \frac{1}{12} T_{ab}{}^{ij} \mathcal{D}\mathcal{D}\mathcal{D}\mathcal{H} \Lambda_{\alpha i} \Lambda_{\beta k} \Lambda_{\gamma l} \chi_{\delta}{}^{kl} j \epsilon^{\alpha\beta} \gamma_{ab}{}^{\gamma\delta} + \frac{1}{24} T_{ab}{}^{ij} \mathcal{D}\mathcal{D}\mathcal{D}\mathcal{H} \Lambda_{\alpha i} \Lambda_{\beta k} \Lambda_{\gamma l} \chi_{\delta}{}^{kl} j \epsilon^{\alpha\delta} \gamma_{ab}{}^{\beta\gamma} \\
& + \frac{1}{12} T_{ab}{}^{ij} \mathcal{D}\mathcal{D}\mathcal{D}\mathcal{H} \Lambda_{\alpha i} \Lambda_{\beta k} \Lambda_{\gamma l} \chi_{\delta}{}^{kl} j \epsilon^{\beta\delta} \gamma_{ab}{}^{\alpha\gamma} + \frac{1}{4} T_{ab}{}^{ij} \mathcal{D}\mathcal{H} \Lambda_{\alpha i} \Lambda_{\beta k} \Lambda^{\dot{\alpha} l} \chi^{\dot{\beta}}{}_{jl}{}^k \epsilon_{\dot{\alpha}\dot{\beta}} \gamma_{ab}{}^{\alpha\beta} - \frac{1}{6} \mathcal{D}^\dagger \bar{\mathcal{I}} \Lambda^{\dot{\alpha} i} \Lambda^{\dot{\beta} j} \epsilon_{\dot{\alpha}\dot{\gamma}} \gamma_{ab\dot{\beta}\dot{\delta}} \nabla_a \Lambda^{\dot{\gamma} k} \nabla_b \Lambda^{\dot{\delta} l} \varepsilon_{ijkl} \\
& - \frac{1}{8} \mathcal{D}^\dagger \bar{\mathcal{H}} \Lambda^{\dot{\alpha} i} \Lambda^{\dot{\beta} j} \chi_{\alpha}{}^{kl}{}_i \chi_{\beta}{}^{mn}{}_j \epsilon^{\alpha\beta} \epsilon_{\dot{\alpha}\dot{\beta}} \varepsilon_{klmn} + \frac{5}{32} \mathcal{D}^\dagger \mathcal{D}^\dagger \mathcal{D}^\dagger \bar{\mathcal{H}} T_{abij} \Lambda^{\dot{\alpha} i} \Lambda^{\dot{\beta} j} \Lambda^{\dot{\gamma} k} R(Q)_{ab}{}^{\dot{\delta}}{}_k \epsilon_{\dot{\alpha}\dot{\gamma}} \epsilon_{\beta\dot{\delta}} + \frac{1}{12} \mathcal{D}^\dagger \mathcal{I} E^{ij} \Lambda_{\alpha i} \Lambda_{\beta j} \Lambda^{\dot{\alpha} k} \epsilon^{\alpha\beta} \gamma_a{}^\gamma{}_{\dot{\alpha}} \nabla_a \Lambda_{\gamma k} \\
& - \frac{3}{8} \mathcal{D}^\dagger \mathcal{I} T_{ab}{}^{ij} \Lambda_{\alpha k} \Lambda_{\beta l} \Lambda^{\dot{\alpha} k} \chi^{\dot{\beta}}{}_{ij}{}^l \epsilon_{\dot{\alpha}\dot{\beta}} \gamma_{ab}{}^{\alpha\beta} + \frac{1}{12} \mathcal{D}\bar{\mathcal{I}} E_{ij} \Lambda_{\alpha k} \Lambda^{\dot{\alpha} i} \Lambda^{\dot{\beta} j} \epsilon_{\dot{\alpha}\dot{\beta}} \gamma_a{}^\alpha{}_{\dot{\gamma}} \nabla_a \Lambda^{\dot{\gamma} k} - \frac{3}{8} \mathcal{D}\bar{\mathcal{I}} T_{abij} \Lambda_{\alpha k} \Lambda^{\dot{\alpha} k} \Lambda^{\dot{\beta} l} \chi_{\beta}{}^{ij}{}_l \epsilon^{\alpha\beta} \gamma_{ab\dot{\alpha}\dot{\beta}} \\
& + \frac{5}{32} \mathcal{D}\mathcal{D}\mathcal{D}\mathcal{H} T_{ab}{}^{ij} \Lambda_{\alpha i} \Lambda_{\beta j} \Lambda_{\gamma k} R(Q)_{ab\delta}{}^k \epsilon^{\alpha\gamma} \epsilon^{\beta\delta} - \frac{1}{6} \mathcal{D}\mathcal{I} \Lambda_{\alpha i} \Lambda_{\beta j} \epsilon^{\alpha\gamma} \gamma_{ab}{}^{\beta\delta} \nabla_a \Lambda_{\gamma k} \nabla_b \Lambda_{\delta l} \varepsilon^{ijkl} - \frac{1}{8} \mathcal{D}\mathcal{H} \Lambda_{\alpha i} \Lambda_{\beta j} \chi^{\dot{\alpha}}{}_{kl}{}^i \chi^{\dot{\beta}}{}_{mn}{}^j \epsilon^{\alpha\beta} \epsilon_{\dot{\alpha}\dot{\beta}} \varepsilon^{klmn} \\
& + \left( -\frac{71}{48} \mathcal{D}^\dagger \bar{\mathcal{H}} + \frac{55}{64} \mathcal{D}\bar{\mathcal{I}} \right) P_a \Lambda_{\alpha i} \Lambda_{\beta j} \Lambda^{\dot{\alpha} i} \epsilon^{\alpha\beta} \epsilon_{\dot{\alpha}\dot{\beta}} \nabla_a \Lambda^{\dot{\beta} j} + \left( -\frac{7}{6} \bar{\mathcal{I}} - \frac{1}{16} \mathcal{D}^\dagger \mathcal{D}^\dagger \bar{\mathcal{H}} \right) T_{abij} \Lambda_{\alpha k} \Lambda^{\dot{\alpha} i} \Lambda^{\dot{\beta} k} \gamma_c{}^\alpha{}_{\dot{\beta}} \gamma_{ab\dot{\alpha}\dot{\gamma}} \nabla_c \Lambda^{\dot{\gamma} j} \\
& + \left( -\frac{7}{12} \bar{\mathcal{I}} - \frac{3}{32} \mathcal{D}^\dagger \mathcal{D}^\dagger \bar{\mathcal{H}} \right) T_{abij} \Lambda_{\alpha k} \Lambda^{\dot{\alpha} i} \Lambda^$$

$$\begin{aligned}
F_{4,cont} = & +(-\frac{5}{48} \mathcal{D}\mathcal{D}\mathcal{D}\mathcal{H} - \frac{1}{18} \mathcal{D}\mathcal{I})T_{ab}{}^{ij}\Lambda_{\alpha i}\Lambda_{\beta j}\Lambda_{\gamma k}R(Q)_{ac\delta}{}^k\epsilon^{\gamma\delta}\gamma_{bc}{}^{\alpha\beta} + (-\frac{3}{32} \mathcal{D}\mathcal{D}\mathcal{H} - \frac{7}{12} \mathcal{I})T_{ab}{}^{ij}\Lambda_{\alpha i}\Lambda_{\beta k}\Lambda^{\dot{\alpha}k}\gamma_c{}^{\alpha}{}_{\dot{\alpha}}\gamma_{ab}{}^{\beta\gamma}\nabla_c\Lambda_{\gamma j} \\
& + (-\frac{1}{12} \bar{\mathcal{I}} - \frac{1}{32} \mathcal{D}^\dagger\mathcal{D}^\dagger\bar{\mathcal{H}})T_{abij}\Lambda^{\dot{\alpha}i}\Lambda^{\dot{\beta}j}\Lambda^{\dot{\gamma}k}\gamma_c{}^{\alpha}{}_{\dot{\alpha}}\gamma_{ab\dot{\beta}\dot{\gamma}}\nabla_c\Lambda_{\alpha k} + (-\frac{1}{12} \mathcal{D}^\dagger\bar{\mathcal{H}} - \frac{7}{48} \mathcal{D}\bar{\mathcal{I}})E_{ij}\Lambda_{\alpha k}\Lambda^{\dot{\alpha}i}\Lambda^{\dot{\beta}k}\epsilon_{\dot{\alpha}\dot{\beta}}\gamma_a{}^{\alpha}{}_{\dot{\gamma}}\nabla_a\Lambda^{\dot{\gamma}j} \\
& + (-\frac{1}{12} \mathcal{D}^\dagger\bar{\mathcal{H}} - \frac{7}{48} \mathcal{D}\bar{\mathcal{I}})E_{ij}\Lambda_{\alpha k}\Lambda^{\dot{\alpha}i}\Lambda^{\dot{\beta}k}\epsilon_{\dot{\beta}\dot{\gamma}}\gamma_a{}^{\alpha}{}_{\dot{\alpha}}\nabla_a\Lambda^{\dot{\gamma}j} + (-\frac{1}{12} \mathcal{D}^\dagger\bar{\mathcal{H}} - \frac{1}{18} \mathcal{D}\bar{\mathcal{I}})E_{ij}\Lambda^{\dot{\alpha}i}\Lambda^{\dot{\beta}j}\Lambda^{\dot{\gamma}k}\epsilon_{\dot{\alpha}\dot{\beta}}\gamma_a{}^{\alpha}{}_{\dot{\gamma}}\nabla_a\Lambda_{\alpha k} \\
& + (-\frac{1}{12} \mathcal{D}^\dagger\bar{\mathcal{H}} - \frac{1}{18} \mathcal{D}\bar{\mathcal{I}})E_{ij}\Lambda^{\dot{\alpha}i}\Lambda^{\dot{\beta}j}\Lambda^{\dot{\gamma}k}\epsilon_{\dot{\alpha}\dot{\gamma}}\gamma_a{}^{\alpha}{}_{\dot{\beta}}\nabla_a\Lambda_{\alpha k} + (-\frac{5}{72} \mathcal{D}^\dagger\mathcal{I} - \frac{1}{18} \mathcal{D}\mathcal{H})\Lambda_{\alpha i}\Lambda_{\beta j}\Lambda^{\dot{\alpha}i}\Lambda_{\gamma k}\epsilon^{\alpha\beta}\gamma_a{}^{\gamma}{}_{\dot{\alpha}}\nabla_aE^{jk} \\
& + (-\frac{1}{16} \bar{\mathcal{H}} + \frac{1}{6} \mathcal{H})\Lambda_{\alpha i}\Lambda^{\dot{\alpha}i}\Lambda^{\dot{\beta}j}R(Q)_{ab}{}^{\dot{\gamma}}{}_j\bar{P}_a\epsilon_{\dot{\alpha}\dot{\gamma}}\gamma_b{}^{\alpha}{}_{\dot{\beta}} + (-\frac{1}{16} \bar{\mathcal{H}} + \frac{1}{6} \mathcal{H})\Lambda_{\alpha i}\Lambda^{\dot{\alpha}i}\Lambda^{\dot{\beta}j}R(Q)_{ab}{}^{\dot{\gamma}}{}_j\bar{P}_a\epsilon_{\dot{\beta}\dot{\gamma}}\gamma_b{}^{\alpha}{}_{\dot{\alpha}} \\
& + (-\frac{1}{16} \mathcal{D}\mathcal{D}\mathcal{H} - \frac{7}{6} \mathcal{I})T_{ab}{}^{ij}\Lambda_{\alpha i}\Lambda_{\beta k}\Lambda^{\dot{\alpha}k}\gamma_c{}^{\beta}{}_{\dot{\alpha}}\gamma_{ab}{}^{\alpha\gamma}\nabla_c\Lambda_{\gamma j} + (-\frac{1}{16} \mathcal{D}\mathcal{D}\mathcal{H} - \frac{1}{6} \mathcal{I})\Lambda_{\alpha i}\Lambda_{\beta j}\Lambda_{\gamma k}\epsilon^{\alpha\beta}\gamma_a{}^{\gamma}{}_{\dot{\alpha}}\nabla_a\chi^{\dot{\alpha}}{}_{lm}{}^i\varepsilon^{jklm} \\
& + (-\frac{1}{18} \mathcal{D}^\dagger\bar{\mathcal{I}} - \frac{5}{48} \mathcal{D}^\dagger\mathcal{D}^\dagger\mathcal{D}^\dagger\bar{\mathcal{H}})T_{abij}\Lambda^{\dot{\alpha}i}\Lambda^{\dot{\beta}j}\Lambda^{\dot{\gamma}k}R(Q)_{ac}{}^{\dot{\delta}}{}_k\epsilon_{\dot{\alpha}\dot{\gamma}}\gamma_{bc\dot{\beta}\dot{\delta}} + (-\frac{1}{18} \mathcal{D}^\dagger\bar{\mathcal{I}} - \frac{5}{48} \mathcal{D}^\dagger\mathcal{D}^\dagger\mathcal{D}^\dagger\bar{\mathcal{H}})T_{abij}\Lambda^{\dot{\alpha}i}\Lambda^{\dot{\beta}j}\Lambda^{\dot{\gamma}k}R(Q)_{ac}{}^{\dot{\delta}}{}_k\epsilon_{\dot{\gamma}\dot{\delta}}\gamma_{bc\dot{\alpha}\dot{\beta}} \\
& + (-\frac{1}{18} \mathcal{D}^\dagger\bar{\mathcal{H}} - \frac{5}{72} \mathcal{D}\bar{\mathcal{I}})\Lambda_{\alpha i}\Lambda^{\dot{\alpha}i}\Lambda^{\dot{\beta}j}\Lambda^{\dot{\gamma}k}\epsilon_{\dot{\alpha}\dot{\beta}}\gamma_a{}^{\alpha}{}_{\dot{\gamma}}\nabla_aE_{jk} + (-\frac{1}{18} \mathcal{D}^\dagger\mathcal{I} - \frac{1}{12} \mathcal{D}\mathcal{H})E^{ij}\Lambda_{\alpha i}\Lambda_{\beta j}\Lambda_{\gamma k}\epsilon^{\alpha\beta}\gamma_a{}^{\gamma}{}_{\dot{\alpha}}\nabla_a\Lambda^{\dot{\alpha}k} \\
& + (-\frac{1}{18} \mathcal{D}^\dagger\mathcal{I} - \frac{1}{12} \mathcal{D}\mathcal{H})E^{ij}\Lambda_{\alpha i}\Lambda_{\beta j}\Lambda_{\gamma k}\epsilon^{\alpha\gamma}\gamma_a{}^{\beta}{}_{\dot{\alpha}}\nabla_a\Lambda^{\dot{\alpha}k} + (-\frac{5}{96} \mathcal{D}\mathcal{D}\mathcal{D}\mathcal{H} - \frac{1}{36} \mathcal{D}\mathcal{I})T_{ab}{}^{ij}\Lambda_{\alpha i}\Lambda_{\beta j}\Lambda_{\gamma k}R(Q)_{ac\delta}{}^k\epsilon^{\alpha\delta}\gamma_{bc}{}^{\beta\gamma} \\
& + (-\frac{59}{1152} \mathcal{D}^\dagger\mathcal{I} + \frac{5}{96} \mathcal{D}\mathcal{H})\Lambda_{\alpha i}\Lambda^{\dot{\alpha}i}\Lambda^{\dot{\beta}j}\bar{P}_a\gamma_a{}^{\alpha}{}_{\dot{\alpha}}\gamma_b{}^{\beta}{}_{\dot{\beta}}\nabla_b\Lambda_{\beta j} + (-\frac{59}{1152} \mathcal{D}^\dagger\mathcal{I} + \frac{5}{96} \mathcal{D}\mathcal{H})\Lambda_{\alpha i}\Lambda^{\dot{\alpha}i}\Lambda^{\dot{\beta}j}\bar{P}_a\gamma_a{}^{\alpha}{}_{\dot{\beta}}\gamma_b{}^{\beta}{}_{\dot{\alpha}}\nabla_b\Lambda_{\beta j} \\
& + (-\frac{59}{1152} \mathcal{D}^\dagger\mathcal{I} + \frac{5}{96} \mathcal{D}\mathcal{H})\Lambda_{\alpha i}\Lambda^{\dot{\alpha}i}\Lambda^{\dot{\beta}j}\bar{P}_a\gamma_a{}^{\beta}{}_{\dot{\alpha}}\gamma_b{}^{\alpha}{}_{\dot{\beta}}\nabla_b\Lambda_{\beta j} + (-\frac{59}{1152} \mathcal{D}^\dagger\mathcal{I} + \frac{5}{96} \mathcal{D}\mathcal{H})\Lambda_{\alpha i}\Lambda^{\dot{\alpha}i}\Lambda^{\dot{\beta}j}\bar{P}_a\gamma_a{}^{\beta}{}_{\dot{\beta}}\gamma_b{}^{\alpha}{}_{\dot{\alpha}}\nabla_b\Lambda_{\beta j} \\
& + (-\frac{1}{24} \bar{\mathcal{I}} + \frac{1}{64} \mathcal{D}^\dagger\mathcal{D}^\dagger\bar{\mathcal{H}})\Lambda^{\dot{\alpha}i}\Lambda^{\dot{\beta}j}\Lambda^{\dot{\gamma}k}R(S)^+{}_{ab}{}^{\dot{\delta}l}\epsilon_{\dot{\alpha}\dot{\delta}}\gamma_{ab\dot{\beta}\dot{\gamma}}\varepsilon_{ijkl} + (-\frac{1}{32} \mathcal{D}\mathcal{D}\mathcal{H} - \frac{5}{12} \mathcal{I})\Lambda_{\alpha i}\Lambda_{\beta j}\Lambda^{\dot{\alpha}i}\Lambda_{\gamma k}\gamma_b{}^{\beta}{}_{\dot{\alpha}}\gamma_{bc}{}^{\alpha\gamma}\nabla_aT_{bc}{}^{jk} \\
& + (-\frac{1}{32} \mathcal{D}\mathcal{D}\mathcal{H} - \frac{1}{12} \mathcal{I})T_{ab}{}^{ij}\Lambda_{\alpha i}\Lambda_{\beta j}\Lambda_{\gamma k}\gamma_c{}^{\alpha}{}_{\dot{\alpha}}\gamma_{ab}{}^{\beta\gamma}\nabla_c\Lambda^{\dot{\alpha}k} + (-\frac{1}{32} \mathcal{D}\mathcal{D}\mathcal{H} + \frac{1}{4} \mathcal{I})\Lambda_{\alpha i}\Lambda_{\beta j}\chi^{\dot{\alpha}}{}_{kl}{}^i\epsilon^{\alpha\beta}\gamma_a{}^{\gamma}{}_{\dot{\alpha}}\nabla_a\Lambda_{\gamma m}\varepsilon^{jklm} \\
& + (-\frac{35}{1152} \mathcal{D}^\dagger\mathcal{I} + \frac{3}{32} \mathcal{D}\mathcal{H})\Lambda_{\alpha i}\Lambda_{\beta j}\Lambda^{\dot{\alpha}i}\bar{P}_a\gamma_a{}^{\alpha}{}_{\dot{\alpha}}\gamma_b{}^{\beta}{}_{\dot{\beta}}\nabla_b\Lambda^{\dot{\beta}j} + (-\frac{35}{1152} \mathcal{D}^\dagger\mathcal{I} + \frac{3}{32} \mathcal{D}\mathcal{H})\Lambda_{\alpha i}\Lambda_{\beta j}\Lambda^{\dot{\alpha}i}\bar{P}_a\gamma_a{}^{\alpha}{}_{\dot{\beta}}\gamma_b{}^{\beta}{}_{\dot{\alpha}}\nabla_b\Lambda^{\dot{\beta}j} \\
& + (-\frac{35}{1152} \mathcal{D}^\dagger\mathcal{I} + \frac{3}{32} \mathcal{D}\mathcal{H})\Lambda_{\alpha i}\Lambda_{\beta j}\Lambda^{\dot{\alpha}i}\bar{P}_a\gamma_a{}^{\beta}{}_{\dot{\alpha}}\gamma_b{}^{\alpha}{}_{\dot{\beta}}\nabla_b\Lambda^{\dot{\beta}j} + (-\frac{35}{1152} \mathcal{D}^\dagger\mathcal{I} + \frac{3}{32} \mathcal{D}\mathcal{H})\Lambda_{\alpha i}\Lambda_{\beta j}\Lambda^{\dot{\alpha}i}\bar{P}_a\gamma_a{}^{\beta}{}_{\dot{\beta}}\gamma_b{}^{\alpha}{}_{\dot{\alpha}}\nabla_b\Lambda^{\dot{\beta}j} \\
& + (-\frac{1}{36} \mathcal{D}^\dagger\bar{\mathcal{I}} - \frac{5}{96} \mathcal{D}^\dagger\mathcal{D}^\dagger\mathcal{D}^\dagger\bar{\mathcal{H}})T_{abij}\Lambda^{\dot{\alpha}i}\Lambda^{\dot{\beta}j}\Lambda^{\dot{\gamma}k}R(Q)_{ac}{}^{\dot{\delta}}{}_k\epsilon_{\dot{\alpha}\dot{\delta}}\gamma_{bc\dot{\beta}\dot{\gamma}} + (-\frac{1}{64} \mathcal{D}\mathcal{D}\mathcal{H} + \frac{1}{24} \mathcal{I})\Lambda_{\alpha i}\Lambda_{\beta j}\Lambda_{\gamma k}R(S)^-{}_{abd\dot{i}}\epsilon^{\alpha\delta}\gamma_{ab}{}^{\beta\gamma}\varepsilon^{ijkl} \\
& + (-\frac{1}{96} \mathcal{D}\mathcal{D}\mathcal{H} + \frac{1}{12} \mathcal{I})\Lambda_{\alpha i}\Lambda_{\beta j}\chi^{\dot{\alpha}}{}_{kl}{}^i\epsilon^{\alpha\gamma}\gamma_a{}^{\beta}{}_{\dot{\alpha}}\nabla_a\Lambda_{\gamma m}\varepsilon^{jklm} + (-\frac{1}{96} \mathcal{D}\mathcal{D}\mathcal{H} + \frac{1}{12} \mathcal{I})\Lambda_{\alpha i}\Lambda_{\beta j}\chi^{\dot{\alpha}}{}_{kl}{}^i\epsilon^{\beta\gamma}\gamma_a{}^{\alpha}{}_{\dot{\alpha}}\nabla_a\Lambda_{\gamma m}\varepsilon^{jklm} \\
& + (\frac{1}{48} \bar{\mathcal{H}} - \frac{5}{48} \mathcal{H})\Lambda_{\alpha i}\Lambda_{\beta j}\Lambda^{\dot{\alpha}i}\Lambda^{\dot{\beta}k}R(V)_{ab}{}^j$$

$$\begin{aligned}
F_{4,cont} = & + \left( \frac{5}{48} \mathcal{D}^\dagger \bar{\mathcal{H}} - \frac{35}{288} \mathcal{D} \bar{\mathcal{I}} \right) \Lambda_{\alpha i} \Lambda_{\beta j} \Lambda^{\dot{\alpha} i} \Lambda^{\dot{\beta} j} \gamma_a{}^\alpha{}_\beta \gamma^b{}_\alpha{}^\beta \nabla_a P_b + \left( \frac{1}{6} \bar{\mathcal{I}} + \frac{5}{24} \mathcal{D}^\dagger \mathcal{D}^\dagger \bar{\mathcal{H}} \right) P_a \Lambda_{\alpha i} \Lambda^{\dot{\alpha} j} \Lambda^{\dot{\beta} k} \chi^{\dot{\beta} k}{}_{\dot{\gamma} j k}{}^i \epsilon^{\dot{\alpha} \dot{\gamma}} \gamma_a{}^\alpha{}_\beta \\
& + \left( \frac{1}{6} \bar{\mathcal{H}} - \frac{1}{16} \mathcal{H} \right) P_a \Lambda_{\alpha i} \Lambda_{\beta j} \Lambda^{\dot{\alpha} i} R(Q)_{ab\gamma}{}^j \epsilon^{\alpha\gamma} \gamma_b{}^\beta{}_\alpha + \left( \frac{1}{6} \bar{\mathcal{H}} - \frac{1}{16} \mathcal{H} \right) P_a \Lambda_{\alpha i} \Lambda_{\beta j} \Lambda^{\dot{\alpha} i} R(Q)_{ab\gamma}{}^j \epsilon^{\beta\gamma} \gamma_b{}^\alpha{}_\alpha \\
& + \left( \frac{19}{96} \mathcal{D}^\dagger \bar{\mathcal{H}} + \frac{53}{192} \mathcal{D} \bar{\mathcal{I}} \right) P_a \Lambda_{\alpha i} \Lambda^{\dot{\alpha} i} \Lambda^{\dot{\beta} j} \epsilon_{\dot{\alpha}\dot{\beta}} \gamma_{ab}{}^{\alpha\beta} \nabla_b \Lambda_{\beta j} + \left( \frac{5}{24} \mathcal{D} \mathcal{D} \mathcal{H} + \frac{1}{6} \mathcal{I} \right) \Lambda_{\alpha i} \Lambda_{\beta j} \Lambda^{\dot{\alpha} k} \bar{P}_a \chi_\gamma{}^{ij}{}_k \epsilon^{\alpha\gamma} \gamma_a{}^\beta{}_\alpha \\
& + \left( \frac{1}{4} \bar{\mathcal{I}} - \frac{1}{32} \mathcal{D}^\dagger \mathcal{D}^\dagger \bar{\mathcal{H}} \right) \Lambda^{\dot{\alpha} i} \Lambda^{\dot{\beta} j} \chi_{\alpha}{}^{kl}{}_{i\epsilon_{\dot{\alpha}\dot{\beta}}} \gamma_a{}^\alpha{}_\gamma \nabla_a \Lambda^{\dot{\gamma} m} \varepsilon_{jklm} + \left( \frac{53}{192} \mathcal{D}^\dagger \mathcal{I} + \frac{7}{96} \mathcal{D} \mathcal{H} \right) \Lambda_{\alpha i} \Lambda^{\dot{\alpha} i} \Lambda^{\dot{\beta} j} \bar{P}_a \epsilon^{\alpha\beta} \gamma_{ab\dot{\alpha}\dot{\beta}} \nabla_b \Lambda_{\beta j} \\
& + \left( \frac{53}{192} \mathcal{D}^\dagger \mathcal{I} + \frac{19}{96} \mathcal{D} \mathcal{H} \right) \Lambda_{\alpha i} \Lambda_{\beta j} \Lambda^{\dot{\alpha} i} \bar{P}_a \epsilon^{\alpha\beta} \gamma_{ab\dot{\alpha}\dot{\beta}} \nabla_b \Lambda^{\dot{\beta} j} + \left( \frac{1}{3} \bar{\mathcal{I}} + \frac{1}{48} \mathcal{D}^\dagger \mathcal{D}^\dagger \bar{\mathcal{H}} \right) T_{abij} \Lambda_{\alpha k} \Lambda^{\dot{\alpha} i} \Lambda^{\dot{\beta} j} \gamma_c{}^\alpha{}_\gamma \gamma_{ab\dot{\alpha}\dot{\beta}} \nabla_c \Lambda^{\dot{\gamma} k} \\
& + \left( \frac{15}{32} \mathcal{D}^\dagger \mathcal{I} - \frac{25}{48} \mathcal{D} \mathcal{H} \right) \Lambda_{\alpha i} \Lambda_{\beta j} \Lambda^{\dot{\alpha} i} \Lambda^{\dot{\beta} j} \epsilon^{\alpha\beta} \epsilon_{\dot{\alpha}\dot{\beta}} \nabla_a \bar{P}_a + \left( \frac{47}{64} \mathcal{D}^\dagger \mathcal{I} - \frac{23}{48} \mathcal{D} \mathcal{H} \right) \Lambda_{\alpha i} \Lambda_{\beta j} \Lambda^{\dot{\alpha} i} \bar{P}_a \epsilon^{\alpha\beta} \epsilon_{\dot{\alpha}\dot{\beta}} \nabla_a \Lambda^{\dot{\beta} j} \\
& + \left( \frac{3}{4} \bar{\mathcal{I}} + \frac{1}{32} \mathcal{D}^\dagger \mathcal{D}^\dagger \bar{\mathcal{H}} \right) \Lambda_{\alpha i} \Lambda^{\dot{\alpha} i} \Lambda^{\dot{\beta} j} \Lambda^{\dot{\gamma} k} \gamma_a{}^\alpha{}_\gamma \gamma_{bc\dot{\beta}\dot{\gamma}} \nabla_a T_{bcjk} + \left( \frac{55}{64} \mathcal{D}^\dagger \mathcal{I} - \frac{71}{48} \mathcal{D} \mathcal{H} \right) \Lambda_{\alpha i} \Lambda^{\dot{\alpha} i} \Lambda^{\dot{\beta} j} \bar{P}_a \epsilon^{\alpha\beta} \epsilon_{\dot{\alpha}\dot{\beta}} \nabla_a \Lambda_{\beta j} \\
& + \left( \frac{83}{72} \bar{\mathcal{I}} + \frac{1}{32} \mathcal{D}^\dagger \mathcal{D}^\dagger \bar{\mathcal{H}} \right) P_a \Lambda_{\alpha i} \Lambda^{\dot{\alpha} i} \Lambda^{\dot{\beta} j} R(Q)_{ab}{}^{\dot{\gamma}}{}_j \epsilon^{\dot{\alpha}\dot{\gamma}} \gamma_b{}^\alpha{}_\beta + \left( \frac{83}{72} \bar{\mathcal{I}} + \frac{1}{32} \mathcal{D}^\dagger \mathcal{D}^\dagger \bar{\mathcal{H}} \right) P_a \Lambda_{\alpha i} \Lambda^{\dot{\alpha} i} \Lambda^{\dot{\beta} j} R(Q)_{ab}{}^{\dot{\gamma}}{}_j \epsilon^{\dot{\beta}\dot{\gamma}} \gamma_b{}^\alpha{}_\alpha \\
& - \frac{1}{96} D^{ij}{}_{kl} \mathcal{D}^\dagger \mathcal{D}^\dagger \mathcal{D}^\dagger \bar{\mathcal{H}} \Lambda^{\dot{\alpha} k} \Lambda^{\dot{\beta} l} \Lambda^{\dot{\gamma} m} \Lambda^{\dot{\delta} n} \epsilon_{\dot{\alpha}\dot{\gamma}} \epsilon_{\dot{\beta}\dot{\delta}} \varepsilon_{ijmn} - \frac{1}{96} D^{ij}{}_{kl} \mathcal{D} \mathcal{D} \mathcal{D} \mathcal{H} \Lambda_{\alpha i} \Lambda_{\beta j} \Lambda_{\gamma m} \Lambda_{\delta n} \epsilon^{\alpha\gamma} \epsilon^{\beta\delta} \varepsilon^{klmn} \\
& + \frac{1}{96} E_{ij} E_{kl} \mathcal{D}^\dagger \mathcal{D}^\dagger \bar{\mathcal{H}} \Lambda^{\dot{\alpha} i} \Lambda^{\dot{\beta} j} \Lambda^{\dot{\gamma} k} \Lambda^{\dot{\delta} l} \epsilon_{\dot{\alpha}\dot{\beta}} \epsilon_{\dot{\gamma}\dot{\delta}} + \frac{1}{96} E_{ij} E_{kl} \mathcal{D}^\dagger \mathcal{D}^\dagger \bar{\mathcal{H}} \Lambda^{\dot{\alpha} i} \Lambda^{\dot{\beta} j} \Lambda^{\dot{\gamma} k} \Lambda^{\dot{\delta} l} \epsilon_{\dot{\alpha}\dot{\gamma}} \epsilon_{\dot{\beta}\dot{\delta}} - \frac{1}{192} E_{ij} T_{abkl} \mathcal{D}^\dagger \mathcal{D}^\dagger \bar{\mathcal{H}} \Lambda^{\dot{\alpha} i} \Lambda^{\dot{\beta} j} \Lambda^{\dot{\gamma} k} \Lambda^{\dot{\delta} l} \epsilon_{\dot{\alpha}\dot{\beta}} \gamma_{ab\dot{\gamma}\dot{\delta}} \\
& - \frac{1}{96} E_{ij} T_{abkl} \mathcal{D}^\dagger \mathcal{D}^\dagger \mathcal{D}^\dagger \bar{\mathcal{H}} \Lambda^{\dot{\alpha} i} \Lambda^{\dot{\beta} j} \Lambda^{\dot{\gamma} k} \Lambda^{\dot{\delta} l} \epsilon_{\dot{\alpha}\dot{\gamma}} \gamma_{ab\dot{\beta}\dot{\delta}} - \frac{1}{48} E_{ij} T_{ab}{}^{kl} \mathcal{D} \mathcal{H} \Lambda_{\alpha k} \Lambda_{\beta l} \Lambda^{\dot{\alpha} i} \Lambda^{\dot{\beta} j} \epsilon_{\dot{\alpha}\dot{\beta}} \gamma_{ab}{}^{\alpha\beta} \\
& - \frac{1}{12} E_{ij} \mathcal{D} \mathcal{D} \mathcal{D} \mathcal{H} \Lambda_{\alpha k} \Lambda_{\beta l} \Lambda_{\gamma m} \chi_{\delta}{}^{ik}{}_{n\epsilon^{\alpha\beta}} \epsilon^{\gamma\delta} \varepsilon^{jlmn} - \frac{1}{24} E_{ij} \mathcal{D} \mathcal{D} \mathcal{H} \Lambda_{\alpha k} \Lambda_{\beta l} \Lambda^{\dot{\alpha} i} \epsilon^{\alpha\gamma} \gamma_a{}^\beta{}_\alpha \nabla_a \Lambda_{\gamma m} \varepsilon^{jklm} \\
& - \frac{1}{6} E_{ij} \mathcal{D} \mathcal{H} \Lambda_{\alpha k} \Lambda_{\beta l} \Lambda^{\dot{\alpha} i} \chi^{\dot{\beta}}{}_{mn}{}^k \epsilon^{\alpha\beta} \epsilon_{\dot{\alpha}\dot{\beta}} \varepsilon^{jlmn} + \frac{1}{96} E^{ij} E^{kl} \mathcal{D} \mathcal{D} \mathcal{H} \Lambda_{\alpha i} \Lambda_{\beta j} \Lambda_{\gamma k} \Lambda_{\delta l} \epsilon^{\alpha\beta} \epsilon^{\gamma\delta} + \frac{1}{96} E^{ij} E^{kl} \mathcal{D} \mathcal{D} \mathcal{H} \Lambda_{\alpha i} \Lambda_{\beta j} \Lambda_{\gamma k} \Lambda_{\delta l} \epsilon^{\alpha\gamma} \epsilon^{\beta\delta} \\
& - \frac{1}{48} E^{ij} T_{abkl} \mathcal{D}^\dagger \bar{\mathcal{H}} \Lambda_{\alpha i} \Lambda_{\beta j} \Lambda^{\dot{\alpha} k} \Lambda^{\dot{\beta} l} \epsilon^{\alpha\beta} \gamma_{ab\dot{\alpha}\dot{\beta}} - \frac{1}{192} E^{ij} T_{ab}{}^{kl} \mathcal{D} \mathcal{D} \mathcal{D} \mathcal{H} \Lambda_{\alpha i} \Lambda_{\beta j} \Lambda_{\gamma k} \Lambda_{\delta l} \epsilon^{\alpha\beta} \gamma_{ab}{}^{\gamma\delta} - \frac{1}{96} E^{ij} T_{ab}{}^{kl} \mathcal{D} \mathcal{D} \mathcal{D} \mathcal{H} \Lambda_{\alpha i} \Lambda_{\beta j} \Lambda_{\gamma k} \Lambda_{\delta l} \epsilon^{\alpha\gamma} \gamma_{ab}{}^{\beta\delta} \\
& - \frac{1}{6} E^{ij} \mathcal{D}^\dagger \bar{\mathcal{H}} \Lambda_{\alpha i} \Lambda^{\dot{\alpha} k} \Lambda^{\dot{\beta} l} \chi_{\beta}{}^{mn}{}_{k\epsilon^{\alpha\beta}} \epsilon_{\dot{\alpha}\dot{\beta}} \varepsilon_{jlmn} - \frac{1}{24} E^{ij} \mathcal{D}^\dagger \mathcal{D}^\dagger \bar{\mathcal{H}} \Lambda_{\alpha i} \Lambda^{\dot{\alpha} k} \Lambda^{\dot{\beta} l} \epsilon_{\dot{\alpha}\dot{\gamma}} \gamma_a{}^\alpha{}_\beta \nabla_a \Lambda^{\dot{\gamma} m} \varepsilon_{jklm} \\
& - \frac{1}{12} E^{ij} \mathcal{D}^\dagger \mathcal{D}^\dagger \mathcal{D}^\dagger \bar{\mathcal{H}} \Lambda^{\dot{\alpha} k} \Lambda^{\dot{\beta} l} \Lambda^{\dot{\gamma} m} \chi^{\dot{\delta}}{}_{ik}{}_{n\epsilon^{\alpha\beta}} \epsilon_{\dot{\alpha}\dot{\beta}} \epsilon_{\dot{\gamma}\dot{\delta}} \varepsilon_{jlmn} + \frac{1}{48} T_{abij} T_{abkl} \mathcal{D}^\dagger \mathcal{D}^\dagger \mathcal{D}^\dagger \mathcal{D}^\dagger \bar{\mathcal{H}} \Lambda^{\dot{\alpha} i} \Lambda^{\dot{\beta} j} \Lambda^{\dot{\gamma} k} \Lambda^{\dot{\delta} l} \epsilon_{\dot{\alpha}\dot{\gamma}} \epsilon_{\dot{\beta}\dot{\delta}} \\
& - \frac{1}{32} T_{abij} T_{ackl} \mathcal{D}^\dagger \mathcal{D}^\dagger \mathcal{D}^\dagger \mathcal{D}^\dagger \bar{\mathcal{H}} \Lambda^{\dot{\alpha} i} \Lambda^{\dot{\beta} j} \Lambda^{\dot{\gamma} k} \Lambda^{\dot{\delta} l} \epsilon_{\dot{\alpha}\dot{\gamma}} \gamma_{bc\dot{\beta}\dot{\delta}} + \frac{1}{768} T_{abij} T_{cdkl} \mathcal{D}^\dagger \mathcal{D}^\dagger \mathcal{D}^\dagger \mathcal{D}^\dagger \bar{\math$$

$$\begin{aligned}
F_{4,cont} = & +(-\frac{1}{8}\bar{\mathcal{H}} - \frac{1}{8}\mathcal{H})T_{abij}\Lambda_{\alpha k}\Lambda_{\beta l}\Lambda^{\dot{\alpha}k}\chi^{\dot{\beta}}{}_{mn}{}^l\epsilon^{\alpha\beta}\gamma_{ab\dot{\alpha}\dot{\beta}}\varepsilon^{ijmn} + (-\frac{1}{8}\bar{\mathcal{H}} - \frac{1}{8}\mathcal{H})T_{ab}{}^{ij}\Lambda_{\alpha k}\Lambda^{\dot{\alpha}k}\Lambda^{\dot{\beta}l}\chi_{\beta}{}^{mn}{}_l\epsilon_{\dot{\alpha}\dot{\beta}}\gamma_{ab}{}^{\alpha\beta}\varepsilon_{ijmn} \\
& + (-\frac{17}{144}\bar{\mathcal{H}} - \frac{17}{144}\mathcal{H})P_a\Lambda_{\alpha i}\Lambda_{\beta j}\Lambda^{\dot{\alpha}i}\Lambda^{\dot{\beta}j}\bar{P}_b\gamma_a{}^{\alpha}{}_{\dot{\alpha}}\gamma_b{}^{\beta}{}_{\dot{\beta}} + (-\frac{17}{144}\bar{\mathcal{H}} - \frac{17}{144}\mathcal{H})P_a\Lambda_{\alpha i}\Lambda_{\beta j}\Lambda^{\dot{\alpha}i}\Lambda^{\dot{\beta}j}\bar{P}_b\gamma_a{}^{\alpha}{}_{\dot{\beta}}\gamma_b{}^{\beta}{}_{\dot{\alpha}} \\
& + (-\frac{3}{32}\mathcal{D}^{\dagger}\bar{\mathcal{H}} + \frac{1}{72}\mathcal{D}\bar{\mathcal{I}})T_{abij}\Lambda_{\alpha k}\Lambda^{\dot{\alpha}i}\Lambda^{\dot{\beta}j}\Lambda^{\dot{\gamma}k}\bar{P}_c\gamma_c{}^{\alpha}{}_{\dot{\alpha}}\gamma_{ab\dot{\beta}\dot{\gamma}} + (-\frac{1}{12}\mathcal{D}^{\dagger}\bar{\mathcal{H}} - \frac{1}{24}\mathcal{D}\bar{\mathcal{I}})E^{ij}\Lambda_{\alpha k}\Lambda^{\dot{\alpha}k}\Lambda^{\dot{\beta}l}\chi_{\beta}{}^{mn}{}_l\epsilon^{\alpha\beta}\epsilon_{\dot{\alpha}\dot{\beta}}\varepsilon_{ijklmn} \\
& + (-\frac{1}{16}\bar{\mathcal{H}} - \frac{1}{16}\mathcal{H})E_{ij}E^{ij}\Lambda_{\alpha k}\Lambda_{\beta l}\Lambda^{\dot{\alpha}k}\Lambda^{\dot{\beta}l}\epsilon^{\alpha\beta}\epsilon_{\dot{\alpha}\dot{\beta}} + (-\frac{1}{24}\mathcal{D}^{\dagger}\mathcal{I} - \frac{1}{12}\mathcal{D}\mathcal{H})E_{ij}\Lambda_{\alpha k}\Lambda_{\beta l}\Lambda^{\dot{\alpha}k}\chi^{\dot{\beta}}{}_{mn}{}^l\epsilon^{\alpha\beta}\epsilon_{\dot{\alpha}\dot{\beta}}\varepsilon^{ijlmn} \\
& + (-\frac{1}{48}\mathcal{D}^{\dagger}\bar{\mathcal{I}} - \frac{1}{64}\mathcal{D}^{\dagger}\mathcal{D}^{\dagger}\mathcal{D}^{\dagger}\bar{\mathcal{H}})\Lambda^{\dot{\alpha}i}\Lambda^{\dot{\beta}j}\Lambda^{\dot{\gamma}k}\Lambda^{\dot{\delta}l}R(V)_{ab}{}^{m}{}_{i}\epsilon_{\dot{\alpha}\dot{\beta}}\gamma_{ab\dot{\gamma}\dot{\delta}}\varepsilon_{ijklm} \\
& + (-\frac{1}{48}\mathcal{D}^{\dagger}\mathcal{I} + \frac{1}{12}\mathcal{D}\mathcal{H})E_{ij}T_{ab}{}^{ik}\Lambda_{\alpha k}\Lambda_{\beta l}\Lambda^{\dot{\alpha}j}\Lambda^{\dot{\beta}l}\epsilon_{\dot{\alpha}\dot{\beta}}\gamma_{ab}{}^{\alpha\beta} + (-\frac{5}{384}\mathcal{D}\mathcal{D}\mathcal{D}\mathcal{H} + \frac{1}{96}\mathcal{D}\mathcal{I})E_{ij}\Lambda_{\alpha k}\Lambda_{\beta l}\Lambda_{\gamma m}R(Q)_{ab\delta}{}^i\epsilon^{\alpha\delta}\gamma_{ab}{}^{\beta\gamma}\varepsilon^{ijklm} \\
& + (-\frac{1}{192}\mathcal{D}^{\dagger}\bar{\mathcal{I}} + \frac{1}{768}\mathcal{D}^{\dagger}\mathcal{D}^{\dagger}\mathcal{D}^{\dagger}\bar{\mathcal{H}})\Lambda^{\dot{\alpha}i}\Lambda^{\dot{\beta}j}\Lambda^{\dot{\gamma}k}\Lambda^{\dot{\delta}l}R(M)_{abcd}\gamma_{ab\dot{\alpha}\dot{\beta}}\gamma_{cd\dot{\gamma}\dot{\delta}}\varepsilon_{ijkl} \\
& + (\frac{1}{768}\mathcal{D}\mathcal{D}\mathcal{D}\mathcal{H} - \frac{1}{192}\mathcal{D}\mathcal{I})\Lambda_{\alpha i}\Lambda_{\beta j}\Lambda_{\gamma k}\Lambda_{\delta l}R(M)_{abcd}\gamma_{ab}{}^{\alpha\beta}\gamma_{cd}{}^{\gamma\delta}\varepsilon^{ijkl} \\
& + (\frac{1}{96}\mathcal{D}^{\dagger}\bar{\mathcal{I}} - \frac{5}{384}\mathcal{D}^{\dagger}\mathcal{D}^{\dagger}\mathcal{D}^{\dagger}\bar{\mathcal{H}})E^{ij}\Lambda^{\dot{\alpha}k}\Lambda^{\dot{\beta}l}\Lambda^{\dot{\gamma}m}R(Q)_{ab}{}^{\delta}{}_{i}\epsilon_{\dot{\alpha}\dot{\beta}}\gamma_{ab\dot{\beta}\dot{\gamma}}\varepsilon_{ijklm} + (\frac{1}{96}\mathcal{D}\mathcal{D}\mathcal{D}\mathcal{H} + \frac{5}{24}\mathcal{D}\mathcal{I})T_{ab}{}^{ij}\Lambda_{\alpha i}\Lambda_{\beta j}\Lambda^{\dot{\alpha}k}\Lambda_{\gamma k}\bar{P}_c\gamma_c{}^{\alpha}{}_{\dot{\alpha}}\gamma_{ab}{}^{\beta\gamma} \\
& + (\frac{1}{72}\mathcal{D}^{\dagger}\mathcal{I} - \frac{3}{32}\mathcal{D}\mathcal{H})P_aT_{bc}{}^{ij}\Lambda_{\alpha i}\Lambda_{\beta j}\Lambda^{\dot{\alpha}k}\Lambda_{\gamma k}\gamma_a{}^{\alpha}{}_{\dot{\alpha}}\gamma_{bc}{}^{\beta\gamma} + (\frac{1}{64}\mathcal{D}^{\dagger}\bar{\mathcal{H}} + \frac{59}{144}\mathcal{D}\bar{\mathcal{I}})T_{abij}\Lambda_{\alpha k}\Lambda^{\dot{\alpha}i}\Lambda^{\dot{\beta}j}\Lambda^{\dot{\gamma}k}\bar{P}_c\gamma_c{}^{\alpha}{}_{\dot{\gamma}}\gamma_{ab\dot{\alpha}\dot{\beta}} \\
& + (\frac{1}{64}\mathcal{D}\mathcal{D}\mathcal{D}\mathcal{H} + \frac{1}{48}\mathcal{D}\mathcal{I})\Lambda_{\alpha i}\Lambda_{\beta j}\Lambda_{\gamma k}\Lambda_{\delta l}R(V)_{ab}{}^i{}_{m}\epsilon^{\alpha\beta}\gamma_{ab}{}^{\gamma\delta}\varepsilon^{ijklm} + (\frac{1}{48}\mathcal{D}\mathcal{D}\mathcal{D}\mathcal{H} - \frac{1}{6}\mathcal{D}\mathcal{I})\Lambda_{\alpha i}\Lambda_{\beta j}\Lambda_{\gamma k}\bar{P}_a\chi^{\dot{\alpha}}{}_{lm}{}^i\epsilon^{\alpha\beta}\gamma_a{}^{\gamma}{}_{\dot{\alpha}}\varepsilon^{ijklm} \\
& + (\frac{1}{36}\bar{\mathcal{H}} + \frac{1}{12}\mathcal{H})E^{ij}P_a\Lambda_{\alpha i}\Lambda_{\beta j}\Lambda^{\dot{\alpha}k}\Lambda_{\gamma k}\epsilon^{\alpha\beta}\gamma_a{}^{\gamma}{}_{\dot{\alpha}} + (\frac{1}{36}\bar{\mathcal{H}} + \frac{1}{12}\mathcal{H})E^{ij}P_a\Lambda_{\alpha i}\Lambda_{\beta j}\Lambda^{\dot{\alpha}k}\Lambda_{\gamma k}\epsilon^{\alpha\gamma}\gamma_a{}^{\beta}{}_{\dot{\alpha}} \\
& + (\frac{1}{32}\mathcal{D}\mathcal{D}\mathcal{D}\mathcal{H} + \frac{37}{48}\mathcal{D}\mathcal{I})T_{ab}{}^{ij}\Lambda_{\alpha i}\Lambda_{\beta j}\Lambda^{\dot{\alpha}k}\Lambda_{\gamma k}\bar{P}_c\gamma_c{}^{\gamma}{}_{\dot{\alpha}}\gamma_{ab}{}^{\alpha\beta} + (\frac{1}{16}\bar{\mathcal{H}} + \frac{1}{16}\mathcal{H})T_{abij}T_{cd}{}^{ij}\Lambda_{\alpha k}\Lambda_{\beta l}\Lambda^{\dot{\alpha}k}\Lambda^{\dot{\beta}l}\gamma_{cd}{}^{\alpha\beta}\gamma_{ab\dot{\alpha}\dot{\beta}} \\
& + (\frac{1}{16}\bar{\mathcal{H}} + \frac{1}{16}\mathcal{H})T_{abij}T_{cd}{}^{kl}\Lambda_{\alpha k}\Lambda_{\beta l}\Lambda^{\dot{\alpha}i}\Lambda^{\dot{\beta}j}\gamma_{cd}{}^{\alpha\beta}\gamma_{ab\dot{\alpha}\dot{\beta}} + (\frac{11}{144}\bar{\mathcal{H}} + \frac{11}{144}\mathcal{H})E_{ij}E^{kl}\Lambda_{\alpha k}\Lambda_{\beta l}\Lambda^{\dot{\alpha}i}\Lambda^{\dot{\beta}j}\epsilon^{\alpha\beta}\epsilon_{\dot{\alpha}\dot{\beta}} \\
& + (\frac{1}{12}\bar{\mathcal{H}} + \frac{1}{36}\mathcal{H})E_{ij}\Lambda_{\alpha k}\Lambda^{\dot{\alpha}i}\Lambda^{\dot{\beta}j}\Lambda^{\dot{\gamma}k}\bar{P}_a\epsilon_{\dot{\alpha}\dot{\beta}}\gamma_a{}^{\alpha}{}_{\dot{\gamma}} + (\frac{1}{12}\bar{\mathcal{H}} + \frac{1}{36}\mathcal{H})E_{ij}\Lambda_{\alpha k}\Lambda^{\dot{\alpha}i}\Lambda^{\dot{\beta}j}\Lambda^{\dot{\gamma}k}\bar{P}_a\epsilon_{\dot{\alpha}\dot{\gamma}}\gamma_a{}^{\alpha}{}_{\dot{\beta}} \\
& + (\frac{1}{12}\mathcal{D}^{\dagger}\bar{\mathcal{H}} - \frac{1}{48}\mathcal{D}\bar{\mathcal{I}})E^{ij}T_{abik}\Lambda_{\alpha j}\Lambda_{\beta l}\Lambda^{\dot{\alpha}k}\Lambda^{\dot{\beta}l}\epsilon^{\alpha\beta}\gamma_{ab\dot{\alpha}\dot{\beta}} + (\frac{1}{6}\mathcal{D}\mathcal{D}\mathcal{H} + \frac{19}{18}\mathcal{I})\Lambda_{\alpha i}\Lambda_{\beta j}\Lambda^{\dot{\alpha}i}\Lambda^{\dot{\beta}j}\bar{P}_a\bar{P}_b\gamma_a{}^{\alpha}{}_{\dot{\alpha}}\gamma_b{}^{\beta}{}_{\dot{\beta}} \\
& + (\frac{1}{6}\mathcal{D}\mathcal{D}\mathcal{H} + \frac{19}{18}\mathcal{I})\Lambda_{\alpha i}\Lambda_{\beta j}\Lambda^{\dot{\alpha}i}\Lambda^{\dot{\beta}j}\bar{P}_a\bar{P}_b\gamma_a{}^{\alpha}{}_{\dot{\beta}}\gamma_b{}^{\beta}{}_{\dot{\alpha}} + (\frac{5}{24}\mathcal{D}^{\dagger}\bar{\mathcal{I}} + \frac{1}{96}\mathcal{D}^{\dagger}\mathcal{D}^{\dagger}\mathcal{D}^{\dagger}\bar{\mathcal{H}})P_aT_{bcij}\Lambda_{\alpha k}\Lambda^{\dot{\alpha}i}\Lambda^{\dot{\beta}j}\Lambda^{\dot{\gamma}k}\gamma_a{}^{\alpha}{}_{\dot{\alpha}}\gamma_{bc\dot{\beta}\dot{\gamma}} \\
& + (\frac{17}{72}\bar{\mathcal{H}} + \frac{17}{72}\mathcal{H})E_{ij}E^{ik}\Lambda_{\alpha k}\Lambda_{\beta l}\Lambda^{\dot{\alpha}j}\Lambda^{\dot{\beta}l}\epsilon^{\alpha\beta}\epsilon_{\dot{\alpha}\dot{\beta}} + (\frac{19}{48}\bar{\mathcal{H}} + \frac{19}{48}\mathcal{H})P_a\Lambda_{\alpha i}\Lambda_{\beta j}\Lambda^{\dot{\alpha}i}\Lambda^{\dot{\beta}j}\bar{P}_a\epsilon^{\alpha\beta}\epsilon_{\dot{\alpha}\dot{\beta}} \\
& + (\frac{59}{144}\mathcal{D}^{\dagger}\mathcal{I} + \frac{1}{64}\mathcal{D}\mathcal{H})P_aT_{bc}{}^{ij}\Lambda_{\alpha i}\Lambda_{\beta j}\Lambda^{\dot{\alpha}k}\Lambda_{\gamma k}\gamma_a{}^{\gamma}{}_{\dot{\alpha}}\gamma_{bc}{}^{\alpha\beta} + (\frac{37}{48}\mathcal{D}^{\dagger}\bar{\mathcal{I}} + \frac{1}{32}\mathcal{D}^{\dagger}\mathcal{D}^{\dagger}\mathcal{D}^{\dagger}\bar{\mathcal{H}})P_aT_{bcij}\Lambda_{\alpha k}\Lambda^{\dot{\alpha}i}\Lambda^{\dot{\beta}j}\Lambda^{\dot{\gamma}k}\gamma_a{}^{\alpha}{}_{\dot{\gamma}}\gamma_{bc\dot{\alpha}\dot{\beta}} \\
& + (\frac{19}{18}\bar{\mathcal{I}} + \frac{1}{6}\mathcal{D}^{\dagger}\mathcal{D}^{\dagger}\bar{\mathcal{H}})P_aP_b\Lambda_{\alpha i}\Lambda_{\beta j}\Lambda^{\dot{\alpha}i}\Lambda^{\dot{\beta}j}\gamma_a{}^{\alpha}{}_{\dot{\alpha}}\gamma_b{}^{\beta}{}_{\dot{\beta}} + (\frac{19}{18}\bar{\mathcal{I}} + \frac{1}{6}\mathcal$$

$$\begin{aligned}
F_6 = & \left(-\frac{1}{4} \mathcal{D}^\dagger \bar{\mathcal{H}} + \frac{1}{12} \mathcal{D} \bar{\mathcal{L}}\right) \Lambda_{\alpha i} \Lambda_{\beta j} \Lambda^{\dot{\alpha} i} \Lambda^{\dot{\beta} k} \Lambda^{\dot{\gamma} l} \chi^{\delta}_{kl} j^{\epsilon} \epsilon^{\alpha \beta} \epsilon_{\dot{\alpha} \dot{\beta}} \epsilon_{\dot{\gamma} \dot{\delta}} \epsilon^{\gamma}{}_{\dot{\gamma}} \nabla_a \Lambda_{\gamma k} \\
& + \left(-\frac{7}{48} \bar{\mathcal{H}} - \frac{1}{48} \mathcal{H}\right) \Lambda_{\alpha i} \Lambda_{\beta j} \Lambda^{\dot{\alpha} i} \Lambda^{\dot{\beta} j} \Lambda^{\dot{\gamma} k} \epsilon^{\alpha \beta} \epsilon_{\dot{\alpha} \dot{\gamma}} \gamma_a{}^{\gamma}{}_{\dot{\beta}} \nabla_a \Lambda_{\gamma k} + \left(-\frac{1}{16} \bar{\mathcal{H}} + \frac{1}{16} \mathcal{H}\right) \Lambda_{\alpha i} \Lambda_{\beta j} \Lambda^{\dot{\alpha} i} \Lambda^{\dot{\beta} j} \Lambda^{\dot{\gamma} k} \epsilon^{\alpha \gamma} \epsilon_{\dot{\alpha} \dot{\gamma}} \gamma_a{}^{\beta}{}_{\dot{\beta}} \nabla_a \Lambda_{\gamma k} \\
& + \left(-\frac{1}{16} \bar{\mathcal{H}} + \frac{1}{16} \mathcal{H}\right) \Lambda_{\alpha i} \Lambda_{\beta j} \Lambda^{\dot{\alpha} i} \Lambda^{\dot{\beta} j} \Lambda^{\dot{\gamma} k} \epsilon^{\alpha \gamma} \epsilon_{\dot{\beta} \dot{\gamma}} \gamma_a{}^{\beta}{}_{\dot{\alpha}} \nabla_a \Lambda_{\gamma k} + \left(-\frac{1}{48} \bar{\mathcal{H}} - \frac{7}{48} \mathcal{H}\right) \Lambda_{\alpha i} \Lambda_{\beta j} \Lambda^{\dot{\alpha} i} \Lambda^{\dot{\beta} j} \Lambda_{\gamma k} \epsilon^{\alpha \beta} \epsilon_{\dot{\alpha} \dot{\beta}} \gamma_a{}^{\gamma}{}_{\dot{\gamma}} \nabla_a \Lambda^{\dot{\gamma} k} \\
& + \left(-\frac{1}{48} \bar{\mathcal{H}} - \frac{7}{48} \mathcal{H}\right) \Lambda_{\alpha i} \Lambda_{\beta j} \Lambda^{\dot{\alpha} i} \Lambda^{\dot{\beta} j} \Lambda_{\gamma k} \epsilon^{\alpha \gamma} \epsilon_{\dot{\alpha} \dot{\beta}} \gamma_a{}^{\beta}{}_{\dot{\gamma}} \nabla_a \Lambda^{\dot{\gamma} k} + \left(\frac{1}{16} \bar{\mathcal{H}} - \frac{1}{16} \mathcal{H}\right) \Lambda_{\alpha i} \Lambda_{\beta j} \Lambda^{\dot{\alpha} i} \Lambda^{\dot{\beta} j} \Lambda_{\gamma k} \epsilon^{\alpha \gamma} \epsilon_{\dot{\alpha} \dot{\gamma}} \gamma_a{}^{\beta}{}_{\dot{\beta}} \nabla_a \Lambda^{\dot{\gamma} k} \\
& + \left(\frac{1}{16} \bar{\mathcal{H}} - \frac{1}{16} \mathcal{H}\right) \Lambda_{\alpha i} \Lambda_{\beta j} \Lambda^{\dot{\alpha} i} \Lambda^{\dot{\beta} j} \Lambda_{\gamma k} \epsilon^{\alpha \gamma} \epsilon_{\dot{\beta} \dot{\gamma}} \gamma_a{}^{\beta}{}_{\dot{\alpha}} \nabla_a \Lambda^{\dot{\gamma} k} + \left(\frac{1}{12} \mathcal{D}^\dagger \mathcal{I} - \frac{1}{4} \mathcal{D} \mathcal{H}\right) \Lambda_{\alpha i} \Lambda_{\beta j} \Lambda^{\dot{\alpha} i} \Lambda^{\dot{\beta} k} \Lambda_{\gamma l} \chi^{\delta j l}{}_{\dot{k}} \epsilon^{\alpha \beta} \epsilon_{\dot{\alpha} \dot{\beta}} \epsilon^{\gamma \delta} \\
& - \frac{1}{3} \bar{\mathcal{L}} \Lambda_{\alpha i} \Lambda^{\dot{\alpha} i} \Lambda^{\dot{\beta} j} \Lambda^{\dot{\gamma} k} \Lambda^{\dot{\delta} l} \chi_{\beta}{}^{mn} j^{\epsilon} \epsilon^{\alpha \beta} \epsilon_{\dot{\alpha} \dot{\gamma}} \epsilon_{\dot{\beta} \dot{\delta}} \varepsilon_{klmn} + \frac{1}{384} \mathcal{D}^\dagger \mathcal{D}^\dagger \mathcal{D}^\dagger \mathcal{D}^\dagger \bar{\mathcal{H}} \Lambda^{\dot{\alpha} i} \Lambda^{\dot{\beta} j} \Lambda^{\dot{\gamma} k} \Lambda^{\dot{\delta} l} \Lambda^{\dot{\epsilon} m} R(Q)_{ab}{}^{\sigma 1}{}_{\dot{i}} \epsilon_{\dot{\alpha} \dot{\beta}} \epsilon_{\dot{\gamma} \sigma 1} \gamma_{ab \dot{\delta} \dot{\epsilon}} \varepsilon_{jklm} \\
& - \frac{1}{96} \mathcal{D}^\dagger \mathcal{D}^\dagger \mathcal{D}^\dagger \mathcal{D}^\dagger \bar{\mathcal{H}} \Lambda^{\dot{\alpha} i} \Lambda^{\dot{\beta} j} \Lambda^{\dot{\gamma} k} \Lambda^{\dot{\delta} l} \Lambda^{\dot{\epsilon} m} \chi^{\sigma 1}{}_{ij}{}^n \epsilon_{\dot{\alpha} \dot{\gamma}} \epsilon_{\dot{\beta} \dot{\delta}} \epsilon_{\dot{\epsilon} \sigma 1} \varepsilon_{klmn} + \frac{1}{384} \mathcal{D} \mathcal{D} \mathcal{D} \mathcal{D} \mathcal{H} \Lambda_{\alpha i} \Lambda_{\beta j} \Lambda_{\gamma k} \Lambda_{\delta l} \Lambda_{\epsilon m} R(Q)_{ab \dot{l}}{}^i \epsilon^{\alpha \beta} \epsilon^{\gamma \epsilon 1} \gamma_{ab}{}^{\delta \epsilon} \varepsilon^{jklm} \\
& - \frac{1}{96} \mathcal{D} \mathcal{D} \mathcal{D} \mathcal{D} \mathcal{H} \Lambda_{\alpha i} \Lambda_{\beta j} \Lambda_{\gamma k} \Lambda_{\delta l} \Lambda_{\epsilon m} \chi_{\epsilon 1}{}^{ij}{}^n \epsilon^{\alpha \gamma} \epsilon^{\beta \delta} \epsilon^{\epsilon 1} \varepsilon^{klmn} - \frac{1}{3} \mathcal{I} \Lambda_{\alpha i} \Lambda_{\beta j} \Lambda^{\dot{\alpha} i} \Lambda_{\gamma k} \Lambda_{\delta l} \chi^{\dot{\beta}}{}_{mn} j^{\epsilon} \epsilon^{\alpha \gamma} \epsilon^{\beta \delta} \epsilon_{\dot{\alpha} \dot{\beta}} \varepsilon^{klmn} \\
& + \left(-\frac{3}{8} \bar{\mathcal{L}} - \frac{3}{64} \mathcal{D}^\dagger \mathcal{D}^\dagger \bar{\mathcal{H}}\right) T_{abij} \Lambda_{\alpha k} \Lambda_{\beta l} \Lambda^{\dot{\alpha} i} \Lambda^{\dot{\beta} j} \Lambda^{\dot{\gamma} k} \Lambda^{\dot{\delta} l} \epsilon^{\alpha \beta} \epsilon_{\dot{\gamma} \dot{\delta}} \gamma_{ab \dot{\alpha} \dot{\beta}} + \left(-\frac{5}{36} \mathcal{D}^\dagger \mathcal{I} + \frac{7}{72} \mathcal{D} \mathcal{H}\right) \Lambda_{\alpha i} \Lambda_{\beta j} \Lambda^{\dot{\alpha} i} \Lambda^{\dot{\beta} j} \Lambda^{\dot{\gamma} k} \Lambda_{\gamma k} \bar{P}_a \epsilon^{\alpha \beta} \epsilon_{\dot{\alpha} \dot{\beta}} \gamma_a{}^{\gamma}{}_{\dot{\gamma}} \\
& + \left(-\frac{5}{36} \mathcal{D}^\dagger \mathcal{I} + \frac{7}{72} \mathcal{D} \mathcal{H}\right) \Lambda_{\alpha i} \Lambda_{\beta j} \Lambda^{\dot{\alpha} i} \Lambda^{\dot{\beta} j} \Lambda^{\dot{\gamma} k} \Lambda_{\gamma k} \bar{P}_a \epsilon^{\alpha \beta} \epsilon_{\dot{\alpha} \dot{\gamma}} \gamma_a{}^{\gamma}{}_{\dot{\beta}} + \left(-\frac{7}{72} \mathcal{D}^\dagger \bar{\mathcal{H}} + \frac{5}{36} \mathcal{D} \bar{\mathcal{L}}\right) P_a \Lambda_{\alpha i} \Lambda_{\beta j} \Lambda^{\dot{\alpha} i} \Lambda^{\dot{\beta} j} \Lambda^{\dot{\gamma} k} \Lambda_{\gamma k} \epsilon^{\alpha \beta} \epsilon_{\dot{\alpha} \dot{\beta}} \gamma_a{}^{\gamma}{}_{\dot{\gamma}} \\
& + \left(-\frac{7}{72} \mathcal{D}^\dagger \bar{\mathcal{H}} + \frac{5}{36} \mathcal{D} \bar{\mathcal{L}}\right) P_a \Lambda_{\alpha i} \Lambda_{\beta j} \Lambda^{\dot{\alpha} i} \Lambda^{\dot{\beta} j} \Lambda^{\dot{\gamma} k} \Lambda_{\gamma k} \epsilon^{\alpha \beta} \epsilon_{\dot{\alpha} \dot{\gamma}} \gamma_a{}^{\gamma}{}_{\dot{\beta}} + \left(-\frac{1}{18} \mathcal{D}^\dagger \mathcal{I} + \frac{5}{144} \mathcal{D} \mathcal{H}\right) E^{ij} \Lambda_{\alpha i} \Lambda_{\beta j} \Lambda^{\dot{\alpha} k} \Lambda^{\dot{\beta} l} \Lambda_{\gamma k} \Lambda_{\delta l} \epsilon^{\alpha \gamma} \epsilon^{\beta \delta} \epsilon_{\dot{\alpha} \dot{\beta}} \\
& + \left(-\frac{1}{18} \mathcal{D}^\dagger \mathcal{I} + \frac{5}{144} \mathcal{D} \mathcal{H}\right) E^{ij} \Lambda_{\alpha i} \Lambda_{\beta j} \Lambda^{\dot{\alpha} k} \Lambda^{\dot{\beta} l} \Lambda_{\gamma k} \Lambda_{\delta l} \epsilon^{\alpha \beta} \epsilon_{\dot{\alpha} \dot{\beta}} \epsilon^{\gamma \delta} + \left(-\frac{3}{64} \mathcal{D} \mathcal{D} \mathcal{H} - \frac{3}{8} \mathcal{I}\right) T_{ab}{}^{ij} \Lambda_{\alpha i} \Lambda_{\beta j} \Lambda^{\dot{\alpha} k} \Lambda^{\dot{\beta} l} \Lambda_{\gamma k} \Lambda_{\delta l} \epsilon_{\dot{\alpha} \dot{\beta}} \epsilon^{\gamma \delta} \gamma_{ab}{}^{\alpha \beta} \\
& + \left(\frac{1}{96} \mathcal{D} \mathcal{D} \mathcal{D} \mathcal{H} + \frac{1}{8} \mathcal{D} \mathcal{I}\right) \Lambda_{\alpha i} \Lambda_{\beta j} \Lambda^{\dot{\alpha} i} \Lambda_{\gamma k} \Lambda_{\delta l} \epsilon^{\alpha \beta} \epsilon^{\gamma \epsilon} \gamma_a{}^{\delta}{}_{\dot{\alpha}} \nabla_a \Lambda_{\epsilon m} \varepsilon^{jklm} + \left(\frac{5}{144} \mathcal{D}^\dagger \bar{\mathcal{H}} - \frac{1}{18} \mathcal{D} \bar{\mathcal{L}}\right) E_{ij} \Lambda_{\alpha k} \Lambda_{\beta l} \Lambda^{\dot{\alpha} i} \Lambda^{\dot{\beta} j} \Lambda^{\dot{\gamma} k} \Lambda^{\dot{\delta} l} \epsilon^{\alpha \beta} \epsilon_{\dot{\alpha} \dot{\beta}} \epsilon_{\dot{\gamma} \dot{\delta}} \\
& + \left(\frac{5}{144} \mathcal{D}^\dagger \bar{\mathcal{H}} - \frac{1}{18} \mathcal{D} \bar{\mathcal{L}}\right) E_{ij} \Lambda_{\alpha k} \Lambda_{\beta l} \Lambda^{\dot{\alpha} i} \Lambda^{\dot{\beta} j} \Lambda^{\dot{\gamma} k} \Lambda^{\dot{\delta} l} \epsilon^{\alpha \beta} \epsilon_{\dot{\alpha} \dot{\gamma}} \epsilon_{\dot{\beta} \dot{\delta}} + \left(\frac{3}{32} \mathcal{D} \mathcal{D} \mathcal{H} + \frac{3}{4} \mathcal{I}\right) T_{ab}{}^{ij} \Lambda_{\alpha i} \Lambda_{\beta j} \Lambda^{\dot{\alpha} k} \Lambda^{\dot{\beta} l} \Lambda_{\gamma k} \Lambda_{\delta l} \epsilon^{\alpha \gamma} \epsilon_{\dot{\alpha} \dot{\beta}} \gamma_{ab}{}^{\beta \delta} \\
& + \left(\frac{1}{8} \mathcal{D}^\dagger \bar{\mathcal{L}} + \frac{1}{96} \mathcal{D}^\dagger \mathcal{D}^\dagger \mathcal{D}^\dagger \bar{\mathcal{H}}\right) \Lambda_{\alpha i} \Lambda^{\dot{\alpha} i} \Lambda^{\dot{\beta} j} \Lambda^{\dot{\gamma} k} \Lambda^{\dot{\delta} l} \epsilon_{\dot{\alpha} \dot{\beta}} \epsilon_{\dot{\gamma} \dot{\epsilon}} \gamma_a{}^{\alpha}{}_{\dot{\delta}} \nabla_a \Lambda^{\dot{\epsilon} m} \varepsilon_{jklm} + \left(\frac{3}{4} \bar{\mathcal{L}} + \frac{3}{32} \mathcal{D}^\dagger \mathcal{D}^\dagger \bar{\mathcal{H}}\right) T_{abij} \Lambda_{\alpha k} \Lambda_{\beta l} \Lambda^{\dot{\alpha} i} \Lambda^{\dot{\beta} j} \Lambda^{\dot{\gamma} k} \Lambda^{\dot{\delta} l} \epsilon^{\alpha \beta}$$
$$\begin{aligned}
F_8 = & \left(-\frac{1}{16} \bar{\mathcal{H}} - \frac{1}{16} \mathcal{H}\right) \Lambda_{\alpha i} \Lambda_{\beta j} \Lambda^{\alpha i} \Lambda^{\beta j} \Lambda^{\gamma k} \Lambda_{\gamma k} \Lambda^{\delta l} \Lambda_{\delta l} \epsilon^{\alpha \beta} \epsilon_{\alpha \beta \epsilon \gamma \delta} \epsilon^{\gamma \delta} + \left(-\frac{1}{16} \bar{\mathcal{H}} - \frac{1}{16} \mathcal{H}\right) \Lambda_{\alpha i} \Lambda_{\beta j} \Lambda^{\dot{\alpha} i} \Lambda^{\dot{\beta} j} \Lambda^{\dot{\gamma} k} \Lambda_{\gamma k} \Lambda^{\dot{\delta} l} \Lambda_{\delta l} \epsilon^{\alpha \beta} \epsilon_{\dot{\alpha} \dot{\beta} \dot{\gamma} \dot{\delta}} \epsilon^{\gamma \delta} \\
& + \frac{1}{46080} \mathcal{D}^\dagger \mathcal{D}^\dagger \mathcal{D}^\dagger \mathcal{D}^\dagger \mathcal{D}^\dagger \mathcal{D}^\dagger \bar{\mathcal{H}} \quad \Lambda^{\alpha i} \Lambda^{\beta j} \Lambda^{\gamma k} \Lambda^{\delta l} \Lambda^{\dot{\epsilon} m} \Lambda^{\sigma 1 n} \Lambda^{\sigma 2 p} \Lambda^{\sigma 3 q} \epsilon_{\alpha \beta} \epsilon_{\gamma \delta} \epsilon_{\epsilon \sigma 1} \epsilon_{\sigma 2 \sigma 3} \epsilon_{i k m p} \epsilon_{j l n q} \\
& + \frac{1}{46080} \mathcal{D} \mathcal{D} \mathcal{D} \mathcal{D} \mathcal{D} \mathcal{D} \mathcal{H} \quad \Lambda_{\alpha i} \Lambda_{\beta j} \Lambda_{\gamma k} \Lambda_{\delta l} \Lambda_{\epsilon m} \Lambda_{\epsilon 1 n} \Lambda_{\epsilon 2 p} \Lambda_{\epsilon 3 q} \epsilon^{\alpha \beta} \epsilon^{\gamma \delta} \epsilon^{\epsilon \epsilon 1} \epsilon^{\epsilon 2 \epsilon 3} \epsilon_{i k m p} \epsilon_{j l n q},
\end{aligned}$$

## The $\Omega$ blocks

We combine  $\Omega_\alpha^i$  and  $\Omega_a^{\dot{\alpha}i}$  into a single spinor-vector  $\hat{\Omega}_a^{\dot{\alpha}i} = \gamma_a^{\dot{\alpha}\alpha} \Omega_\alpha^i + \Omega_a^{\dot{\alpha}i}$ . The one-fermion terms are:

$$\begin{aligned}
[\hat{\Omega}_a^{\dot{\alpha}i}]_1 = & \left( -\frac{1}{8} \mathcal{D}^\dagger \bar{\mathcal{H}} - \frac{1}{4} \mathcal{D} \bar{\mathcal{L}} \right) \nabla_b \nabla_b \nabla_a \Lambda^{\dot{\alpha}i} - \frac{1}{4} E^{ij} \mathcal{D} \bar{\mathcal{L}} \nabla_b R(Q)_{ab}{}^{\dot{\alpha}}{}_j + \frac{1}{2} P_b \mathcal{D} \bar{\mathcal{L}} R(S)^+{}_{ab}{}^{\dot{\alpha}i} + \frac{1}{2} \bar{\mathcal{L}} P_a \nabla_b \nabla_b \Lambda^{\dot{\alpha}i} + \bar{\mathcal{L}} P_b \nabla_a \nabla_b \Lambda^{\dot{\alpha}i} \\
& + \frac{1}{2} \bar{\mathcal{L}} \Lambda^{\dot{\alpha}i} \nabla_a \nabla_b P_b + \bar{\mathcal{L}} \nabla_b P_a \nabla_b \Lambda^{\dot{\alpha}i} + \frac{1}{2} \bar{\mathcal{L}} \nabla_b P_b \nabla_a \Lambda^{\dot{\alpha}i} + \frac{1}{2} \bar{\mathcal{H}} T_{ab}{}^{jk} \nabla_b \chi^{\dot{\alpha}}{}_{jk}{}^i - \frac{1}{12} \mathcal{D}^\dagger \bar{\mathcal{H}} \Lambda^{\dot{\alpha}j} \nabla_b R(V)_{ab}{}^i{}_j - \frac{1}{4} \mathcal{D} \bar{\mathcal{L}} R(Q)_{ab}{}^{\dot{\alpha}}{}_j \nabla_b E^{ij} \\
& + \left( -\frac{1}{3} \bar{\mathcal{H}} + \frac{1}{3} \mathcal{H} \right) T_{bc}{}^{ij} \nabla_b R(Q)_{ac}{}^{\dot{\alpha}}{}_j + \left( -\frac{1}{3} \bar{\mathcal{H}} + \frac{1}{3} \mathcal{H} \right) R(Q)_{ab}{}^{\dot{\alpha}}{}_j \nabla_c T_{bc}{}^{ij} + \left( -\frac{1}{4} \bar{\mathcal{H}} + \frac{1}{4} \mathcal{H} \right) \gamma_b{}^{\dot{\alpha}\alpha} \nabla_c \nabla_b R(Q)_{ac\alpha}{}^i \\
& + \left( -\frac{1}{8} \mathcal{D}^\dagger \bar{\mathcal{H}} - \frac{1}{4} \mathcal{D} \bar{\mathcal{L}} \right) \gamma_{ab}{}^{\dot{\alpha}}{}_{\dot{\beta}} \nabla_c \nabla_c \nabla_b \Lambda^{\dot{\beta}i} + \left( -\frac{5}{48} \bar{\mathcal{H}} + \frac{5}{48} \mathcal{H} \right) \nabla_a \Lambda^{\dot{\alpha}i} \nabla_b \bar{P}_b + \left( -\frac{1}{24} \bar{\mathcal{H}} + \frac{1}{24} \mathcal{H} \right) \bar{P}_b \nabla_a \nabla_b \Lambda^{\dot{\alpha}i} + \left( \frac{1}{48} \bar{\mathcal{H}} - \frac{1}{48} \mathcal{H} \right) \nabla_b \Lambda^{\dot{\alpha}i} \nabla_a \bar{P}_b \\
& + \left( \frac{1}{48} \bar{\mathcal{H}} - \frac{1}{48} \mathcal{H} \right) \nabla_b \Lambda^{\dot{\alpha}i} \nabla_b \bar{P}_a + \left( \frac{1}{16} \bar{\mathcal{H}} - \frac{1}{16} \mathcal{H} \right) \Lambda^{\dot{\alpha}i} \nabla_a \nabla_b \bar{P}_b + \left( \frac{5}{48} \bar{\mathcal{H}} - \frac{5}{48} \mathcal{H} \right) \bar{P}_a \nabla_b \nabla_b \Lambda^{\dot{\alpha}i} + \left( \frac{1}{8} \mathcal{D}^\dagger \bar{\mathcal{H}} + \frac{5}{12} \mathcal{D} \bar{\mathcal{L}} \right) R(V)_{ab}{}^i{}_j \nabla_b \Lambda^{\dot{\alpha}j} \\
& + \left( \frac{3}{8} \bar{\mathcal{H}} - \frac{3}{8} \mathcal{H} \right) \chi^{\dot{\alpha}}{}_{jk}{}^i \nabla_b T_{ab}{}^{jk} + \frac{1}{32} E^{ij} \mathcal{D} \bar{\mathcal{L}} \Lambda^{\dot{\alpha}k} \nabla_a E_{jk} + P_b T_{bc}{}^{ij} \mathcal{D} \bar{\mathcal{L}} R(Q)_{ac}{}^{\dot{\alpha}}{}_j + \frac{5}{24} P_b \mathcal{D} \bar{\mathcal{L}} \Lambda^{\dot{\alpha}i} \nabla_a \bar{P}_b + \frac{1}{4} T_{abjk} \mathcal{D} \bar{\mathcal{L}} \nabla_c R(Q)_{bc}{}^{\dot{\alpha}}{}_l \varepsilon^{ijkl} \\
& + \frac{1}{4} T_{bcjk} \mathcal{D} \bar{\mathcal{L}} \nabla_b R(Q)_{ac}{}^{\dot{\alpha}}{}_l \varepsilon^{ijkl} + \frac{3}{4} T_{ab}{}^{jk} \mathcal{D}^\dagger \bar{\mathcal{L}} \bar{P}_b \chi^{\dot{\alpha}}{}_{jk}{}^i + \frac{1}{6} T_{ab}{}^{ij} \mathcal{D}^\dagger \bar{\mathcal{L}} \gamma_b{}^{\dot{\alpha}\alpha} \nabla_c \nabla_c \Lambda_{\alpha j} - \frac{1}{2} T_{ab}{}^{ij} \mathcal{D}^\dagger \bar{\mathcal{L}} \gamma_c{}^{\dot{\alpha}\alpha} \nabla_b \nabla_c \Lambda_{\alpha j} \\
& + \frac{1}{6} T_{bc}{}^{ij} \mathcal{D}^\dagger \bar{\mathcal{L}} \gamma_b{}^{\dot{\alpha}\alpha} \nabla_a \nabla_c \Lambda_{\alpha j} + \frac{1}{2} \bar{\mathcal{L}} P_b \gamma_{ab}{}^{\dot{\alpha}}{}_{\dot{\beta}} \nabla_c \nabla_c \Lambda^{\dot{\beta}i} + \bar{\mathcal{L}} P_b \gamma_{ac}{}^{\dot{\alpha}}{}_{\dot{\beta}} \nabla_b \nabla_c \Lambda^{\dot{\beta}i} + \frac{1}{2} \bar{\mathcal{L}} \Lambda^{\dot{\beta}i} \gamma_{ab}{}^{\dot{\alpha}}{}_{\dot{\beta}} \nabla_b \nabla_c P_c + \bar{\mathcal{L}} \gamma_{ab}{}^{\dot{\alpha}}{}_{\dot{\beta}} \nabla_c P_b \nabla_c \Lambda^{\dot{\beta}i} \\
& + \frac{1}{2} \bar{\mathcal{L}} \gamma_{ab}{}^{\dot{\alpha}}{}_{\dot{\beta}} \nabla_c P_c \nabla_b \Lambda^{\dot{\beta}i} + \mathcal{D}^\dagger \bar{\mathcal{L}} P_a P_b \nabla_b \Lambda^{\dot{\alpha}i} + \frac{1}{2} \mathcal{D}^\dagger \bar{\mathcal{L}} P_b P_b \nabla_a \Lambda^{\dot{\alpha}i} + \frac{1}{2} \mathcal{D}^\dagger \bar{\mathcal{L}} P_a \Lambda^{\dot{\alpha}i} \nabla_b P_b + \mathcal{D}^\dagger \bar{\mathcal{L}} P_b \Lambda^{\dot{\alpha}i} \nabla_b P_a - \frac{1}{32} \mathcal{D}^\dagger \bar{\mathcal{H}} E_{jk} \Lambda^{\dot{\alpha}i} \nabla_a E^{jk} \\
& + \frac{1}{2} \mathcal{D}^\dagger \bar{\mathcal{H}} P_b T_{ab}{}^{jk} \chi^{\dot{\alpha}}{}_{jk}{}^i + \frac{1}{12} \mathcal{D}^\dagger \mathcal{D}^\dagger \bar{\mathcal{H}} E^{ij} T_{abjk} \nabla_b \Lambda^{\dot{\alpha}k} + \frac{1}{8} \mathcal{D}^\dagger \bar{\mathcal{L}} \Lambda^{\dot{\alpha}i} \bar{P}_a \nabla_b \bar{P}_b + \frac{7}{24} \mathcal{D}^\dagger \bar{\mathcal{L}} \Lambda^{\dot{\alpha}i} \bar{P}_b \nabla_a \bar{P}_b - \frac{1}{24} \mathcal{D}^\dagger \bar{\mathcal{L}} \Lambda^{\dot{\alpha}i} \bar{P}_b \nabla_b \bar{P}_a \\
& - \frac{1}{4} \mathcal{D}^\dagger \bar{\mathcal{L}} R(Q)_{ab\alpha}{}^i \gamma_c{}^{\dot{\alpha}\alpha} \nabla_b \bar{P}_c - \frac{1}{4} \mathcal{D}^\dagger \bar{\mathcal{L}} R(Q)_{ab\alpha}{}^i \gamma_c{}^{\dot{\alpha}\alpha} \nabla_c \bar{P}_b + \frac{1}{4} \mathcal{D}^\dagger \bar{\mathcal{L}} R(Q)_{bca}{}^i \gamma_a{}^{\dot{\alpha}\alpha} \nabla_b \bar{P}_c + \frac{1}{12} \mathcal{D}^\dagger \bar{\mathcal{L}} \bar{P}_a \bar{P}_b \nabla_b \Lambda^{\dot{\alpha}i} \\
& - \frac{5}{24} \mathcal{D}^\dagger \bar{\mathcal{L}} \bar{P}_b \bar{P}_b \nabla_a \Lambda^{\dot{\alpha}i} - \frac{1}{2} \mathcal{D}^\dagger \bar{\mathcal{L}} \bar{P}_b \gamma_b{}^{\dot{\alpha}\alpha} \nabla_c R(Q)_{ac\alpha}{}^i - \frac{1}{2} \mathcal{D}^\dagger \bar{\mathcal{L}} \bar{P}_b \gamma_c{}^{\dot{\alpha}\alpha} \nabla_c R(Q)_{ab\alpha}{}^i + \frac{1}{6} \mathcal{D}^\dagger \bar{\mathcal{L}} \gamma_b{}^{\dot{\alpha}\alpha} \nabla_a T_{bc}{}^{ij} \nabla_c \Lambda_{\alpha j} \\
& - \frac{1}{2} \mathcal{D}^\dagger \bar{\mathcal{L}} \gamma_b{}^{\dot{\alpha}\alpha} \nabla_b T_{ac}{}^{ij} \nabla_c \Lambda_{\alpha j} + \frac{1}{3} \mathcal{D}^\dagger \bar{\mathcal{L}} \gamma_b{}^{\dot{\alpha}\alpha} \nabla_c T_{ab}{}^{ij} \nabla_c \Lambda_{\alpha j} - \frac{1}{2} \mathcal{D}^\dagger \bar{\mathcal{L}} \gamma_b{}^{\dot{\alpha}\alpha} \nabla_c T_{ac}{}^{ij} \nabla_b \Lambda_{\alpha j} + \frac{1}{6} \mathcal{D}^\dagger \bar{\mathcal{L}} \gamma_b{}^{\dot{\alpha}\alpha} \nabla_c T_{bc}{}^{ij} \nabla_a \Lambda_{\alpha j} \\
& + \frac{1}{8} \mathcal{D} \bar{\mathcal{L}} \Lambda^{\dot{\beta}i} R(K)_{bca} \gamma_{bc}{}^{\dot{\alpha}}{}_{\dot{\beta}} - \frac{1}{8} \mathcal{D} \bar{\mathcal{L}} R(M)_{abcd} \gamma_{cd}{}^{\dot{\alpha}}{}_{\dot{\beta}} \nabla_b \Lambda^{\dot{\beta}i} - \frac{1}{4} \mathcal{D} \bar{\mathcal{L}} R(Q)_{ab}{}^{\dot{\alpha}}{}_j \nabla_c T_{bckl} \varepsilon^{ijkl} - \frac{1}{4} \mathcal{D} \bar{\mathcal{L}} R(Q)_{bc}{}^{\dot{\alpha}}{}_j \nabla_b T_{ackl} \varepsilon^{ijkl} \\
& + \frac{1}{2} \mathcal{H} R(M)_{abcd} R(Q)_{cd\alpha}{}^i \gamma_b{}^{\dot{\alpha}\alpha} + \left( -\mathcal{D}^\dagger \bar{\mathcal{H}} - \frac{3}{2} \mathcal{D} \bar{\mathcal{L}} \right) T_{bcjk} \Lambda^{\dot{\alpha}j} \nabla_b T_{ac}{}^{ik} + \left( -\frac{2}{3} \mathcal{D}^\dagger \bar{\mathcal{H}} - \frac{5}{6} \mathcal{D} \bar{\mathcal{L}} \right) T_{bcjk} T_{ab}{}^{jk} \nabla_c \Lambda^{\dot{\alpha}i} \\
& + \left( -\frac{1}{2} \mathcal{D}^\dagger \bar{\mathcal{L}} - \frac{1}{3} \mathcal{D} \mathcal{H} \right) \Lambda_{\alpha j} \gamma_b{}^{\dot{\alpha}\alpha} \nabla_a \nabla_c T_{bc}{}^{ij} + \left( -\frac{1}{3} \bar{\mathcal{L}} + \frac{1}{12} \mathcal{D}^\dagger \mathcal{D}^\dagger \bar{\mathcal{H}} \right) E^{ij} \Lambda^{\dot{\alpha}k} \nabla_b T_{abjk} + \left( -\frac{1}{3} \mathcal{D}^\dagger \bar{\mathcal{H}} - \mathcal{D} \bar{\mathcal{L}} \right) T_{bcjk} T_{ab}{}^{ij} \nabla_c \Lambda^{\dot{\alpha}k} \\
& + \left( -\frac{1}{6} \mathcal{D}^\dagger \bar{\mathcal{H}} - \frac{1}{5} \mathcal{D} \bar{\mathcal{L}} \right) T_{bc}{}^{ij} \Lambda^{\dot{\alpha}k} \nabla_b T_{acjk} + \left( -\frac{1}{6} \mathcal{D}^\dagger \bar{\mathcal{L}} - \frac{1}{6} \mathcal{D} \mathcal{H} \right) \Lambda_{\alpha j} \gamma_b{}^{\dot{\alpha}\alpha} \nabla_c \nabla_c T_{ab}{}^{ij} + \left( -\frac{7}{48} \bar{\mathcal{H}} - \frac{3}{16} \mathcal{H} \right) \Lambda^{\dot{\alpha}j} R(V)_{ab}{}^i{}_j \bar{P}_b \\
& + \left( -\frac{1}{8} \bar{\mathcal{H}} - \frac{3}{8} \mathcal{H} \right) R(V)_{ab}{}^j{}_k \chi^{\dot{\alpha}}{}_{jk}{}^i \gamma_b{}^{\dot{\alpha}\alpha} + \left( -\frac{1}{8} \bar{\mathcal{H}} + \frac{1}{24} \mathcal{H} \right) E_{jk} T_{ab}{}^{ij} \nabla_b \Lambda^{\dot{\alpha}k} + \left( -\frac{1}{8} \mathcal{D}^\dagger \bar{\mathcal{H}} - \frac{1}{4} \mathcal{D} \bar{\mathcal{L}} \right) T_{bcjk} \nabla_a R(Q)_{bc}{}^{\dot{\alpha}}{}_l \varepsilon^{ijkl} \\
& + \left( -\frac{1}{8} \mathcal{D}^\dagger \bar{\mathcal{H}} - \frac{1}{6} \mathcal{D} \bar{\mathcal{L}} \right) R(V)_{ab}{}^i{}_j \gamma_{bc}{}^{\dot{\alpha}}{}_{\dot{\beta}} \nabla_c \Lambda^{\dot{\beta}j} + \left( -\frac{1}{12} \mathcal{D}^\dagger \bar{\mathcal{H}} - \frac{1}{24} \mathcal{D} \bar{\mathcal{L}} \right) \Lambda^{\dot{\alpha}i} \bar{P}_b \nabla_a P_b + \left( -\frac{1}{16} \bar{\mathcal{H}} - \frac{3}{16} \mathcal{H} \right) D^{ij}{}_{kl} \chi_{\alpha}{}^{kl}{}_j \gamma_a{}^{\dot{\alpha}\alpha} \\
& + \left( -\frac{1}{16} \bar{\mathcal{H}} + \frac{1}{16} \mathcal{H} \right) E^{ij} R(Q)_{ab}{}^{\dot{\alpha}}{}_j \bar{P}_b + \left( -\frac{1}{16} \bar{\mathcal{H}} + \frac{1}{16} \mathcal{H} \right) \chi^{\dot{\beta}}{}_{jk}{}^i \gamma_{ab}{}^{\dot{\alpha}}{}_{\dot{\beta}} \nabla_c T_{bc}{}^{jk} + \left( -\frac{1}{16} \bar{\mathcal{H}} + \frac{1}{16} \mathcal{H} \right) \gamma_{ab}{}^{\dot{\alpha}}{}_{\dot{\beta}} \nabla_c \Lambda^{\dot{\beta}i} \nabla_b \bar{P}_c \\
& + \left( -\frac{1}{16} \mathcal{D}^\dagger \bar{\mathcal{H}} - \frac{1}{8} \mathcal{D} \bar{\mathcal{L}} \right) P_b \gamma_a{}^{\dot{\alpha}\alpha} \nabla_c R(Q)_{bca}{}^i + \left( -\frac{1}{16} \mathcal{D}^\dagger \bar{\mathcal{H}} - \frac{1}{8} \mathcal{D} \bar{\mathcal{L}} \right) P_b \gamma_c{}^{\dot{\alpha}\alpha} \nabla_c R(Q)_{aba}{}^i + \left( -\frac{1}{16} \mathcal{D}^\dagger \bar{\mathcal{H}} - \frac{1}{8} \mathcal{D} \bar{\mathcal{L}} \right) R(V)_{bc}{}^i{}_j \gamma_{bc}{}^{\dot{\alpha}}{}_{\dot{\beta}} \nabla_a \Lambda^{\dot{\beta}j} \\
& + \left( -\frac{5}{96} \bar{\mathcal{H}} + \frac{5}{96} \mathcal{H} \right) \gamma_b{}^{\dot{\alpha}\alpha} \nabla_a E^{ij} \nabla_b \Lambda_{\alpha j} + \left( -\frac{1}{32} \bar{\mathcal{H}} + \frac{1}{32} \mathcal{H} \right) \chi^{\dot{\alpha}}{}_{jk}{}^l \nabla_a E_{lm} \varepsilon^{ijkm} + \left( -\frac{1}{48} \bar{\mathcal{H}} - \frac{11}{48} \mathcal{H} \right) T_{ab}{}^{ij} R(S)^-{}_{bcaj} \gamma_c{}^{\dot{\alpha}\alpha} \\
& + \left( -\frac{1}{48} \bar{\mathcal{H}} + \frac{1}{48} \mathcal{H} \right) \Lambda_{\alpha j} \gamma_b{}^{\dot{\alpha}\alpha} \nabla_a \nabla_b E^{ij} + \left( -\frac{1}{48} \bar{\mathcal{H}} + \frac{1}{48} \mathcal{H} \right) \Lambda^{\dot{\beta}i} \gamma_{ab}{}^{\dot{\alpha}}{}_{\dot{\beta}} \nabla_b \nabla_c \bar{P}_c + \left( -\frac{1}{48} \bar{\mathcal{H}} + \frac{1}{48} \mathcal{H} \right) \bar{P}_b \gamma_{ab}{}^{\dot{\alpha}}{}_{\dot{\beta}} \nabla_c \nabla_c \Lambda^{\dot{\beta}i} \\
& + \left( -\frac{1}{48} \mathcal{D}^\dagger \bar{\mathcal{H}} - \frac{3}{8} \mathcal{D} \bar{\mathcal{L}} \right) P_b \bar{P}_a \nabla_b \Lambda^{\dot{\alpha}i} + \left( -\frac{1}{48} \mathcal{D}^\dagger \bar{\mathcal{H}} + \frac{1}{48} \mathcal{D} \bar{\mathcal{L}} \right) E_{jk} E^{jk} \nabla_a \Lambda^{\dot{\alpha}i} + \left( -\frac{1}{48} \mathcal{D}^\dagger \bar{\mathcal{H}} + \frac{3}{40} \mathcal{D} \bar{\mathcal{L}} \right) T_{ab}{}^{jk} \Lambda^{\dot{\alpha}i} \nabla_c T_{bcjk} \\
& + \left( -\frac{1}{96} \bar{\mathcal{H}} - \frac{11}{96} \mathcal{H} \right) T_{bc}{}^{ij} R(S)^-{}_{bcaj} \gamma_a{}^{\dot{\alpha}\alpha} + \left( -\frac{1}{96} \bar{\mathcal{H}} + \frac{1}{96} \mathcal{H} \right) E^{ij} \gamma_a{}^{\dot{\alpha}\alpha} \nabla_b \nabla_b \Lambda_{\alpha j} + \left( -\frac{1}{120} \mathcal{D}^\dagger \bar{\mathcal{H}} + \frac{1}{240} \mathcal{D} \bar{\mathcal{L}} \right) \Lambda^{\dot{\beta}j} \gamma_{bc}{}^{\dot{\alpha}}{}_{\dot{\beta}} \nabla_b R(V)_{ac}{}^i{}_j \\
& + \left( \frac{1}{240} \mathcal{D}^\dagger \bar{\mathcal{H}} - \frac{7}{160} \mathcal{D} \bar{\mathcal{L}} \right) \Lambda^{\dot{\beta}j} \gamma_{bc}{}^{\dot{\alpha}}{}_{\dot{\beta}} \nabla_a R(V)_{bc}{}^i{}_j + \left( \frac{1}{96} \bar{\mathcal{H}} - \frac{1}{96} \mathcal{H} \right) \gamma_a{}^{\dot{\alpha}\alpha} \nabla_b E^{ij} \nabla_b \Lambda_{\alpha j} + \left( \frac{1}{96} \bar{\mathcal{H}} - \frac{1}{96} \mathcal{H} \right) \gamma_b{}^{\dot{\alpha}\alpha} \nabla_b E^{ij} \nabla_a \Lambda_{\alpha j} + 1 \dots
\end{aligned}$$



$$\begin{aligned}
[\hat{\Omega}_a^{\dot{\alpha}i}]_{1,cont.} = & + \left(\frac{1}{96} \mathcal{D}^\dagger \bar{\mathcal{H}} - \frac{1}{96} \mathcal{D} \bar{\mathcal{L}}\right) E^{jk} \Lambda^{\dot{\alpha}i} \nabla_a E_{jk} + \left(\frac{1}{48} \bar{\mathcal{H}} - \frac{1}{48} \mathcal{H}\right) \gamma_{ab}^{\dot{\alpha}} \dot{\beta} \nabla_c \Lambda^{\dot{\beta}i} \nabla_c \bar{P}_b + \left(\frac{1}{32} \mathcal{D}^\dagger \bar{\mathcal{H}} + \frac{1}{16} \mathcal{D} \bar{\mathcal{L}}\right) \Lambda^{\dot{\beta}i} \gamma_{bc}^{\dot{\alpha}} \dot{\beta} \nabla_d R(M)_{adbc} \\
& + \left(\frac{1}{24} \bar{\mathcal{H}} - \frac{13}{24} \mathcal{H}\right) R(Q)_{bca}{}^j R(V)_{bc}{}^i{}_{j\gamma a}{}^{\dot{\alpha}\alpha} + \left(\frac{1}{24} \bar{\mathcal{H}} - \frac{1}{24} \mathcal{H}\right) E^{ij} \gamma_b^{\dot{\alpha}\alpha} \nabla_a \nabla_b \Lambda_{\alpha j} + \left(\frac{1}{24} \bar{\mathcal{H}} - \frac{1}{24} \mathcal{H}\right) \bar{P}_b \gamma_{bc}^{\dot{\alpha}} \dot{\beta} \nabla_a \nabla_c \Lambda^{\dot{\beta}i} \\
& + \left(\frac{1}{24} \mathcal{D}^\dagger \bar{\mathcal{H}} - \frac{1}{8} \mathcal{D} \bar{\mathcal{L}}\right) P_b \Lambda^{\dot{\alpha}i} \nabla_b \bar{P}_a + \left(\frac{1}{24} \mathcal{D}^\dagger \bar{\mathcal{H}} + \frac{5}{24} \mathcal{D} \bar{\mathcal{L}}\right) P_a \Lambda^{\dot{\alpha}i} \nabla_b \bar{P}_b + \left(\frac{1}{16} \bar{\mathcal{H}} - \frac{1}{16} \mathcal{H}\right) \chi^{\dot{\beta}}{}_{jk}{}^i \gamma_{bc}^{\dot{\alpha}} \dot{\beta} \nabla_b T_{ac}{}^{jk} \\
& + \left(\frac{1}{16} \bar{\mathcal{H}} - \frac{1}{16} \mathcal{H}\right) \gamma_{ab}^{\dot{\alpha}} \dot{\beta} \nabla_b \Lambda^{\dot{\beta}i} \nabla_c \bar{P}_c + \left(\frac{1}{16} \bar{\mathcal{H}} + \frac{1}{16} \mathcal{H}\right) E_{jk} \nabla_a \chi^{\dot{\alpha}}{}_{lm}{}^j \varepsilon^{iklm} + \left(\frac{1}{16} \bar{\mathcal{H}} + \frac{13}{48} \mathcal{H}\right) T_{ab}{}^{ij} \Lambda^{\dot{\alpha}k} \nabla_b E_{jk} \\
& + \left(\frac{1}{16} \bar{\mathcal{H}} + \frac{11}{16} \mathcal{H}\right) T_{bc}{}^{ij} R(S)^-{}_{ab\alpha j} \gamma_c^{\dot{\alpha}\alpha} + \left(\frac{1}{16} \mathcal{D}^\dagger \bar{\mathcal{H}} + \frac{1}{8} \mathcal{D} \bar{\mathcal{L}}\right) P_b \gamma_b^{\dot{\alpha}\alpha} \nabla_c R(Q)_{aca}{}^i + \left(\frac{1}{16} \mathcal{D}^\dagger \bar{\mathcal{H}} + \frac{1}{8} \mathcal{D} \bar{\mathcal{L}}\right) \Lambda^{\dot{\beta}i} \gamma_{bc}^{\dot{\alpha}} \dot{\beta} \nabla_d R(M)_{abcd} \\
& + \left(\frac{1}{16} \mathcal{D}^\dagger \bar{\mathcal{H}} + \frac{5}{24} \mathcal{D} \bar{\mathcal{L}}\right) R(V)_{bc}{}^i{}_{j\gamma d} \Lambda^{\dot{\alpha}j} \varepsilon_{abcd} + \left(\frac{1}{12} \bar{\mathcal{H}} - \frac{1}{12} \mathcal{H}\right) \gamma_{bc}^{\dot{\alpha}} \dot{\beta} \nabla_a \Lambda^{\dot{\beta}i} \nabla_b \bar{P}_c + \left(\frac{1}{12} \bar{\mathcal{H}} - \frac{1}{12} \mathcal{H}\right) \gamma_{bc}^{\dot{\alpha}} \dot{\beta} \nabla_b \Lambda^{\dot{\beta}i} \nabla_a \bar{P}_c \\
& + \left(\frac{1}{12} \mathcal{D}^\dagger \bar{\mathcal{H}} + \frac{1}{12} \mathcal{D} \bar{\mathcal{L}}\right) \Lambda^{\dot{\beta}j} \gamma_{ab}^{\dot{\alpha}} \dot{\beta} \nabla_c R(V)_{bc}{}^i{}_{j\gamma} + \left(\frac{1}{12} \mathcal{D}^\dagger \bar{\mathcal{H}} + \frac{5}{48} \mathcal{D} \bar{\mathcal{L}}\right) E_{jk} E^{ij} \nabla_a \Lambda^{\dot{\alpha}k} + \left(\frac{1}{12} \mathcal{D}^\dagger \bar{\mathcal{H}} + \frac{5}{48} \mathcal{D} \bar{\mathcal{L}}\right) E_{jk} \Lambda^{\dot{\alpha}j} \nabla_a E^{ik} \\
& + \left(\frac{11}{96} \bar{\mathcal{H}} + \frac{1}{96} \mathcal{H}\right) \Lambda_{\alpha j} \gamma_a^{\dot{\alpha}\alpha} \nabla_b \nabla_b E^{ij} + \left(\frac{1}{8} \bar{\mathcal{H}} + \frac{1}{8} \mathcal{H}\right) T_{ab}{}^{jk} \gamma_{bc}^{\dot{\alpha}} \dot{\beta} \nabla_c \chi^{\dot{\beta}}{}_{jk}{}^i + \left(\frac{1}{8} \bar{\mathcal{H}} + \frac{1}{8} \mathcal{H}\right) T_{bc}{}^{jk} \gamma_{ab}^{\dot{\alpha}} \dot{\beta} \nabla_c \chi^{\dot{\beta}}{}_{jk}{}^i \\
& + \left(\frac{1}{8} \bar{\mathcal{H}} + \frac{7}{24} \mathcal{H}\right) E_{jk} \Lambda^{\dot{\alpha}j} \nabla_b T_{ab}{}^{ik} + \left(\frac{1}{8} \mathcal{D}^\dagger \bar{\mathcal{H}} + \frac{1}{8} \mathcal{D} \bar{\mathcal{L}}\right) \Lambda^{\dot{\alpha}i} \bar{P}_a \nabla_b P_b + \left(\frac{1}{8} \mathcal{D}^\dagger \bar{\mathcal{H}} + \frac{1}{6} \mathcal{D} \bar{\mathcal{L}}\right) R(V)_{bc}{}^i{}_{j\gamma ab}^{\dot{\alpha}} \dot{\beta} \nabla_c \Lambda^{\dot{\beta}j} \\
& + \left(\frac{7}{48} \mathcal{D}^\dagger \bar{\mathcal{H}} - \frac{11}{120} \mathcal{D} \bar{\mathcal{L}}\right) T_{bc}{}^{jk} \Lambda^{\dot{\alpha}i} \nabla_b T_{acjk} + \left(\frac{1}{6} \mathcal{D}^\dagger \bar{\mathcal{H}} + \frac{2}{15} \mathcal{D} \bar{\mathcal{L}}\right) T_{ab}{}^{ij} \Lambda^{\dot{\alpha}k} \nabla_c T_{bcjk} + \left(\frac{1}{6} \mathcal{D}^\dagger \bar{\mathcal{H}} + \frac{5}{12} \mathcal{D} \bar{\mathcal{L}}\right) P_b \bar{P}_b \nabla_a \Lambda^{\dot{\alpha}i} \\
& + \left(\frac{1}{6} \mathcal{D}^\dagger \bar{\mathcal{H}} + \frac{7}{12} \mathcal{D} \bar{\mathcal{L}}\right) T_{bcjk} \Lambda^{\dot{\alpha}i} \nabla_b T_{ac}{}^{jk} + \left(\frac{1}{6} \mathcal{D}^\dagger \bar{\mathcal{H}} + \frac{1}{3} \mathcal{D} \bar{\mathcal{H}}\right) \Lambda_{\alpha j} \gamma_b^{\dot{\alpha}\alpha} \nabla_b \nabla_c T_{ac}{}^{ij} + \left(\frac{1}{4} \mathcal{D}^\dagger \bar{\mathcal{H}} + \frac{1}{3} \mathcal{D} \bar{\mathcal{L}}\right) T_{abjk} \nabla_b \chi^{\dot{\alpha}}{}_{lm}{}^i \varepsilon^{jklm} \\
& + \left(\frac{1}{4} \mathcal{D}^\dagger \bar{\mathcal{H}} + \frac{1}{3} \mathcal{D} \bar{\mathcal{L}}\right) \chi^{\dot{\alpha}}{}_{jk}{}^i \nabla_b T_{ablm} \varepsilon^{jklm} + \left(\frac{17}{48} \mathcal{D}^\dagger \bar{\mathcal{H}} + \frac{17}{24} \mathcal{D} \bar{\mathcal{L}}\right) P_a \bar{P}_b \nabla_b \Lambda^{\dot{\alpha}i} + \left(\frac{3}{8} \mathcal{D}^\dagger \bar{\mathcal{H}} + \frac{5}{8} \mathcal{D} \bar{\mathcal{L}}\right) \Lambda^{\dot{\alpha}i} \bar{P}_b \nabla_b P_a \\
& + \left(\frac{1}{2} \bar{\mathcal{L}} - \frac{1}{12} \mathcal{D}^\dagger \mathcal{D}^\dagger \bar{\mathcal{H}}\right) P_b \Lambda^{\dot{\alpha}j} R(V)_{ab}{}^i{}_{j\gamma} + \left(\frac{2}{3} \bar{\mathcal{L}} - \frac{1}{12} \mathcal{D}^\dagger \mathcal{D}^\dagger \bar{\mathcal{H}}\right) T_{abjk} \Lambda^{\dot{\alpha}j} \nabla_b E^{ik} + \left(\frac{3}{2} \bar{\mathcal{L}} + \frac{1}{8} \mathcal{D}^\dagger \mathcal{D}^\dagger \bar{\mathcal{H}}\right) E^{ij} P_b R(Q)_{ab}{}^{\dot{\alpha}}{}_{j\gamma} \\
& - \frac{1}{2} E_{jk} T_{ab}{}^{jl} \mathcal{D} \mathcal{H} \chi_{\alpha}{}^{ik}{}_{l\gamma b}^{\dot{\alpha}\alpha} - \frac{1}{16} E_{jk} \mathcal{D}^\dagger \bar{\mathcal{L}} \bar{P}_a \chi^{\dot{\alpha}}{}_{lm}{}^j \varepsilon^{iklm} + \frac{1}{36} E_{jk} \mathcal{D} \bar{\mathcal{L}} \Lambda^{\dot{\alpha}j} \nabla_b T_{ablm} \varepsilon^{iklm} - \frac{1}{48} E^{ij} P_b \mathcal{D} \bar{\mathcal{L}} \gamma_a^{\dot{\alpha}\alpha} \nabla_b \Lambda_{\alpha j} \\
& - \frac{1}{48} E^{ij} \mathcal{D}^\dagger \bar{\mathcal{L}} \Lambda_{\alpha j} \gamma_a^{\dot{\alpha}\alpha} \nabla_b \bar{P}_b + \frac{3}{40} E^{ij} \mathcal{D}^\dagger \bar{\mathcal{L}} \Lambda_{\alpha j} \gamma_b^{\dot{\alpha}\alpha} \nabla_a \bar{P}_b + \frac{1}{120} E^{ij} \mathcal{D}^\dagger \bar{\mathcal{L}} \Lambda_{\alpha j} \gamma_b^{\dot{\alpha}\alpha} \nabla_b \bar{P}_a + \frac{1}{12} E^{ij} \mathcal{D}^\dagger \bar{\mathcal{L}} \bar{P}_a \gamma_b^{\dot{\alpha}\alpha} \nabla_b \Lambda_{\alpha j} \\
& - \frac{1}{24} E^{ij} \mathcal{D}^\dagger \bar{\mathcal{L}} \bar{P}_b \gamma_a^{\dot{\alpha}\alpha} \nabla_b \Lambda_{\alpha j} + \frac{1}{12} E^{ij} \mathcal{D}^\dagger \bar{\mathcal{L}} \bar{P}_b \gamma_b^{\dot{\alpha}\alpha} \nabla_a \Lambda_{\alpha j} + \frac{1}{96} E^{jk} \mathcal{D} \bar{\mathcal{L}} \Lambda^{\dot{\beta}i} \gamma_{ab}^{\dot{\alpha}} \dot{\beta} \nabla_b E_{jk} + \frac{1}{8} P_b \mathcal{D} \bar{\mathcal{L}} \Lambda^{\dot{\beta}i} \gamma_{ac}^{\dot{\alpha}} \dot{\beta} \nabla_c \bar{P}_b \\
& - \frac{1}{2} T_{bcjk} \mathcal{D} \bar{\mathcal{L}} \Lambda^{\dot{\beta}j} \gamma_{bd}^{\dot{\alpha}} \dot{\beta} \nabla_c T_{ad}{}^{ik} - \frac{1}{24} T_{abjk} \mathcal{D} \bar{\mathcal{L}} \gamma_{bc}^{\dot{\alpha}} \dot{\beta} \nabla_c \chi^{\dot{\beta}}{}_{lm}{}^i \varepsilon^{jklm} + \frac{1}{24} T_{bcjk} \mathcal{D} \bar{\mathcal{L}} \gamma_{ab}^{\dot{\alpha}} \dot{\beta} \nabla_c \chi^{\dot{\beta}}{}_{lm}{}^i \varepsilon^{jklm} \\
& - \frac{1}{8} T_{ab}{}^{jk} \mathcal{D}^\dagger \bar{\mathcal{L}} \bar{P}_c \chi^{\dot{\beta}}{}_{jk}{}^i \gamma_{bc}^{\dot{\alpha}} \dot{\beta} + \frac{1}{8} T_{bc}{}^{jk} \mathcal{D}^\dagger \bar{\mathcal{L}} \bar{P}_b \chi^{\dot{\beta}}{}_{jk}{}^i \gamma_{ac}^{\dot{\alpha}} \dot{\beta} - \frac{1}{8} T_{ab}{}^{jk} \mathcal{D} \bar{\mathcal{L}} \Lambda^{\dot{\beta}i} \gamma_{cd}^{\dot{\alpha}} \dot{\beta} \nabla_b T_{cdjk} + \frac{1}{6} \bar{\mathcal{L}} E^{ij} T_{bcjk} \gamma_{bc}^{\dot{\alpha}} \dot{\beta} \nabla_a \Lambda^{\dot{\beta}k} \\
& + \frac{1}{12} \bar{\mathcal{L}} E^{ij} \Lambda^{\dot{\beta}k} \gamma_{bc}^{\dot{\alpha}} \dot{\beta} \nabla_a T_{bcjk} - \frac{7}{12} \bar{\mathcal{L}} P_a P_b \Lambda^{\dot{\alpha}i} \bar{P}_b - \bar{\mathcal{L}} P_b P_c R(Q)_{aba}{}^i \gamma_c^{\dot{\alpha}\alpha} + \frac{1}{3} \bar{\mathcal{L}} P_a T_{bcjk} R(Q)_{bc}{}^{\dot{\alpha}}{}_{l\gamma} \varepsilon^{ijkl} \\
& + \frac{1}{4} \bar{\mathcal{L}} P_a \Lambda^{\dot{\beta}j} R(V)_{bc}{}^i{}_{j\gamma bc}^{\dot{\alpha}} \dot{\beta} - \frac{1}{4} \bar{\mathcal{L}} T_{bcjk} T_{bclm} \nabla_a \Lambda^{\dot{\alpha}i} \varepsilon^{jklm} - \frac{1}{6} \bar{\mathcal{L}} T_{bcjk} \Lambda^{\dot{\beta}j} \gamma_{bc}^{\dot{\alpha}} \dot{\beta} \nabla_a E^{ik} + \frac{1}{3} \bar{\mathcal{L}} T_{abjk} \Lambda^{\dot{\alpha}i} \nabla_c T_{bclm} \varepsilon^{jklm} \\
& - \frac{3}{8} \bar{\mathcal{L}} T_{bcjk} \Lambda^{\dot{\alpha}i} \nabla_a T_{bclm} \varepsilon^{jklm} + \frac{1}{3} \bar{\mathcal{L}} T_{bcjk} \Lambda^{\dot{\alpha}i} \nabla_b T_{aclm} \varepsilon^{jklm} + \frac{1}{12} \bar{\mathcal{L}} T_{bcjk} \Lambda^{\dot{\alpha}j} \nabla_a T_{bclm} \varepsilon^{iklm} - \frac{1}{12} \bar{\mathcal{L}} T_{bcjk} \Lambda^{\dot{\alpha}l} \nabla_a T_{bclm} \varepsilon^{ijkm} \\
& + \frac{2}{3} \bar{\mathcal{H}} P_b \Lambda_{\alpha j} \gamma_b^{\dot{\alpha}\alpha} \nabla_c T_{ac}{}^{ij} - \frac{2}{3} \bar{\mathcal{H}} P_b \Lambda_{\alpha j} \gamma_c^{\dot{\alpha}\alpha} \nabla_a T_{bc}{}^{ij} + \frac{1}{2} \mathcal{D}^\dagger \bar{\mathcal{L}} P_b P_b \gamma_{ac}^{\dot{\alpha}} \dot{\beta} \nabla_c \Lambda^{\dot{\beta}i} + \mathcal{D}^\dagger \bar{\mathcal{L}} P_b P_c \gamma_{ab}^{\dot{\alpha}} \dot{\beta} \nabla_c \Lambda^{\dot{\beta}i} \\
& + \frac{1}{2} \mathcal{D}^\dagger \bar{\mathcal{L}} P_b \Lambda^{\dot{\beta}i} \gamma_{ab}^{\dot{\alpha}} \dot{\beta} \nabla_c P_c + \mathcal{D}^\dagger \bar{\mathcal{L}} P_b \Lambda^{\dot{\beta}i} \gamma_{ac}^{\dot{\alpha}} \dot{\beta} \nabla_b P_c - \frac{1}{48} \mathcal{D}^\dagger \bar{\mathcal{H}} E_{jk} E^{jk} \gamma_{ab}^{\dot{\alpha}} \dot{\beta} \nabla_b \Lambda^{\dot{\beta}i} - \frac{1}{48} \mathcal{D}^\dagger \bar{\mathcal{H}} E_{jk} \Lambda^{\dot{\beta}i} \gamma_{ab}^{\dot{\alpha}} \dot{\beta} \nabla_b E^{jk} \\
& + \frac{1}{24} \mathcal{D}^\dagger \bar{\mathcal{H}} P_b \Lambda^{\dot{\beta}i} \gamma_{ab}^{\dot{\alpha}} \dot{\beta} \nabla_c \bar{P}_c + \frac{1}{24} \mathcal{D}^\dagger \bar{\mathcal{H}} P_b \Lambda^{\dot{\beta}i} \gamma_{ac}^{\dot{\alpha}} \dot{\beta} \nabla_b \bar{P}_c - \frac{1}{48} \mathcal{D}^\dagger \bar{\mathcal{H}} P_b \bar{P}_c \gamma_{ac}^{\dot{\alpha}} \dot{\beta} \nabla_b \Lambda^{\dot{\beta}i} - \frac{1}{3} \mathcal{D}^\dagger \bar{\mathcal{H}} T_{ab}{}^{ij} \Lambda^{\dot{\beta}k} \gamma_{bc}^{\dot{\alpha}} \dot{\beta} \nabla_d T_{cdjk} \\
& + \frac{1}{2} \mathcal{D}^\dagger \mathcal{D}^\dagger \bar{\mathcal{L}} P_a P_b P_b \Lambda^{\dot{\alpha}i} + \frac{1}{48} \mathcal{D}^\dagger \mathcal{D}^\dagger \bar{\mathcal{H}} E^{ij} T_{abjk} \gamma_{bc}^{\dot{\alpha}} \dot{\beta} \nabla_c \Lambda^{\dot{\beta}k} - \frac{1}{48} \mathcal{D}^\dagger \mathcal{D}^\dagger \bar{\mathcal{H}} E^{ij} T_{bcjk} \gamma_{ab}^{\dot{\alpha}} \dot{\beta} \nabla_c \Lambda^{\dot{\beta}k} \\
& - \frac{1}{48} \mathcal{D}^\dagger \mathcal{D}^\dagger \bar{\mathcal{H}} T_{abjk} \Lambda^{\dot{\beta}j} \gamma_{bc}^{\dot{\alpha}} \dot{\beta} \nabla_c E^{ik} + \frac{1}{48} \mathcal{D}^\dagger \mathcal{D}^\dagger \bar{\mathcal{H}} T_{bcjk} \Lambda^{\dot{\beta}j} \gamma_{ab}^{\dot{\alpha}} \dot{\beta} \nabla_c E^{ik} + \frac{3}{8} \mathcal{D}^\dagger \bar{\mathcal{L}} D^{ij}{}_{kl} T_{ab}{}^{kl} \Lambda_{\alpha j} \gamma_b^{\dot{\alpha}\alpha} \\
& + \frac{1}{48} \mathcal{D}^\dagger \bar{\mathcal{L}} \Lambda_{\alpha j} \bar{P}_a \gamma_b^{\dot{\alpha}\alpha} \nabla_b E^{ij} + \frac{1}{48} \mathcal{D}^\dagger \bar{\mathcal{L}} \Lambda_{\alpha j} \bar{P}_b \gamma_a^{\dot{\alpha}\alpha} \nabla_b E^{ij} - \frac{5}{48} \mathcal{D}^\dagger \bar{\mathcal{L}} \Lambda_{\alpha j} \bar{P}_b \gamma_b^{\dot{\alpha}\alpha} \nabla_a E^{ij} + \frac{5}{24} \mathcal{D}^\dagger \bar{\mathcal{L}} \Lambda^{\dot{\beta}i} \bar{P}_a \gamma_{bc}^{\dot{\alpha}} \dot{\beta} \nabla_b \bar{P}_c \\
& - \frac{1}{24} \mathcal{D}^\dagger \bar{\mathcal{L}} \Lambda^{\dot{\beta}i} \bar{P}_b \gamma_{ab}^{\dot{\alpha}} \dot{\beta} \nabla_c \bar{P}_c - \frac{1}{8} \mathcal{D}^\dagger \bar{\mathcal{L}} \Lambda^{\dot{\beta}i} \bar{P}_b \gamma_{ac}^{\dot{\alpha}} \dot{\beta} \nabla_b \bar{P}_c + \frac{1}{24} \mathcal{D}^\dagger \bar{\mathcal{L}} \Lambda^{\dot{\beta}i} \bar{P}_b \gamma_{ac}^{\dot{\alpha}} \dot{\beta} \nabla_c \bar{P}_b + \frac{1}{24} \mathcal{D}^\dagger \bar{\mathcal{L}} \Lambda^{\dot{\beta}i} \bar{P}_b \gamma_{bc}^{\dot{\alpha}} \dot{\beta} \nabla_a \bar{P}_c \\
& - \frac{1}{24} \mathcal{D}^\dagger \bar{\mathcal{L}} \Lambda^{\dot{\beta}i} \bar{P}_b \gamma_{bc}^{\dot{\alpha}} \dot{\beta} \nabla_c \bar{P}_a - \frac{1}{6} \mathcal{D}^\dagger \bar{\mathcal{L}} \bar{P}_a \bar{P}_b \gamma_{bc}^{\dot{\alpha}} \dot{\beta} \nabla_c \Lambda^{\dot{\beta}i} + \frac{1}{8} \mathcal{D}^\dagger \bar{\mathcal{L}} \bar{P}_b \bar{P}_b \gamma_{ac}^{\dot{\alpha}} \dot{\beta} \nabla_c \Lambda^{\dot{\beta}i} - \frac{1}{12} \mathcal{D}^\dagger \bar{\mathcal{L}} \bar{P}_b \bar{P}_c \gamma_{ab}^{\dot{\alpha}} \dot{\beta} \nabla_c \Lambda^{\dot{\beta}i} + 2 \dots
\end{aligned}$$

$$\begin{aligned}
[\hat{\Omega}_a^{\dot{\alpha}i}]_{1,cont.} = & +\frac{1}{24}\mathcal{D}\bar{\mathcal{L}}R(Q)_{bc}{}^{\dot{\beta}}{}_j\gamma_{ad}{}^{\dot{\alpha}}{}_{\dot{\beta}}\nabla_dT_{bckl}\varepsilon^{ijkl}-\frac{1}{12}\mathcal{D}\mathcal{D}\mathcal{H}T_{ab}{}^{ij}\Lambda_{\alpha j}\gamma_b{}^{\dot{\alpha}\alpha}\nabla_c\bar{P}_c+\frac{1}{12}\mathcal{D}\mathcal{D}\mathcal{H}T_{ab}{}^{ij}\Lambda_{\alpha j}\gamma_c{}^{\dot{\alpha}\alpha}\nabla_c\bar{P}_b \\
& -\frac{1}{12}\mathcal{D}\mathcal{D}\mathcal{H}T_{bc}{}^{ij}\Lambda_{\alpha j}\gamma_a{}^{\dot{\alpha}\alpha}\nabla_b\bar{P}_c-\frac{1}{12}\mathcal{D}\mathcal{D}\mathcal{H}T_{bc}{}^{ij}\Lambda_{\alpha j}\gamma_b{}^{\dot{\alpha}\alpha}\nabla_c\bar{P}_a-\frac{1}{6}\mathcal{D}\mathcal{D}\mathcal{H}\Lambda_{\alpha j}\bar{P}_b\gamma_c{}^{\dot{\alpha}\alpha}\nabla_bT_{ac}{}^{ij}+\frac{2}{3}\mathcal{I}T_{bc}{}^{ij}\Lambda_{\alpha j}\gamma_b{}^{\dot{\alpha}\alpha}\nabla_a\bar{P}_c \\
& +\frac{1}{3}\mathcal{H}P_b\Lambda_{\alpha j}\gamma_a{}^{\dot{\alpha}\alpha}\nabla_cT_{bc}{}^{ij}-\frac{1}{3}\mathcal{H}P_b\Lambda_{\alpha j}\gamma_c{}^{\dot{\alpha}\alpha}\nabla_bT_{ac}{}^{ij}-\frac{1}{6}\mathcal{H}T_{bc}{}^{ij}\Lambda^{\dot{\alpha}k}\nabla_aT_{bc}{}^{lm}\varepsilon_{jklm}-\frac{1}{6}\mathcal{H}T_{bc}{}^{jk}\Lambda^{\dot{\alpha}l}\nabla_aT_{bc}{}^{im}\varepsilon_{jklm} \\
& +(-\frac{9}{4}\bar{\mathcal{L}}+\frac{1}{16}\mathcal{D}^\dagger\mathcal{D}^\dagger\bar{\mathcal{H}})P_bP_b\Lambda^{\dot{\alpha}i}\bar{P}_a+(-\frac{4}{3}\bar{\mathcal{L}}-\frac{1}{6}\mathcal{D}^\dagger\mathcal{D}^\dagger\bar{\mathcal{H}})P_bT_{bcjk}T_{ac}{}^{ij}\Lambda^{\dot{\alpha}k}+(-\frac{4}{3}\bar{\mathcal{L}}+\frac{1}{4}\mathcal{D}^\dagger\mathcal{D}^\dagger\bar{\mathcal{H}})P_bT_{bcjk}T_{ac}{}^{jk}\Lambda^{\dot{\alpha}i} \\
& +(-\frac{17}{24}\bar{\mathcal{H}}-\frac{5}{8}\mathcal{H})T_{bc}{}^{ij}\Lambda_{\alpha j}\gamma_a{}^{\dot{\alpha}\alpha}\nabla_bP_c+(-\frac{2}{3}\bar{\mathcal{L}}-\frac{1}{24}\mathcal{D}^\dagger\mathcal{D}^\dagger\bar{\mathcal{H}})T_{abjk}T_{bclm}\nabla_c\Lambda^{\dot{\alpha}j}\varepsilon^{iklm}+(-\frac{2}{3}\bar{\mathcal{L}}+\frac{1}{12}\mathcal{D}^\dagger\mathcal{D}^\dagger\bar{\mathcal{H}})P_bT_{abjk}\chi^{\dot{\alpha}}{}_{lm}{}^i\varepsilon^{jklm} \\
& +(-\frac{7}{12}\bar{\mathcal{H}}-\frac{1}{12}\mathcal{H})P_a\Lambda_{\alpha j}\gamma_b{}^{\dot{\alpha}\alpha}\nabla_cT_{bc}{}^{ij}+(-\frac{7}{12}\bar{\mathcal{H}}-\frac{1}{12}\mathcal{H})P_b\Lambda_{\alpha j}\gamma_c{}^{\dot{\alpha}\alpha}\nabla_cT_{ab}{}^{ij}+(-\frac{7}{12}\bar{\mathcal{H}}-\frac{1}{12}\mathcal{H})T_{ab}{}^{ij}\Lambda_{\alpha j}\gamma_b{}^{\dot{\alpha}\alpha}\nabla_cP_c \\
& +(-\frac{1}{2}\bar{\mathcal{L}}-\frac{1}{8}\mathcal{D}^\dagger\mathcal{D}^\dagger\bar{\mathcal{H}})P_bT_{bcjk}R(Q)_{ac}{}^{\dot{\alpha}}{}_l\varepsilon^{ijkl}+(-\frac{3}{8}\bar{\mathcal{H}}-\frac{1}{8}\mathcal{H})T_{bcjk}T_{ab}{}^{il}\chi_{\alpha}{}^{jk}{}_l\gamma_c{}^{\dot{\alpha}\alpha}+(-\frac{1}{3}\bar{\mathcal{L}}-\frac{1}{24}\mathcal{D}^\dagger\mathcal{D}^\dagger\bar{\mathcal{H}})T_{abjk}\Lambda^{\dot{\alpha}j}\nabla_cT_{bclm}\varepsilon^{iklm} \\
& +(-\frac{1}{3}\bar{\mathcal{L}}-\frac{1}{24}\mathcal{D}^\dagger\mathcal{D}^\dagger\bar{\mathcal{H}})T_{bcjk}\Lambda^{\dot{\alpha}j}\nabla_bT_{aclm}\varepsilon^{iklm}+(-\frac{1}{3}\bar{\mathcal{L}}-\frac{1}{48}\mathcal{D}^\dagger\mathcal{D}^\dagger\bar{\mathcal{H}})E^{ij}\Lambda^{\dot{\beta}k}\gamma_{ab}{}^{\dot{\alpha}}{}_{\dot{\beta}}\nabla_cT_{bcjk} \\
& +(-\frac{1}{3}\bar{\mathcal{L}}-\frac{1}{48}\mathcal{D}^\dagger\mathcal{D}^\dagger\bar{\mathcal{H}})E^{ij}\Lambda^{\dot{\beta}k}\gamma_{bc}{}^{\dot{\alpha}}{}_{\dot{\beta}}\nabla_bT_{acjk}+(-\frac{1}{3}\bar{\mathcal{H}}-\frac{1}{6}\mathcal{H})\Lambda_{\alpha j}\gamma_b{}^{\dot{\alpha}\alpha}\nabla_b\nabla_cT_{ackl}\varepsilon^{ijkl}+(-\frac{1}{3}\mathcal{D}^\dagger\bar{\mathcal{L}}+\frac{1}{12}\mathcal{D}^\dagger\mathcal{D}^\dagger\bar{\mathcal{H}})E^{ij}P_bT_{abjk}\Lambda^{\dot{\alpha}k} \\
& +(-\frac{1}{3}\mathcal{D}^\dagger\bar{\mathcal{H}}-\frac{1}{6}\mathcal{D}\bar{\mathcal{L}})T_{ab}{}^{jk}\Lambda^{\dot{\beta}i}\gamma_{bc}{}^{\dot{\alpha}}{}_{\dot{\beta}}\nabla_dT_{cdjk}+(-\frac{7}{24}\mathcal{D}^\dagger\mathcal{I}+\frac{1}{4}\mathcal{D}\mathcal{H})E_{jk}T_{bc}{}^{ij}R(Q)_{bca}{}^k\gamma_a{}^{\dot{\alpha}\alpha} \\
& +(-\frac{7}{24}\mathcal{D}^\dagger\mathcal{I}+\frac{1}{4}\mathcal{D}\mathcal{H})T_{bc}{}^{ij}\Lambda_{\alpha k}R(V)_{bc}{}^k{}_j\gamma_a{}^{\dot{\alpha}\alpha}+(-\frac{7}{24}\mathcal{D}^\dagger\mathcal{I}+\frac{1}{3}\mathcal{D}\mathcal{H})E_{jk}T_{ab}{}^{ij}\Lambda^{\dot{\alpha}k}\bar{P}_b+(-\frac{1}{4}\bar{\mathcal{L}}-\frac{1}{24}\mathcal{D}^\dagger\mathcal{D}^\dagger\bar{\mathcal{H}})P_b\Lambda^{\dot{\alpha}j}R(V)_{cd}{}^i{}_j\varepsilon_{abcd} \\
& +(-\frac{1}{4}\bar{\mathcal{L}}+\frac{1}{32}\mathcal{D}^\dagger\mathcal{D}^\dagger\bar{\mathcal{H}})E_{jk}E^{ij}P_a\Lambda^{\dot{\alpha}k}+(-\frac{1}{4}\mathcal{D}^\dagger\bar{\mathcal{H}}-\frac{1}{4}\mathcal{D}\bar{\mathcal{L}})P_bT_{ac}{}^{jk}\chi^{\dot{\beta}}{}_{jk}{}^i\gamma_{bc}{}^{\dot{\alpha}}{}_{\dot{\beta}}+(-\frac{1}{4}\mathcal{D}^\dagger\bar{\mathcal{H}}-\frac{1}{4}\mathcal{D}\bar{\mathcal{L}})P_bT_{bc}{}^{jk}\chi^{\dot{\beta}}{}_{jk}{}^i\gamma_{ac}{}^{\dot{\alpha}}{}_{\dot{\beta}} \\
& +(-\frac{1}{4}\mathcal{D}^\dagger\mathcal{I}+\frac{1}{3}\mathcal{D}\mathcal{H})T_{ab}{}^{ij}\Lambda_{\alpha k}R(V)_{bc}{}^k{}_j\gamma_c{}^{\dot{\alpha}\alpha}+(-\frac{7}{32}\bar{\mathcal{H}}+\frac{5}{96}\mathcal{H})P_a\Lambda^{\dot{\alpha}i}\bar{P}_b\bar{P}_b+(-\frac{1}{6}\bar{\mathcal{L}}+\frac{1}{24}\mathcal{D}^\dagger\mathcal{D}^\dagger\bar{\mathcal{H}})P_b\Lambda^{\dot{\beta}j}R(V)_{ac}{}^i{}_j\gamma_{bc}{}^{\dot{\alpha}}{}_{\dot{\beta}} \\
& +(-\frac{1}{6}\mathcal{D}^\dagger\bar{\mathcal{H}}-\frac{1}{3}\mathcal{D}\bar{\mathcal{L}})E^{ij}T_{abjk}\Lambda^{\dot{\alpha}k}\bar{P}_b+(-\frac{1}{6}\mathcal{D}^\dagger\bar{\mathcal{H}}-\frac{1}{12}\mathcal{D}\bar{\mathcal{L}})T_{ab}{}^{jk}\Lambda^{\dot{\alpha}l}\nabla_bE^{im}\varepsilon_{jklm}+(-\frac{1}{6}\mathcal{D}^\dagger\mathcal{I}+\frac{2}{3}\mathcal{D}\mathcal{H})T_{bc}{}^{ij}\Lambda_{\alpha j}R(M)_{adbc}\gamma_d{}^{\dot{\alpha}\alpha} \\
& +(-\frac{1}{6}\mathcal{D}\mathcal{D}\mathcal{H}-\frac{4}{3}\mathcal{I})T_{ab}{}^{ij}\bar{P}_c\gamma_b{}^{\dot{\alpha}\alpha}\nabla_c\Lambda_{\alpha j}+(-\frac{7}{48}\mathcal{D}^\dagger\bar{\mathcal{H}}-\frac{3}{8}\mathcal{D}\bar{\mathcal{L}})P_b\bar{P}_c\nabla_d\Lambda^{\dot{\alpha}i}\varepsilon_{abcd}+(-\frac{7}{48}\mathcal{D}^\dagger\bar{\mathcal{H}}-\frac{1}{4}\mathcal{D}\bar{\mathcal{L}})P_b\bar{P}_a\gamma_{bc}{}^{\dot{\alpha}}{}_{\dot{\beta}}\nabla_c\Lambda^{\dot{\beta}i} \\
& +(-\frac{1}{8}\bar{\mathcal{H}}-\frac{5}{24}\mathcal{H})T_{ab}{}^{ij}\Lambda_{\alpha j}\gamma_c{}^{\dot{\alpha}\alpha}\nabla_cP_b+(-\frac{1}{8}\bar{\mathcal{H}}-\frac{1}{24}\mathcal{H})T_{abjk}T_{bc}{}^{il}\chi_{\alpha}{}^{jk}{}_l\gamma_c{}^{\dot{\alpha}\alpha}+(-\frac{1}{8}\bar{\mathcal{H}}+\frac{1}{8}\mathcal{H})T_{bcjk}R(Q)_{ab}{}^{\dot{\alpha}}{}_l\bar{P}_c\varepsilon^{ijkl} \\
& +(-\frac{1}{8}\mathcal{D}^\dagger\bar{\mathcal{H}}-\frac{5}{24}\mathcal{D}\bar{\mathcal{L}})T_{bcjk}\gamma_{ad}{}^{\dot{\alpha}}{}_{\dot{\beta}}\nabla_dR(Q)_{bc}{}^{\dot{\beta}}{}_l\varepsilon^{ijkl}+(-\frac{5}{48}\bar{\mathcal{H}}+\frac{5}{48}\mathcal{H})T_{abjk}\gamma_b{}^{\dot{\alpha}\alpha}\nabla_c\nabla_c\Lambda_{\alpha l}\varepsilon^{ijkl} \\
& +(-\frac{5}{48}\bar{\mathcal{H}}+\frac{5}{48}\mathcal{H})\gamma_b{}^{\dot{\alpha}\alpha}\nabla_cT_{bcjk}\nabla_a\Lambda_{\alpha l}\varepsilon^{ijkl}+(-\frac{1}{12}\bar{\mathcal{H}}+\frac{1}{12}\mathcal{H})P_bT_{ac}{}^{ij}\gamma_c{}^{\dot{\alpha}\alpha}\nabla_b\Lambda_{\alpha j}+(-\frac{1}{12}\bar{\mathcal{H}}+\frac{3}{4}\mathcal{H})P_bT_{bc}{}^{ij}\gamma_a{}^{\dot{\alpha}\alpha}\nabla_c\Lambda_{\alpha j} \\
& +(-\frac{1}{12}\mathcal{D}^\dagger\bar{\mathcal{H}}-\frac{5}{12}\mathcal{D}\bar{\mathcal{L}})T_{bcjk}\Lambda^{\dot{\beta}i}\gamma_{bc}{}^{\dot{\alpha}}{}_{\dot{\beta}}\nabla_dT_{ad}{}^{jk}+(-\frac{1}{12}\mathcal{D}^\dagger\bar{\mathcal{H}}-\frac{5}{36}\mathcal{D}\bar{\mathcal{L}})E_{jk}T_{ablm}\nabla_b\Lambda^{\dot{\alpha}j}\varepsilon^{iklm} \\
& +(-\frac{1}{12}\mathcal{D}^\dagger\bar{\mathcal{H}}-\frac{1}{8}\mathcal{D}\bar{\mathcal{L}})\Lambda^{\dot{\beta}i}\bar{P}_b\gamma_{ac}{}^{\dot{\alpha}}{}_{\dot{\beta}}\nabla_cP_b+(-\frac{1}{12}\mathcal{D}^\dagger\bar{\mathcal{H}}-\frac{1}{16}\mathcal{D}\bar{\mathcal{L}})E^{ij}P_a\gamma_b{}^{\dot{\alpha}\alpha}\nabla_b\Lambda_{\alpha j}+(-\frac{1}{12}\mathcal{D}^\dagger\bar{\mathcal{H}}+\frac{1}{12}\mathcal{D}\bar{\mathcal{L}})E_{jk}P_bT_{ab}{}^{ij}\Lambda^{\dot{\alpha}k} \\
& +(-\frac{1}{12}\mathcal{D}^\dagger\bar{\mathcal{H}}+\frac{1}{12}\mathcal{D}\bar{\mathcal{L}})T_{bcjk}\Lambda^{\dot{\beta}j}\gamma_{bc}{}^{\dot{\alpha}}{}_{\dot{\beta}}\nabla_dT_{ad}{}^{ik}+(-\frac{1}{12}\mathcal{D}^\dagger\mathcal{I}-\frac{1}{3}\mathcal{D}\mathcal{H})T_{ab}{}^{jk}\Lambda_{\alpha j}R(V)_{bc}{}^i{}_k\gamma_c{}^{\dot{\alpha}\alpha} \\
& +(-\frac{1}{12}\mathcal{D}\mathcal{D}\mathcal{H}-\frac{2}{3}\mathcal{I})T_{bc}{}^{ij}\bar{P}_a\gamma_b{}^{\dot{\alpha}\alpha}\nabla_c\Lambda_{\alpha j}+(-\frac{1}{12}\mathcal{D}\mathcal{D}\mathcal{H}+\frac{2}{3}\mathcal{I})\Lambda_{\alpha j}\bar{P}_a\gamma_b{}^{\dot{\alpha}\alpha}\nabla_cT_{bc}{}^{ij}+(-\frac{1}{15}\mathcal{D}^\dagger\bar{\mathcal{H}}-\frac{1}{12}\mathcal{D}\bar{\mathcal{L}})E^{ij}\Lambda_{\alpha j}\gamma_b{}^{\dot{\alpha}\alpha}\nabla_aP_b \\
& +(-\frac{1}{16}\bar{\mathcal{H}}-\frac{1}{48}\mathcal{H})E_{jk}E^{ij}\Lambda^{\dot{\alpha}k}\bar{P}_a+(-\frac{1}{16}\bar{\mathcal{H}}-\frac{1}{48}\mathcal{H})E_{jk}T_{bc}{}^{ij}\gamma_{ab}{}^{\dot{\alpha}}{}_{\dot{\beta}}\nabla_c\Lambda^{\dot{\beta}k}+(-\frac{1}{16}\bar{\mathcal{H}}+\frac{1}{16}\mathcal{H})E^{ij}R(Q)_{ab}{}^{\dot{\beta}}{}_j\bar{P}_c\gamma_{bc}{}^{\dot{\alpha}}{}_{\dot{\beta}} \\
& +(-\frac{1}{16}\bar{\mathcal{H}}+\frac{1}{16}\mathcal{H})\Lambda^{\dot{\beta}i}R(M)_{abcd}\bar{P}_b\gamma_{cd}{}^{\dot{\alpha}}{}_{\dot{\beta}}+(-\frac{1}{16}\bar{\mathcal{H}}+\frac{1}{16}\mathcal{H})\Lambda^{\dot{\beta}j}R(V)_{bc}{}^i{}_j\bar{P}_b\gamma_{ac}{}^{\dot{\alpha}}{}_{\dot{\beta}}+(-\frac{1}{16}\bar{\mathcal{H}}+\frac{1}{16}\mathcal{H})\gamma_b{}^{\dot{\alpha}\alpha}\nabla_bT_{acjk}\nabla_c\Lambda_{\alpha l}\varepsilon^{ijkl} \\
& +(-\frac{1}{16}\bar{\mathcal{H}}+\frac{1}{16}\mathcal{H})\gamma_b{}^{\dot{\alpha}\alpha}\nabla_cT_{abjk}\nabla_c\Lambda_{\alpha l}\varepsilon^{ijkl}+(-\frac{1}{16}\bar{\mathcal{H}}+\frac{1}{16}\mathcal{H})\gamma_b{}^{\dot{\alpha}\alpha}\nabla_cT_{acjk}\nabla_b\Lambda_{\alpha l}\varepsilon^{ijkl}+(-\frac{1}{16}\bar{\mathcal{H}}+\frac{5}{16}\mathcal{H})R(V)_{bc}{}^j{}_k\chi_{\alpha}{}^{ik}{}_j\gamma_d{}^{\dot{\alpha}\alpha}\varepsilon_{abcd} \\
& +(-\frac{1}{16}\mathcal{D}^\dagger\bar{\mathcal{H}}-\frac{9}{32}\mathcal{D}\bar{\mathcal{L}})\Lambda^{\dot{\beta}i}\bar{P}_b\gamma_{bc}{}^{\dot{\alpha}}{}_{\dot{\beta}}\nabla_cP_a+(-\frac{1}{16}\mathcal{D}^\dagger\bar{\mathcal{H}}-\frac{1}{8}\mathcal{D}\bar{\mathcal{L}})T_{bcjk}\gamma_{bc}{}^{\dot{\alpha}}{}_{\dot{\beta}}\nabla_a\chi^{\dot{\beta}}{}_{lm}{}^i\varepsilon^{jklm} \\
& +(-\frac{1}{16}\mathcal{D}^\dagger\bar{\mathcal{H}}-\frac{1}{8}\mathcal{D}\bar{\mathcal{L}})\chi^{\dot{\beta}}{}_{jk}{}^i\gamma_{bc}{}^{\dot{\alpha}}{}_{\dot{\beta}}\nabla_aT_{bclm}\varepsilon^{jklm}+(-\frac{1}{16}\mathcal{D}^\dagger\bar{\mathcal{H}}-\frac{1}{32}\mathcal{D}\bar{\mathcal{L}})\Lambda^{\dot{\beta}i}\bar{P}_a\gamma_{bc}{}^{\dot{\alpha}}{}_{\dot{\beta}}\nabla_bP_c+(-\frac{1}{16}\mathcal{D}\mathcal{D}\mathcal{H}-\frac{1}{2}\mathcal{I})\Lambda^{\dot{\alpha}i}\bar{P}_a\bar{P}_b\bar{P}_b \\
& +(-\frac{1}{18}\bar{\mathcal{H}}-\frac{1}{9}\mathcal{H})T_{ab}{}^{ij}\Lambda^{\dot{\beta}k}\gamma_{bc}{}^{\dot{\alpha}}{}_{\dot{\beta}}\nabla_cE_{jk}+(-\frac{1}{24}\bar{\mathcal{L}}-\frac{1}{32}\mathcal{D}^\dagger\mathcal{D}^\dagger\bar{\mathcal{H}})E_{jk}E^{jk}P_a\Lambda^{\dot{\alpha}i}+(-\frac{1}{24}\bar{\mathcal{H}}+\frac{1}{24}\mathcal{H})T_{abjk}\gamma_c{}^{\dot{\alpha}\alpha}\nabla_b\nabla_c\Lambda_{\alpha l}\varepsilon^{ijkl}+3\cdots
\end{aligned}$$

$$\begin{aligned}
[\hat{\Omega}_a^{\dot{\alpha}i}]_{1,cont.} = & +(-\frac{1}{24}\bar{\mathcal{H}} + \frac{1}{24}\mathcal{H})T_{bcjk}\gamma_b^{\dot{\alpha}\alpha}\nabla_a\nabla_c\Lambda_{\alpha l}\varepsilon^{ijkl} + (-\frac{1}{24}\bar{\mathcal{H}} + \frac{1}{12}\mathcal{H})E^{ij}\Lambda_{\alpha k}R(V)_{ab}{}^k{}_j\gamma_b^{\dot{\alpha}\alpha} + (-\frac{1}{24}\bar{\mathcal{H}} + \frac{7}{24}\mathcal{H})T_{ab}{}^{jk}T_{bc}{}^{il}\nabla_c\Lambda^{\dot{\alpha}m}\varepsilon_{jklm} \\
& + (-\frac{1}{24}\mathcal{D}^\dagger\bar{\mathcal{H}} - \frac{1}{24}\mathcal{D}\bar{\mathcal{L}})P_a\Lambda_{\alpha j}\gamma_b^{\dot{\alpha}\alpha}\nabla_bE^{ij} + (-\frac{1}{32}\bar{\mathcal{H}} - \frac{1}{96}\mathcal{H})E^{jk}\Lambda_{\alpha j}R(V)_{ab}{}^i{}_k\gamma_b^{\dot{\alpha}\alpha} + (-\frac{1}{32}\bar{\mathcal{H}} + \frac{1}{32}\mathcal{H})P_b\Lambda^{\dot{\alpha}i}\bar{P}_a\bar{P}_b \\
& + (-\frac{1}{32}\bar{\mathcal{H}} + \frac{1}{32}\mathcal{H})\gamma_b^{\dot{\alpha}\alpha}\nabla_cE^{ij}\nabla_d\Lambda_{\alpha j}\varepsilon_{abcd} + (-\frac{1}{32}\bar{\mathcal{H}} + \frac{7}{96}\mathcal{H})T_{bc}{}^{jk}\Lambda^{\dot{\alpha}i}\nabla_aT_{bc}{}^{lm}\varepsilon_{jklm} + (-\frac{1}{48}\bar{\mathcal{H}} + \frac{1}{48}\mathcal{H})E_{jk}T_{ab}{}^{ij}\gamma_{bc}{}^{\dot{\alpha}}{}_{\dot{\beta}}\nabla_c\Lambda^{\dot{\beta}k} \\
& + (-\frac{1}{48}\bar{\mathcal{H}} + \frac{1}{48}\mathcal{H})\Lambda^{\dot{\beta}j}R(V)_{ab}{}^i{}_j\bar{P}_c\gamma_{bc}{}^{\dot{\alpha}}{}_{\dot{\beta}} + (-\frac{1}{48}\bar{\mathcal{H}} + \frac{1}{48}\mathcal{H})\gamma_a^{\dot{\alpha}\alpha}\nabla_bT_{bcjk}\nabla_c\Lambda_{\alpha l}\varepsilon^{ijkl} + (-\frac{1}{48}\bar{\mathcal{H}} + \frac{1}{48}\mathcal{H})\gamma_b^{\dot{\alpha}\alpha}\nabla_aT_{bcjk}\nabla_c\Lambda_{\alpha l}\varepsilon^{ijkl} \\
& + (-\frac{1}{48}\mathcal{D}^\dagger\bar{\mathcal{H}} - \frac{3}{32}\mathcal{D}\bar{\mathcal{L}})P_b\Lambda^{\dot{\beta}i}\gamma_{bc}{}^{\dot{\alpha}}{}_{\dot{\beta}}\nabla_c\bar{P}_a + (-\frac{1}{48}\mathcal{D}^\dagger\bar{\mathcal{H}} - \frac{1}{96}\mathcal{D}\bar{\mathcal{L}})P_a\Lambda^{\dot{\beta}i}\gamma_{bc}{}^{\dot{\alpha}}{}_{\dot{\beta}}\nabla_b\bar{P}_c + (\frac{1}{576}\bar{\mathcal{H}} - \frac{1}{576}\mathcal{H})E_{jk}\Lambda^{\dot{\beta}j}\gamma_{bc}{}^{\dot{\alpha}}{}_{\dot{\beta}}\nabla_aT_{bc}{}^{ik} \\
& + (\frac{1}{96}\bar{\mathcal{H}} - \frac{1}{96}\mathcal{H})\chi^{\dot{\beta}}{}_{jk}{}^l\gamma_{ab}{}^{\dot{\alpha}}{}_{\dot{\beta}}\nabla_bE_{lm}\varepsilon^{ijkm} + (\frac{5}{288}\bar{\mathcal{H}} + \frac{43}{288}\mathcal{H})E_{jk}\Lambda^{\dot{\beta}j}\gamma_{bc}{}^{\dot{\alpha}}{}_{\dot{\beta}}\nabla_bT_{ac}{}^{ik} + (\frac{1}{48}\mathcal{D}^\dagger\bar{\mathcal{H}} - \frac{1}{32}\mathcal{D}\bar{\mathcal{L}})P_b\Lambda^{\dot{\beta}i}\gamma_{bc}{}^{\dot{\alpha}}{}_{\dot{\beta}}\nabla_a\bar{P}_c \\
& + (\frac{1}{32}\bar{\mathcal{H}} - \frac{1}{32}\mathcal{H})\Lambda^{\dot{\beta}j}R(V)_{bc}{}^i{}_j\bar{P}_a\gamma_{bc}{}^{\dot{\alpha}}{}_{\dot{\beta}} + (\frac{1}{32}\bar{\mathcal{H}} + \frac{1}{32}\mathcal{H})E_{jk}E^{jk}\Lambda^{\dot{\alpha}i}\bar{P}_a + (\frac{1}{32}\bar{\mathcal{H}} + \frac{13}{96}\mathcal{H})\Lambda^{\dot{\alpha}j}R(V)_{bc}{}^i{}_j\bar{P}_d\varepsilon_{abcd} \\
& + (\frac{5}{144}\bar{\mathcal{H}} + \frac{19}{144}\mathcal{H})T_{bc}{}^{ij}\Lambda^{\dot{\beta}k}\gamma_{ab}{}^{\dot{\alpha}}{}_{\dot{\beta}}\nabla_cE_{jk} + (\frac{1}{24}\bar{\mathcal{H}} - \frac{3}{8}\mathcal{H})T_{bc}{}^{ij}\Lambda_{\alpha j}\gamma_b^{\dot{\alpha}\alpha}\nabla_cP_a + (\frac{1}{24}\bar{\mathcal{H}} - \frac{7}{24}\mathcal{H})T_{ab}{}^{ij}T_{bc}{}^{kl}\nabla_c\Lambda^{\dot{\alpha}m}\varepsilon_{jklm} \\
& + (\frac{1}{24}\bar{\mathcal{H}} + \frac{1}{12}\mathcal{H})E_{jk}\gamma_{ab}{}^{\dot{\alpha}}{}_{\dot{\beta}}\nabla_b\chi^{\dot{\beta}}{}_{lm}{}^j\varepsilon^{iklm} + (\frac{1}{24}\bar{\mathcal{H}} + \frac{7}{24}\mathcal{H})T_{ab}{}^{ij}\Lambda_{\alpha j}\gamma_c^{\dot{\alpha}\alpha}\nabla_bP_c + (\frac{1}{24}\bar{\mathcal{H}} + \frac{7}{24}\mathcal{H})T_{bc}{}^{ij}\Lambda_{\alpha j}\gamma_b^{\dot{\alpha}\alpha}\nabla_aP_c \\
& + (\frac{1}{24}\bar{\mathcal{H}} + \frac{11}{24}\mathcal{H})P_bR(Q)_{bca}{}^i\bar{P}_c\gamma_a^{\dot{\alpha}\alpha} + (\frac{1}{24}\mathcal{D}^\dagger\bar{\mathcal{H}} - \frac{1}{24}\mathcal{D}\bar{\mathcal{L}})E_{jk}P_a\chi^{\dot{\beta}}{}_{lm}{}^j\varepsilon^{iklm} + (\frac{1}{24}\mathcal{D}^\dagger\bar{\mathcal{H}} + \frac{1}{24}\mathcal{D}\bar{\mathcal{L}})E_{jk}\Lambda^{\dot{\beta}j}\gamma_{ab}{}^{\dot{\alpha}}{}_{\dot{\beta}}\nabla_bE^{ik} \\
& + (\frac{1}{24}\mathcal{D}^\dagger\bar{\mathcal{H}} + \frac{7}{96}\mathcal{D}\bar{\mathcal{L}})E^{ij}\Lambda^{\dot{\beta}k}\gamma_{ab}{}^{\dot{\alpha}}{}_{\dot{\beta}}\nabla_bE_{jk} + (\frac{1}{24}\mathcal{D}^\dagger\bar{\mathcal{H}} + \frac{1}{8}\mathcal{D}\bar{\mathcal{L}})P_b\Lambda_{\alpha j}\gamma_b^{\dot{\alpha}\alpha}\nabla_aE^{ij} + (\frac{5}{96}\bar{\mathcal{H}} + \frac{1}{48}\mathcal{H})T_{bc}{}^{jk}T_{bc}{}^{lm}\nabla_a\Lambda^{\dot{\alpha}i}\varepsilon_{jklm} \\
& + (\frac{1}{16}\bar{\mathcal{H}} - \frac{1}{16}\mathcal{H})T_{bcjk}R(Q)_{bc}{}^{\dot{\alpha}}{}_l\bar{P}_a\varepsilon^{ijkl} + (\frac{1}{16}\mathcal{D}^\dagger\bar{\mathcal{H}} + \frac{5}{32}\mathcal{D}\bar{\mathcal{L}})\Lambda^{\dot{\beta}i}\bar{P}_b\gamma_{bc}{}^{\dot{\alpha}}{}_{\dot{\beta}}\nabla_aP_c + (\frac{1}{15}\mathcal{D}^\dagger\bar{\mathcal{H}} + \frac{1}{8}\mathcal{D}\bar{\mathcal{L}})E^{ij}\Lambda_{\alpha j}\gamma_b^{\dot{\alpha}\alpha}\nabla_bP_a \\
& + (\frac{1}{12}\bar{\mathcal{H}} - \frac{1}{12}\mathcal{H})P_bR(Q)_{aca}{}^i\bar{P}_c\gamma_b^{\dot{\alpha}\alpha} + (\frac{1}{12}\mathcal{D}^\dagger\bar{\mathcal{H}} - \frac{1}{12}\mathcal{D}\bar{\mathcal{L}})E^{ij}T_{ab}{}^{kl}\nabla_b\Lambda^{\dot{\alpha}m}\varepsilon_{jklm} + (\frac{1}{12}\mathcal{D}^\dagger\bar{\mathcal{H}} - \frac{1}{48}\mathcal{D}\bar{\mathcal{L}})E^{ij}\Lambda^{\dot{\alpha}k}\nabla_bT_{ab}{}^{lm}\varepsilon_{jklm} \\
& + (\frac{1}{12}\mathcal{D}^\dagger\bar{\mathcal{H}} + \frac{1}{8}\mathcal{D}\bar{\mathcal{L}})E_{jk}E^{ij}\gamma_{ab}{}^{\dot{\alpha}}{}_{\dot{\beta}}\nabla_b\Lambda^{\dot{\beta}k} + (\frac{1}{12}\mathcal{D}^\dagger\bar{\mathcal{H}} + \frac{19}{144}\mathcal{D}\bar{\mathcal{L}})T_{abjk}\Lambda^{\dot{\alpha}l}\nabla_bE_{lm}\varepsilon^{ijkm} \\
& + (\frac{1}{12}\mathcal{D}^\dagger\bar{\mathcal{H}} + \frac{7}{48}\mathcal{D}\bar{\mathcal{L}})E^{ij}P_b\gamma_b^{\dot{\alpha}\alpha}\nabla_a\Lambda_{\alpha j} + (\frac{1}{12}\mathcal{D}^\dagger\bar{\mathcal{H}} + \frac{1}{3}\mathcal{D}\mathcal{H})T_{bc}{}^{jk}\Lambda_{\alpha j}R(V)_{ab}{}^i{}_k\gamma_c^{\dot{\alpha}\alpha} + (\frac{1}{12}\mathcal{D}\mathcal{D}\mathcal{H} - \frac{2}{3}\mathcal{I})\Lambda_{\alpha j}\bar{P}_b\gamma_c^{\dot{\alpha}\alpha}\nabla_aT_{bc}{}^{ij} \\
& + (\frac{1}{12}\mathcal{D}\mathcal{D}\mathcal{H} + \frac{2}{3}\mathcal{I})T_{bc}{}^{ij}\bar{P}_b\gamma_c^{\dot{\alpha}\alpha}\nabla_a\Lambda_{\alpha j} + (\frac{3}{32}\bar{\mathcal{H}} + \frac{1}{32}\mathcal{H})E_{jk}E^{jl}\chi_{\alpha}{}^{ik}{}_l\gamma_a^{\dot{\alpha}\alpha} + (\frac{29}{288}\bar{\mathcal{H}} + \frac{43}{288}\mathcal{H})E_{jk}\Lambda^{\dot{\beta}j}\gamma_{ab}{}^{\dot{\alpha}}{}_{\dot{\beta}}\nabla_cT_{bc}{}^{ik} \\
& + (\frac{5}{48}\bar{\mathcal{H}} + \frac{7}{48}\mathcal{H})\Lambda_{\alpha j}\gamma_b^{\dot{\alpha}\alpha}\nabla_c\nabla_cT_{abkl}\varepsilon^{ijkl} + (\frac{1}{8}\bar{\mathcal{H}} - \frac{7}{24}\mathcal{H})T_{abjk}T_{bc}{}^{jl}\chi_{\alpha}{}^{ik}{}_l\gamma_c^{\dot{\alpha}\alpha} + (\frac{1}{8}\bar{\mathcal{H}} - \frac{1}{8}\mathcal{H})T_{abjk}R(Q)_{bc}{}^{\dot{\alpha}}{}_l\bar{P}_c\varepsilon^{ijkl} \\
& + (\frac{1}{8}\bar{\mathcal{H}} - \frac{1}{8}\mathcal{H})T_{abjk}\bar{P}_b\chi^{\dot{\beta}}{}_{lm}{}^i\varepsilon^{jklm} + (\frac{1}{8}\mathcal{D}^\dagger\bar{\mathcal{H}} + \frac{1}{4}\mathcal{D}\bar{\mathcal{L}})\Lambda^{\dot{\beta}i}\bar{P}_b\gamma_{ab}{}^{\dot{\alpha}}{}_{\dot{\beta}}\nabla_cP_c + (\frac{1}{8}\mathcal{D}^\dagger\bar{\mathcal{H}} + \frac{7}{24}\mathcal{D}\bar{\mathcal{L}})\chi^{\dot{\beta}}{}_{jk}{}^i\gamma_{ab}{}^{\dot{\alpha}}{}_{\dot{\beta}}\nabla_cT_{bclm}\varepsilon^{jklm} \\
& + (\frac{1}{8}\mathcal{D}^\dagger\bar{\mathcal{H}} + \frac{7}{24}\mathcal{D}\bar{\mathcal{L}})\chi^{\dot{\beta}}{}_{jk}{}^i\gamma_{bc}{}^{\dot{\alpha}}{}_{\dot{\beta}}\nabla_bT_{aclm}\varepsilon^{jklm} + (\frac{7}{48}\bar{\mathcal{H}} - \frac{9}{16}\mathcal{H})T_{ab}{}^{ij}\Lambda^{\dot{\alpha}k}\nabla_cT_{bc}{}^{lm}\varepsilon_{jklm} + (\frac{7}{48}\bar{\mathcal{H}} - \frac{9}{16}\mathcal{H})T_{ab}{}^{jk}\Lambda^{\dot{\alpha}l}\nabla_cT_{bc}{}^{im}\varepsilon_{jklm} \\
& + (\frac{7}{48}\mathcal{D}^\dagger\bar{\mathcal{H}} + \frac{1}{6}\mathcal{D}\bar{\mathcal{L}})P_a\bar{P}_b\gamma_{bc}{}^{\dot{\alpha}}{}_{\dot{\beta}}\nabla_c\Lambda^{\dot{\beta}i} + (\frac{7}{48}\mathcal{D}^\dagger\bar{\mathcal{H}} + \frac{3}{8}\mathcal{D}\bar{\mathcal{L}})P_b\bar{P}_c\gamma_{bc}{}^{\dot{\alpha}}{}_{\dot{\beta}}\nabla_a\Lambda^{\dot{\beta}i} + (\frac{1}{6}\bar{\mathcal{L}} - \frac{1}{24}\mathcal{D}^\dagger\bar{\mathcal{H}})P_b\Lambda^{\dot{\beta}j}R(V)_{bc}{}^i{}_j\gamma_{ac}{}^{\dot{\alpha}}{}_{\dot{\beta}} \\
& + (\frac{1}{6}\bar{\mathcal{H}} - \frac{19}{18}\mathcal{H})T_{bcjk}T_{ab}{}^{ij}\Lambda^{\dot{\alpha}k}\bar{P}_c + (\frac{1}{6}\bar{\mathcal{H}} - \frac{1}{2}\mathcal{H})T_{abjk}T_{cd}{}^{ij}R(Q)_{cda}{}^k\gamma_b^{\dot{\alpha}\alpha} + (\frac{1}{6}\bar{\mathcal{H}} - \frac{1}{6}\mathcal{H})P_bT_{ac}{}^{ij}\gamma_b^{\dot{\alpha}\alpha}\nabla_c\Lambda_{\alpha j} \\
& + (\frac{1}{6}\bar{\mathcal{H}} - \frac{1}{6}\mathcal{H})P_bT_{bc}{}^{ij}\gamma_c^{\dot{\alpha}\alpha}\nabla_a\Lambda_{\alpha j} + (\frac{1}{6}\bar{\mathcal{H}} - \frac{1}{6}\mathcal{H})P_bR(Q)_{aba}{}^i\bar{P}_c\gamma_c^{\dot{\alpha}\alpha} + (\frac{1}{6}\mathcal{D}^\dagger\bar{\mathcal{H}} + \frac{1}{12}\mathcal{D}\bar{\mathcal{L}})E^{jk}T_{abjl}\chi_{\alpha}{}^{il}{}_k\gamma_b^{\dot{\alpha}\alpha} \\
& + (\frac{1}{6}\mathcal{D}^\dagger\bar{\mathcal{H}} + \frac{5}{48}\mathcal{D}\bar{\mathcal{L}})E^{ij}\Lambda_{\alpha j}\gamma_a^{\dot{\alpha}\alpha}\nabla_bP_b + (\frac{1}{6}\mathcal{D}^\dagger\bar{\mathcal{H}} + \frac{1}{3}\mathcal{D}\bar{\mathcal{L}})E^{ij}T_{abkl}\chi_{\alpha}{}^{kl}{}_j\gamma_b^{\dot{\alpha}\alpha} + (\frac{1}{6}\mathcal{D}^\dagger\bar{\mathcal{H}} + \frac{1}{3}\mathcal{D}\bar{\mathcal{L}})P_b\bar{P}_b\gamma_{ac}{}^{\dot{\alpha}}{}_{\dot{\beta}}\nabla_c\Lambda^{\dot{\beta}i} \\
& + (\frac{1}{6}\mathcal{D}\mathcal{D}\mathcal{H} + \frac{2}{3}\mathcal{I})T_{ab}{}^{ij}\Lambda_{\alpha j}\gamma_c^{\dot{\alpha}\alpha}\nabla_b\bar{P}_c + (\frac{17}{96}\bar{\mathcal{H}} - \frac{5}{96}\mathcal{H})T_{ab}{}^{jk}\Lambda^{\dot{\alpha}i}\nabla_cT_{bc}{}^{lm}\varepsilon_{jklm} + (\frac{5}{24}\bar{\mathcal{H}} + \frac{1}{8}\mathcal{H})T_{abjk}T_{cd}{}^{jk}R(Q)_{cda}{}^i\gamma_b^{\dot{\alpha}\alpha} \\
& + (\frac{5}{24}\mathcal{D}^\dagger\bar{\mathcal{H}} - \frac{1}{24}\mathcal{D}\bar{\mathcal{L}})P_b\Lambda_{\alpha j}\gamma_a^{\dot{\alpha}\alpha}\nabla_bE^{ij} + (\frac{1}{4}\mathcal{D}^\dagger\bar{\mathcal{H}} + \frac{1}{8}\mathcal{D}\bar{\mathcal{L}})T_{bcjk}T_{ad}{}^{jk}\gamma_{bc}{}^{\dot{\alpha}}{}_{\dot{\beta}}\nabla_d\Lambda^{\dot{\beta}i} + (\frac{1}{4}\mathcal{D}^\dagger\bar{\mathcal{H}} + \frac{1}{6}\mathcal{D}\bar{\mathcal{L}})T_{bcjk}T_{ad}{}^{ij}\gamma_{bc}{}^{\dot{\alpha}}{}_{\dot{\beta}}\nabla_d\Lambda^{\dot{\beta}k} \\
& + (\frac{1}{4}\mathcal{D}^\dagger\bar{\mathcal{H}} - \frac{1}{3}\mathcal{D}\mathcal{H})T_{bc}{}^{ij}\Lambda_{\alpha k}R(V)_{ab}{}^k{}_j\gamma_c^{\dot{\alpha}\alpha} + (\frac{1}{4}\mathcal{D}\mathcal{D}\mathcal{H} + \frac{2}{3}\mathcal{I})\Lambda_{\alpha j}\bar{P}_b\gamma_b^{\dot{\alpha}\alpha}\nabla_cT_{ac}{}^{ij} + (\frac{1}{4}\mathcal{D}\mathcal{D}\mathcal{H} + \frac{2}{3}\mathcal{I})\Lambda_{\alpha j}\bar{P}_b\gamma_c^{\dot{\alpha}\alpha}\nabla_cT_{ab}{}^{ij} \\
& + (\frac{1}{4}\mathcal{D}\mathcal{D}\mathcal{H} + 2\mathcal{I})T_{ab}{}^{ij}\bar{P}_b\gamma_c^{\dot{\alpha}\alpha}\nabla_c\Lambda_{\alpha j} + (\frac{1}{4}\mathcal{D}\mathcal{D}\mathcal{H} + 2\mathcal{I})T_{ab}{}^{ij}\bar{P}_c\gamma_c^{\dot{\alpha}\alpha}\nabla_b\Lambda_{\alpha j} + (\frac{1}{4}\mathcal{D}\mathcal{D}\mathcal{H} + 2\mathcal{I})R(Q)_{aba}{}^i\bar{P}_b\bar{P}_c\gamma_c^{\dot{\alpha}\alpha} + 4\cdots
\end{aligned}$$

$$\begin{aligned}
[\hat{\Omega}_a^{\dot{\alpha}i}]_{1,cont.} = & + \left(\frac{7}{24} \bar{\mathcal{H}} + \frac{5}{24} \mathcal{H}\right) \Lambda_{\alpha j} \gamma_b^{\dot{\alpha}} \nabla_a \nabla_c T_{bckl} \varepsilon^{ijkl} + \left(\frac{7}{24} \mathcal{D}^\dagger \bar{\mathcal{I}} + \frac{1}{4} \mathcal{D} \mathcal{H}\right) T_{bc}{}^{jk} \Lambda_{\alpha j} R(V)_{bc}{}^i{}_k \gamma_a^{\dot{\alpha}} + \left(\frac{1}{3} \bar{\mathcal{I}} + \frac{1}{24} \mathcal{D}^\dagger \mathcal{D}^\dagger \bar{\mathcal{H}}\right) T_{abjk} \Lambda^{\dot{\alpha}l} \nabla_c T_{bclm} \varepsilon^{ijkm} \\
& + \left(\frac{1}{3} \bar{\mathcal{I}} + \frac{1}{24} \mathcal{D}^\dagger \mathcal{D}^\dagger \bar{\mathcal{H}}\right) T_{bcjk} \Lambda^{\dot{\alpha}l} \nabla_b T_{aclm} \varepsilon^{ijkm} + \left(\frac{1}{3} \mathcal{D}^\dagger \bar{\mathcal{H}} + \frac{1}{6} \mathcal{D} \bar{\mathcal{I}}\right) T_{bcjk} T_{ab}{}^{jk} \gamma_{cd}{}^{\dot{\alpha}}{}_{\dot{\beta}} \nabla_d \Lambda^{\dot{\beta}i} + \left(\frac{1}{3} \mathcal{D}^\dagger \bar{\mathcal{H}} + \frac{11}{12} \mathcal{D} \bar{\mathcal{I}}\right) T_{bcjk} \Lambda^{\dot{\beta}i} \gamma_{bd}{}^{\dot{\alpha}}{}_{\dot{\beta}} \nabla_c T_{ad}{}^{jk} \\
& + \left(\frac{17}{48} \mathcal{D}^\dagger \bar{\mathcal{H}} + \frac{3}{4} \mathcal{D} \bar{\mathcal{I}}\right) P_b \bar{P}_c \gamma_{ab}{}^{\dot{\alpha}}{}_{\dot{\beta}} \nabla_c \Lambda^{\dot{\beta}i} + \left(\frac{3}{8} \bar{\mathcal{H}} - \frac{7}{8} \mathcal{H}\right) T_{bcjk} T_{ab}{}^{jl} \chi_a{}^{ik}{}_l \gamma_c^{\dot{\alpha}} + \left(\frac{3}{8} \mathcal{D}^\dagger \bar{\mathcal{H}} + \frac{3}{4} \mathcal{D} \bar{\mathcal{I}}\right) \Lambda^{\dot{\beta}i} \bar{P}_b \gamma_{ac}{}^{\dot{\alpha}}{}_{\dot{\beta}} \nabla_b P_c \\
& + \left(\frac{1}{2} \bar{\mathcal{I}} + \frac{1}{8} \mathcal{D}^\dagger \mathcal{D}^\dagger \bar{\mathcal{H}}\right) P_b T_{acjk} R(Q)_{bc}{}^{\dot{\alpha}}{}_l \varepsilon^{ijkl} + \left(\frac{2}{3} \bar{\mathcal{I}} + \frac{1}{24} \mathcal{D}^\dagger \mathcal{D}^\dagger \bar{\mathcal{H}}\right) T_{abjk} T_{bclm} \nabla_c \Lambda^{\dot{\alpha}l} \varepsilon^{ijkm} + \left(\frac{2}{3} \mathcal{D}^\dagger \bar{\mathcal{H}} + \frac{2}{3} \mathcal{D} \bar{\mathcal{I}}\right) T_{bcjk} T_{ab}{}^{ij} \gamma_{cd}{}^{\dot{\alpha}}{}_{\dot{\beta}} \nabla_d \Lambda^{\dot{\beta}k} \\
& + \left(\frac{3}{4} \bar{\mathcal{I}} + \frac{1}{16} \mathcal{D}^\dagger \mathcal{D}^\dagger \bar{\mathcal{H}}\right) P_b \Lambda^{\dot{\beta}i} R(M)_{abcd} \gamma_{cd}{}^{\dot{\alpha}}{}_{\dot{\beta}} + \left(\frac{5}{6} \bar{\mathcal{H}} - \frac{5}{18} \mathcal{H}\right) T_{bcjk} T_{ab}{}^{jk} \Lambda^{\dot{\alpha}i} \bar{P}_c - \frac{1}{16} E_{jk} E_{lm} \mathcal{D} \mathcal{H} \chi_a{}^{jl}{}_n \gamma_a^{\dot{\alpha}} \varepsilon^{ikmn} \\
& + \frac{1}{24} E_{jk} P_b T_{ac}{}^{ij} \mathcal{D} \bar{\mathcal{I}} \Lambda^{\dot{\beta}k} \gamma_{bc}{}^{\dot{\alpha}}{}_{\dot{\beta}} + \frac{1}{48} E_{jk} \mathcal{D}^\dagger \bar{\mathcal{I}} \bar{P}_b \chi^{\dot{\beta}}{}_{lm}{}^j \gamma_{ab}{}^{\dot{\alpha}}{}_{\dot{\beta}} \varepsilon^{iklm} + \frac{1}{24} E^{ij} T_{abjk} \mathcal{D} \bar{\mathcal{I}} \Lambda^{\dot{\beta}k} \bar{P}_c \gamma_{bc}{}^{\dot{\alpha}}{}_{\dot{\beta}} + \frac{1}{24} E^{ij} T_{bcjk} \mathcal{D} \bar{\mathcal{I}} \Lambda^{\dot{\beta}k} \bar{P}_b \gamma_{ac}{}^{\dot{\alpha}}{}_{\dot{\beta}} \\
& + \frac{1}{48} E^{ij} T_{ab}{}^{kl} \mathcal{D} \bar{\mathcal{I}} \gamma_{bc}{}^{\dot{\alpha}}{}_{\dot{\beta}} \nabla_c \Lambda^{\dot{\beta}m} \varepsilon_{jklm} + \frac{1}{6} P_a P_b T_{bc}{}^{ij} \mathcal{D} \bar{\mathcal{I}} \Lambda_{\alpha j} \gamma_c^{\dot{\alpha}} + \frac{1}{6} P_b P_c T_{ab}{}^{ij} \mathcal{D} \bar{\mathcal{I}} \Lambda_{\alpha j} \gamma_c^{\dot{\alpha}} - \frac{1}{72} P_a T_{bcjk} \mathcal{D} \bar{\mathcal{I}} \gamma_b^{\dot{\alpha}} \nabla_c \Lambda_{\alpha l} \varepsilon^{ijkl} \\
& + \frac{13}{72} P_b T_{abjk} \mathcal{D} \bar{\mathcal{I}} \gamma_c^{\dot{\alpha}} \nabla_c \Lambda_{\alpha l} \varepsilon^{ijkl} + \frac{1}{72} P_b T_{acjk} \mathcal{D} \bar{\mathcal{I}} \gamma_b^{\dot{\alpha}} \nabla_c \Lambda_{\alpha l} \varepsilon^{ijkl} + \frac{5}{72} P_b T_{acjk} \mathcal{D} \bar{\mathcal{I}} \gamma_c^{\dot{\alpha}} \nabla_b \Lambda_{\alpha l} \varepsilon^{ijkl} - \frac{5}{24} P_b T_{bcjk} \mathcal{D} \bar{\mathcal{I}} \gamma_c^{\dot{\alpha}} \nabla_a \Lambda_{\alpha l} \varepsilon^{ijkl} \\
& + \frac{1}{8} T_{abjk} T_{bclm} \mathcal{D} \bar{\mathcal{I}} \chi_a{}^{jk}{}_n \gamma_c^{\dot{\alpha}} \varepsilon^{ilmn} - \frac{1}{8} T_{abjk} T_{bclm} \mathcal{D} \bar{\mathcal{I}} \chi_a{}^{lm}{}_n \gamma_c^{\dot{\alpha}} \varepsilon^{ijkn} + \frac{1}{8} T_{abjk} \mathcal{D}^\dagger \bar{\mathcal{I}} \Lambda_{\alpha l} \gamma_c^{\dot{\alpha}} \nabla_b \bar{P}_c \varepsilon^{ijkl} \\
& - \frac{5}{24} T_{abjk} \mathcal{D}^\dagger \bar{\mathcal{I}} \Lambda_{\alpha l} \gamma_c^{\dot{\alpha}} \nabla_c \bar{P}_b \varepsilon^{ijkl} + \frac{1}{24} T_{bcjk} \mathcal{D}^\dagger \bar{\mathcal{I}} \Lambda_{\alpha l} \gamma_b^{\dot{\alpha}} \nabla_a \bar{P}_c \varepsilon^{ijkl} - \frac{1}{8} T_{bcjk} \mathcal{D}^\dagger \bar{\mathcal{I}} \Lambda_{\alpha l} \gamma_b^{\dot{\alpha}} \nabla_c \bar{P}_a \varepsilon^{ijkl} \\
& - \frac{1}{12} T_{abjk} \mathcal{D}^\dagger \bar{\mathcal{I}} \bar{P}_b \gamma_c^{\dot{\alpha}} \nabla_c \Lambda_{\alpha l} \varepsilon^{ijkl} - \frac{5}{12} T_{abjk} \mathcal{D}^\dagger \bar{\mathcal{I}} \bar{P}_c \gamma_b^{\dot{\alpha}} \nabla_c \Lambda_{\alpha l} \varepsilon^{ijkl} - \frac{1}{12} T_{abjk} \mathcal{D}^\dagger \bar{\mathcal{I}} \bar{P}_c \gamma_c^{\dot{\alpha}} \nabla_b \Lambda_{\alpha l} \varepsilon^{ijkl} \\
& - \frac{1}{12} T_{bcjk} \mathcal{D}^\dagger \bar{\mathcal{I}} \bar{P}_a \gamma_b^{\dot{\alpha}} \nabla_c \Lambda_{\alpha l} \varepsilon^{ijkl} + \frac{1}{12} T_{bcjk} \mathcal{D}^\dagger \bar{\mathcal{I}} \bar{P}_b \gamma_c^{\dot{\alpha}} \nabla_a \Lambda_{\alpha l} \varepsilon^{ijkl} - \frac{7}{288} T_{abjk} \mathcal{D} \bar{\mathcal{I}} \Lambda^{\dot{\beta}l} \gamma_{bc}{}^{\dot{\alpha}}{}_{\dot{\beta}} \nabla_c E_{lm} \varepsilon^{ijkm} \\
& + \frac{7}{288} T_{bcjk} \mathcal{D} \bar{\mathcal{I}} \Lambda^{\dot{\beta}l} \gamma_{ab}{}^{\dot{\alpha}}{}_{\dot{\beta}} \nabla_c E_{lm} \varepsilon^{ijkm} + \frac{1}{64} T_{bcjk} \mathcal{D} \bar{\mathcal{I}} \Lambda^{\dot{\beta}l} \gamma_{bc}{}^{\dot{\alpha}}{}_{\dot{\beta}} \nabla_a E_{lm} \varepsilon^{ijkm} - \frac{61}{576} T_{bc}{}^{jk} T_{bc}{}^{lm} \mathcal{D}^\dagger \bar{\mathcal{I}} \Lambda^{\dot{\alpha}i} \bar{P}_a \varepsilon_{jklm} \\
& + \frac{1}{6} T_{ab}{}^{jk} T_{cd}{}^{lm} \mathcal{D}^\dagger \bar{\mathcal{I}} R(Q)_{cd\alpha}{}^i \gamma_b^{\dot{\alpha}} \varepsilon_{jklm} - \frac{5}{4} \bar{\mathcal{I}} P_b P_b \Lambda^{\dot{\beta}i} \bar{P}_c \gamma_{ac}{}^{\dot{\alpha}}{}_{\dot{\beta}} + \frac{1}{3} \bar{\mathcal{I}} P_a T_{bcjk} \chi^{\dot{\beta}}{}_{lm}{}^i \gamma_{bc}{}^{\dot{\alpha}}{}_{\dot{\beta}} \varepsilon^{jklm} - \frac{1}{6} \bar{\mathcal{I}} T_{bcjk} T_{bdlm} \gamma_{cd}{}^{\dot{\alpha}}{}_{\dot{\beta}} \nabla_a \Lambda^{\dot{\beta}j} \varepsilon^{iklm} \\
& + \frac{1}{6} \bar{\mathcal{I}} T_{bcjk} T_{bdlm} \gamma_{cd}{}^{\dot{\alpha}}{}_{\dot{\beta}} \nabla_a \Lambda^{\dot{\beta}l} \varepsilon^{ijkm} + \frac{1}{24} \bar{\mathcal{I}} T_{bcjk} \Lambda^{\dot{\beta}i} \gamma_{bd}{}^{\dot{\alpha}}{}_{\dot{\beta}} \nabla_a T_{cdlm} \varepsilon^{jklm} + \frac{1}{6} \bar{\mathcal{I}} T_{bcjk} \Lambda^{\dot{\beta}j} \gamma_{ad}{}^{\dot{\alpha}}{}_{\dot{\beta}} \nabla_d T_{bclm} \varepsilon^{iklm} \\
& + \frac{1}{4} \bar{\mathcal{I}} T_{bcjk} \Lambda^{\dot{\beta}j} \gamma_{bd}{}^{\dot{\alpha}}{}_{\dot{\beta}} \nabla_a T_{cdlm} \varepsilon^{iklm} - \frac{1}{6} \bar{\mathcal{I}} T_{bcjk} \Lambda^{\dot{\beta}l} \gamma_{ad}{}^{\dot{\alpha}}{}_{\dot{\beta}} \nabla_d T_{bclm} \varepsilon^{ijkm} - \frac{1}{4} \bar{\mathcal{I}} T_{bcjk} \Lambda^{\dot{\beta}l} \gamma_{bd}{}^{\dot{\alpha}}{}_{\dot{\beta}} \nabla_a T_{cdlm} \varepsilon^{ijkm} \\
& - \frac{1}{24} \bar{\mathcal{H}} E_{jk} E^{kl} E^{\dot{\alpha}i} \Lambda_{\alpha l} \gamma_a^{\dot{\alpha}} + \frac{1}{6} \mathcal{D}^\dagger \bar{\mathcal{I}} E^{ij} P_a T_{bcjk} \Lambda^{\dot{\beta}k} \gamma_{bc}{}^{\dot{\alpha}}{}_{\dot{\beta}} - \frac{1}{4} \mathcal{D}^\dagger \bar{\mathcal{I}} P_a T_{bcjk} T_{bclm} \Lambda^{\dot{\alpha}i} \varepsilon^{jklm} + \frac{1}{24} \mathcal{D}^\dagger \bar{\mathcal{H}} E_{jk} P_b \chi^{\dot{\beta}}{}_{lm}{}^j \gamma_{ab}{}^{\dot{\alpha}}{}_{\dot{\beta}} \varepsilon^{iklm} \\
& + \frac{5}{96} \mathcal{D}^\dagger \bar{\mathcal{H}} P_a T_{bc}{}^{jk} T_{bc}{}^{lm} \Lambda^{\dot{\alpha}i} \varepsilon_{jklm} + \frac{1}{2} \mathcal{D}^\dagger \mathcal{D}^\dagger \bar{\mathcal{I}} P_b P_b P_c \Lambda^{\dot{\beta}i} \gamma_{ac}{}^{\dot{\alpha}}{}_{\dot{\beta}} - \frac{1}{48} \mathcal{D}^\dagger \mathcal{D}^\dagger \bar{\mathcal{H}} E_{jk} E^{jk} P_b \Lambda^{\dot{\beta}i} \gamma_{ab}{}^{\dot{\alpha}}{}_{\dot{\beta}} + \frac{1}{8} \mathcal{D}^\dagger \mathcal{D}^\dagger \bar{\mathcal{H}} E^{ij} P_b T_{ab}{}^{kl} \Lambda^{\dot{\alpha}m} \varepsilon_{jklm} \\
& - \frac{1}{16} \mathcal{D}^\dagger \bar{\mathcal{I}} \Lambda_{\alpha j} \bar{P}_b \gamma_c^{\dot{\alpha}} \nabla_d E^{ij} \varepsilon_{abcd} + \frac{1}{24} \mathcal{D}^\dagger \bar{\mathcal{I}} \Lambda_{\alpha j} \bar{P}_b \gamma_a^{\dot{\alpha}} \nabla_c T_{bckl} \varepsilon^{ijkl} - \frac{1}{8} \mathcal{D}^\dagger \bar{\mathcal{I}} \Lambda_{\alpha j} \bar{P}_b \gamma_c^{\dot{\alpha}} \nabla_b T_{ackl} \varepsilon^{ijkl} \\
& + \frac{1}{6} \mathcal{D} \mathcal{D} \mathcal{H} E_{jk} T_{bc}{}^{ij} T_{bc}{}^{kl} \Lambda_{\alpha l} \gamma_a^{\dot{\alpha}} - \frac{1}{3} \mathcal{H} T_{abjk} \Lambda_{\alpha l} R(V)_{bc}{}^i{}_m \gamma_c^{\dot{\alpha}} \varepsilon^{jklm} - \frac{1}{12} \mathcal{H} T_{bc}{}^{ij} \Lambda^{\dot{\beta}k} \gamma_{ad}{}^{\dot{\alpha}}{}_{\dot{\beta}} \nabla_d T_{bc}{}^{lm} \varepsilon_{jklm} \\
& - \frac{1}{12} \mathcal{H} T_{bc}{}^{jk} \Lambda^{\dot{\beta}l} \gamma_{ad}{}^{\dot{\alpha}}{}_{\dot{\beta}} \nabla_d T_{bc}{}^{im} \varepsilon_{jklm} + \left(-\frac{9}{4} \bar{\mathcal{I}} - \frac{1}{48} \mathcal{D}^\dagger \mathcal{D}^\dagger \bar{\mathcal{H}}\right) P_b P_c \Lambda^{\dot{\beta}i} \bar{P}_b \gamma_{ac}{}^{\dot{\alpha}}{}_{\dot{\beta}} + \left(-\frac{3}{4} \mathcal{D}^\dagger \bar{\mathcal{I}} + \frac{1}{3} \mathcal{D} \mathcal{H}\right) P_b T_{bc}{}^{ij} \Lambda_{\alpha j} \bar{P}_c \gamma_a^{\dot{\alpha}} \\
& + \left(-\frac{2}{3} \bar{\mathcal{H}} - \frac{2}{9} \mathcal{H}\right) T_{bcjk} T_{ab}{}^{ij} \Lambda^{\dot{\beta}k} \bar{P}_d \gamma_{cd}{}^{\dot{\alpha}}{}_{\dot{\beta}} + \left(-\frac{2}{3} \bar{\mathcal{H}} + \frac{2}{9} \mathcal{H}\right) T_{bcjk} T_{ab}{}^{jk} \Lambda^{\dot{\beta}i} \bar{P}_d \gamma_{cd}{}^{\dot{\alpha}}{}_{\dot{\beta}} + \left(-\frac{1}{2} \bar{\mathcal{I}} - \frac{1}{16} \mathcal{D}^\dagger \mathcal{D}^\dagger \bar{\mathcal{H}}\right) P_a P_b \Lambda^{\dot{\beta}i} \bar{P}_c \gamma_{bc}{}^{\dot{\alpha}}{}_{\dot{\beta}} \\
& + \left(-\frac{1}{2} \mathcal{D}^\dagger \bar{\mathcal{I}} - \frac{1}{24} \mathcal{D}^\dagger \mathcal{D}^\dagger \mathcal{D}^\dagger \bar{\mathcal{H}}\right) P_b T_{acjk} T_{bclm} \Lambda^{\dot{\alpha}l} \varepsilon^{ijkm} + \left(-\frac{1}{2} \mathcal{D}^\dagger \bar{\mathcal{I}} + \frac{1}{4} \mathcal{D} \mathcal{H}\right) T_{bcjk} T_{ad}{}^{ij} T_{bd}{}^{kl} \Lambda_{\alpha l} \gamma_c^{\dot{\alpha}} \\
& + \left(-\frac{1}{2} \mathcal{D}^\dagger \bar{\mathcal{I}} + \frac{1}{4} \mathcal{D} \mathcal{H}\right) T_{bcjk} T_{ad}{}^{jl} T_{bd}{}^{ik} \Lambda_{\alpha l} \gamma_c^{\dot{\alpha}} + \left(-\frac{11}{24} \mathcal{D}^\dagger \bar{\mathcal{I}} - \frac{1}{6} \mathcal{D} \mathcal{H}\right) \Lambda_{\alpha j} \bar{P}_b \gamma_b^{\dot{\alpha}} \nabla_c T_{ackl} \varepsilon^{ijkl} \\
& + \left(-\frac{5}{12} \mathcal{D}^\dagger \bar{\mathcal{I}} - \frac{1}{3} \mathcal{D} \mathcal{H}\right) P_b T_{bc}{}^{ij} \Lambda_{\alpha j} \bar{P}_a \gamma_c^{\dot{\alpha}} + \left(-\frac{29}{72} \mathcal{D}^\dagger \bar{\mathcal{I}} + \frac{1}{6} \mathcal{D} \mathcal{H}\right) T_{ab}{}^{jk} T_{bc}{}^{il} \Lambda^{\dot{\alpha}m} \bar{P}_c \varepsilon_{jklm} \\
& + \left(-\frac{1}{3} \bar{\mathcal{I}} - \frac{1}{48} \mathcal{D}^\dagger \mathcal{D}^\dagger \bar{\mathcal{H}}\right) P_b T_{acjk} \chi^{\dot{\beta}}{}_{lm}{}^i \gamma_{bc}{}^{\dot{\alpha}}{}_{\dot{\beta}} \varepsilon^{jklm} + \left(-\frac{1}{3} \bar{\mathcal{I}} + \frac{1}{6} \mathcal{D}^\dagger \mathcal{D}^\dagger \bar{\mathcal{H}}\right) P_b T_{cdjk} T_{ab}{}^{ij} \Lambda^{\dot{\beta}k} \gamma_{cd}{}^{\dot{\alpha}}{}_{\dot{\beta}} + 5 \dots
\end{aligned}$$

$$\begin{aligned}
[\hat{\Omega}_a^{\dot{\alpha}i}]_{1,cont.} = & +(-\frac{1}{3}\mathcal{D}^\dagger\bar{\mathcal{H}} - \frac{13}{36}\mathcal{D}\bar{\mathcal{I}})T_{bcjk}\Lambda_{\alpha l}\gamma_a^{\dot{\alpha}\alpha}\nabla_b P_c\varepsilon^{ijkl} + (-\frac{1}{3}\mathcal{D}^\dagger\bar{\mathcal{H}} + \frac{1}{2}\mathcal{D}\bar{\mathcal{I}})P_bP_bT_{ac}^{ij}\Lambda_{\alpha j}\gamma_c^{\dot{\alpha}\alpha} + (-\frac{1}{3}\mathcal{D}^\dagger\bar{\mathcal{I}} - \frac{1}{2}\mathcal{D}\mathcal{H})T_{abjk}T_{cd}^{ij}T_{cd}^{kl}\Lambda_{\alpha l}\gamma_b^{\dot{\alpha}\alpha} \\
& + (-\frac{7}{24}\mathcal{D}\mathcal{D}\mathcal{H} + \frac{2}{3}\mathcal{I})E_{jk}T_{ab}^{jl}T_{bc}^{ik}\Lambda_{\alpha l}\gamma_c^{\dot{\alpha}\alpha} + (-\frac{13}{48}\bar{\mathcal{H}} - \frac{7}{48}\mathcal{H})T_{bcjk}\Lambda_{\alpha l}R(M)_{adbc}\gamma_d^{\dot{\alpha}\alpha}\varepsilon^{ijkl} \\
& + (-\frac{1}{4}\bar{\mathcal{I}} - \frac{1}{96}\mathcal{D}^\dagger\mathcal{D}^\dagger\bar{\mathcal{H}})T_{bcjk}\Lambda^{\dot{\beta}i}\gamma_{ad}^{\dot{\alpha}}\nabla_d T_{bclm}\varepsilon^{jklm} + (-\frac{1}{4}\bar{\mathcal{H}} - \frac{1}{12}\mathcal{H})T_{bcjk}T_{ad}^{jk}\Lambda^{\dot{\beta}i}\bar{P}_d\gamma_{bc}^{\dot{\alpha}}\nabla_{\dot{\beta}} \\
& + (-\frac{1}{4}\mathcal{D}^\dagger\bar{\mathcal{H}} + \frac{1}{18}\mathcal{D}\bar{\mathcal{I}})P_b\Lambda_{\alpha j}\gamma_b^{\dot{\alpha}\alpha}\nabla_c T_{ackl}\varepsilon^{ijkl} + (-\frac{1}{4}\mathcal{D}^\dagger\bar{\mathcal{H}} + \frac{1}{12}\mathcal{D}\bar{\mathcal{I}})P_b\Lambda_{\alpha j}\gamma_c^{\dot{\alpha}\alpha}\nabla_a T_{bckl}\varepsilon^{ijkl} \\
& + (-\frac{1}{4}\mathcal{D}^\dagger\bar{\mathcal{H}} + \frac{2}{9}\mathcal{D}\bar{\mathcal{I}})P_b\Lambda_{\alpha j}\gamma_c^{\dot{\alpha}\alpha}\nabla_c T_{abkl}\varepsilon^{ijkl} + (-\frac{1}{4}\mathcal{D}^\dagger\bar{\mathcal{I}} - \frac{1}{3}\mathcal{D}\mathcal{H})P_aT_{bc}^{ij}\Lambda_{\alpha j}\bar{P}_b\gamma_c^{\dot{\alpha}\alpha} \\
& + (-\frac{1}{4}\mathcal{D}^\dagger\bar{\mathcal{I}} - \frac{1}{6}\mathcal{D}\mathcal{H})T_{abjk}T_{cd}^{il}T_{cd}^{jk}\Lambda_{\alpha l}\gamma_b^{\dot{\alpha}\alpha} + (-\frac{5}{24}\bar{\mathcal{H}} - \frac{1}{8}\mathcal{H})T_{bcjk}T_{ad}^{ij}\Lambda^{\dot{\beta}k}\bar{P}_d\gamma_{bc}^{\dot{\alpha}}\nabla_{\dot{\beta}} + (-\frac{1}{6}\bar{\mathcal{I}} - \frac{1}{48}\mathcal{D}^\dagger\mathcal{D}^\dagger\bar{\mathcal{H}})E^{ij}P_aP_b\Lambda_{\alpha j}\gamma_b^{\dot{\alpha}\alpha} \\
& + (-\frac{1}{6}\bar{\mathcal{I}} + \frac{1}{96}\mathcal{D}^\dagger\mathcal{D}^\dagger\bar{\mathcal{H}})T_{abjk}T_{cdlm}\gamma_{cd}^{\dot{\alpha}}\nabla_b\Lambda^{\dot{\beta}j}\varepsilon^{iklm} + (-\frac{1}{6}\bar{\mathcal{I}} + \frac{1}{96}\mathcal{D}^\dagger\mathcal{D}^\dagger\bar{\mathcal{H}})T_{abjk}\Lambda^{\dot{\beta}j}\gamma_{cd}^{\dot{\alpha}}\nabla_b T_{cdlm}\varepsilon^{iklm} \\
& + (-\frac{1}{6}\bar{\mathcal{I}} + \frac{1}{48}\mathcal{D}^\dagger\mathcal{D}^\dagger\bar{\mathcal{H}})E_{jk}E^{ij}P_b\Lambda^{\dot{\beta}k}\gamma_{ab}^{\dot{\alpha}}\nabla_{\dot{\beta}} + (-\frac{1}{6}\bar{\mathcal{I}} + \frac{3}{16}\mathcal{D}^\dagger\mathcal{D}^\dagger\bar{\mathcal{H}})P_bT_{cdjk}T_{ab}^{jk}\Lambda^{\dot{\beta}i}\gamma_{cd}^{\dot{\alpha}}\nabla_{\dot{\beta}} \\
& + (-\frac{1}{6}\mathcal{D}^\dagger\bar{\mathcal{H}} - \frac{1}{12}\mathcal{D}\bar{\mathcal{I}})T_{abjk}T_{bclm}\Lambda^{\dot{\alpha}l}\bar{P}_c\varepsilon^{ijkl} + (-\frac{1}{6}\mathcal{D}^\dagger\bar{\mathcal{H}} - \frac{5}{72}\mathcal{D}\bar{\mathcal{I}})T_{abjk}\Lambda_{\alpha l}\gamma_c^{\dot{\alpha}\alpha}\nabla_c P_b\varepsilon^{ijkl} \\
& + (-\frac{1}{6}\mathcal{D}^\dagger\bar{\mathcal{H}} + \frac{1}{72}\mathcal{D}\bar{\mathcal{I}})T_{abjk}\Lambda_{\alpha l}\gamma_c^{\dot{\alpha}\alpha}\nabla_b P_c\varepsilon^{ijkl} + (-\frac{1}{6}\mathcal{D}^\dagger\bar{\mathcal{I}} + \frac{1}{12}\mathcal{D}\mathcal{H})T_{abjk}T_{cd}^{ij}T_{bc}^{kl}\Lambda_{\alpha l}\gamma_d^{\dot{\alpha}\alpha} \\
& + (-\frac{1}{6}\mathcal{D}^\dagger\bar{\mathcal{I}} + \frac{1}{12}\mathcal{D}\mathcal{H})T_{bcjk}T_{bd}^{ij}T_{cd}^{kl}\Lambda_{\alpha l}\gamma_a^{\dot{\alpha}\alpha} + (-\frac{1}{6}\mathcal{D}^\dagger\bar{\mathcal{I}} + \frac{1}{3}\mathcal{D}\mathcal{H})T_{abjk}T_{cd}^{il}T_{bc}^{jk}\Lambda_{\alpha l}\gamma_d^{\dot{\alpha}\alpha} + (-\frac{25}{192}\bar{\mathcal{H}} + \frac{3}{64}\mathcal{H})E^{ij}P_a\Lambda_{\alpha j}\bar{P}_b\gamma_b^{\dot{\alpha}\alpha} \\
& + (-\frac{1}{8}\bar{\mathcal{H}} - \frac{1}{24}\mathcal{H})T_{bcjk}\Lambda_{\alpha l}R(V)_{ab}{}^i{}_m\gamma_c^{\dot{\alpha}\alpha}\varepsilon^{jklm} + (-\frac{1}{8}\mathcal{D}^\dagger\bar{\mathcal{H}} - \frac{1}{16}\mathcal{D}\bar{\mathcal{I}})T_{bc}^{jk}\Lambda^{\dot{\beta}l}\gamma_{ab}^{\dot{\alpha}}\nabla_c E^{im}\varepsilon_{jklm} \\
& + (-\frac{1}{8}\mathcal{D}^\dagger\bar{\mathcal{I}} - \frac{1}{6}\mathcal{D}\mathcal{H})T_{bcjk}\Lambda_{\alpha l}\gamma_a^{\dot{\alpha}\alpha}\nabla_b\bar{P}_c\varepsilon^{ijkl} + (-\frac{11}{96}\bar{\mathcal{H}} - \frac{1}{96}\mathcal{H})T_{ab}^{jk}T_{cd}^{lm}\gamma_{bc}^{\dot{\alpha}}\nabla_d\Lambda^{\dot{\beta}i}\varepsilon_{jklm} \\
& + (-\frac{5}{48}\mathcal{D}^\dagger\bar{\mathcal{H}} - \frac{7}{48}\mathcal{D}\bar{\mathcal{I}})T_{bcjk}T_{bclm}\Lambda^{\dot{\alpha}i}\bar{P}_a\varepsilon^{jklm} + (-\frac{17}{192}\bar{\mathcal{H}} + \frac{5}{192}\mathcal{H})E^{jk}\Lambda_{\alpha j}R(V)_{bc}{}^i{}_k\gamma_d^{\dot{\alpha}\alpha}\varepsilon_{abcd} \\
& + (-\frac{1}{12}\bar{\mathcal{I}} - \frac{1}{192}\mathcal{D}^\dagger\mathcal{D}^\dagger\bar{\mathcal{H}})T_{bcjk}T_{bclm}\gamma_{ad}^{\dot{\alpha}}\nabla_d\Lambda^{\dot{\beta}i}\varepsilon^{jklm} + (-\frac{1}{12}\bar{\mathcal{I}} + \frac{1}{96}\mathcal{D}^\dagger\mathcal{D}^\dagger\bar{\mathcal{H}})T_{bcjk}\Lambda^{\dot{\beta}l}\gamma_{bc}^{\dot{\alpha}}\nabla_d T_{adlm}\varepsilon^{jklm} \\
& + (-\frac{1}{12}\bar{\mathcal{I}} + \frac{1}{64}\mathcal{D}^\dagger\mathcal{D}^\dagger\bar{\mathcal{H}})T_{abjk}T_{cdlm}\gamma_{cd}^{\dot{\alpha}}\nabla_b\Lambda^{\dot{\beta}i}\varepsilon^{jklm} + (-\frac{1}{12}\bar{\mathcal{I}} + \frac{11}{96}\mathcal{D}^\dagger\mathcal{D}^\dagger\bar{\mathcal{H}})E^{ij}P_bP_b\Lambda_{\alpha j}\gamma_a^{\dot{\alpha}\alpha} \\
& + (-\frac{1}{12}\mathcal{D}^\dagger\bar{\mathcal{I}} - \frac{1}{48}\mathcal{D}^\dagger\mathcal{D}^\dagger\bar{\mathcal{H}})E^{ij}P_bT_{acjk}\Lambda^{\dot{\beta}k}\gamma_{bc}^{\dot{\alpha}}\nabla_{\dot{\beta}} + (-\frac{1}{12}\mathcal{D}^\dagger\bar{\mathcal{H}} - \frac{11}{48}\mathcal{D}\bar{\mathcal{I}})E^{ij}P_b\gamma_c^{\dot{\alpha}\alpha}\nabla_d\Lambda_{\alpha j}\varepsilon_{abcd} \\
& + (-\frac{1}{12}\mathcal{D}^\dagger\bar{\mathcal{H}} - \frac{1}{12}\mathcal{D}\bar{\mathcal{I}})P_bT_{ac}^{ij}T_{bc}^{kl}\Lambda^{\dot{\alpha}m}\varepsilon_{jklm} + (-\frac{1}{12}\mathcal{D}^\dagger\bar{\mathcal{I}} - \frac{1}{12}\mathcal{D}\mathcal{H})E_{jk}E^{jk}T_{ab}^{il}\Lambda_{\alpha l}\gamma_b^{\dot{\alpha}\alpha} \\
& + (-\frac{1}{12}\mathcal{D}^\dagger\bar{\mathcal{I}} + \frac{1}{8}\mathcal{D}\mathcal{H})T_{bc}^{ij}T_{bc}^{kl}\chi_{\alpha}{}^{mn}{}_j\gamma_a^{\dot{\alpha}\alpha}\varepsilon_{klmn} + (-\frac{1}{12}\mathcal{D}^\dagger\bar{\mathcal{I}} + \frac{1}{4}\mathcal{D}\mathcal{H})T_{ab}^{ij}T_{bc}^{kl}\chi_{\alpha}{}^{mn}{}_j\gamma_c^{\dot{\alpha}\alpha}\varepsilon_{klmn} \\
& + (-\frac{1}{12}\mathcal{D}\mathcal{D}\mathcal{D}\mathcal{H} - \frac{1}{3}\mathcal{D}\mathcal{I})T_{ab}^{ij}\Lambda_{\alpha j}\bar{P}_c\bar{P}_c\gamma_b^{\dot{\alpha}\alpha} + (-\frac{7}{96}\bar{\mathcal{H}} + \frac{1}{32}\mathcal{H})D^{ij}{}_{kl}T_{abmn}\Lambda_{\alpha j}\gamma_b^{\dot{\alpha}\alpha}\varepsilon^{klmn} \\
& + (-\frac{1}{16}\bar{\mathcal{H}} - \frac{3}{16}\mathcal{H})E_{jk}T_{ablm}\chi_{\alpha}{}^{ij}{}_n\gamma_b^{\dot{\alpha}\alpha}\varepsilon^{klmn} + (-\frac{1}{16}\bar{\mathcal{H}} - \frac{1}{8}\mathcal{H})T_{ab}^{ij}T_{cd}^{kl}\gamma_{bc}^{\dot{\alpha}}\nabla_d\Lambda^{\dot{\beta}m}\varepsilon_{jklm} \\
& + (-\frac{5}{96}\bar{\mathcal{H}} - \frac{7}{96}\mathcal{H})E^{jk}T_{ab}^{il}\chi_{\alpha}{}^{mn}{}_j\gamma_b^{\dot{\alpha}\alpha}\varepsilon_{klmn} + (-\frac{1}{24}\bar{\mathcal{I}} + \frac{1}{64}\mathcal{D}^\dagger\mathcal{D}^\dagger\bar{\mathcal{H}})T_{bcjk}\Lambda^{\dot{\beta}i}\gamma_{bc}^{\dot{\alpha}}\nabla_d T_{adlm}\varepsilon^{jklm} \\
& + (-\frac{1}{24}\bar{\mathcal{H}} - \frac{1}{8}\mathcal{H})E^{ij}P_b\Lambda_{\alpha j}\bar{P}_b\gamma_a^{\dot{\alpha}\alpha} + (-\frac{1}{24}\mathcal{D}^\dagger\bar{\mathcal{H}} - \frac{1}{12}\mathcal{D}\bar{\mathcal{I}})P_b\Lambda_{\alpha j}\gamma_c^{\dot{\alpha}\alpha}\nabla_d E^{ij}\varepsilon_{abcd} \\
& + (-\frac{1}{24}\mathcal{D}^\dagger\bar{\mathcal{H}} - \frac{1}{36}\mathcal{D}\bar{\mathcal{I}})E_{jk}T_{bclm}\gamma_{ab}^{\dot{\alpha}}\nabla_c\Lambda^{\dot{\beta}j}\varepsilon^{iklm} + (-\frac{1}{24}\mathcal{D}^\dagger\bar{\mathcal{H}} - \frac{1}{36}\mathcal{D}\bar{\mathcal{I}})E_{jk}\Lambda^{\dot{\beta}j}\gamma_{ab}^{\dot{\alpha}}\nabla_c T_{bclm}\varepsilon^{iklm} \\
& + (-\frac{1}{24}\mathcal{D}^\dagger\bar{\mathcal{H}} - \frac{1}{36}\mathcal{D}\bar{\mathcal{I}})E_{jk}\Lambda^{\dot{\beta}j}\gamma_{bc}^{\dot{\alpha}}\nabla_b T_{aclm}\varepsilon^{iklm} + (-\frac{1}{24}\mathcal{D}\mathcal{D}\mathcal{H} - \frac{1}{3}\mathcal{I})E^{ij}\Lambda_{\alpha j}\bar{P}_a\bar{P}_b\gamma_b^{\dot{\alpha}\alpha} \\
& + (-\frac{1}{48}\bar{\mathcal{H}} - \frac{1}{24}\mathcal{H})T_{ab}^{ij}T_{bc}^{kl}\gamma_{cd}^{\dot{\alpha}}\nabla_d\Lambda^{\dot{\beta}m}\varepsilon_{jklm} + (-\frac{1}{48}\mathcal{D}^\dagger\bar{\mathcal{H}} - \frac{1}{96}\mathcal{D}\bar{\mathcal{I}})E^{ij}E^{kl}\chi_{\alpha}{}^{mn}{}_k\gamma_a^{\dot{\alpha}\alpha}\varepsilon_{jlmn} \\
& + (-\frac{1}{96}\bar{\mathcal{H}} + \frac{1}{96}\mathcal{H})P_b\Lambda^{\dot{\beta}i}\bar{P}_b\bar{P}_c\gamma_{ac}^{\dot{\alpha}}\nabla_{\dot{\beta}} + (-\frac{1}{96}\bar{\mathcal{H}} + \frac{3}{32}\mathcal{H})E^{ij}T_{bc}^{kl}R(Q)_{bc\alpha}{}^m\gamma_a^{\dot{\alpha}\alpha}\varepsilon_{jklm} \\
& + (-\frac{1}{384}\bar{\mathcal{H}} + \frac{17}{384}\mathcal{H})T_{bc}^{jk}T_{bc}^{lm}\gamma_{ad}^{\dot{\alpha}}\nabla_d\Lambda^{\dot{\beta}i}\varepsilon_{jklm} + (\frac{1}{192}\bar{\mathcal{H}} + \frac{1}{64}\mathcal{H})E_{jk}E^{il}E^{jk}\Lambda_{\alpha l}\gamma_a^{\dot{\alpha}\alpha} + (\frac{1}{192}\bar{\mathcal{H}} + \frac{5}{64}\mathcal{H})E^{ij}P_b\Lambda_{\alpha j}\bar{P}_a\gamma_b^{\dot{\alpha}\alpha} + 6\cdots
\end{aligned}$$

$$\begin{aligned}
[\hat{\Omega}_a^{\dot{\alpha}i}]_{1,cont.} = & + \left(\frac{1}{96} \bar{\mathcal{H}} + \frac{1}{32} \mathcal{H}\right) E_{jk} E^{jk} \Lambda^{\dot{\beta}i} \bar{P}_b \gamma_{ab}^{\dot{\alpha}}{}_{\dot{\beta}} + \left(\frac{1}{96} \bar{\mathcal{H}} + \frac{1}{32} \mathcal{H}\right) T_{bc}{}^{jk} \Lambda^{\dot{\beta}i} \gamma_{ad}^{\dot{\alpha}}{}_{\dot{\beta}} \nabla_d T_{bc}{}^{lm} \varepsilon_{jklm} + \left(\frac{1}{96} \mathcal{D}^\dagger \bar{\mathcal{I}} - \frac{1}{24} \mathcal{D} \mathcal{H}\right) D^{ij}{}_{kl} E_{jm} \Lambda_{\alpha n} \gamma_a^{\dot{\alpha}}{}_{\dot{\beta}} \varepsilon^{klmn} \\
& + \left(\frac{1}{96} \mathcal{D} \mathcal{D} \mathcal{H} + \frac{1}{12} \mathcal{I}\right) E^{ij} \Lambda_{\alpha j} \bar{P}_b \bar{P}_b \gamma_a^{\dot{\alpha}}{}_{\dot{\beta}} + \left(\frac{1}{48} \bar{\mathcal{H}} - \frac{5}{48} \mathcal{H}\right) T_{ab}{}^{ij} \Lambda^{\dot{\beta}k} \gamma_{bc}^{\dot{\alpha}}{}_{\dot{\beta}} \nabla_d T_{cd}{}^{lm} \varepsilon_{jklm} \\
& + \left(\frac{1}{48} \bar{\mathcal{H}} - \frac{5}{48} \mathcal{H}\right) T_{ab}{}^{jk} \Lambda^{\dot{\beta}l} \gamma_{bc}^{\dot{\alpha}}{}_{\dot{\beta}} \nabla_d T_{cd}{}^{im} \varepsilon_{jklm} + \left(\frac{1}{48} \bar{\mathcal{H}} - \frac{1}{48} \mathcal{H}\right) T_{bcjk} \Lambda_{\alpha l} R(V)_{ab}{}^l{}_m \gamma_c^{\dot{\alpha}}{}_{\dot{\beta}} \varepsilon^{ijkm} \\
& + \left(\frac{1}{48} \bar{\mathcal{H}} + \frac{1}{24} \mathcal{H}\right) T_{ab}{}^{jk} T_{bc}{}^{il} \gamma_{cd}^{\dot{\alpha}}{}_{\dot{\beta}} \nabla_d \Lambda^{\dot{\beta}m} \varepsilon_{jklm} + \left(\frac{1}{48} \bar{\mathcal{H}} + \frac{7}{48} \mathcal{H}\right) T_{abjk} \Lambda_{\alpha l} R(V)_{bc}{}^l{}_m \gamma_c^{\dot{\alpha}}{}_{\dot{\beta}} \varepsilon^{ijkm} \\
& + \left(\frac{1}{48} \mathcal{D}^\dagger \bar{\mathcal{H}} + \frac{1}{96} \mathcal{D} \bar{\mathcal{I}}\right) E_{jk} T_{bclm} \gamma_{bc}^{\dot{\alpha}}{}_{\dot{\beta}} \nabla_a \Lambda^{\dot{\beta}j} \varepsilon^{iklm} + \left(\frac{1}{48} \mathcal{D}^\dagger \bar{\mathcal{H}} + \frac{1}{96} \mathcal{D} \bar{\mathcal{I}}\right) E_{jk} \Lambda^{\dot{\beta}j} \gamma_{bc}^{\dot{\alpha}}{}_{\dot{\beta}} \nabla_a T_{bclm} \varepsilon^{iklm} \\
& + \left(\frac{1}{48} \mathcal{D}^\dagger \bar{\mathcal{I}} - \frac{1}{12} \mathcal{D} \mathcal{H}\right) E_{jk} \Lambda_{\alpha l} R(V)_{ab}{}^j{}_m \gamma_b^{\dot{\alpha}}{}_{\dot{\beta}} \varepsilon^{iklm} + \left(\frac{1}{48} \mathcal{D} \mathcal{D} \mathcal{H} + \frac{1}{6} \mathcal{I}\right) \Lambda^{\dot{\beta}i} \bar{P}_b \bar{P}_b \gamma_{ac}^{\dot{\alpha}}{}_{\dot{\beta}} + \left(\frac{1}{32} \bar{\mathcal{H}} - \frac{1}{32} \mathcal{H}\right) T_{bcjk} \bar{P}_a \chi^{\dot{\beta}}{}_{lm}{}^i \gamma_{bc}^{\dot{\alpha}}{}_{\dot{\beta}} \varepsilon^{jklm} \\
& + \left(\frac{1}{24} \bar{\mathcal{H}} + \frac{1}{72} \mathcal{H}\right) E^{ij} T_{ab}{}^{kl} \Lambda^{\dot{\alpha}m} \bar{P}_b \varepsilon_{jklm} + \left(\frac{1}{24} \bar{\mathcal{H}} + \frac{1}{12} \mathcal{H}\right) T_{bc}{}^{ij} T_{bd}{}^{kl} \gamma_{cd}^{\dot{\alpha}}{}_{\dot{\beta}} \nabla_a \Lambda^{\dot{\beta}m} \varepsilon_{jklm} + \left(\frac{1}{24} \bar{\mathcal{H}} + \frac{17}{72} \mathcal{H}\right) E^{ij} T_{bckl} T_{ab}{}^{kl} \Lambda_{\alpha j} \gamma_c^{\dot{\alpha}}{}_{\dot{\beta}} \\
& + \left(\frac{1}{24} \mathcal{D}^\dagger \bar{\mathcal{H}} - \frac{1}{48} \mathcal{D} \bar{\mathcal{I}}\right) E^{ij} \Lambda^{\dot{\beta}k} \gamma_{bc}^{\dot{\alpha}}{}_{\dot{\beta}} \nabla_b T_{ac}{}^{lm} \varepsilon_{jklm} + \left(\frac{1}{24} \mathcal{D}^\dagger \bar{\mathcal{H}} + \frac{1}{48} \mathcal{D} \bar{\mathcal{I}}\right) E^{ij} E^{kl} T_{abjk} \Lambda_{\alpha l} \gamma_b^{\dot{\alpha}}{}_{\dot{\beta}} \\
& + \left(\frac{1}{24} \mathcal{D}^\dagger \bar{\mathcal{H}} + \frac{1}{48} \mathcal{D} \bar{\mathcal{I}}\right) T_{ab}{}^{jk} \Lambda^{\dot{\beta}l} \gamma_{bc}^{\dot{\alpha}}{}_{\dot{\beta}} \nabla_c E^{im} \varepsilon_{jklm} + \left(\frac{1}{24} \mathcal{D}^\dagger \bar{\mathcal{H}} + \frac{1}{36} \mathcal{D} \bar{\mathcal{I}}\right) E_{jk} T_{ablm} \gamma_{bc}^{\dot{\alpha}}{}_{\dot{\beta}} \nabla_c \Lambda^{\dot{\beta}j} \varepsilon^{iklm} \\
& + \left(\frac{1}{24} \mathcal{D}^\dagger \bar{\mathcal{H}} + \frac{1}{24} \mathcal{D} \bar{\mathcal{I}}\right) E^{ij} T_{bcjk} \Lambda^{\dot{\beta}k} \bar{P}_a \gamma_{bc}^{\dot{\alpha}}{}_{\dot{\beta}} + \left(\frac{1}{24} \mathcal{D}^\dagger \bar{\mathcal{H}} + \frac{1}{24} \mathcal{D} \bar{\mathcal{I}}\right) E^{ij} \Lambda^{\dot{\beta}k} \gamma_{ab}^{\dot{\alpha}}{}_{\dot{\beta}} \nabla_c T_{bc}{}^{lm} \varepsilon_{jklm} \\
& + \left(\frac{1}{24} \mathcal{D}^\dagger \bar{\mathcal{I}} + \frac{1}{12} \mathcal{D} \mathcal{H}\right) E_{jk} E^{jl} T_{ab}{}^{ik} \Lambda_{\alpha l} \gamma_b^{\dot{\alpha}}{}_{\dot{\beta}} + \left(\frac{5}{96} \bar{\mathcal{H}} + \frac{7}{96} \mathcal{H}\right) E^{jk} T_{ab}{}^{lm} \chi_{\alpha}{}^{in}{}_j \gamma_b^{\dot{\alpha}}{}_{\dot{\beta}} \varepsilon_{klmn} \\
& + \left(\frac{1}{16} \bar{\mathcal{H}} + \frac{1}{8} \mathcal{H}\right) T_{ab}{}^{jk} T_{cd}{}^{il} \gamma_{bc}^{\dot{\alpha}}{}_{\dot{\beta}} \nabla_d \Lambda^{\dot{\beta}m} \varepsilon_{jklm} + \left(\frac{5}{72} \mathcal{D}^\dagger \bar{\mathcal{I}} - \frac{1}{6} \mathcal{D} \mathcal{H}\right) E_{jk} T_{bc}{}^{ij} \Lambda^{\dot{\beta}k} \bar{P}_b \gamma_{ac}^{\dot{\alpha}}{}_{\dot{\beta}} \\
& + \left(\frac{7}{96} \bar{\mathcal{H}} - \frac{1}{96} \mathcal{H}\right) E^{ij} \Lambda_{\alpha k} R(V)_{bc}{}^k{}_j \gamma_d^{\dot{\alpha}}{}_{\dot{\beta}} \varepsilon_{abcd} + \left(\frac{1}{12} \bar{\mathcal{I}} - \frac{1}{96} \mathcal{D}^\dagger \mathcal{D}^\dagger \bar{\mathcal{H}}\right) T_{bcjk} \Lambda^{\dot{\beta}j} \gamma_{bc}^{\dot{\alpha}}{}_{\dot{\beta}} \nabla_d T_{adlm} \varepsilon^{iklm} \\
& + \left(\frac{1}{12} \bar{\mathcal{I}} + \frac{1}{64} \mathcal{D}^\dagger \mathcal{D}^\dagger \bar{\mathcal{H}}\right) T_{abjk} \Lambda^{\dot{\beta}i} \gamma_{cd}^{\dot{\alpha}}{}_{\dot{\beta}} \nabla_b T_{cdlm} \varepsilon^{jklm} + \left(\frac{1}{12} \bar{\mathcal{H}} - \frac{1}{12} \mathcal{H}\right) T_{bcjk} \Lambda_{\alpha l} R(V)_{bc}{}^i{}_m \gamma_a^{\dot{\alpha}}{}_{\dot{\beta}} \varepsilon^{jklm} \\
& + \left(\frac{1}{12} \mathcal{D}^\dagger \bar{\mathcal{I}} + \frac{1}{48} \mathcal{D}^\dagger \mathcal{D}^\dagger \mathcal{D}^\dagger \bar{\mathcal{H}}\right) E^{ij} P_b T_{bcjk} \Lambda^{\dot{\beta}k} \gamma_{ac}^{\dot{\alpha}}{}_{\dot{\beta}} + \left(\frac{1}{12} \mathcal{D}^\dagger \bar{\mathcal{H}} - \frac{1}{24} \mathcal{D} \bar{\mathcal{I}}\right) E_{jk} P_b T_{bc}{}^{ij} \Lambda^{\dot{\beta}k} \gamma_{ac}^{\dot{\alpha}}{}_{\dot{\beta}} \\
& + \left(\frac{1}{12} \mathcal{D}^\dagger \bar{\mathcal{H}} + \frac{1}{48} \mathcal{D} \bar{\mathcal{I}}\right) E^{ij} T_{bc}{}^{kl} \gamma_{ab}^{\dot{\alpha}}{}_{\dot{\beta}} \nabla_c \Lambda^{\dot{\beta}m} \varepsilon_{jklm} + \left(\frac{1}{12} \mathcal{D}^\dagger \bar{\mathcal{H}} + \frac{1}{12} \mathcal{D} \bar{\mathcal{I}}\right) P_b T_{ac}{}^{jk} T_{bc}{}^{il} \Lambda^{\dot{\alpha}m} \varepsilon_{jklm} \\
& + \left(\frac{1}{12} \mathcal{D}^\dagger \bar{\mathcal{H}} + \frac{2}{9} \mathcal{D} \bar{\mathcal{I}}\right) P_b \Lambda_{\alpha j} \gamma_a^{\dot{\alpha}}{}_{\dot{\beta}} \nabla_c T_{bckl} \varepsilon^{ijkl} + \left(\frac{1}{12} \mathcal{D}^\dagger \bar{\mathcal{I}} - \frac{1}{3} \mathcal{D} \mathcal{H}\right) P_b T_{ac}{}^{ij} \Lambda_{\alpha j} \bar{P}_c \gamma_b^{\dot{\alpha}}{}_{\dot{\beta}} \\
& + \left(\frac{1}{12} \mathcal{D}^\dagger \bar{\mathcal{I}} - \frac{1}{4} \mathcal{D} \mathcal{H}\right) T_{ab}{}^{jk} T_{bc}{}^{il} \chi_{\alpha}{}^{mn}{}_l \gamma_c^{\dot{\alpha}}{}_{\dot{\beta}} \varepsilon_{jkmn} + \left(\frac{1}{12} \mathcal{D}^\dagger \bar{\mathcal{I}} + \frac{1}{12} \mathcal{D} \mathcal{H}\right) E_{jk} E^{ij} T_{ab}{}^{kl} \Lambda_{\alpha l} \gamma_b^{\dot{\alpha}}{}_{\dot{\beta}} \\
& + \left(\frac{1}{12} \mathcal{D} \mathcal{D} \mathcal{D} \mathcal{H} - \frac{1}{3} \mathcal{D} \bar{\mathcal{I}}\right) T_{bc}{}^{ij} \Lambda_{\alpha j} \bar{P}_a \bar{P}_b \gamma_c^{\dot{\alpha}}{}_{\dot{\beta}} + \left(\frac{3}{32} \bar{\mathcal{H}} - \frac{25}{96} \mathcal{H}\right) P_b \Lambda^{\dot{\beta}i} \bar{P}_c \gamma_{ab}^{\dot{\alpha}}{}_{\dot{\beta}} + \left(\frac{1}{9} \bar{\mathcal{I}} - \frac{1}{72} \mathcal{D}^\dagger \mathcal{D}^\dagger \bar{\mathcal{H}}\right) E_{jk} P_b T_{ablm} \Lambda^{\dot{\alpha}j} \varepsilon^{iklm} \\
& + \left(\frac{1}{9} \mathcal{D}^\dagger \bar{\mathcal{I}} - \frac{1}{6} \mathcal{D} \mathcal{H}\right) E_{jk} T_{ab}{}^{ij} \Lambda^{\dot{\beta}k} \bar{P}_c \gamma_{bc}^{\dot{\alpha}}{}_{\dot{\beta}} + \left(\frac{11}{96} \bar{\mathcal{H}} + \frac{1}{96} \mathcal{H}\right) T_{ab}{}^{jk} \Lambda^{\dot{\beta}i} \gamma_{bc}^{\dot{\alpha}}{}_{\dot{\beta}} \nabla_d T_{cd}{}^{lm} \varepsilon_{jklm} \\
& + \left(\frac{11}{96} \bar{\mathcal{H}} + \frac{5}{96} \mathcal{H}\right) T_{bcjk} \Lambda_{\alpha l} R(V)_{bc}{}^l{}_m \gamma_a^{\dot{\alpha}}{}_{\dot{\beta}} \varepsilon^{ijkm} + \left(\frac{1}{8} \bar{\mathcal{H}} - \frac{1}{8} \mathcal{H}\right) P_b \Lambda^{\dot{\beta}i} \bar{P}_a \bar{P}_c \gamma_{bc}^{\dot{\alpha}}{}_{\dot{\beta}} + \left(\frac{1}{8} \bar{\mathcal{H}} + \frac{11}{72} \mathcal{H}\right) E^{jk} T_{bcjl} T_{ab}{}^{il} \Lambda_{\alpha k} \gamma_c^{\dot{\alpha}}{}_{\dot{\beta}} \\
& + \left(\frac{1}{8} \bar{\mathcal{H}} + \frac{5}{24} \mathcal{H}\right) E_{jk} T_{ablm} \Lambda^{\dot{\alpha}j} \bar{P}_b \varepsilon^{iklm} + \left(\frac{1}{8} \bar{\mathcal{H}} + \frac{3}{8} \mathcal{H}\right) E^{ij} T_{bcjk} T_{ab}{}^{kl} \Lambda_{\alpha l} \gamma_c^{\dot{\alpha}}{}_{\dot{\beta}} + \left(\frac{1}{8} \mathcal{D}^\dagger \bar{\mathcal{H}} + \frac{3}{16} \mathcal{D} \bar{\mathcal{I}}\right) T_{bcjk} T_{bclm} \chi_{\alpha}{}^{jk}{}_n \gamma_a^{\dot{\alpha}}{}_{\dot{\beta}} \varepsilon^{ilmn} \\
& + \left(\frac{1}{8} \mathcal{D}^\dagger \bar{\mathcal{I}} + \frac{1}{6} \mathcal{D} \mathcal{H}\right) T_{abjk} \Lambda_{\alpha l} \gamma_b^{\dot{\alpha}}{}_{\dot{\beta}} \nabla_c \bar{P}_c \varepsilon^{ijkl} + \left(\frac{1}{8} \mathcal{D}^\dagger \bar{\mathcal{I}} + \frac{1}{6} \mathcal{D} \mathcal{H}\right) \Lambda_{\alpha j} \bar{P}_a \gamma_b^{\dot{\alpha}}{}_{\dot{\beta}} \nabla_c T_{bckl} \varepsilon^{ijkl} + \left(\frac{25}{192} \bar{\mathcal{H}} + \frac{1}{64} \mathcal{H}\right) E^{ij} T_{ab}{}^{kl} \chi_{\alpha}{}^{mn}{}_j \gamma_b^{\dot{\alpha}}{}_{\dot{\beta}} \varepsilon_{klmn} \\
& + \left(\frac{1}{6} \bar{\mathcal{I}} - \frac{1}{96} \mathcal{D}^\dagger \mathcal{D}^\dagger \bar{\mathcal{H}}\right) T_{abjk} T_{cdlm} \gamma_{cd}^{\dot{\alpha}}{}_{\dot{\beta}} \nabla_b \Lambda^{\dot{\beta}l} \varepsilon^{ijkm} + \left(\frac{1}{6} \bar{\mathcal{I}} - \frac{1}{96} \mathcal{D}^\dagger \mathcal{D}^\dagger \bar{\mathcal{H}}\right) T_{abjk} \Lambda^{\dot{\beta}l} \gamma_{cd}^{\dot{\alpha}}{}_{\dot{\beta}} \nabla_b T_{cdlm} \varepsilon^{ijkm} \\
& + \left(\frac{1}{6} \mathcal{D}^\dagger \bar{\mathcal{H}} - \frac{1}{8} \mathcal{D} \bar{\mathcal{I}}\right) T_{bcjk} \Lambda_{\alpha l} \gamma_b^{\dot{\alpha}}{}_{\dot{\beta}} \nabla_c P_a \varepsilon^{ijkl} + \left(\frac{1}{6} \mathcal{D}^\dagger \bar{\mathcal{H}} + \frac{5}{72} \mathcal{D} \bar{\mathcal{I}}\right) T_{abjk} \Lambda_{\alpha l} \gamma_b^{\dot{\alpha}}{}_{\dot{\beta}} \nabla_c P_c \varepsilon^{ijkl} + \left(\frac{1}{6} \mathcal{D}^\dagger \bar{\mathcal{H}} + \frac{1}{12} \mathcal{D} \bar{\mathcal{I}}\right) T_{abjk} T_{bclm} \Lambda^{\dot{\alpha}j} \bar{P}_c \varepsilon^{iklm} \\
& + \left(\frac{1}{6} \mathcal{D}^\dagger \bar{\mathcal{H}} + \frac{11}{72} \mathcal{D} \bar{\mathcal{I}}\right) T_{bcjk} \Lambda_{\alpha l} \gamma_b^{\dot{\alpha}}{}_{\dot{\beta}} \nabla_a P_c \varepsilon^{ijkl} + \left(\frac{1}{6} \mathcal{D}^\dagger \bar{\mathcal{H}} + \frac{31}{72} \mathcal{D} \bar{\mathcal{I}}\right) P_b T_{bcjk} \gamma_a^{\dot{\alpha}}{}_{\dot{\beta}} \nabla_c \Lambda_{\alpha l} \varepsilon^{ijkl} + 7 \dots
\end{aligned}$$

$$\begin{aligned}
[\hat{\Omega}_a^{\dot{\alpha}i}]_{1,cont.} = & + \left(\frac{1}{6} \mathcal{D}^\dagger \mathcal{I} - \frac{1}{3} \mathcal{D} \mathcal{H}\right) T_{abjk} T_{bc}{}^{il} T_{cd}{}^{jk} \Lambda_{\alpha l} \gamma_d{}^{\dot{\alpha}\alpha} + \left(\frac{1}{6} \mathcal{D}^\dagger \mathcal{I} - \frac{1}{12} \mathcal{D} \mathcal{H}\right) T_{abjk} T_{bc}{}^{ij} T_{cd}{}^{kl} \Lambda_{\alpha l} \gamma_d{}^{\dot{\alpha}\alpha} \\
& + \left(\frac{5}{24} \mathcal{D}^\dagger \mathcal{I} + \frac{1}{6} \mathcal{D} \mathcal{H}\right) \Lambda_{\alpha j} \bar{P}_b \gamma_c{}^{\dot{\alpha}\alpha} \nabla_c T_{abkl} \varepsilon^{ijkl} + \left(\frac{1}{4} \mathcal{D}^\dagger \bar{\mathcal{H}} - \frac{5}{36} \mathcal{D} \bar{\mathcal{I}}\right) P_a \Lambda_{\alpha j} \gamma_b{}^{\dot{\alpha}\alpha} \nabla_c T_{bckl} \varepsilon^{ijkl} \\
& + \left(\frac{1}{4} \mathcal{D}^\dagger \bar{\mathcal{H}} + \frac{1}{36} \mathcal{D} \bar{\mathcal{I}}\right) P_b \Lambda_{\alpha j} \gamma_c{}^{\dot{\alpha}\alpha} \nabla_b T_{ackl} \varepsilon^{ijkl} + \left(\frac{1}{4} \mathcal{D}^\dagger \mathcal{I} - \frac{1}{3} \mathcal{D} \mathcal{H}\right) P_b T_{ab}{}^{ij} \Lambda_{\alpha j} \bar{P}_c \gamma_c{}^{\dot{\alpha}\alpha} \\
& + \left(\frac{1}{4} \mathcal{D} \mathcal{D} \mathcal{D} \mathcal{H} + \frac{5}{3} \mathcal{D} \mathcal{I}\right) T_{ab}{}^{ij} \Lambda_{\alpha j} \bar{P}_b \bar{P}_c \gamma_c{}^{\dot{\alpha}\alpha} + \left(\frac{7}{24} \mathcal{D} \mathcal{D} \mathcal{H} - \frac{2}{3} \mathcal{I}\right) E_{jk} T_{ab}{}^{ij} T_{bc}{}^{kl} \Lambda_{\alpha l} \gamma_c{}^{\dot{\alpha}\alpha} \\
& + \left(\frac{1}{3} \bar{\mathcal{I}} + \frac{1}{48} \mathcal{D}^\dagger \mathcal{D}^\dagger \bar{\mathcal{H}}\right) P_b T_{bcjk} \chi^{\dot{\beta}}{}_{lm}{}^i \gamma_{ac}{}^{\dot{\alpha}}{}_{\dot{\beta}} \varepsilon^{jklm} + \left(\frac{3}{8} \mathcal{D}^\dagger \mathcal{I} + \frac{1}{6} \mathcal{D} \mathcal{H}\right) \Lambda_{\alpha j} \bar{P}_b \gamma_c{}^{\dot{\alpha}\alpha} \nabla_a T_{bckl} \varepsilon^{ijkl} \\
& + \left(\frac{29}{72} \mathcal{D}^\dagger \mathcal{I} - \frac{1}{6} \mathcal{D} \mathcal{H}\right) T_{ab}{}^{ij} T_{bc}{}^{kl} \Lambda^{\dot{\alpha}m} \bar{P}_c \varepsilon_{jklm} + \left(\frac{5}{12} \bar{\mathcal{I}} - \frac{1}{48} \mathcal{D}^\dagger \mathcal{D}^\dagger \bar{\mathcal{H}}\right) P_b T_{cdjk} R(Q)_{cd}{}^{\dot{\beta}}{}_{l\gamma ab}{}^{\dot{\alpha}}{}_{\dot{\beta}} \varepsilon^{ijkl} \\
& + \left(\frac{1}{2} \mathcal{D}^\dagger \bar{\mathcal{I}} + \frac{1}{24} \mathcal{D}^\dagger \mathcal{D}^\dagger \mathcal{D}^\dagger \bar{\mathcal{H}}\right) P_b T_{acjk} T_{bclm} \Lambda^{\dot{\alpha}j} \varepsilon^{iklm} + \left(\frac{1}{2} \mathcal{D}^\dagger \mathcal{I} + \frac{1}{3} \mathcal{D} \mathcal{H}\right) P_b T_{ac}{}^{ij} \Lambda_{\alpha j} \bar{P}_b \gamma_c{}^{\dot{\alpha}\alpha} \\
& + \left(\frac{2}{3} \bar{\mathcal{I}} - \frac{1}{4} \mathcal{D}^\dagger \mathcal{D}^\dagger \bar{\mathcal{H}}\right) P_b T_{cdjk} T_{ac}{}^{jk} \Lambda^{\dot{\beta}i} \gamma_{bd}{}^{\dot{\alpha}}{}_{\dot{\beta}} + \left(\frac{3}{4} \mathcal{D}^\dagger \mathcal{I} - \frac{1}{2} \mathcal{D} \mathcal{H}\right) T_{ab}{}^{jk} T_{cd}{}^{il} R(Q)_{cd\alpha}{}^m \gamma_b{}^{\dot{\alpha}\alpha} \varepsilon_{jklm} \\
& + \left(\frac{4}{3} \bar{\mathcal{I}} - \frac{1}{3} \mathcal{D}^\dagger \mathcal{D}^\dagger \bar{\mathcal{H}}\right) P_b T_{cdjk} T_{ac}{}^{ij} \Lambda^{\dot{\beta}k} \gamma_{bd}{}^{\dot{\alpha}}{}_{\dot{\beta}} - \frac{1}{16} E_{jk} E_{lm} T_{ab}{}^{jl} \mathcal{D} \mathcal{D} \mathcal{H} \Lambda_{\alpha n} \gamma_b{}^{\dot{\alpha}\alpha} \varepsilon^{ikmn} - \frac{1}{32} T_{bcjk} T_{bclm} \mathcal{D} \bar{\mathcal{I}} \Lambda^{\dot{\beta}i} \bar{P}_d \gamma_{ad}{}^{\dot{\alpha}}{}_{\dot{\beta}} \varepsilon^{jklm} \\
& + \frac{5}{288} T_{ab}{}^{ij} T_{bc}{}^{kl} \mathcal{D}^\dagger \mathcal{I} \Lambda^{\dot{\beta}m} \bar{P}_d \gamma_{cd}{}^{\dot{\alpha}}{}_{\dot{\beta}} \varepsilon_{jklm} - \frac{5}{96} T_{ab}{}^{ij} T_{cd}{}^{kl} \mathcal{D}^\dagger \mathcal{I} \Lambda^{\dot{\beta}m} \bar{P}_c \gamma_{bd}{}^{\dot{\alpha}}{}_{\dot{\beta}} \varepsilon_{jklm} - \frac{5}{288} T_{ab}{}^{jk} T_{bc}{}^{il} \mathcal{D}^\dagger \mathcal{I} \Lambda^{\dot{\beta}m} \bar{P}_d \gamma_{cd}{}^{\dot{\alpha}}{}_{\dot{\beta}} \varepsilon_{jklm} \\
& + \frac{5}{96} T_{ab}{}^{jk} T_{cd}{}^{il} \mathcal{D}^\dagger \mathcal{I} \Lambda^{\dot{\beta}m} \bar{P}_c \gamma_{bd}{}^{\dot{\alpha}}{}_{\dot{\beta}} \varepsilon_{jklm} - \frac{5}{144} T_{bc}{}^{ij} T_{bd}{}^{kl} \mathcal{D}^\dagger \mathcal{I} \Lambda^{\dot{\beta}m} \bar{P}_a \gamma_{cd}{}^{\dot{\alpha}}{}_{\dot{\beta}} \varepsilon_{jklm} - \frac{1}{24} \bar{\mathcal{H}} E_{jk} T_{bclm} \Lambda^{\dot{\beta}j} \bar{P}_a \gamma_{bc}{}^{\dot{\alpha}}{}_{\dot{\beta}} \varepsilon^{iklm} \\
& - \frac{1}{6} \mathcal{D}^\dagger \bar{\mathcal{I}} P_a T_{bcjk} T_{bdlm} \Lambda^{\dot{\beta}j} \gamma_{cd}{}^{\dot{\alpha}}{}_{\dot{\beta}} \varepsilon^{iklm} + \frac{1}{6} \mathcal{D}^\dagger \bar{\mathcal{I}} P_a T_{bcjk} T_{bdlm} \Lambda^{\dot{\beta}l} \gamma_{cd}{}^{\dot{\alpha}}{}_{\dot{\beta}} \varepsilon^{ijkm} + \frac{1}{24} \mathcal{D}^\dagger \bar{\mathcal{H}} P_a T_{bc}{}^{ij} T_{bd}{}^{kl} \Lambda^{\dot{\beta}m} \gamma_{cd}{}^{\dot{\alpha}}{}_{\dot{\beta}} \varepsilon_{jklm} \\
& + \frac{1}{16} \mathcal{D}^\dagger \bar{\mathcal{H}} P_b T_{ac}{}^{ij} T_{bd}{}^{kl} \Lambda^{\dot{\beta}m} \gamma_{cd}{}^{\dot{\alpha}}{}_{\dot{\beta}} \varepsilon_{jklm} + \frac{1}{48} \mathcal{D}^\dagger \bar{\mathcal{H}} P_b T_{ac}{}^{ij} T_{cd}{}^{kl} \Lambda^{\dot{\beta}m} \gamma_{bd}{}^{\dot{\alpha}}{}_{\dot{\beta}} \varepsilon_{jklm} - \frac{1}{16} \mathcal{D}^\dagger \bar{\mathcal{H}} P_b T_{ac}{}^{jk} T_{bd}{}^{il} \Lambda^{\dot{\beta}m} \gamma_{cd}{}^{\dot{\alpha}}{}_{\dot{\beta}} \varepsilon_{jklm} \\
& - \frac{1}{48} \mathcal{D}^\dagger \bar{\mathcal{H}} P_b T_{ac}{}^{jk} T_{cd}{}^{il} \Lambda^{\dot{\beta}m} \gamma_{bd}{}^{\dot{\alpha}}{}_{\dot{\beta}} \varepsilon_{jklm} - \frac{1}{12} \mathcal{D} \mathcal{D} \mathcal{H} T_{ab}{}^{ij} T_{cd}{}^{kl} T_{cd}{}^{mn} \Lambda_{\alpha j} \gamma_b{}^{\dot{\alpha}\alpha} \varepsilon_{klmn} + \frac{1}{16} \mathcal{D} \mathcal{D} \mathcal{H} T_{bc}{}^{ij} T_{bd}{}^{kl} T_{cd}{}^{mn} \Lambda_{\alpha k} \gamma_a{}^{\dot{\alpha}\alpha} \varepsilon_{jlmn} \\
& - \frac{1}{16} \mathcal{D} \mathcal{D} \mathcal{H} T_{bc}{}^{ij} T_{bd}{}^{kl} T_{cd}{}^{mn} \Lambda_{\alpha m} \gamma_a{}^{\dot{\alpha}\alpha} \varepsilon_{jklm} + \left(-\frac{1}{3} \bar{\mathcal{I}} - \frac{23}{72} \mathcal{D}^\dagger \mathcal{D}^\dagger \bar{\mathcal{H}}\right) P_a P_b T_{bcjk} \Lambda_{\alpha l} \gamma_c{}^{\dot{\alpha}\alpha} \varepsilon^{ijkl} \\
& + \left(-\frac{5}{18} \bar{\mathcal{H}} - \frac{1}{6} \mathcal{H}\right) P_b T_{acjk} \Lambda_{\alpha l} \bar{P}_b \gamma_c{}^{\dot{\alpha}\alpha} \varepsilon^{ijkl} + \left(-\frac{2}{9} \bar{\mathcal{I}} - \frac{11}{36} \mathcal{D}^\dagger \mathcal{D}^\dagger \bar{\mathcal{H}}\right) P_b P_c T_{abjk} \Lambda_{\alpha l} \gamma_c{}^{\dot{\alpha}\alpha} \varepsilon^{ijkl} \\
& + \left(-\frac{1}{6} \mathcal{D}^\dagger \mathcal{I} + \frac{1}{12} \mathcal{D} \mathcal{H}\right) E_{jk} T_{bclm} T_{ab}{}^{jn} \Lambda_{\alpha n} \gamma_c{}^{\dot{\alpha}\alpha} \varepsilon^{iklm} + \left(-\frac{7}{48} \mathcal{D}^\dagger \mathcal{I} - \frac{1}{12} \mathcal{D} \mathcal{H}\right) E^{ij} T_{ab}{}^{kl} T_{bc}{}^{mn} \Lambda_{\alpha m} \gamma_c{}^{\dot{\alpha}\alpha} \varepsilon_{jklm} \\
& + \left(-\frac{1}{8} \mathcal{D}^\dagger \bar{\mathcal{I}} + \frac{1}{96} \mathcal{D}^\dagger \mathcal{D}^\dagger \mathcal{D}^\dagger \bar{\mathcal{H}}\right) P_b T_{abjk} T_{cdlm} \Lambda^{\dot{\beta}j} \gamma_{cd}{}^{\dot{\alpha}}{}_{\dot{\beta}} \varepsilon^{iklm} + \left(-\frac{5}{48} \mathcal{D}^\dagger \bar{\mathcal{I}} - \frac{1}{192} \mathcal{D}^\dagger \mathcal{D}^\dagger \mathcal{D}^\dagger \bar{\mathcal{H}}\right) P_b T_{cdjk} T_{cdlm} \Lambda^{\dot{\beta}i} \gamma_{ab}{}^{\dot{\alpha}}{}_{\dot{\beta}} \varepsilon^{jklm} \\
& + \left(-\frac{5}{48} \mathcal{D}^\dagger \bar{\mathcal{H}} - \frac{17}{96} \mathcal{D} \bar{\mathcal{I}}\right) T_{abjk} T_{cdlm} \Lambda^{\dot{\beta}j} \bar{P}_b \gamma_{cd}{}^{\dot{\alpha}}{}_{\dot{\beta}} \varepsilon^{jklm} + \left(-\frac{11}{144} \mathcal{D}^\dagger \mathcal{I} - \frac{1}{12} \mathcal{D} \mathcal{H}\right) E^{jk} T_{ab}{}^{il} T_{bc}{}^{mn} \Lambda_{\alpha j} \gamma_c{}^{\dot{\alpha}\alpha} \varepsilon_{klmn} \\
& + \left(-\frac{7}{96} \bar{\mathcal{H}} + \frac{23}{96} \mathcal{H}\right) P_b T_{bcjk} \Lambda_{\alpha l} \bar{P}_c \gamma_a{}^{\dot{\alpha}\alpha} \varepsilon^{ijkl} + \left(-\frac{1}{16} \bar{\mathcal{H}} - \frac{1}{48} \mathcal{H}\right) E^{ij} T_{ab}{}^{kl} \Lambda^{\dot{\beta}m} \bar{P}_c \gamma_{bc}{}^{\dot{\alpha}}{}_{\dot{\beta}} \varepsilon_{jklm} \\
& + \left(-\frac{1}{18} \bar{\mathcal{I}} + \frac{1}{36} \mathcal{D}^\dagger \mathcal{D}^\dagger \bar{\mathcal{H}}\right) E_{jk} P_b T_{bclm} \Lambda^{\dot{\beta}j} \gamma_{ac}{}^{\dot{\alpha}}{}_{\dot{\beta}} \varepsilon^{iklm} + \left(-\frac{1}{18} \bar{\mathcal{I}} + \frac{19}{144} \mathcal{D}^\dagger \mathcal{D}^\dagger \bar{\mathcal{H}}\right) P_b P_b T_{acjk} \Lambda_{\alpha l} \gamma_c{}^{\dot{\alpha}\alpha} \varepsilon^{ijkl} \\
& + \left(-\frac{1}{24} \mathcal{D}^\dagger \bar{\mathcal{H}} - \frac{1}{16} \mathcal{D} \bar{\mathcal{I}}\right) T_{abjk} T_{cdlm} \Lambda^{\dot{\beta}j} \bar{P}_b \gamma_{cd}{}^{\dot{\alpha}}{}_{\dot{\beta}} \varepsilon^{iklm} + \left(-\frac{1}{24} \mathcal{D}^\dagger \bar{\mathcal{H}} - \frac{1}{24} \mathcal{D} \bar{\mathcal{I}}\right) T_{bcjk} T_{bdlm} \Lambda^{\dot{\beta}j} \bar{P}_a \gamma_{cd}{}^{\dot{\alpha}}{}_{\dot{\beta}} \varepsilon^{iklm} \\
& + \left(-\frac{1}{24} \mathcal{D}^\dagger \bar{\mathcal{H}} + \frac{5}{48} \mathcal{D} \bar{\mathcal{I}}\right) E^{jk} T_{abjl} T_{bcmn} \Lambda_{\alpha k} \gamma_c{}^{\dot{\alpha}\alpha} \varepsilon^{ilmn} + \left(-\frac{1}{24} \mathcal{D}^\dagger \bar{\mathcal{H}} + \frac{7}{48} \mathcal{D} \bar{\mathcal{I}}\right) E^{ij} T_{abjk} T_{bclm} \Lambda_{\alpha n} \gamma_c{}^{\dot{\alpha}\alpha} \varepsilon^{klmn} \\
& + \left(-\frac{1}{24} \mathcal{D} \mathcal{D} \mathcal{H} - \frac{1}{3} \mathcal{I}\right) T_{bcjk} \Lambda_{\alpha l} \bar{P}_a \bar{P}_b \gamma_c{}^{\dot{\alpha}\alpha} \varepsilon^{ijkl} + \left(-\frac{17}{576} \mathcal{D}^\dagger \mathcal{I} - \frac{1}{48} \mathcal{D} \mathcal{H}\right) E^{ij} T_{bc}{}^{kl} T_{bc}{}^{mn} \Lambda_{\alpha j} \gamma_a{}^{\dot{\alpha}\alpha} \varepsilon_{klmn} \\
& + \left(-\frac{5}{192} \bar{\mathcal{H}} + \frac{7}{64} \mathcal{H}\right) E^{ij} P_b \Lambda_{\alpha j} \bar{P}_c \gamma_d{}^{\dot{\alpha}\alpha} \varepsilon_{abcd} + \left(-\frac{11}{480} \mathcal{D}^\dagger \mathcal{I} + \frac{1}{360} \mathcal{D} \mathcal{H}\right) T_{bc}{}^{jk} T_{bc}{}^{lm} \Lambda^{\dot{\beta}i} \bar{P}_d \gamma_{ad}{}^{\dot{\alpha}}{}_{\dot{\beta}} \varepsilon_{jklm} \\
& + \left(-\frac{1}{48} \bar{\mathcal{H}} - \frac{1}{16} \mathcal{H}\right) E_{jk} T_{ablm} \Lambda^{\dot{\beta}j} \bar{P}_c \gamma_{bc}{}^{\dot{\alpha}}{}_{\dot{\beta}} \varepsilon^{iklm} + \left(-\frac{1}{48} \bar{\mathcal{H}} - \frac{1}{16} \mathcal{H}\right) E_{jk} T_{bclm} \Lambda^{\dot{\beta}j} \bar{P}_b \gamma_{ac}{}^{\dot{\alpha}}{}_{\dot{\beta}} \varepsilon^{iklm} \\
& + \left(-\frac{1}{48} \mathcal{D}^\dagger \bar{\mathcal{I}} + \frac{1}{64} \mathcal{D}^\dagger \mathcal{D}^\dagger \mathcal{D}^\dagger \bar{\mathcal{H}}\right) P_b T_{abjk} T_{cdlm} \Lambda^{\dot{\beta}i} \gamma_{cd}{}^{\dot{\alpha}}{}_{\dot{\beta}} \varepsilon^{jklm} + \left(-\frac{1}{48} \mathcal{D}^\dagger \bar{\mathcal{H}} - \frac{1}{192} \mathcal{D} \bar{\mathcal{I}}\right) E^{ij} T_{bckl} T_{bcmn} \Lambda_{\alpha j} \gamma_a{}^{\dot{\alpha}\alpha} \varepsilon^{klmn} + 8 \dots
\end{aligned}$$

$$\begin{aligned}
[\hat{\Omega}_a^{\dot{\alpha}i}]_{1,cont.} = & +(-\frac{1}{72}\bar{\mathcal{I}} + \frac{1}{64}\mathcal{D}^\dagger\mathcal{D}^\dagger\bar{\mathcal{H}})E_{jk}P_aT_{bclm}\Lambda^{\dot{\beta}j}\gamma_{bc}^{\dot{\alpha}}\dot{\beta}\varepsilon^{iklm} + (-\frac{1}{192}\mathcal{D}^\dagger\bar{\mathcal{H}} + \frac{1}{192}\mathcal{D}\bar{\mathcal{I}})T_{bcjk}T_{bdlm}\Lambda^{\dot{\beta}j}\bar{P}_c\gamma_{ad}^{\dot{\alpha}}\dot{\beta}\varepsilon^{iklm} \\
& + (-\frac{1}{192}\mathcal{D}^\dagger\bar{\mathcal{H}} + \frac{1}{192}\mathcal{D}\bar{\mathcal{I}})T_{bcjk}T_{bdlm}\Lambda^{\dot{\beta}j}\bar{P}_d\gamma_{ac}^{\dot{\alpha}}\dot{\beta}\varepsilon^{iklm} + (\frac{1}{720}\mathcal{D}^\dagger\mathcal{I} - \frac{1}{90}\mathcal{D}\mathcal{H})T_{ab}{}^{jk}T_{cd}{}^{lm}\Lambda^{\dot{\beta}i}\bar{P}_c\gamma_{bd}^{\dot{\alpha}}\dot{\beta}\varepsilon_{jklm} \\
& + (\frac{1}{192}\mathcal{D}^\dagger\bar{\mathcal{H}} - \frac{1}{192}\mathcal{D}\bar{\mathcal{I}})T_{bcjk}T_{bdlm}\Lambda^{\dot{\beta}l}\bar{P}_c\gamma_{ad}^{\dot{\alpha}}\dot{\beta}\varepsilon^{ijkm} + (\frac{1}{192}\mathcal{D}^\dagger\bar{\mathcal{H}} - \frac{1}{192}\mathcal{D}\bar{\mathcal{I}})T_{bcjk}T_{bdlm}\Lambda^{\dot{\beta}l}\bar{P}_d\gamma_{ac}^{\dot{\alpha}}\dot{\beta}\varepsilon^{ijkm} \\
& + (\frac{1}{96}\mathcal{D}^\dagger\mathcal{I} + \frac{1}{12}\mathcal{D}\mathcal{H})E_{jk}\Lambda_{\alpha l}R(V)_{bc}{}^j{}_m\gamma_d{}^{\dot{\alpha}\alpha}\varepsilon_{abcd}\varepsilon^{iklm} + (\frac{1}{64}\bar{\mathcal{H}} + \frac{3}{64}\mathcal{H})E_{jk}E^{ij}T_{ablm}\Lambda_{\alpha n}\gamma_b{}^{\dot{\alpha}\alpha}\varepsilon^{klmn} \\
& + (\frac{1}{48}\bar{\mathcal{H}} + \frac{1}{144}\mathcal{H})E^{ij}E^{kl}T_{ab}{}^{mn}\Lambda_{\alpha k}\gamma_b{}^{\dot{\alpha}\alpha}\varepsilon_{jlmn} + (\frac{1}{48}\bar{\mathcal{H}} + \frac{1}{144}\mathcal{H})E^{ij}T_{bc}{}^{kl}\Lambda^{\dot{\beta}m}\bar{P}_b\gamma_{ac}^{\dot{\alpha}}\dot{\beta}\varepsilon_{jklm} \\
& + (\frac{13}{576}\bar{\mathcal{H}} - \frac{1}{64}\mathcal{H})E_{jk}E^{jk}T_{ablm}\Lambda_{\alpha n}\gamma_b{}^{\dot{\alpha}\alpha}\varepsilon_{ilmn} + (\frac{5}{192}\bar{\mathcal{H}} - \frac{1}{192}\mathcal{H})E_{jk}E^{jl}T_{abmn}\Lambda_{\alpha l}\gamma_b{}^{\dot{\alpha}\alpha}\varepsilon^{ikmn} \\
& + (\frac{1}{24}\mathcal{D}^\dagger\bar{\mathcal{H}} - \frac{7}{48}\mathcal{D}\bar{\mathcal{I}})E^{ij}T_{abkl}T_{bcjm}\Lambda_{\alpha n}\gamma_c{}^{\dot{\alpha}\alpha}\varepsilon^{klmn} + (\frac{1}{24}\mathcal{D}^\dagger\bar{\mathcal{H}} - \frac{5}{48}\mathcal{D}\bar{\mathcal{I}})E^{jk}T_{ablm}T_{bcjn}\Lambda_{\alpha k}\gamma_c{}^{\dot{\alpha}\alpha}\varepsilon^{ilmn} \\
& + (\frac{1}{24}\mathcal{D}^\dagger\bar{\mathcal{H}} - \frac{5}{48}\mathcal{D}\bar{\mathcal{I}})P_bT_{ac}{}^{jk}T_{bd}{}^{lm}\Lambda^{\dot{\beta}i}\gamma_{cd}^{\dot{\alpha}}\dot{\beta}\varepsilon_{jklm} + (\frac{1}{24}\mathcal{D}^\dagger\bar{\mathcal{H}} + \frac{1}{24}\mathcal{D}\bar{\mathcal{I}})T_{bcjk}T_{bdlm}\Lambda^{\dot{\beta}l}\bar{P}_a\gamma_{cd}^{\dot{\alpha}}\dot{\beta}\varepsilon^{ijkm} \\
& + (\frac{1}{24}\mathcal{D}^\dagger\bar{\mathcal{H}} + \frac{1}{16}\mathcal{D}\bar{\mathcal{I}})T_{abjk}T_{cdlm}\Lambda^{\dot{\beta}l}\bar{P}_b\gamma_{cd}^{\dot{\alpha}}\dot{\beta}\varepsilon^{ijkm} + (\frac{1}{24}\mathcal{D}^\dagger\bar{\mathcal{H}} + \frac{5}{64}\mathcal{D}\bar{\mathcal{I}})P_bT_{cd}{}^{jk}T_{cd}{}^{lm}\Lambda^{\dot{\beta}i}\gamma_{ab}^{\dot{\alpha}}\dot{\beta}\varepsilon_{jklm} \\
& + (\frac{1}{24}\mathcal{D}\mathcal{D}\mathcal{H} + \frac{1}{3}\mathcal{I})T_{abjk}\Lambda_{\alpha l}\bar{P}_b\bar{P}_c\gamma_c{}^{\dot{\alpha}\alpha}\varepsilon^{ijkl} + (\frac{1}{18}\bar{\mathcal{I}} - \frac{1}{36}\mathcal{D}^\dagger\mathcal{D}^\dagger\bar{\mathcal{H}})E_{jk}P_bT_{aclm}\Lambda^{\dot{\beta}j}\gamma_{bc}^{\dot{\alpha}}\dot{\beta}\varepsilon^{iklm} \\
& + (\frac{1}{16}\bar{\mathcal{H}} + \frac{3}{16}\mathcal{H})T_{bcjk}T_{bclm}T_{ad}{}^{lm}\Lambda_{\alpha n}\gamma_d{}^{\dot{\alpha}\alpha}\varepsilon^{ijkn} + (\frac{11}{144}\mathcal{D}^\dagger\mathcal{I} + \frac{1}{12}\mathcal{D}\mathcal{H})E^{jk}T_{ab}{}^{lm}T_{bc}{}^{in}\Lambda_{\alpha j}\gamma_c{}^{\dot{\alpha}\alpha}\varepsilon_{klmn} \\
& + (\frac{1}{12}\bar{\mathcal{I}} - \frac{3}{32}\mathcal{D}^\dagger\mathcal{D}^\dagger\bar{\mathcal{H}})E^{ij}P_bT_{bc}{}^{kl}\Lambda^{\dot{\beta}m}\gamma_{ac}^{\dot{\alpha}}\dot{\beta}\varepsilon_{jklm} + (\frac{1}{12}\bar{\mathcal{I}} + \frac{1}{32}\mathcal{D}^\dagger\mathcal{D}^\dagger\bar{\mathcal{H}})E^{ij}P_bT_{ac}{}^{kl}\Lambda^{\dot{\beta}m}\gamma_{bc}^{\dot{\alpha}}\dot{\beta}\varepsilon_{jklm} \\
& + (\frac{3}{32}\bar{\mathcal{H}} - \frac{5}{96}\mathcal{H})T_{bcjk}T_{bclm}T_{ad}{}^{in}\Lambda_{\alpha n}\gamma_d{}^{\dot{\alpha}\alpha}\varepsilon^{jklm} + (\frac{5}{48}\mathcal{D}\mathcal{D}\mathcal{H} + \frac{1}{6}\mathcal{I})T_{abjk}\Lambda_{\alpha l}\bar{P}_c\bar{P}_b\gamma_b{}^{\dot{\alpha}\alpha}\varepsilon^{ijkl} \\
& + (\frac{1}{8}\mathcal{D}^\dagger\bar{\mathcal{I}} - \frac{1}{96}\mathcal{D}^\dagger\mathcal{D}^\dagger\mathcal{D}^\dagger\bar{\mathcal{H}})P_bT_{abjk}T_{cdlm}\Lambda^{\dot{\beta}l}\gamma_{cd}^{\dot{\alpha}}\dot{\beta}\varepsilon^{ijkm} + (\frac{7}{48}\mathcal{D}^\dagger\mathcal{I} + \frac{1}{12}\mathcal{D}\mathcal{H})E^{ij}T_{ab}{}^{kl}T_{bc}{}^{mn}\Lambda_{\alpha k}\gamma_c{}^{\dot{\alpha}\alpha}\varepsilon_{jlmn} \\
& + (\frac{1}{6}\mathcal{D}\mathcal{D}\mathcal{H} + \frac{1}{3}\mathcal{I})T_{ab}{}^{jk}T_{cd}{}^{il}T_{cd}{}^{mn}\Lambda_{\alpha l}\gamma_b{}^{\dot{\alpha}\alpha}\varepsilon_{jkmn} + (\frac{7}{32}\bar{\mathcal{H}} + \frac{1}{32}\mathcal{H})P_aT_{bcjk}\Lambda_{\alpha l}\bar{P}_b\gamma_c{}^{\dot{\alpha}\alpha}\varepsilon^{ijkl} \\
& + (\frac{1}{4}\mathcal{D}^\dagger\mathcal{I} - \frac{1}{4}\mathcal{D}\mathcal{H})E_{jk}T_{bclm}T_{ab}{}^{ij}\Lambda_{\alpha n}\gamma_c{}^{\dot{\alpha}\alpha}\varepsilon^{klmn} + (\frac{9}{32}\bar{\mathcal{H}} + \frac{13}{96}\mathcal{H})P_bT_{abjk}\Lambda_{\alpha l}\bar{P}_c\gamma_c{}^{\dot{\alpha}\alpha}\varepsilon^{ijkl} + (\frac{29}{96}\bar{\mathcal{H}} - \frac{5}{96}\mathcal{H})P_bT_{acjk}\Lambda_{\alpha l}\bar{P}_c\gamma_b{}^{\dot{\alpha}\alpha}\varepsilon^{ijkl} \\
& + (\frac{43}{96}\bar{\mathcal{H}} - \frac{1}{32}\mathcal{H})P_bT_{bcjk}\Lambda_{\alpha l}\bar{P}_a\gamma_c{}^{\dot{\alpha}\alpha}\varepsilon^{ijkl} - \frac{1}{192}E_{jk}E_{lm}E_{np}\mathcal{D}\mathcal{D}\mathcal{H}\Lambda_{\alpha q}\gamma_a{}^{\dot{\alpha}\alpha}\varepsilon^{ijln}\varepsilon^{kmpq} - \frac{1}{12}E_{jk}T_{ablm}T_{bcnp}\Lambda_{\alpha q}\bar{\mathcal{H}}\gamma_c{}^{\dot{\alpha}\alpha}\varepsilon^{ijlm}\varepsilon^{knpq} \\
& + \frac{1}{12}E_{jk}T_{ablm}T_{bcnp}\Lambda_{\alpha q}\bar{\mathcal{H}}\gamma_c{}^{\dot{\alpha}\alpha}\varepsilon^{ijnp}\varepsilon^{klmq} - \frac{7}{96}T_{bcjk}T_{bdlm}T_{cdnp}\mathcal{D}\bar{\mathcal{I}}\Lambda_{\alpha q}\gamma_a{}^{\dot{\alpha}\alpha}\varepsilon^{ijkl}\varepsilon^{mnpq} + \frac{7}{96}T_{bcjk}T_{bdlm}T_{cdnp}\mathcal{D}\bar{\mathcal{I}}\Lambda_{\alpha q}\gamma_a{}^{\dot{\alpha}\alpha}\varepsilon^{ilnp}\varepsilon^{jkmq} \\
& + (\frac{1}{96}\mathcal{D}^\dagger\bar{\mathcal{H}} - \frac{3}{64}\mathcal{D}\bar{\mathcal{I}})T_{abjk}T_{cdlm}T_{cdnp}\Lambda_{\alpha q}\gamma_b{}^{\dot{\alpha}\alpha}\varepsilon^{ijkq}\varepsilon^{lmnp} + (\frac{1}{96}\mathcal{D}^\dagger\mathcal{I} - \frac{1}{96}\mathcal{D}\mathcal{H})E_{jk}E_{lm}T_{abnp}\Lambda_{\alpha q}\gamma_b{}^{\dot{\alpha}\alpha}\varepsilon^{ijlq}\varepsilon^{kmnp} \\
& + (\frac{1}{48}\mathcal{D}^\dagger\bar{\mathcal{H}} + \frac{5}{96}\mathcal{D}\bar{\mathcal{I}})T_{abjk}T_{cdlm}T_{cdnp}\Lambda_{\alpha q}\gamma_b{}^{\dot{\alpha}\alpha}\varepsilon^{ilmq}\varepsilon^{jknq} + (\frac{11}{192}\bar{\mathcal{H}} + \frac{3}{64}\mathcal{H})E_{jk}T_{bclm}T_{bcnp}\Lambda_{\alpha q}\gamma_a{}^{\dot{\alpha}\alpha}\varepsilon^{ijlm}\varepsilon^{knpq}
\end{aligned}$$



$$\begin{aligned}
[\hat{\Omega}_a^{\alpha i}]_3 = & \frac{1}{6} \bar{\mathcal{I}} \Lambda^{\alpha j} \Lambda^{\beta k} \epsilon_{\beta \dot{\gamma}} \nabla_a \chi^{\dot{\gamma}}{}_{jk}{}^i - \frac{1}{12} \bar{\mathcal{I}} \Lambda^{\beta i} \Lambda^{\dot{\gamma} j} \gamma_{bc\beta\dot{\gamma}} \nabla_a R(Q)_{bc}{}^{\dot{\alpha}}{}_{\dot{j}} - \frac{1}{24} \bar{\mathcal{I}} \Lambda^{\beta i} R(Q)_{ab}{}^{\dot{\alpha}}{}_{\dot{j}} \epsilon_{\beta\dot{\gamma}} \nabla_b \Lambda^{\dot{\gamma} j} - \frac{1}{3} \bar{\mathcal{I}} \Lambda^{\beta j} R(Q)_{ab}{}^{\dot{\alpha}}{}_{\dot{j}} \epsilon_{\beta\dot{\gamma}} \nabla_b \Lambda^{\dot{\gamma} i} \\
& + \frac{1}{24} \bar{\mathcal{I}} \Lambda^{\beta i} R(Q)_{bc}{}^{\dot{\alpha}}{}_{\dot{j}} \gamma_{bc\beta\dot{\gamma}} \nabla_a \Lambda^{\dot{\gamma} j} + \frac{1}{12} \bar{\mathcal{I}} \Lambda^{\beta j} R(Q)_{bc}{}^{\dot{\alpha}}{}_{\dot{j}} \gamma_{bc\beta\dot{\gamma}} \nabla_a \Lambda^{\dot{\gamma} i} - \frac{1}{16} \mathcal{D}^\dagger \bar{\mathcal{H}} \Lambda^{\dot{\alpha} i} \chi_{\alpha}{}^{jk}{}_{\dot{l}} \chi^{\dot{\beta}}{}_{jk}{}^l \gamma_a{}^{\alpha}{}_{\dot{\beta}} - \frac{1}{48} \mathcal{D}^\dagger \mathcal{D}^\dagger \bar{\mathcal{H}} \Lambda^{\dot{\alpha} j} \Lambda^{\dot{\beta} k} \gamma_{ab\beta\dot{\gamma}} \nabla_b \chi^{\dot{\gamma}}{}_{jk}{}^i \\
& - \frac{1}{48} \mathcal{D}^\dagger \mathcal{D}^\dagger \bar{\mathcal{H}} \Lambda^{\dot{\beta} j} R(Q)_{ab}{}^{\dot{\alpha}}{}_{\dot{j}} \gamma_{bc\beta\dot{\gamma}} \nabla_c \Lambda^{\dot{\gamma} i} + \frac{1}{48} \mathcal{D}^\dagger \mathcal{D}^\dagger \bar{\mathcal{H}} \Lambda^{\dot{\beta} j} R(Q)_{bc}{}^{\dot{\alpha}}{}_{\dot{j}} \gamma_{ab\beta\dot{\gamma}} \nabla_c \Lambda^{\dot{\gamma} i} + \frac{1}{6} \mathcal{D} \bar{\mathcal{I}} \Lambda_{\alpha j} \Lambda^{\dot{\alpha} j} \gamma_b{}^{\alpha}{}_{\dot{\beta}} \nabla_a \nabla_b \Lambda^{\dot{\beta} i} \\
& + \frac{1}{8} \mathcal{D} \bar{\mathcal{I}} \Lambda_{\alpha j} \Lambda^{\dot{\beta} j} \gamma_b{}^{\alpha}{}_{\dot{\beta}} \nabla_a \nabla_b \Lambda^{\dot{\alpha} i} - \frac{1}{4} \mathcal{D} \bar{\mathcal{I}} \Lambda^{\dot{\beta} j} R(Q)_{ab}{}^{\dot{\alpha}}{}_{\dot{j}} k \chi_{\alpha}{}^{ik}{}_{\dot{j}} \gamma_b{}^{\alpha}{}_{\dot{\beta}} + (-\frac{7}{12} \bar{\mathcal{I}} + \frac{1}{48} \mathcal{D}^\dagger \mathcal{D}^\dagger \bar{\mathcal{H}}) \Lambda^{\dot{\alpha} j} \Lambda^{\dot{\beta} i} \epsilon_{\beta\dot{\gamma}} \nabla_b R(Q)_{ab}{}^{\dot{\gamma}}{}_{\dot{j}} \\
& + (-\frac{11}{20} \bar{\mathcal{I}} + \frac{1}{480} \mathcal{D}^\dagger \mathcal{D}^\dagger \bar{\mathcal{H}}) \Lambda^{\dot{\beta} j} \chi^{\dot{\alpha}}{}_{jk}{}^i \epsilon_{\beta\dot{\gamma}} \nabla_a \Lambda^{\dot{\gamma} k} + (-\frac{1}{2} \bar{\mathcal{I}} + \frac{1}{48} \mathcal{D}^\dagger \mathcal{D}^\dagger \bar{\mathcal{H}}) \Lambda^{\dot{\beta} j} \chi^{\dot{\alpha}}{}_{jk}{}^i \gamma_{ab\beta\dot{\gamma}} \nabla_b \Lambda^{\dot{\gamma} k} \\
& + (-\frac{1}{4} \bar{\mathcal{I}} - \frac{1}{16} \mathcal{D}^\dagger \mathcal{D}^\dagger \bar{\mathcal{H}}) \Lambda^{\dot{\beta} i} \Lambda^{\dot{\gamma} j} \epsilon_{\beta\dot{\gamma}} \nabla_b R(Q)_{ab}{}^{\dot{\alpha}}{}_{\dot{j}} + (-\frac{1}{4} \bar{\mathcal{I}} - \frac{1}{48} \mathcal{D}^\dagger \mathcal{D}^\dagger \bar{\mathcal{H}}) \Lambda^{\dot{\beta} i} R(Q)_{bc}{}^{\dot{\alpha}}{}_{\dot{j}} \gamma_{ab\beta\dot{\gamma}} \nabla_c \Lambda^{\dot{\gamma} j} \\
& + (-\frac{7}{32} \mathcal{D}^\dagger \bar{\mathcal{H}} - \frac{53}{96} \mathcal{D} \bar{\mathcal{I}}) \Lambda_{\alpha j} \gamma_a{}^{\alpha}{}_{\dot{\beta}} \nabla_b \Lambda^{\dot{\alpha} i} \nabla_b \Lambda^{\dot{\beta} j} + (-\frac{7}{32} \mathcal{D}^\dagger \bar{\mathcal{H}} - \frac{15}{32} \mathcal{D} \bar{\mathcal{I}}) \Lambda^{\dot{\beta} j} \gamma_a{}^{\alpha}{}_{\dot{\beta}} \nabla_b \Lambda_{\alpha j} \nabla_b \Lambda^{\dot{\alpha} i} + (-\frac{3}{16} \bar{\mathcal{H}} - \frac{5}{48} \mathcal{H}) \Lambda_{\alpha j} \Lambda^{\dot{\beta} i} R(S)^+{}_{ab}{}^{\dot{\alpha} j} \gamma_b{}^{\alpha}{}_{\dot{\beta}} \\
& + (-\frac{3}{16} \mathcal{D}^\dagger \bar{\mathcal{H}} - \frac{35}{96} \mathcal{D} \bar{\mathcal{I}}) \Lambda^{\dot{\beta} i} \gamma_a{}^{\alpha}{}_{\dot{\beta}} \nabla_b \Lambda_{\alpha j} \nabla_b \Lambda^{\dot{\alpha} j} + (-\frac{1}{6} \mathcal{D}^\dagger \bar{\mathcal{H}} - \frac{5}{24} \mathcal{D} \bar{\mathcal{I}}) \Lambda^{\dot{\beta} j} \chi_{\alpha}{}^{kl}{}_{\dot{j}} \chi^{\dot{\alpha}}{}_{kl}{}^i \gamma_a{}^{\alpha}{}_{\dot{\beta}} + (-\frac{1}{6} \mathcal{D}^\dagger \bar{\mathcal{H}} - \frac{1}{12} \mathcal{D} \bar{\mathcal{I}}) \Lambda^{\dot{\beta} j} \chi_{\alpha}{}^{ik}{}_{\dot{l}} \chi^{\dot{\alpha}}{}_{jk}{}^l \gamma_a{}^{\alpha}{}_{\dot{\beta}} \\
& + (-\frac{1}{8} \mathcal{D}^\dagger \bar{\mathcal{H}} - \frac{5}{12} \mathcal{D} \bar{\mathcal{I}}) \Lambda_{\alpha j} \Lambda^{\dot{\alpha} j} \gamma_a{}^{\alpha}{}_{\dot{\beta}} \nabla_b \nabla_b \Lambda^{\dot{\beta} i} + (-\frac{5}{48} \bar{\mathcal{H}} - \frac{1}{48} \mathcal{H}) \Lambda_{\alpha j} \Lambda^{\dot{\alpha} i} \epsilon^{\alpha\beta} \nabla_b R(Q)_{ab\beta}{}^j + (-\frac{3}{32} \mathcal{D}^\dagger \bar{\mathcal{H}} - \frac{23}{96} \mathcal{D} \bar{\mathcal{I}}) \Lambda_{\alpha j} \Lambda^{\dot{\alpha} i} \gamma_a{}^{\alpha}{}_{\dot{\beta}} \nabla_b \nabla_b \Lambda^{\dot{\beta} j} \\
& + (-\frac{3}{32} \mathcal{D}^\dagger \bar{\mathcal{H}} - \frac{5}{96} \mathcal{D} \bar{\mathcal{I}}) \Lambda_{\alpha j} \gamma_b{}^{\alpha}{}_{\dot{\beta}} \nabla_a \Lambda^{\dot{\beta} j} \nabla_b \Lambda^{\dot{\alpha} i} + (-\frac{17}{192} \mathcal{D}^\dagger \bar{\mathcal{H}} - \frac{25}{48} \mathcal{D} \bar{\mathcal{I}}) \Lambda_{\alpha j} \gamma_a{}^{\alpha}{}_{\dot{\beta}} \nabla_b \Lambda^{\dot{\alpha} j} \nabla_b \Lambda^{\dot{\beta} i} \\
& + (-\frac{1}{16} \bar{\mathcal{H}} + \frac{1}{16} \mathcal{H}) \Lambda_{\alpha j} \chi_{\beta}{}^{ij}{}_{\dot{k}} \gamma_{ab}{}^{\alpha\beta} \nabla_b \Lambda^{\dot{\alpha} k} + (-\frac{3}{64} \mathcal{D}^\dagger \bar{\mathcal{H}} - \frac{1}{24} \mathcal{D} \bar{\mathcal{I}}) \Lambda^{\dot{\alpha} j} \gamma_b{}^{\alpha}{}_{\dot{\beta}} \nabla_a \Lambda_{\alpha j} \nabla_b \Lambda^{\dot{\beta} i} + (-\frac{1}{24} \bar{\mathcal{H}} + \frac{1}{24} \mathcal{H}) \Lambda^{\dot{\alpha} j} R(Q)_{ab\alpha}{}^i \epsilon^{\alpha\beta} \nabla_b \Lambda_{\beta j} \\
& + (-\frac{7}{192} \mathcal{D}^\dagger \bar{\mathcal{H}} + \frac{5}{48} \mathcal{D} \bar{\mathcal{I}}) \Lambda_{\alpha j} \gamma_b{}^{\alpha}{}_{\dot{\beta}} \nabla_a \Lambda^{\dot{\alpha} j} \nabla_b \Lambda^{\dot{\beta} i} + (-\frac{1}{32} \bar{\mathcal{H}} + \frac{1}{32} \mathcal{H}) \Lambda_{\alpha j} \Lambda^{\dot{\alpha} k} \epsilon^{\alpha\beta} \nabla_a \chi_{\beta}{}^{ij}{}_{\dot{k}} + (-\frac{1}{32} \mathcal{D}^\dagger \bar{\mathcal{H}} - \frac{23}{192} \mathcal{D} \bar{\mathcal{I}}) \Lambda^{\dot{\beta} i} \gamma_b{}^{\alpha}{}_{\dot{\beta}} \nabla_a \Lambda_{\alpha j} \nabla_b \Lambda^{\dot{\alpha} j} \\
& + (-\frac{1}{32} \mathcal{D}^\dagger \bar{\mathcal{H}} - \frac{5}{48} \mathcal{D} \bar{\mathcal{I}}) \Lambda^{\dot{\alpha} j} \gamma_b{}^{\alpha}{}_{\dot{\beta}} \nabla_b \Lambda_{\alpha j} \nabla_a \Lambda^{\dot{\beta} i} + (-\frac{1}{32} \mathcal{D}^\dagger \bar{\mathcal{H}} - \frac{1}{48} \mathcal{D} \bar{\mathcal{I}}) \Lambda^{\dot{\alpha} j} \Lambda^{\dot{\beta} i} \gamma_a{}^{\alpha}{}_{\dot{\beta}} \nabla_b \nabla_b \Lambda_{\alpha j} \\
& + (-\frac{1}{48} \mathcal{D}^\dagger \bar{\mathcal{H}} - \frac{17}{192} \mathcal{D} \bar{\mathcal{I}}) \Lambda^{\dot{\alpha} i} \gamma_b{}^{\alpha}{}_{\dot{\beta}} \nabla_b \Lambda_{\alpha j} \nabla_a \Lambda^{\dot{\beta} j} + (-\frac{1}{96} \mathcal{D}^\dagger \bar{\mathcal{H}} - \frac{1}{96} \mathcal{D} \bar{\mathcal{I}}) \Lambda^{\dot{\alpha} i} \Lambda^{\dot{\beta} j} \gamma_b{}^{\alpha}{}_{\dot{\beta}} \nabla_a \nabla_b \Lambda_{\alpha j} \\
& + (-\frac{1}{192} \mathcal{D}^\dagger \bar{\mathcal{H}} + \frac{5}{96} \mathcal{D} \bar{\mathcal{I}}) \Lambda^{\dot{\beta} j} \gamma_b{}^{\alpha}{}_{\dot{\beta}} \nabla_b \Lambda_{\alpha j} \nabla_a \Lambda^{\dot{\alpha} i} + (\frac{1}{96} \bar{\mathcal{H}} - \frac{1}{96} \mathcal{H}) \Lambda^{\dot{\alpha} i} R(Q)_{ab\alpha}{}^j \epsilon^{\alpha\beta} \nabla_b \Lambda_{\beta j} + (\frac{1}{96} \mathcal{D}^\dagger \bar{\mathcal{H}} + \frac{1}{96} \mathcal{D} \bar{\mathcal{I}}) \Lambda^{\dot{\alpha} j} \Lambda^{\dot{\beta} i} \gamma_b{}^{\alpha}{}_{\dot{\beta}} \nabla_a \nabla_b \Lambda_{\alpha j} \\
& + (\frac{1}{96} \mathcal{D}^\dagger \bar{\mathcal{H}} + \frac{5}{96} \mathcal{D} \bar{\mathcal{I}}) \Lambda^{\dot{\beta} j} \gamma_b{}^{\alpha}{}_{\dot{\beta}} \nabla_a \Lambda_{\alpha j} \nabla_b \Lambda^{\dot{\alpha} i} + (\frac{1}{48} \bar{\mathcal{H}} - \frac{1}{48} \mathcal{H}) \Lambda_{\alpha j} \chi_{\beta}{}^{ij}{}_{\dot{k}}$$

$$\begin{aligned} [\hat{\Omega}_a^{\dot{\alpha}i}]_{3,cont.} = & -\frac{1}{3} \bar{\mathcal{I}} T_{abjk} \Lambda^{\dot{\alpha}l} \Lambda^{\dot{\beta}j} \chi_{\alpha}{}^i{}_{l\gamma b}{}^{\dot{\alpha}}{}_{\dot{\beta}} + \frac{1}{8} \bar{\mathcal{H}} T_{ab}{}^{jk} \Lambda_{\alpha l} \Lambda^{\dot{\alpha}i} \chi^{\dot{\beta}}{}_{jk}{}^l{}_{\gamma b}{}^{\alpha}{}_{\dot{\beta}} + \frac{1}{12} \bar{\mathcal{H}} \Lambda_{\alpha j} \Lambda^{\dot{\beta}j} \bar{P}_b \gamma_a{}^{\alpha}{}_{\dot{\beta}} \nabla_b \Lambda^{\dot{\alpha}i} - \frac{1}{6} \bar{\mathcal{H}} \Lambda_{\alpha j} \chi^{\dot{\alpha}}{}_{kl}{}^j \chi^{\dot{\beta}}{}_{mn}{}^i \gamma_a{}^{\alpha}{}_{\dot{\beta}} \varepsilon^{klmn} \\ & + \frac{1}{12} \mathcal{D}^{\dagger} \bar{\mathcal{I}} P_a \Lambda^{\dot{\beta}i} \Lambda^{\dot{\gamma}j} R(Q)_{bc}{}^{\dot{\alpha}}{}_{\dot{j}} \gamma_{bc\dot{\beta}\dot{\gamma}} + \frac{1}{3} \mathcal{D}^{\dagger} \bar{\mathcal{I}} P_a \Lambda^{\dot{\alpha}j} \Lambda^{\dot{\beta}k} \chi^{\dot{\gamma}}{}_{jk}{}^i{}_{\epsilon\dot{\beta}\dot{\gamma}} + \frac{1}{6} \mathcal{D}^{\dagger} \bar{\mathcal{I}} T_{bcjk} \Lambda^{\dot{\alpha}i} \Lambda^{\dot{\beta}j} \gamma_{bc\dot{\beta}\dot{\gamma}} \nabla_a \Lambda^{\dot{\gamma}k} \\ & - \frac{1}{6} \mathcal{D}^{\dagger} \bar{\mathcal{I}} T_{bcjk} \Lambda^{\dot{\alpha}j} \Lambda^{\dot{\beta}i} \gamma_{bc\dot{\beta}\dot{\gamma}} \nabla_a \Lambda^{\dot{\gamma}k} + \frac{1}{6} \mathcal{D}^{\dagger} \bar{\mathcal{I}} T_{bcjk} \Lambda^{\dot{\beta}j} \Lambda^{\dot{\gamma}k} \gamma_{bc\dot{\beta}\dot{\gamma}} \nabla_a \Lambda^{\dot{\alpha}i} + \frac{1}{36} \mathcal{D}^{\dagger} \bar{\mathcal{I}} \Lambda^{\dot{\alpha}i} \Lambda^{\dot{\beta}j} \Lambda^{\dot{\gamma}k} \gamma_{bc\dot{\beta}\dot{\gamma}} \nabla_a T_{bcjk} \\ & - \frac{1}{18} \mathcal{D}^{\dagger} \bar{\mathcal{I}} \Lambda^{\dot{\alpha}j} \Lambda^{\dot{\beta}i} \Lambda^{\dot{\gamma}k} \gamma_{bc\dot{\beta}\dot{\gamma}} \nabla_a T_{bcjk} + \frac{1}{24} \mathcal{D}^{\dagger} \bar{\mathcal{H}} E_{jk} \Lambda^{\dot{\alpha}l} \Lambda^{\dot{\beta}j} \chi_{\alpha}{}^{ik}{}_{l\gamma a}{}^{\alpha}{}_{\dot{\beta}} + \frac{1}{48} \mathcal{D}^{\dagger} \bar{\mathcal{H}} \Lambda_{\alpha j} \Lambda^{\dot{\alpha}i} \Lambda^{\dot{\beta}k} R(V)_{ab}{}^j{}_{k\gamma b}{}^{\alpha}{}_{\dot{\beta}} \\ & - \frac{1}{48} \mathcal{D}^{\dagger} \bar{\mathcal{H}} \Lambda_{\alpha j} \Lambda^{\dot{\alpha}k} \Lambda^{\dot{\beta}i} R(V)_{ab}{}^j{}_{k\gamma b}{}^{\alpha}{}_{\dot{\beta}} + \frac{1}{8} \mathcal{D}^{\dagger} \mathcal{D}^{\dagger} \bar{\mathcal{H}} T_{abjk} \Lambda^{\dot{\alpha}j} \Lambda^{\dot{\beta}l} \chi_{\alpha}{}^{ik}{}_{l\gamma b}{}^{\alpha}{}_{\dot{\beta}} - \frac{1}{12} \mathcal{D}^{\dagger} \mathcal{D}^{\dagger} \mathcal{D}^{\dagger} \bar{\mathcal{H}} T_{abjk} \Lambda^{\dot{\beta}i} \Lambda^{\dot{\gamma}j} \epsilon_{\dot{\beta}\dot{\gamma}} \nabla_b \Lambda^{\dot{\alpha}k} \\ & - \frac{2}{9} \mathcal{D}^{\dagger} \mathcal{I} T_{ab}{}^{ij} \Lambda_{\alpha j} \Lambda^{\dot{\alpha}k} \epsilon^{\alpha\beta} \nabla_b \Lambda_{\beta k} + \frac{1}{16} \mathcal{D}^{\dagger} \mathcal{I} \Lambda_{\alpha j} \Lambda_{\beta k} \Lambda^{\dot{\alpha}j} \gamma_{ab}{}^{\alpha\beta} \nabla_c T_{bc}{}^{ik} + \frac{1}{16} \mathcal{D}^{\dagger} \mathcal{I} \Lambda_{\alpha j} \Lambda_{\beta k} \Lambda^{\dot{\alpha}j} \gamma_{bc}{}^{\alpha\beta} \nabla_b T_{ac}{}^{ik} \\ & - \frac{5}{48} \mathcal{D}^{\dagger} \mathcal{I} \Lambda_{\alpha j} \Lambda^{\dot{\alpha}i} R(Q)_{ab\beta}{}^j \bar{P}_b \epsilon^{\alpha\beta} + \frac{1}{8} \mathcal{D}^{\dagger} \mathcal{I} \Lambda_{\alpha j} \Lambda^{\dot{\alpha}j} R(Q)_{ab\beta}{}^i \bar{P}_b \epsilon^{\alpha\beta} - \frac{1}{48} \mathcal{D}^{\dagger} \mathcal{I} \Lambda_{\alpha j} \chi^{\dot{\alpha}}{}_{kl}{}^i \epsilon^{\alpha\beta} \nabla_a \Lambda_{\beta m} \varepsilon^{jklm} \\ & + \frac{1}{48} \mathcal{D}^{\dagger} \mathcal{I} \Lambda_{\alpha j} \chi^{\dot{\alpha}}{}_{kl}{}^j \epsilon^{\alpha\beta} \nabla_a \Lambda_{\beta m} \varepsilon^{iklm} + \frac{1}{24} \mathcal{D}^{\dagger} \mathcal{I} \Lambda_{\alpha j} \chi^{\dot{\alpha}}{}_{kl}{}^m \epsilon^{\alpha\beta} \nabla_a \Lambda_{\beta m} \varepsilon^{ijkl} + \frac{1}{36} \mathcal{D}^{\dagger} \mathcal{I} \Lambda_{\alpha j} \chi^{\dot{\alpha}}{}_{kl}{}^i \gamma_{ab}{}^{\alpha\beta} \nabla_b \Lambda_{\beta m} \varepsilon^{jklm} \\ & + \frac{1}{72} \mathcal{D}^{\dagger} \mathcal{I} \Lambda_{\alpha j} \chi^{\dot{\alpha}}{}_{kl}{}^j \gamma_{ab}{}^{\alpha\beta} \nabla_b \Lambda_{\beta m} \varepsilon^{iklm} - \frac{1}{72} \mathcal{D}^{\dagger} \mathcal{I} \Lambda_{\alpha j} \chi^{\dot{\alpha}}{}_{kl}{}^m \gamma_{ab}{}^{\alpha\beta} \nabla_b \Lambda_{\beta m} \varepsilon^{ijkl} - \frac{1}{48} \mathcal{D} \bar{\mathcal{I}} D^{ij}{}_{kl} \Lambda_{\alpha j} \Lambda^{\dot{\alpha}k} \Lambda^{\dot{\beta}l} \gamma_a{}^{\alpha}{}_{\dot{\beta}} \\ & + \frac{1}{48} \mathcal{D} \bar{\mathcal{I}} E^{ij} \Lambda_{\alpha k} \Lambda^{\dot{\alpha}l} \chi^{\dot{\beta}}{}_{jl}{}^k \gamma_a{}^{\alpha}{}_{\dot{\beta}} + \frac{1}{6} \mathcal{D} \bar{\mathcal{I}} \Lambda_{\alpha j} \Lambda^{\dot{\beta}j} \gamma_b{}^{\dot{\alpha}\alpha} \gamma_{ac\dot{\beta}\dot{\gamma}} \nabla_b \nabla_c \Lambda^{\dot{\gamma}i} - \frac{1}{64} \mathcal{D} \bar{\mathcal{I}} \Lambda_{\alpha j} \gamma_b{}^{\alpha}{}_{\dot{\beta}} \nabla_c \Lambda^{\dot{\alpha}i} \nabla_d \Lambda^{\dot{\beta}j} \varepsilon_{abcd} \\ & + \frac{1}{24} \mathcal{D} \bar{\mathcal{I}} \Lambda^{\dot{\beta}i} \Lambda^{\dot{\gamma}j} \epsilon_{\dot{\beta}\dot{\gamma}} \gamma_b{}^{\dot{\alpha}\alpha} \nabla_a \nabla_b \Lambda_{\alpha j} + \frac{1}{20} \mathcal{D} \mathcal{H} \Lambda_{\alpha j} R(Q)_{bc\gamma}{}^i R(Q)_{bc\gamma}{}^j \epsilon^{\beta\gamma} \gamma_a{}^{\dot{\alpha}\alpha} - \frac{1}{3} \mathcal{D} \mathcal{H} \Lambda_{\alpha j} \chi_{\beta}{}^{ik}{}_{l\chi\gamma}{}^{jl}{}_{k\epsilon} \epsilon^{\alpha\beta} \gamma_a{}^{\dot{\alpha}\gamma} \\ & - \frac{1}{6} \mathcal{D} \mathcal{H} \Lambda_{\alpha j} \chi_{\beta}{}^{ik}{}_{l\chi\gamma}{}^{jl}{}_{k\epsilon} \epsilon^{\alpha\gamma} \gamma_a{}^{\dot{\alpha}\beta} + \frac{1}{6} \mathcal{D} \mathcal{H} \Lambda_{\alpha j} \chi_{\beta}{}^{ik}{}_{l\chi\gamma}{}^{jl}{}_{k\epsilon} \epsilon^{\beta\gamma} \gamma_a{}^{\dot{\alpha}\alpha} + \frac{1}{12} \mathcal{H} \Lambda_{\alpha j} \Lambda^{\dot{\beta}k} \gamma_a{}^{\alpha}{}_{\dot{\beta}} \gamma_b{}^{\dot{\alpha}\beta} \nabla_b \chi_{\beta}{}^{ij}{}_{\gamma k} \\ & + (-\frac{17}{12} \bar{\mathcal{I}} - \frac{103}{576} \mathcal{D}^{\dagger} \mathcal{D}^{\dagger} \bar{\mathcal{H}}) P_b \Lambda_{\alpha j} \Lambda^{\dot{\beta}i} \gamma_a{}^{\alpha}{}_{\dot{\beta}} \nabla_b \Lambda^{\dot{\alpha}j} + (-\bar{\mathcal{I}} - \frac{1}{18} \mathcal{D}^{\dagger} \mathcal{D}^{\dagger} \bar{\mathcal{H}}) P_b \Lambda_{\alpha j} \Lambda^{\dot{\beta}j} \gamma_a{}^{\alpha}{}_{\dot{\beta}} \nabla_b \Lambda^{\dot{\alpha}i} \\ & + (-\frac{17}{18} \bar{\mathcal{I}} - \frac{1}{12} \mathcal{D}^{\dagger} \mathcal{D}^{\dagger} \bar{\mathcal{H}}) P_b \Lambda_{\alpha j} \Lambda^{\dot{\alpha}j} \gamma_b{}^{\alpha}{}_{\dot{\beta}} \nabla_a \Lambda^{\dot{\beta}i} + (-\frac{5}{6} \bar{\mathcal{I}} - \frac{5}{72} \mathcal{D}^{\dagger} \mathcal{D}^{\dagger} \bar{\mathcal{H}}) P_a \Lambda_{\alpha j} \Lambda^{\dot{\beta}j} \gamma_b{}^{\alpha}{}_{\dot{\beta}} \nabla_b \Lambda^{\dot{\alpha}i} \\ & + (-\frac{23}{36} \bar{\mathcal{I}} - \frac{13}{144} \mathcal{D}^{\dagger} \mathcal{D}^{\dagger} \bar{\mathcal{H}}) P_a \Lambda_{\alpha j} \Lambda^{\dot{\alpha}j} \gamma_b{}^{\alpha}{}_{\dot{\beta}} \nabla_b \Lambda^{\dot{\beta}i} + (-\frac{19}{36} \bar{\mathcal{I}} - \frac{1}{16} \mathcal{D}^{\dagger} \mathcal{D}^{\dagger} \bar{\mathcal{H}}) P_b \Lambda_{\alpha j} \Lambda^{\dot{\beta}j} \gamma_b{}^{\alpha}{}_{\dot{\beta}} \nabla_a \Lambda^{\dot{\alpha}i} \\ & + (-\frac{1}{2} \mathcal{D}^{\dagger} \bar{\mathcal{I}} - \frac{1}{16} \mathcal{D}^{\dagger} \mathcal{D}^{\dagger} \mathcal{D}^{\dagger} \bar{\mathcal{H}}) P_b \Lambda^{\dot{\beta}i} \Lambda^{\dot{\gamma}j} R(Q)_{ab}{}^{\dot{\alpha}}{}_{\dot{j}} \epsilon_{\dot{\beta}\dot{\gamma}} + (-\frac{17}{40} \mathcal{D}^{\dagger} \bar{\mathcal{I}} + \frac{17}{240} \mathcal{D}^{\dagger} \mathcal{D}^{\dagger} \mathcal{D}^{\dagger} \bar{\mathcal{H}}) T_{abjk} \Lambda^{\dot{\alpha}j} \Lambda^{\dot{\beta}k} \epsilon_{\dot{\beta}\dot{\gamma}} \nabla_b \Lambda^{\dot{\gamma}i} \\ & + (-\frac{35}{96} \bar{\mathcal{I}} + \frac{1}{288} \mathcal{D}^{\dagger} \mathcal{D}^{\dagger} \bar{\mathcal{H}}) P_b \Lambda^{\dot{\alpha}i} \Lambda^{\dot{\beta}j} \gamma_a{}^{\alpha}{}_{\dot{\beta}} \nabla_b \Lambda_{\alpha j} + (-\frac{1}{3} \bar{\mathcal{H}} + \frac{1}{12} \mathcal{H}) \Lambda_{\alpha j} \chi_{\beta}{}^{ij}{}_{k\gamma b}{}^{\alpha}{}_{\dot{\beta}} \gamma_a{}^{\dot{\alpha}\beta} \nabla_b \Lambda^{\dot{\beta$$

$$\begin{aligned}
[\hat{\Omega}_a^{\dot{\alpha}i}]_{3,cont.} = & +(-\frac{131}{2304}\bar{\mathcal{H}} + \frac{67}{2304}\mathcal{H})\Lambda_{\alpha j}\Lambda^{\dot{\beta}i}\bar{P}_a\gamma_b{}^\alpha{}_{\dot{\beta}}\nabla_b\Lambda^{\dot{\alpha}j} + (-\frac{163}{2880}\mathcal{D}^\dagger\bar{\mathcal{I}} + \frac{3}{80}\mathcal{D}\mathcal{H})T_{bc}{}^{ij}\Lambda_{\alpha k}\Lambda^{\dot{\alpha}k}\gamma_{bc}{}^{\alpha\beta}\nabla_a\Lambda_{\beta j} \\
& + (-\frac{1}{18}\bar{\mathcal{I}} + \frac{1}{48}\mathcal{D}^\dagger\mathcal{D}^\dagger\bar{\mathcal{H}})E_{jk}\Lambda^{\dot{\beta}i}\Lambda^{\dot{\gamma}j}\gamma_{ab\dot{\beta}\dot{\gamma}}\nabla_b\Lambda^{\dot{\alpha}k} + (-\frac{5}{96}\bar{\mathcal{H}} - \frac{1}{32}\mathcal{H})\Lambda_{\alpha j}\Lambda^{\dot{\beta}k}\gamma_a{}^\beta{}_{\dot{\beta}}\gamma_b{}^{\dot{\alpha}\alpha}\nabla_b\chi_{\beta}{}^{ij}{}_k \\
& + (-\frac{5}{96}\bar{\mathcal{H}} - \frac{1}{32}\mathcal{H})\Lambda_{\alpha j}\chi^{\dot{\alpha}}{}_{kl}{}^i\chi^{\dot{\beta}}{}_{mn}{}^j\gamma_a{}^\alpha{}_{\dot{\beta}}\epsilon^{\dot{\beta}klmn} + (-\frac{5}{96}\bar{\mathcal{H}} + \frac{1}{32}\mathcal{H})\Lambda_{\alpha j}\Lambda^{\dot{\beta}i}\gamma_a{}^\beta{}_{\dot{\beta}}\gamma_b{}^{\dot{\alpha}\alpha}\nabla_c R(Q)_{bc\beta}{}^j \\
& + (-\frac{1}{144}\bar{\mathcal{I}} + \frac{1}{64}\mathcal{D}^\dagger\mathcal{D}^\dagger\bar{\mathcal{H}})E_{jk}\Lambda^{\dot{\alpha}i}\Lambda^{\dot{\beta}j}\epsilon_{\dot{\beta}\dot{\gamma}}\nabla_a\Lambda^{\dot{\gamma}k} + (-\frac{107}{2304}\bar{\mathcal{H}} - \frac{13}{256}\mathcal{H})\Lambda^{\dot{\alpha}j}\Lambda^{\dot{\beta}i}\bar{P}_b\gamma_a{}^\alpha{}_{\dot{\beta}}\nabla_b\Lambda_{\alpha j} \\
& + (-\frac{1}{24}\bar{\mathcal{I}} + \frac{1}{64}\mathcal{D}^\dagger\mathcal{D}^\dagger\bar{\mathcal{H}})E_{jk}\Lambda^{\dot{\beta}j}\Lambda^{\dot{\gamma}k}\epsilon_{\dot{\beta}\dot{\gamma}}\nabla_a\Lambda^{\dot{\alpha}i} + (-\frac{1}{24}\bar{\mathcal{H}} - \frac{1}{24}\mathcal{H})\Lambda^{\dot{\beta}j}\chi_{\alpha}{}^{ik}{}_j\gamma_a{}^\beta{}_{\dot{\beta}}\gamma_b{}^{\dot{\alpha}\alpha}\nabla_b\Lambda_{\beta k} \\
& + (-\frac{1}{24}\bar{\mathcal{H}} + \frac{1}{24}\mathcal{H})T_{ab}{}^{ij}\Lambda_{\alpha k}\Lambda^{\dot{\alpha}l}\chi^{\dot{\beta}}{}_{jl}{}^k\gamma_b{}^\alpha{}_{\dot{\beta}} + (-\frac{1}{24}\mathcal{D}^\dagger\bar{\mathcal{H}} - \frac{1}{24}\mathcal{D}\bar{\mathcal{I}})\Lambda^{\dot{\beta}j}\gamma_a{}^{\dot{\alpha}\alpha}\gamma_{bc\dot{\beta}\dot{\gamma}}\nabla_b\Lambda_{\alpha j}\nabla_c\Lambda^{\dot{\gamma}i} \\
& + (-\frac{1}{24}\mathcal{D}^\dagger\bar{\mathcal{I}} - \frac{1}{12}\mathcal{D}\mathcal{H})T_{bc}{}^{jk}\Lambda_{\alpha j}\Lambda_{\beta k}\gamma_{ab}{}^{\alpha\beta}\nabla_c\Lambda^{\dot{\alpha}i} + (-\frac{11}{288}\bar{\mathcal{H}} + \frac{19}{288}\mathcal{H})\Lambda_{\alpha j}\Lambda^{\dot{\beta}j}\bar{P}_a\gamma_b{}^\alpha{}_{\dot{\beta}}\nabla_b\Lambda^{\dot{\alpha}i} \\
& + (-\frac{3}{80}\mathcal{D}^\dagger\bar{\mathcal{I}} + \frac{13}{480}\mathcal{D}^\dagger\mathcal{D}^\dagger\mathcal{D}^\dagger\bar{\mathcal{H}})T_{bcjk}\Lambda^{\dot{\alpha}j}\Lambda^{\dot{\beta}k}\gamma_{ab\dot{\beta}\dot{\gamma}}\nabla_c\Lambda^{\dot{\gamma}i} + (-\frac{1}{30}\mathcal{D}^\dagger\bar{\mathcal{H}} - \frac{1}{48}\mathcal{D}\bar{\mathcal{I}})E^{ij}\Lambda_{\alpha j}\Lambda^{\dot{\beta}k}R(Q)_{ab}{}^{\dot{\alpha}}{}_k\gamma_b{}^\alpha{}_{\dot{\beta}} \\
& + (-\frac{1}{32}\bar{\mathcal{H}} + \frac{3}{32}\mathcal{H})\Lambda_{\alpha j}\Lambda^{\dot{\beta}i}\gamma_b{}^\alpha{}_{\dot{\beta}}\gamma_c{}^{\dot{\alpha}\beta}\nabla_b R(Q)_{ac\beta}{}^j + (-\frac{43}{1536}\bar{\mathcal{H}} - \frac{5}{1536}\mathcal{H})E^{ij}\Lambda_{\alpha j}\Lambda_{\beta k}\epsilon^{\alpha\beta}\nabla_a\Lambda^{\dot{\alpha}k} \\
& + (-\frac{1}{36}\bar{\mathcal{I}} - \frac{1}{192}\mathcal{D}^\dagger\mathcal{D}^\dagger\bar{\mathcal{H}})\Lambda^{\dot{\alpha}i}\Lambda^{\dot{\beta}j}\Lambda^{\dot{\gamma}k}\epsilon_{\dot{\beta}\dot{\gamma}}\nabla_a E_{jk} + (-\frac{13}{480}\mathcal{D}^\dagger\bar{\mathcal{H}} - \frac{283}{5760}\mathcal{D}\bar{\mathcal{I}})\Lambda^{\dot{\alpha}j}\gamma_b{}^\alpha{}_{\dot{\beta}}\nabla_c\Lambda_{\alpha j}\nabla_d\Lambda^{\dot{\beta}i}\epsilon_{abcd} \\
& + (-\frac{19}{720}\mathcal{D}^\dagger\bar{\mathcal{I}} - \frac{7}{320}\mathcal{D}\mathcal{H})\Lambda_{\alpha j}\Lambda_{\beta k}\Lambda^{\dot{\alpha}i}\gamma_{bc}{}^{\alpha\beta}\nabla_a T_{bc}{}^{jk} + (-\frac{5}{192}\bar{\mathcal{H}} - \frac{7}{192}\mathcal{H})\Lambda_{\alpha j}R(Q)_{bc\beta}{}^i\gamma_a{}^\beta{}_{\dot{\beta}}\gamma_b{}^{\dot{\alpha}\alpha}\nabla_c\Lambda^{\dot{\beta}j} \\
& + (-\frac{5}{192}\bar{\mathcal{H}} + \frac{17}{192}\mathcal{H})\Lambda_{\alpha j}\Lambda^{\dot{\beta}j}\gamma_b{}^\alpha{}_{\dot{\beta}}\gamma_c{}^{\dot{\alpha}\beta}\nabla_b R(Q)_{ac\beta}{}^i + (-\frac{103}{4608}\bar{\mathcal{H}} + \frac{125}{1536}\mathcal{H})\Lambda_{\alpha j}\Lambda^{\dot{\beta}i}\Lambda^{\dot{\beta}j}\gamma_b{}^\alpha{}_{\dot{\beta}}\nabla_b\bar{P}_a \\
& + (-\frac{1}{48}\bar{\mathcal{H}} + \frac{1}{48}\mathcal{H})\Lambda^{\dot{\beta}j}\chi_{\alpha}{}^{ik}{}_j\gamma_b{}^\beta{}_{\dot{\beta}}\gamma_a{}^{\dot{\alpha}\alpha}\nabla_b\Lambda_{\beta k} + (-\frac{1}{48}\mathcal{D}^\dagger\bar{\mathcal{I}} - \frac{1}{4}\mathcal{D}\mathcal{H})T_{bc}{}^{ij}\Lambda_{\alpha j}\Lambda_{\beta k}\gamma_{ab}{}^{\alpha\beta}\nabla_c\Lambda^{\dot{\alpha}k} \\
& + (-\frac{1}{48}\mathcal{D}^\dagger\bar{\mathcal{I}} - \frac{1}{24}\mathcal{D}\mathcal{H})\Lambda_{\alpha j}\Lambda_{\beta k}\gamma_{bc}{}^{\alpha\beta}\nabla_b R(Q)_{ac}{}^{\dot{\alpha}}{}_l\epsilon^{ijkl} + (-\frac{1}{48}\mathcal{D}^\dagger\bar{\mathcal{I}} - \frac{1}{24}\mathcal{D}\mathcal{H})\Lambda_{\alpha j}R(Q)_{ab}{}^{\dot{\alpha}}{}_k\epsilon^{\alpha\beta}\nabla_b\Lambda_{\beta l}\epsilon^{ijkl} \\
& + (-\frac{1}{48}\mathcal{D}^\dagger\bar{\mathcal{I}} - \frac{1}{24}\mathcal{D}\mathcal{H})\Lambda_{\alpha j}R(Q)_{ab}{}^{\dot{\alpha}}{}_k\gamma_{bc}{}^{\alpha\beta}\nabla_c\Lambda_{\beta l}\epsilon^{ijkl} + (-\frac{11}{576}\bar{\mathcal{H}} + \frac{5}{64}\mathcal{H})\Lambda_{\alpha j}\Lambda^{\dot{\alpha}i}\Lambda^{\dot{\beta}j}\gamma_a{}^\alpha{}_{\dot{\beta}}\nabla_b\bar{P}_b \\
& + (-\frac{43}{2304}\bar{\mathcal{H}} + \frac{3}{256}\mathcal{H})\Lambda^{\dot{\alpha}j}\Lambda^{\dot{\beta}i}\bar{P}_a\gamma_b{}^\alpha{}_{\dot{\beta}}\nabla_b\Lambda_{\alpha j} + (-\frac{5}{288}\bar{\mathcal{H}} + \frac{5}{288}\mathcal{H})E^{jk}\Lambda_{\alpha j}\Lambda^{\dot{\alpha}i}\gamma_{ab}{}^{\alpha\beta}\nabla_b\Lambda_{\beta k} \\
& + (-\frac{1}{60}\mathcal{D}^\dagger\bar{\mathcal{I}} - \frac{11}{480}\mathcal{D}^\dagger\mathcal{D}^\dagger\mathcal{D}^\dagger\bar{\mathcal{H}})T_{abjk}\Lambda^{\dot{\beta}i}\Lambda^{\dot{\gamma}j}\gamma_{bc\dot{\beta}\dot{\gamma}}\nabla_c\Lambda^{\dot{\alpha}k} + (-\frac{1}{64}\bar{\mathcal{H}} + \frac{5}{64}\mathcal{H})\Lambda^{\dot{\beta}j}R(Q)_{ab\alpha}{}^i\gamma_c{}^\beta{}_{\dot{\beta}}\gamma_b{}^{\dot{\alpha}\alpha}\nabla_c\Lambda_{\beta j} \\
& + (-\frac{1}{64}\mathcal{D}^\dagger\bar{\mathcal{H}} - \frac{7}{384}\mathcal{D}\bar{\mathcal{I}})\Lambda^{\dot{\alpha}j}\Lambda^{\dot{\beta}i}R(Q)_{ab}{}^{\dot{\gamma}}{}_j\bar{P}_b\epsilon_{\dot{\beta}\dot{\gamma}} + (-\frac{1}{72}\bar{\mathcal{I}} + \frac{1}{96}\mathcal{D}^\dagger\mathcal{D}^\dagger\bar{\mathcal{H}})E_{jk}\Lambda^{\dot{\alpha}j}\Lambda^{\dot{\beta}i}\gamma_{ab\dot{\beta}\dot{\gamma}}\nabla_b\Lambda^{\dot{\gamma}k} \\
& + (-\frac{1}{72}\mathcal{D}^\dagger\bar{\mathcal{I}} + \frac{1}{96}\mathcal{D}^\dagger\mathcal{D}^\dagger\mathcal{D}^\dagger\bar{\mathcal{H}})\Lambda^{\dot{\alpha}i}\Lambda^{\dot{\beta}j}\Lambda^{\dot{\gamma}k}\gamma_{ab\dot{\beta}\dot{\gamma}}\nabla_c T_{bcjk} + (-\frac{1}{72}\mathcal{D}^\dagger\bar{\mathcal{I}} + \frac{1}{96}\mathcal{D}^\dagger\mathcal{D}^\dagger\mathcal{D}^\dagger\bar{\mathcal{H}})\Lambda^{\dot{\alpha}i}\Lambda^{\dot{\beta}j}\Lambda^{\dot{\gamma}k}\gamma_{bc\dot{\beta}\dot{\gamma}}\nabla_b T_{acjk} \\
& + (-\frac{5}{384}\bar{\mathcal{H}} - \frac{7}{384}\mathcal{H})\Lambda_{\alpha j}R(Q)_{bc\beta}{}^j\gamma_a{}^\alpha{}_{\dot{\beta}}\gamma_b{}^{\dot{\alpha}\beta}\nabla_c\Lambda^{\dot{\beta}i} + (-\frac{3}{256}\bar{\mathcal{H}} - \frac{37}{2304}\mathcal{H})\Lambda^{\dot{\alpha}i}\Lambda^{\dot{\beta}j}\bar{P}_b\gamma_b{}^\alpha{}_{\dot{\beta}}\nabla_a\Lambda_{\alpha j} \\
& + (-\frac{1}{96}\bar{\mathcal{H}} + \frac{3}{32}\mathcal{H})\Lambda^{\dot{\beta}j}R(Q)_{bc\alpha}{}^i\gamma_a{}^\beta{}_{\dot{\beta}}\gamma_b{}^{\dot{\alpha}\alpha}\nabla_c\Lambda_{\beta j} + (-\frac{1}{96}\mathcal{D}^\dagger\bar{\mathcal{H}} - \frac{1}{32}\mathcal{D}\bar{\mathcal{I}})\Lambda^{\dot{\beta}i}\Lambda^{\dot{\gamma}j}\gamma_b{}^{\dot{\alpha}\alpha}\gamma_{ac\dot{\beta}\dot{\gamma}}\nabla_b\nabla_c\Lambda_{\alpha j} \\
& + (-\frac{1}{96}\mathcal{D}^\dagger\bar{\mathcal{I}} - \frac{1}{80}\mathcal{D}\mathcal{H})T_{bc}{}^{jk}\Lambda_{\alpha j}\Lambda^{\dot{\alpha}i}\gamma_{bc}{}^{\alpha\beta}\nabla_a\Lambda_{\beta k} + (-\frac{5}{576}\bar{\mathcal{H}} + \frac{5}{576}\mathcal{H})E^{ij}\Lambda_{\alpha k}\Lambda^{\dot{\alpha}k}\gamma_{ab}{}^{\alpha\beta}\nabla_b\Lambda_{\beta j} \\
& + (-\frac{1}{120}\mathcal{D}^\dagger\bar{\mathcal{I}} + \frac{1}{320}\mathcal{D}^\dagger\mathcal{D}^\dagger\mathcal{D}^\dagger\bar{\mathcal{H}})T_{abjk}\Lambda^{\dot{\alpha}i}\Lambda^{\dot{\beta}j}\gamma_{bc\dot{\beta}\dot{\gamma}}\nabla_c\Lambda^{\dot{\gamma}k} + (-\frac{1}{120}\mathcal{D}^\dagger\bar{\mathcal{I}} + \frac{1}{320}\mathcal{D}^\dagger\mathcal{D}^\dagger\mathcal{D}^\dagger\bar{\mathcal{H}})T_{bcjk}\Lambda^{\dot{\alpha}j}\Lambda^{\dot{\beta}i}\gamma_{ab\dot{\beta}\dot{\gamma}}\nabla_c\Lambda^{\dot{\gamma}k} \\
& + (-\frac{11}{1440}\mathcal{D}^\dagger\bar{\mathcal{I}} - \frac{1}{120}\mathcal{D}\mathcal{H})T_{bc}{}^{jk}\Lambda_{\alpha j}\Lambda_{\beta k}\gamma_{bc}{}^{\alpha\beta}\nabla_a\Lambda^{\dot{\alpha}i} + (-\frac{1}{160}\mathcal{D}^\dagger\bar{\mathcal{H}} - \frac{19}{2880}\mathcal{D}\bar{\mathcal{I}})\Lambda^{\dot{\alpha}i}\gamma_b{}^\alpha{}_{\dot{\beta}}\nabla_c\Lambda_{\alpha j}\nabla_d\Lambda^{\dot{\beta}j}\epsilon_{abcd} \\
& + (-\frac{1}{192}\bar{\mathcal{H}} - \frac{23}{192}\mathcal{H})\Lambda^{\dot{\beta}i}R(Q)_{ab\alpha}{}^j\gamma_c{}^\alpha{}_{\dot{\beta}}\gamma_b{}^{\dot{\alpha}\beta}\nabla_c\Lambda_{\beta j} + (-\frac{1}{192}\bar{\mathcal{H}} + \frac{3}{64}\mathcal{H})\Lambda^{\dot{\beta}i}R(Q)_{bc\alpha}{}^j\gamma_a{}^\alpha{}_{\dot{\beta}}\gamma_b{}^{\dot{\alpha}\beta}\nabla_c\Lambda_{\beta j} \\
& + (-\frac{1}{240}\mathcal{D}^\dagger\bar{\mathcal{I}} + \frac{17}{960}\mathcal{D}^\dagger\mathcal{D}^\dagger\mathcal{D}^\dagger\bar{\mathcal{H}})T_{abjk}\Lambda^{\dot{\beta}j}\Lambda^{\dot{\gamma}k}\gamma_{bc\dot{\beta}\dot{\gamma}}\nabla_c\Lambda^{\dot{\alpha}i} + (-\frac{1}{256}\mathcal{D}^\dagger\bar{\mathcal{H}} - \frac{13}{384}\mathcal{D}\bar{\mathcal{I}})\Lambda^{\dot{\beta}i}\gamma_a{}^{\dot{\alpha}\alpha}\gamma_{bc\dot{\beta}\dot{\gamma}}\nabla_b\Lambda_{\alpha j}\nabla_c\Lambda^{\dot{\gamma}j} \\
& + (-\frac{7}{2304}\bar{\mathcal{H}} - \frac{329}{2304}\mathcal{H})\Lambda_{\alpha j}\Lambda^{\dot{\alpha}i}\bar{P}_a\gamma_b{}^\alpha{}_{\dot{\beta}}\nabla_b\Lambda^{\dot{\beta}j} + (-\frac{1}{640}\mathcal{D}^\dagger\bar{\mathcal{H}} + \frac{7}{5760}\mathcal{D}\bar{\mathcal{I}})\Lambda^{\dot{\beta}i}\gamma_b{}^\alpha{}_{\dot{\beta}}\nabla_c\Lambda_{\alpha j}\nabla_d\Lambda^{\dot{\alpha}j}\epsilon_{abcd} \\
& + (-\frac{1}{1152}\bar{\mathcal{H}} - \frac{139}{5760}\mathcal{H})E^{ij}\Lambda_{\alpha j}\Lambda^{\dot{\alpha}k}\epsilon^{\alpha\beta}\nabla_a\Lambda_{\beta k} + (\frac{1}{384}\bar{\mathcal{H}} - \frac{3}{128}\mathcal{H})\Lambda^{\dot{\beta}i}R(Q)_{bc\alpha}{}^j\gamma_a{}^\beta{}_{\dot{\beta}}\gamma_b{}^{\dot{\alpha}\alpha}\nabla_c\Lambda_{\beta j} \\
& + (\frac{1}{384}\bar{\mathcal{H}} + \frac{23}{384}\mathcal{H})\Lambda^{\dot{\beta}i}R(Q)_{ab\alpha}{}^j\gamma_c{}^\beta{}_{\dot{\beta}}\gamma_b{}^{\dot{\alpha}\alpha}\nabla_c\Lambda_{\beta j} + (\frac{1}{240}\mathcal{D}^\dagger\bar{\mathcal{I}} - \frac{17}{960}\mathcal{D}^\dagger\mathcal{D}^\dagger\mathcal{D}^\dagger\bar{\mathcal{H}})T_{bcjk}\Lambda^{\dot{\beta}j}\Lambda^{\dot{\gamma}k}\gamma_{ab\dot{\beta}\dot{\gamma}}\nabla_c\Lambda^{\dot{\alpha}i} \\
& + (\frac{1}{192}\mathcal{D}^\dagger\bar{\mathcal{H}} - \frac{1}{24}\mathcal{D}\bar{\mathcal{I}})\Lambda^{\dot{\beta}j}\gamma_b{}^{\dot{\alpha}\alpha}\gamma_{ac\dot{\beta}\dot{\gamma}}\nabla_b\Lambda_{\alpha j}\nabla_c\Lambda^{\dot{\gamma}i} + (\frac{1}{160}\mathcal{D}^\dagger\bar{\mathcal{H}} + \frac{83}{1440}\mathcal{D}\bar{\mathcal{I}})\Lambda^{\dot{\beta}j}\gamma_b{}^\alpha{}_{\dot{\beta}}\nabla_c\Lambda_{\alpha j}\nabla_d\Lambda^{\dot{\alpha}i}\epsilon_{abcd} + 3\cdots
\end{aligned}$$

$$\begin{aligned}
[\hat{\Omega}_a^{\dot{\alpha}i}]_{3,cont.} = & +(\frac{5}{768} \mathcal{D}^\dagger \bar{\mathcal{H}} + \frac{3}{128} \mathcal{D} \bar{\mathcal{L}}) \Lambda^{\dot{\beta}i} \gamma_b^{\dot{\alpha}\alpha} \gamma_{ac\dot{\beta}\dot{\gamma}} \nabla_c \Lambda_{\alpha j} \nabla_b \Lambda^{\dot{\gamma}j} + (\frac{1}{120} \mathcal{D}^\dagger \bar{\mathcal{L}} - \frac{1}{320} \mathcal{D}^\dagger \mathcal{D}^\dagger \bar{\mathcal{H}}) T_{abjk} \Lambda^{\dot{\alpha}j} \Lambda^{\dot{\beta}i} \gamma_{bc\dot{\beta}\dot{\gamma}} \nabla_c \Lambda^{\dot{\gamma}k} \\
& + (\frac{1}{120} \mathcal{D}^\dagger \bar{\mathcal{L}} - \frac{1}{320} \mathcal{D}^\dagger \mathcal{D}^\dagger \bar{\mathcal{H}}) T_{bcjk} \Lambda^{\dot{\alpha}i} \Lambda^{\dot{\beta}j} \gamma_{ab\dot{\beta}\dot{\gamma}} \nabla_c \Lambda^{\dot{\gamma}k} + (\frac{5}{576} \bar{\mathcal{H}} - \frac{5}{576} \mathcal{H}) \Lambda_{\alpha j} \Lambda_{\beta k} \Lambda^{\dot{\alpha}j} \gamma_{ab}^{\alpha\beta} \nabla_b E^{ik} \\
& + (\frac{1}{96} \bar{\mathcal{H}} + \frac{1}{48} \mathcal{H}) \Lambda_{\alpha j} \Lambda_{\beta k} \Lambda^{\dot{\alpha}i} \epsilon^{\alpha\beta} \nabla_a E^{jk} + (\frac{1}{96} \mathcal{D}^\dagger \bar{\mathcal{L}} + \frac{1}{72} \mathcal{D} \mathcal{H}) \Lambda_{\alpha j} \Lambda_{\beta k} \gamma_{ab}^{\alpha\beta} \nabla_b \chi^{\dot{\alpha}}_{lm} \epsilon^{ijklm} \\
& + (\frac{1}{96} \mathcal{D}^\dagger \bar{\mathcal{L}} + \frac{1}{72} \mathcal{D} \mathcal{H}) \Lambda_{\alpha j} \Lambda_{\beta k} \gamma_{ab}^{\alpha\beta} \nabla_b \chi^{\dot{\alpha}}_{lm} \epsilon^{ijklm} + (\frac{3}{256} \bar{\mathcal{H}} + \frac{37}{2304} \mathcal{H}) \Lambda^{\dot{\alpha}j} \Lambda^{\dot{\beta}i} \bar{P}_b \gamma_b^{\alpha}{}_{\dot{\beta}} \nabla_a \Lambda_{\alpha j} \\
& + (\frac{5}{384} \bar{\mathcal{H}} + \frac{7}{384} \mathcal{H}) \Lambda_{\alpha j} R(Q)_{bc\beta}{}^i \gamma_a^{\alpha}{}_{\dot{\beta}} \gamma_b^{\dot{\alpha}\beta} \nabla_c \Lambda^{\dot{\beta}j} + (\frac{1}{72} \bar{\mathcal{L}} - \frac{1}{96} \mathcal{D}^\dagger \mathcal{D}^\dagger \bar{\mathcal{H}}) E_{jk} \Lambda^{\dot{\alpha}i} \Lambda^{\dot{\beta}j} \gamma_{ab\dot{\beta}\dot{\gamma}} \nabla_b \Lambda^{\dot{\gamma}k} \\
& + (\frac{11}{768} \mathcal{D}^\dagger \bar{\mathcal{H}} + \frac{9}{128} \mathcal{D} \bar{\mathcal{L}}) \Lambda^{\dot{\beta}i} \gamma_b^{\dot{\alpha}\alpha} \gamma_{ac\dot{\beta}\dot{\gamma}} \nabla_b \Lambda_{\alpha j} \nabla_c \Lambda^{\dot{\gamma}j} + (\frac{1}{64} \mathcal{D}^\dagger \bar{\mathcal{H}} + \frac{7}{384} \mathcal{D} \bar{\mathcal{L}}) \Lambda^{\dot{\alpha}i} \Lambda^{\dot{\beta}j} R(Q)_{ab}{}^{\dot{\gamma}} \bar{P}_b \epsilon_{\dot{\beta}\dot{\gamma}} \\
& + (\frac{1}{64} \mathcal{D}^\dagger \bar{\mathcal{H}} + \frac{1}{48} \mathcal{D} \bar{\mathcal{L}}) \Lambda_{\alpha j} \gamma_a^{\dot{\alpha}\alpha} \gamma_{bc\dot{\beta}\dot{\gamma}} \nabla_b \Lambda^{\dot{\beta}i} \nabla_c \Lambda^{\dot{\gamma}j} + (\frac{1}{60} \mathcal{D}^\dagger \bar{\mathcal{L}} + \frac{11}{480} \mathcal{D}^\dagger \mathcal{D}^\dagger \bar{\mathcal{H}}) T_{bcjk} \Lambda^{\dot{\beta}i} \Lambda^{\dot{\gamma}j} \gamma_{ab\dot{\beta}\dot{\gamma}} \nabla_c \Lambda^{\dot{\alpha}k} \\
& + (\frac{43}{2304} \bar{\mathcal{H}} - \frac{3}{256} \mathcal{H}) \Lambda^{\dot{\alpha}i} \Lambda^{\dot{\beta}j} \bar{P}_a \gamma_b^{\alpha}{}_{\dot{\beta}} \nabla_b \Lambda_{\alpha j} + (\frac{11}{576} \bar{\mathcal{H}} - \frac{5}{64} \mathcal{H}) \Lambda_{\alpha j} \Lambda^{\dot{\alpha}j} \Lambda^{\dot{\beta}i} \gamma_a^{\alpha}{}_{\dot{\beta}} \nabla_b \bar{P}_b + (\frac{1}{48} \bar{\mathcal{L}} - \frac{1}{64} \mathcal{D}^\dagger \mathcal{D}^\dagger \bar{\mathcal{H}}) E_{jk} \Lambda^{\dot{\beta}i} \Lambda^{\dot{\gamma}j} \epsilon_{\dot{\beta}\dot{\gamma}} \nabla_a \Lambda^{\dot{\alpha}k} \\
& + (\frac{1}{48} \bar{\mathcal{H}} - \frac{3}{16} \mathcal{H}) \Lambda^{\dot{\beta}j} R(Q)_{bca}{}^i \gamma_a^{\alpha}{}_{\dot{\beta}} \gamma_b^{\dot{\alpha}\beta} \nabla_c \Lambda_{\beta j} + (\frac{1}{48} \bar{\mathcal{H}} + \frac{11}{48} \mathcal{H}) \Lambda^{\dot{\beta}j} \chi_{\alpha}{}^{ik}{}_{j\gamma_b}{}^{\alpha}{}_{\dot{\beta}} \gamma_a^{\dot{\alpha}\beta} \nabla_b \Lambda_{\beta k} \\
& + (\frac{1}{48} \mathcal{D}^\dagger \bar{\mathcal{H}} - \frac{1}{8} \mathcal{D} \bar{\mathcal{L}}) \Lambda_{\alpha j} \gamma_b^{\dot{\alpha}\alpha} \gamma_{ac\dot{\beta}\dot{\gamma}} \nabla_c \Lambda^{\dot{\beta}i} \nabla_b \Lambda^{\dot{\gamma}j} + (\frac{1}{48} \mathcal{D}^\dagger \bar{\mathcal{L}} + \frac{1}{4} \mathcal{D} \mathcal{H}) T_{ab}{}^{ij} \Lambda_{\alpha j} \Lambda_{\beta k} \gamma_{bc}^{\alpha\beta} \nabla_c \Lambda^{\dot{\alpha}k} \\
& + (\frac{103}{4608} \bar{\mathcal{H}} - \frac{125}{1536} \mathcal{H}) \Lambda_{\alpha j} \Lambda^{\dot{\alpha}i} \Lambda^{\dot{\beta}j} \gamma_b^{\alpha}{}_{\dot{\beta}} \nabla_b \bar{P}_a + (\frac{3}{128} \mathcal{D}^\dagger \bar{\mathcal{H}} + \frac{65}{768} \mathcal{D} \bar{\mathcal{L}}) \Lambda^{\dot{\beta}i} \Lambda^{\dot{\gamma}j} R(Q)_{bc}{}^{\dot{\alpha}}{}_{j\gamma_b} \bar{P}_a \gamma_{bc\dot{\beta}\dot{\gamma}} \\
& + (\frac{5}{192} \bar{\mathcal{H}} - \frac{17}{192} \mathcal{H}) \Lambda_{\alpha j} \Lambda^{\dot{\beta}j} \gamma_b^{\beta}{}_{\dot{\beta}} \gamma_c^{\dot{\alpha}\alpha} \nabla_b R(Q)_{ac\beta}{}^i + (\frac{5}{192} \bar{\mathcal{H}} + \frac{7}{192} \mathcal{H}) \Lambda_{\alpha j} R(Q)_{bc\beta}{}^j \gamma_a^{\beta}{}_{\dot{\beta}} \gamma_b^{\dot{\alpha}\alpha} \nabla_c \Lambda^{\dot{\beta}i} \\
& + (\frac{1}{36} \bar{\mathcal{L}} + \frac{1}{192} \mathcal{D}^\dagger \mathcal{D}^\dagger \bar{\mathcal{H}}) \Lambda^{\dot{\alpha}j} \Lambda^{\dot{\beta}i} \Lambda^{\dot{\gamma}k} \epsilon_{\dot{\beta}\dot{\gamma}} \nabla_a E_{jk} + (\frac{1}{36} \mathcal{D}^\dagger \bar{\mathcal{L}} - \frac{1}{48} \mathcal{D}^\dagger \mathcal{D}^\dagger \bar{\mathcal{H}}) \Lambda^{\dot{\alpha}j} \Lambda^{\dot{\beta}i} \Lambda^{\dot{\gamma}k} \gamma_{ab\dot{\beta}\dot{\gamma}} \nabla_c T_{bcjk} \\
& + (\frac{1}{36} \mathcal{D}^\dagger \bar{\mathcal{L}} - \frac{1}{48} \mathcal{D}^\dagger \mathcal{D}^\dagger \bar{\mathcal{H}}) \Lambda^{\dot{\alpha}j} \Lambda^{\dot{\beta}i} \Lambda^{\dot{\gamma}k} \gamma_{bc\dot{\beta}\dot{\gamma}} \nabla_b T_{acjk} + (\frac{1}{32} \bar{\mathcal{H}} - \frac{5}{32} \mathcal{H}) \Lambda^{\dot{\beta}j} R(Q)_{aba}{}^i \gamma_c^{\alpha}{}_{\dot{\beta}} \gamma_b^{\dot{\alpha}\beta} \nabla_c \Lambda_{\beta j} \\
& + (\frac{1}{32} \bar{\mathcal{H}} - \frac{3}{32} \mathcal{H}) \Lambda_{\alpha j} \Lambda^{\dot{\beta}i} \gamma_b^{\beta}{}_{\dot{\beta}} \gamma_c^{\dot{\alpha}\alpha} \nabla_b R(Q)_{ac\beta}{}^j + (\frac{7}{192} \bar{\mathcal{H}} + \frac{1}{192} \mathcal{H}) E^{jk} \Lambda_{\alpha j} \Lambda_{\beta k} \epsilon^{\alpha\beta} \nabla_a \Lambda^{\dot{\alpha}i} \\
& + (\frac{3}{80} \mathcal{D}^\dagger \bar{\mathcal{L}} - \frac{13}{480} \mathcal{D}^\dagger \mathcal{D}^\dagger \bar{\mathcal{H}}) T_{abjk} \Lambda^{\dot{\alpha}j} \Lambda^{\dot{\beta}k} \gamma_{bc\dot{\beta}\dot{\gamma}} \nabla_c \Lambda^{\dot{\gamma}i} + (\frac{11}{288} \bar{\mathcal{H}} - \frac{41}{480} \mathcal{H}) E^{ij} \Lambda_{\alpha k} \Lambda^{\dot{\alpha}k} \epsilon^{\alpha\beta} \nabla_a \Lambda_{\beta j} \\
& + (\frac{5}{128} \bar{\mathcal{H}} - \frac{1}{128} \mathcal{H}) \Lambda_{\alpha j} R(Q)_{ab\beta}{}^i \gamma_c^{\alpha}{}_{\dot{\beta}} \gamma_b^{\dot{\alpha}\beta} \nabla_c \Lambda^{\dot{\beta}j} + (\frac{113}{2880} \bar{\mathcal{H}} - \frac{49}{2880} \mathcal{H}) E^{jk} \Lambda_{\alpha j} \Lambda^{\dot{\alpha}i} \epsilon^{\alpha\beta} \nabla_a \Lambda_{\beta k} \\
& + (\frac{1}{24} \bar{\mathcal{H}} - \frac{1}{8} \mathcal{H}) \Lambda^{\dot{\beta}j} \chi_{\alpha}{}^{ik}{}_{j\gamma_a}{}^{\alpha}{}_{\dot{\beta}} \gamma_b^{\dot{\alpha}\beta} \nabla_b \Lambda_{\beta k} + (\frac{1}{24} \bar{\mathcal{H}} - \frac{1}{16} \mathcal{H}) \Lambda_{\alpha j} \Lambda_{\beta k} \Lambda^{\dot{\alpha}j} \epsilon^{\alpha\beta} \nabla_a E^{ik} + (\frac{1}{24} \mathcal{D}^\dagger \bar{\mathcal{H}} - \frac{1}{48} \mathcal{D} \bar{\mathcal{L}}) E_{jk} \Lambda^{\dot{\alpha}j} \Lambda^{\dot{\beta}l} \chi_{\alpha}{}^{ik}{}_{l\gamma_a}{}^{\alpha}{}_{\dot{\beta}} \\
& + (\frac{1}{24} \mathcal{D}^\dagger \bar{\mathcal{L}} + \frac{1}{12} \mathcal{D} \mathcal{H}) T_{ab}{}^{jk} \Lambda_{\alpha j} \Lambda_{\beta k} \gamma_{bc}^{\alpha\beta} \nabla_c \Lambda^{\dot{\alpha}i} + (\frac{107}{2304} \bar{\mathcal{H}} + \frac{13}{256} \mathcal{H}) \Lambda^{\dot{\alpha}i} \Lambda^{\dot{\beta}j} \bar{P}_b \gamma_a^{\alpha}{}_{\dot{\beta}} \nabla_b \Lambda_{\alpha j} \\
& + (\frac{3}{64} \mathcal{D}^\dagger \bar{\mathcal{H}} + \frac{1}{384} \mathcal{D} \bar{\mathcal{L}}) \Lambda^{\dot{\beta}i} \Lambda^{\dot{\gamma}j} R(Q)_{ab}{}^{\dot{\alpha}}{}_{j\gamma_b} \bar{P}_c \gamma_{bc\dot{\beta}\dot{\gamma}} + (\frac{3}{64} \mathcal{D}^\dagger \bar{\mathcal{H}} + \frac{1}{384} \mathcal{D} \bar{\mathcal{L}}) \Lambda^{\dot{\beta}i} \Lambda^{\dot{\gamma}j} R(Q)_{bc}{}^{\dot{\alpha}}{}_{j\gamma_b} \bar{P}_c \gamma_{ac\dot{\beta}\dot{\gamma}} \\
& + (\frac{7}{144} \bar{\mathcal{L}} - \frac{1}{64} \mathcal{D}^\dagger \mathcal{D}^\dagger \bar{\mathcal{H}}) E_{jk} \Lambda^{\dot{\alpha}j} \Lambda^{\dot{\beta}i} \epsilon_{\dot{\beta}\dot{\gamma}} \nabla_a \Lambda^{\dot{\gamma}k} + (\frac{71}{1440} \mathcal{D}^\dagger \bar{\mathcal{L}} + \frac{1}{120} \mathcal{D} \mathcal{H}) T_{bc}{}^{ij} \Lambda_{\alpha j} \Lambda_{\beta k} \gamma_{bc}^{\alpha\beta} \nabla_a \Lambda^{\dot{\alpha}k} \\
& + (\frac{5}{96} \bar{\mathcal{H}} - \frac{1}{32} \mathcal{H}) \Lambda_{\alpha j} \Lambda^{\dot{\beta}i} \gamma_a^{\alpha}{}_{\dot{\beta}} \gamma_b^{\dot{\alpha}\beta} \nabla_c R(Q)_{bc\beta}{}^j + (\frac{5}{96} \mathcal{D}^\dagger \bar{\mathcal{L}} - \frac{1}{80} \mathcal{D} \mathcal{H}) T_{bc}{}^{ij} \Lambda_{\alpha j} \Lambda^{\dot{\alpha}k} \gamma_{bc}^{\alpha\beta} \nabla_a \Lambda_{\beta k} \\
& + (\frac{17}{288} \bar{\mathcal{H}} + \frac{7}{288} \mathcal{H}) \Lambda_{\alpha j} \Lambda^{\dot{\alpha}j} \bar{P}_a \gamma_b^{\alpha}{}_{\dot{\beta}} \nabla_b \Lambda^{\dot{\beta}i} + (\frac{1}{16} \bar{\mathcal{H}} + \frac{5}{144} \mathcal{H}) \Lambda_{\alpha j} R(Q)_{ab}{}^{\dot{\alpha}}{}_{k\chi^{\dot{\beta}}_{lm}}{}^j \gamma_b^{\alpha}{}_{\dot{\beta}} \epsilon^{iklm} \\
& + (\frac{1}{16} \mathcal{D}^\dagger \bar{\mathcal{H}} + \frac{3}{32} \mathcal{D} \bar{\mathcal{L}}) \Lambda_{\alpha j} \Lambda^{\dot{\alpha}j} \Lambda^{\dot{\beta}k} R(V)_{ab}{}^i{}_{k\gamma_b}{}^{\alpha}{}_{\dot{\beta}} + (\frac{311}{4608} \bar{\mathcal{H}} - \frac{103}{4608} \mathcal{H}) \Lambda_{\alpha j} \Lambda^{\dot{\alpha}j} \Lambda^{\dot{\beta}i} \gamma_b^{\alpha}{}_{\dot{\beta}} \nabla_a \bar{P}_b \\
& + (\frac{7}{96} \bar{\mathcal{H}} + \frac{3}{32} \mathcal{H}) \Lambda_{\alpha j} \Lambda^{\dot{\beta}j} \bar{P}_b \gamma_b^{\alpha}{}_{\dot{\beta}} \nabla_a \Lambda^{\dot{\alpha}i} + (\frac{7}{96} \mathcal{D}^\dagger \bar{\mathcal{H}} - \frac{1}{96} \mathcal{D} \bar{\mathcal{L}}) \Lambda_{\alpha j} \Lambda^{\dot{\beta}i} \gamma_b^{\dot{\alpha}\alpha} \gamma_{ac\dot{\beta}\dot{\gamma}} \nabla_b \nabla_c \Lambda^{\dot{\gamma}j} \\
& + (\frac{5}{64} \mathcal{D}^\dagger \bar{\mathcal{H}} - \frac{27}{128} \mathcal{D} \bar{\mathcal{L}}) \Lambda^{\dot{\beta}i} \Lambda^{\dot{\gamma}j} R(Q)_{ab}{}^{\dot{\alpha}}{}_{j\gamma_b} \bar{P}_c \epsilon_{\dot{\beta}\dot{\gamma}} + (\frac{1}{12} \bar{\mathcal{H}} - \frac{1}{12} \mathcal{H}) T_{ab}{}^{ij} \Lambda_{\alpha j} \Lambda^{\dot{\beta}k} R(Q)_{bc}{}^{\dot{\alpha}}{}_{k\gamma_c}{}^{\alpha}{}_{\dot{\beta}} \\
& + (\frac{1}{12} \mathcal{D}^\dagger \bar{\mathcal{L}} + \frac{1}{48} \mathcal{D}^\dagger \mathcal{D}^\dagger \bar{\mathcal{H}}) \bar{P}_b \Lambda^{\dot{\beta}i} \Lambda^{\dot{\gamma}j} R(Q)_{ac}{}^{\dot{\alpha}}{}_{j\gamma_b} \gamma_{bc\dot{\beta}\dot{\gamma}} + (\frac{1}{12} \mathcal{D}^\dagger \bar{\mathcal{H}} - \frac{1}{16} \mathcal{D} \bar{\mathcal{L}}) E^{ij} \Lambda_{\alpha k} \Lambda^{\dot{\beta}l} \chi^{\dot{\alpha}}{}_{jl}{}^k \gamma_a^{\alpha}{}_{\dot{\beta}} \\
& + (\frac{1}{12} \mathcal{D}^\dagger \bar{\mathcal{H}} + \frac{1}{8} \mathcal{D} \bar{\mathcal{L}}) \Lambda^{\dot{\alpha}j} \Lambda^{\dot{\beta}k} \bar{P}_a \chi^{\dot{\gamma}}{}_{jk}{}^i \epsilon_{\dot{\beta}\dot{\gamma}} + (\frac{1}{12} \mathcal{D}^\dagger \bar{\mathcal{H}} + \frac{5}{32} \mathcal{D} \bar{\mathcal{L}}) \Lambda^{\dot{\beta}i} \Lambda^{\dot{\gamma}j} \epsilon_{\dot{\beta}\dot{\gamma}} \gamma_a^{\dot{\alpha}\alpha} \nabla_b \nabla_b \Lambda_{\alpha j} \\
& + (\frac{1}{12} \mathcal{D}^\dagger \bar{\mathcal{H}} + \frac{1}{6} \mathcal{D} \bar{\mathcal{L}}) \Lambda^{\dot{\beta}j} \Lambda^{\dot{\gamma}k} \bar{P}_b \chi^{\dot{\alpha}}{}_{jk}{}^i \gamma_{ab\dot{\beta}\dot{\gamma}} + (\frac{19}{180} \mathcal{D}^\dagger \bar{\mathcal{L}} + \frac{7}{80} \mathcal{D} \mathcal{H}) \Lambda_{\alpha j} \Lambda_{\beta k} \Lambda^{\dot{\alpha}j} \gamma_{bc}^{\alpha\beta} \nabla_a T_{bc}{}^{ik} + 4 \dots
\end{aligned}$$

$$\begin{aligned} [\hat{\Omega}_a^{\dot{\alpha}\dot{i}}]_{3,cont.} = & + \left( \frac{7}{64} \mathcal{D}^\dagger \bar{\mathcal{H}} + \frac{1}{16} \mathcal{D} \bar{\mathcal{I}} \right) \Lambda_{\alpha j} \gamma_b^{\dot{\alpha}} \epsilon^{\dot{\beta} i} \nabla_b \Lambda^{\dot{\beta} i} \nabla_c \Lambda^{\dot{\gamma} j} + \left( \frac{23}{192} \mathcal{D}^\dagger \bar{\mathcal{H}} - \frac{29}{192} \mathcal{D} \bar{\mathcal{I}} \right) E^{jk} \Lambda_{\alpha j} \Lambda^{\dot{\beta} i} R(Q)_{ab}{}^{\dot{\alpha}} k \gamma_b^{\dot{\alpha}}{}_\beta \\ & + \left( \frac{1}{8} \bar{\mathcal{H}} + \frac{5}{72} \mathcal{H} \right) \Lambda_{\alpha j} R(Q)_{ab}{}^{\dot{\alpha}}{}_k \chi^{\dot{\beta}}{}_{lm}{}^k \gamma_b^{\dot{\alpha}}{}_\beta \epsilon^{\dot{\beta} ijl m} + \left( \frac{25}{192} \bar{\mathcal{H}} - \frac{15}{64} \mathcal{H} \right) \Lambda_{\alpha j} \Lambda^{\dot{\beta} j} \gamma_a^{\dot{\beta}}{}_\beta \gamma_b^{\dot{\alpha}}{}_\beta \epsilon^{\dot{\beta} i} \nabla_c R(Q)_{bc\beta}{}^i \\ & + \left( \frac{9}{64} \bar{\mathcal{H}} + \frac{3}{64} \mathcal{H} \right) \Lambda_{\alpha j} R(Q)_{ab\beta}{}^j \gamma_c^{\dot{\beta}}{}_\beta \gamma_b^{\dot{\alpha}}{}_\beta \epsilon^{\dot{\beta} i} \nabla_c \Lambda^{\dot{\beta} i} + \left( \frac{7}{48} \bar{\mathcal{H}} - \frac{7}{48} \mathcal{H} \right) \Lambda_{\alpha j} \chi_\beta^{\dot{\beta} ij}{}^k \gamma_b^{\dot{\beta}}{}_\beta \gamma_a^{\dot{\alpha}}{}_\beta \epsilon^{\dot{\beta} i} \nabla_b \Lambda^{\dot{\beta} k} \\ & + \left( \frac{3}{20} \mathcal{D}^\dagger \bar{\mathcal{I}} + \frac{1}{160} \mathcal{D}^\dagger \mathcal{D}^\dagger \mathcal{D}^\dagger \bar{\mathcal{H}} \right) T_{abjk} \Lambda^{\dot{\alpha} i} \Lambda^{\dot{\beta} j} \epsilon_{\dot{\beta} \dot{\gamma}} \nabla_b \Lambda^{\dot{\gamma} k} + \left( \frac{1}{6} \mathcal{D}^\dagger \bar{\mathcal{I}} + \frac{1}{48} \mathcal{D}^\dagger \mathcal{D}^\dagger \mathcal{D}^\dagger \bar{\mathcal{H}} \right) P_b \Lambda^{\dot{\alpha} j} \Lambda^{\dot{\beta} i} R(Q)_{ab}{}^{\dot{\gamma}}{}_j \epsilon_{\dot{\beta} \dot{\gamma}} \\ & + \left( \frac{19}{96} \bar{\mathcal{H}} + \frac{5}{96} \mathcal{H} \right) \Lambda_{\alpha j} \Lambda^{\dot{\beta} k} \gamma_b^{\dot{\alpha}}{}_\beta \gamma_a^{\dot{\alpha} \dot{\beta}} \nabla_b \chi_\beta^{\dot{\beta} ij}{}^k + \left( \frac{1}{5} \mathcal{D}^\dagger \bar{\mathcal{H}} + \frac{11}{24} \mathcal{D} \bar{\mathcal{I}} \right) P_b \Lambda_{\alpha j} \Lambda^{\dot{\alpha} j} R(Q)_{ab\beta}{}^i \epsilon^{\alpha \beta} \\ & + \left( \frac{5}{24} \mathcal{D}^\dagger \bar{\mathcal{I}} - \frac{1}{96} \mathcal{D}^\dagger \mathcal{D}^\dagger \mathcal{D}^\dagger \bar{\mathcal{H}} \right) P_b \Lambda^{\dot{\beta} j} \Lambda^{\dot{\gamma} k} \chi^{\dot{\alpha}}{}_{jk}{}^i \gamma_{ab\dot{\beta} \dot{\gamma}} + \left( \frac{7}{32} \bar{\mathcal{I}} + \frac{1}{576} \mathcal{D}^\dagger \mathcal{D}^\dagger \bar{\mathcal{H}} \right) P_a \Lambda^{\dot{\alpha} i} \Lambda^{\dot{\beta} j} \gamma_b^{\dot{\alpha}}{}_\beta \nabla_b \Lambda_{\alpha j} \\ & + \left( \frac{2}{9} \bar{\mathcal{I}} + \frac{5}{72} \mathcal{D}^\dagger \mathcal{D}^\dagger \bar{\mathcal{H}} \right) P_a \Lambda_{\alpha j} \Lambda^{\dot{\alpha} i} \gamma_b^{\dot{\alpha}}{}_\beta \nabla_b \Lambda^{\dot{\beta} j} + \left( \frac{1}{4} \bar{\mathcal{H}} - \frac{1}{4} \mathcal{H} \right) T_{ab}{}^{jk} \Lambda_{\alpha j} \Lambda^{\dot{\alpha} l} \chi^{\dot{\beta}}{}_{kl}{}^i \gamma_b^{\dot{\alpha}}{}_\beta + \left( \frac{1}{4} \bar{\mathcal{H}} - \frac{1}{4} \mathcal{H} \right) T_{ab}{}^{jk} \Lambda_{\alpha l} \Lambda^{\dot{\alpha} l} \chi^{\dot{\beta}}{}_{jk}{}^i \gamma_b^{\dot{\alpha}}{}_\beta \\ & + \left( \frac{77}{288} \bar{\mathcal{I}} + \frac{13}{576} \mathcal{D}^\dagger \mathcal{D}^\dagger \bar{\mathcal{H}} \right) \Lambda_{\alpha j} \Lambda^{\dot{\alpha} i} \Lambda^{\dot{\beta} j} \gamma_b^{\dot{\alpha}}{}_\beta \nabla_a P_b + \left( \frac{107}{384} \bar{\mathcal{H}} + \frac{7}{128} \mathcal{H} \right) \Lambda_{\alpha j} \Lambda^{\dot{\beta} i} \bar{P}_b \gamma_a^{\dot{\alpha}}{}_\beta \nabla_b \Lambda^{\dot{\alpha} j} \\ & + \left( \frac{85}{288} \bar{\mathcal{I}} - \frac{1}{48} \mathcal{D}^\dagger \mathcal{D}^\dagger \bar{\mathcal{H}} \right) P_b \Lambda^{\dot{\alpha} i} \Lambda^{\dot{\beta} j} \gamma_b^{\dot{\alpha}}{}_\beta \nabla_a \Lambda_{\alpha j} + \left( \frac{89}{288} \bar{\mathcal{H}} - \frac{25}{288} \mathcal{H} \right) \Lambda_{\alpha j} \Lambda^{\dot{\alpha} j} \bar{P}_b \gamma_b^{\dot{\alpha}}{}_\beta \nabla_a \Lambda^{\dot{\beta} i} \\ & + \left( \frac{5}{16} \bar{\mathcal{I}} + \frac{19}{576} \mathcal{D}^\dagger \mathcal{D}^\dagger \bar{\mathcal{H}} \right) \Lambda_{\alpha j} \Lambda^{\dot{\alpha} j} \Lambda^{\dot{\beta} i} \gamma_a^{\dot{\alpha}}{}_\beta \nabla_b P_b + \left( \frac{5}{16} \bar{\mathcal{I}} + \frac{13}{144} \mathcal{D}^\dagger \mathcal{D}^\dagger \bar{\mathcal{H}} \right) P_a \Lambda_{\alpha j} \Lambda^{\dot{\beta} i} \gamma_b^{\dot{\alpha}}{}_\beta \nabla_b \Lambda^{\dot{\alpha} j} \\ & + \left( \frac{95}{288} \bar{\mathcal{I}} + \frac{11}{192} \mathcal{D}^\dagger \mathcal{D}^\dagger \bar{\mathcal{H}} \right) \Lambda_{\alpha j} \Lambda^{\dot{\alpha} i} \Lambda^{\dot{\beta} j} \gamma_b^{\dot{\alpha}}{}_\beta \nabla_b P_a + \left( \frac{49}{144} \bar{\mathcal{I}} + \frac{17}{192} \mathcal{D}^\dagger \mathcal{D}^\dagger \bar{\mathcal{H}} \right) P_b \Lambda_{\alpha j} \Lambda^{\dot{\beta} i} \gamma_b^{\dot{\alpha}}{}_\beta \nabla_a \Lambda^{\dot{\alpha} j} \\ & + \left( \frac{35}{96} \bar{\mathcal{I}} - \frac{1}{288} \mathcal{D}^\dagger \mathcal{D}^\dagger \bar{\mathcal{H}} \right) P_b \Lambda^{\dot{\alpha} j} \Lambda^{\dot{\beta} i} \gamma_a^{\dot{\alpha}}{}_\beta \nabla_b \Lambda_{\alpha j} + \left( \frac{41}{72} \bar{\mathcal{I}} + \frac{13}{192} \mathcal{D}^\dagger \mathcal{D}^\dagger \bar{\mathcal{H}} \right) P_b \Lambda_{\alpha j} \Lambda^{\dot{\alpha} i} \gamma_b^{\dot{\alpha}}{}_\beta \nabla_a \Lambda^{\dot{\beta} j} \\ & + \left( \frac{97}{144} \bar{\mathcal{I}} + \frac{29}{576} \mathcal{D}^\dagger \mathcal{D}^\dagger \bar{\mathcal{H}} \right) P_b \Lambda_{\alpha j} \Lambda^{\dot{\alpha} i} \gamma_a^{\dot{\alpha}}{}_\beta \nabla_b \Lambda^{\dot{\beta} j} + \left( \frac{37}{48} \mathcal{D}^\dagger \bar{\mathcal{I}} - \frac{1}{6} \mathcal{D} \mathcal{H} \right) T_{ab}{}^{ij} \Lambda_{\alpha j} \Lambda_{\beta k} \epsilon^{\alpha \beta} \nabla_b \Lambda^{\dot{\alpha} k} \\ & + \left( \frac{5}{4} \mathcal{D}^\dagger \bar{\mathcal{I}} - \frac{1}{3} \mathcal{D} \mathcal{H} \right) \Lambda_{\alpha j} \Lambda_{\beta k} \Lambda^{\dot{\alpha} j} \epsilon^{\alpha \beta} \nabla_b T_{ab}{}^{ik} + \left( \frac{89}{36} \bar{\mathcal{I}} + \frac{25}{144} \mathcal{D}^\dagger \mathcal{D}^\dagger \bar{\mathcal{H}} \right) P_b \Lambda_{\alpha j} \Lambda^{\dot{\alpha} j} \gamma_a^{\dot{\alpha}}{}_\beta \nabla_b \Lambda^{\dot{\beta} i} \\ & - \frac{13}{1152} E_{jk} \mathcal{D}^\dagger \bar{\mathcal{I}} \Lambda_{\alpha l} \Lambda^{\dot{\alpha} j} \epsilon^{\alpha \beta} \nabla_a \Lambda_{\beta m} \epsilon^{iklm} + \frac{1}{72} E_{jk} \mathcal{D}^\dagger \bar{\mathcal{I}} \Lambda_{\alpha l} \Lambda^{\dot{\alpha} j} \gamma_{ab}{}^{\alpha \beta} \nabla_b \Lambda_{\beta m} \epsilon^{iklm} - \frac{1}{12} E_{jk} \mathcal{H} T_{ab}{}^{ij} \Lambda_{\alpha l} \Lambda^{\dot{\alpha} k} \Lambda^{\dot{\beta} l} \gamma_b^{\dot{\alpha}}{}_\beta \\ & + \frac{1}{12} E_{jk} \mathcal{H} T_{ab}{}^{ij} \Lambda_{\alpha l} \Lambda^{\dot{\alpha} l} \Lambda^{\dot{\beta} k} \gamma_b^{\dot{\alpha}}{}_\beta + \frac{5}{144} E^{ij} P_b \mathcal{D} \bar{\mathcal{I}} \Lambda_{\alpha j} \Lambda_{\beta k} \Lambda^{\dot{\alpha} k} \gamma_{ab}{}^{\alpha \beta} + \frac{1}{18} E^{ij} \Lambda_{\alpha k} \Lambda^{\dot{\beta} k} \bar{\mathcal{H}} \gamma_a^{\dot{\alpha}}{}_\beta \gamma_b^{\dot{\alpha} \dot{\beta}} \nabla_b \Lambda_{\beta j} \\ & - \frac{1}{24} P_b \mathcal{D} \bar{\mathcal{I}} \Lambda_{\alpha j} \Lambda^{\dot{\beta} k} \chi_\beta^{\dot{\beta} ij}{}^k \gamma_a^{\dot{\beta}}{}_\beta \gamma_b^{\dot{\alpha}}{}_\beta \epsilon^{\dot{\beta} i} + \frac{1}{18} T_{abjk} \mathcal{D} \bar{\mathcal{I}} \Lambda_{\alpha l} \Lambda^{\dot{\beta} m} R(Q)_{bc}{}^{\dot{\alpha}}{}_m \gamma_c^{\dot{\alpha}}{}_\beta \epsilon^{\dot{\beta} i j k l} - \frac{1}{6} T_{bcjk} \mathcal{D} \bar{\mathcal{I}} \Lambda_{\alpha l} \Lambda^{\dot{\beta} m} R(Q)_{ab}{}^{\dot{\alpha}}{}_m \gamma_c^{\dot{\alpha}}{}_\beta \epsilon^{\dot{\beta} i j k l} \\ & + \frac{3}{8} T_{abjk} \mathcal{D} \bar{\mathcal{I}} \Lambda_{\alpha l} \Lambda^{\dot{\beta} m} \chi^{\dot{\alpha}}{}_{mn}{}^i \gamma_b^{\dot{\alpha}}{}_\beta \epsilon^{\dot{\beta} i j k l n} - \frac{1}{24} T_{ab}{}^{jk} \mathcal{D} \bar{\mathcal{I}} \Lambda^{\dot{\alpha} l} \Lambda^{\dot{\beta} i} \chi_{\alpha}{}^{mn}{}_{l \gamma b}{}^{\alpha} \epsilon_{\dot{\beta} \dot{\gamma} j k m n} - \frac{1}{24} T_{ab}{}^{jk} \mathcal{D} \bar{\mathcal{I}} \Lambda^{\dot{\alpha} l} \Lambda^{\dot{\beta} m} \chi_{\alpha}{}^{in}{}_{m \gamma b}{}^{\alpha} \epsilon_{\dot{\beta} \dot$$

$$\begin{aligned}
[\hat{\Omega}_a^{\dot{\alpha}i}]_{3,cont.} = & +(-\frac{239}{360}\mathcal{D}^\dagger\mathcal{I} + \frac{73}{240}\mathcal{D}\mathcal{H})\Lambda_{\alpha j}\Lambda_{\beta k}\Lambda^{\dot{\beta}j}\epsilon^{\alpha\beta}\gamma_{ab}{}^{\dot{\alpha}}{}_{\dot{\beta}}\nabla_c T_{bc}{}^{ik} + (-\frac{31}{48}\mathcal{D}^\dagger\mathcal{I} + \frac{1}{6}\mathcal{D}\mathcal{H})\Lambda_{\alpha j}\Lambda^{\dot{\beta}j}R(Q)_{bc\beta}{}^i\bar{P}_b\gamma_a{}^\beta{}_{\dot{\beta}}\gamma_c{}^{\dot{\alpha}\alpha} \\
& + (-\frac{7}{12}\mathcal{D}^\dagger\bar{\mathcal{I}} - \frac{19}{576}\mathcal{D}^\dagger\mathcal{D}^\dagger\mathcal{D}^\dagger\bar{\mathcal{H}})P_bP_b\Lambda_{\alpha j}\Lambda^{\dot{\alpha}i}\Lambda^{\dot{\beta}j}\gamma_a{}^\alpha{}_{\dot{\beta}} + (-\frac{25}{48}\mathcal{D}^\dagger\mathcal{I} + \frac{1}{48}\mathcal{D}\mathcal{H})T_{ab}{}^{ij}\Lambda_{\alpha j}\Lambda^{\dot{\beta}k}\gamma_c{}^\alpha{}_{\dot{\beta}}\gamma_b{}^{\dot{\alpha}\beta}\nabla_c\Lambda_{\beta k} \\
& + (-\frac{61}{120}\mathcal{D}^\dagger\mathcal{I} - \frac{5}{48}\mathcal{D}\mathcal{H})T_{ab}{}^{jk}\Lambda_{\alpha j}\Lambda^{\dot{\beta}i}\gamma_c{}^\alpha{}_{\dot{\beta}}\gamma_b{}^{\dot{\alpha}\beta}\nabla_c\Lambda_{\beta k} + (-\frac{179}{360}\mathcal{D}^\dagger\mathcal{I} + \frac{11}{80}\mathcal{D}\mathcal{H})\Lambda_{\alpha j}\Lambda_{\beta k}\Lambda^{\dot{\beta}j}\epsilon^{\alpha\beta}\gamma_{bc}{}^{\dot{\alpha}}{}_{\dot{\beta}}\nabla_b T_{ac}{}^{ik} \\
& + (-\frac{15}{32}\bar{\mathcal{I}} - \frac{1}{480}\mathcal{D}^\dagger\mathcal{D}^\dagger\bar{\mathcal{H}})\Lambda_{\alpha j}\Lambda^{\dot{\beta}i}\Lambda^{\dot{j}j}\epsilon_{\dot{\beta}\dot{\gamma}}\gamma_b{}^{\dot{\alpha}\alpha}\nabla_b P_a + (-\frac{5}{12}\mathcal{D}^\dagger\mathcal{I} - \frac{5}{24}\mathcal{D}\mathcal{H})\Lambda_{\alpha j}\Lambda_{\beta k}\Lambda^{\dot{\beta}i}\gamma_a{}^\alpha{}_{\dot{\beta}}\gamma_b{}^{\dot{\alpha}\beta}\nabla_c T_{bc}{}^{jk} \\
& + (-\frac{293}{720}\mathcal{D}^\dagger\mathcal{I} + \frac{59}{240}\mathcal{D}\mathcal{H})T_{bc}{}^{ij}\Lambda_{\alpha k}\Lambda^{\dot{\beta}k}\gamma_b{}^\alpha{}_{\dot{\beta}}\gamma_a{}^{\dot{\alpha}\beta}\nabla_c\Lambda_{\beta j} + (-\frac{287}{720}\mathcal{D}^\dagger\mathcal{I} - \frac{41}{120}\mathcal{D}\mathcal{H})\Lambda_{\alpha j}\Lambda_{\beta k}\Lambda^{\dot{\beta}j}\gamma_b{}^\alpha{}_{\dot{\beta}}\gamma_a{}^{\dot{\alpha}\beta}\nabla_c T_{bc}{}^{ik} \\
& + (-\frac{287}{720}\mathcal{D}^\dagger\mathcal{I} - \frac{41}{120}\mathcal{D}\mathcal{H})\Lambda_{\alpha j}\Lambda_{\beta k}\Lambda^{\dot{\beta}j}\gamma_b{}^\beta{}_{\dot{\beta}}\gamma_a{}^{\dot{\alpha}\alpha}\nabla_c T_{bc}{}^{ik} + (-\frac{17}{48}\bar{\mathcal{H}} + \frac{43}{144}\mathcal{H})P_bT_{ab}{}^{ij}\Lambda_{\alpha j}\Lambda_{\beta k}\Lambda^{\dot{\alpha}k}\epsilon^{\alpha\beta} \\
& + (-\frac{19}{60}\mathcal{D}^\dagger\mathcal{I} - \frac{2}{15}\mathcal{D}\mathcal{H})T_{bc}{}^{ij}\Lambda_{\alpha k}\Lambda^{\dot{\beta}k}\gamma_a{}^\alpha{}_{\dot{\beta}}\gamma_b{}^{\dot{\alpha}\beta}\nabla_c\Lambda_{\beta j} + (-\frac{11}{40}\bar{\mathcal{I}} + \frac{31}{480}\mathcal{D}^\dagger\mathcal{D}^\dagger\bar{\mathcal{H}})T_{ab}{}^{jk}\Lambda^{\dot{\alpha}l}\Lambda^{\dot{\beta}m}\epsilon_{\dot{\beta}\dot{\gamma}}\nabla_b\Lambda^{\dot{\gamma}i}\epsilon_{jklm} \\
& + (-\frac{79}{288}\mathcal{D}^\dagger\mathcal{I} + \frac{1}{720}\mathcal{D}\mathcal{H})T_{bc}{}^{ij}\Lambda_{\alpha j}\Lambda_{\beta k}\epsilon^{\alpha\beta}\gamma_{ab}{}^{\dot{\alpha}}{}_{\dot{\beta}}\nabla_c\Lambda^{\dot{\beta}k} + (-\frac{25}{96}\bar{\mathcal{I}} - \frac{1}{192}\mathcal{D}^\dagger\mathcal{D}^\dagger\bar{\mathcal{H}})P_b\Lambda^{\dot{\beta}i}\Lambda^{\dot{j}j}\epsilon_{\dot{\beta}\dot{\gamma}}\gamma_b{}^{\dot{\alpha}\alpha}\nabla_a\Lambda_{\alpha j} \\
& + (-\frac{349}{1440}\bar{\mathcal{I}} + \frac{65}{1152}\mathcal{D}^\dagger\mathcal{D}^\dagger\bar{\mathcal{H}})P_b\Lambda_{\alpha j}\Lambda^{\dot{\alpha}i}\gamma_c{}^\alpha{}_{\dot{\beta}}\nabla_d\Lambda^{\dot{\beta}j}\epsilon_{abcd} + (-\frac{167}{720}\mathcal{D}^\dagger\mathcal{I} - \frac{7}{60}\mathcal{D}\mathcal{H})T_{bc}{}^{ij}\Lambda_{\alpha j}\Lambda_{\beta k}\gamma_{bc}{}^{\alpha\beta}\gamma_{ad}{}^{\dot{\alpha}}{}_{\dot{\beta}}\nabla_d\Lambda^{\dot{\beta}k} \\
& + (-\frac{2}{9}\mathcal{D}^\dagger\mathcal{D}^\dagger\bar{\mathcal{I}} + \frac{1}{18}\mathcal{D}^\dagger\mathcal{D}^\dagger\mathcal{D}^\dagger\bar{\mathcal{H}})P_bT_{abjk}\Lambda^{\dot{\alpha}j}\Lambda^{\dot{\beta}i}\Lambda^{\dot{\gamma}k}\epsilon_{\dot{\beta}\dot{\gamma}} + (-\frac{13}{60}\bar{\mathcal{I}} - \frac{3}{80}\mathcal{D}^\dagger\mathcal{D}^\dagger\bar{\mathcal{H}})T_{ab}{}^{ij}\Lambda^{\dot{\alpha}k}\Lambda^{\dot{\beta}l}\epsilon_{\dot{\beta}\dot{\gamma}}\nabla_b\Lambda^{\dot{\gamma}m}\epsilon_{jklm} \\
& + (-\frac{13}{60}\bar{\mathcal{I}} - \frac{1}{160}\mathcal{D}^\dagger\mathcal{D}^\dagger\bar{\mathcal{H}})T_{bc}{}^{ij}\Lambda^{\dot{\beta}k}\Lambda^{\dot{\gamma}l}\gamma_{ab\dot{\beta}\dot{\gamma}}\nabla_c\Lambda^{\dot{\alpha}m}\epsilon_{jklm} + (-\frac{5}{24}\bar{\mathcal{H}} - \frac{3}{8}\mathcal{H})\Lambda_{\alpha j}\Lambda_{\beta k}\Lambda^{\dot{\alpha}j}\epsilon^{\alpha\beta}\nabla_b T_{ablm}\epsilon^{iklm} \\
& + (-\frac{19}{96}\mathcal{D}\mathcal{D}\mathcal{H} - \frac{7}{12}\mathcal{I})T_{bc}{}^{ij}\Lambda_{\alpha j}\Lambda_{\beta k}R(Q)_{bc\gamma}{}^k\epsilon^{\alpha\beta}\gamma_a{}^{\dot{\alpha}\gamma} + (-\frac{7}{36}\bar{\mathcal{I}} + \frac{1}{144}\mathcal{D}^\dagger\mathcal{D}^\dagger\bar{\mathcal{H}})T_{bcjk}\Lambda^{\dot{\alpha}i}\Lambda^{\dot{\beta}j}\Lambda^{\dot{\gamma}k}\bar{P}_a\gamma_{bc\dot{\beta}\dot{\gamma}} \\
& + (-\frac{23}{120}\bar{\mathcal{I}} + \frac{47}{960}\mathcal{D}^\dagger\mathcal{D}^\dagger\bar{\mathcal{H}})T_{bc}{}^{jk}\Lambda^{\dot{\beta}l}\Lambda^{\dot{\gamma}m}\gamma_{ab\dot{\beta}\dot{\gamma}}\nabla_c\Lambda^{\dot{\alpha}i}\epsilon_{jklm} + (-\frac{11}{60}\mathcal{D}^\dagger\bar{\mathcal{H}} - \frac{13}{48}\mathcal{D}\bar{\mathcal{I}})P_b\Lambda_{\alpha j}\Lambda^{\dot{\beta}j}R(Q)_{bc\beta}{}^i\gamma_a{}^\beta{}_{\dot{\beta}}\gamma_c{}^{\dot{\alpha}\alpha} \\
& + (-\frac{13}{72}\mathcal{D}^\dagger\mathcal{I} + \frac{1}{288}\mathcal{D}\mathcal{H})\Lambda_{\alpha j}\Lambda^{\dot{\alpha}i}\Lambda^{\dot{\beta}j}\bar{P}_b\bar{P}_b\gamma_a{}^\alpha{}_{\dot{\beta}} + (-\frac{43}{240}\bar{\mathcal{I}} + \frac{49}{1280}\mathcal{D}^\dagger\mathcal{D}^\dagger\bar{\mathcal{H}})P_b\Lambda^{\dot{\alpha}j}\Lambda^{\dot{\beta}i}\gamma_c{}^\alpha{}_{\dot{\beta}}\nabla_d\Lambda_{\alpha j}\epsilon_{abcd} \\
& + (-\frac{137}{768}\bar{\mathcal{H}} + \frac{769}{11520}\mathcal{H})T_{abjk}\Lambda_{\alpha l}\Lambda^{\dot{\alpha}m}\epsilon^{\alpha\beta}\nabla_b\Lambda_{\beta m}\epsilon^{ijkl} + (-\frac{61}{360}\mathcal{D}^\dagger\mathcal{I} + \frac{3}{40}\mathcal{D}\mathcal{H})\Lambda_{\alpha j}\Lambda_{\beta k}\Lambda^{\dot{\beta}j}\gamma_b{}^\alpha{}_{\dot{\beta}}\gamma_c{}^{\dot{\alpha}\beta}\nabla_b T_{ac}{}^{ik} \\
& + (-\frac{61}{360}\mathcal{D}^\dagger\mathcal{I} + \frac{3}{40}\mathcal{D}\mathcal{H})\Lambda_{\alpha j}\Lambda_{\beta k}\Lambda^{\dot{\beta}j}\gamma_b{}^\beta{}_{\dot{\beta}}\gamma_c{}^{\dot{\alpha}\alpha}\nabla_b T_{ac}{}^{ik} + (-\frac{1}{6}\bar{\mathcal{I}} - \frac{1}{8}\mathcal{D}^\dagger\mathcal{D}^\dagger\bar{\mathcal{H}})T_{ab}{}^{jk}\Lambda^{\dot{\beta}i}\Lambda^{\dot{\gamma}l}\epsilon_{\dot{\beta}\dot{\gamma}}\nabla_b\Lambda^{\dot{\alpha}m}\epsilon_{jklm} \\
& + (-\frac{1}{6}\bar{\mathcal{I}} + \frac{1}{32}\mathcal{D}^\dagger\mathcal{D}^\dagger\bar{\mathcal{H}})T_{bcjk}\Lambda^{\dot{\beta}j}\Lambda^{\dot{\gamma}l}\chi_{\alpha}{}^{ik}{}_{\iota}\gamma_a{}^{\dot{\alpha}\alpha}\gamma_{bc\dot{\beta}\dot{\gamma}} + (-\frac{1}{6}\mathcal{D}^\dagger\bar{\mathcal{H}} - \frac{7}{24}\mathcal{D}\bar{\mathcal{I}})T_{abjk}\Lambda_{\alpha l}\Lambda^{\dot{\alpha}m}\chi^{\dot{\beta}}{}_{mn}\gamma_b{}^\alpha{}_{\dot{\beta}}\epsilon^{jklm} \\
& + (-\frac{1}{6}\mathcal{D}^\dagger\mathcal{I} + \frac{1}{24}\mathcal{D}\mathcal{H})\Lambda_{\alpha j}\Lambda_{\beta k}\Lambda^{\dot{\beta}i}\gamma_b{}^\alpha{}_{\dot{\beta}}\gamma_c{}^{\dot{\alpha}\beta}\nabla_c T_{ab}{}^{jk} + (-\frac{101}{720}\bar{\mathcal{I}} - \frac{23}{5760}\mathcal{D}^\dagger\mathcal{D}^\dagger\bar{\mathcal{H}})P_b\Lambda_{\alpha j}\Lambda^{\dot{\beta}j}\gamma_c{}^\alpha{}_{\dot{\beta}}\nabla_d\Lambda^{\dot{\alpha}i}\epsilon_{abcd} \\
& + (-\frac{5}{36}\bar{\mathcal{I}} + \frac{1}{192}\mathcal{D}^\dagger\mathcal{D}^\dagger\bar{\mathcal{H}})\Lambda_{\alpha j}\Lambda^{\dot{\beta}i}\Lambda^{\dot{j}j}\gamma_b{}^{\dot{\alpha}\alpha}\gamma_{ac\dot{\beta}\dot{\gamma}}\nabla_c P_b + (-\frac{19}{144}\bar{\mathcal{H}} - \frac{1}{96}\mathcal{H})\Lambda_{\alpha j}\Lambda^{\dot{\beta}i}\Lambda^{\dot{j}j}\gamma_b{}^{\dot{\alpha}\alpha}\gamma_{ac\dot{\beta}\dot{\gamma}}\nabla_b\bar{P}_c \\
& + (-\frac{373}{2880}\mathcal{D}^\dagger\mathcal{I} + \frac{1}{72}\mathcal{D}\mathcal{H})E^{ij}\Lambda_{\alpha j}\Lambda_{\beta k}\Lambda^{\dot{\alpha}k}\bar{P}_a\epsilon^{\alpha\beta} + (-\frac{1441}{11520}\bar{\mathcal{H}} + \frac{563}{2304}\mathcal{H})T_{abjk}\Lambda_{\alpha l}\Lambda^{\dot{\alpha}l}\epsilon^{\alpha\beta}\nabla_b\Lambda_{\beta m}\epsilon^{ijkm} \\
& + (-\frac{1}{8}\bar{\mathcal{H}} - \frac{5}{72}\mathcal{H})P_b\Lambda_{\alpha j}\Lambda_{\beta k}R(Q)_{ac}{}^{\dot{\alpha}}{}_{\iota}\gamma_{bc}{}^{\alpha\beta}\epsilon^{ijkl} + (-\frac{1}{8}\mathcal{D}^\dagger\bar{\mathcal{H}} - \frac{3}{16}\mathcal{D}\bar{\mathcal{I}})T_{abjk}T_{bc}{}^{ij}\Lambda_{\alpha l}\Lambda^{\dot{\alpha}l}\Lambda^{\dot{\beta}k}\gamma_c{}^\alpha{}_{\dot{\beta}} \\
& + (-\frac{1}{8}\mathcal{D}^\dagger\bar{\mathcal{H}} - \frac{3}{16}\mathcal{D}\bar{\mathcal{I}})T_{bcjk}T_{ab}{}^{ij}\Lambda_{\alpha l}\Lambda^{\dot{\alpha}l}\Lambda^{\dot{\beta}k}\gamma_c{}^\alpha{}_{\dot{\beta}} + (-\frac{1}{8}\mathcal{D}^\dagger\bar{\mathcal{H}} + \frac{5}{16}\mathcal{D}\bar{\mathcal{I}})T_{bcjk}\Lambda_{\alpha l}\Lambda^{\dot{\beta}l}R(Q)_{ab}{}^{\dot{\alpha}}{}_{m}\gamma_c{}^\alpha{}_{\dot{\beta}}\epsilon^{ijkm} \\
& + (-\frac{1}{8}\mathcal{D}\mathcal{D}\mathcal{H} - \frac{1}{4}\mathcal{I})T_{bc}{}^{jk}\Lambda_{\alpha j}\Lambda_{\beta l}\chi_{\gamma}{}^{il}{}_{k}\gamma_a{}^{\dot{\alpha}\alpha}\gamma_{bc}{}^{\beta\gamma} + (-\frac{95}{768}\bar{\mathcal{H}} + \frac{11}{11520}\mathcal{H})\Lambda_{\alpha j}\Lambda^{\dot{\beta}i}\bar{P}_b\gamma_c{}^{\dot{\alpha}\alpha}\gamma_{ab\dot{\beta}\dot{\gamma}}\nabla_c\Lambda^{\dot{\gamma}j} \\
& + (-\frac{7}{60}\mathcal{D}^\dagger\mathcal{I} - \frac{43}{240}\mathcal{D}\mathcal{H})T_{bc}{}^{jk}\Lambda_{\alpha j}\Lambda^{\dot{\beta}i}\gamma_b{}^\alpha{}_{\dot{\beta}}\gamma_a{}^{\dot{\alpha}\beta}\nabla_c\Lambda_{\beta k} + (-\frac{7}{60}\mathcal{D}^\dagger\mathcal{I} + \frac{17}{240}\mathcal{D}\mathcal{H})T_{ab}{}^{jk}\Lambda_{\alpha j}\Lambda^{\dot{\beta}i}\gamma_c{}^\beta{}_{\dot{\beta}}\gamma_b{}^{\dot{\alpha}\alpha}\nabla_c\Lambda_{\beta k} \\
& + (-\frac{9}{80}\mathcal{D}^\dagger\mathcal{I} + \frac{1}{15}\mathcal{D}\mathcal{H})T_{ab}{}^{ij}\Lambda_{\alpha j}\Lambda_{\beta k}\gamma_c{}^\alpha{}_{\dot{\beta}}\gamma_b{}^{\dot{\alpha}\beta}\nabla_c\Lambda^{\dot{\beta}k} + (-\frac{9}{80}\mathcal{D}^\dagger\mathcal{I} + \frac{1}{15}\mathcal{D}\mathcal{H})T_{ab}{}^{ij}\Lambda_{\alpha j}\Lambda_{\beta k}\gamma_c{}^\beta{}_{\dot{\beta}}\gamma_b{}^{\dot{\alpha}\alpha}\nabla_c\Lambda^{\dot{\beta}k} \\
& + (-\frac{317}{2880}\bar{\mathcal{H}} - \frac{63}{640}\mathcal{H})\Lambda_{\alpha j}\Lambda^{\dot{\alpha}i}\bar{P}_b\gamma_c{}^\alpha{}_{\dot{\beta}}\nabla_d\Lambda^{\dot{\beta}j}\epsilon_{abcd} + (-\frac{13}{120}\bar{\mathcal{I}} - \frac{29}{480}\mathcal{D}^\dagger\mathcal{D}^\dagger\bar{\mathcal{H}})T_{ab}{}^{jk}\Lambda^{\dot{\alpha}i}\Lambda^{\dot{\beta}l}\epsilon_{\dot{\beta}\dot{\gamma}}\nabla_b\Lambda^{\dot{\gamma}m}\epsilon_{jklm} \\
& + (-\frac{19}{180}\bar{\mathcal{I}} - \frac{79}{1440}\mathcal{D}^\dagger\mathcal{D}^\dagger\bar{\mathcal{H}})T_{bc}{}^{jk}\Lambda^{\dot{\beta}i}\Lambda^{\dot{\gamma}l}\gamma_{ab\dot{\beta}\dot{\gamma}}\nabla_c\Lambda^{\dot{\alpha}m}\epsilon_{jklm} + (-\frac{33}{320}\mathcal{D}^\dagger\bar{\mathcal{H}} - \frac{341}{1920}\mathcal{D}\bar{\mathcal{I}})T_{bcjk}\Lambda_{\alpha l}\Lambda^{\dot{\alpha}l}R(Q)_{bc}{}^{\dot{\beta}}{}_{m}\gamma_a{}^\alpha{}_{\dot{\beta}}\epsilon^{ijkm} \\
& + (-\frac{7}{72}\bar{\mathcal{H}} + \frac{7}{72}\mathcal{H})P_bT_{bc}{}^{ij}\Lambda_{\alpha j}\Lambda_{\beta k}\Lambda^{\dot{\alpha}k}\gamma_{ac}{}^{\alpha\beta} + (-\frac{5}{54}\bar{\mathcal{I}} + \frac{5}{216}\mathcal{D}^\dagger\mathcal{D}^\dagger\bar{\mathcal{H}})T_{abjk}\Lambda^{\dot{\alpha}i}\Lambda^{\dot{\beta}j}\Lambda^{\dot{\gamma}k}\bar{P}_c\gamma_{bc\dot{\beta}\dot{\gamma}} \\
& + (-\frac{5}{54}\bar{\mathcal{I}} + \frac{5}{216}\mathcal{D}^\dagger\mathcal{D}^\dagger\bar{\mathcal{H}})T_{bcjk}\Lambda^{\dot{\alpha}i}\Lambda^{\dot{\beta}j}\Lambda^{\dot{\gamma}k}\bar{P}_b\gamma_{ac\dot{\beta}\dot{\gamma}} + (-\frac{35}{384}\mathcal{D}\mathcal{D}\mathcal{H} + \frac{1}{48}\mathcal{I})T_{bc}{}^{ij}\Lambda_{\alpha j}\Lambda_{\beta k}R(Q)_{ad\gamma}{}^k\gamma_d{}^{\dot{\alpha}\alpha}\gamma_{bc}{}^{\beta\gamma} \\
& + (-\frac{35}{384}\mathcal{D}\mathcal{D}\mathcal{H} + \frac{1}{48}\mathcal{I})T_{bc}{}^{ij}\Lambda_{\alpha j}\Lambda_{\beta k}R(Q)_{ad\gamma}{}^k\gamma_d{}^{\dot{\alpha}\beta}\gamma_{bc}{}^{\alpha\gamma} + (-\frac{13}{144}\mathcal{D}^\dagger\bar{\mathcal{H}} + \frac{25}{64}\mathcal{D}\bar{\mathcal{I}})P_b\Lambda_{\alpha j}\Lambda^{\dot{\alpha}i}\Lambda^{\dot{\beta}j}\bar{P}_a\gamma_b{}^\alpha{}_{\dot{\beta}} + 6\cdots
\end{aligned}$$

$$\begin{aligned}
[\hat{\Omega}_a^{\dot{\alpha}i}]_{3,cont.} = & +(-\frac{13}{144} \mathcal{D}^\dagger \mathcal{I} - \frac{11}{80} \mathcal{D} \mathcal{H}) T_{bc}{}^{ij} \Lambda_{\alpha j} \Lambda^{\dot{\beta}k} \gamma_b{}^\alpha{}_{\dot{\beta}} \gamma_a{}^{\dot{\alpha}\beta} \nabla_c \Lambda_{\beta k} + (-\frac{4}{45} \bar{\mathcal{I}} + \frac{47}{3840} \mathcal{D}^\dagger \mathcal{D}^\dagger \bar{\mathcal{H}}) P_b \Lambda^{\dot{\alpha}i} \Lambda^{\dot{\beta}j} \gamma_c{}^\alpha{}_{\dot{\beta}} \nabla_d \Lambda_{\alpha j} \varepsilon_{abcd} \\
& + (-\frac{7}{80} \mathcal{D}^\dagger \bar{\mathcal{H}} + \frac{1}{6} \mathcal{D} \bar{\mathcal{I}}) P_b \Lambda_{\alpha j} \Lambda^{\dot{\beta}i} R(Q)_{ac\beta}{}^j \gamma_b{}^\beta{}_{\dot{\beta}} \gamma_c{}^{\dot{\alpha}\alpha} + (-\frac{1}{12} \mathcal{D}^\dagger \bar{\mathcal{H}} - \frac{1}{48} \mathcal{D} \bar{\mathcal{I}}) T_{abjk} \Lambda_{\alpha l} \Lambda^{\dot{\beta}l} \chi^{\dot{\alpha}}{}_{mn}{}^i \gamma_b{}^\alpha{}_{\dot{\beta}} \varepsilon^{jkmn} \\
& + (-\frac{1}{12} \mathcal{D}^\dagger \bar{\mathcal{H}} + \frac{1}{8} \mathcal{D} \bar{\mathcal{I}}) P_b \Lambda_{\alpha j} \Lambda^{\dot{\beta}k} \chi_\beta{}^{ij}{}_k \gamma_b{}^\beta{}_{\dot{\beta}} \gamma_a{}^{\dot{\alpha}\alpha} + (-\frac{119}{1440} \bar{\mathcal{H}} - \frac{19}{1440} \mathcal{H}) T_{bcjk} \Lambda_{\alpha l} \Lambda_{\beta m} \gamma_{ab}{}^{\alpha\beta} \nabla_c \Lambda^{\dot{\alpha}j} \varepsilon^{iklm} \\
& + (-\frac{23}{288} \mathcal{D}^\dagger \mathcal{I} + \frac{7}{72} \mathcal{D} \mathcal{H}) \Lambda_{\alpha j} \Lambda^{\dot{\beta}j} R(Q)_{ab\beta}{}^i \bar{P}_c \gamma_c{}^\alpha{}_{\dot{\beta}} \gamma_b{}^{\dot{\alpha}\beta} + (-\frac{11}{144} \bar{\mathcal{H}} + \frac{1}{120} \mathcal{H}) \Lambda_{\alpha j} \Lambda^{\dot{\beta}j} \bar{P}_b \gamma_a{}^{\dot{\alpha}\alpha} \gamma_{bc\dot{\beta}\dot{\gamma}} \nabla_c \Lambda^{\dot{\gamma}i} \\
& + (-\frac{11}{144} \mathcal{D}^\dagger \bar{\mathcal{H}} - \frac{5}{144} \mathcal{D} \bar{\mathcal{I}}) E_{jk} \Lambda^{\dot{\alpha}i} \Lambda^{\dot{\beta}j} \Lambda^{\dot{\gamma}k} \bar{P}_a \epsilon_{\dot{\beta}\dot{\gamma}} + (-\frac{71}{960} \bar{\mathcal{H}} - \frac{1}{2880} \mathcal{H}) T_{bcjk} \Lambda_{\alpha l} \Lambda_{\beta m} \gamma_{ab}{}^{\alpha\beta} \nabla_c \Lambda^{\dot{\alpha}i} \varepsilon^{jklm} \\
& + (-\frac{7}{96} \mathcal{D}^\dagger \bar{\mathcal{H}} - \frac{5}{24} \mathcal{D} \bar{\mathcal{I}}) T_{abjk} T_{bc}{}^{jl} \Lambda_{\alpha l} \Lambda^{\dot{\alpha}i} \Lambda^{\dot{\beta}k} \gamma_c{}^\alpha{}_{\dot{\beta}} + (-\frac{7}{96} \mathcal{D}^\dagger \bar{\mathcal{H}} - \frac{5}{24} \mathcal{D} \bar{\mathcal{I}}) T_{bcjk} T_{ab}{}^{jl} \Lambda_{\alpha l} \Lambda^{\dot{\alpha}i} \Lambda^{\dot{\beta}k} \gamma_c{}^\alpha{}_{\dot{\beta}} \\
& + (-\frac{7}{96} \mathcal{D}^\dagger \bar{\mathcal{H}} - \frac{7}{48} \mathcal{D} \bar{\mathcal{I}}) T_{abjk} T_{bc}{}^{jk} \Lambda_{\alpha l} \Lambda^{\dot{\alpha}l} \Lambda^{\dot{\beta}i} \gamma_c{}^\alpha{}_{\dot{\beta}} + (-\frac{7}{96} \mathcal{D}^\dagger \bar{\mathcal{H}} - \frac{7}{48} \mathcal{D} \bar{\mathcal{I}}) T_{bcjk} T_{ab}{}^{jk} \Lambda_{\alpha l} \Lambda^{\dot{\alpha}l} \Lambda^{\dot{\beta}i} \gamma_c{}^\alpha{}_{\dot{\beta}} \\
& + (-\frac{7}{96} \mathcal{D}^\dagger \mathcal{I} + \frac{1}{48} \mathcal{D} \mathcal{H}) \Lambda_{\alpha j} \Lambda^{\dot{\beta}i} R(Q)_{bc\beta}{}^j \bar{P}_b \gamma_a{}^\alpha{}_{\dot{\beta}} \gamma_c{}^{\dot{\alpha}\beta} + (-\frac{17}{240} \mathcal{D}^\dagger \mathcal{I} + \frac{7}{30} \mathcal{D} \mathcal{H}) T_{bc}{}^{ij} \Lambda_{\alpha j} \Lambda_{\beta k} \gamma_b{}^\alpha{}_{\dot{\beta}} \gamma_a{}^{\dot{\alpha}\beta} \nabla_c \Lambda^{\dot{\beta}k} \\
& + (-\frac{17}{240} \mathcal{D}^\dagger \mathcal{I} + \frac{7}{30} \mathcal{D} \mathcal{H}) T_{bc}{}^{ij} \Lambda_{\alpha j} \Lambda_{\beta k} \gamma_b{}^\beta{}_{\dot{\beta}} \gamma_a{}^{\dot{\alpha}\alpha} \nabla_c \Lambda^{\dot{\beta}k} + (-\frac{9}{128} \mathcal{D} \mathcal{D} \mathcal{H} + \frac{3}{16} \mathcal{I}) T_{bc}{}^{jk} \Lambda_{\alpha j} \Lambda_{\beta k} R(Q)_{ad\gamma}{}^i \gamma_d{}^{\dot{\alpha}\alpha} \gamma_{bc}{}^{\beta\gamma} \\
& + (-\frac{101}{1440} \mathcal{D}^\dagger \mathcal{I} - \frac{1}{20} \mathcal{D} \mathcal{H}) T_{bc}{}^{jk} \Lambda_{\alpha j} \Lambda_{\beta k} \gamma_{bc}{}^{\alpha\beta} \gamma_{ad}{}^{\dot{\alpha}}{}_{\dot{\beta}} \nabla_d \Lambda^{\dot{\beta}i} + (-\frac{13}{192} \mathcal{D} \mathcal{D} \mathcal{H} - \frac{1}{24} \mathcal{I}) T_{bc}{}^{ij} \Lambda_{\alpha k} \Lambda_{\beta l} \chi_\gamma{}^{kl}{}_j \gamma_a{}^{\dot{\alpha}\gamma} \gamma_{bc}{}^{\alpha\beta} \\
& + (-\frac{19}{288} \mathcal{D}^\dagger \mathcal{I} - \frac{5}{144} \mathcal{D} \mathcal{H}) \Lambda_{\alpha j} \Lambda^{\dot{\beta}i} R(Q)_{ab\beta}{}^j \bar{P}_c \gamma_c{}^\alpha{}_{\dot{\beta}} \gamma_b{}^{\dot{\alpha}\beta} + (-\frac{1}{16} \bar{\mathcal{H}} - \frac{5}{144} \mathcal{H}) E_{jk} \Lambda_{\alpha l} \Lambda^{\dot{\beta}j} R(Q)_{ab}{}^{\dot{\alpha}}{}_{m} \gamma_b{}^\alpha{}_{\dot{\beta}} \varepsilon^{iklm} \\
& + (-\frac{11}{180} \mathcal{D}^\dagger \mathcal{I} - \frac{29}{240} \mathcal{D} \mathcal{H}) \Lambda_{\alpha j} \Lambda_{\beta k} \Lambda^{\dot{\beta}i} \gamma_b{}^\alpha{}_{\dot{\beta}} \gamma_c{}^{\dot{\alpha}\beta} \nabla_b T_{ac}{}^{jk} + (-\frac{1}{18} \bar{\mathcal{I}} - \frac{1}{144} \mathcal{D}^\dagger \mathcal{D}^\dagger \bar{\mathcal{H}}) E^{ij} T_{abkl} \Lambda_{\alpha j} \Lambda^{\dot{\alpha}k} \Lambda^{\dot{\beta}l} \gamma_b{}^\alpha{}_{\dot{\beta}} \\
& + (-\frac{1}{18} \mathcal{D}^\dagger \mathcal{D}^\dagger \bar{\mathcal{I}} - \frac{1}{48} \mathcal{D}^\dagger \mathcal{D}^\dagger \mathcal{D}^\dagger \bar{\mathcal{H}}) P_b T_{acjk} \Lambda^{\dot{\alpha}j} \Lambda^{\dot{\beta}i} \Lambda^{\dot{\gamma}k} \gamma_{bc\dot{\beta}\dot{\gamma}} + (-\frac{1}{18} \mathcal{D}^\dagger \mathcal{I} - \frac{1}{144} \mathcal{D} \mathcal{H}) \Lambda_{\alpha j} \Lambda^{\dot{\alpha}j} \Lambda^{\dot{\beta}i} \bar{P}_a \bar{P}_b \gamma_b{}^\alpha{}_{\dot{\beta}} \\
& + (-\frac{7}{128} \bar{\mathcal{H}} + \frac{29}{384} \mathcal{H}) \Lambda^{\dot{\beta}i} \Lambda^{\dot{\gamma}j} \bar{P}_a \epsilon_{\dot{\beta}\dot{\gamma}} \gamma_b{}^{\dot{\alpha}\alpha} \nabla_b \Lambda_{\alpha j} + (-\frac{13}{240} \mathcal{D}^\dagger \bar{\mathcal{I}} - \frac{11}{960} \mathcal{D}^\dagger \mathcal{D}^\dagger \mathcal{D}^\dagger \bar{\mathcal{H}}) T_{bcjk} \Lambda^{\dot{\beta}i} \Lambda^{\dot{\gamma}j} \gamma_{ad\dot{\beta}\dot{\gamma}} \gamma_{bc}{}^{\dot{\alpha}}{}_{\dot{\gamma}} \nabla_d \Lambda^{\dot{\delta}k} \\
& + (-\frac{13}{240} \mathcal{D}^\dagger \bar{\mathcal{I}} - \frac{11}{960} \mathcal{D}^\dagger \mathcal{D}^\dagger \mathcal{D}^\dagger \bar{\mathcal{H}}) T_{bcjk} \Lambda^{\dot{\beta}i} \Lambda^{\dot{\gamma}j} \gamma_{ad\dot{\gamma}\dot{\delta}} \gamma_{bc}{}^{\dot{\alpha}}{}_{\dot{\beta}} \nabla_d \Lambda^{\dot{\delta}k} + (-\frac{13}{240} \mathcal{D}^\dagger \mathcal{I} - \frac{1}{30} \mathcal{D} \mathcal{H}) E^{jk} \Lambda_{\alpha j} \Lambda_{\beta l} \chi_\gamma{}^{il}{}_k \epsilon^{\alpha\gamma} \gamma_a{}^{\dot{\alpha}\beta} \\
& + (-\frac{19}{360} \bar{\mathcal{I}} - \frac{23}{360} \mathcal{D}^\dagger \mathcal{D}^\dagger \bar{\mathcal{H}}) T_{bc}{}^{jk} \Lambda^{\dot{\alpha}l} \Lambda^{\dot{\beta}i} \gamma_{ab\dot{\beta}\dot{\gamma}} \nabla_c \Lambda^{\dot{\gamma}m} \varepsilon_{jklm} + (-\frac{19}{360} \mathcal{D}^\dagger \mathcal{I} + \frac{1}{30} \mathcal{D} \mathcal{H}) T_{ab}{}^{jk} \Lambda_{\alpha j} \Lambda_{\beta k} \gamma_c{}^\alpha{}_{\dot{\beta}} \gamma_b{}^{\dot{\alpha}\beta} \nabla_c \Lambda^{\dot{\beta}i} \\
& + (-\frac{19}{360} \mathcal{D}^\dagger \mathcal{I} + \frac{1}{30} \mathcal{D} \mathcal{H}) T_{bc}{}^{jk} \Lambda_{\alpha j} \Lambda_{\beta k} \gamma_b{}^\alpha{}_{\dot{\beta}} \gamma_a{}^{\dot{\alpha}\beta} \nabla_c \Lambda^{\dot{\beta}i} + (-\frac{121}{2304} \bar{\mathcal{H}} - \frac{67}{2304} \mathcal{H}) \Lambda^{\dot{\beta}i} \Lambda^{\dot{\gamma}j} \bar{P}_b \gamma_c{}^{\dot{\alpha}\alpha} \gamma_{ab\dot{\beta}\dot{\gamma}} \nabla_c \Lambda_{\alpha j} \\
& + (-\frac{5}{96} \bar{\mathcal{H}} + \frac{5}{96} \mathcal{H}) \Lambda^{\dot{\beta}i} \Lambda^{\dot{\gamma}j} \bar{P}_b \epsilon_{\dot{\beta}\dot{\gamma}} \gamma_b{}^{\dot{\alpha}\alpha} \nabla_a \Lambda_{\alpha j} + (-\frac{73}{1440} \bar{\mathcal{H}} - \frac{29}{360} \mathcal{H}) P_a T_{bc}{}^{jk} \Lambda_{\alpha j} \Lambda_{\beta k} \Lambda^{\dot{\alpha}i} \gamma_{bc}{}^{\alpha\beta} \\
& + (-\frac{73}{1440} \bar{\mathcal{H}} + \frac{29}{320} \mathcal{H}) \Lambda^{\dot{\alpha}i} \Lambda^{\dot{\beta}j} \bar{P}_b \gamma_c{}^\alpha{}_{\dot{\beta}} \nabla_d \Lambda_{\alpha j} \varepsilon_{abcd} + (-\frac{1}{20} \mathcal{D}^\dagger \bar{\mathcal{H}} - \frac{1}{96} \mathcal{D} \bar{\mathcal{I}}) P_b \Lambda_{\alpha j} \Lambda^{\dot{\beta}j} R(Q)_{ac\beta}{}^i \gamma_b{}^\alpha{}_{\dot{\beta}} \gamma_c{}^{\dot{\alpha}\beta} \\
& + (-\frac{19}{384} \mathcal{D}^\dagger \bar{\mathcal{H}} + \frac{1}{240} \mathcal{D} \bar{\mathcal{I}}) \Lambda_{\alpha j} \Lambda^{\dot{\alpha}k} \Lambda^{\dot{\beta}j} R(V)_{bc}{}^i{}_k \gamma_d{}^{\dot{\alpha}}{}_{\dot{\beta}} \varepsilon_{abcd} + (-\frac{7}{144} \mathcal{D}^\dagger \bar{\mathcal{H}} + \frac{53}{192} \mathcal{D} \bar{\mathcal{I}}) P_a \Lambda_{\alpha j} \Lambda^{\dot{\alpha}i} \Lambda^{\dot{\beta}j} \bar{P}_b \gamma_b{}^\alpha{}_{\dot{\beta}} \\
& + (-\frac{1}{24} \bar{\mathcal{H}} + \frac{1}{24} \mathcal{H}) P_a \Lambda_{\alpha j} \Lambda_{\beta k} \chi^{\dot{\alpha}}{}_{lm}{}^j \epsilon^{\alpha\beta} \varepsilon^{iklm} + (-\frac{1}{24} \mathcal{D}^\dagger \bar{\mathcal{H}} - \frac{5}{48} \mathcal{D} \bar{\mathcal{I}}) T_{abjk} \Lambda_{\alpha l} \Lambda^{\dot{\beta}l} \chi^{\dot{\alpha}}{}_{mn}{}^i \gamma_b{}^\alpha{}_{\dot{\beta}} \varepsilon^{jkmn} \\
& + (-\frac{1}{24} \mathcal{D}^\dagger \mathcal{I} + \frac{1}{12} \mathcal{D} \mathcal{H}) \Lambda_{\alpha j} \Lambda^{\dot{\beta}k} \bar{P}_b \chi_\beta{}^{ij}{}_k \gamma_b{}^\alpha{}_{\dot{\beta}} \gamma_a{}^{\dot{\alpha}\beta} + (-\frac{1}{24} \mathcal{D} \mathcal{D} \mathcal{H} - \frac{1}{3} \mathcal{I}) T_{ab}{}^{ij} \Lambda_{\alpha j} \Lambda_{\beta k} \Lambda^{\dot{\alpha}k} \bar{P}_c \gamma_{bc}{}^{\alpha\beta} \\
& + (-\frac{1}{24} \mathcal{D} \mathcal{D} \mathcal{H} - \frac{1}{3} \mathcal{I}) T_{bc}{}^{ij} \Lambda_{\alpha j} \Lambda_{\beta k} \Lambda^{\dot{\alpha}k} \bar{P}_b \gamma_{ac}{}^{\alpha\beta} + (-\frac{1}{24} \mathcal{D} \mathcal{D} \mathcal{H} - \frac{1}{6} \mathcal{I}) T_{bc}{}^{ij} \Lambda_{\alpha j} \Lambda_{\beta k} R(Q)_{bc\gamma}{}^k \epsilon^{\alpha\gamma} \gamma_a{}^{\dot{\alpha}\beta} \\
& + (-\frac{1}{24} \mathcal{D} \mathcal{D} \mathcal{H} - \frac{1}{6} \mathcal{I}) T_{bc}{}^{ij} \Lambda_{\alpha j} \Lambda_{\beta k} R(Q)_{bc\gamma}{}^k \epsilon^{\beta\gamma} \gamma_a{}^{\dot{\alpha}\alpha} + (-\frac{19}{480} \mathcal{D}^\dagger \bar{\mathcal{H}} - \frac{293}{2880} \mathcal{D} \bar{\mathcal{I}}) T_{bcjk} \Lambda_{\alpha l} \Lambda^{\dot{\beta}m} R(Q)_{bc}{}^{\dot{\alpha}}{}_{m} \gamma_a{}^\alpha{}_{\dot{\beta}} \varepsilon^{ijkl} \\
& + (-\frac{11}{288} \bar{\mathcal{H}} + \frac{83}{1440} \mathcal{H}) E^{ij} \Lambda_{\alpha k} \Lambda^{\dot{\beta}k} \gamma_b{}^\alpha{}_{\dot{\beta}} \gamma_a{}^{\dot{\alpha}\beta} \nabla_b \Lambda_{\beta j} + (-\frac{3}{80} \mathcal{D}^\dagger \bar{\mathcal{I}} - \frac{7}{640} \mathcal{D}^\dagger \mathcal{D}^\dagger \mathcal{D}^\dagger \bar{\mathcal{H}}) T_{bcjk} \Lambda^{\dot{\beta}j} \Lambda^{\dot{\gamma}k} \gamma_{ad\dot{\beta}\dot{\gamma}} \gamma_{bc}{}^{\dot{\alpha}}{}_{\dot{\gamma}} \nabla_d \Lambda^{\dot{\delta}i} \\
& + (-\frac{53}{1440} \bar{\mathcal{H}} + \frac{37}{960} \mathcal{H}) \Lambda^{\dot{\alpha}j} \Lambda^{\dot{\beta}i} \bar{P}_b \gamma_c{}^\alpha{}_{\dot{\beta}} \nabla_d \Lambda_{\alpha j} \varepsilon_{abcd} + (-\frac{29}{864} \bar{\mathcal{H}} - \frac{5}{288} \mathcal{H}) E_{jk} \Lambda_{\alpha l} \Lambda^{\dot{\beta}j} \chi^{\dot{\alpha}}{}_{mn}{}^l \gamma_a{}^\alpha{}_{\dot{\beta}} \varepsilon^{ikmn} \\
& + (-\frac{1}{30} \mathcal{D}^\dagger \bar{\mathcal{H}} - \frac{1}{384} \mathcal{D} \bar{\mathcal{I}}) P_b \Lambda_{\alpha j} \Lambda^{\dot{\beta}i} R(Q)_{bc\beta}{}^j \gamma_a{}^\alpha{}_{\dot{\beta}} \gamma_c{}^{\dot{\alpha}\beta} + (-\frac{37}{1152} \bar{\mathcal{H}} + \frac{419}{5760} \mathcal{H}) T_{abjk} \Lambda_{\alpha l} \Lambda^{\dot{\alpha}j} \epsilon^{\alpha\beta} \nabla_b \Lambda_{\beta m} \varepsilon^{iklm} \\
& + (-\frac{1}{32} \mathcal{D}^\dagger \bar{\mathcal{I}} - \frac{1}{384} \mathcal{D}^\dagger \mathcal{D}^\dagger \mathcal{D}^\dagger \bar{\mathcal{H}}) E^{ij} \Lambda^{\dot{\beta}k} \Lambda^{\dot{\gamma}l} \gamma_{ab\dot{\beta}\dot{\gamma}} \nabla_b \Lambda^{\dot{\alpha}m} \varepsilon_{jklm} + (-\frac{1}{32} \mathcal{D}^\dagger \mathcal{I} - \frac{1}{80} \mathcal{D} \mathcal{H}) T_{bc}{}^{ij} \Lambda_{\alpha j} \Lambda^{\dot{\beta}k} \gamma_{bc}{}^{\alpha\beta} \gamma_{ad}{}^{\dot{\alpha}}{}_{\dot{\beta}} \nabla_d \Lambda_{\beta k} \\
& + (-\frac{17}{576} \bar{\mathcal{H}} - \frac{17}{960} \mathcal{H}) E^{ij} \Lambda_{\alpha k} \Lambda^{\dot{\beta}k} \gamma_b{}^\beta{}_{\dot{\beta}} \gamma_a{}^{\dot{\alpha}\alpha} \nabla_b \Lambda_{\beta j} + (-\frac{7}{240} \mathcal{D}^\dagger \mathcal{I} + \frac{1}{30} \mathcal{D} \mathcal{H}) E^{jk} \Lambda_{\alpha j} \Lambda_{\beta l} \chi_\gamma{}^{il}{}_k \epsilon^{\beta\gamma} \gamma_a{}^{\dot{\alpha}\alpha} \\
& + (-\frac{1}{36} \bar{\mathcal{I}} - \frac{1}{72} \mathcal{D}^\dagger \mathcal{D}^\dagger \bar{\mathcal{H}}) T_{ab}{}^{jk} \Lambda^{\dot{\alpha}i} \Lambda^{\dot{\beta}l} \gamma_{bc\dot{\beta}\dot{\gamma}} \nabla_c \Lambda^{\dot{\gamma}m} \varepsilon_{jklm} + (-\frac{1}{36} \bar{\mathcal{I}} - \frac{1}{288} \mathcal{D}^\dagger \mathcal{D}^\dagger \bar{\mathcal{H}}) E^{jk} T_{abjl} \Lambda_{\alpha k} \Lambda^{\dot{\alpha}l} \Lambda^{\dot{\beta}i} \gamma_b{}^\alpha{}_{\dot{\beta}} + 7 \dots
\end{aligned}$$

$$\begin{aligned}
[\hat{\Omega}_a^{\dot{\alpha}i}]_{3,cont.} = & +(-\frac{1}{36}\bar{\mathcal{I}} + \frac{1}{96}\mathcal{D}^\dagger\mathcal{D}^\dagger\bar{\mathcal{H}})E_{jk}\Lambda^{\dot{\beta}j}\Lambda^{\dot{\gamma}k}\epsilon_{\dot{\beta}\dot{\gamma}}\gamma_{ab}^{\dot{\alpha}}\nabla_b\Lambda^{\dot{\delta}i} + (-\frac{1}{36}\bar{\mathcal{H}} + \frac{1}{36}\mathcal{H})P_bT_{bc}{}^{jk}\Lambda_{\alpha j}\Lambda_{\beta k}\Lambda^{\dot{\alpha}i}\gamma_{ac}{}^{\alpha\beta} \\
& + (-\frac{1}{36}\mathcal{D}^\dagger\bar{\mathcal{I}} + \frac{1}{96}\mathcal{D}^\dagger\mathcal{D}^\dagger\mathcal{D}^\dagger\bar{\mathcal{H}})E_{jk}P_a\Lambda^{\dot{\alpha}i}\Lambda^{\dot{\beta}j}\Lambda^{\dot{\gamma}k}\epsilon_{\dot{\beta}\dot{\gamma}} + (-\frac{1}{36}\mathcal{D}^\dagger\bar{\mathcal{H}} + \frac{7}{18}\mathcal{D}\bar{\mathcal{I}})P_b\Lambda_{\alpha j}\Lambda^{\dot{\alpha}j}\Lambda^{\dot{\beta}i}\bar{P}_b\gamma_a{}^{\alpha}{}_{\dot{\beta}} \\
& + (-\frac{1}{36}\mathcal{D}^\dagger\mathcal{D}^\dagger\bar{\mathcal{I}} - \frac{1}{96}\mathcal{D}^\dagger\mathcal{D}^\dagger\mathcal{D}^\dagger\mathcal{D}^\dagger\bar{\mathcal{H}})P_bT_{bcjk}\Lambda^{\dot{\alpha}i}\Lambda^{\dot{\beta}j}\Lambda^{\dot{\gamma}k}\gamma_{ac\dot{\beta}\dot{\gamma}} + (-\frac{1}{36}\mathcal{D}^\dagger\mathcal{I} - \frac{1}{288}\mathcal{D}\mathcal{H})E^{jk}\Lambda_{\alpha j}\Lambda_{\beta k}\Lambda^{\dot{\alpha}i}\bar{P}_a\epsilon^{\alpha\beta} \\
& + (-\frac{19}{720}\mathcal{D}^\dagger\mathcal{I} - \frac{7}{320}\mathcal{D}\mathcal{H})\Lambda_{\alpha j}\Lambda_{\beta k}\Lambda^{\dot{\beta}i}\gamma_{bc}{}^{\alpha\beta}\gamma_{ad}{}^{\dot{\alpha}}{}_{\dot{\beta}}\nabla_dT_{bc}{}^{jk} + (-\frac{5}{192}\mathcal{D}\mathcal{D}\mathcal{H} + \frac{1}{8}\mathcal{I})\Lambda_{\alpha j}\Lambda_{\beta k}R(Q)_{ab}{}^{\dot{\alpha}}{}_{\dot{\beta}}\bar{P}_c\gamma_{bc}{}^{\alpha\beta}\epsilon^{ijkl} \\
& + (-\frac{11}{432}\bar{\mathcal{H}} + \frac{1}{144}\mathcal{H})E_{jk}\Lambda_{\alpha l}\Lambda^{\dot{\beta}j}\chi^{\dot{\alpha}}{}_{mn}{}^k\gamma_a{}^{\alpha}{}_{\dot{\beta}}\epsilon^{ilmn} + (-\frac{3}{128}\mathcal{D}^\dagger\bar{\mathcal{H}} + \frac{31}{384}\mathcal{D}\bar{\mathcal{I}})T_{abjk}\Lambda_{\alpha l}\Lambda^{\dot{\beta}i}R(Q)_{bc}{}^{\dot{\alpha}}{}_{\dot{m}}\gamma_c{}^{\alpha}{}_{\dot{\beta}}\epsilon^{jklm} \\
& + (-\frac{5}{216}\bar{\mathcal{H}} - \frac{1}{36}\mathcal{H})E_{jk}\Lambda_{\alpha l}\Lambda^{\dot{\alpha}j}\chi^{\dot{\beta}}{}_{mn}{}^i\gamma_a{}^{\alpha}{}_{\dot{\beta}}\epsilon^{klmn} + (-\frac{7}{320}\mathcal{D}^\dagger\bar{\mathcal{H}} - \frac{19}{1920}\mathcal{D}\bar{\mathcal{I}})T_{bc}{}^{jk}\Lambda^{\dot{\alpha}l}\Lambda^{\dot{\beta}m}R(Q)_{bca}{}^i\gamma_a{}^{\alpha}{}_{\dot{\beta}}\epsilon_{jklm} \\
& + (-\frac{49}{2304}\bar{\mathcal{H}} - \frac{1541}{11520}\mathcal{H})\Lambda_{\alpha j}\Lambda^{\dot{\beta}i}\bar{P}_b\gamma_b{}^{\dot{\alpha}\alpha}\gamma_{ac\dot{\beta}\dot{\gamma}}\nabla_c\Lambda^{\dot{\gamma}j} + (-\frac{1}{48}\bar{\mathcal{I}} + \frac{1}{64}\mathcal{D}^\dagger\mathcal{D}^\dagger\bar{\mathcal{H}})E^{jk}\Lambda^{\dot{\alpha}i}\Lambda^{\dot{\beta}l}\chi_{\alpha}{}^{\dot{\beta}l}{}_{\dot{j}}\gamma_a{}^{\alpha}{}_{\dot{\beta}}\epsilon_{klmn} \\
& + (-\frac{1}{48}\bar{\mathcal{H}} - \frac{1}{18}\mathcal{H})E_{jk}T_{ab}{}^{jl}\Lambda_{\alpha l}\Lambda^{\dot{\alpha}k}\Lambda^{\dot{\beta}i}\gamma_b{}^{\alpha}{}_{\dot{\beta}} + (-\frac{1}{48}\bar{\mathcal{H}} - \frac{1}{32}\mathcal{H})E^{jk}\Lambda_{\alpha j}\Lambda^{\dot{\beta}i}\gamma_a{}^{\alpha}{}_{\dot{\beta}}\gamma_b{}^{\dot{\alpha}\beta}\nabla_b\Lambda_{\beta k} \\
& + (-\frac{1}{48}\mathcal{D}^\dagger\bar{\mathcal{H}} - \frac{1}{12}\mathcal{D}\bar{\mathcal{I}})\Lambda_{\alpha j}\Lambda^{\dot{\beta}i}\Lambda^{\dot{\gamma}k}R(V)_{ab}{}^j{}_k\epsilon_{\dot{\beta}\dot{\gamma}}\gamma_b{}^{\dot{\alpha}\alpha} + (-\frac{1}{48}\mathcal{D}^\dagger\mathcal{I} - \frac{1}{36}\mathcal{D}\mathcal{H})\Lambda_{\alpha j}\chi^{\dot{\beta}}{}_{kl}{}^m\gamma_b{}^{\beta}{}_{\dot{\beta}}\gamma_a{}^{\dot{\alpha}\alpha}\nabla_b\Lambda_{\beta m}\epsilon^{ijkl} \\
& + (-\frac{11}{576}\bar{\mathcal{H}} + \frac{11}{576}\mathcal{H})E^{jk}\Lambda_{\alpha j}\Lambda_{\beta k}\epsilon^{\alpha\beta}\gamma_{ab}{}^{\dot{\alpha}}{}_{\dot{\beta}}\nabla_b\Lambda^{\dot{\beta}i} + (-\frac{5}{288}\mathcal{D}^\dagger\mathcal{I} - \frac{1}{36}\mathcal{D}\mathcal{H})\Lambda_{\alpha j}\chi^{\dot{\beta}}{}_{kl}{}^i\gamma_a{}^{\alpha}{}_{\dot{\beta}}\gamma_b{}^{\dot{\alpha}\beta}\nabla_b\Lambda_{\beta m}\epsilon^{jklm} \\
& + (-\frac{1}{64}\mathcal{D}\mathcal{D}\mathcal{H} - \frac{1}{24}\mathcal{I})\Lambda_{\alpha j}\gamma_b{}^{\dot{\alpha}\beta}\gamma_{ac}{}^{\alpha\gamma}\nabla_b\Lambda_{\beta k}\nabla_c\Lambda_{\gamma l}\epsilon^{ijkl} + (-\frac{11}{960}\bar{\mathcal{H}} + \frac{19}{2880}\mathcal{H})E^{jk}\Lambda_{\alpha j}\Lambda^{\dot{\beta}i}\gamma_b{}^{\alpha}{}_{\dot{\beta}}\gamma_a{}^{\dot{\alpha}\beta}\nabla_b\Lambda_{\beta k} \\
& + (-\frac{13}{1152}\bar{\mathcal{H}} + \frac{13}{1152}\mathcal{H})\Lambda_{\alpha j}\Lambda_{\beta k}\Lambda^{\dot{\beta}j}\gamma_a{}^{\alpha}{}_{\dot{\beta}}\gamma_b{}^{\dot{\alpha}\beta}\nabla_bE^{ik} + (-\frac{13}{1152}\bar{\mathcal{H}} + \frac{13}{1152}\mathcal{H})\Lambda_{\alpha j}\Lambda_{\beta k}\Lambda^{\dot{\beta}j}\gamma_a{}^{\beta}{}_{\dot{\beta}}\gamma_b{}^{\dot{\alpha}\alpha}\nabla_bE^{ik} \\
& + (-\frac{41}{3840}\mathcal{D}^\dagger\bar{\mathcal{H}} + \frac{73}{3840}\mathcal{D}\bar{\mathcal{I}})T_{bcjk}\Lambda_{\alpha l}\Lambda^{\dot{\beta}i}R(Q)_{bc}{}^{\dot{\alpha}}{}_{\dot{m}}\gamma_a{}^{\alpha}{}_{\dot{\beta}}\epsilon^{jklm} + (-\frac{1}{96}\bar{\mathcal{H}} + \frac{1}{96}\mathcal{H})E_{jk}\Lambda_{\alpha l}\Lambda^{\dot{\beta}l}\chi^{\dot{\alpha}}{}_{mn}{}^j\gamma_a{}^{\alpha}{}_{\dot{\beta}}\epsilon^{ikmn} \\
& + (-\frac{1}{96}\mathcal{D}^\dagger\bar{\mathcal{I}} + \frac{1}{384}\mathcal{D}^\dagger\mathcal{D}^\dagger\mathcal{D}^\dagger\bar{\mathcal{H}})\Lambda^{\dot{\alpha}j}\Lambda^{\dot{\beta}k}\Lambda^{\dot{\gamma}l}\gamma_{ab\dot{\beta}\dot{\gamma}}\nabla_bE^{im}\epsilon_{jklm} + (-\frac{1}{96}\mathcal{D}^\dagger\bar{\mathcal{H}} + \frac{1}{192}\mathcal{D}\bar{\mathcal{I}})E_{jk}E^{jl}\Lambda_{\alpha l}\Lambda^{\dot{\alpha}i}\Lambda^{\dot{\beta}k}\gamma_a{}^{\alpha}{}_{\dot{\beta}} \\
& + (-\frac{1}{96}\mathcal{D}^\dagger\mathcal{I} - \frac{1}{72}\mathcal{D}\mathcal{H})\Lambda_{\alpha j}\chi^{\dot{\beta}}{}_{kl}{}^j\gamma_b{}^{\beta}{}_{\dot{\beta}}\gamma_a{}^{\dot{\alpha}\alpha}\nabla_b\Lambda_{\beta m}\epsilon^{iklm} + (-\frac{1}{96}\mathcal{D}^\dagger\mathcal{I} - \frac{1}{80}\mathcal{D}\mathcal{H})T_{bc}{}^{jk}\Lambda_{\alpha j}\Lambda^{\dot{\beta}i}\gamma_{bc}{}^{\alpha\beta}\gamma_{ad}{}^{\dot{\alpha}}{}_{\dot{\beta}}\nabla_d\Lambda_{\beta k} \\
& + (-\frac{1}{96}\mathcal{D}\mathcal{D}\mathcal{H} - \frac{1}{12}\mathcal{I})\Lambda_{\alpha j}\epsilon^{\beta\gamma}\gamma_b{}^{\dot{\alpha}\alpha}\nabla_a\Lambda_{\beta k}\nabla_b\Lambda_{\gamma l}\epsilon^{ijkl} + (-\frac{1}{96}\mathcal{D}\mathcal{D}\mathcal{H} - \frac{1}{12}\mathcal{I})\Lambda_{\alpha j}\gamma_a{}^{\dot{\alpha}\beta}\gamma_{bc}{}^{\alpha\gamma}\nabla_b\Lambda_{\beta k}\nabla_c\Lambda_{\gamma l}\epsilon^{ijkl} \\
& + (-\frac{1}{96}\mathcal{D}\mathcal{D}\mathcal{H} - \frac{1}{12}\mathcal{I})\Lambda_{\alpha j}\gamma_b{}^{\dot{\alpha}\alpha}\gamma_{ac}{}^{\beta\gamma}\nabla_b\Lambda_{\beta k}\nabla_c\Lambda_{\gamma l}\epsilon^{ijkl} + (-\frac{1}{96}\mathcal{D}\mathcal{D}\mathcal{H} + \frac{1}{12}\mathcal{I})T_{bc}{}^{ij}\Lambda_{\alpha k}\Lambda_{\beta l}\chi_{\gamma}{}^{kl}{}_j\gamma_a{}^{\dot{\alpha}\alpha}\gamma_{bc}{}^{\beta\gamma} \\
& + (-\frac{1}{96}\mathcal{D}\mathcal{D}\mathcal{H} + \frac{1}{12}\mathcal{I})\Lambda_{\alpha j}\Lambda_{\beta k}\gamma_b{}^{\dot{\alpha}\gamma}\gamma_{ac}{}^{\alpha\beta}\nabla_b\nabla_c\Lambda_{\gamma l}\epsilon^{ijkl} + (-\frac{37}{3840}\mathcal{D}^\dagger\bar{\mathcal{H}} + \frac{17}{7680}\mathcal{D}\bar{\mathcal{I}})T_{bc}{}^{jk}\Lambda^{\dot{\alpha}l}\Lambda^{\dot{\beta}i}R(Q)_{bca}{}^m\gamma_a{}^{\alpha}{}_{\dot{\beta}}\epsilon_{jklm} \\
& + (-\frac{101}{11520}\bar{\mathcal{H}} + \frac{461}{11520}\mathcal{H})T_{bcjk}\Lambda_{\alpha l}\Lambda^{\dot{\alpha}i}\gamma_{ab}{}^{\alpha\beta}\nabla_c\Lambda_{\beta m}\epsilon^{jklm} + (-\frac{67}{7680}\bar{\mathcal{H}} - \frac{25}{1536}\mathcal{H})\Lambda_{\alpha j}\Lambda^{\dot{\beta}i}\Lambda^{\dot{\gamma}j}\epsilon_{\dot{\beta}\dot{\gamma}}\gamma_b{}^{\dot{\alpha}\alpha}\nabla_a\bar{P}_b \\
& + (-\frac{1}{144}\bar{\mathcal{H}} + \frac{1}{288}\mathcal{H})E^{jk}\Lambda_{\alpha j}\Lambda^{\dot{\beta}i}\gamma_a{}^{\beta}{}_{\dot{\beta}}\gamma_b{}^{\dot{\alpha}\alpha}\nabla_b\Lambda_{\beta k} + (-\frac{19}{2880}\mathcal{D}\mathcal{D}\mathcal{H} + \frac{7}{720}\mathcal{I})T_{bc}{}^{jk}\Lambda_{\alpha j}\Lambda_{\beta k}\Lambda^{\dot{\alpha}i}\bar{P}_a\gamma_{bc}{}^{\alpha\beta} \\
& + (-\frac{1}{192}\bar{\mathcal{H}} + \frac{13}{960}\mathcal{H})E^{ij}\Lambda_{\alpha k}\Lambda^{\dot{\beta}k}\epsilon^{\alpha\beta}\gamma_{ab}{}^{\dot{\alpha}}{}_{\dot{\beta}}\nabla_b\Lambda_{\beta j} + (-\frac{1}{192}\mathcal{D}^\dagger\bar{\mathcal{H}} - \frac{1}{72}\mathcal{D}\bar{\mathcal{I}})\Lambda_{\alpha j}\Lambda^{\dot{\beta}j}\Lambda^{\dot{\gamma}k}R(V)_{bc}{}^i{}_k\gamma_b{}^{\dot{\alpha}\alpha}\gamma_{ac\dot{\beta}\dot{\gamma}} \\
& + (-\frac{1}{192}\mathcal{D}^\dagger\mathcal{I} - \frac{1}{72}\mathcal{D}\mathcal{H})E_{jk}\Lambda_{\alpha l}\Lambda_{\beta m}\gamma_{ab}{}^{\alpha\beta}\nabla_b\Lambda^{\dot{\alpha}j}\epsilon^{iklm} + (-\frac{1}{192}\mathcal{D}\mathcal{D}\mathcal{H} - \frac{1}{24}\mathcal{I})\Lambda_{\alpha j}\Lambda_{\beta k}\gamma_b{}^{\dot{\alpha}\alpha}\gamma_{ac}{}^{\beta\gamma}\nabla_b\nabla_c\Lambda_{\gamma l}\epsilon^{ijkl} \\
& + (-\frac{1}{192}\mathcal{D}\mathcal{D}\mathcal{H} + \frac{1}{24}\mathcal{I})\Lambda_{\alpha j}\Lambda_{\beta k}\epsilon^{\alpha\gamma}\gamma_a{}^{\dot{\alpha}\beta}\nabla_b\nabla_b\Lambda_{\gamma l}\epsilon^{ijkl} + (-\frac{1}{192}\mathcal{D}\mathcal{D}\mathcal{H} + \frac{1}{24}\mathcal{I})\Lambda_{\alpha j}\epsilon^{\alpha\beta}\gamma_b{}^{\dot{\alpha}\gamma}\nabla_a\Lambda_{\gamma k}\nabla_b\Lambda_{\beta l}\epsilon^{ijkl} \\
& + (-\frac{1}{192}\mathcal{D}\mathcal{D}\mathcal{H} + \frac{1}{24}\mathcal{I})\Lambda_{\alpha j}\gamma_b{}^{\dot{\alpha}\beta}\gamma_{ac}{}^{\alpha\gamma}\nabla_b\Lambda_{\gamma k}\nabla_c\Lambda_{\beta l}\epsilon^{ijkl} + (-\frac{1}{216}\bar{\mathcal{I}} + \frac{1}{576}\mathcal{D}^\dagger\mathcal{D}^\dagger\bar{\mathcal{H}})\Lambda^{\dot{\beta}i}\Lambda^{\dot{\gamma}j}\Lambda^{\dot{\delta}k}\epsilon_{\dot{\gamma}\dot{\delta}}\gamma_{ab}{}^{\dot{\alpha}}{}_{\dot{\beta}}\nabla_bE_{jk} \\
& + (-\frac{1}{216}\bar{\mathcal{H}} + \frac{1}{36}\mathcal{H})E_{jk}\Lambda_{\alpha l}\Lambda^{\dot{\alpha}j}\chi^{\dot{\beta}}{}_{mn}{}^k\gamma_a{}^{\alpha}{}_{\dot{\beta}}\epsilon^{ilmn} + (-\frac{1}{288}\mathcal{D}^\dagger\bar{\mathcal{H}} + \frac{1}{576}\mathcal{D}\bar{\mathcal{I}})E_{jk}E^{ij}\Lambda_{\alpha l}\Lambda^{\dot{\alpha}k}\Lambda^{\dot{\beta}l}\gamma_a{}^{\alpha}{}_{\dot{\beta}} \\
& + (-\frac{1}{384}\mathcal{D}^\dagger\bar{\mathcal{H}} - \frac{9}{320}\mathcal{D}\bar{\mathcal{I}})\Lambda_{\alpha j}\Lambda^{\dot{\alpha}i}\Lambda^{\dot{\beta}k}R(V)_{bc}{}^j{}_k\gamma_d{}^{\alpha}{}_{\dot{\beta}}\epsilon_{abcd} + (-\frac{1}{384}\mathcal{D}^\dagger\bar{\mathcal{H}} + \frac{1}{144}\mathcal{D}\bar{\mathcal{I}})E_{jk}E^{jk}\Lambda_{\alpha l}\Lambda^{\dot{\alpha}i}\Lambda^{\dot{\beta}l}\gamma_a{}^{\alpha}{}_{\dot{\beta}} \\
& + (-\frac{1}{512}\mathcal{D}^\dagger\bar{\mathcal{H}} + \frac{13}{2304}\mathcal{D}\bar{\mathcal{I}})\Lambda_{\alpha j}\Lambda^{\dot{\beta}i}\Lambda^{\dot{\gamma}k}R(V)_{bc}{}^j{}_k\gamma_a{}^{\dot{\alpha}\alpha}\gamma_{bc\dot{\beta}\dot{\gamma}} + (-\frac{17}{11520}\bar{\mathcal{H}} + \frac{193}{11520}\mathcal{H})E^{ij}\Lambda_{\alpha j}\Lambda^{\dot{\beta}k}\gamma_a{}^{\beta}{}_{\dot{\beta}}\gamma_b{}^{\dot{\alpha}\alpha}\nabla_b\Lambda_{\beta k} \\
& + (-\frac{1}{1440}\bar{\mathcal{H}} + \frac{13}{1440}\mathcal{H})E^{ij}\Lambda_{\alpha j}\Lambda^{\dot{\beta}k}\gamma_b{}^{\beta}{}_{\dot{\beta}}\gamma_a{}^{\dot{\alpha}\alpha}\nabla_b\Lambda_{\beta k} + (\frac{17}{7680}\bar{\mathcal{H}} + \frac{67}{1536}\mathcal{H})\Lambda_{\alpha j}\Lambda^{\dot{\beta}i}\Lambda^{\dot{\gamma}j}\epsilon_{\dot{\beta}\dot{\gamma}}\gamma_b{}^{\dot{\alpha}\alpha}\nabla_b\bar{P}_a \\
& + (\frac{19}{7680}\bar{\mathcal{H}} + \frac{29}{7680}\mathcal{H})E^{ij}\Lambda_{\alpha j}\Lambda_{\beta k}\gamma_a{}^{\alpha}{}_{\dot{\beta}}\gamma_b{}^{\dot{\alpha}\beta}\nabla_b\Lambda^{\dot{\beta}k} + (\frac{19}{7680}\bar{\mathcal{H}} + \frac{29}{7680}\mathcal{H})E^{ij}\Lambda_{\alpha j}\Lambda_{\beta k}\gamma_a{}^{\beta}{}_{\dot{\beta}}\gamma_b{}^{\dot{\alpha}\alpha}\nabla_b\Lambda^{\dot{\beta}k} \\
& + (\frac{1}{384}\mathcal{D}^\dagger\bar{\mathcal{H}} - \frac{1}{144}\mathcal{D}\bar{\mathcal{I}})E_{jk}E^{jk}\Lambda_{\alpha l}\Lambda^{\dot{\alpha}l}\Lambda^{\dot{\beta}i}\gamma_a{}^{\alpha}{}_{\dot{\beta}} + (\frac{1}{384}\mathcal{D}^\dagger\bar{\mathcal{H}} + \frac{9}{320}\mathcal{D}\bar{\mathcal{I}})\Lambda_{\alpha j}\Lambda^{\dot{\alpha}j}\Lambda^{\dot{\beta}k}R(V)_{bc}{}^i{}_k\gamma_d{}^{\alpha}{}_{\dot{\beta}}\epsilon_{abcd} + 8\cdots
\end{aligned}$$



$$\begin{aligned}
[\hat{\Omega}_a^{\dot{\alpha}i}]_{3,cont.} = & + \left( \frac{1}{320} \bar{\mathcal{H}} - \frac{43}{960} \mathcal{H} \right) \Lambda_{\alpha j} \Lambda_{\beta k} \Lambda^{\dot{\alpha}j} \gamma_{ab}^{\alpha\beta} \nabla_c T_{bclm} \varepsilon^{iklm} + \left( \frac{1}{320} \bar{\mathcal{H}} + \frac{37}{960} \mathcal{H} \right) \Lambda_{\alpha j} \Lambda_{\beta k} \Lambda^{\dot{\alpha}l} \gamma_{ab}^{\alpha\beta} \nabla_c T_{bclm} \varepsilon^{ijkm} \\
& + \left( \frac{1}{288} \bar{\mathcal{H}} + \frac{1}{288} \mathcal{H} \right) \Lambda_{\alpha j} \Lambda_{\beta k} \Lambda^{\dot{\beta}i} \epsilon^{\alpha\beta} \gamma_{ab}^{\dot{\alpha}} \nabla_b E^{jk} + \left( \frac{1}{288} \mathcal{D}^\dagger \bar{\mathcal{H}} - \frac{1}{576} \mathcal{D} \bar{\mathcal{I}} \right) E_{jk} E^{ij} \Lambda_{\alpha l} \Lambda^{\dot{\alpha}l} \Lambda^{\dot{\beta}k} \gamma_a^{\alpha} \gamma_{\dot{\beta}} \\
& + \left( \frac{1}{256} \mathcal{D}^\dagger \bar{\mathcal{H}} + \frac{11}{1152} \mathcal{D} \bar{\mathcal{I}} \right) \Lambda_{\alpha j} \Lambda^{\dot{\beta}i} \Lambda^{\dot{\gamma}k} R(V)_{bc}{}^j{}_{k\gamma b}{}^{\dot{\alpha}} \gamma_{ac\dot{\beta}\dot{\gamma}} + \left( \frac{49}{11520} \bar{\mathcal{H}} - \frac{511}{11520} \mathcal{H} \right) T_{abjk} \Lambda_{\alpha l} \Lambda^{\dot{\alpha}i} \epsilon^{\alpha\beta} \nabla_b \Lambda_{\beta m} \varepsilon^{ijklm} \\
& + \left( \frac{1}{216} \bar{\mathcal{I}} - \frac{1}{576} \mathcal{D}^\dagger \mathcal{D}^\dagger \bar{\mathcal{H}} \right) \Lambda^{\dot{\beta}i} \Lambda^{\dot{\gamma}j} \Lambda^{\dot{\delta}k} \epsilon_{\dot{\beta}\dot{\gamma}} \gamma_{ab}^{\dot{\alpha}} \nabla_b E_{jk} + \left( \frac{1}{192} \mathcal{D} \mathcal{D} \mathcal{H} + \frac{1}{24} \mathcal{I} \right) \Lambda_{\alpha j} \Lambda_{\beta k} \epsilon^{\alpha\gamma} \gamma_b^{\dot{\alpha}\beta} \nabla_a \nabla_b \Lambda_{\gamma l} \varepsilon^{ijkl} \\
& + \left( \frac{1}{192} \mathcal{D} \mathcal{D} \mathcal{H} + \frac{1}{8} \mathcal{I} \right) \Lambda_{\alpha j} \epsilon^{\alpha\beta} \gamma_b^{\dot{\alpha}\gamma} \nabla_a \Lambda_{\beta k} \nabla_b \Lambda_{\gamma l} \varepsilon^{ijkl} + \left( \frac{1}{144} \mathcal{D}^\dagger \bar{\mathcal{I}} - \frac{1}{576} \mathcal{D}^\dagger \mathcal{D}^\dagger \mathcal{D}^\dagger \bar{\mathcal{H}} \right) \Lambda^{\dot{\beta}i} \Lambda^{\dot{\gamma}j} \Lambda^{\dot{\delta}k} \gamma_{bc\dot{\gamma}\dot{\delta}} \gamma_{ad}^{\dot{\alpha}} \nabla_d T_{bcjk} \\
& + \left( \frac{1}{144} \mathcal{D}^\dagger \mathcal{I} + \frac{7}{240} \mathcal{D} \mathcal{H} \right) T_{ab}{}^{ij} \Lambda_{\alpha j} \Lambda^{\dot{\beta}k} \gamma_c^{\beta} \gamma_b^{\dot{\beta}} \gamma_a^{\dot{\alpha}} \nabla_c \Lambda_{\beta k} + \left( \frac{1}{128} \bar{\mathcal{H}} - \frac{17}{1152} \mathcal{H} \right) \Lambda_{\alpha j} \Lambda_{\beta k} \Lambda^{\dot{\beta}j} \gamma_b^{\alpha} \gamma_a^{\dot{\beta}} \nabla_b E^{ik} \\
& + \left( \frac{1}{128} \bar{\mathcal{H}} - \frac{17}{1152} \mathcal{H} \right) \Lambda_{\alpha j} \Lambda_{\beta k} \Lambda^{\dot{\beta}j} \gamma_b^{\beta} \gamma_a^{\dot{\alpha}} \nabla_b E^{ik} + \left( \frac{7}{864} \bar{\mathcal{H}} + \frac{7}{288} \mathcal{H} \right) E_{jk} \Lambda_{\alpha l} \Lambda^{\dot{\beta}j} \chi^{\dot{\alpha}}{}_{mn}{}^i \gamma_a^{\alpha} \gamma_{\dot{\beta}} \varepsilon^{klmn} \\
& + \left( \frac{1}{120} \mathcal{D}^\dagger \mathcal{I} + \frac{4}{15} \mathcal{D} \mathcal{H} \right) T_{bc}{}^{ij} \Lambda_{\alpha j} \Lambda^{\dot{\beta}k} \gamma_a^{\alpha} \gamma_{\dot{\beta}} \gamma_b^{\dot{\alpha}\beta} \nabla_c \Lambda_{\beta k} + \left( \frac{5}{576} \bar{\mathcal{H}} - \frac{13}{576} \mathcal{H} \right) E^{ij} \Lambda_{\alpha k} \Lambda^{\dot{\beta}k} \gamma_a^{\beta} \gamma_b^{\dot{\beta}} \gamma_a^{\dot{\alpha}} \nabla_b \Lambda_{\beta j} \\
& + \left( \frac{13}{1440} \bar{\mathcal{H}} - \frac{13}{1440} \mathcal{H} \right) E^{ij} \Lambda_{\alpha j} \Lambda^{\dot{\beta}k} \epsilon^{\alpha\beta} \gamma_{ab}^{\dot{\alpha}} \nabla_b \Lambda_{\beta k} + \left( \frac{1}{108} \bar{\mathcal{H}} - \frac{1}{108} \mathcal{H} \right) P_b \Lambda_{\alpha j} \Lambda_{\beta k} \chi^{\dot{\alpha}}{}_{lm}{}^i \gamma_{ab}^{\alpha\beta} \varepsilon^{ijklm} \\
& + \left( \frac{1}{108} \bar{\mathcal{H}} - \frac{1}{108} \mathcal{H} \right) P_b \Lambda_{\alpha j} \Lambda_{\beta k} \chi^{\dot{\alpha}}{}_{lm}{}^j \gamma_{ab}^{\alpha\beta} \varepsilon^{iklm} + \left( \frac{37}{3840} \mathcal{D}^\dagger \bar{\mathcal{H}} - \frac{17}{7680} \mathcal{D} \bar{\mathcal{I}} \right) T_{bc}{}^{jk} \Lambda^{\dot{\alpha}i} \Lambda^{\dot{\beta}l} R(Q)_{bca}{}^m \gamma_a^{\alpha} \gamma_{\dot{\beta}} \varepsilon^{ijklm} \\
& + \left( \frac{19}{1920} \mathcal{D}^\dagger \bar{\mathcal{H}} - \frac{499}{3840} \mathcal{D} \bar{\mathcal{I}} \right) T_{bcjk} \Lambda_{\alpha l} \Lambda^{\dot{\alpha}i} R(Q)_{bc}{}^{\dot{\beta}}{}_{m\gamma a}{}^{\alpha} \dot{\beta} \varepsilon^{ijklm} + \left( \frac{1}{96} \mathcal{D}^\dagger \bar{\mathcal{H}} - \frac{1}{192} \mathcal{D} \bar{\mathcal{I}} \right) E_{jk} E^{jl} \Lambda_{\alpha l} \Lambda^{\dot{\alpha}k} \Lambda^{\dot{\beta}i} \gamma_a^{\alpha} \gamma_{\dot{\beta}} \\
& + \left( \frac{1}{96} \mathcal{D}^\dagger \mathcal{I} + \frac{1}{72} \mathcal{D} \mathcal{H} \right) \Lambda_{\alpha j} \chi^{\dot{\beta}}{}_{kl}{}^i \gamma_b^{\beta} \gamma_a^{\dot{\alpha}} \nabla_b \Lambda_{\beta m} \varepsilon^{ijklm} + \left( \frac{11}{960} \bar{\mathcal{H}} + \frac{61}{2880} \mathcal{H} \right) E^{jk} \Lambda_{\alpha j} \Lambda^{\dot{\beta}i} \gamma_b^{\beta} \gamma_a^{\dot{\alpha}} \nabla_b \Lambda_{\beta k} \\
& + \left( \frac{1}{80} \bar{\mathcal{H}} + \frac{1}{80} \mathcal{H} \right) E^{ij} \Lambda_{\alpha j} \Lambda_{\beta k} \gamma_b^{\alpha} \gamma_a^{\dot{\beta}} \nabla_b \Lambda^{\dot{\beta}k} + \left( \frac{1}{80} \bar{\mathcal{H}} + \frac{1}{80} \mathcal{H} \right) E^{ij} \Lambda_{\alpha j} \Lambda_{\beta k} \gamma_b^{\beta} \gamma_a^{\dot{\alpha}} \nabla_b \Lambda^{\dot{\beta}k} \\
& + \left( \frac{1}{72} \bar{\mathcal{H}} + \frac{37}{640} \mathcal{H} \right) \Lambda_{\alpha j} \Lambda^{\dot{\beta}i} \bar{P}_b \gamma_a^{\dot{\alpha}} \gamma_{bc\dot{\beta}\dot{\gamma}} \nabla_c \Lambda^{\dot{\gamma}j} + \left( \frac{1}{72} \mathcal{D}^\dagger \bar{\mathcal{I}} - \frac{1}{288} \mathcal{D}^\dagger \mathcal{D}^\dagger \mathcal{D}^\dagger \bar{\mathcal{H}} \right) \Lambda^{\dot{\beta}i} \Lambda^{\dot{\gamma}j} \Lambda^{\dot{\delta}k} \gamma_{bc\dot{\beta}\dot{\gamma}} \gamma_{ad}^{\dot{\alpha}} \nabla_d T_{bcjk} \\
& + \left( \frac{1}{72} \mathcal{D} \mathcal{D} \mathcal{H} + \frac{1}{9} \mathcal{I} \right) \Lambda_{\alpha j} \Lambda_{\beta k} \bar{P}_b \chi^{\dot{\alpha}}{}_{lm}{}^i \gamma_{ab}^{\alpha\beta} \varepsilon^{ijklm} + \left( \frac{1}{72} \mathcal{D} \mathcal{D} \mathcal{H} + \frac{1}{9} \mathcal{I} \right) \Lambda_{\alpha j} \Lambda_{\beta k} \bar{P}_b \chi^{\dot{\alpha}}{}_{lm}{}^j \gamma_{ab}^{\alpha\beta} \varepsilon^{iklm} \\
& + \left( \frac{13}{768} \bar{\mathcal{H}} - \frac{15}{256} \mathcal{H} \right) \Lambda^{\dot{\beta}i} \Lambda^{\dot{\gamma}j} \bar{P}_b \epsilon_{\dot{\beta}\dot{\gamma}} \gamma_a^{\dot{\alpha}} \nabla_b \Lambda_{\alpha j} + \left( \frac{5}{288} \bar{\mathcal{H}} - \frac{1}{32} \mathcal{H} \right) E^{ij} \Lambda_{\alpha j} \Lambda^{\dot{\beta}k} \gamma_a^{\alpha} \gamma_{\dot{\beta}} \gamma_b^{\dot{\alpha}\beta} \nabla_b \Lambda_{\beta k} \\
& + \left( \frac{5}{288} \mathcal{D}^\dagger \mathcal{I} + \frac{1}{36} \mathcal{D} \mathcal{H} \right) \Lambda_{\alpha j} \Lambda_{\beta k} \gamma_b^{\alpha} \gamma_a^{\dot{\beta}} \nabla_b \chi^{\dot{\beta}}{}_{lm}{}^i \varepsilon^{ijklm} + \left( \frac{1}{54} \bar{\mathcal{H}} + \frac{1}{18} \mathcal{H} \right) E_{jk} \Lambda_{\alpha l} \Lambda^{\dot{\alpha}j} \chi^{\dot{\beta}}{}_{mn}{}^l \gamma_a^{\alpha} \gamma_{\dot{\beta}} \varepsilon^{ikmn} \\
& + \left( \frac{3}{160} \mathcal{D}^\dagger \bar{\mathcal{H}} + \frac{131}{960} \mathcal{D} \bar{\mathcal{I}} \right) T_{bcjk} \Lambda_{\alpha l} \Lambda^{\dot{\beta}l} R(Q)_{bc}{}^{\dot{\alpha}}{}_{m\gamma a}{}^{\alpha} \dot{\beta} \varepsilon^{ijkm} + \left( \frac{221}{11520} \bar{\mathcal{H}} - \frac{1061}{11520} \mathcal{H} \right) T_{bcjk} \Lambda_{\alpha l} \Lambda^{\dot{\alpha}l} \gamma_{ab}^{\alpha\beta} \nabla_c \Lambda_{\beta m} \varepsilon^{ijkm} \\
& + \left( \frac{37}{1920} \bar{\mathcal{H}} - \frac{37}{1920} \mathcal{H} \right) \Lambda_{\alpha j} \Lambda_{\beta k} \Lambda^{\dot{\alpha}i} \gamma_{ab}^{\alpha\beta} \nabla_c T_{bclm} \varepsilon^{ijklm} + \left( \frac{1}{48} \bar{\mathcal{H}} + \frac{1}{18} \mathcal{H} \right) E_{jk} T_{ab}{}^{jl} \Lambda_{\alpha l} \Lambda^{\dot{\alpha}i} \Lambda^{\dot{\beta}k} \gamma_b^{\alpha} \gamma_{\dot{\beta}} \\
& + \left( \frac{1}{48} \mathcal{D}^\dagger \bar{\mathcal{I}} - \frac{1}{192} \mathcal{D}^\dagger \mathcal{D}^\dagger \mathcal{D}^\dagger \bar{\mathcal{H}} \right) E^{ij} \Lambda^{\dot{\alpha}k} \Lambda^{\dot{\beta}l} \gamma_{ab\dot{\gamma}} \nabla_b \Lambda^{\dot{\gamma}m} \varepsilon_{ijklm} + \left( \frac{121}{5760} \bar{\mathcal{H}} - \frac{1}{5760} \mathcal{H} \right) T_{bcjk} \Lambda_{\alpha l} \Lambda^{\dot{\alpha}j} \gamma_{ab}^{\alpha\beta} \nabla_c \Lambda_{\beta m} \varepsilon^{ijklm} \\
& + \left( \frac{3}{128} \mathcal{D}^\dagger \bar{\mathcal{H}} + \frac{17}{288} \mathcal{D} \bar{\mathcal{I}} \right) \Lambda_{\alpha j} \Lambda^{\dot{\beta}j} \Lambda^{\dot{\gamma}k} R(V)_{bc}{}^i{}_{k\gamma a}{}^{\dot{\alpha}} \gamma_{bc\dot{\beta}\dot{\gamma}} + \left( \frac{77}{2880} \mathcal{D}^\dagger \mathcal{I} + \frac{3}{80} \mathcal{D} \mathcal{H} \right) T_{bc}{}^{ij} \Lambda_{\alpha k} \Lambda^{\dot{\beta}k} \gamma_{bc}^{\alpha\beta} \gamma_{ad}^{\dot{\alpha}} \nabla_d \Lambda_{\beta j} \\
& + \left( \frac{1}{36} \bar{\mathcal{I}} + \frac{1}{288} \mathcal{D}^\dagger \mathcal{D}^\dagger \bar{\mathcal{H}} \right) E^{jk} T_{abjl} \Lambda_{\alpha k} \Lambda^{\dot{\alpha}i} \Lambda^{\dot{\beta}l} \gamma_b^{\alpha} \gamma_{\dot{\beta}} + \left( \frac{1}{36} \bar{\mathcal{I}} + \frac{1}{72} \mathcal{D}^\dagger \mathcal{D}^\dagger \bar{\mathcal{H}} \right) T_{ab}{}^{jk} \Lambda^{\dot{\alpha}l} \Lambda^{\dot{\beta}i} \gamma_{bc\dot{\beta}\dot{\gamma}} \nabla_c \Lambda^{\dot{\gamma}m} \varepsilon_{ijklm} \\
& + \left( \frac{1}{36} \bar{\mathcal{H}} - \frac{1}{36} \mathcal{H} \right) P_b T_{ac}{}^{jk} \Lambda_{\alpha j} \Lambda_{\beta k} \Lambda^{\dot{\alpha}i} \gamma_{bc}^{\alpha\beta} + \left( \frac{1}{36} \bar{\mathcal{H}} - \frac{1}{360} \mathcal{H} \right) E^{ij} \Lambda_{\alpha j} \Lambda^{\dot{\beta}k} \gamma_b^{\alpha} \gamma_{\dot{\beta}} \gamma_a^{\dot{\alpha}\beta} \nabla_b \Lambda_{\beta k} \\
& + \left( \frac{1}{36} \bar{\mathcal{H}} + \frac{1}{144} \mathcal{H} \right) \Lambda_{\alpha j} \Lambda_{\beta k} \Lambda^{\dot{\beta}j} \epsilon^{\alpha\beta} \gamma_{ab}^{\dot{\alpha}} \nabla_b E^{ik} + \left( \frac{1}{36} \mathcal{D}^\dagger \bar{\mathcal{I}} - \frac{1}{96} \mathcal{D}^\dagger \mathcal{D}^\dagger \mathcal{D}^\dagger \bar{\mathcal{H}} \right) E_{jk} P_a \Lambda^{\dot{\alpha}j} \Lambda^{\dot{\beta}i} \Lambda^{\dot{\gamma}k} \epsilon_{\dot{\beta}\dot{\gamma}} \\
& + \left( \frac{1}{36} \mathcal{D}^\dagger \bar{\mathcal{H}} - \frac{7}{18} \mathcal{D} \bar{\mathcal{I}} \right) P_b \Lambda_{\alpha j} \Lambda^{\dot{\alpha}i} \Lambda^{\dot{\beta}j} \bar{P}_b \gamma_a^{\alpha} \gamma_{\dot{\beta}} + \left( \frac{1}{36} \mathcal{D}^\dagger \mathcal{D}^\dagger \bar{\mathcal{I}} + \frac{1}{96} \mathcal{D}^\dagger \mathcal{D}^\dagger \mathcal{D}^\dagger \bar{\mathcal{H}} \right) P_b T_{acjk} \Lambda^{\dot{\alpha}i} \Lambda^{\dot{\beta}j} \Lambda^{\dot{\gamma}k} \gamma_{bc\dot{\beta}\dot{\gamma}} \\
& + \left( \frac{25}{768} \bar{\mathcal{H}} - \frac{5}{768} \mathcal{H} \right) \Lambda^{\dot{\beta}i} \Lambda^{\dot{\gamma}j} \bar{P}_b \gamma_b^{\dot{\alpha}} \gamma_{ac\dot{\beta}\dot{\gamma}} \nabla_c \Lambda_{\alpha j} + \left( \frac{1}{30} \mathcal{D}^\dagger \bar{\mathcal{I}} + \frac{13}{960} \mathcal{D}^\dagger \mathcal{D}^\dagger \mathcal{D}^\dagger \bar{\mathcal{H}} \right) T_{bcjk} \Lambda^{\dot{\beta}i} \Lambda^{\dot{\gamma}j} \gamma_{bc\dot{\beta}\dot{\gamma}} \gamma_{ad}^{\dot{\alpha}} \nabla_d \Lambda^{\dot{\delta}k} \\
& + \left( \frac{1}{30} \mathcal{D}^\dagger \mathcal{I} - \frac{1}{60} \mathcal{D} \mathcal{H} \right) T_{bc}{}^{jk} \Lambda_{\alpha j} \Lambda^{\dot{\beta}i} \gamma_a^{\beta} \gamma_b^{\dot{\beta}} \gamma_a^{\dot{\alpha}} \nabla_c \Lambda_{\beta k} + \left( \frac{103}{2880} \bar{\mathcal{H}} - \frac{79}{2880} \mathcal{H} \right) E^{jk} \Lambda_{\alpha j} \Lambda^{\dot{\beta}i} \epsilon^{\alpha\beta} \gamma_{ab}^{\dot{\alpha}} \nabla_b \Lambda_{\beta k} \\
& + \left( \frac{11}{288} \mathcal{D}^\dagger \mathcal{I} + \frac{1}{36} \mathcal{D} \mathcal{H} \right) \Lambda_{\alpha j} \chi^{\dot{\beta}}{}_{kl}{}^i \gamma_a^{\alpha} \gamma_{\dot{\beta}} \gamma_b^{\dot{\alpha}\beta} \nabla_b \Lambda_{\beta m} \varepsilon^{iklm} + \left( \frac{19}{480} \mathcal{D}^\dagger \bar{\mathcal{I}} + \frac{1}{480} \mathcal{D}^\dagger \mathcal{D}^\dagger \mathcal{D}^\dagger \bar{\mathcal{H}} \right) T_{bcjk} \Lambda^{\dot{\beta}j} \Lambda^{\dot{\gamma}k} \gamma_{bc\dot{\beta}\dot{\gamma}} \gamma_{ad}^{\dot{\alpha}} \nabla_d \Lambda^{\dot{\delta}i} \\
& + \left( \frac{1}{24} \bar{\mathcal{I}} - \frac{1}{192} \mathcal{D}^\dagger \mathcal{D}^\dagger \bar{\mathcal{H}} \right) E^{ij} \Lambda^{\dot{\alpha}k} \Lambda^{\dot{\beta}l} \chi_{\alpha}{}^{mn}{}_{j\gamma a}{}^{\alpha} \dot{\beta} \varepsilon_{klmn} + \left( \frac{1}{24} \bar{\mathcal{I}} - \frac{1}{192} \mathcal{D}^\dagger \mathcal{D}^\dagger \bar{\mathcal{H}} \right) E^{ij} \Lambda^{\dot{\alpha}k} \Lambda^{\dot{\beta}l} \chi_{\alpha}{}^{mn}{}_{l\gamma a}{}^{\alpha} \dot{\beta} \varepsilon_{jkmn} \\
& + \left( \frac{1}{24} \bar{\mathcal{I}} + \frac{1}{192} \mathcal{D}^\dagger \mathcal{D}^\dagger \bar{\mathcal{H}} \right) P_b \Lambda_{\alpha j} \Lambda^{\dot{\beta}i} \gamma_a^{\dot{\alpha}} \gamma_{bc\dot{\beta}\dot{\gamma}} \nabla_c \Lambda^{\dot{\gamma}j} + \left( \frac{1}{24} \mathcal{D}^\dagger \bar{\mathcal{H}} - \frac{5}{48} \mathcal{D} \bar{\mathcal{I}} \right) T_{abjk} \Lambda_{\alpha l} \Lambda^{\dot{\beta}l} R(Q)_{bc}{}^{\dot{\alpha}}{}_{m\gamma c}{}^{\alpha} \dot{\beta} \varepsilon^{ijkm} + 9 \dots
\end{aligned}$$

$$\begin{aligned}
[\hat{\Omega}_a^{\dot{\alpha}i}]_{3,cont.} = & + \left( \frac{1}{24} \mathcal{D}^\dagger \bar{\mathcal{H}} + \frac{7}{48} \mathcal{D} \bar{\mathcal{I}} \right) T_{abjk} \Lambda_{\alpha l} \Lambda^{\dot{\alpha} l} \chi^{\dot{\beta}}{}_{mn} \gamma_b{}^\alpha{}_{\dot{\beta}} \varepsilon^{jkmn} + \left( \frac{1}{24} \mathcal{D}^\dagger \mathcal{I} + \frac{1}{12} \mathcal{D} \mathcal{H} \right) \Lambda_{\alpha j} \Lambda^{\dot{\beta} k} \bar{P}_b \chi_{\beta}{}^{ij}{}_{\dot{k}} \gamma_a{}^\alpha{}_{\dot{\beta}} \gamma_b{}^{\dot{\alpha} \beta} \\
& + \left( \frac{11}{256} \bar{\mathcal{H}} + \frac{7}{768} \mathcal{H} \right) \Lambda_{\alpha j} \Lambda^{\dot{\beta} i} \Lambda^{\dot{\gamma} j} \epsilon_{\dot{\beta} \dot{\gamma}} \gamma_a{}^{\dot{\alpha} \alpha} \nabla_b \bar{P}_b + \left( \frac{499}{11520} \bar{\mathcal{H}} + \frac{341}{11520} \mathcal{H} \right) T_{bcjk} \Lambda_{\alpha l} \Lambda^{\dot{\alpha} m} \gamma_{ab}{}^{\alpha \beta} \nabla_c \Lambda_{\beta m} \varepsilon^{ijkl} \\
& + \left( \frac{1001}{23040} \bar{\mathcal{H}} - \frac{1049}{23040} \mathcal{H} \right) E^{ij} \Lambda_{\alpha j} \Lambda_{\beta k} \epsilon^{\alpha \beta} \gamma_{ab}{}^{\dot{\alpha}}{}_{\dot{\beta}} \nabla_b \Lambda^{\dot{\beta} k} + \left( \frac{7}{160} \mathcal{D}^\dagger \bar{\mathcal{H}} - \frac{1}{12} \mathcal{D} \bar{\mathcal{I}} \right) P_b \Lambda_{\alpha j} \Lambda^{\dot{\beta} i} R(Q)_{ac\beta}{}^j \gamma_b{}^\alpha{}_{\dot{\beta}} \gamma_c{}^{\dot{\alpha} \beta} \\
& + \left( \frac{17}{384} \mathcal{D}^\dagger \bar{\mathcal{H}} - \frac{13}{960} \mathcal{D} \bar{\mathcal{I}} \right) \Lambda_{\alpha j} \Lambda^{\dot{\alpha} k} \Lambda^{\dot{\beta} i} R(V)_{bc}{}^j{}_{\dot{k}} \gamma_d{}^\alpha{}_{\dot{\beta}} \varepsilon_{abcd} + \left( \frac{2}{45} \bar{\mathcal{H}} + \frac{17}{240} \mathcal{H} \right) \Lambda_{\alpha j} \Lambda^{\dot{\alpha} j} \bar{P}_b \gamma_c{}^\alpha{}_{\dot{\beta}} \nabla_d \Lambda^{\dot{\beta} i} \varepsilon_{abcd} \\
& + \left( \frac{13}{288} \mathcal{D}^\dagger \bar{\mathcal{H}} - \frac{1}{72} \mathcal{D} \bar{\mathcal{I}} \right) E^{jk} P_a \Lambda_{\alpha j} \Lambda_{\beta k} \Lambda^{\dot{\alpha} i} \epsilon^{\alpha \beta} + \left( \frac{55}{1152} \bar{\mathcal{H}} + \frac{1}{128} \mathcal{H} \right) T_{abjk} \Lambda_{\alpha l} \Lambda_{\beta m} \epsilon^{\alpha \beta} \nabla_b \Lambda^{\dot{\alpha} l} \varepsilon^{ijkm} \\
& + \left( \frac{7}{144} \bar{\mathcal{I}} + \frac{1}{72} \mathcal{D}^\dagger \bar{\mathcal{H}} \right) P_b \Lambda^{\dot{\beta} i} \Lambda^{\dot{\gamma} j} \gamma_a{}^{\dot{\alpha} \alpha} \gamma_{bc\dot{\beta}\dot{\gamma}} \nabla_c \Lambda_{\alpha j} + \left( \frac{7}{144} \mathcal{D}^\dagger \bar{\mathcal{H}} - \frac{53}{192} \mathcal{D} \bar{\mathcal{I}} \right) P_a \Lambda_{\alpha j} \Lambda^{\dot{\alpha} j} \Lambda^{\dot{\beta} i} \bar{P}_b \gamma_b{}^\alpha{}_{\dot{\beta}} \\
& + \left( \frac{1}{20} \mathcal{D}^\dagger \mathcal{I} + \frac{1}{10} \mathcal{D} \mathcal{H} \right) T_{bc}{}^{jk} \Lambda_{\alpha j} \Lambda^{\dot{\beta} i} \gamma_a{}^\alpha{}_{\dot{\beta}} \gamma_b{}^{\dot{\alpha} \beta} \nabla_c \Lambda_{\beta k} + \left( \frac{1}{20} \mathcal{D}^\dagger \mathcal{I} + \frac{5}{48} \mathcal{D} \mathcal{H} \right) T_{ab}{}^{ij} \Lambda_{\alpha k} \Lambda^{\dot{\beta} k} \gamma_c{}^\alpha{}_{\dot{\beta}} \gamma_b{}^{\dot{\alpha} \beta} \nabla_c \Lambda_{\beta j} \\
& + \left( \frac{1}{20} \mathcal{D}^\dagger \mathcal{I} + \frac{5}{48} \mathcal{D} \mathcal{H} \right) T_{bc}{}^{ij} \Lambda_{\alpha k} \Lambda^{\dot{\beta} k} \gamma_b{}^\beta{}_{\dot{\beta}} \gamma_a{}^{\dot{\alpha} \alpha} \nabla_c \Lambda_{\beta j} + \left( \frac{37}{720} \bar{\mathcal{H}} + \frac{1}{40} \mathcal{H} \right) \Lambda_{\alpha j} \Lambda^{\dot{\beta} j} \bar{P}_b \gamma_c{}^\alpha{}_{\dot{\beta}} \nabla_d \Lambda^{\dot{\alpha} i} \varepsilon_{abcd} \\
& + \left( \frac{19}{360} \bar{\mathcal{I}} + \frac{23}{360} \mathcal{D}^\dagger \mathcal{D}^\dagger \bar{\mathcal{H}} \right) T_{bc}{}^{jk} \Lambda^{\dot{\alpha} i} \Lambda^{\dot{\beta} l} \gamma_{ab\dot{\beta}\dot{\gamma}} \nabla_c \Lambda^{\dot{\gamma} m} \varepsilon_{jklm} + \left( \frac{1}{18} \bar{\mathcal{I}} + \frac{1}{36} \mathcal{D}^\dagger \mathcal{D}^\dagger \bar{\mathcal{H}} \right) T_{ab}{}^{jk} \Lambda^{\dot{\beta} i} \Lambda^{\dot{\gamma} l} \gamma_{bc\dot{\beta}\dot{\gamma}} \nabla_c \Lambda^{\dot{\alpha} m} \varepsilon_{jklm} \\
& + \left( \frac{1}{18} \mathcal{D}^\dagger \mathcal{D}^\dagger \bar{\mathcal{I}} + \frac{1}{48} \mathcal{D}^\dagger \mathcal{D}^\dagger \mathcal{D}^\dagger \bar{\mathcal{H}} \right) P_b T_{bcjk} \Lambda^{\dot{\alpha} j} \Lambda^{\dot{\beta} i} \Lambda^{\dot{\gamma} k} \gamma_{ac\dot{\beta}\dot{\gamma}} + \left( \frac{1}{18} \mathcal{D}^\dagger \mathcal{I} + \frac{1}{144} \mathcal{D} \mathcal{H} \right) \Lambda_{\alpha j} \Lambda^{\dot{\alpha} i} \Lambda^{\dot{\beta} j} \bar{P}_a \bar{P}_b \gamma_b{}^\alpha{}_{\dot{\beta}} \\
& + \left( \frac{1}{18} \mathcal{D}^\dagger \mathcal{I} + \frac{1}{18} \mathcal{D} \mathcal{H} \right) \Lambda_{\alpha j} \chi^{\dot{\beta}}{}_{kl}{}^m \gamma_a{}^\alpha{}_{\dot{\beta}} \gamma_b{}^{\dot{\alpha} \beta} \nabla_b \Lambda_{\beta m} \varepsilon^{ijkl} + \left( \frac{17}{288} \bar{\mathcal{H}} - \frac{1}{288} \mathcal{H} \right) \Lambda_{\alpha j} \Lambda^{\dot{\beta} i} \Lambda^{\dot{\gamma} j} \gamma_a{}^{\dot{\alpha} \alpha} \gamma_{bc\dot{\beta}\dot{\gamma}} \nabla_b \bar{P}_c \\
& + \left( \frac{23}{384} \mathcal{D}^\dagger \bar{\mathcal{H}} - \frac{61}{384} \mathcal{D} \bar{\mathcal{I}} \right) \Lambda_{\alpha j} \Lambda^{\dot{\beta} i} \Lambda^{\dot{\gamma} j} R(M)_{abcd} \gamma_b{}^{\dot{\alpha} \alpha} \gamma_{cd\dot{\beta}\dot{\gamma}} + \left( \frac{35}{576} \mathcal{D} \mathcal{D} \mathcal{H} + \frac{53}{72} \mathcal{I} \right) T_{bc}{}^{ij} \Lambda_{\alpha j} \Lambda_{\beta k} \Lambda^{\dot{\alpha} k} \bar{P}_a \gamma_{bc}{}^{\alpha \beta} \\
& + \left( \frac{1}{16} \mathcal{D}^\dagger \bar{\mathcal{H}} + \frac{1}{96} \mathcal{D} \bar{\mathcal{I}} \right) \Lambda_{\alpha j} \Lambda^{\dot{\beta} j} \Lambda^{\dot{\gamma} k} R(V)_{ab}{}^i{}_{\dot{k}} \epsilon_{\dot{\beta} \dot{\gamma}} \gamma_b{}^{\dot{\alpha} \alpha} + \left( \frac{1}{15} \mathcal{D}^\dagger \bar{\mathcal{H}} + \frac{1}{192} \mathcal{D} \bar{\mathcal{I}} \right) P_b \Lambda_{\alpha j} \Lambda^{\dot{\beta} i} R(Q)_{bc\beta}{}^j \gamma_a{}^\beta{}_{\dot{\beta}} \gamma_c{}^{\dot{\alpha} \alpha} \\
& + \left( \frac{97}{1440} \mathcal{D}^\dagger \mathcal{I} + \frac{1}{144} \mathcal{D} \mathcal{H} \right) E^{ij} \Lambda_{\alpha j} \Lambda_{\beta k} R(Q)_{ab\gamma}{}^k \epsilon^{\alpha \gamma} \gamma_b{}^{\dot{\alpha} \beta} + \left( \frac{97}{1440} \mathcal{D}^\dagger \mathcal{I} + \frac{1}{144} \mathcal{D} \mathcal{H} \right) E^{ij} \Lambda_{\alpha j} \Lambda_{\beta k} R(Q)_{ab\gamma}{}^k \epsilon^{\beta \gamma} \gamma_b{}^{\dot{\alpha} \alpha} \\
& + \left( \frac{5}{72} \bar{\mathcal{I}} - \frac{1}{96} \mathcal{D}^\dagger \mathcal{D}^\dagger \bar{\mathcal{H}} \right) E_{jk} \Lambda^{\dot{\beta} i} \Lambda^{\dot{\gamma} j} \epsilon_{\dot{\beta} \dot{\gamma}} \gamma_{ab}{}^{\dot{\alpha}}{}_{\dot{\delta}} \nabla_b \Lambda^{\dot{\delta} k} + \left( \frac{9}{128} \mathcal{D}^\dagger \bar{\mathcal{H}} - \frac{31}{128} \mathcal{D} \bar{\mathcal{I}} \right) T_{bcjk} \Lambda_{\alpha l} \Lambda^{\dot{\beta} i} R(Q)_{ab}{}^{\dot{\alpha}}{}_{\dot{m}} \gamma_c{}^\alpha{}_{\dot{\beta}} \varepsilon^{jklm} \\
& + \left( \frac{7}{96} \bar{\mathcal{H}} - \frac{43}{1440} \mathcal{H} \right) \Lambda_{\alpha j} \Lambda^{\dot{\beta} j} \bar{P}_b \gamma_c{}^{\dot{\alpha} \alpha} \gamma_{ab\dot{\beta}\dot{\gamma}} \nabla_c \Lambda^{\dot{\gamma} i} + \left( \frac{7}{96} \mathcal{D}^\dagger \bar{\mathcal{H}} - \frac{1}{48} \mathcal{D} \bar{\mathcal{I}} \right) T_{ab}{}^{jk} \Lambda^{\dot{\alpha} i} \Lambda^{\dot{\beta} l} \chi_{\alpha}{}^{mn}{}_{\dot{l}} \gamma_b{}^\alpha{}_{\dot{\beta}} \varepsilon_{jkmn} \\
& + \left( \frac{7}{96} \mathcal{D}^\dagger \bar{\mathcal{H}} + \frac{7}{48} \mathcal{D} \bar{\mathcal{I}} \right) T_{abjk} T_{bc}{}^{jk} \Lambda_{\alpha l} \Lambda^{\dot{\alpha} i} \Lambda^{\dot{\beta} l} \gamma_c{}^\alpha{}_{\dot{\beta}} + \left( \frac{7}{96} \mathcal{D}^\dagger \bar{\mathcal{H}} + \frac{7}{48} \mathcal{D} \bar{\mathcal{I}} \right) T_{bcjk} T_{ab}{}^{jk} \Lambda_{\alpha l} \Lambda^{\dot{\alpha} i} \Lambda^{\dot{\beta} l} \gamma_c{}^\alpha{}_{\dot{\beta}} \\
& + \left( \frac{7}{96} \mathcal{D}^\dagger \bar{\mathcal{H}} + \frac{5}{24} \mathcal{D} \bar{\mathcal{I}} \right) T_{abjk} T_{bc}{}^{jl} \Lambda_{\alpha l} \Lambda^{\dot{\alpha} k} \Lambda^{\dot{\beta} i} \gamma_c{}^\alpha{}_{\dot{\beta}} + \left( \frac{7}{96} \mathcal{D}^\dagger \bar{\mathcal{H}} + \frac{5}{24} \mathcal{D} \bar{\mathcal{I}} \right) T_{bcjk} T_{ab}{}^{jl} \Lambda_{\alpha l} \Lambda^{\dot{\alpha} k} \Lambda^{\dot{\beta} i} \gamma_c{}^\alpha{}_{\dot{\beta}} \\
& + \left( \frac{107}{1440} \mathcal{D}^\dagger \mathcal{I} + \frac{7}{80} \mathcal{D} \mathcal{H} \right) \Lambda_{\alpha j} \Lambda_{\beta k} \Lambda^{\dot{\beta} j} \gamma_{bc}{}^{\alpha \beta} \gamma_{ad}{}^{\dot{\alpha}}{}_{\dot{\beta}} \nabla_d T_{bc}{}^{ik} + \left( \frac{11}{144} \mathcal{D}^\dagger \bar{\mathcal{H}} + \frac{5}{144} \mathcal{D} \bar{\mathcal{I}} \right) E_{jk} \Lambda^{\dot{\alpha} j} \Lambda^{\dot{\beta} i} \Lambda^{\dot{\gamma} k} \bar{P}_a \gamma_{bc\dot{\gamma}}{}^{\dot{\alpha} \beta} \\
& + \left( \frac{7}{90} \mathcal{D}^\dagger \bar{\mathcal{H}} + \frac{29}{576} \mathcal{D} \bar{\mathcal{I}} \right) E^{ij} P_a \Lambda_{\alpha j} \Lambda_{\beta k} \Lambda^{\dot{\alpha} k} \epsilon^{\alpha \beta} + \left( \frac{61}{768} \bar{\mathcal{H}} - \frac{175}{2304} \mathcal{H} \right) \Lambda_{\alpha j} \Lambda^{\dot{\beta} i} \Lambda^{\dot{\gamma} j} \gamma_b{}^{\dot{\alpha} \alpha} \gamma_{ac\dot{\beta}\dot{\gamma}} \nabla_c \bar{P}_b \\
& + \left( \frac{23}{288} \mathcal{D}^\dagger \mathcal{I} - \frac{1}{72} \mathcal{D} \mathcal{H} \right) \Lambda_{\alpha j} \Lambda_{\beta k} \gamma_b{}^\alpha{}_{\dot{\beta}} \gamma_a{}^{\dot{\alpha} \beta} \nabla_b \chi^{\dot{\beta}}{}_{lm}{}^k \varepsilon^{ijlm} + \left( \frac{1}{12} \bar{\mathcal{I}} - \frac{1}{96} \mathcal{D}^\dagger \mathcal{D}^\dagger \bar{\mathcal{H}} \right) E^{ij} \Lambda^{\dot{\alpha} k} \Lambda^{\dot{\beta} l} \chi_{\alpha}{}^{mn}{}_{\dot{l}} \gamma_a{}^\alpha{}_{\dot{\beta}} \varepsilon_{jlmn} \\
& + \left( \frac{1}{12} \mathcal{D}^\dagger \bar{\mathcal{H}} - \frac{5}{24} \mathcal{D} \bar{\mathcal{I}} \right) T_{abjk} \Lambda_{\alpha l} \Lambda^{\dot{\beta} m} \chi^{\dot{\alpha}}{}_{mn}{}^l \gamma_b{}^\alpha{}_{\dot{\beta}} \varepsilon^{ijkn} + \left( \frac{1}{12} \mathcal{D}^\dagger \bar{\mathcal{H}} + \frac{1}{6} \mathcal{D} \bar{\mathcal{I}} \right) T_{abjk} T_{bc}{}^{il} \Lambda_{\alpha l} \Lambda^{\dot{\alpha} j} \Lambda^{\dot{\beta} k} \gamma_c{}^\alpha{}_{\dot{\beta}} \\
& + \left( \frac{1}{12} \mathcal{D}^\dagger \bar{\mathcal{H}} + \frac{1}{6} \mathcal{D} \bar{\mathcal{I}} \right) T_{bcjk} T_{ab}{}^{il} \Lambda_{\alpha l} \Lambda^{\dot{\alpha} j} \Lambda^{\dot{\beta} k} \gamma_c{}^\alpha{}_{\dot{\beta}} + \left( \frac{13}{144} \mathcal{D}^\dagger \bar{\mathcal{H}} - \frac{25}{64} \mathcal{D} \bar{\mathcal{I}} \right) P_b \Lambda_{\alpha j} \Lambda^{\dot{\alpha} j} \Lambda^{\dot{\beta} i} \bar{P}_a \gamma_b{}^\alpha{}_{\dot{\beta}} \\
& + \left( \frac{11}{120} \mathcal{D}^\dagger \bar{\mathcal{H}} + \frac{13}{96} \mathcal{D} \bar{\mathcal{I}} \right) P_b \Lambda_{\alpha j} \Lambda^{\dot{\beta} j} R(Q)_{bc\beta}{}^i \gamma_a{}^\alpha{}_{\dot{\beta}} \gamma_c{}^{\dot{\alpha} \beta} + \left( \frac{3}{32} \mathcal{D} \mathcal{D} \mathcal{H} - \frac{5}{12} \mathcal{I} \right) T_{bc}{}^{jk} \Lambda_{\alpha j} \Lambda_{\beta k} R(Q)_{bc\gamma}{}^i \epsilon^{\alpha \gamma} \gamma_a{}^{\dot{\alpha} \beta} \\
& + \left( \frac{23}{240} \mathcal{D}^\dagger \mathcal{I} + \frac{3}{40} \mathcal{D} \mathcal{H} \right) E^{jk} \Lambda_{\alpha j} \Lambda_{\beta l} \chi_{\gamma}{}^{il}{}_{\dot{k}} \epsilon^{\alpha \beta} \gamma_a{}^{\dot{\alpha} \gamma} + \left( \frac{7}{72} \bar{\mathcal{H}} - \frac{7}{72} \mathcal{H} \right) P_b T_{ac}{}^{ij} \Lambda_{\alpha j} \Lambda_{\beta k} \Lambda^{\dot{\alpha} k} \gamma_{bc}{}^{\alpha \beta} \\
& + \left( \frac{7}{72} \mathcal{D}^\dagger \mathcal{I} + \frac{1}{72} \mathcal{D} \mathcal{H} \right) \Lambda_{\alpha j} \Lambda_{\beta k} \gamma_b{}^\alpha{}_{\dot{\beta}} \gamma_a{}^{\dot{\alpha} \beta} \nabla_b \chi^{\dot{\beta}}{}_{lm}{}^j \varepsilon^{iklm} + \left( \frac{1}{10} \mathcal{D}^\dagger \bar{\mathcal{H}} + \frac{1}{48} \mathcal{D} \bar{\mathcal{I}} \right) P_b \Lambda_{\alpha j} \Lambda^{\dot{\beta} j} R(Q)_{ac\beta}{}^i \gamma_b{}^\beta{}_{\dot{\beta}} \gamma_c{}^{\dot{\alpha} \alpha} \\
& + \left( \frac{29}{288} \bar{\mathcal{H}} + \frac{73}{1440} \mathcal{H} \right) \Lambda_{\alpha j} \Lambda^{\dot{\beta} j} \bar{P}_b \gamma_b{}^{\dot{\alpha} \alpha} \gamma_{ac\dot{\beta}\dot{\gamma}} \nabla_c \Lambda^{\dot{\gamma} i} + \left( \frac{49}{480} \mathcal{D}^\dagger \bar{\mathcal{I}} + \frac{7}{1920} \mathcal{D}^\dagger \mathcal{D}^\dagger \bar{\mathcal{H}} \right) T_{bcjk} \Lambda^{\dot{\beta} j} \Lambda^{\dot{\gamma} k} \gamma_{bc\dot{\beta}\dot{\gamma}} \gamma_{ad}{}^{\dot{\alpha}}{}_{\dot{\gamma}} \nabla_d \Lambda^{\dot{\delta} i} \\
& + \left( \frac{33}{320} \mathcal{D}^\dagger \bar{\mathcal{H}} + \frac{163}{5760} \mathcal{D} \bar{\mathcal{I}} \right) T_{bcjk} \Lambda_{\alpha l} \Lambda^{\dot{\alpha} m} R(Q)_{bc}{}^{\dot{\beta}}{}_{\dot{m}} \gamma_a{}^\alpha{}_{\dot{\beta}} \varepsilon^{ijkl} + \left( \frac{5}{48} \mathcal{D}^\dagger \mathcal{I} + \frac{1}{6} \mathcal{D} \mathcal{H} \right) \Lambda_{\alpha j} \Lambda_{\beta k} R(S)_{ab\gamma l}{}^{\dot{\alpha} \gamma} \gamma_b{}^{\dot{\alpha} \beta} \varepsilon^{ijkl} \\
& + \left( \frac{13}{120} \bar{\mathcal{I}} - \frac{1}{80} \mathcal{D}^\dagger \mathcal{D}^\dagger \bar{\mathcal{H}} \right) T_{bc}{}^{jk} \Lambda^{\dot{\alpha} l} \Lambda^{\dot{\beta} m} \gamma_{ab\dot{\beta}\dot{\gamma}} \nabla_c \Lambda^{\dot{\gamma} i} \varepsilon_{jklm} + \left( \frac{13}{120} \bar{\mathcal{I}} + \frac{29}{480} \mathcal{D}^\dagger \mathcal{D}^\dagger \bar{\mathcal{H}} \right) T_{ab}{}^{jk} \Lambda^{\dot{\alpha} l} \Lambda^{\dot{\beta} i} \epsilon_{\dot{\beta} \dot{\gamma}} \nabla_b \Lambda^{\dot{\gamma} m} \varepsilon_{jklm} \\
& + \left( \frac{1}{9} \bar{\mathcal{I}} - \frac{1}{48} \mathcal{D}^\dagger \mathcal{D}^\dagger \bar{\mathcal{H}} \right) \Lambda^{\dot{\alpha} j} \Lambda^{\dot{\beta} k} \Lambda^{\dot{\gamma} l} \gamma_{ab\dot{\beta}\dot{\gamma}} \nabla_c T_{bc}{}^{im} \varepsilon_{jklm} + \left( \frac{17}{144} \mathcal{D}^\dagger \mathcal{I} - \frac{7}{48} \mathcal{D} \mathcal{H} \right) T_{bc}{}^{ij} \Lambda_{\alpha j} \Lambda^{\dot{\beta} k} \gamma_b{}^\beta{}_{\dot{\beta}} \gamma_a{}^{\dot{\alpha} \alpha} \nabla_c \Lambda_{\beta k} + 10 \dots
\end{aligned}$$

$$\begin{aligned}
[\hat{\Omega}_a^{\dot{\alpha}i}]_{3,cont.} = & + \left( \frac{1}{8} \bar{\mathcal{I}} - \frac{1}{64} \mathcal{D}^\dagger \mathcal{D}^\dagger \bar{\mathcal{H}} \right) T_{bcjk} \Lambda^{\dot{\beta}i} \Lambda^{\dot{\gamma}l} \chi_\alpha^{\dot{\gamma}k} \gamma_a^{\dot{\alpha}\alpha} \gamma_{bc\dot{\beta}\dot{\gamma}} + \left( \frac{1}{8} \mathcal{D}^\dagger \bar{\mathcal{H}} + \frac{3}{16} \mathcal{D} \bar{\mathcal{I}} \right) T_{abjk} T_{bc}{}^{ij} \Lambda_{\alpha l} \Lambda^{\dot{\alpha}k} \Lambda^{\dot{\beta}l} \gamma_c{}^\alpha{}_{\dot{\beta}} \\
& + \left( \frac{1}{8} \mathcal{D}^\dagger \bar{\mathcal{H}} + \frac{3}{16} \mathcal{D} \bar{\mathcal{I}} \right) T_{bcjk} T_{ab}{}^{ij} \Lambda_{\alpha l} \Lambda^{\dot{\alpha}k} \Lambda^{\dot{\beta}l} \gamma_c{}^\alpha{}_{\dot{\beta}} + \left( \frac{1}{8} \mathcal{D}^\dagger \mathcal{I} - \frac{1}{12} \mathcal{D} \mathcal{H} \right) \Lambda_{\alpha j} \Lambda^{\dot{\beta}k} \bar{P}_b \chi_\beta^{\dot{\gamma}j} \gamma_a{}^\beta{}_{\dot{\beta}} \gamma_b{}^{\dot{\alpha}\alpha} \\
& + \left( \frac{1}{8} \mathcal{D} \mathcal{D} \mathcal{H} + \frac{1}{4} \mathcal{I} \right) T_{bc}{}^{jk} \Lambda_{\alpha j} \Lambda_{\beta l} \chi_\gamma^{\dot{\gamma}l} \gamma_a{}^{\dot{\alpha}\gamma} \gamma_{bc}{}^{\alpha\beta} + \left( \frac{37}{288} \mathcal{D}^\dagger \mathcal{I} - \frac{1}{720} \mathcal{D} \mathcal{H} \right) T_{ab}{}^{ij} \Lambda_{\alpha j} \Lambda_{\beta k} \epsilon^{\alpha\beta} \gamma_{bc}{}^{\dot{\alpha}}{}_{\dot{\beta}} \nabla_c \Lambda^{\dot{\beta}k} \\
& + \left( \frac{19}{144} \mathcal{D}^\dagger \mathcal{I} + \frac{5}{72} \mathcal{D} \mathcal{H} \right) \Lambda_{\alpha j} \Lambda^{\dot{\beta}i} R(Q)_{ab\beta}{}^j \bar{P}_c \gamma_c{}^\beta{}_{\dot{\beta}} \gamma_b{}^{\dot{\alpha}\alpha} + \left( \frac{2}{15} \mathcal{D}^\dagger \mathcal{I} + \frac{1}{60} \mathcal{D} \mathcal{H} \right) T_{ab}{}^{jk} \Lambda_{\alpha j} \Lambda^{\dot{\beta}i} \gamma_b{}^\beta{}_{\dot{\beta}} \gamma_c{}^{\dot{\alpha}\alpha} \nabla_c \Lambda_{\beta k} \\
& + \left( \frac{17}{120} \mathcal{D}^\dagger \bar{\mathcal{I}} - \frac{1}{1920} \mathcal{D}^\dagger \mathcal{D}^\dagger \mathcal{D}^\dagger \bar{\mathcal{H}} \right) T_{bcjk} \Lambda^{\dot{\beta}i} \Lambda^{\dot{\gamma}j} \gamma_{bc\dot{\beta}\dot{\delta}} \gamma_{ad}{}^{\dot{\alpha}}{}_{\dot{\gamma}} \nabla_d \Lambda^{\dot{\delta}k} + \left( \frac{17}{120} \mathcal{D}^\dagger \bar{\mathcal{I}} - \frac{1}{1920} \mathcal{D}^\dagger \mathcal{D}^\dagger \mathcal{D}^\dagger \bar{\mathcal{H}} \right) T_{bcjk} \Lambda^{\dot{\beta}i} \Lambda^{\dot{\gamma}j} \gamma_{bc\dot{\gamma}\dot{\delta}} \gamma_{ad}{}^{\dot{\alpha}}{}_{\dot{\beta}} \nabla_d \Lambda^{\dot{\delta}k} \\
& + \left( \frac{7}{48} \mathcal{D}^\dagger \mathcal{I} - \frac{1}{24} \mathcal{D} \mathcal{H} \right) \Lambda_{\alpha j} \Lambda^{\dot{\beta}i} R(Q)_{bc\beta}{}^j \bar{P}_b \gamma_a{}^\beta{}_{\dot{\beta}} \gamma_c{}^{\dot{\alpha}\alpha} + \left( \frac{223}{1440} \bar{\mathcal{I}} - \frac{209}{2880} \mathcal{D}^\dagger \mathcal{D}^\dagger \bar{\mathcal{H}} \right) P_b \Lambda_{\alpha j} \Lambda^{\dot{\beta}i} \gamma_c{}^\alpha{}_{\dot{\beta}} \nabla_d \Lambda^{\dot{\alpha}j} \epsilon_{abcd} \\
& + \left( \frac{19}{120} \mathcal{D}^\dagger \mathcal{I} + \frac{7}{48} \mathcal{D} \mathcal{H} \right) T_{bc}{}^{jk} \Lambda_{\alpha j} \Lambda^{\dot{\beta}i} \gamma_b{}^\beta{}_{\dot{\beta}} \gamma_a{}^{\dot{\alpha}\alpha} \nabla_c \Lambda_{\beta k} + \left( \frac{23}{144} \mathcal{D}^\dagger \mathcal{I} - \frac{7}{36} \mathcal{D} \mathcal{H} \right) \Lambda_{\alpha j} \Lambda^{\dot{\beta}j} R(Q)_{ab\beta}{}^i \bar{P}_c \gamma_c{}^\beta{}_{\dot{\beta}} \gamma_b{}^{\dot{\alpha}\alpha} \\
& + \left( \frac{473}{2880} \bar{\mathcal{H}} - \frac{19}{640} \mathcal{H} \right) \Lambda_{\alpha j} \Lambda^{\dot{\beta}i} \bar{P}_b \gamma_c{}^\alpha{}_{\dot{\beta}} \nabla_d \Lambda^{\dot{\alpha}j} \epsilon_{abcd} + \left( \frac{1}{6} \bar{\mathcal{I}} + \frac{1}{16} \mathcal{D}^\dagger \mathcal{D}^\dagger \bar{\mathcal{H}} \right) \Lambda^{\dot{\alpha}j} \Lambda^{\dot{\beta}i} \Lambda^{\dot{\gamma}k} \epsilon_{\dot{\beta}\dot{\gamma}} \nabla_b T_{ab}{}^{lm} \epsilon_{ijklm} \\
& + \left( \frac{1}{6} \mathcal{D}^\dagger \bar{\mathcal{H}} - \frac{1}{4} \mathcal{D} \bar{\mathcal{I}} \right) P_b \Lambda_{\alpha j} \Lambda^{\dot{\beta}k} \chi_\beta^{\dot{\gamma}j} \gamma_b{}^{\dot{\alpha}\beta} \gamma_a{}^{\dot{\alpha}\beta} + \left( \frac{49}{288} \bar{\mathcal{H}} - \frac{79}{1440} \mathcal{H} \right) T_{bcjk} \Lambda_{\alpha l} \Lambda_{\beta m} \gamma_{ab}{}^{\alpha\beta} \nabla_c \Lambda^{\dot{\alpha}l} \epsilon^{ijkm} \\
& + \left( \frac{13}{72} \mathcal{D}^\dagger \mathcal{I} - \frac{1}{288} \mathcal{D} \mathcal{H} \right) \Lambda_{\alpha j} \Lambda^{\dot{\alpha}j} \Lambda^{\dot{\beta}i} \bar{P}_b \bar{P}_b \gamma_a{}^\alpha{}_{\dot{\beta}} + \left( \frac{11}{60} \mathcal{D}^\dagger \mathcal{I} - \frac{2}{15} \mathcal{D} \mathcal{H} \right) T_{ab}{}^{ij} \Lambda_{\alpha k} \Lambda^{\dot{\beta}k} \gamma_b{}^\beta{}_{\dot{\beta}} \gamma_c{}^{\dot{\alpha}\alpha} \nabla_c \Lambda_{\beta j} \\
& + \left( \frac{5}{27} \bar{\mathcal{I}} - \frac{5}{108} \mathcal{D}^\dagger \mathcal{D}^\dagger \bar{\mathcal{H}} \right) T_{abjk} \Lambda^{\dot{\alpha}j} \Lambda^{\dot{\beta}i} \Lambda^{\dot{\gamma}k} \bar{P}_c \gamma_{bc\dot{\beta}\dot{\gamma}} + \left( \frac{5}{27} \bar{\mathcal{I}} - \frac{5}{108} \mathcal{D}^\dagger \mathcal{D}^\dagger \bar{\mathcal{H}} \right) T_{bcjk} \Lambda^{\dot{\alpha}j} \Lambda^{\dot{\beta}i} \Lambda^{\dot{\gamma}k} \bar{P}_b \gamma_{ac\dot{\beta}\dot{\gamma}} \\
& + \left( \frac{13}{60} \bar{\mathcal{I}} + \frac{1}{60} \mathcal{D}^\dagger \mathcal{D}^\dagger \bar{\mathcal{H}} \right) T_{bc}{}^{ij} \Lambda^{\dot{\alpha}k} \Lambda^{\dot{\beta}l} \gamma_{ab\dot{\beta}\dot{\gamma}} \nabla_c \Lambda^{\dot{\gamma}m} \epsilon_{ijklm} + \left( \frac{79}{360} \bar{\mathcal{I}} + \frac{1}{288} \mathcal{D}^\dagger \mathcal{D}^\dagger \bar{\mathcal{H}} \right) P_b \Lambda_{\alpha j} \Lambda^{\dot{\beta}i} \gamma_c{}^\alpha{}_{\dot{\beta}} \nabla_d \Lambda^{\dot{\beta}i} \epsilon_{abcd} \\
& + \left( \frac{2}{9} \mathcal{D}^\dagger \bar{\mathcal{I}} + \frac{1}{72} \mathcal{D}^\dagger \mathcal{D}^\dagger \mathcal{D}^\dagger \bar{\mathcal{H}} \right) \Lambda^{\dot{\beta}i} \Lambda^{\dot{\gamma}j} \Lambda^{\dot{\delta}k} \epsilon_{\dot{\beta}\dot{\gamma}} \gamma_{ab}{}^{\dot{\alpha}}{}_{\dot{\delta}} \nabla_c T_{bcjk} + \left( \frac{2}{9} \mathcal{D}^\dagger \bar{\mathcal{I}} + \frac{1}{72} \mathcal{D}^\dagger \mathcal{D}^\dagger \mathcal{D}^\dagger \bar{\mathcal{H}} \right) \Lambda^{\dot{\beta}i} \Lambda^{\dot{\gamma}j} \Lambda^{\dot{\delta}k} \epsilon_{\dot{\beta}\dot{\gamma}} \gamma_{bc}{}^{\dot{\alpha}}{}_{\dot{\delta}} \nabla_b T_{acjk} \\
& + \left( \frac{17}{72} \bar{\mathcal{I}} + \frac{11}{576} \mathcal{D}^\dagger \mathcal{D}^\dagger \bar{\mathcal{H}} \right) P_b \Lambda^{\dot{\beta}i} \Lambda^{\dot{\gamma}j} \gamma_c{}^{\dot{\alpha}\alpha} \gamma_{ab\dot{\beta}\dot{\gamma}} \nabla_c \Lambda_{\alpha j} + \left( \frac{25}{96} \bar{\mathcal{I}} + \frac{5}{192} \mathcal{D}^\dagger \mathcal{D}^\dagger \bar{\mathcal{H}} \right) P_a \Lambda^{\dot{\beta}i} \Lambda^{\dot{\gamma}j} \epsilon_{\dot{\beta}\dot{\gamma}} \gamma_b{}^{\dot{\alpha}\alpha} \nabla_b \Lambda_{\alpha j} \\
& + \left( \frac{97}{360} \bar{\mathcal{H}} - \frac{53}{180} \mathcal{H} \right) P_a T_{bc}{}^{ij} \Lambda_{\alpha j} \Lambda_{\beta k} \Lambda^{\dot{\alpha}k} \gamma_{bc}{}^{\alpha\beta} + \left( \frac{13}{48} \bar{\mathcal{I}} + \frac{41}{576} \mathcal{D}^\dagger \mathcal{D}^\dagger \bar{\mathcal{H}} \right) P_b \Lambda_{\alpha j} \Lambda^{\dot{\beta}i} \gamma_b{}^{\dot{\alpha}\alpha} \gamma_{ac\dot{\beta}\dot{\gamma}} \nabla_c \Lambda^{\dot{\gamma}j} \\
& + \left( \frac{49}{180} \mathcal{D}^\dagger \mathcal{I} + \frac{31}{240} \mathcal{D} \mathcal{H} \right) \Lambda_{\alpha j} \Lambda_{\beta k} \Lambda^{\dot{\beta}i} \gamma_b{}^\alpha{}_{\dot{\beta}} \gamma_a{}^{\dot{\alpha}\beta} \nabla_c T_{bc}{}^{jk} + \left( \frac{17}{60} \mathcal{D}^\dagger \mathcal{I} - \frac{1}{10} \mathcal{D} \mathcal{H} \right) T_{ab}{}^{ij} \Lambda_{\alpha j} \Lambda^{\dot{\beta}k} \gamma_b{}^\alpha{}_{\dot{\beta}} \gamma_c{}^{\dot{\alpha}\beta} \nabla_c \Lambda_{\beta k} \\
& + \left( \frac{5}{16} \bar{\mathcal{I}} + \frac{1}{12} \mathcal{D}^\dagger \mathcal{D}^\dagger \bar{\mathcal{H}} \right) P_b \Lambda_{\alpha j} \Lambda^{\dot{\beta}i} \gamma_c{}^{\dot{\alpha}\alpha} \gamma_{ab\dot{\beta}\dot{\gamma}} \nabla_c \Lambda^{\dot{\gamma}j} + \left( \frac{113}{360} \mathcal{D}^\dagger \mathcal{I} - \frac{1}{15} \mathcal{D} \mathcal{H} \right) T_{ab}{}^{ij} \Lambda_{\alpha j} \Lambda^{\dot{\beta}k} \gamma_b{}^\beta{}_{\dot{\beta}} \gamma_c{}^{\dot{\alpha}\alpha} \nabla_c \Lambda_{\beta k} \\
& + \left( \frac{31}{96} \mathcal{D}^\dagger \mathcal{I} - \frac{1}{12} \mathcal{D} \mathcal{H} \right) \Lambda_{\alpha j} \Lambda^{\dot{\beta}j} R(Q)_{bc\beta}{}^i \bar{P}_b \gamma_a{}^\alpha{}_{\dot{\beta}} \gamma_c{}^{\dot{\alpha}\beta} + \left( \frac{7}{18} \bar{\mathcal{I}} - \frac{1}{72} \mathcal{D}^\dagger \mathcal{D}^\dagger \bar{\mathcal{H}} \right) T_{bcjk} \Lambda^{\dot{\alpha}j} \Lambda^{\dot{\beta}i} \Lambda^{\dot{\gamma}k} \bar{P}_a \gamma_{bc\dot{\beta}\dot{\gamma}} \\
& + \left( \frac{19}{48} \mathcal{D}^\dagger \mathcal{I} - \frac{1}{12} \mathcal{D} \mathcal{H} \right) \Lambda_{\alpha j} \Lambda_{\beta k} \Lambda^{\dot{\beta}j} \gamma_b{}^\alpha{}_{\dot{\beta}} \gamma_c{}^{\dot{\alpha}\beta} \nabla_c T_{ab}{}^{ik} + \left( \frac{19}{48} \mathcal{D}^\dagger \mathcal{I} - \frac{1}{12} \mathcal{D} \mathcal{H} \right) \Lambda_{\alpha j} \Lambda_{\beta k} \Lambda^{\dot{\beta}j} \gamma_b{}^\beta{}_{\dot{\beta}} \gamma_c{}^{\dot{\alpha}\alpha} \nabla_c T_{ab}{}^{ik} \\
& + \left( \frac{19}{45} \mathcal{D}^\dagger \mathcal{I} - \frac{1}{10} \mathcal{D} \mathcal{H} \right) T_{bc}{}^{ij} \Lambda_{\alpha j} \Lambda^{\dot{\beta}k} \gamma_a{}^\beta{}_{\dot{\beta}} \gamma_b{}^{\dot{\alpha}\alpha} \nabla_c \Lambda_{\beta k} + \left( \frac{43}{96} \bar{\mathcal{I}} + \frac{1}{80} \mathcal{D}^\dagger \mathcal{D}^\dagger \bar{\mathcal{H}} \right) \Lambda_{\alpha j} \Lambda^{\dot{\beta}i} \Lambda^{\dot{\gamma}j} \epsilon_{\dot{\beta}\dot{\gamma}} \gamma_b{}^{\dot{\alpha}\alpha} \nabla_a P_b \\
& + \left( \frac{9}{20} \mathcal{D}^\dagger \mathcal{I} - \frac{1}{10} \mathcal{D} \mathcal{H} \right) T_{ab}{}^{jk} \Lambda_{\alpha j} \Lambda^{\dot{\beta}i} \gamma_b{}^\alpha{}_{\dot{\beta}} \gamma_c{}^{\dot{\alpha}\beta} \nabla_c \Lambda_{\beta k} + \left( \frac{367}{720} \mathcal{D}^\dagger \mathcal{I} - \frac{61}{240} \mathcal{D} \mathcal{H} \right) T_{ab}{}^{ij} \Lambda_{\alpha k} \Lambda^{\dot{\beta}k} \gamma_c{}^\beta{}_{\dot{\beta}} \gamma_b{}^{\dot{\alpha}\alpha} \nabla_c \Lambda_{\beta j} \\
& + \left( \frac{13}{24} \mathcal{D}^\dagger \mathcal{I} + \frac{1}{3} \mathcal{D} \mathcal{H} \right) \Lambda_{\alpha j} \Lambda_{\beta k} \Lambda^{\dot{\beta}j} \gamma_a{}^\alpha{}_{\dot{\beta}} \gamma_b{}^{\dot{\alpha}\beta} \nabla_c T_{bc}{}^{ik} + \left( \frac{13}{24} \mathcal{D}^\dagger \mathcal{I} + \frac{1}{3} \mathcal{D} \mathcal{H} \right) \Lambda_{\alpha j} \Lambda_{\beta k} \Lambda^{\dot{\beta}j} \gamma_a{}^\beta{}_{\dot{\beta}} \gamma_b{}^{\dot{\alpha}\alpha} \nabla_c T_{bc}{}^{ik} \\
& + \left( \frac{17}{30} \mathcal{D}^\dagger \mathcal{I} - \frac{1}{30} \mathcal{D} \mathcal{H} \right) T_{bc}{}^{ij} \Lambda_{\alpha k} \Lambda^{\dot{\beta}k} \gamma_a{}^\beta{}_{\dot{\beta}} \gamma_b{}^{\dot{\alpha}\alpha} \nabla_c \Lambda_{\beta j} + \left( \frac{7}{12} \mathcal{D}^\dagger \bar{\mathcal{I}} + \frac{19}{576} \mathcal{D}^\dagger \mathcal{D}^\dagger \mathcal{D}^\dagger \bar{\mathcal{H}} \right) P_b P_b \Lambda_{\alpha j} \Lambda^{\dot{\alpha}j} \Lambda^{\dot{\beta}i} \gamma_a{}^\alpha{}_{\dot{\beta}} \\
& + \left( \frac{121}{144} \bar{\mathcal{I}} + \frac{41}{576} \mathcal{D}^\dagger \mathcal{D}^\dagger \bar{\mathcal{H}} \right) \Lambda_{\alpha j} \Lambda^{\dot{\beta}i} \Lambda^{\dot{\gamma}j} \gamma_b{}^{\dot{\alpha}\alpha} \gamma_{ac\dot{\beta}\dot{\gamma}} \nabla_b P_c + \left( \frac{43}{36} \mathcal{D}^\dagger \bar{\mathcal{I}} + \frac{23}{288} \mathcal{D}^\dagger \mathcal{D}^\dagger \mathcal{D}^\dagger \bar{\mathcal{H}} \right) P_a P_b \Lambda_{\alpha j} \Lambda^{\dot{\alpha}i} \Lambda^{\dot{\beta}j} \gamma_b{}^\alpha{}_{\dot{\beta}} \\
& + \left( \frac{56}{27} \bar{\mathcal{I}} - \frac{2}{9} \mathcal{D}^\dagger \mathcal{D}^\dagger \bar{\mathcal{H}} \right) T_{abjk} \Lambda^{\dot{\alpha}j} \Lambda^{\dot{\beta}i} \Lambda^{\dot{\gamma}k} \bar{P}_b \epsilon_{\dot{\beta}\dot{\gamma}} - \frac{1}{576} E_{jk} \mathcal{D}^\dagger \mathcal{I} \Lambda_{\alpha l} \Lambda_{\beta m} \gamma_a{}^\alpha{}_{\dot{\beta}} \gamma_b{}^{\dot{\alpha}\beta} \nabla_b \Lambda^{\dot{\beta}j} \epsilon^{iklm} \\
& - \frac{5}{1152} E_{jk} \mathcal{D}^\dagger \mathcal{I} \Lambda_{\alpha l} \Lambda^{\dot{\beta}j} \epsilon^{\alpha\beta} \gamma_{ab}{}^{\dot{\alpha}}{}_{\dot{\beta}} \nabla_b \Lambda_{\beta m} \epsilon^{iklm} - \frac{1}{96} E^{ij} E^{kl} \mathcal{D}^\dagger \mathcal{D}^\dagger \bar{\mathcal{H}} \Lambda_{\alpha k} \Lambda^{\dot{\alpha}m} \Lambda^{\dot{\beta}n} \gamma_a{}^\alpha{}_{\dot{\beta}} \epsilon^{ijlmn} \\
& - \frac{1}{36} P_b \mathcal{D}^\dagger \mathcal{I} \Lambda_{\alpha j} \Lambda_{\beta k} \gamma_b{}^{\dot{\alpha}\alpha} \gamma_{ac}{}^{\beta\gamma} \nabla_c \Lambda_{\gamma l} \epsilon^{ijkl} - \frac{1}{96} P_b \mathcal{D}^\dagger \mathcal{I} \Lambda_{\alpha j} \Lambda_{\beta k} \gamma_b{}^{\dot{\alpha}\gamma} \gamma_{ac}{}^{\alpha\beta} \nabla_c \Lambda_{\gamma l} \epsilon^{ijkl} + \frac{1}{24} \Lambda_{\alpha j} \Lambda_{\beta k} \Lambda^{\dot{\beta}i} \bar{\mathcal{H}} \gamma_b{}^\alpha{}_{\dot{\beta}} \gamma_c{}^{\dot{\alpha}\beta} \nabla_b T_{aclm} \epsilon^{jklm} \\
& - \frac{1}{40} \Lambda_{\alpha j} \Lambda_{\beta k} \Lambda^{\dot{\beta}j} \bar{\mathcal{H}} \gamma_b{}^\alpha{}_{\dot{\beta}} \gamma_c{}^{\dot{\alpha}\beta} \nabla_b T_{aclm} \epsilon^{iklm} - \frac{1}{40} \Lambda_{\alpha j} \Lambda_{\beta k} \Lambda^{\dot{\beta}j} \bar{\mathcal{H}} \gamma_b{}^\beta{}_{\dot{\beta}} \gamma_c{}^{\dot{\alpha}\alpha} \nabla_b T_{aclm} \epsilon^{iklm} + \frac{1}{20} \Lambda_{\alpha j} \Lambda_{\beta k} \Lambda^{\dot{\beta}l} \bar{\mathcal{H}} \gamma_b{}^\alpha{}_{\dot{\beta}} \gamma_c{}^{\dot{\alpha}\beta} \nabla_b T_{aclm} \epsilon^{ijkm} \\
& - \frac{1}{9} \mathcal{D}^\dagger \mathcal{D}^\dagger \bar{\mathcal{I}} P_a T_{bcjk} \Lambda^{\dot{\beta}i} \Lambda^{\dot{\gamma}j} \Lambda^{\dot{\delta}k} \epsilon_{\dot{\beta}\dot{\gamma}} \gamma_{bc}{}^{\dot{\alpha}}{}_{\dot{\delta}} + \frac{1}{96} \mathcal{D}^\dagger \mathcal{D}^\dagger \bar{\mathcal{H}} E^{ij} \Lambda^{\dot{\alpha}k} \Lambda^{\dot{\beta}l} \Lambda^{\dot{\gamma}m} \bar{P}_b \gamma_{ab\dot{\beta}\dot{\gamma}} \epsilon_{jklm} + 11 \dots
\end{aligned}$$

$$\begin{aligned}
[\hat{\Omega}_a^{\dot{\alpha}i}]_{3,cont.} = & + \frac{1}{12} \mathcal{D}^\dagger \mathcal{D}^\dagger \mathcal{D}^\dagger \bar{\mathcal{H}} P_b T_{ab}{}^{jk} \Lambda^{\dot{\alpha}l} \Lambda^{\dot{\beta}i} \Lambda^{\dot{\gamma}m} \epsilon_{\dot{\beta}\dot{\gamma}} \epsilon_{jklm} - \frac{1}{384} \mathcal{D}^\dagger \mathcal{D}^\dagger \mathcal{D}^\dagger \bar{\mathcal{H}} E^{ij} P_b \Lambda^{\dot{\alpha}k} \Lambda^{\dot{\beta}l} \Lambda^{\dot{\gamma}m} \gamma_{ab\dot{\beta}\dot{\gamma}} \epsilon_{ijklm} \\
& + \frac{5}{288} \mathcal{D}^\dagger \mathcal{I} E^{ij} \Lambda_{\alpha j} \Lambda_{\beta k} \Lambda^{\dot{\beta}k} \bar{P}_b \gamma_a{}^\alpha{}_{\dot{\beta}} \gamma_b{}^{\dot{\alpha}\beta} + \frac{5}{288} \mathcal{D}^\dagger \mathcal{I} E^{ij} \Lambda_{\alpha j} \Lambda_{\beta k} \Lambda^{\dot{\beta}k} \bar{P}_b \gamma_a{}^\beta{}_{\dot{\beta}} \gamma_b{}^{\dot{\alpha}\alpha} - \frac{1}{24} \mathcal{D}^\dagger \mathcal{I} T_{abjk} \Lambda_{\alpha l} \Lambda_{\beta m} \chi_\gamma{}^{lm}{}_n \epsilon^{\alpha\gamma} \gamma_b{}^{\dot{\alpha}\beta} \epsilon^{ijkn} \\
& - \frac{1}{6} \mathcal{D} \bar{\mathcal{I}} T_{bcjk} T_{ad}{}^{ij} \Lambda_{\alpha l} \Lambda^{\dot{\beta}k} \Lambda^{\dot{\gamma}l} \gamma_d{}^{\dot{\alpha}\alpha} \gamma_{bc\dot{\beta}\dot{\gamma}} + \frac{1}{96} \mathcal{D} \bar{\mathcal{I}} T_{bcjk} \Lambda_{\alpha l} \Lambda^{\dot{\beta}m} \chi^{\dot{\gamma}}{}_{mn}{}^l \gamma_a{}^{\dot{\alpha}\alpha} \gamma_{bc\dot{\beta}\dot{\gamma}} \epsilon^{ijkn} \\
& - \frac{29}{320} \mathcal{D} \mathcal{D} \mathcal{H} E_{jk} \Lambda_{\alpha l} \Lambda_{\beta m} \chi_\gamma{}^{ij}{}_n \epsilon^{\alpha\gamma} \gamma_a{}^{\dot{\alpha}\beta} \epsilon^{klmn} + \frac{1}{144} \mathcal{D} \mathcal{D} \mathcal{H} \Lambda_{\alpha j} \Lambda_{\beta k} \bar{P}_b \chi^{\dot{\beta}}{}_{lm}{}^j \gamma_b{}^\beta{}_{\dot{\beta}} \gamma_a{}^{\dot{\alpha}\alpha} \epsilon^{iklm} \\
& - \frac{1}{32} \mathcal{D} \mathcal{I} \Lambda_{\alpha j} \Lambda_{\beta k} \Lambda_{\gamma l} \gamma_a{}^{\dot{\alpha}\alpha} \gamma_{bc}{}^{\beta\gamma} \nabla_b \bar{P}_c \epsilon^{ijkl} + \frac{1}{32} \mathcal{D} \mathcal{I} \Lambda_{\alpha j} \Lambda_{\beta k} \Lambda_{\gamma l} \gamma_b{}^{\dot{\alpha}\alpha} \gamma_{ac}{}^{\beta\gamma} \nabla_b \bar{P}_c \epsilon^{ijkl} - \frac{1}{144} \mathcal{D} \mathcal{H} E^{jk} \Lambda_{\alpha j} \Lambda_{\beta k} \Lambda^{\dot{\beta}i} \bar{P}_b \epsilon^{\alpha\beta} \gamma_{ab}{}^{\dot{\alpha}}{}_{\dot{\beta}} \\
& + \frac{5}{576} \mathcal{D} \mathcal{H} \Lambda_{\alpha j} \Lambda_{\beta k} \Lambda_{\gamma l} \gamma_b{}^{\dot{\alpha}\alpha} \gamma_{ac}{}^{\beta\gamma} \nabla_c P_b \epsilon^{ijkl} - \frac{1}{54} \mathcal{I} E^{ij} T_{bc}{}^{kl} \Lambda_{\alpha j} \Lambda_{\beta k} \Lambda_{\gamma l} \gamma_a{}^{\dot{\alpha}\alpha} \gamma_{bc}{}^{\beta\gamma} - \frac{1}{27} \mathcal{I} E^{ij} T_{bc}{}^{kl} \Lambda_{\alpha j} \Lambda_{\beta k} \Lambda_{\gamma l} \gamma_a{}^{\dot{\alpha}\beta} \gamma_{bc}{}^{\alpha\gamma} \\
& - \frac{1}{2} \mathcal{I} T_{bc}{}^{jk} \Lambda_{\alpha j} \Lambda_{\beta k} \Lambda^{\dot{\beta}i} \bar{P}_b \gamma_a{}^\alpha{}_{\dot{\beta}} \gamma_c{}^{\dot{\alpha}\beta} + \frac{1}{3} \mathcal{H} P_b T_{bc}{}^{ij} \Lambda_{\alpha j} \Lambda_{\beta k} \Lambda^{\dot{\beta}k} \gamma_a{}^\alpha{}_{\dot{\beta}} \gamma_c{}^{\dot{\alpha}\beta} + \frac{1}{3} \mathcal{H} P_b T_{bc}{}^{ij} \Lambda_{\alpha j} \Lambda_{\beta k} \Lambda^{\dot{\beta}k} \gamma_a{}^\beta{}_{\dot{\beta}} \gamma_c{}^{\dot{\alpha}\alpha} \\
& + (-\frac{13}{12} \mathcal{D}^\dagger \bar{\mathcal{I}} - \frac{11}{192} \mathcal{D}^\dagger \mathcal{D}^\dagger \mathcal{D}^\dagger \bar{\mathcal{H}}) P_b P_c \Lambda_{\alpha j} \Lambda^{\dot{\beta}i} \Lambda^{\dot{\gamma}j} \epsilon_{\dot{\beta}\dot{\gamma}} \gamma_a{}^{\dot{\alpha}\alpha} + (-\frac{4}{9} \mathcal{D}^\dagger \bar{\mathcal{H}} + \frac{13}{144} \mathcal{D} \bar{\mathcal{I}}) P_b T_{abjk} \Lambda_{\alpha l} \Lambda_{\beta m} \Lambda^{\dot{\alpha}l} \epsilon^{\alpha\beta} \epsilon^{ijkm} \\
& + (-\frac{101}{240} \bar{\mathcal{H}} + \frac{73}{240} \mathcal{H}) P_b T_{ac}{}^{ij} \Lambda_{\alpha j} \Lambda_{\beta k} \Lambda^{\dot{\beta}k} \gamma_b{}^\alpha{}_{\dot{\beta}} \gamma_c{}^{\dot{\alpha}\beta} + (-\frac{101}{240} \bar{\mathcal{H}} + \frac{73}{240} \mathcal{H}) P_b T_{ac}{}^{ij} \Lambda_{\alpha j} \Lambda_{\beta k} \Lambda^{\dot{\beta}k} \gamma_b{}^\beta{}_{\dot{\beta}} \gamma_c{}^{\dot{\alpha}\alpha} \\
& + (-\frac{10}{27} \bar{\mathcal{I}} - \frac{1}{54} \mathcal{D}^\dagger \mathcal{D}^\dagger \bar{\mathcal{H}}) T_{bcjk} \Lambda^{\dot{\beta}i} \Lambda^{\dot{\gamma}j} \Lambda^{\dot{\delta}k} \bar{P}_d \gamma_{bc\dot{\beta}\dot{\gamma}} \gamma_{ad}{}^{\dot{\alpha}}{}_{\dot{\delta}} + (-\frac{487}{1440} \bar{\mathcal{H}} + \frac{157}{5760} \mathcal{H}) \Lambda_{\alpha j} \Lambda_{\beta k} \Lambda^{\dot{\beta}j} \epsilon^{\alpha\beta} \gamma_{ab}{}^{\dot{\alpha}}{}_{\dot{\beta}} \nabla_c T_{bclm} \epsilon^{iklm} \\
& + (-\frac{481}{1440} \mathcal{D} \mathcal{D} \mathcal{H} - \frac{17}{10} \mathcal{I}) T_{bc}{}^{ij} \Lambda_{\alpha j} \Lambda_{\beta k} \Lambda^{\dot{\beta}k} \bar{P}_b \epsilon^{\alpha\beta} \gamma_{ac}{}^{\dot{\alpha}}{}_{\dot{\beta}} + (-\frac{29}{96} \mathcal{D} \mathcal{D} \mathcal{H} - \frac{23}{12} \mathcal{I}) T_{ab}{}^{ij} \Lambda_{\alpha j} \Lambda_{\beta k} \Lambda^{\dot{\beta}k} \bar{P}_c \gamma_c{}^\alpha{}_{\dot{\beta}} \gamma_b{}^{\dot{\alpha}\beta} \\
& + (-\frac{29}{96} \mathcal{D} \mathcal{D} \mathcal{H} - \frac{23}{12} \mathcal{I}) T_{ab}{}^{ij} \Lambda_{\alpha j} \Lambda_{\beta k} \Lambda^{\dot{\beta}k} \bar{P}_c \gamma_c{}^\beta{}_{\dot{\beta}} \gamma_b{}^{\dot{\alpha}\alpha} + (-\frac{7}{24} \mathcal{D}^\dagger \mathcal{I} + \frac{1}{48} \mathcal{D} \mathcal{H}) \Lambda_{\alpha j} \Lambda^{\dot{\beta}i} \Lambda^{\dot{\gamma}j} \bar{P}_a \bar{P}_b \epsilon_{\dot{\beta}\dot{\gamma}} \gamma_b{}^{\dot{\alpha}\alpha} \\
& + (-\frac{5}{18} \mathcal{D}^\dagger \bar{\mathcal{H}} - \frac{2}{9} \mathcal{D} \bar{\mathcal{I}}) T_{ab}{}^{jk} \Lambda^{\dot{\alpha}l} \Lambda^{\dot{\beta}i} \Lambda^{\dot{\gamma}m} \bar{P}_b \epsilon_{\dot{\beta}\dot{\gamma}} \epsilon_{jklm} + (-\frac{239}{960} \bar{\mathcal{H}} + \frac{707}{11520} \mathcal{H}) T_{bcjk} \Lambda_{\alpha l} \Lambda^{\dot{\beta}m} \gamma_b{}^\beta{}_{\dot{\beta}} \gamma_a{}^{\dot{\alpha}\alpha} \nabla_c \Lambda_{\beta m} \epsilon^{ijkl} \\
& + (-\frac{59}{288} \bar{\mathcal{H}} - \frac{77}{1152} \mathcal{H}) T_{bcjk} \Lambda_{\alpha l} \Lambda_{\beta m} \gamma_b{}^\alpha{}_{\dot{\beta}} \gamma_a{}^{\dot{\alpha}\beta} \nabla_c \Lambda^{\dot{\beta}i} \epsilon^{jklm} + (-\frac{5}{27} \bar{\mathcal{I}} - \frac{1}{108} \mathcal{D}^\dagger \mathcal{D}^\dagger \bar{\mathcal{H}}) T_{bcjk} \Lambda^{\dot{\beta}i} \Lambda^{\dot{\gamma}j} \Lambda^{\dot{\delta}k} \bar{P}_d \gamma_{bc\dot{\beta}\dot{\gamma}} \delta \gamma_{ad}{}^{\dot{\alpha}}{}_{\dot{\delta}} \\
& + (-\frac{7}{40} \bar{\mathcal{H}} - \frac{1}{10} \mathcal{H}) P_b T_{bc}{}^{jk} \Lambda_{\alpha j} \Lambda_{\beta k} \Lambda^{\dot{\beta}i} \gamma_c{}^\alpha{}_{\dot{\beta}} \gamma_a{}^{\dot{\alpha}\beta} + (-\frac{119}{720} \bar{\mathcal{H}} + \frac{181}{720} \mathcal{H}) P_b T_{ac}{}^{ij} \Lambda_{\alpha j} \Lambda_{\beta k} \Lambda^{\dot{\beta}k} \epsilon^{\alpha\beta} \gamma_{bc}{}^{\dot{\alpha}}{}_{\dot{\beta}} \\
& + (-\frac{95}{576} \bar{\mathcal{H}} - \frac{49}{1440} \mathcal{H}) T_{bcjk} \Lambda_{\alpha l} \Lambda^{\dot{\beta}j} \gamma_b{}^\alpha{}_{\dot{\beta}} \gamma_a{}^{\dot{\alpha}\beta} \nabla_c \Lambda_{\beta m} \epsilon^{iklm} + (-\frac{7}{48} \mathcal{D}^\dagger \bar{\mathcal{H}} - \frac{11}{64} \mathcal{D} \bar{\mathcal{I}}) P_a \Lambda_{\alpha j} \Lambda^{\dot{\beta}i} \Lambda^{\dot{\gamma}j} \bar{P}_b \epsilon_{\dot{\beta}\dot{\gamma}} \gamma_b{}^{\dot{\alpha}\alpha} \\
& + (-\frac{101}{720} \bar{\mathcal{I}} - \frac{169}{2880} \mathcal{D}^\dagger \mathcal{D}^\dagger \bar{\mathcal{H}}) \Lambda^{\dot{\beta}i} \Lambda^{\dot{\gamma}j} \Lambda^{\dot{\delta}k} \epsilon_{\dot{\beta}\dot{\gamma}} \gamma_{bc}{}^{\dot{\alpha}}{}_{\dot{\delta}} \nabla_b T_{ac}{}^{lm} \epsilon_{jklm} + (-\frac{101}{720} \mathcal{D} \mathcal{D} \mathcal{H} - \frac{157}{180} \mathcal{I}) T_{ab}{}^{jk} \Lambda_{\alpha j} \Lambda_{\beta k} \Lambda^{\dot{\beta}i} \bar{P}_c \gamma_c{}^\alpha{}_{\dot{\beta}} \gamma_b{}^{\dot{\alpha}\beta} \\
& + (-\frac{5}{36} \mathcal{D}^\dagger \bar{\mathcal{H}} - \frac{1}{12} \mathcal{D} \bar{\mathcal{I}}) T_{bc}{}^{ij} \Lambda^{\dot{\alpha}k} \Lambda^{\dot{\beta}l} \Lambda^{\dot{\gamma}m} \bar{P}_b \gamma_{ac\dot{\beta}\dot{\gamma}} \epsilon_{jklm} + (-\frac{47}{360} \bar{\mathcal{H}} + \frac{43}{180} \mathcal{H}) P_b T_{ac}{}^{jk} \Lambda_{\alpha j} \Lambda_{\beta k} \Lambda^{\dot{\beta}i} \gamma_b{}^\alpha{}_{\dot{\beta}} \gamma_c{}^{\dot{\alpha}\beta} \\
& + (-\frac{61}{480} \mathcal{D}^\dagger \mathcal{I} + \frac{1}{8} \mathcal{D} \mathcal{H}) T_{abjk} \Lambda_{\alpha l} \Lambda_{\beta m} \chi_\gamma{}^{il}{}_n \epsilon^{\alpha\beta} \gamma_b{}^{\dot{\alpha}\gamma} \epsilon^{jkmn} + (-\frac{1}{8} \mathcal{D}^\dagger \bar{\mathcal{H}} - \frac{1}{16} \mathcal{D} \bar{\mathcal{I}}) T_{abjk} T_{bc}{}^{ij} \Lambda_{\alpha l} \Lambda^{\dot{\beta}k} \Lambda^{\dot{\gamma}l} \epsilon_{\dot{\beta}\dot{\gamma}} \gamma_c{}^{\dot{\alpha}\alpha} \\
& + (-\frac{1}{8} \mathcal{D}^\dagger \bar{\mathcal{H}} - \frac{1}{16} \mathcal{D} \bar{\mathcal{I}}) T_{bcjk} T_{ab}{}^{ij} \Lambda_{\alpha l} \Lambda^{\dot{\beta}k} \Lambda^{\dot{\gamma}l} \epsilon_{\dot{\beta}\dot{\gamma}} \gamma_c{}^{\dot{\alpha}\alpha} + (-\frac{47}{384} \bar{\mathcal{H}} - \frac{29}{1920} \mathcal{H}) T_{bcjk} \Lambda_{\alpha l} \Lambda_{\beta m} \epsilon^{\alpha\beta} \gamma_{ab}{}^{\dot{\alpha}}{}_{\dot{\beta}} \nabla_c \Lambda^{\dot{\beta}l} \epsilon^{ijkm} \\
& + (-\frac{173}{1440} \bar{\mathcal{H}} + \frac{83}{5760} \mathcal{H}) \Lambda_{\alpha j} \Lambda_{\beta k} \Lambda^{\dot{\beta}j} \epsilon^{\alpha\beta} \gamma_{bc}{}^{\dot{\alpha}}{}_{\dot{\beta}} \nabla_b T_{aclm} \epsilon^{iklm} + (-\frac{31}{288} \mathcal{D} \mathcal{D} \mathcal{H} + \frac{3}{4} \mathcal{I}) T_{bc}{}^{ij} \Lambda_{\alpha j} \Lambda_{\beta k} \Lambda^{\dot{\beta}k} \bar{P}_b \gamma_c{}^\alpha{}_{\dot{\beta}} \gamma_a{}^{\dot{\alpha}\beta} \\
& + (-\frac{31}{288} \mathcal{D} \mathcal{D} \mathcal{H} + \frac{3}{4} \mathcal{I}) T_{bc}{}^{ij} \Lambda_{\alpha j} \Lambda_{\beta k} \Lambda^{\dot{\beta}k} \bar{P}_b \gamma_c{}^\beta{}_{\dot{\beta}} \gamma_a{}^{\dot{\alpha}\alpha} + (-\frac{5}{48} \bar{\mathcal{H}} - \frac{1}{36} \mathcal{H}) E_{jk} T_{ab}{}^{jl} \Lambda_{\alpha l} \Lambda^{\dot{\beta}i} \Lambda^{\dot{\gamma}k} \epsilon_{\dot{\beta}\dot{\gamma}} \gamma_b{}^{\dot{\alpha}\alpha} \\
& + (-\frac{71}{720} \mathcal{D} \mathcal{D} \mathcal{D} \mathcal{H} + \frac{11}{180} \mathcal{D} \mathcal{I}) T_{ab}{}^{ij} T_{bc}{}^{kl} \Lambda_{\alpha j} \Lambda_{\beta k} \Lambda_{\gamma l} \epsilon^{\alpha\beta} \gamma_c{}^{\dot{\alpha}\gamma} + (-\frac{371}{3840} \bar{\mathcal{H}} + \frac{371}{3840} \mathcal{H}) T_{abjk} \Lambda_{\alpha l} \Lambda^{\dot{\beta}m} \gamma_b{}^\alpha{}_{\dot{\beta}} \gamma_c{}^{\dot{\alpha}\beta} \nabla_c \Lambda_{\beta m} \epsilon^{ijkl} \\
& + (-\frac{23}{240} \mathcal{D} \mathcal{D} \mathcal{D} \mathcal{H} + \frac{49}{180} \mathcal{D} \mathcal{I}) T_{ab}{}^{jk} T_{bc}{}^{il} \Lambda_{\alpha j} \Lambda_{\beta k} \Lambda_{\gamma l} \epsilon^{\alpha\gamma} \gamma_c{}^{\dot{\alpha}\beta} + (-\frac{13}{144} \bar{\mathcal{I}} - \frac{13}{288} \mathcal{D}^\dagger \mathcal{D}^\dagger \bar{\mathcal{H}}) E^{jk} T_{bcjl} \Lambda_{\alpha k} \Lambda^{\dot{\beta}i} \Lambda^{\dot{\gamma}l} \gamma_a{}^{\dot{\alpha}\alpha} \gamma_{bc\dot{\beta}\dot{\gamma}} \\
& + (-\frac{43}{480} \bar{\mathcal{H}} - \frac{77}{480} \mathcal{H}) T_{abjk} \Lambda_{\alpha l} \Lambda^{\dot{\beta}i} \gamma_c{}^\alpha{}_{\dot{\beta}} \gamma_b{}^{\dot{\alpha}\beta} \nabla_c \Lambda_{\beta m} \epsilon^{jklm} + (-\frac{11}{128} \mathcal{D} \mathcal{D} \mathcal{H} + \frac{1}{16} \mathcal{I}) E_{jk} \Lambda_{\alpha l} \Lambda_{\beta m} R(Q)_{ab\gamma}{}^j \epsilon^{\alpha\gamma} \gamma_b{}^{\dot{\alpha}\beta} \epsilon^{iklm} \\
& + (-\frac{1}{12} \mathcal{D}^\dagger \mathcal{I} + \frac{1}{24} \mathcal{D} \mathcal{H}) T_{abjk} \Lambda_{\alpha l} \Lambda_{\beta m} R(Q)_{bc\gamma}{}^l \epsilon^{\alpha\gamma} \gamma_c{}^{\dot{\alpha}\beta} \epsilon^{ijkm} + (-\frac{1}{12} \mathcal{D}^\dagger \mathcal{I} + \frac{1}{24} \mathcal{D} \mathcal{H}) T_{abjk} \Lambda_{\alpha l} \Lambda_{\beta m} R(Q)_{bc\gamma}{}^l \epsilon^{\beta\gamma} \gamma_c{}^{\dot{\alpha}\alpha} \epsilon^{ijkm} \\
& + (-\frac{47}{576} \bar{\mathcal{H}} - \frac{1}{64} \mathcal{H}) T_{abjk} \Lambda_{\alpha l} \Lambda^{\dot{\beta}m} \gamma_b{}^\beta{}_{\dot{\beta}} \gamma_c{}^{\dot{\alpha}\alpha} \nabla_c \Lambda_{\beta m} \epsilon^{ijkl} + (-\frac{29}{384} \bar{\mathcal{I}} - \frac{7}{384} \mathcal{D}^\dagger \mathcal{D}^\dagger \bar{\mathcal{H}}) T_{bcjk} T_{bclm} \Lambda_{\alpha n} \Lambda^{\dot{\alpha}i} \Lambda^{\dot{\beta}n} \gamma_a{}^\alpha{}_{\dot{\beta}} \epsilon^{jklm} \\
& + (-\frac{3}{40} \mathcal{D}^\dagger \mathcal{I} + \frac{1}{32} \mathcal{D} \mathcal{H}) T_{bcjk} \Lambda_{\alpha l} \Lambda_{\beta m} \Lambda^{\dot{\alpha}i} \bar{P}_b \gamma_{ac}{}^{\alpha\beta} \epsilon^{jklm} + (-\frac{43}{576} \mathcal{D}^\dagger \mathcal{I} - \frac{1}{24} \mathcal{D} \mathcal{H}) P_b \Lambda_{\alpha j} \Lambda_{\beta k} \gamma_a{}^{\dot{\alpha}\gamma} \gamma_{bc}{}^{\alpha\beta} \nabla_c \Lambda_{\gamma l} \epsilon^{ijkl} + 12 \dots
\end{aligned}$$

$$\begin{aligned}
[\hat{\Omega}_a^{\dot{\alpha}i}]_{3,cont.} = & +(-\frac{41}{576}\bar{\mathcal{H}} - \frac{5}{192}\mathcal{H})T_{bcjk}\Lambda_{\alpha l}\Lambda^{\dot{\beta}m}\gamma_b^{\beta}\gamma_c^{\dot{\alpha}}\nabla_a\Lambda_{\beta m}\varepsilon^{ijkl} + (-\frac{101}{1440}\bar{\mathcal{H}} + \frac{31}{1440}\mathcal{H})T_{bcjk}\Lambda_{\alpha l}\Lambda_{\beta m}\gamma_a^{\alpha}\gamma_b^{\dot{\alpha}\beta}\nabla_c\Lambda^{\dot{\beta}l}\varepsilon^{ijkm} \\
& + (-\frac{187}{2880}\bar{\mathcal{H}} + \frac{19}{960}\mathcal{H})T_{bcjk}\Lambda_{\alpha l}\Lambda^{\dot{\beta}m}\gamma_a^{\beta}\gamma_b^{\dot{\alpha}}\nabla_c\Lambda_{\beta m}\varepsilon^{ijkl} + (-\frac{367}{5760}\bar{\mathcal{H}} + \frac{227}{2880}\mathcal{H})T_{bcjk}\Lambda_{\alpha l}\Lambda^{\dot{\beta}i}\gamma_b^{\alpha}\gamma_a^{\dot{\alpha}\beta}\nabla_c\Lambda_{\beta m}\varepsilon^{jklm} \\
& + (-\frac{181}{2880}\bar{\mathcal{H}} + \frac{1}{48}\mathcal{H})T_{bcjk}\Lambda_{\alpha l}\Lambda^{\dot{\beta}l}\gamma_a^{\alpha}\gamma_b^{\dot{\alpha}\beta}\nabla_c\Lambda_{\beta m}\varepsilon^{ijkm} + (-\frac{17}{288}\mathcal{D}^{\dagger}\bar{\mathcal{H}} - \frac{25}{288}\mathcal{D}\bar{\mathcal{I}})E_{jk}E^{ij}\Lambda_{\alpha l}\Lambda^{\dot{\beta}k}\Lambda^{\dot{\gamma}l}\epsilon_{\dot{\beta}\dot{\gamma}}\gamma_a^{\dot{\alpha}} \\
& + (-\frac{329}{5760}\bar{\mathcal{H}} + \frac{173}{5760}\mathcal{H})T_{bcjk}\Lambda_{\alpha l}\Lambda^{\dot{\beta}j}\epsilon^{\alpha\beta}\gamma_{bc}^{\dot{\alpha}}\nabla_a\Lambda_{\beta m}\varepsilon^{iklm} + (-\frac{649}{11520}\bar{\mathcal{H}} - \frac{803}{11520}\mathcal{H})\Lambda_{\alpha j}\Lambda_{\beta k}\Lambda^{\dot{\beta}i}\gamma_b^{\alpha}\gamma_a^{\dot{\alpha}\beta}\nabla_cT_{bclm}\varepsilon^{jklm} \\
& + (-\frac{9}{160}\mathcal{D}\mathcal{D}\mathcal{D}\mathcal{H} - \frac{13}{120}\mathcal{D}\mathcal{I})T_{bc}^{ij}T_{bc}^{kl}\Lambda_{\alpha j}\Lambda_{\beta k}\Lambda_{\gamma l}\epsilon^{\alpha\beta}\gamma_a^{\dot{\alpha}}\gamma + (-\frac{1}{18}\mathcal{D}^{\dagger}\mathcal{D}^{\dagger}\bar{\mathcal{I}} - \frac{1}{72}\mathcal{D}^{\dagger}\mathcal{D}^{\dagger}\mathcal{D}^{\dagger}\bar{\mathcal{H}})P_bT_{bcjk}\Lambda^{\dot{\beta}i}\Lambda^{\dot{\gamma}j}\Lambda^{\dot{\delta}k}\epsilon_{\dot{\beta}\dot{\gamma}}\gamma_{ac}^{\dot{\alpha}}\gamma_{\dot{\delta}} \\
& + (-\frac{103}{1920}\bar{\mathcal{H}} + \frac{5}{144}\mathcal{H})T_{bcjk}\Lambda_{\alpha l}\Lambda_{\beta m}\gamma_b^{\alpha}\gamma_a^{\dot{\alpha}\beta}\nabla_c\Lambda^{\dot{\beta}m}\varepsilon^{ijkl} + (-\frac{7}{144}\mathcal{D}^{\dagger}\bar{\mathcal{H}} - \frac{25}{288}\mathcal{D}\bar{\mathcal{I}})E^{ij}T_{ab}^{kl}\Lambda_{\alpha j}\Lambda^{\dot{\alpha}m}\Lambda^{\dot{\beta}n}\gamma_b^{\alpha}\gamma_{\dot{\beta}}\varepsilon_{klmn} \\
& + (-\frac{17}{360}\bar{\mathcal{H}} - \frac{1}{16}\mathcal{H})T_{bcjk}\Lambda_{\alpha l}\Lambda^{\dot{\beta}m}\gamma_a^{\alpha}\gamma_b^{\dot{\alpha}\beta}\nabla_c\Lambda_{\beta m}\varepsilon^{ijkl} + (-\frac{11}{240}\bar{\mathcal{I}} - \frac{1}{96}\mathcal{D}^{\dagger}\mathcal{D}^{\dagger}\bar{\mathcal{H}})T_{abjk}T_{bclm}\Lambda_{\alpha n}\Lambda^{\dot{\alpha}i}\Lambda^{\dot{\beta}l}\gamma_c^{\alpha}\gamma_{\dot{\beta}}\varepsilon^{jkmn} \\
& + (-\frac{11}{240}\bar{\mathcal{I}} - \frac{1}{96}\mathcal{D}^{\dagger}\mathcal{D}^{\dagger}\bar{\mathcal{H}})T_{abjk}T_{bclm}\Lambda_{\alpha n}\Lambda^{\dot{\alpha}j}\Lambda^{\dot{\beta}i}\gamma_c^{\alpha}\gamma_{\dot{\beta}}\varepsilon^{klmn} + (-\frac{13}{288}\mathcal{D}^{\dagger}\mathcal{I} + \frac{1}{72}\mathcal{D}\mathcal{H})P_b\Lambda_{\alpha j}\Lambda_{\beta k}\gamma_c^{\dot{\alpha}}\gamma_{ab}^{\beta\gamma}\nabla_c\Lambda_{\gamma l}\varepsilon^{ijkl} \\
& + (-\frac{7}{160}\mathcal{D}^{\dagger}\mathcal{I} + \frac{1}{24}\mathcal{D}\mathcal{H})T_{abjk}\Lambda_{\alpha l}\Lambda_{\beta m}\chi_{\gamma}^{il}\epsilon^{\beta\gamma}\gamma_b^{\dot{\alpha}}\gamma_c^{\dot{\alpha}}\varepsilon^{jkmn} + (-\frac{25}{576}\mathcal{D}^{\dagger}\bar{\mathcal{H}} - \frac{1}{32}\mathcal{D}\bar{\mathcal{I}})E^{ij}T_{ab}^{kl}\Lambda_{\alpha m}\Lambda^{\dot{\alpha}m}\Lambda^{\dot{\beta}n}\gamma_b^{\alpha}\gamma_{\dot{\beta}}\varepsilon_{jklm} \\
& + (-\frac{1}{24}\mathcal{D}^{\dagger}\bar{\mathcal{H}} - \frac{1}{24}\mathcal{D}\bar{\mathcal{I}})T_{bcjk}T_{ad}^{il}\Lambda_{\alpha l}\Lambda^{\dot{\beta}j}\Lambda^{\dot{\gamma}k}\gamma_d^{\dot{\alpha}}\gamma_{bc\dot{\beta}\dot{\gamma}}^{\dot{\alpha}} + (-\frac{23}{576}\mathcal{D}^{\dagger}\mathcal{I} - \frac{1}{24}\mathcal{D}\mathcal{H})P_b\Lambda_{\alpha j}\Lambda_{\beta k}\epsilon^{\alpha\gamma}\gamma_b^{\dot{\alpha}\beta}\nabla_a\Lambda_{\gamma l}\varepsilon^{ijkl} \\
& + (-\frac{59}{1536}\mathcal{D}^{\dagger}\bar{\mathcal{H}} - \frac{79}{2304}\mathcal{D}\bar{\mathcal{I}})P_b\Lambda_{\alpha j}\Lambda^{\dot{\beta}i}\Lambda^{\dot{\gamma}j}\bar{P}_c\gamma_b^{\dot{\alpha}}\gamma_{ac\dot{\beta}\dot{\gamma}}^{\dot{\alpha}} + (-\frac{1}{27}\mathcal{D}^{\dagger}\bar{\mathcal{H}} - \frac{13}{432}\mathcal{D}\bar{\mathcal{I}})E_{jk}\Lambda^{\dot{\beta}i}\Lambda^{\dot{\gamma}j}\Lambda^{\dot{\delta}k}\bar{P}_b\epsilon_{\dot{\gamma}\dot{\delta}}\gamma_{ab}^{\dot{\alpha}}\gamma_{\dot{\beta}} \\
& + (-\frac{137}{3840}\mathcal{D}^{\dagger}\bar{\mathcal{H}} - \frac{221}{2560}\mathcal{D}\bar{\mathcal{I}})T_{bc}^{jk}\Lambda^{\dot{\beta}i}\Lambda^{\dot{\gamma}l}R(Q)_{bca}{}^m\epsilon_{\dot{\beta}\dot{\gamma}}\gamma_a^{\dot{\alpha}}\varepsilon_{jklm} + (-\frac{41}{1152}\bar{\mathcal{H}} - \frac{5}{384}\mathcal{H})T_{abjk}\Lambda_{\alpha l}\Lambda_{\beta m}\gamma_b^{\alpha}\gamma_c^{\dot{\alpha}\beta}\nabla_c\Lambda^{\dot{\beta}l}\varepsilon^{ijkm} \\
& + (-\frac{41}{1152}\bar{\mathcal{H}} - \frac{5}{384}\mathcal{H})T_{bcjk}\Lambda_{\alpha l}\Lambda_{\beta m}\gamma_b^{\alpha}\gamma_c^{\dot{\alpha}\beta}\nabla_a\Lambda^{\dot{\beta}l}\varepsilon^{ijkm} + (-\frac{49}{1440}\bar{\mathcal{H}} - \frac{71}{1440}\mathcal{H})T_{abjk}\Lambda_{\alpha l}\Lambda^{\dot{\beta}m}\gamma_c^{\alpha}\gamma_b^{\dot{\alpha}\beta}\nabla_c\Lambda_{\beta m}\varepsilon^{ijkl} \\
& + (-\frac{1}{32}\mathcal{D}^{\dagger}\mathcal{I} + \frac{1}{48}\mathcal{D}\mathcal{H})E_{jk}\Lambda_{\alpha l}\Lambda^{\dot{\beta}j}\gamma_a^{\beta}\gamma_b^{\dot{\alpha}}\nabla_b\Lambda_{\beta m}\varepsilon^{iklm} + (-\frac{143}{4608}\mathcal{D}^{\dagger}\bar{\mathcal{H}} + \frac{1711}{2304}\mathcal{D}\bar{\mathcal{I}})P_b\Lambda_{\alpha j}\Lambda^{\dot{\beta}i}\Lambda^{\dot{\gamma}j}\bar{P}_c\gamma_c^{\dot{\alpha}}\gamma_{ab\dot{\beta}\dot{\gamma}}^{\dot{\alpha}} \\
& + (-\frac{39}{1280}\bar{\mathcal{H}} + \frac{17}{11520}\mathcal{H})T_{bcjk}\Lambda_{\alpha l}\Lambda^{\dot{\beta}i}\epsilon^{\alpha\beta}\gamma_{bc}^{\dot{\alpha}}\nabla_a\Lambda_{\beta m}\varepsilon^{jklm} + (-\frac{17}{576}\mathcal{D}^{\dagger}\bar{\mathcal{H}} - \frac{1}{72}\mathcal{D}\bar{\mathcal{I}})E^{jk}T_{ab}^{lm}\Lambda_{\alpha j}\Lambda^{\dot{\alpha}n}\Lambda^{\dot{\beta}i}\gamma_b^{\alpha}\gamma_{\dot{\beta}}\varepsilon_{klmn} \\
& + (-\frac{7}{240}\bar{\mathcal{H}} - \frac{1}{24}\mathcal{H})\Lambda_{\alpha j}\Lambda_{\beta k}\Lambda^{\dot{\beta}l}\gamma_a^{\alpha}\gamma_b^{\dot{\alpha}\beta}\nabla_cT_{bclm}\varepsilon^{ijkm} + (-\frac{1}{36}\bar{\mathcal{I}} + \frac{1}{48}\mathcal{D}^{\dagger}\mathcal{D}^{\dagger}\bar{\mathcal{H}})T_{abjk}T_{bclm}\Lambda_{\alpha n}\Lambda^{\dot{\alpha}l}\Lambda^{\dot{\beta}n}\gamma_c^{\alpha}\gamma_{\dot{\beta}}\varepsilon^{ijkm} \\
& + (-\frac{1}{36}\bar{\mathcal{I}} + \frac{1}{48}\mathcal{D}^{\dagger}\mathcal{D}^{\dagger}\bar{\mathcal{H}})T_{abjk}T_{bclm}\Lambda_{\alpha n}\Lambda^{\dot{\alpha}n}\Lambda^{\dot{\beta}j}\gamma_c^{\alpha}\gamma_{\dot{\beta}}\varepsilon^{iklm} + (-\frac{1}{36}\mathcal{D}^{\dagger}\bar{\mathcal{I}} + \frac{1}{48}\mathcal{D}^{\dagger}\mathcal{D}^{\dagger}\mathcal{D}^{\dagger}\bar{\mathcal{H}})P_bT_{bc}^{ij}\Lambda^{\dot{\alpha}k}\Lambda^{\dot{\beta}l}\Lambda^{\dot{\gamma}m}\gamma_{ac\dot{\beta}\dot{\gamma}}^{\dot{\alpha}}\varepsilon_{jklm} \\
& + (-\frac{1}{36}\mathcal{D}\mathcal{D}\mathcal{D}\mathcal{H} - \frac{1}{15}\mathcal{D}\mathcal{I})T_{ab}^{jk}T_{cd}^{il}\Lambda_{\alpha j}\Lambda_{\beta k}\Lambda_{\gamma l}\gamma_b^{\dot{\alpha}}\gamma_{cd}^{\beta\gamma} + (-\frac{19}{720}\mathcal{D}\mathcal{D}\mathcal{H} + \frac{19}{60}\mathcal{I})T_{bc}^{jk}\Lambda_{\alpha j}\Lambda_{\beta k}\Lambda^{\dot{\beta}i}\bar{P}_b\gamma_c^{\alpha}\gamma_a^{\dot{\alpha}\beta} \\
& + (-\frac{571}{23040}\bar{\mathcal{H}} - \frac{37}{5760}\mathcal{H})T_{bcjk}\Lambda_{\alpha l}\Lambda^{\dot{\beta}i}\gamma_{ad}^{\alpha\beta}\gamma_{bc}^{\dot{\alpha}}\nabla_d\Lambda_{\beta m}\varepsilon^{jklm} + (-\frac{19}{768}\bar{\mathcal{H}} + \frac{13}{640}\mathcal{H})T_{bcjk}\Lambda_{\alpha l}\Lambda^{\dot{\beta}i}\epsilon^{\alpha\beta}\gamma_{ab}^{\dot{\alpha}}\nabla_c\Lambda_{\beta m}\varepsilon^{jklm} \\
& + (-\frac{31}{1280}\bar{\mathcal{H}} + \frac{59}{3840}\mathcal{H})T_{bcjk}\Lambda_{\alpha l}\Lambda_{\beta m}\gamma_{ad}^{\alpha\beta}\gamma_{bc}^{\dot{\alpha}}\nabla_d\Lambda^{\dot{\beta}j}\varepsilon^{iklm} + (-\frac{37}{1536}\mathcal{D}^{\dagger}\bar{\mathcal{H}} + \frac{607}{2304}\mathcal{D}\bar{\mathcal{I}})P_b\Lambda_{\alpha j}\Lambda^{\dot{\beta}i}\Lambda^{\dot{\gamma}j}\bar{P}_c\gamma_a^{\dot{\alpha}}\gamma_{bc\dot{\beta}\dot{\gamma}}^{\dot{\alpha}} \\
& + (-\frac{11}{480}\bar{\mathcal{H}} - \frac{1}{15}\mathcal{H})P_bT_{cd}^{jk}\Lambda_{\alpha j}\Lambda_{\beta k}\Lambda^{\dot{\beta}i}\gamma_{cd}^{\alpha\beta}\gamma_{ab}^{\dot{\alpha}}\gamma_{\dot{\beta}} + (-\frac{11}{480}\bar{\mathcal{H}} - \frac{1}{48}\mathcal{H})\Lambda_{\alpha j}\Lambda_{\beta k}\Lambda^{\dot{\beta}i}\gamma_a^{\alpha}\gamma_b^{\dot{\alpha}\beta}\nabla_cT_{bclm}\varepsilon^{jklm} \\
& + (-\frac{11}{480}\bar{\mathcal{H}} + \frac{1}{16}\mathcal{H})\Lambda_{\alpha j}\Lambda_{\beta k}\Lambda^{\dot{\beta}j}\gamma_a^{\alpha}\gamma_b^{\dot{\alpha}\beta}\nabla_cT_{bclm}\varepsilon^{iklm} + (-\frac{11}{480}\bar{\mathcal{H}} + \frac{1}{16}\mathcal{H})\Lambda_{\alpha j}\Lambda_{\beta k}\Lambda^{\dot{\beta}j}\gamma_a^{\beta}\gamma_b^{\dot{\alpha}}\nabla_cT_{bclm}\varepsilon^{iklm} \\
& + (-\frac{61}{2880}\mathcal{D}^{\dagger}\mathcal{I} - \frac{1}{72}\mathcal{D}\mathcal{H})E^{ij}\Lambda_{\alpha j}\Lambda_{\beta k}\Lambda^{\dot{\beta}k}\bar{P}_b\gamma_b^{\alpha}\gamma_a^{\dot{\alpha}\beta} + (-\frac{61}{2880}\mathcal{D}^{\dagger}\mathcal{I} - \frac{1}{72}\mathcal{D}\mathcal{H})E^{ij}\Lambda_{\alpha j}\Lambda_{\beta k}\Lambda^{\dot{\beta}k}\bar{P}_b\gamma_b^{\beta}\gamma_a^{\dot{\alpha}} \\
& + (-\frac{1}{48}\bar{\mathcal{H}} - \frac{1}{24}\mathcal{H})T_{bcjk}\Lambda_{\alpha l}\Lambda^{\dot{\beta}j}\gamma_a^{\beta}\gamma_b^{\dot{\alpha}}\nabla_c\Lambda_{\beta m}\varepsilon^{iklm} + (-\frac{1}{48}\mathcal{D}^{\dagger}\bar{\mathcal{H}} - \frac{1}{64}\mathcal{D}\bar{\mathcal{I}})E_{jk}E^{il}\Lambda_{\alpha l}\Lambda^{\dot{\beta}j}\Lambda^{\dot{\gamma}k}\epsilon_{\dot{\beta}\dot{\gamma}}\gamma_a^{\dot{\alpha}} \\
& + (-\frac{1}{48}\mathcal{D}^{\dagger}\bar{\mathcal{H}} + \frac{7}{216}\mathcal{D}\bar{\mathcal{I}})P_bT_{bcjk}\Lambda_{\alpha l}\Lambda_{\beta m}\Lambda^{\dot{\alpha}i}\gamma_{ac}^{\alpha\beta}\varepsilon_{jklm} + (-\frac{1}{48}\mathcal{D}^{\dagger}\bar{\mathcal{H}} + \frac{7}{96}\mathcal{D}\bar{\mathcal{I}})T_{bcjk}\Lambda_{\alpha l}\Lambda^{\dot{\beta}m}\chi^{\dot{\gamma}}{}_{mn}{}^i\gamma_a^{\dot{\alpha}}\gamma_{bc\dot{\beta}\dot{\gamma}}^{\dot{\alpha}}\varepsilon^{jklm} \\
& + (-\frac{1}{48}\mathcal{D}\mathcal{D}\mathcal{H} + \frac{5}{54}\mathcal{I})E^{ij}T_{ab}^{kl}\Lambda_{\alpha j}\Lambda_{\beta k}\Lambda_{\gamma l}\epsilon^{\alpha\beta}\gamma_b^{\dot{\alpha}}\gamma_c^{\dot{\alpha}}\nabla_bT_{cdlm}\varepsilon^{iklm} \\
& + (-\frac{1}{54}\bar{\mathcal{H}} + \frac{1}{108}\mathcal{H})P_b\Lambda_{\alpha j}\Lambda_{\beta k}\chi^{\dot{\beta}}{}_{lm}{}^j\gamma_b^{\alpha}\gamma_a^{\dot{\alpha}\beta}\varepsilon^{iklm} + (-\frac{1}{54}\mathcal{D}^{\dagger}\bar{\mathcal{I}} + \frac{1}{144}\mathcal{D}^{\dagger}\mathcal{D}^{\dagger}\mathcal{D}^{\dagger}\bar{\mathcal{H}})E_{jk}P_b\Lambda^{\dot{\beta}i}\Lambda^{\dot{\gamma}j}\Lambda^{\dot{\delta}k}\epsilon_{\dot{\gamma}\dot{\delta}}\gamma_{ab}^{\dot{\alpha}}\gamma_{\dot{\beta}} \\
& + (-\frac{7}{384}\bar{\mathcal{H}} + \frac{11}{384}\mathcal{H})T_{bc}^{ij}T_{bc}^{kl}\Lambda_{\alpha j}\Lambda^{\dot{\alpha}m}\Lambda^{\dot{\beta}n}\gamma_a^{\alpha}\gamma_{\dot{\beta}}\varepsilon_{klmn} + (-\frac{5}{288}\mathcal{D}\mathcal{D}\mathcal{D}\mathcal{H} - \frac{11}{360}\mathcal{D}\mathcal{I})T_{ab}^{ij}T_{cd}^{kl}\Lambda_{\alpha j}\Lambda_{\beta k}\Lambda_{\gamma l}\gamma_b^{\dot{\alpha}\beta}\gamma_{cd}^{\alpha\gamma} \\
& + (-\frac{1}{60}\bar{\mathcal{H}} - \frac{1}{5}\mathcal{H})P_bT_{bc}^{ij}\Lambda_{\alpha j}\Lambda_{\beta k}\Lambda^{\dot{\beta}k}\gamma_c^{\alpha}\gamma_a^{\dot{\alpha}\beta} + (-\frac{1}{60}\bar{\mathcal{H}} - \frac{1}{5}\mathcal{H})P_bT_{bc}^{ij}\Lambda_{\alpha j}\Lambda_{\beta k}\Lambda^{\dot{\beta}k}\gamma_c^{\beta}\gamma_a^{\dot{\alpha}} \\
& + (-\frac{1}{60}\mathcal{D}^{\dagger}\mathcal{I} - \frac{1}{48}\mathcal{D}\mathcal{H})T_{bcjk}\Lambda_{\alpha l}\Lambda_{\beta m}\Lambda^{\dot{\alpha}j}\bar{P}_b\gamma_{ac}^{\alpha\beta}\varepsilon^{iklm} + (-\frac{1}{64}\bar{\mathcal{H}} - \frac{1}{64}\mathcal{H})T_{ab}^{jk}T_{bc}^{lm}\Lambda_{\alpha j}\Lambda^{\dot{\alpha}i}\Lambda^{\dot{\beta}n}\gamma_c^{\alpha}\gamma_{\dot{\beta}}\varepsilon_{klmn} + 13\cdots
\end{aligned}$$

$$\begin{aligned}
[\hat{\Omega}_a^{\dot{\alpha}i}]_{3,cont.} = & +(-\frac{1}{64}\bar{\mathcal{H}} - \frac{1}{64}\mathcal{H})T_{ab}{}^{jk}T_{bc}{}^{lm}\Lambda_{\alpha l}\Lambda^{\dot{\alpha}n}\Lambda^{\dot{\beta}i}\gamma_c{}^{\alpha}{}_{\dot{\beta}}\varepsilon_{jkmn} + (-\frac{1}{64}\bar{\mathcal{H}} + \frac{1}{64}\mathcal{H})T_{ab}{}^{ij}T_{bc}{}^{kl}\Lambda_{\alpha m}\Lambda^{\dot{\alpha}n}\Lambda^{\dot{\beta}m}\gamma_c{}^{\alpha}{}_{\dot{\beta}}\varepsilon_{jklm} \\
& + (-\frac{1}{64}\bar{\mathcal{H}} + \frac{1}{64}\mathcal{H})T_{ab}{}^{jk}T_{bc}{}^{il}\Lambda_{\alpha m}\Lambda^{\dot{\alpha}m}\Lambda^{\dot{\beta}n}\gamma_c{}^{\alpha}{}_{\dot{\beta}}\varepsilon_{jklm} + (-\frac{1}{64}\mathcal{DDDH} - \frac{1}{48}\mathcal{DI})\Lambda_{\alpha j}\Lambda_{\beta k}\bar{P}_b\gamma_c{}^{\dot{\alpha}\alpha}\gamma_{ab}{}^{\beta\gamma}\nabla_c\Lambda_{\gamma l}\varepsilon^{ijkl} \\
& + (-\frac{179}{11520}\bar{\mathcal{H}} - \frac{49}{2880}\mathcal{H})T_{bcjk}\Lambda_{\alpha l}\Lambda^{\dot{\beta}j}\gamma_{ad}{}^{\alpha\beta}\gamma_{bc}{}^{\dot{\alpha}}{}_{\dot{\beta}}\nabla_d\Lambda_{\beta m}\varepsilon^{iklm} + (-\frac{59}{3840}\bar{\mathcal{H}} + \frac{19}{1920}\mathcal{H})T_{bcjk}\Lambda_{\alpha l}\Lambda^{\dot{\beta}m}\epsilon^{\alpha\beta}\gamma_{ab}{}^{\dot{\alpha}}{}_{\dot{\beta}}\nabla_c\Lambda_{\beta m}\varepsilon^{ijkl} \\
& + (-\frac{1}{72}\bar{\mathcal{H}} + \frac{1}{72}\mathcal{H})T_{abjk}\Lambda_{\alpha l}\Lambda_{\beta m}\gamma_b{}^{\alpha}{}_{\dot{\beta}}\gamma_c{}^{\dot{\alpha}\beta}\nabla_c\Lambda^{\dot{\beta}j}\varepsilon^{iklm} + (-\frac{1}{72}\mathcal{DDDH} - \frac{1}{30}\mathcal{DI})T_{ab}{}^{jk}T_{cd}{}^{il}\Lambda_{\alpha j}\Lambda_{\beta k}\Lambda_{\gamma l}\gamma_b{}^{\dot{\alpha}\gamma}\gamma_{cd}{}^{\alpha\beta} \\
& + (-\frac{5}{384}\bar{\mathcal{H}} + \frac{13}{768}\mathcal{H})T_{bc}{}^{jk}T_{bc}{}^{lm}\Lambda_{\alpha n}\Lambda^{\dot{\alpha}n}\Lambda^{\dot{\beta}i}\gamma_a{}^{\alpha}{}_{\dot{\beta}}\varepsilon_{jklm} + (-\frac{5}{384}\mathcal{DDH} + \frac{1}{288}\mathcal{I})\Lambda_{\alpha j}\Lambda_{\beta k}\Lambda_{\gamma l}R(V)_{bc}{}^j{}_m\gamma_b{}^{\dot{\alpha}\beta}\gamma_{ac}{}^{\alpha\gamma}\varepsilon^{iklm} \\
& + (-\frac{5}{384}\mathcal{DDH} + \frac{1}{288}\mathcal{I})\Lambda_{\alpha j}\Lambda_{\beta k}\Lambda_{\gamma l}R(V)_{bc}{}^j{}_m\gamma_b{}^{\dot{\alpha}\beta}\gamma_{ac}{}^{\alpha\gamma}\varepsilon^{iklm} + (-\frac{277}{23040}\bar{\mathcal{H}} + \frac{41}{7680}\mathcal{H})T_{bcjk}\Lambda_{\alpha l}\Lambda_{\beta m}\gamma_{ad}{}^{\alpha\beta}\gamma_{bc}{}^{\dot{\alpha}}{}_{\dot{\beta}}\nabla_d\Lambda^{\dot{\beta}i}\varepsilon^{jklm} \\
& + (-\frac{3}{256}\mathcal{DDH} + \frac{1}{32}\mathcal{I})\Lambda_{\alpha j}\Lambda_{\beta k}\Lambda_{\gamma l}R(M)_{abcd}\gamma_b{}^{\dot{\alpha}\alpha}\gamma_{cd}{}^{\beta\gamma}\varepsilon^{ijkl} + (-\frac{127}{11520}\bar{\mathcal{H}} + \frac{13}{3840}\mathcal{H})T_{abjk}\Lambda_{\alpha l}\Lambda^{\dot{\beta}m}\gamma_c{}^{\beta}{}_{\dot{\beta}}\gamma_b{}^{\dot{\alpha}\alpha}\nabla_c\Lambda_{\beta m}\varepsilon^{ijkl} \\
& + (-\frac{1}{96}\mathcal{D}^\dagger\bar{\mathcal{H}} - \frac{1}{12}\mathcal{D}\bar{\mathcal{I}})T_{abjk}T_{bc}{}^{jl}\Lambda_{\alpha l}\Lambda^{\dot{\beta}i}\Lambda^{\dot{\gamma}k}\epsilon_{\dot{\beta}\dot{\gamma}}\gamma_c{}^{\dot{\alpha}\alpha} + (-\frac{1}{96}\mathcal{D}^\dagger\bar{\mathcal{H}} - \frac{1}{12}\mathcal{D}\bar{\mathcal{I}})T_{bcjk}T_{ab}{}^{jl}\Lambda_{\alpha l}\Lambda^{\dot{\beta}i}\Lambda^{\dot{\gamma}k}\epsilon_{\dot{\beta}\dot{\gamma}}\gamma_c{}^{\dot{\alpha}\alpha} \\
& + (-\frac{1}{96}\mathcal{D}^\dagger\bar{\mathcal{H}} + \frac{1}{72}\mathcal{D}\bar{\mathcal{I}})E^{jk}T_{ab}{}^{il}\Lambda_{\alpha j}\Lambda^{\dot{\alpha}m}\Lambda^{\dot{\beta}n}\gamma_b{}^{\alpha}{}_{\dot{\beta}}\varepsilon_{klmn} + (-\frac{1}{96}\mathcal{D}^\dagger\mathcal{I} + \frac{1}{36}\mathcal{DH})P_b\Lambda_{\alpha j}\Lambda_{\beta k}\epsilon^{\alpha\gamma}\gamma_a{}^{\dot{\alpha}\beta}\nabla_b\Lambda_{\gamma l}\varepsilon^{ijkl} \\
& + (-\frac{1}{96}\mathcal{DDDH} + \frac{1}{24}\mathcal{DI})\Lambda_{\alpha j}\Lambda_{\beta k}\bar{P}_b\gamma_a{}^{\dot{\alpha}\alpha}\gamma_{bc}{}^{\beta\gamma}\nabla_c\Lambda_{\gamma l}\varepsilon^{ijkl} + (-\frac{1}{96}\mathcal{DDDH} + \frac{1}{24}\mathcal{DI})\Lambda_{\alpha j}\Lambda_{\beta k}\bar{P}_b\gamma_c{}^{\dot{\alpha}\gamma}\gamma_{ab}{}^{\alpha\beta}\nabla_c\Lambda_{\gamma l}\varepsilon^{ijkl} \\
& + (-\frac{101}{11520}\bar{\mathcal{H}} - \frac{119}{11520}\mathcal{H})T_{abjk}\Lambda_{\alpha l}\Lambda^{\dot{\beta}l}\gamma_c{}^{\beta}{}_{\dot{\beta}}\gamma_b{}^{\dot{\alpha}\alpha}\nabla_c\Lambda_{\beta m}\varepsilon^{ijkm} + (-\frac{5}{576}\mathcal{DDDH} - \frac{11}{720}\mathcal{DI})T_{ab}{}^{ij}T_{cd}{}^{kl}\Lambda_{\alpha j}\Lambda_{\beta k}\Lambda_{\gamma l}\gamma_b{}^{\dot{\alpha}\alpha}\gamma_{cd}{}^{\beta\gamma} \\
& + (-\frac{1}{128}\mathcal{D}^\dagger\bar{\mathcal{H}} + \frac{83}{8640}\mathcal{D}\bar{\mathcal{I}})E_{jk}T_{ablm}\Lambda_{\alpha n}\Lambda^{\dot{\alpha}j}\Lambda^{\dot{\beta}i}\gamma_b{}^{\alpha}{}_{\dot{\beta}}\varepsilon^{klmn} + (-\frac{11}{1440}\bar{\mathcal{H}} - \frac{383}{11520}\mathcal{H})T_{bcjk}\Lambda_{\alpha l}\Lambda^{\dot{\beta}l}\gamma_b{}^{\beta}{}_{\dot{\beta}}\gamma_a{}^{\dot{\alpha}\alpha}\nabla_c\Lambda_{\beta m}\varepsilon^{ijkm} \\
& + (-\frac{17}{2304}\mathcal{DDH} + \frac{5}{288}\mathcal{I})\Lambda_{\alpha j}\Lambda_{\beta k}\Lambda_{\gamma l}R(V)_{bc}{}^i{}_m\gamma_a{}^{\dot{\alpha}\alpha}\gamma_{bc}{}^{\beta\gamma}\varepsilon^{jklm} + (-\frac{1}{144}\bar{\mathcal{H}} - \frac{1}{432}\mathcal{H})P_b\Lambda_{\alpha j}\Lambda_{\beta k}\chi^{\dot{\beta}}{}_{lm}{}^j{}_m\gamma_a{}^{\alpha}{}_{\dot{\beta}}\gamma_b{}^{\dot{\alpha}\beta}\varepsilon^{iklm} \\
& + (-\frac{1}{144}\bar{\mathcal{H}} + \frac{1}{144}\mathcal{H})T_{abjk}\Lambda_{\alpha l}\Lambda_{\beta m}\gamma_b{}^{\alpha}{}_{\dot{\beta}}\gamma_c{}^{\dot{\alpha}\beta}\nabla_c\Lambda^{\dot{\beta}i}\varepsilon^{jklm} + (-\frac{1}{144}\bar{\mathcal{H}} + \frac{1}{144}\mathcal{H})\Lambda_{\alpha j}\Lambda_{\beta k}\Lambda^{\dot{\beta}l}\gamma_b{}^{\alpha}{}_{\dot{\beta}}\gamma_c{}^{\dot{\alpha}\beta}\nabla_cT_{ablm}\varepsilon^{ijkm} \\
& + (-\frac{1}{144}\mathcal{DDH} + \frac{1}{18}\mathcal{I})\Lambda_{\alpha j}\Lambda_{\beta k}\bar{P}_b\chi^{\dot{\beta}}{}_{lm}{}^j{}_m\gamma_a{}^{\alpha}{}_{\dot{\beta}}\gamma_b{}^{\dot{\alpha}\beta}\varepsilon^{iklm} + (-\frac{19}{2880}\bar{\mathcal{H}} + \frac{19}{2880}\mathcal{H})T_{bcjk}\Lambda_{\alpha l}\Lambda_{\beta m}\gamma_a{}^{\alpha}{}_{\dot{\beta}}\gamma_b{}^{\dot{\alpha}\beta}\nabla_c\Lambda^{\dot{\beta}j}\varepsilon^{iklm} \\
& + (-\frac{19}{2880}\mathcal{DDH} + \frac{7}{720}\mathcal{I})T_{bc}{}^{jk}\Lambda_{\alpha j}\Lambda_{\beta k}\Lambda^{\dot{\beta}i}\bar{P}_d\gamma_{bc}{}^{\alpha\beta}\gamma_{ad}{}^{\dot{\alpha}}{}_{\dot{\beta}} + (-\frac{7}{1152}\mathcal{D}^\dagger\bar{\mathcal{H}} - \frac{107}{8640}\mathcal{D}\bar{\mathcal{I}})E_{jk}T_{ablm}\Lambda_{\alpha n}\Lambda^{\dot{\alpha}n}\Lambda^{\dot{\beta}j}\gamma_b{}^{\alpha}{}_{\dot{\beta}}\varepsilon^{iklm} \\
& + (-\frac{67}{11520}\bar{\mathcal{H}} + \frac{157}{11520}\mathcal{H})T_{bcjk}\Lambda_{\alpha l}\Lambda_{\beta m}\gamma_{ad}{}^{\alpha\beta}\gamma_{bc}{}^{\dot{\alpha}}{}_{\dot{\beta}}\nabla_d\Lambda^{\dot{\beta}l}\varepsilon^{ijkm} + (-\frac{11}{1920}\bar{\mathcal{H}} - \frac{1}{192}\mathcal{H})T_{bcjk}\Lambda_{\alpha l}\Lambda^{\dot{\beta}j}\epsilon^{\alpha\beta}\gamma_{ab}{}^{\dot{\alpha}}{}_{\dot{\beta}}\nabla_c\Lambda_{\beta m}\varepsilon^{iklm} \\
& + (-\frac{1}{192}\mathcal{DDDH} - \frac{1}{16}\mathcal{DI})\Lambda_{\alpha j}\Lambda_{\beta k}\bar{P}_b\gamma_b{}^{\dot{\alpha}\alpha}\gamma_{ac}{}^{\beta\gamma}\nabla_c\Lambda_{\gamma l}\varepsilon^{ijkl} + (-\frac{1}{192}\mathcal{DDDH} - \frac{1}{96}\mathcal{DI})\Lambda_{\alpha j}\Lambda_{\beta k}\Lambda_{\gamma l}\gamma_b{}^{\dot{\alpha}\alpha}\gamma_{ac}{}^{\beta\gamma}\nabla_c\bar{P}_b\varepsilon^{ijkl} \\
& + (-\frac{1}{192}\mathcal{DDDH} + \frac{5}{48}\mathcal{DI})\Lambda_{\alpha j}\Lambda_{\beta k}\bar{P}_a\epsilon^{\alpha\gamma}\gamma_b{}^{\dot{\alpha}\beta}\nabla_b\Lambda_{\gamma l}\varepsilon^{ijkl} + (-\frac{1}{288}\bar{\mathcal{H}} + \frac{1}{288}\mathcal{H})T_{abjk}\Lambda_{\alpha l}\Lambda^{\dot{\beta}l}\gamma_b{}^{\beta}{}_{\dot{\beta}}\gamma_c{}^{\dot{\alpha}\alpha}\nabla_c\Lambda_{\beta m}\varepsilon^{ijkm} \\
& + (-\frac{1}{288}\bar{\mathcal{H}} + \frac{1}{288}\mathcal{H})\Lambda_{\alpha j}\Lambda_{\beta k}\Lambda^{\dot{\beta}i}\gamma_b{}^{\alpha}{}_{\dot{\beta}}\gamma_c{}^{\dot{\alpha}\beta}\nabla_cT_{ablm}\varepsilon^{ijkm} + (-\frac{1}{288}\mathcal{D}^\dagger\bar{\mathcal{H}} - \frac{1}{48}\mathcal{D}\bar{\mathcal{I}})E^{ij}T_{ab}{}^{kl}\Lambda_{\alpha k}\Lambda^{\dot{\alpha}m}\Lambda^{\dot{\beta}n}\gamma_b{}^{\alpha}{}_{\dot{\beta}}\varepsilon_{jlmn} \\
& + (-\frac{1}{288}\mathcal{D}^\dagger\mathcal{I} - \frac{1}{144}\mathcal{DH})E^{ij}E^{kl}\Lambda_{\alpha j}\Lambda_{\beta k}\Lambda_{\gamma l}\epsilon^{\beta\gamma}\gamma_a{}^{\dot{\alpha}\alpha} + (-\frac{1}{288}\mathcal{DDH} + \frac{1}{12}\mathcal{I})\Lambda_{\alpha j}\Lambda_{\beta k}\bar{P}_b\chi^{\dot{\beta}}{}_{lm}{}^j{}_m\gamma_a{}^{\alpha}{}_{\dot{\beta}}\gamma_b{}^{\dot{\alpha}\beta}\varepsilon^{iklm} \\
& + (-\frac{1}{384}\bar{\mathcal{H}} - \frac{7}{384}\mathcal{H})\Lambda_{\alpha j}R(Q)_{bc}{}^{\dot{\alpha}}{}_kR(Q)_{de}{}^{\dot{\beta}}{}_l\gamma_a{}^{\alpha}{}_{\dot{\gamma}}\gamma_{bc\dot{\beta}\dot{\gamma}}\gamma_{de}{}^{\dot{\gamma}\delta}\varepsilon^{ijkl} + (-\frac{11}{5760}\bar{\mathcal{H}} - \frac{79}{5760}\mathcal{H})T_{abjk}\Lambda_{\alpha l}\Lambda_{\beta m}\gamma_c{}^{\alpha}{}_{\dot{\beta}}\gamma_b{}^{\dot{\alpha}\beta}\nabla_c\Lambda^{\dot{\beta}l}\varepsilon^{ijkm} \\
& + (-\frac{1}{576}\bar{\mathcal{H}} - \frac{37}{960}\mathcal{H})T_{abjk}\Lambda_{\alpha l}\Lambda_{\beta m}\epsilon^{\alpha\beta}\gamma_{bc}{}^{\dot{\alpha}}{}_{\dot{\beta}}\nabla_c\Lambda^{\dot{\beta}l}\varepsilon^{ijkm} + (-\frac{1}{576}\mathcal{D}^\dagger\bar{\mathcal{H}} - \frac{7}{4320}\mathcal{D}\bar{\mathcal{I}})E_{jk}T_{ablm}\Lambda_{\alpha n}\Lambda^{\dot{\alpha}j}\Lambda^{\dot{\beta}l}\gamma_b{}^{\alpha}{}_{\dot{\beta}}\varepsilon^{ikmn} \\
& + (-\frac{1}{576}\mathcal{D}^\dagger\mathcal{I} + \frac{1}{144}\mathcal{DH})\Lambda_{\alpha j}\Lambda_{\beta k}\Lambda^{\dot{\beta}l}\gamma_a{}^{\alpha}{}_{\dot{\beta}}\gamma_b{}^{\dot{\alpha}\beta}\nabla_bE_{lm}\varepsilon^{ijkm} + (-\frac{1}{576}\mathcal{D}^\dagger\mathcal{I} + \frac{1}{144}\mathcal{DH})\Lambda_{\alpha j}\Lambda_{\beta k}\Lambda^{\dot{\beta}l}\gamma_b{}^{\alpha}{}_{\dot{\beta}}\gamma_a{}^{\dot{\alpha}\beta}\nabla_bE_{lm}\varepsilon^{ijkm} \\
& + (-\frac{1}{576}\mathcal{DDH} + \frac{17}{72}\mathcal{I})T_{bc}{}^{ij}\Lambda_{\alpha j}\Lambda_{\beta k}\Lambda^{\dot{\beta}k}\bar{P}_d\gamma_{bc}{}^{\alpha\beta}\gamma_{ad}{}^{\dot{\alpha}}{}_{\dot{\beta}} + (-\frac{1}{1280}\bar{\mathcal{H}} + \frac{37}{1920}\mathcal{H})T_{abjk}\Lambda_{\alpha l}\Lambda^{\dot{\beta}l}\epsilon^{\alpha\beta}\gamma_{bc}{}^{\dot{\alpha}}{}_{\dot{\beta}}\nabla_c\Lambda_{\beta m}\varepsilon^{ijkm} \\
& + (-\frac{1}{2880}\bar{\mathcal{H}} + \frac{49}{2880}\mathcal{H})\Lambda_{\alpha j}\Lambda_{\beta k}\Lambda^{\dot{\beta}l}\gamma_{ab}{}^{\alpha\beta}\gamma_{cd}{}^{\dot{\alpha}}{}_{\dot{\beta}}\nabla_bT_{cdlm}\varepsilon^{ijkm} + (-\frac{1}{5760}\bar{\mathcal{H}} + \frac{1}{5760}\mathcal{H})T_{bcjk}\Lambda_{\alpha l}\Lambda_{\beta m}\gamma_a{}^{\alpha}{}_{\dot{\beta}}\gamma_b{}^{\dot{\alpha}\beta}\nabla_c\Lambda^{\dot{\beta}i}\varepsilon^{jklm} \\
& + (\frac{1}{1280}\bar{\mathcal{H}} - \frac{37}{1920}\mathcal{H})T_{bcjk}\Lambda_{\alpha l}\Lambda^{\dot{\beta}l}\epsilon^{\alpha\beta}\gamma_{ab}{}^{\dot{\alpha}}{}_{\dot{\beta}}\nabla_c\Lambda_{\beta m}\varepsilon^{ijkm} + (\frac{1}{864}\bar{\mathcal{H}} + \frac{1}{288}\mathcal{H})E_{jk}E_{lm}\Lambda_{\alpha n}\Lambda^{\dot{\alpha}j}\Lambda^{\dot{\beta}l}\gamma_a{}^{\alpha}{}_{\dot{\beta}}\varepsilon^{ikmn} \\
& + (\frac{1}{576}\mathcal{D}^\dagger\bar{\mathcal{H}} + \frac{7}{4320}\mathcal{D}\bar{\mathcal{I}})E_{jk}T_{ablm}\Lambda_{\alpha n}\Lambda^{\dot{\alpha}l}\Lambda^{\dot{\beta}j}\gamma_b{}^{\alpha}{}_{\dot{\beta}}\varepsilon^{ikmn} + (\frac{11}{5760}\bar{\mathcal{H}} + \frac{79}{5760}\mathcal{H})T_{abjk}\Lambda_{\alpha l}\Lambda_{\beta m}\gamma_c{}^{\alpha}{}_{\dot{\beta}}\gamma_b{}^{\dot{\alpha}\beta}\nabla_c\Lambda^{\dot{\beta}m}\varepsilon^{ijkl} \\
& + (\frac{1}{384}\mathcal{D}^\dagger\mathcal{I} + \frac{1}{144}\mathcal{DH})E_{jk}\Lambda_{\alpha l}\Lambda^{\dot{\beta}j}\gamma_b{}^{\beta}{}_{\dot{\beta}}\gamma_a{}^{\dot{\alpha}\alpha}\nabla_b\Lambda_{\beta m}\varepsilon^{iklm} + (\frac{1}{360}\mathcal{D}^\dagger\bar{\mathcal{H}} + \frac{19}{576}\mathcal{D}\bar{\mathcal{I}})E^{ij}P_b\Lambda_{\alpha j}\Lambda_{\beta k}\Lambda^{\dot{\beta}k}\gamma_b{}^{\alpha}{}_{\dot{\beta}}\gamma_a{}^{\dot{\alpha}\beta} \\
& + (\frac{1}{360}\mathcal{D}^\dagger\bar{\mathcal{H}} + \frac{19}{576}\mathcal{D}\bar{\mathcal{I}})E^{ij}P_b\Lambda_{\alpha j}\Lambda_{\beta k}\Lambda^{\dot{\beta}k}\gamma_b{}^{\beta}{}_{\dot{\beta}}\gamma_a{}^{\dot{\alpha}\alpha} + (\frac{1}{288}\bar{\mathcal{H}} - \frac{1}{288}\mathcal{H})T_{abjk}\Lambda_{\alpha l}\Lambda^{\dot{\beta}i}\gamma_b{}^{\beta}{}_{\dot{\beta}}\gamma_c{}^{\dot{\alpha}\alpha}\nabla_c\Lambda_{\beta m}\varepsilon^{jklm} + 14\cdots
\end{aligned}$$

$$\begin{aligned}
[\hat{\Omega}_a^{\dot{\alpha}i}]_{3,cont.} = & + \left( \frac{1}{288} \bar{\mathcal{H}} - \frac{1}{288} \mathcal{H} \right) \Lambda_{\alpha j} \Lambda_{\beta k} \Lambda^{\dot{\beta}j} \gamma_b^{\alpha} \dot{\beta} \gamma_c^{\dot{\alpha}\beta} \nabla_c T_{ablm} \varepsilon^{iklm} + \left( \frac{1}{288} \bar{\mathcal{H}} - \frac{1}{288} \mathcal{H} \right) \Lambda_{\alpha j} \Lambda_{\beta k} \Lambda^{\dot{\beta}j} \gamma_b^{\beta} \dot{\beta} \gamma_c^{\dot{\alpha}\alpha} \nabla_c T_{ablm} \varepsilon^{iklm} \\
& + \left( \frac{1}{288} \mathcal{D}^\dagger \mathcal{I} + \frac{1}{144} \mathcal{D} \mathcal{H} \right) E^{ij} E^{kl} \Lambda_{\alpha j} \Lambda_{\beta k} \Lambda_{\gamma l} \epsilon^{\alpha\beta} \gamma_a^{\dot{\alpha}\gamma} + \left( \frac{1}{288} \mathcal{D} \mathcal{D} \mathcal{H} + \frac{1}{12} \mathcal{I} \right) \Lambda_{\alpha j} \Lambda_{\beta k} \bar{P}_b \chi^{\dot{\beta}}_{lm} \dot{\gamma}_b^{\alpha} \dot{\beta} \gamma_a^{\dot{\alpha}\beta} \varepsilon^{jklm} \\
& + \left( \frac{1}{240} \bar{\mathcal{H}} - \frac{1}{240} \mathcal{H} \right) T_{abjk} \Lambda_{\alpha l} \Lambda^{\dot{\beta}j} \gamma_c^{\alpha} \dot{\beta} \gamma_b^{\dot{\alpha}\beta} \nabla_c \Lambda_{\beta m} \varepsilon^{iklm} + \left( \frac{5}{1152} \mathcal{D}^\dagger \mathcal{I} - \frac{1}{16} \mathcal{D} \mathcal{H} \right) E_{jk} \Lambda_{\alpha l} \Lambda^{\dot{\beta}j} \gamma_b^{\alpha} \dot{\beta} \gamma_a^{\dot{\alpha}\beta} \nabla_b \Lambda_{\beta m} \varepsilon^{iklm} \\
& + \left( \frac{5}{1152} \mathcal{D} \mathcal{D} \mathcal{H} - \frac{1}{144} \mathcal{I} \right) \Lambda_{\alpha j} \Lambda_{\beta k} \Lambda_{\gamma l} R(V)_{bc}{}^i{}_m \gamma_b^{\dot{\alpha}\alpha} \gamma_{ac}{}^{\beta\gamma} \varepsilon^{jklm} + \left( \frac{1}{192} \mathcal{D} \mathcal{D} \mathcal{D} \mathcal{H} + \frac{1}{16} \mathcal{D} \mathcal{I} \right) \Lambda_{\alpha j} \Lambda_{\beta k} \bar{P}_b \epsilon^{\alpha\gamma} \gamma_b^{\dot{\alpha}\beta} \nabla_a \Lambda_{\gamma l} \varepsilon^{ijkl} \\
& + \left( \frac{11}{1920} \bar{\mathcal{H}} + \frac{1}{192} \mathcal{H} \right) T_{abjk} \Lambda_{\alpha l} \Lambda^{\dot{\beta}j} \epsilon^{\alpha\beta} \gamma_{bc}{}^{\dot{\alpha}} \dot{\beta} \nabla_c \Lambda_{\beta m} \varepsilon^{iklm} + \left( \frac{7}{1152} \mathcal{D}^\dagger \bar{\mathcal{H}} + \frac{107}{8640} \mathcal{D} \bar{\mathcal{I}} \right) E_{jk} T_{ablm} \Lambda_{\alpha n} \Lambda^{\dot{\alpha}j} \Lambda^{\dot{\beta}n} \gamma_b^{\alpha} \dot{\beta} \varepsilon^{iklm} \\
& + \left( \frac{1}{160} \bar{\mathcal{H}} + \frac{11}{240} \mathcal{H} \right) T_{bcjk} \Lambda_{\alpha l} \Lambda^{\dot{\beta}i} \gamma_a^{\beta} \dot{\beta} \gamma_b^{\dot{\alpha}\alpha} \nabla_c \Lambda_{\beta m} \varepsilon^{jklm} + \left( \frac{1}{144} \bar{\mathcal{H}} - \frac{1}{144} \mathcal{H} \right) T_{abjk} \Lambda_{\alpha l} \Lambda^{\dot{\beta}j} \gamma_b^{\beta} \dot{\beta} \gamma_c^{\dot{\alpha}\alpha} \nabla_c \Lambda_{\beta m} \varepsilon^{iklm} \\
& + \left( \frac{1}{144} \mathcal{D}^\dagger \mathcal{I} + \frac{1}{192} \mathcal{D} \mathcal{H} \right) \Lambda_{\alpha j} \Lambda_{\beta k} \Lambda_{\gamma l} \gamma_b^{\dot{\alpha}\alpha} \gamma_{ac}{}^{\beta\gamma} \nabla_b P_c \varepsilon^{ijkl} + \left( \frac{1}{144} \mathcal{D}^\dagger \mathcal{I} + \frac{13}{576} \mathcal{D} \mathcal{H} \right) \Lambda_{\alpha j} \Lambda_{\beta k} \Lambda_{\gamma l} \gamma_a^{\dot{\alpha}\alpha} \gamma_{bc}{}^{\beta\gamma} \nabla_b P_c \varepsilon^{ijkl} \\
& + \left( \frac{1}{144} \mathcal{D} \mathcal{D} \mathcal{H} - \frac{1}{18} \mathcal{I} \right) \Lambda_{\alpha j} \Lambda_{\beta k} \bar{P}_b \chi^{\dot{\beta}}_{lm} \dot{\gamma}_a^{\alpha} \dot{\beta} \gamma_b^{\dot{\alpha}\beta} \varepsilon^{jklm} + \left( \frac{1}{144} \mathcal{D} \mathcal{D} \mathcal{H} + \frac{1}{18} \mathcal{I} \right) E_{jk} \Lambda_{\alpha l} \Lambda_{\beta m} \Lambda^{\dot{\alpha}j} \bar{P}_b \gamma_{ab}{}^{\alpha\beta} \varepsilon^{iklm} \\
& + \left( \frac{1}{128} \mathcal{D}^\dagger \bar{\mathcal{H}} - \frac{83}{8640} \mathcal{D} \bar{\mathcal{I}} \right) E_{jk} T_{ablm} \Lambda_{\alpha n} \Lambda^{\dot{\alpha}i} \Lambda^{\dot{\beta}j} \gamma_b^{\alpha} \dot{\beta} \varepsilon^{klmn} + \left( \frac{5}{576} \mathcal{D}^\dagger \mathcal{I} + \frac{1}{72} \mathcal{D} \mathcal{H} \right) E_{jk} \Lambda_{\alpha l} \Lambda_{\beta m} \gamma_b^{\alpha} \dot{\beta} \gamma_a^{\dot{\alpha}\beta} \nabla_b \Lambda^{\dot{\beta}j} \varepsilon^{iklm} \\
& + \left( \frac{1}{96} \mathcal{D}^\dagger \mathcal{I} + \frac{1}{240} \mathcal{D} \mathcal{H} \right) \Lambda_{\alpha j} R(Q)_{bc\beta}{}^i R(Q)_{de\gamma}{}^j \epsilon^{\alpha\gamma} \gamma_a^{\dot{\alpha}\delta} \gamma_{bc\delta\epsilon} \gamma_{de}{}^{\beta\epsilon} + \left( \frac{1}{96} \mathcal{D}^\dagger \mathcal{I} + \frac{1}{144} \mathcal{D} \mathcal{H} \right) E_{jk} \Lambda_{\alpha l} \Lambda^{\dot{\beta}j} \gamma_a^{\alpha} \dot{\beta} \gamma_b^{\dot{\alpha}\beta} \nabla_b \Lambda_{\beta m} \varepsilon^{iklm} \\
& + \left( \frac{13}{1152} \bar{\mathcal{H}} + \frac{31}{5760} \mathcal{H} \right) \Lambda_{\alpha j} \Lambda_{\beta k} \Lambda^{\dot{\beta}i} \gamma_{ab}{}^{\alpha\beta} \gamma_{cd}{}^{\dot{\alpha}} \dot{\beta} \nabla_b T_{cdlm} \varepsilon^{jklm} + \left( \frac{5}{432} \bar{\mathcal{H}} - \frac{5}{432} \mathcal{H} \right) E_{jk} P_b \Lambda_{\alpha l} \Lambda_{\beta m} \Lambda^{\dot{\alpha}j} \gamma_{ab}{}^{\alpha\beta} \varepsilon^{iklm} \\
& + \left( \frac{7}{576} \mathcal{D} \mathcal{D} \mathcal{D} \mathcal{H} + \frac{1}{720} \mathcal{D} \mathcal{I} \right) T_{bc}{}^{ij} T_{bd}{}^{kl} \Lambda_{\alpha j} \Lambda_{\beta k} \Lambda_{\gamma l} \gamma_a^{\dot{\alpha}\alpha} \gamma_{cd}{}^{\beta\gamma} + \left( \frac{149}{11520} \bar{\mathcal{H}} - \frac{1}{11520} \mathcal{H} \right) T_{abjk} \Lambda_{\alpha l} \Lambda^{\dot{\beta}i} \gamma_c^{\beta} \dot{\beta} \gamma_b^{\dot{\alpha}\alpha} \nabla_c \Lambda_{\beta m} \varepsilon^{jklm} \\
& + \left( \frac{5}{384} \bar{\mathcal{H}} - \frac{13}{768} \mathcal{H} \right) T_{bc}{}^{jk} T_{bc}{}^{lm} \Lambda_{\alpha n} \Lambda^{\dot{\alpha}i} \Lambda^{\dot{\beta}n} \gamma_a^{\alpha} \dot{\beta} \varepsilon_{ijklm} + \left( \frac{5}{384} \mathcal{D} \mathcal{D} \mathcal{H} - \frac{1}{288} \mathcal{I} \right) \Lambda_{\alpha j} \Lambda_{\beta k} \Lambda_{\gamma l} R(V)_{bc}{}^j{}_m \gamma_a^{\dot{\alpha}\beta} \gamma_{bc}{}^{\alpha\gamma} \varepsilon^{iklm} \\
& + \left( \frac{5}{384} \mathcal{D} \mathcal{D} \mathcal{H} - \frac{1}{288} \mathcal{I} \right) \Lambda_{\alpha j} \Lambda_{\beta k} \Lambda_{\gamma l} R(V)_{bc}{}^j{}_m \gamma_b^{\dot{\alpha}\alpha} \gamma_{ac}{}^{\beta\gamma} \varepsilon^{iklm} + \left( \frac{1}{72} \bar{\mathcal{H}} - \frac{1}{216} \mathcal{H} \right) P_b \Lambda_{\alpha j} \Lambda_{\beta k} \chi^{\dot{\beta}}_{lm} \dot{\gamma}_a^{\alpha} \dot{\beta} \gamma_b^{\dot{\alpha}\beta} \varepsilon^{jklm} \\
& + \left( \frac{1}{72} \mathcal{D}^\dagger \bar{\mathcal{H}} - \frac{1}{72} \mathcal{D} \bar{\mathcal{I}} \right) E^{ij} P_b \Lambda_{\alpha j} \Lambda_{\beta k} \Lambda^{\dot{\beta}k} \gamma_a^{\alpha} \dot{\beta} \gamma_b^{\dot{\alpha}\beta} + \left( \frac{1}{72} \mathcal{D}^\dagger \bar{\mathcal{H}} - \frac{1}{72} \mathcal{D} \bar{\mathcal{I}} \right) E^{ij} P_b \Lambda_{\alpha j} \Lambda_{\beta k} \Lambda^{\dot{\beta}k} \gamma_a^{\beta} \dot{\beta} \gamma_b^{\dot{\alpha}\alpha} \\
& + \left( \frac{1}{72} \mathcal{D}^\dagger \bar{\mathcal{H}} + \frac{5}{144} \mathcal{D} \bar{\mathcal{I}} \right) E^{jk} P_b \Lambda_{\alpha j} \Lambda_{\beta k} \Lambda^{\dot{\beta}i} \epsilon^{\alpha\beta} \gamma_{ab}{}^{\dot{\alpha}} \dot{\beta} + \left( \frac{1}{72} \mathcal{D} \mathcal{D} \mathcal{H} - \frac{1}{9} \mathcal{I} \right) \Lambda_{\alpha j} \Lambda_{\beta k} \bar{P}_b \chi^{\dot{\beta}}_{lm} \dot{\gamma}_a^{\beta} \dot{\beta} \gamma_b^{\dot{\alpha}\alpha} \varepsilon^{iklm} \\
& + \left( \frac{59}{3840} \bar{\mathcal{H}} - \frac{19}{1920} \mathcal{H} \right) T_{abjk} \Lambda_{\alpha l} \Lambda^{\dot{\beta}m} \epsilon^{\alpha\beta} \gamma_{bc}{}^{\dot{\alpha}} \dot{\beta} \nabla_c \Lambda_{\beta m} \varepsilon^{ijkl} + \left( \frac{1}{64} \bar{\mathcal{H}} - \frac{1}{64} \mathcal{H} \right) T_{ab}{}^{ij} T_{bc}{}^{kl} \Lambda_{\alpha m} \Lambda^{\dot{\alpha}m} \Lambda^{\dot{\beta}n} \gamma_c^{\alpha} \dot{\beta} \varepsilon_{jklm} \\
& + \left( \frac{1}{64} \bar{\mathcal{H}} - \frac{1}{64} \mathcal{H} \right) T_{ab}{}^{jk} T_{bc}{}^{il} \Lambda_{\alpha m} \Lambda^{\dot{\alpha}n} \Lambda^{\dot{\beta}m} \gamma_c^{\alpha} \dot{\beta} \varepsilon_{jklm} + \left( \frac{1}{64} \bar{\mathcal{H}} + \frac{1}{192} \mathcal{H} \right) T_{ab}{}^{ij} T_{bc}{}^{kl} \Lambda_{\alpha j} \Lambda^{\dot{\alpha}m} \Lambda^{\dot{\beta}n} \gamma_c^{\alpha} \dot{\beta} \varepsilon_{klmn} \\
& + \left( \frac{1}{64} \bar{\mathcal{H}} + \frac{1}{192} \mathcal{H} \right) T_{ab}{}^{jk} T_{bc}{}^{il} \Lambda_{\alpha l} \Lambda^{\dot{\alpha}m} \Lambda^{\dot{\beta}n} \gamma_c^{\alpha} \dot{\beta} \varepsilon_{jkmn} + \left( \frac{1}{64} \bar{\mathcal{H}} + \frac{1}{64} \mathcal{H} \right) T_{ab}{}^{jk} T_{bc}{}^{lm} \Lambda_{\alpha j} \Lambda^{\dot{\alpha}n} \Lambda^{\dot{\beta}i} \gamma_c^{\alpha} \dot{\beta} \varepsilon_{klmn} \\
& + \left( \frac{1}{64} \bar{\mathcal{H}} + \frac{1}{64} \mathcal{H} \right) T_{ab}{}^{jk} T_{bc}{}^{lm} \Lambda_{\alpha l} \Lambda^{\dot{\alpha}i} \Lambda^{\dot{\beta}n} \gamma_c^{\alpha} \dot{\beta} \varepsilon_{jkmn} + \left( \frac{1}{64} \mathcal{D} \mathcal{D} \mathcal{H} + \frac{1}{24} \mathcal{I} \right) D^{ij}{}_{kl} \Lambda_{\alpha j} \Lambda_{\beta m} \Lambda_{\gamma n} \epsilon^{\alpha\beta} \gamma_a^{\dot{\alpha}\gamma} \varepsilon^{klmn} \\
& + \left( \frac{13}{768} \bar{\mathcal{H}} - \frac{49}{3840} \mathcal{H} \right) T_{bcjk} \Lambda_{\alpha l} \Lambda_{\beta m} \epsilon^{\alpha\beta} \gamma_{bc}{}^{\dot{\alpha}} \dot{\beta} \nabla_a \Lambda^{\dot{\beta}i} \varepsilon^{ijkm} + \left( \frac{5}{288} \mathcal{D}^\dagger \bar{\mathcal{H}} - \frac{1}{144} \mathcal{D} \bar{\mathcal{I}} \right) E_{jk} E^{jl} \Lambda_{\alpha l} \Lambda^{\dot{\beta}i} \Lambda^{\dot{\gamma}k} \epsilon_{\dot{\beta}\dot{\gamma}} \gamma_a^{\dot{\alpha}\alpha} \\
& + \left( \frac{17}{960} \mathcal{D} \mathcal{D} \mathcal{H} + \frac{1}{60} \mathcal{I} \right) E_{jk} \Lambda_{\alpha l} \Lambda_{\beta m} \chi_{\gamma}{}^{jl}{}_n \epsilon^{\beta\gamma} \gamma_a^{\dot{\alpha}\alpha} \varepsilon^{ikmn} + \left( \frac{13}{720} \bar{\mathcal{I}} - \frac{5}{576} \mathcal{D}^\dagger \mathcal{D}^\dagger \bar{\mathcal{H}} \right) T_{abjk} T_{bclm} \Lambda_{\alpha n} \Lambda^{\dot{\alpha}j} \Lambda^{\dot{\beta}k} \gamma_c^{\alpha} \dot{\beta} \varepsilon^{ilmn} \\
& + \left( \frac{13}{720} \bar{\mathcal{I}} - \frac{5}{576} \mathcal{D}^\dagger \mathcal{D}^\dagger \bar{\mathcal{H}} \right) T_{abjk} T_{bclm} \Lambda_{\alpha n} \Lambda^{\dot{\alpha}l} \Lambda^{\dot{\beta}m} \gamma_c^{\alpha} \dot{\beta} \varepsilon^{ijkn} + \left( \frac{7}{384} \mathcal{D} \mathcal{D} \mathcal{H} + \frac{11}{96} \mathcal{I} \right) \Lambda_{\alpha j} \Lambda_{\beta k} \Lambda_{\gamma l} R(V)_{ab}{}^j{}_m \epsilon^{\alpha\beta} \gamma_b^{\dot{\alpha}\gamma} \varepsilon^{iklm} \\
& + \left( \frac{1}{54} \bar{\mathcal{H}} + \frac{1}{54} \mathcal{H} \right) P_b \Lambda_{\alpha j} \Lambda_{\beta k} \chi^{\dot{\beta}}_{lm} \dot{\gamma}_a^{\alpha} \dot{\beta} \gamma_b^{\dot{\alpha}\beta} \varepsilon^{jklm} + \left( \frac{1}{54} \mathcal{D}^\dagger \bar{\mathcal{I}} - \frac{1}{144} \mathcal{D}^\dagger \mathcal{D}^\dagger \mathcal{D}^\dagger \bar{\mathcal{H}} \right) E_{jk} P_b \Lambda^{\dot{\beta}i} \Lambda^{\dot{\gamma}j} \Lambda^{\dot{\delta}k} \epsilon_{\dot{\beta}\dot{\gamma}} \gamma_{ab}{}^{\dot{\alpha}} \dot{\delta} \\
& + \left( \frac{1}{48} \bar{\mathcal{H}} - \frac{1}{432} \mathcal{H} \right) P_b \Lambda_{\alpha j} \Lambda_{\beta k} \chi^{\dot{\beta}}_{lm} \dot{\gamma}_a^{\beta} \dot{\beta} \gamma_b^{\dot{\alpha}\alpha} \varepsilon^{iklm} + \left( \frac{1}{48} \mathcal{D}^\dagger \bar{\mathcal{H}} + \frac{1}{12} \mathcal{D} \bar{\mathcal{I}} \right) T_{bcjk} \Lambda_{\alpha l} \Lambda^{\dot{\beta}l} \chi^{\dot{\gamma}}{}_{mn} \dot{\gamma}_a^{\dot{\alpha}\alpha} \gamma_{bc\dot{\beta}\dot{\gamma}} \varepsilon^{jkmn} \\
& + \left( \frac{1}{48} \mathcal{D} \mathcal{D} \mathcal{H} + \frac{1}{18} \mathcal{I} \right) E^{jk} T_{ab}{}^{il} \Lambda_{\alpha j} \Lambda_{\beta k} \Lambda_{\gamma l} \epsilon^{\alpha\beta} \gamma_b^{\dot{\alpha}\gamma} + \left( \frac{1}{48} \mathcal{D} \mathcal{D} \mathcal{H} + \frac{1}{18} \mathcal{I} \right) E^{jk} T_{ab}{}^{il} \Lambda_{\alpha j} \Lambda_{\beta k} \Lambda_{\gamma l} \epsilon^{\alpha\gamma} \gamma_b^{\dot{\alpha}\beta} \\
& + \left( \frac{3}{128} \mathcal{D}^\dagger \bar{\mathcal{H}} - \frac{1}{192} \mathcal{D} \bar{\mathcal{I}} \right) E_{jk} E^{jk} \Lambda_{\alpha l} \Lambda^{\dot{\beta}i} \Lambda^{\dot{\gamma}l} \epsilon_{\dot{\beta}\dot{\gamma}} \gamma_a^{\dot{\alpha}\alpha} + \left( \frac{139}{5760} \bar{\mathcal{H}} - \frac{19}{5760} \mathcal{H} \right) T_{abjk} \Lambda_{\alpha l} \Lambda^{\dot{\beta}j} \gamma_c^{\beta} \dot{\beta} \gamma_b^{\dot{\alpha}\alpha} \nabla_c \Lambda_{\beta m} \varepsilon^{iklm} \\
& + \left( \frac{559}{23040} \bar{\mathcal{H}} + \frac{49}{5760} \mathcal{H} \right) T_{bcjk} \Lambda_{\alpha l} \Lambda^{\dot{\beta}l} \gamma_{ad}{}^{\alpha\beta} \gamma_{bc}{}^{\dot{\alpha}} \dot{\beta} \nabla_d \Lambda_{\beta m} \varepsilon^{ijkm} + \left( \frac{7}{288} \mathcal{D} \mathcal{D} \mathcal{D} \mathcal{H} + \frac{1}{360} \mathcal{D} \mathcal{I} \right) T_{bc}{}^{ij} T_{bd}{}^{kl} \Lambda_{\alpha j} \Lambda_{\beta k} \Lambda_{\gamma l} \gamma_a^{\dot{\alpha}\beta} \gamma_{cd}{}^{\alpha\gamma} \\
& + \left( \frac{19}{768} \bar{\mathcal{H}} - \frac{13}{640} \mathcal{H} \right) T_{abjk} \Lambda_{\alpha l} \Lambda^{\dot{\beta}i} \epsilon^{\alpha\beta} \gamma_{bc}{}^{\dot{\alpha}} \dot{\beta} \nabla_c \Lambda_{\beta m} \varepsilon^{jklm} + \left( \frac{5}{192} \mathcal{D}^\dagger \mathcal{I} - \frac{7}{480} \mathcal{D} \mathcal{H} \right) \Lambda_{\alpha j} R(Q)_{bc\beta}{}^i R(Q)_{de\gamma}{}^j \epsilon^{\alpha\beta} \gamma_a^{\dot{\alpha}\delta} \gamma_{de\delta\epsilon} \gamma_{bc}{}^{\alpha\gamma} \\
& + \left( \frac{31}{1152} \bar{\mathcal{H}} - \frac{1}{5760} \mathcal{H} \right) T_{abjk} \Lambda_{\alpha l} \Lambda_{\beta m} \gamma_c^{\alpha} \dot{\beta} \gamma_b^{\dot{\alpha}\beta} \nabla_c \Lambda^{\dot{\beta}i} \varepsilon^{jklm} + \left( \frac{1}{36} \bar{\mathcal{I}} - \frac{1}{48} \mathcal{D}^\dagger \mathcal{D}^\dagger \bar{\mathcal{H}} \right) T_{abjk} T_{bclm} \Lambda_{\alpha n} \Lambda^{\dot{\alpha}j} \Lambda^{\dot{\beta}n} \gamma_c^{\alpha} \dot{\beta} \varepsilon^{iklm} + 15 \dots
\end{aligned}$$

$$\begin{aligned} [\bar{\Omega}_a^{\dot{\alpha}i}]_{3,cont.} = & + (\frac{1}{36} \bar{\mathcal{I}} - \frac{1}{48} \mathcal{D}^\dagger \mathcal{D}^\dagger \bar{\mathcal{H}}) T_{abjk} T_{bclm} \Lambda_{\alpha n} \Lambda^{\dot{\alpha} n} \Lambda^{\dot{\beta} l} \gamma_c^\alpha \epsilon^{\dot{\beta} ijk m} + (\frac{1}{36} \bar{\mathcal{I}} + \frac{1}{144} \mathcal{D}^\dagger \mathcal{D}^\dagger \bar{\mathcal{H}}) E^{ij} T_{bckl} \Lambda_{\alpha j} \Lambda^{\dot{\beta} k} \Lambda^{\dot{\gamma} l} \gamma_a^\alpha \epsilon^{\dot{\beta} \gamma bc \dot{\alpha} \dot{\gamma}} \\ & + (\frac{1}{36} \bar{\mathcal{I}} + \frac{1}{72} \mathcal{D}^\dagger \mathcal{D}^\dagger \bar{\mathcal{H}}) E^{ij} T_{bckl} \Lambda_{\alpha j} \Lambda^{\dot{\beta} k} \Lambda^{\dot{\gamma} l} \gamma_a^{\dot{\alpha} \alpha} \gamma_{bc \dot{\beta} \dot{\gamma}} + (\frac{1}{36} \bar{\mathcal{I}} + \frac{1}{72} \mathcal{D}^\dagger \mathcal{D}^\dagger \bar{\mathcal{H}}) T_{ab}{}^{jk} \Lambda^{\dot{\beta} i} \Lambda^{\dot{\gamma} l} \epsilon_{\dot{\beta} \dot{\gamma}} \gamma_{bc}{}^{\dot{\alpha}}{}_{\dot{\delta}} \nabla_c \Lambda^{\dot{\delta} m} \epsilon_{jklm} \\ & + (\frac{1}{36} \mathcal{D}^\dagger \bar{\mathcal{H}} + \frac{1}{60} \mathcal{D} \bar{\mathcal{I}}) P_b T_{bcjk} \Lambda_{\alpha l} \Lambda_{\beta m} \Lambda^{\dot{\alpha} j} \gamma_{ac}{}^{\alpha \beta} \epsilon^{iklm} + (\frac{1}{36} \mathcal{D}^\dagger \mathcal{D}^\dagger \bar{\mathcal{I}} - \frac{1}{576} \mathcal{D}^\dagger \mathcal{D}^\dagger \mathcal{D}^\dagger \bar{\mathcal{H}}) P_b T_{cdjk} \Lambda^{\dot{\beta} i} \Lambda^{\dot{\gamma} j} \Lambda^{\dot{\delta} k} \gamma_{cd \dot{\gamma} \dot{\delta}} \gamma_{ab}{}^{\dot{\alpha}}{}_{\dot{\beta}} \\ & + (\frac{83}{2880} \bar{\mathcal{H}} - \frac{203}{11520} \mathcal{H}) \Lambda_{\alpha j} \Lambda_{\beta k} \Lambda^{\dot{\beta} j} \epsilon^{\alpha \beta} \gamma_{bc}{}^{\dot{\alpha}}{}_{\dot{\beta}} \nabla_a T_{bclm} \epsilon^{iklm} + (\frac{17}{576} \mathcal{D}^\dagger \bar{\mathcal{H}} + \frac{1}{72} \mathcal{D} \bar{\mathcal{I}}) E^{jk} T_{ab}{}^{lm} \Lambda_{\alpha j} \Lambda^{\dot{\alpha} i} \Lambda^{\dot{\beta} n} \gamma_b{}^\alpha \epsilon_{iklmn} \\ & + (\frac{41}{1152} \bar{\mathcal{H}} + \frac{5}{384} \mathcal{H}) T_{abjk} \Lambda_{\alpha l} \Lambda_{\beta m} \gamma_b{}^\alpha \epsilon_{\dot{\beta} \dot{\gamma} c} \dot{\alpha} \dot{\beta} \nabla_c \Lambda^{\dot{\delta} m} \epsilon^{ijkl} + (\frac{41}{1152} \bar{\mathcal{H}} + \frac{5}{384} \mathcal{H}) T_{bcjk} \Lambda_{\alpha l} \Lambda_{\beta m} \gamma_b{}^\alpha \epsilon_{\dot{\beta} \dot{\gamma} c} \dot{\alpha} \dot{\beta} \nabla_a \Lambda^{\dot{\delta} m} \epsilon^{ijkl} \\ & + (\frac{1}{27} \bar{\mathcal{I}} + \frac{7}{432} \mathcal{D}^\dagger \mathcal{D}^\dagger \bar{\mathcal{H}}) T_{bcjk} \Lambda^{\dot{\beta} i} \Lambda^{\dot{\gamma} j} \Lambda^{\dot{\delta} k} \bar{P}_d \gamma_{ad \dot{\gamma} \dot{\delta}} \gamma_{bc}{}^{\dot{\alpha}}{}_{\dot{\beta}} + (\frac{1}{27} \bar{\mathcal{H}} + \frac{1}{108} \mathcal{H}) P_b \Lambda_{\alpha j} \Lambda_{\beta k} \chi^{\dot{\beta}}{}_{lm}{}^j \gamma_b{}^\beta \epsilon_{\dot{\beta} \dot{\gamma} a} \dot{\alpha} \epsilon^{iklm} \\ & + (\frac{1}{27} \mathcal{D}^\dagger \bar{\mathcal{H}} + \frac{13}{432} \mathcal{D} \bar{\mathcal{I}}) E_{jk} \Lambda^{\dot{\beta} i} \Lambda^{\dot{\gamma} j} \Lambda^{\dot{\delta} k} \bar{P}_b \epsilon_{\dot{\beta} \dot{\gamma}} \gamma_{ab}{}^{\dot{\alpha}}{}_{\dot{\delta}} + (\frac{37}{960} \mathcal{D} \mathcal{D} \mathcal{H} - \frac{1}{60} \mathcal{I}) E_{jk} \Lambda_{\alpha l} \Lambda_{\beta m} \chi_{\gamma}{}^{jl}{}_n \epsilon^{\alpha \gamma} \gamma_a{}^{\dot{\alpha} \beta} \epsilon^{ikmn} \\ & + (\frac{907}{23040} \bar{\mathcal{H}} + \frac{23}{5760} \mathcal{H}) T_{bcjk} \Lambda_{\alpha l} \Lambda^{\dot{\beta} m} \gamma_{ad}{}^{\alpha \beta} \gamma_{bc}{}^{\dot{\alpha}}{}_{\dot{\beta}} \nabla_d \Lambda_{\beta m} \epsilon^{ijkl} + (\frac{1}{24} \mathcal{D}^\dagger \bar{\mathcal{H}} - \frac{5}{48} \mathcal{D} \bar{\mathcal{I}}) T_{bcjk} T_{ad}{}^{jk} \Lambda_{\alpha l} \Lambda^{\dot{\beta} i} \Lambda^{\dot{\gamma} l} \gamma_d^{\dot{\alpha} \alpha} \gamma_{bc \dot{\beta} \dot{\gamma}} \\ & + (\frac{1}{24} \mathcal{D}^\dagger \bar{\mathcal{H}} + \frac{207}{320} \mathcal{D} \bar{\mathcal{I}}) P_b \Lambda_{\alpha j} \Lambda^{\dot{\alpha} i} \Lambda^{\dot{\beta} j} \bar{P}_c \gamma_d{}^\alpha \epsilon_{abcd} + (\frac{121}{2880} \bar{\mathcal{H}} - \frac{19}{2880} \mathcal{H}) T_{abjk} \Lambda_{\alpha l} \Lambda_{\beta m} \gamma_c{}^\alpha \epsilon_{\dot{\beta} \dot{\gamma} b} \dot{\alpha} \dot{\beta} \nabla_c \Lambda^{\dot{\beta} j} \epsilon^{iklm} \\ & + (\frac{25}{576} \mathcal{D}^\dagger \bar{\mathcal{H}} + \frac{1}{32} \mathcal{D} \bar{\mathcal{I}}) E^{ij} T_{ab}{}^{kl} \Lambda_{\alpha m} \Lambda^{\dot{\alpha} n} \Lambda^{\dot{\beta} m} \gamma_b{}^\alpha \epsilon_{jklm} + (\frac{7}{160} \bar{\mathcal{H}} - \frac{11}{80} \mathcal{H}) T_{bcjk} \Lambda_{\alpha l} \Lambda^{\dot{\beta} l} \gamma_a{}^\beta \epsilon_{\dot{\beta} \dot{\gamma} b} \dot{\alpha} \alpha \nabla_c \Lambda_{\beta m} \epsilon^{ijkm} \\ & + (\frac{7}{160} \mathcal{D}^\dagger \mathcal{I} - \frac{1}{24} \mathcal{D} \mathcal{H}) T_{abjk} \Lambda_{\alpha l} \Lambda_{\beta m} \chi_{\gamma}{}^{il}{}_n \epsilon^{\alpha \gamma} \gamma_b{}^{\dot{\alpha} \beta} \epsilon^{jkmn} + (\frac{11}{240} \bar{\mathcal{I}} + \frac{1}{96} \mathcal{D}^\dagger \mathcal{D}^\dagger \bar{\mathcal{H}}) T_{abjk} T_{bclm} \Lambda_{\alpha n} \Lambda^{\dot{\alpha} i} \Lambda^{\dot{\beta} j} \gamma_c{}^\alpha \epsilon^{\dot{\beta} klmn} \\ & + (\frac{11}{240} \bar{\mathcal{I}} + \frac{1}{96} \mathcal{D}^\dagger \mathcal{D}^\dagger \bar{\mathcal{H}}) T_{abjk} T_{bclm} \Lambda_{\alpha n} \Lambda^{\dot{\alpha} l} \Lambda^{\dot{\beta} i} \gamma_c{}^\alpha \epsilon_{\dot{\beta} \dot{\gamma}} \epsilon^{jkmn} + (\frac{59}{1280} \bar{\mathcal{H}} - \frac{47}{11520} \mathcal{H}) T_{bcjk} \Lambda_{\alpha l} \Lambda^{\dot{\beta} l} \epsilon^{\alpha \beta} \gamma_{bc}{}^{\dot{\alpha}}{}_{\dot{\beta}} \nabla_a \Lambda_{\beta m} \epsilon^{ijkm} \\ & + (\frac{73}{1440} \bar{\mathcal{I}} + \frac{13}{1152} \mathcal{D}^\dagger \mathcal{D}^\dagger \bar{\mathcal{H}}) T_{bcjk} T_{bclm} \Lambda_{\alpha n} \Lambda^{\dot{\alpha} l} \Lambda^{\dot{\beta} m} \gamma_a{}^\alpha \epsilon_{\dot{\beta} \dot{\gamma}} \epsilon^{ijkn} + (\frac{5}{96} \mathcal{D} \mathcal{D} \mathcal{H} + \frac{1}{60} \mathcal{I}) E_{jk} \Lambda_{\alpha l} \Lambda_{\beta m} \chi_{\gamma}{}^{jl}{}_n \epsilon^{\alpha \gamma} \gamma_a{}^{\dot{\alpha} \beta} \epsilon^{ikmn} \\ & + (\frac{103}{1920} \bar{\mathcal{H}} - \frac{5}{144} \mathcal{H}) T_{bcjk} \Lambda_{\alpha l} \Lambda_{\beta m} \gamma_b{}^\alpha \epsilon_{\dot{\beta} \dot{\gamma} a} \dot{\alpha} \dot{\beta} \nabla_c \Lambda^{\dot{\delta} l} \epsilon^{ijkm} + (\frac{1}{18} \bar{\mathcal{I}} - \frac{11}{144} \mathcal{D}^\dagger \mathcal{D}^\dagger \bar{\mathcal{H}}) T_{bc}{}^{jk} \Lambda^{\dot{\beta} i} \Lambda^{\dot{\gamma} l} \epsilon_{\dot{\beta} \dot{\gamma}} \gamma_{ab}{}^{\dot{\alpha}}{}_{\dot{\delta}} \nabla_c \Lambda^{\dot{\delta} m} \epsilon_{jklm} \\ & + (\frac{1}{18} \bar{\mathcal{H}} - \frac{1}{4} \mathcal{H}) P_b T_{ac}{}^{jk} \Lambda_{\alpha j} \Lambda_{\beta k} \Lambda^{\dot{\beta} i} \gamma_c{}^\alpha \epsilon_{\dot{\beta} \dot{\gamma} b} \dot{\alpha} \dot{\beta} + (\frac{1}{18} \mathcal{D}^\dagger \bar{\mathcal{H}} - \frac{1}{60} \mathcal{D} \bar{\mathcal{I}}) P_b T_{bcjk} \Lambda_{\alpha l} \Lambda_{\beta m} \Lambda^{\dot{\alpha} l} \gamma_{ac}{}^{\alpha \beta} \epsilon^{ijkm} \\ & + (\frac{1}{18} \mathcal{D}^\dagger \mathcal{D}^\dagger \bar{\mathcal{I}} - \frac{1}{288} \mathcal{D}^\dagger \mathcal{D}^\dagger \mathcal{D}^\dagger \mathcal{D}^\dagger \bar{\mathcal{H}}) P_b T_{cdjk} \Lambda^{\dot{\beta} i} \Lambda^{\dot{\gamma} j} \Lambda^{\dot{\delta} k} \gamma_{cd \dot{\beta} \dot{\gamma}} \gamma_{ab}{}^{\dot{\alpha}}{}_{\dot{\delta}} + (\frac{1}{18} \mathcal{D}^\dagger \mathcal{D}^\dagger \bar{\mathcal{I}} + \frac{1}{72} \mathcal{D}^\dagger \mathcal{D}^\dagger \mathcal{D}^\dagger \mathcal{D}^\dagger \bar{\mathcal{H}}) P_b T_{acjk} \Lambda^{\dot{\beta} i} \Lambda^{\dot{\gamma} j} \Lambda^{\dot{\delta} k} \epsilon_{\dot{\beta} \dot{\gamma}} \gamma_{bc}{}^{\dot{\alpha}}{}_{\dot{\delta}} \\ & + (\frac{9}{160} \bar{\mathcal{H}} + \frac{13}{480} \mathcal{H}) T_{abjk} \Lambda_{\alpha l} \Lambda^{\dot{\beta} l} \gamma_c{}^\alpha \epsilon_{\dot{\beta} \dot{\gamma} b} \dot{\alpha} \dot{\beta} \nabla_c \Lambda_{\beta m} \epsilon^{ijkm} + (\frac{163}{2880} \bar{\mathcal{H}} - \frac{1}{48} \mathcal{H}) T_{bcjk} \Lambda_{\alpha l} \Lambda^{\dot{\beta} i} \gamma_a{}^\alpha \epsilon_{\dot{\beta} \dot{\gamma} b} \dot{\alpha} \dot{\beta} \nabla_c \Lambda_{\beta m} \epsilon^{jklm} \\ & + (\frac{7}{120} \bar{\mathcal{H}} - \frac{1}{24} \mathcal{H}) T_{bcjk} \Lambda_{\alpha l} \Lambda^{\dot{\beta} j} \gamma_a{}^\alpha \epsilon_{\dot{\beta} \dot{\gamma} b} \dot{\alpha} \dot{\beta} \nabla_c \Lambda_{\beta m} \epsilon^{iklm} + (\frac{17}{288} \bar$$



$$\begin{aligned}
[\hat{\Omega}_a^{\dot{\alpha}i}]_{3,cont.} = & + \left( \frac{3}{32} \mathcal{D}^\dagger \bar{\mathcal{H}} + \frac{3}{16} \mathcal{D} \bar{\mathcal{I}} \right) T_{bcjk} T_{ab}{}^{jk} \Lambda_{\alpha l} \Lambda^{\dot{\beta}i} \Lambda^{\dot{\gamma}l} \epsilon_{\dot{\beta}\dot{\gamma}} \gamma_c^{\dot{\alpha}\alpha} + \left( \frac{7}{72} \bar{\mathcal{H}} - \frac{35}{72} \mathcal{H} \right) P_b T_{ac}{}^{ij} \Lambda_{\alpha j} \Lambda_{\beta k} \Lambda^{\dot{\beta}k} \gamma_c^{\alpha}{}_{\dot{\beta}} \gamma_b^{\dot{\alpha}\beta} \\
& + \left( \frac{7}{72} \bar{\mathcal{H}} - \frac{35}{72} \mathcal{H} \right) P_b T_{ac}{}^{ij} \Lambda_{\alpha j} \Lambda_{\beta k} \Lambda^{\dot{\beta}k} \gamma_c^{\beta}{}_{\dot{\beta}} \gamma_b^{\dot{\alpha}\alpha} + \left( \frac{7}{72} \mathcal{D}^\dagger \bar{\mathcal{I}} - \frac{1}{36} \mathcal{D} \mathcal{H} \right) \Lambda_{\alpha j} \Lambda^{\dot{\beta}i} \Lambda^{\dot{\gamma}j} \bar{P}_b \bar{P}_c \gamma_b^{\dot{\alpha}\alpha} \gamma_{ac\dot{\beta}\dot{\gamma}} \\
& + \left( \frac{149}{1440} \mathcal{D} \mathcal{D} \mathcal{H} + \frac{26}{45} \mathcal{I} \right) T_{ab}{}^{ij} \Lambda_{\alpha j} \Lambda_{\beta k} \Lambda^{\dot{\beta}k} \bar{P}_c \epsilon^{\alpha\beta} \gamma_{bc}^{\dot{\alpha}}{}_{\dot{\beta}} + \left( \frac{5}{48} \bar{\mathcal{I}} + \frac{23}{384} \mathcal{D}^\dagger \mathcal{D}^\dagger \bar{\mathcal{H}} \right) E^{ij} T_{bcjk} \Lambda_{\alpha l} \Lambda^{\dot{\beta}k} \Lambda^{\dot{\gamma}l} \gamma_a^{\alpha}{}_{\dot{\beta}} \gamma_{bc}^{\dot{\alpha}}{}_{\dot{\gamma}} \\
& + \left( \frac{5}{48} \bar{\mathcal{I}} + \frac{23}{384} \mathcal{D}^\dagger \mathcal{D}^\dagger \bar{\mathcal{H}} \right) E^{ij} T_{bcjk} \Lambda_{\alpha l} \Lambda^{\dot{\beta}k} \Lambda^{\dot{\gamma}l} \gamma_a^{\alpha}{}_{\dot{\beta}} \gamma_{bc}^{\dot{\alpha}}{}_{\dot{\gamma}} + \left( \frac{5}{48} \mathcal{D}^\dagger \bar{\mathcal{H}} + \frac{73}{192} \mathcal{D} \bar{\mathcal{I}} \right) P_b \Lambda_{\alpha j} \Lambda^{\dot{\beta}i} \Lambda^{\dot{\gamma}j} \bar{P}_a \epsilon_{\dot{\beta}\dot{\gamma}} \gamma_b^{\dot{\alpha}\alpha} \\
& + \left( \frac{79}{720} \bar{\mathcal{H}} + \frac{13}{576} \mathcal{H} \right) T_{bcjk} \Lambda_{\alpha l} \Lambda_{\beta m} \gamma_b^{\alpha}{}_{\dot{\beta}} \gamma_a^{\dot{\alpha}\beta} \nabla_c \Lambda^{\dot{\beta}j} \epsilon^{iklm} + \left( \frac{643}{5760} \bar{\mathcal{H}} - \frac{113}{2880} \mathcal{H} \right) T_{bcjk} \Lambda_{\alpha l} \Lambda^{\dot{\beta}l} \gamma_b^{\alpha}{}_{\dot{\beta}} \gamma_a^{\dot{\alpha}\beta} \nabla_c \Lambda_{\beta m} \epsilon^{ijkm} \\
& + \left( \frac{1}{8} \mathcal{D}^\dagger \bar{\mathcal{H}} - \frac{11}{24} \mathcal{D} \bar{\mathcal{I}} \right) P_b \Lambda_{\alpha j} \Lambda^{\dot{\beta}i} \Lambda^{\dot{\gamma}j} \bar{P}_b \epsilon_{\dot{\beta}\dot{\gamma}} \gamma_a^{\dot{\alpha}\alpha} + \left( \frac{1}{8} \mathcal{D}^\dagger \bar{\mathcal{I}} - \frac{1}{8} \mathcal{D} \mathcal{H} \right) T_{abjk} \Lambda_{\alpha l} \Lambda_{\beta m} R(Q)_{bc\gamma}{}^i \epsilon^{\alpha\gamma} \gamma_c^{\dot{\alpha}\beta} \epsilon^{jklm} \\
& + \left( \frac{197}{1440} \bar{\mathcal{H}} - \frac{239}{5760} \mathcal{H} \right) T_{bcjk} \Lambda_{\alpha l} \Lambda^{\dot{\beta}j} \gamma_b^{\beta}{}_{\dot{\beta}} \gamma_a^{\dot{\alpha}\alpha} \nabla_c \Lambda_{\beta m} \epsilon^{iklm} + \left( \frac{5}{36} \bar{\mathcal{H}} + \frac{1}{18} \mathcal{H} \right) E_{jk} T_{ab}{}^{il} \Lambda_{\alpha l} \Lambda^{\dot{\beta}j} \Lambda^{\dot{\gamma}k} \epsilon_{\dot{\beta}\dot{\gamma}} \gamma_b^{\dot{\alpha}\alpha} \\
& + \left( \frac{809}{5760} \bar{\mathcal{H}} + \frac{403}{5760} \mathcal{H} \right) \Lambda_{\alpha j} \Lambda_{\beta k} \Lambda^{\dot{\beta}l} \gamma_b^{\alpha}{}_{\dot{\beta}} \gamma_a^{\dot{\alpha}\beta} \nabla_c T_{bclm} \epsilon^{ijkm} + \left( \frac{29}{192} \mathcal{D}^\dagger \bar{\mathcal{H}} - \frac{91}{240} \mathcal{D} \bar{\mathcal{I}} \right) P_b \Lambda_{\alpha j} \Lambda^{\dot{\beta}i} \Lambda^{\dot{\gamma}j} \bar{P}_c \gamma_d^{\alpha}{}_{\dot{\beta}} \epsilon_{abcd} \\
& + \left( \frac{11}{72} \bar{\mathcal{H}} + \frac{7}{72} \mathcal{H} \right) E_{jk} T_{ab}{}^{ij} \Lambda_{\alpha l} \Lambda^{\dot{\beta}k} \Lambda^{\dot{\gamma}l} \epsilon_{\dot{\beta}\dot{\gamma}} \gamma_b^{\dot{\alpha}\alpha} + \left( \frac{893}{5760} \bar{\mathcal{H}} - \frac{893}{5760} \mathcal{H} \right) T_{abjk} \Lambda_{\alpha l} \Lambda^{\dot{\beta}j} \gamma_b^{\alpha}{}_{\dot{\beta}} \gamma_c^{\dot{\alpha}\beta} \nabla_c \Lambda_{\beta m} \epsilon^{iklm} \\
& + \left( \frac{29}{180} \mathcal{D}^\dagger \bar{\mathcal{H}} + \frac{49}{576} \mathcal{D} \bar{\mathcal{I}} \right) E^{ij} P_b \Lambda_{\alpha j} \Lambda_{\beta k} \Lambda^{\dot{\beta}k} \epsilon^{\alpha\beta} \gamma_{ab}^{\dot{\alpha}}{}_{\dot{\beta}} + \left( \frac{121}{720} \bar{\mathcal{H}} - \frac{73}{11520} \mathcal{H} \right) T_{bcjk} \Lambda_{\alpha l} \Lambda^{\dot{\beta}i} \gamma_b^{\beta}{}_{\dot{\beta}} \gamma_a^{\dot{\alpha}\alpha} \nabla_c \Lambda_{\beta m} \epsilon^{jklm} \\
& + \left( \frac{5}{24} \mathcal{D} \mathcal{D} \mathcal{H} + \frac{7}{6} \mathcal{I} \right) T_{ab}{}^{jk} \Lambda_{\alpha j} \Lambda_{\beta k} \Lambda^{\dot{\beta}i} \bar{P}_c \gamma_b^{\alpha}{}_{\dot{\beta}} \gamma_c^{\dot{\alpha}\beta} + \left( \frac{53}{240} \bar{\mathcal{H}} - \frac{19}{240} \mathcal{H} \right) P_b T_{cd}{}^{ij} \Lambda_{\alpha j} \Lambda_{\beta k} \Lambda^{\dot{\beta}k} \gamma_{cd}^{\alpha\beta} \gamma_{ab}^{\dot{\alpha}}{}_{\dot{\beta}} \\
& + \left( \frac{7}{24} \bar{\mathcal{I}} - \frac{7}{192} \mathcal{D}^\dagger \mathcal{D}^\dagger \bar{\mathcal{H}} \right) E^{ij} T_{bcjk} \Lambda_{\alpha l} \Lambda^{\dot{\beta}k} \Lambda^{\dot{\gamma}l} \gamma_a^{\dot{\alpha}\alpha} \gamma_{bc\dot{\beta}\dot{\gamma}} + \left( \frac{337}{1152} \bar{\mathcal{H}} + \frac{167}{2880} \mathcal{H} \right) T_{bcjk} \Lambda_{\alpha l} \Lambda^{\dot{\beta}m} \gamma_b^{\alpha}{}_{\dot{\beta}} \gamma_a^{\dot{\alpha}\beta} \nabla_c \Lambda_{\beta m} \epsilon^{ijkl} \\
& + \left( \frac{7}{18} \bar{\mathcal{I}} - \frac{1}{72} \mathcal{D}^\dagger \mathcal{D}^\dagger \bar{\mathcal{H}} \right) T_{bcjk} \Lambda^{\dot{\beta}i} \Lambda^{\dot{\gamma}j} \Lambda^{\dot{\delta}k} \bar{P}_a \epsilon_{\dot{\beta}\dot{\gamma}} \gamma_{bc}^{\dot{\alpha}}{}_{\dot{\delta}} + \left( \frac{11}{24} \mathcal{D} \mathcal{D} \mathcal{H} + \frac{8}{3} \mathcal{I} \right) T_{ab}{}^{ij} \Lambda_{\alpha j} \Lambda_{\beta k} \Lambda^{\dot{\beta}k} \bar{P}_c \gamma_b^{\alpha}{}_{\dot{\beta}} \gamma_c^{\dot{\alpha}\beta} \\
& + \left( \frac{11}{24} \mathcal{D} \mathcal{D} \mathcal{H} + \frac{8}{3} \mathcal{I} \right) T_{ab}{}^{ij} \Lambda_{\alpha j} \Lambda_{\beta k} \Lambda^{\dot{\beta}k} \bar{P}_c \gamma_b^{\beta}{}_{\dot{\beta}} \gamma_c^{\dot{\alpha}\alpha} + \left( \frac{17}{30} \mathcal{D}^\dagger \bar{\mathcal{I}} - \frac{5}{48} \mathcal{D} \mathcal{H} \right) T_{bcjk} \Lambda_{\alpha l} \Lambda_{\beta m} \Lambda^{\dot{\alpha}l} \bar{P}_b \gamma_{ac}^{\alpha\beta} \epsilon^{ijkm} \\
& + \left( \frac{7}{12} \bar{\mathcal{I}} - \frac{19}{96} \mathcal{D}^\dagger \mathcal{D}^\dagger \bar{\mathcal{H}} \right) E^{ij} T_{abjk} \Lambda_{\alpha l} \Lambda^{\dot{\beta}k} \Lambda^{\dot{\gamma}l} \epsilon_{\dot{\beta}\dot{\gamma}} \gamma_b^{\dot{\alpha}\alpha} + \left( \frac{247}{360} \bar{\mathcal{H}} - \frac{29}{180} \mathcal{H} \right) P_b T_{bc}{}^{ij} \Lambda_{\alpha j} \Lambda_{\beta k} \Lambda^{\dot{\beta}k} \epsilon^{\alpha\beta} \gamma_{ac}^{\dot{\alpha}}{}_{\dot{\beta}} \\
& + \left( \frac{73}{72} \mathcal{D}^\dagger \bar{\mathcal{I}} + \frac{1}{36} \mathcal{D} \mathcal{H} \right) T_{abjk} \Lambda_{\alpha l} \Lambda_{\beta m} \Lambda^{\dot{\alpha}l} \bar{P}_b \epsilon^{\alpha\beta} \epsilon^{ijkm} + \left( \frac{11}{9} \mathcal{D}^\dagger \bar{\mathcal{I}} + \frac{11}{144} \mathcal{D}^\dagger \mathcal{D}^\dagger \mathcal{D}^\dagger \bar{\mathcal{H}} \right) P_b P_c \Lambda_{\alpha j} \Lambda^{\dot{\beta}i} \Lambda^{\dot{\gamma}j} \gamma_b^{\dot{\alpha}\alpha} \gamma_{ac\dot{\beta}\dot{\gamma}} \\
& + \frac{1}{12} E_{jk} T_{ab}{}^{il} \mathcal{D} \mathcal{D} \mathcal{D} \mathcal{H} \Lambda_{\alpha l} \Lambda_{\beta m} \Lambda_{\gamma n} \epsilon^{\alpha\beta} \gamma_b^{\dot{\alpha}\gamma} \epsilon^{ikmn} + \frac{5}{216} P_b T_{acjk} \mathcal{D} \bar{\mathcal{I}} \Lambda_{\alpha l} \Lambda_{\beta m} \Lambda^{\dot{\beta}i} \gamma_c^{\alpha}{}_{\dot{\beta}} \gamma_b^{\dot{\alpha}\beta} \epsilon^{jklm} \\
& + \frac{1}{135} P_b T_{acjk} \mathcal{D} \bar{\mathcal{I}} \Lambda_{\alpha l} \Lambda_{\beta m} \Lambda^{\dot{\beta}j} \gamma_c^{\alpha}{}_{\dot{\beta}} \gamma_b^{\dot{\alpha}\beta} \epsilon^{iklm} + \frac{13}{540} P_b T_{acjk} \mathcal{D} \bar{\mathcal{I}} \Lambda_{\alpha l} \Lambda_{\beta m} \Lambda^{\dot{\beta}l} \gamma_c^{\alpha}{}_{\dot{\beta}} \gamma_b^{\dot{\alpha}\beta} \epsilon^{ijkm} \\
& + \frac{13}{540} P_b T_{acjk} \mathcal{D} \bar{\mathcal{I}} \Lambda_{\alpha l} \Lambda_{\beta m} \Lambda^{\dot{\beta}l} \gamma_c^{\beta}{}_{\dot{\beta}} \gamma_b^{\dot{\alpha}\alpha} \epsilon^{ijkm} - \frac{7}{60} T_{abjk} \mathcal{D}^\dagger \bar{\mathcal{I}} \Lambda_{\alpha l} \Lambda_{\beta m} \Lambda^{\dot{\beta}i} \bar{P}_c \gamma_b^{\alpha}{}_{\dot{\beta}} \gamma_c^{\dot{\alpha}\beta} \epsilon^{jklm} \\
& - \frac{13}{30} T_{abjk} \mathcal{D}^\dagger \bar{\mathcal{I}} \Lambda_{\alpha l} \Lambda_{\beta m} \Lambda^{\dot{\beta}j} \bar{P}_c \gamma_b^{\alpha}{}_{\dot{\beta}} \gamma_c^{\dot{\alpha}\beta} \epsilon^{iklm} - \frac{13}{60} T_{abjk} \mathcal{D}^\dagger \bar{\mathcal{I}} \Lambda_{\alpha l} \Lambda_{\beta m} \Lambda^{\dot{\beta}l} \bar{P}_c \gamma_b^{\alpha}{}_{\dot{\beta}} \gamma_c^{\dot{\alpha}\beta} \epsilon^{ijkm} \\
& - \frac{13}{60} T_{abjk} \mathcal{D}^\dagger \bar{\mathcal{I}} \Lambda_{\alpha l} \Lambda_{\beta m} \Lambda^{\dot{\beta}l} \bar{P}_c \gamma_b^{\beta}{}_{\dot{\beta}} \gamma_c^{\dot{\alpha}\alpha} \epsilon^{ijkm} + \frac{1}{40} T_{ab}{}^{jk} \mathcal{D} \bar{\mathcal{I}} \Lambda^{\dot{\beta}i} \Lambda^{\dot{\gamma}l} \Lambda^{\dot{\delta}m} \bar{P}_c \epsilon_{\dot{\beta}\dot{\gamma}} \gamma_{bc}^{\dot{\alpha}}{}_{\dot{\delta}} \epsilon_{jklm} \\
& - \frac{1}{36} \bar{\mathcal{I}} T_{abjk} T_{cdlm} \Lambda_{\alpha n} \Lambda^{\dot{\beta}j} \Lambda^{\dot{\gamma}n} \gamma_b^{\dot{\alpha}\alpha} \gamma_{cd\dot{\beta}\dot{\gamma}} \epsilon^{iklm} + \frac{1}{36} \bar{\mathcal{I}} T_{abjk} T_{cdlm} \Lambda_{\alpha n} \Lambda^{\dot{\beta}l} \Lambda^{\dot{\gamma}n} \gamma_b^{\dot{\alpha}\alpha} \gamma_{cd\dot{\beta}\dot{\gamma}} \epsilon^{ijkm} \\
& - \frac{1}{192} \mathcal{D} \mathcal{D} \mathcal{D} \mathcal{D} \mathcal{H} \Lambda_{\alpha j} \Lambda_{\beta k} \Lambda_{\gamma l} \bar{P}_b \bar{P}_c \gamma_b^{\dot{\alpha}\alpha} \gamma_{ac}^{\beta\gamma} \epsilon^{ijkl} + \frac{7}{96} \mathcal{H} T_{ab}{}^{jk} T_{bc}{}^{lm} \Lambda_{\alpha j} \Lambda^{\dot{\beta}i} \Lambda^{\dot{\gamma}n} \epsilon_{\dot{\beta}\dot{\gamma}} \gamma_c^{\dot{\alpha}\alpha} \epsilon_{klmn} \\
& - \frac{7}{96} \mathcal{H} T_{ab}{}^{jk} T_{bc}{}^{lm} \Lambda_{\alpha l} \Lambda^{\dot{\beta}i} \Lambda^{\dot{\gamma}n} \epsilon_{\dot{\beta}\dot{\gamma}} \gamma_c^{\dot{\alpha}\alpha} \epsilon_{jkmn} + \left( -\frac{3}{8} \bar{\mathcal{I}} - \frac{17}{192} \mathcal{D}^\dagger \mathcal{D}^\dagger \bar{\mathcal{H}} \right) T_{abjk} T_{bclm} \Lambda_{\alpha n} \Lambda^{\dot{\beta}l} \Lambda^{\dot{\gamma}n} \epsilon_{\dot{\beta}\dot{\gamma}} \gamma_c^{\dot{\alpha}\alpha} \epsilon^{ijkm} \\
& + \left( -\frac{11}{48} \bar{\mathcal{I}} - \frac{11}{192} \mathcal{D}^\dagger \mathcal{D}^\dagger \bar{\mathcal{H}} \right) T_{abjk} T_{bclm} \Lambda_{\alpha n} \Lambda^{\dot{\beta}i} \Lambda^{\dot{\gamma}l} \epsilon_{\dot{\beta}\dot{\gamma}} \gamma_c^{\dot{\alpha}\alpha} \epsilon^{jkmn} + \left( -\frac{5}{24} \mathcal{D}^\dagger \bar{\mathcal{H}} + \frac{1}{12} \mathcal{D} \bar{\mathcal{I}} \right) E^{ij} T_{ab}{}^{kl} \Lambda_{\alpha m} \Lambda^{\dot{\beta}m} \Lambda^{\dot{\gamma}n} \epsilon_{\dot{\beta}\dot{\gamma}} \gamma_b^{\dot{\alpha}\alpha} \epsilon_{jklm} \\
& + \left( -\frac{7}{36} \bar{\mathcal{I}} - \frac{1}{384} \mathcal{D}^\dagger \mathcal{D}^\dagger \bar{\mathcal{H}} \right) T_{bcjk} T_{bdlm} \Lambda_{\alpha n} \Lambda^{\dot{\beta}j} \Lambda^{\dot{\gamma}n} \gamma_a^{\dot{\alpha}\alpha} \gamma_{cd\dot{\beta}\dot{\gamma}} \epsilon^{iklm} + \left( -\frac{7}{36} \mathcal{D}^\dagger \bar{\mathcal{H}} + \frac{29}{360} \mathcal{D} \bar{\mathcal{I}} \right) T_{bc}{}^{jk} \Lambda^{\dot{\beta}i} \Lambda^{\dot{\gamma}l} \Lambda^{\dot{\delta}m} \bar{P}_b \epsilon_{\dot{\beta}\dot{\gamma}} \gamma_{ac}^{\dot{\alpha}}{}_{\dot{\delta}} \epsilon_{jklm} \\
& + \left( -\frac{13}{80} \mathcal{D}^\dagger \bar{\mathcal{I}} - \frac{43}{480} \mathcal{D} \mathcal{H} \right) T_{bcjk} \Lambda_{\alpha l} \Lambda_{\beta m} \Lambda^{\dot{\beta}l} \bar{P}_b \gamma_a^{\alpha}{}_{\dot{\beta}} \gamma_c^{\dot{\alpha}\beta} \epsilon^{ijkm} + \left( -\frac{13}{80} \mathcal{D}^\dagger \bar{\mathcal{I}} - \frac{43}{480} \mathcal{D} \mathcal{H} \right) T_{bcjk} \Lambda_{\alpha l} \Lambda_{\beta m} \Lambda^{\dot{\beta}l} \bar{P}_b \gamma_a^{\beta}{}_{\dot{\beta}} \gamma_c^{\dot{\alpha}\alpha} \epsilon^{ijkm} \\
& + \left( -\frac{11}{90} \mathcal{D}^\dagger \bar{\mathcal{I}} - \frac{9}{64} \mathcal{D} \mathcal{H} \right) T_{bcjk} \Lambda_{\alpha l} \Lambda_{\beta m} \Lambda^{\dot{\beta}l} \bar{P}_b \epsilon^{\alpha\beta} \gamma_{ac}^{\dot{\alpha}}{}_{\dot{\beta}} \epsilon^{ijkm} + \left( -\frac{1}{10} \mathcal{D}^\dagger \bar{\mathcal{I}} - \frac{3}{160} \mathcal{D}^\dagger \mathcal{D}^\dagger \mathcal{D}^\dagger \bar{\mathcal{H}} \right) P_b T_{ac}{}^{jk} \Lambda^{\dot{\beta}i} \Lambda^{\dot{\gamma}l} \Lambda^{\dot{\delta}m} \epsilon_{\dot{\beta}\dot{\gamma}} \gamma_{bc}^{\dot{\alpha}}{}_{\dot{\delta}} \epsilon_{jklm} \\
& + \left( -\frac{233}{2880} \mathcal{D}^\dagger \bar{\mathcal{H}} - \frac{977}{8640} \mathcal{D} \bar{\mathcal{I}} \right) P_b T_{acjk} \Lambda_{\alpha l} \Lambda_{\beta m} \Lambda^{\dot{\beta}i} \gamma_b^{\alpha}{}_{\dot{\beta}} \gamma_c^{\dot{\alpha}\beta} \epsilon^{jklm} + \left( -\frac{19}{240} \bar{\mathcal{I}} - \frac{5}{384} \mathcal{D}^\dagger \mathcal{D}^\dagger \bar{\mathcal{H}} \right) T_{bcjk} T_{bdlm} \Lambda_{\alpha n} \Lambda^{\dot{\beta}i} \Lambda^{\dot{\gamma}j} \gamma_a^{\dot{\alpha}\alpha} \gamma_{cd\dot{\beta}\dot{\gamma}} \epsilon^{klmn} \\
& + \left( -\frac{3}{40} \mathcal{D}^\dagger \bar{\mathcal{I}} - \frac{5}{192} \mathcal{D} \mathcal{H} \right) T_{bcjk} \Lambda_{\alpha l} \Lambda_{\beta m} \Lambda^{\dot{\beta}i} \bar{P}_b \gamma_c^{\alpha}{}_{\dot{\beta}} \gamma_a^{\dot{\alpha}\beta} \epsilon^{jklm} + \left( -\frac{41}{720} \mathcal{D}^\dagger \bar{\mathcal{H}} - \frac{101}{5760} \mathcal{D} \bar{\mathcal{I}} \right) E_{jk} T_{ablm} \Lambda_{\alpha n} \Lambda^{\dot{\beta}j} \Lambda^{\dot{\gamma}l} \epsilon_{\dot{\beta}\dot{\gamma}} \gamma_b^{\dot{\alpha}\alpha} \epsilon^{ikmn} + 17 \dots
\end{aligned}$$



$$\begin{aligned}
[\hat{\Omega}_a^{\dot{\alpha}i}]_{3,cont.} = & + \left( \frac{103}{1440} \mathcal{D}^\dagger \bar{\mathcal{H}} - \frac{7}{96} \mathcal{D} \bar{\mathcal{I}} \right) P_b T_{bcjk} \Lambda_{\alpha l} \Lambda_{\beta m} \Lambda^{\dot{\beta}j} \gamma_a^\alpha \epsilon_{\dot{\beta}}^{\dot{\alpha}} \gamma_c^{\dot{\alpha}\beta} \epsilon^{iklm} + \left( \frac{2}{27} \mathcal{D}^\dagger \mathcal{I} + \frac{1}{108} \mathcal{D} \mathcal{H} \right) E^{jk} T_{abjl} \Lambda_{\alpha k} \Lambda_{\beta m} \Lambda_{\gamma n} \epsilon^{\alpha\beta} \gamma_b^{\dot{\alpha}\gamma} \epsilon^{\dot{\alpha}\gamma} \epsilon^{ilmn} \\
& + \left( \frac{19}{240} \bar{\mathcal{I}} + \frac{5}{384} \mathcal{D}^\dagger \mathcal{D}^\dagger \bar{\mathcal{H}} \right) T_{bcjk} T_{bdlm} \Lambda_{\alpha n} \Lambda^{\dot{\beta}i} \Lambda^{\dot{\gamma}l} \gamma_a^{\dot{\alpha}\alpha} \gamma_{cd\dot{\beta}\dot{\gamma}} \epsilon^{jkmn} + \left( \frac{89}{960} \mathcal{D}^\dagger \bar{\mathcal{H}} + \frac{101}{3456} \mathcal{D} \bar{\mathcal{I}} \right) P_b T_{bcjk} \Lambda_{\alpha l} \Lambda_{\beta m} \Lambda^{\dot{\beta}i} \gamma_c^\alpha \epsilon_{\dot{\beta}}^{\dot{\alpha}} \gamma_a^{\dot{\alpha}\beta} \epsilon^{jklm} \\
& + \left( \frac{91}{960} \mathcal{D}^\dagger \bar{\mathcal{H}} + \frac{275}{3456} \mathcal{D} \bar{\mathcal{I}} \right) P_b T_{bcjk} \Lambda_{\alpha l} \Lambda_{\beta m} \Lambda^{\dot{\beta}l} \gamma_c^\alpha \epsilon_{\dot{\beta}}^{\dot{\alpha}} \gamma_a^{\dot{\alpha}\beta} \epsilon^{ijkm} + \left( \frac{91}{960} \mathcal{D}^\dagger \bar{\mathcal{H}} + \frac{275}{3456} \mathcal{D} \bar{\mathcal{I}} \right) P_b T_{bcjk} \Lambda_{\alpha l} \Lambda_{\beta m} \Lambda^{\dot{\beta}l} \gamma_c^\beta \epsilon_{\dot{\beta}}^{\dot{\alpha}} \gamma_a^{\dot{\alpha}\alpha} \epsilon^{ijkm} \\
& + \left( \frac{13}{120} \mathcal{D}^\dagger \mathcal{I} - \frac{7}{240} \mathcal{D} \mathcal{H} \right) T_{bcjk} \Lambda_{\alpha l} \Lambda_{\beta m} \Lambda^{\dot{\beta}j} \bar{P}_b \gamma_a^\alpha \epsilon_{\dot{\beta}}^{\dot{\alpha}} \gamma_c^{\dot{\alpha}\beta} \epsilon^{iklm} + \left( \frac{3}{20} \mathcal{D}^\dagger \mathcal{I} + \frac{1}{96} \mathcal{D} \mathcal{H} \right) T_{bcjk} \Lambda_{\alpha l} \Lambda_{\beta m} \Lambda^{\dot{\beta}j} \bar{P}_b \gamma_c^\alpha \epsilon_{\dot{\beta}}^{\dot{\alpha}} \gamma_a^{\dot{\alpha}\beta} \epsilon^{iklm} \\
& + \left( \frac{7}{36} \bar{\mathcal{I}} + \frac{1}{384} \mathcal{D}^\dagger \mathcal{D}^\dagger \bar{\mathcal{H}} \right) T_{bcjk} T_{bdlm} \Lambda_{\alpha n} \Lambda^{\dot{\beta}l} \Lambda^{\dot{\gamma}n} \gamma_a^{\dot{\alpha}\alpha} \gamma_{cd\dot{\beta}\dot{\gamma}} \epsilon^{ijkm} + \left( \frac{11}{48} \bar{\mathcal{I}} + \frac{11}{192} \mathcal{D}^\dagger \mathcal{D}^\dagger \bar{\mathcal{H}} \right) T_{abjk} T_{bclm} \Lambda_{\alpha n} \Lambda^{\dot{\beta}i} \Lambda^{\dot{\gamma}j} \epsilon_{\dot{\beta}\dot{\gamma}}^{\dot{\alpha}} \gamma_c^{\dot{\alpha}\alpha} \epsilon^{klmn} \\
& + \left( \frac{29}{120} \mathcal{D}^\dagger \mathcal{I} - \frac{23}{192} \mathcal{D} \mathcal{H} \right) T_{bcjk} \Lambda_{\alpha l} \Lambda_{\beta m} \Lambda^{\dot{\beta}l} \bar{P}_b \gamma_c^\alpha \epsilon_{\dot{\beta}}^{\dot{\alpha}} \gamma_a^{\dot{\alpha}\beta} \epsilon^{ijkm} + \left( \frac{29}{120} \mathcal{D}^\dagger \mathcal{I} - \frac{23}{192} \mathcal{D} \mathcal{H} \right) T_{bcjk} \Lambda_{\alpha l} \Lambda_{\beta m} \Lambda^{\dot{\beta}l} \bar{P}_b \gamma_c^\beta \epsilon_{\dot{\beta}}^{\dot{\alpha}} \gamma_a^{\dot{\alpha}\alpha} \epsilon^{ijkm} \\
& + \left( \frac{35}{128} \bar{\mathcal{I}} + \frac{7}{768} \mathcal{D}^\dagger \mathcal{D}^\dagger \bar{\mathcal{H}} \right) T_{bcjk} T_{bclm} \Lambda_{\alpha n} \Lambda^{\dot{\beta}i} \Lambda^{\dot{\gamma}n} \epsilon_{\dot{\beta}\dot{\gamma}}^{\dot{\alpha}} \gamma_a^{\dot{\alpha}\alpha} \epsilon^{ijklm} + \left( \frac{3}{8} \bar{\mathcal{I}} + \frac{17}{192} \mathcal{D}^\dagger \mathcal{D}^\dagger \bar{\mathcal{H}} \right) T_{abjk} T_{bclm} \Lambda_{\alpha n} \Lambda^{\dot{\beta}j} \Lambda^{\dot{\gamma}n} \epsilon_{\dot{\beta}\dot{\gamma}}^{\dot{\alpha}} \gamma_c^{\dot{\alpha}\alpha} \epsilon^{ijklm} \\
& + \left( \frac{1439}{2880} \mathcal{D}^\dagger \bar{\mathcal{H}} - \frac{521}{2160} \mathcal{D} \bar{\mathcal{I}} \right) P_b T_{bcjk} \Lambda_{\alpha l} \Lambda_{\beta m} \Lambda^{\dot{\beta}l} \epsilon^{\alpha\beta} \gamma_{ac}^{\dot{\alpha}} \epsilon_{\dot{\beta}}^{\dot{\alpha}} \epsilon^{ijkm} + \frac{1}{192} E_{jk} E_{lm} \mathcal{D} \mathcal{D} \mathcal{D} \mathcal{H} \Lambda_{\alpha n} \Lambda_{\beta p} \Lambda_{\gamma q} \epsilon^{\alpha\beta} \gamma_a^{\dot{\alpha}\gamma} \epsilon^{\dot{\alpha}\gamma} \epsilon^{ijn} \epsilon^{kmpq} \\
& + \left( -\frac{17}{2880} \mathcal{D} \mathcal{D} \mathcal{H} - \frac{29}{720} \mathcal{I} \right) E_{jk} T_{ablm} \Lambda_{\alpha n} \Lambda_{\beta p} \Lambda_{\gamma q} \epsilon^{\alpha\beta} \gamma_b^{\dot{\alpha}\gamma} \epsilon^{\dot{\alpha}\gamma} \epsilon^{ijn} \epsilon^{kmpq} \\
& + \left( \frac{1}{48} \mathcal{D}^\dagger \mathcal{I} - \frac{1}{48} \mathcal{D} \mathcal{H} \right) T_{bcjk} T_{bclm} \Lambda_{\alpha n} \Lambda_{\beta p} \Lambda_{\gamma q} \epsilon^{\alpha\beta} \gamma_a^{\dot{\alpha}\gamma} \epsilon^{\dot{\alpha}\gamma} \epsilon^{ijkn} \epsilon^{lmpq} + \left( \frac{163}{5760} \mathcal{D} \mathcal{D} \mathcal{H} + \frac{91}{1440} \mathcal{I} \right) E_{jk} T_{ablm} \Lambda_{\alpha n} \Lambda_{\beta p} \Lambda_{\gamma q} \epsilon^{\alpha\beta} \gamma_b^{\dot{\alpha}\gamma} \epsilon^{\dot{\alpha}\gamma} \epsilon^{ijnq} \epsilon^{klmp}
\end{aligned}$$

The five fermion terms are:

[illegible]



$$\begin{aligned}
[\hat{\Omega}_a^{\dot{\alpha}i}]_{5,cont.} = & +(-\frac{5}{864}\bar{\mathcal{H}} - \frac{19}{864}\mathcal{H})E^{ij}\Lambda_{\alpha j}\Lambda_{\beta k}\Lambda^{\dot{\alpha}k}\Lambda^{\dot{\beta}l}\Lambda_{\gamma l}\epsilon^{\alpha\beta}\gamma_a{}^\gamma{}_{\dot{\beta}}{}^\alpha + (-\frac{1}{360}\bar{\mathcal{H}} - \frac{7}{384}\mathcal{H})\Lambda_{\alpha j}\Lambda_{\beta k}\Lambda^{\dot{\alpha}j}\Lambda^{\dot{\beta}i}\Lambda^{\dot{\gamma}k}\bar{P}_b\gamma_a{}^\beta{}_{\dot{\gamma}}{}^\gamma{}_{\dot{b}}{}^\alpha{}_{\dot{\beta}} \\
& +(-\frac{7}{2880}\mathcal{D}^\dagger\bar{\mathcal{I}} + \frac{3}{2560}\mathcal{D}^\dagger\mathcal{D}^\dagger\bar{\mathcal{H}})\Lambda^{\dot{\alpha}j}\Lambda^{\dot{\beta}i}\Lambda^{\dot{\gamma}k}\Lambda^{\dot{\delta}l}\chi_{\alpha}{}^{mn}{}_k\epsilon_{\dot{\beta}\dot{\delta}}\gamma_a{}^\alpha{}_{\dot{\gamma}}\epsilon_{jlmn} + (-\frac{1}{576}\bar{\mathcal{I}} + \frac{1}{1536}\mathcal{D}^\dagger\mathcal{D}^\dagger\bar{\mathcal{H}})E_{jk}\Lambda_{\alpha l}\Lambda^{\dot{\alpha}l}\Lambda^{\dot{\beta}i}\Lambda^{\dot{\gamma}j}\Lambda^{\dot{\delta}k}\epsilon_{\dot{\beta}\dot{\gamma}}\gamma_a{}^\alpha{}_{\dot{\delta}} \\
& +(-\frac{1}{864}\bar{\mathcal{H}} - \frac{1}{288}\mathcal{H})E^{jk}\Lambda_{\alpha j}\Lambda_{\beta k}\Lambda^{\dot{\alpha}i}\Lambda^{\dot{\beta}l}\Lambda_{\gamma l}\epsilon^{\alpha\beta}\gamma_a{}^\gamma{}_{\dot{\beta}}{}^\alpha + (-\frac{1}{864}\bar{\mathcal{H}} - \frac{1}{288}\mathcal{H})E^{jk}\Lambda_{\alpha j}\Lambda_{\beta k}\Lambda^{\dot{\alpha}i}\Lambda^{\dot{\beta}l}\Lambda_{\gamma l}\epsilon^{\alpha\gamma}\gamma_a{}^\beta{}_{\dot{\beta}} \\
& +(-\frac{5}{12288}\bar{\mathcal{H}} - \frac{9}{4096}\mathcal{H})\Lambda_{\alpha j}\Lambda_{\beta k}\Lambda^{\dot{\alpha}i}\Lambda^{\dot{\beta}j}R(Q)_{bc\gamma}{}^k\epsilon^{\alpha\gamma}\gamma_a{}^\delta{}_{\dot{\beta}}\gamma_{bcd}{}^\beta + (\frac{5}{12288}\bar{\mathcal{H}} + \frac{9}{4096}\mathcal{H})\Lambda_{\alpha j}\Lambda_{\beta k}\Lambda^{\dot{\alpha}j}\Lambda^{\dot{\beta}i}R(Q)_{bc\gamma}{}^k\epsilon^{\alpha\gamma}\gamma_a{}^\delta{}_{\dot{\beta}}\gamma_{bcd}{}^\beta \\
& +(\frac{1}{576}\bar{\mathcal{I}} - \frac{1}{1536}\mathcal{D}^\dagger\mathcal{D}^\dagger\bar{\mathcal{H}})E_{jk}\Lambda_{\alpha l}\Lambda^{\dot{\alpha}j}\Lambda^{\dot{\beta}i}\Lambda^{\dot{\gamma}k}\Lambda^{\dot{\delta}l}\epsilon_{\dot{\beta}\dot{\gamma}}\gamma_a{}^\alpha{}_{\dot{\delta}} + (\frac{1}{384}\mathcal{D}^\dagger\mathcal{D}^\dagger\bar{\mathcal{I}} - \frac{1}{1536}\mathcal{D}^\dagger\mathcal{D}^\dagger\mathcal{D}^\dagger\bar{\mathcal{H}})\Lambda^{\dot{\alpha}j}\Lambda^{\dot{\beta}k}\Lambda^{\dot{\gamma}l}\Lambda^{\dot{\delta}m}\epsilon_{\dot{\beta}\dot{\epsilon}}\gamma_{ab\dot{\gamma}\dot{\delta}}\nabla_b\Lambda^{\dot{\epsilon}i}\epsilon_{jklm} \\
& +(\frac{13}{2880}\mathcal{D}^\dagger\bar{\mathcal{I}} - \frac{23}{23040}\mathcal{D}^\dagger\mathcal{D}^\dagger\bar{\mathcal{H}})\Lambda^{\dot{\alpha}i}\Lambda^{\dot{\beta}j}\Lambda^{\dot{\gamma}k}\Lambda^{\dot{\delta}l}\chi_{\alpha}{}^{mn}{}_j\epsilon_{\dot{\beta}\dot{\gamma}}\gamma_a{}^\alpha{}_{\dot{\delta}}\epsilon_{klmn} \\
& +(\frac{1}{192}\mathcal{D}^\dagger\mathcal{D}^\dagger\bar{\mathcal{I}} - \frac{1}{768}\mathcal{D}^\dagger\mathcal{D}^\dagger\mathcal{D}^\dagger\bar{\mathcal{H}})\Lambda^{\dot{\alpha}j}\Lambda^{\dot{\beta}i}\Lambda^{\dot{\gamma}k}\Lambda^{\dot{\delta}l}\epsilon_{\dot{\beta}\dot{\gamma}}\gamma_{ab\dot{\delta}\dot{\epsilon}}\nabla_b\Lambda^{\dot{\epsilon}m}\epsilon_{jklm} \\
& +(\frac{1}{192}\mathcal{DDH} - \frac{1}{144}\mathcal{I})\Lambda_{\alpha j}\Lambda_{\beta k}\Lambda^{\dot{\alpha}i}\Lambda_{\gamma l}\epsilon^{\alpha\delta}\gamma_{ab}{}^{\beta\gamma}\nabla_b\Lambda_{\delta m}\epsilon^{jklm} + (\frac{1}{144}\mathcal{D}^\dagger\bar{\mathcal{I}} + \frac{1}{144}\mathcal{DH})T_{bc}{}^{jk}\Lambda_{\alpha j}\Lambda_{\beta k}\Lambda^{\dot{\alpha}l}\Lambda^{\dot{\beta}i}\Lambda_{\gamma l}\gamma_a{}^\gamma{}_{\dot{\beta}}\gamma_{bc}{}^{\alpha\beta} \\
& +(\frac{1}{128}\mathcal{D}^\dagger\mathcal{D}^\dagger\bar{\mathcal{I}} + \frac{1}{1536}\mathcal{D}^\dagger\mathcal{D}^\dagger\mathcal{D}^\dagger\bar{\mathcal{H}})\Lambda^{\dot{\beta}i}\Lambda^{\dot{\gamma}j}\Lambda^{\dot{\delta}k}\Lambda^{\dot{\epsilon}l}\epsilon_{\dot{\beta}\dot{\gamma}}\gamma_{ab\dot{\delta}\dot{\epsilon}}\nabla_b\Lambda^{\dot{\alpha}m}\epsilon_{jklm} \\
& +(\frac{3}{256}\mathcal{DDH} - \frac{17}{288}\mathcal{I})\Lambda_{\alpha j}\Lambda_{\beta k}\Lambda^{\dot{\alpha}l}\Lambda_{\gamma m}\epsilon^{\alpha\delta}\gamma_{ab}{}^{\beta\gamma}\nabla_b\Lambda_{\delta l}\epsilon^{ijkm} \\
& +(\frac{3}{256}\mathcal{DDH} - \frac{1}{32}\mathcal{I})\Lambda_{\alpha j}\Lambda_{\beta k}\Lambda_{\gamma l}\Lambda_{\delta m}\epsilon^{\alpha\beta}\gamma_{ab}{}^{\gamma\delta}\nabla_b\Lambda^{\dot{\alpha}j}\epsilon^{iklm} + (\frac{1}{72}\mathcal{D}^\dagger\bar{\mathcal{I}} + \frac{1}{72}\mathcal{DH})T_{bc}{}^{jk}\Lambda_{\alpha j}\Lambda_{\beta k}\Lambda^{\dot{\alpha}l}\Lambda^{\dot{\beta}i}\Lambda_{\gamma l}\gamma_a{}^\alpha{}_{\dot{\beta}}\gamma_{bc}{}^{\beta\gamma} \\
& +(\frac{41}{2880}\bar{\mathcal{H}} + \frac{7}{576}\mathcal{H})\Lambda_{\alpha j}\Lambda_{\beta k}\Lambda^{\dot{\alpha}i}\Lambda^{\dot{\beta}j}\Lambda^{\dot{\gamma}k}\bar{P}_b\gamma_a{}^\alpha{}_{\dot{\beta}}\gamma_b{}^\beta{}_{\dot{\gamma}}{}^\alpha + (\frac{5}{288}\mathcal{D}^\dagger\bar{\mathcal{I}} - \frac{73}{768}\mathcal{D}^\dagger\mathcal{D}^\dagger\bar{\mathcal{H}})T_{abjk}\Lambda_{\alpha l}\Lambda^{\dot{\alpha}j}\Lambda^{\dot{\beta}i}\Lambda^{\dot{\gamma}k}\Lambda^{\dot{\delta}l}\epsilon_{\dot{\gamma}\dot{\delta}}\gamma_b{}^\alpha{}_{\dot{\beta}} \\
& +(\frac{53}{2880}\mathcal{D}^\dagger\bar{\mathcal{I}} - \frac{59}{11520}\mathcal{D}^\dagger\mathcal{D}^\dagger\bar{\mathcal{H}})\Lambda^{\dot{\alpha}j}\Lambda^{\dot{\beta}i}\Lambda^{\dot{\gamma}k}\Lambda^{\dot{\delta}l}\chi_{\alpha}{}^{mn}{}_k\epsilon_{\dot{\gamma}\dot{\delta}}\gamma_a{}^\alpha{}_{\dot{\beta}}\epsilon_{jlmn} + (\frac{329}{15360}\bar{\mathcal{H}} + \frac{9}{1024}\mathcal{H})\Lambda_{\alpha j}\Lambda_{\beta k}\Lambda^{\dot{\beta}i}\Lambda^{\dot{\gamma}j}R(Q)_{ab\gamma}{}^k\epsilon^{\beta\gamma}\epsilon_{\dot{\beta}\dot{\gamma}}\gamma_b{}^{\dot{\alpha}\alpha} \\
& +(\frac{23}{864}\bar{\mathcal{H}} + \frac{1}{864}\mathcal{H})E^{ij}\Lambda_{\alpha j}\Lambda_{\beta k}\Lambda^{\dot{\alpha}k}\Lambda^{\dot{\beta}l}\Lambda_{\gamma l}\epsilon^{\alpha\gamma}\gamma_a{}^\beta{}_{\dot{\beta}}{}^\alpha + (\frac{35}{1152}\bar{\mathcal{I}} + \frac{1}{384}\mathcal{D}^\dagger\mathcal{D}^\dagger\bar{\mathcal{H}})\Lambda_{\alpha j}\Lambda^{\dot{\beta}i}\Lambda^{\dot{\gamma}j}\Lambda^{\dot{\delta}k}R(Q)_{bc}{}^{\dot{\alpha}}{}_k\epsilon_{\dot{\beta}\dot{\gamma}}\gamma_a{}^\alpha{}_{\dot{\epsilon}}\gamma_{bc}{}^{\dot{\epsilon}}{}_{\dot{\delta}} \\
& +(\frac{7}{216}\bar{\mathcal{H}} + \frac{5}{216}\mathcal{H})E^{ij}\Lambda_{\alpha j}\Lambda_{\beta k}\Lambda^{\dot{\alpha}k}\Lambda^{\dot{\beta}l}\Lambda_{\gamma l}\epsilon^{\beta\gamma}\gamma_a{}^\alpha{}_{\dot{\beta}}{}^\alpha + (\frac{19}{576}\bar{\mathcal{I}} - \frac{19}{1536}\mathcal{D}^\dagger\mathcal{D}^\dagger\bar{\mathcal{H}})E_{jk}\Lambda_{\alpha l}\Lambda^{\dot{\alpha}j}\Lambda^{\dot{\beta}i}\Lambda^{\dot{\gamma}k}\Lambda^{\dot{\delta}l}\epsilon_{\dot{\gamma}\dot{\delta}}\gamma_a{}^\alpha{}_{\dot{\beta}} \\
& +(\frac{1}{30}\mathcal{D}^\dagger\bar{\mathcal{I}} - \frac{17}{640}\mathcal{DH})\Lambda_{\alpha j}\Lambda_{\beta k}\Lambda^{\dot{\beta}l}\Lambda_{\gamma m}\chi^{\dot{\alpha}}{}_{ln}{}^j\epsilon^{\alpha\beta}\gamma_a{}^\gamma{}_{\dot{\beta}}\epsilon^{ikmn} + (\frac{5}{144}\mathcal{D}^\dagger\bar{\mathcal{I}} - \frac{1}{36}\mathcal{DH})T_{ab}{}^{jk}\Lambda_{\alpha j}\Lambda_{\beta k}\Lambda^{\dot{\alpha}l}\Lambda^{\dot{\beta}i}\Lambda_{\gamma l}\epsilon^{\alpha\gamma}\gamma_b{}^\beta{}_{\dot{\beta}} \\
& +(\frac{923}{23040}\bar{\mathcal{H}} - \frac{1}{1536}\mathcal{H})\Lambda_{\alpha j}\Lambda_{\beta k}\Lambda^{\dot{\alpha}j}\Lambda^{\dot{\beta}i}\Lambda^{\dot{\gamma}k}\bar{P}_b\gamma_a{}^\alpha{}_{\dot{\gamma}}\gamma_b{}^\beta{}_{\dot{\beta}}{}^\alpha + (\frac{25}{576}\mathcal{D}^\dagger\bar{\mathcal{I}} - \frac{7}{768}\mathcal{D}^\dagger\mathcal{D}^\dagger\bar{\mathcal{H}})T_{bcjk}\Lambda_{\alpha l}\Lambda^{\dot{\alpha}l}\Lambda^{\dot{\beta}i}\Lambda^{\dot{\gamma}j}\Lambda^{\dot{\delta}k}\gamma_a{}^\alpha{}_{\dot{\gamma}}\gamma_{bc}\dot{\delta} \\
& +(\frac{29}{576}\bar{\mathcal{I}} + \frac{73}{2304}\mathcal{D}^\dagger\mathcal{D}^\dagger\bar{\mathcal{H}})\Lambda_{\alpha j}\Lambda^{\dot{\beta}i}\Lambda^{\dot{\gamma}j}\Lambda^{\dot{\delta}k}R(Q)_{bc}{}^{\dot{\epsilon}}{}_k\epsilon_{\dot{\beta}\dot{\epsilon}}\gamma_a{}^{\dot{\alpha}\alpha}\gamma_{bc\dot{\gamma}\dot{\delta}} + (\frac{1187}{23040}\bar{\mathcal{H}} - \frac{17}{1536}\mathcal{H})\Lambda_{\alpha j}\Lambda_{\beta k}\Lambda^{\dot{\alpha}j}\Lambda^{\dot{\beta}i}\Lambda^{\dot{\gamma}k}\bar{P}_b\gamma_a{}^\alpha{}_{\dot{\beta}}\gamma_b{}^\beta{}_{\dot{\gamma}}{}^\alpha \\
& +(\frac{263}{4608}\bar{\mathcal{H}} + \frac{137}{4608}\mathcal{H})\Lambda_{\alpha j}\Lambda_{\beta k}\Lambda^{\dot{\alpha}i}\Lambda^{\dot{\beta}j}\Lambda^{\dot{\gamma}k}\bar{P}_b\gamma_a{}^\alpha{}_{\dot{\gamma}}\gamma_b{}^\beta{}_{\dot{\beta}}{}^\alpha + (\frac{1}{16}\mathcal{DDH} + \frac{5}{72}\mathcal{I})\Lambda_{\alpha j}\Lambda_{\beta k}\Lambda^{\dot{\alpha}j}\Lambda_{\gamma l}\epsilon^{\alpha\beta}\gamma_{ab}{}^{\gamma\delta}\nabla_b\Lambda_{\delta m}\epsilon^{iklm} \\
& +(\frac{41}{576}\mathcal{D}^\dagger\bar{\mathcal{I}} + \frac{1}{768}\mathcal{D}^\dagger\mathcal{D}^\dagger\bar{\mathcal{H}})T_{bcjk}\Lambda_{\alpha l}\Lambda^{\dot{\alpha}l}\Lambda^{\dot{\beta}i}\Lambda^{\dot{\gamma}j}\Lambda^{\dot{\delta}k}\gamma_a{}^\alpha{}_{\dot{\beta}}\gamma_{bc\dot{\gamma}\dot{\delta}} + (\frac{13}{144}\mathcal{D}^\dagger\bar{\mathcal{I}} + \frac{5}{384}\mathcal{D}^\dagger\mathcal{D}^\dagger\bar{\mathcal{H}})T_{bcjk}\Lambda_{\alpha l}\Lambda^{\dot{\alpha}j}\Lambda^{\dot{\beta}i}\Lambda^{\dot{\gamma}k}\Lambda^{\dot{\delta}l}\gamma_a{}^\alpha{}_{\dot{\beta}}\gamma_{bc\dot{\gamma}\dot{\delta}} \\
& +(\frac{3}{32}\mathcal{D}^\dagger\bar{\mathcal{I}} + \frac{9}{256}\mathcal{D}^\dagger\mathcal{D}^\dagger\bar{\mathcal{H}})T_{abjk}\Lambda_{\alpha l}\Lambda^{\dot{\alpha}j}\Lambda^{\dot{\beta}i}\Lambda^{\dot{\gamma}k}\Lambda^{\dot{\delta}l}\epsilon_{\dot{\beta}\dot{\gamma}}\gamma_b{}^\alpha{}_{\dot{\delta}} + (\frac{3}{32}\mathcal{D}^\dagger\bar{\mathcal{I}} + \frac{9}{256}\mathcal{D}^\dagger\mathcal{D}^\dagger\bar{\mathcal{H}})T_{abjk}\Lambda_{\alpha l}\Lambda^{\dot{\alpha}l}\Lambda^{\dot{\beta}i}\Lambda^{\dot{\gamma}j}\Lambda^{\dot{\delta}k}\epsilon_{\dot{\beta}\dot{\gamma}}\gamma_b{}^\alpha{}_{\dot{\delta}} \\
& +(\frac{31}{288}\mathcal{D}^\dagger\bar{\mathcal{I}} + \frac{1}{96}\mathcal{D}^\dagger\mathcal{D}^\dagger\bar{\mathcal{H}})T_{bcjk}\Lambda_{\alpha l}\Lambda^{\dot{\alpha}i}\Lambda^{\dot{\beta}j}\Lambda^{\dot{\gamma}k}\Lambda^{\dot{\delta}l}\gamma_a{}^\alpha{}_{\dot{\beta}}\gamma_{bc\dot{\gamma}\dot{\delta}} + (\frac{7}{64}\bar{\mathcal{H}} - \frac{29}{576}\mathcal{H})\Lambda_{\alpha j}\Lambda_{\beta k}\Lambda^{\dot{\alpha}j}\Lambda^{\dot{\beta}i}\Lambda^{\dot{\gamma}k}\bar{P}_a\epsilon^{\alpha\beta}\epsilon_{\dot{\beta}\dot{\gamma}} \\
& +(\frac{113}{960}\bar{\mathcal{I}} - \frac{1}{480}\mathcal{D}^\dagger\mathcal{D}^\dagger\bar{\mathcal{H}})P_b\Lambda_{\alpha j}\Lambda_{\beta k}\Lambda^{\dot{\alpha}j}\Lambda^{\dot{\beta}i}\Lambda^{\dot{\gamma}k}\gamma_a{}^\alpha{}_{\dot{\gamma}}\gamma_b{}^\beta{}_{\dot{\beta}}{}^\alpha + (\frac{29}{240}\bar{\mathcal{H}} - \frac{17}{128}\mathcal{H})\Lambda_{\alpha j}\Lambda_{\beta k}\Lambda^{\dot{\beta}j}\Lambda^{\dot{\gamma}l}\chi_{\gamma}{}^{ik}{}_l\epsilon^{\beta\gamma}\epsilon_{\dot{\beta}\dot{\gamma}}\gamma_a{}^{\dot{\alpha}\alpha} \\
& +(\frac{1}{8}\mathcal{D}^\dagger\bar{\mathcal{I}} - \frac{337}{11520}\mathcal{DH})\Lambda_{\alpha j}\Lambda_{\beta k}\Lambda^{\dot{\beta}j}\Lambda_{\gamma l}\chi^{\dot{\alpha}}{}_{mn}{}^k\epsilon^{\alpha\gamma}\gamma_a{}^\beta{}_{\dot{\beta}}\epsilon^{\dot{\alpha}ilmn} + (\frac{77}{576}\bar{\mathcal{I}} - \frac{77}{11520}\mathcal{D}^\dagger\mathcal{D}^\dagger\bar{\mathcal{H}})P_b\Lambda_{\alpha j}\Lambda_{\beta k}\Lambda^{\dot{\alpha}j}\Lambda^{\dot{\beta}i}\Lambda^{\dot{\gamma}k}\gamma_a{}^\alpha{}_{\dot{\beta}}\gamma_b{}^\beta{}_{\dot{\gamma}}{}^\alpha \\
& +(\frac{659}{2880}\bar{\mathcal{I}} + \frac{91}{3840}\mathcal{D}^\dagger\mathcal{D}^\dagger\bar{\mathcal{H}})\Lambda_{\alpha j}\Lambda^{\dot{\beta}i}\Lambda^{\dot{\gamma}j}\Lambda^{\dot{\delta}k}R(Q)_{ab}{}^{\dot{\epsilon}}{}_k\epsilon_{\dot{\beta}\dot{\gamma}}\epsilon_{\dot{\delta}\dot{\epsilon}}\gamma_b{}^{\dot{\alpha}\alpha} + (\frac{83}{288}\mathcal{D}^\dagger\bar{\mathcal{I}} + \frac{1}{768}\mathcal{D}^\dagger\mathcal{D}^\dagger\bar{\mathcal{H}})T_{abjk}\Lambda_{\alpha l}\Lambda^{\dot{\alpha}i}\Lambda^{\dot{\beta}j}\Lambda^{\dot{\gamma}k}\Lambda^{\dot{\delta}l}\epsilon_{\dot{\beta}\dot{\delta}}\gamma_b{}^\alpha{}_{\dot{\gamma}} \\
& +(\frac{1831}{2880}\bar{\mathcal{I}} + \frac{551}{3840}\mathcal{D}^\dagger\mathcal{D}^\dagger\bar{\mathcal{H}})P_a\Lambda_{\alpha j}\Lambda_{\beta k}\Lambda^{\dot{\alpha}i}\Lambda^{\dot{\beta}j}\Lambda^{\dot{\gamma}k}\epsilon^{\alpha\beta}\epsilon_{\dot{\beta}\dot{\gamma}} + (\frac{541}{720}\bar{\mathcal{I}} + \frac{389}{3840}\mathcal{D}^\dagger\mathcal{D}^\dagger\bar{\mathcal{H}})P_b\Lambda_{\alpha j}\Lambda_{\beta k}\Lambda^{\dot{\alpha}j}\Lambda^{\dot{\beta}i}\Lambda^{\dot{\gamma}k}\epsilon_{\dot{\beta}\dot{\gamma}}\gamma_{ab}{}^{\alpha\beta} \\
& +(\frac{31}{12}\bar{\mathcal{I}} + \frac{2729}{5760}\mathcal{D}^\dagger\mathcal{D}^\dagger\bar{\mathcal{H}})P_b\Lambda_{\alpha j}\Lambda_{\beta k}\Lambda^{\dot{\alpha}j}\Lambda^{\dot{\beta}i}\Lambda^{\dot{\gamma}k}\epsilon^{\alpha\beta}\gamma_{ab\dot{\beta}\dot{\gamma}} - \frac{1}{1920}P_b\mathcal{D}^\dagger\mathcal{D}^\dagger\mathcal{D}^\dagger\mathcal{D}^\dagger\bar{\mathcal{H}}\Lambda^{\dot{\alpha}j}\Lambda^{\dot{\beta}i}\Lambda^{\dot{\gamma}k}\Lambda^{\dot{\delta}l}\Lambda^{\dot{\epsilon}m}\epsilon_{\dot{\beta}\dot{\gamma}}\gamma_{ab\dot{\delta}\dot{\epsilon}}\epsilon_{jklm} \\
& -\frac{1}{96}\mathcal{D}^\dagger\mathcal{D}^\dagger\mathcal{D}^\dagger\bar{\mathcal{H}}E^{ij}\Lambda_{\alpha k}\Lambda^{\dot{\alpha}l}\Lambda^{\dot{\beta}k}\Lambda^{\dot{\gamma}m}\Lambda^{\dot{\delta}n}\epsilon_{\dot{\beta}\dot{\gamma}}\gamma_a{}^\alpha{}_{\dot{\delta}}\epsilon_{jlmn} + \frac{1}{120}\mathcal{DDDH}\Lambda_{\alpha j}\Lambda_{\beta k}\Lambda_{\gamma l}\Lambda_{\delta m}\chi_{\epsilon}{}^{jk}{}_n\epsilon^{\alpha\gamma}\epsilon^{\beta\delta}\gamma_a{}^{\dot{\alpha}\epsilon}\epsilon^{\dot{\alpha}ilmn} \\
& -\frac{7}{960}\mathcal{DDDH}\Lambda_{\alpha j}\Lambda_{\beta k}\Lambda_{\gamma l}\Lambda_{\delta m}\chi_{\epsilon}{}^{jk}{}_n\epsilon^{\alpha\gamma}\epsilon^{\beta\epsilon}\gamma_a{}^{\dot{\alpha}\delta}\epsilon^{\dot{\alpha}ilmn} - \frac{11}{960}\mathcal{DDDH}\Lambda_{\alpha j}\Lambda_{\beta k}\Lambda_{\gamma l}\Lambda_{\delta m}\chi_{\epsilon}{}^{jk}{}_n\epsilon^{\alpha\gamma}\epsilon^{\delta\epsilon}\gamma_a{}^{\dot{\alpha}\beta}\epsilon^{\dot{\alpha}ilmn} \\
& +(-\frac{301}{2304}\mathcal{D}^\dagger\bar{\mathcal{I}} + \frac{47}{3840}\mathcal{DH})\Lambda_{\alpha j}\Lambda_{\beta k}\Lambda^{\dot{\beta}j}\Lambda_{\gamma l}\chi^{\dot{\alpha}}{}_{mn}{}^k\epsilon^{\alpha\gamma}\epsilon_{\dot{\beta}\dot{\gamma}}\gamma_a{}^{\dot{\alpha}\beta}\epsilon^{\dot{\alpha}ilmn} + (-\frac{25}{288}\bar{\mathcal{H}} + \frac{5}{288}\mathcal{H})T_{abjk}\Lambda_{\alpha l}\Lambda_{\beta m}\Lambda^{\dot{\alpha}j}\Lambda^{\dot{\beta}l}\Lambda_{\gamma n}\epsilon^{\alpha\beta}\gamma_b{}^\gamma{}_{\dot{\beta}}\epsilon^{ikmn} \\
& +(-\frac{1}{16}\bar{\mathcal{I}} - \frac{1}{16}\mathcal{D}^\dagger\mathcal{D}^\dagger\bar{\mathcal{H}})T_{ab}{}^{jk}\Lambda_{\alpha l}\Lambda^{\dot{\alpha}m}\Lambda^{\dot{\beta}i}\Lambda^{\dot{\gamma}l}\Lambda^{\dot{\delta}n}\epsilon_{\dot{\gamma}\dot{\delta}}\gamma_b{}^\alpha{}_{\dot{\beta}}\epsilon_{\dot{\gamma}jkmn} + (-\frac{7}{288}\bar{\mathcal{H}} + \frac{35}{288}\mathcal{H})T_{abjk}\Lambda_{\alpha l}\Lambda_{\beta m}\Lambda^{\dot{\alpha}l}\Lambda^{\dot{\beta}i}\Lambda_{\gamma n}\epsilon^{\alpha\beta}\gamma_b{}^\gamma{}_{\dot{\beta}}\epsilon^{jkmn} \\
& +(-\frac{7}{360}\mathcal{D}^\dagger\bar{\mathcal{I}} + \frac{131}{23040}\mathcal{D}^\dagger\mathcal{D}^\dagger\bar{\mathcal{H}})\Lambda^{\dot{\beta}i}\Lambda^{\dot{\gamma}j}\Lambda^{\dot{\delta}k}\Lambda^{\dot{\epsilon}l}\chi_{\alpha}{}^{mn}{}_j\epsilon_{\dot{\beta}\dot{\delta}}\epsilon_{\dot{\gamma}\dot{\epsilon}}\gamma_a{}^{\dot{\alpha}\alpha}\epsilon_{klmn} \\
& +(-\frac{7}{576}\mathcal{D}^\dagger\bar{\mathcal{I}} + \frac{1}{144}\mathcal{DH})E_{jk}\Lambda_{\alpha l}\Lambda_{\beta m}\Lambda^{\dot{\alpha}l}\Lambda^{\dot{\beta}j}\Lambda_{\gamma n}\epsilon^{\alpha\beta}\gamma_a{}^\gamma{}_{\dot{\beta}}\epsilon^{ikmn} + 3\cdots
\end{aligned}$$

47

The seven fermion terms are:

$$\begin{aligned}
[\hat{\Omega}_a^{\dot{\alpha}i}]_7 = & \left(-\frac{1}{256} \mathcal{D}^\dagger \bar{\mathcal{H}} + \frac{1}{96} \mathcal{D} \bar{\mathcal{L}}\right) \Lambda_{\alpha j} \Lambda_{\beta k} \Lambda^{\dot{\alpha}j} \Lambda^{\dot{\beta}i} \Lambda^{\dot{\gamma}k} \Lambda^{\dot{\delta}l} \Lambda_{\gamma l} \epsilon^{\alpha\beta} \epsilon_{\dot{\beta}\dot{\gamma}} \gamma_a{}^\gamma{}_{\dot{\delta}} + \left(-\frac{1}{256} \mathcal{D}^\dagger \bar{\mathcal{H}} + \frac{1}{96} \mathcal{D} \bar{\mathcal{L}}\right) \Lambda_{\alpha j} \Lambda_{\beta k} \Lambda^{\dot{\alpha}j} \Lambda^{\dot{\beta}i} \Lambda^{\dot{\gamma}k} \Lambda^{\dot{\delta}l} \Lambda_{\gamma l} \epsilon^{\beta\gamma} \epsilon_{\dot{\gamma}\dot{\delta}} \gamma_a{}^\alpha{}_{\dot{\beta}} \\
& + \left(\frac{1}{256} \mathcal{D}^\dagger \bar{\mathcal{H}} - \frac{1}{96} \mathcal{D} \bar{\mathcal{L}}\right) \Lambda_{\alpha j} \Lambda_{\beta k} \Lambda^{\dot{\alpha}i} \Lambda^{\dot{\beta}j} \Lambda^{\dot{\gamma}k} \Lambda^{\dot{\delta}l} \Lambda_{\gamma l} \epsilon^{\alpha\beta} \epsilon_{\dot{\beta}\dot{\delta}} \gamma_a{}^\gamma{}_{\dot{\gamma}} + \left(\frac{1}{256} \mathcal{D}^\dagger \bar{\mathcal{H}} - \frac{1}{96} \mathcal{D} \bar{\mathcal{L}}\right) \Lambda_{\alpha j} \Lambda_{\beta k} \Lambda^{\dot{\alpha}i} \Lambda^{\dot{\beta}j} \Lambda^{\dot{\gamma}k} \Lambda^{\dot{\delta}l} \Lambda_{\gamma l} \epsilon^{\alpha\beta} \epsilon_{\dot{\beta}\dot{\gamma}} \gamma_a{}^\gamma{}_{\dot{\delta}} \\
& + \left(\frac{1}{256} \mathcal{D}^\dagger \bar{\mathcal{H}} - \frac{1}{96} \mathcal{D} \bar{\mathcal{L}}\right) \Lambda_{\alpha j} \Lambda_{\beta k} \Lambda^{\dot{\alpha}j} \Lambda^{\dot{\beta}i} \Lambda^{\dot{\gamma}k} \Lambda^{\dot{\delta}l} \Lambda_{\gamma l} \epsilon^{\alpha\beta} \epsilon_{\dot{\gamma}\dot{\delta}} \gamma_a{}^\gamma{}_{\dot{\beta}} + \left(\frac{1}{256} \mathcal{D}^\dagger \bar{\mathcal{H}} - \frac{1}{96} \mathcal{D} \bar{\mathcal{L}}\right) \Lambda_{\alpha j} \Lambda_{\beta k} \Lambda^{\dot{\alpha}j} \Lambda^{\dot{\beta}i} \Lambda^{\dot{\gamma}k} \Lambda^{\dot{\delta}l} \Lambda_{\gamma l} \epsilon^{\beta\gamma} \epsilon_{\dot{\beta}\dot{\gamma}} \gamma_a{}^\alpha{}_{\dot{\delta}} \\
& + \frac{1}{384} \mathcal{D}^\dagger \mathcal{D}^\dagger \mathcal{D}^\dagger \mathcal{D}^\dagger \bar{\mathcal{H}} \Lambda_{\alpha j} \Lambda^{\dot{\alpha}k} \Lambda^{\dot{\beta}i} \Lambda^{\dot{\gamma}j} \Lambda^{\dot{\delta}l} \Lambda^{\dot{\epsilon}m} \Lambda^{\sigma 1n} \epsilon_{\dot{\beta}\dot{\delta}} \epsilon_{\dot{\gamma}\dot{\epsilon}} \gamma_a{}^\alpha{}_{\sigma 1} \epsilon_{klmn} + \frac{1}{32} \mathcal{D} \mathcal{D} \mathcal{H} \Lambda_{\alpha j} \Lambda_{\beta k} \Lambda^{\dot{\alpha}j} \Lambda^{\dot{\beta}k} \Lambda_{\gamma l} \Lambda_{\delta m} \Lambda_{\epsilon n} \epsilon^{\alpha\gamma} \epsilon^{\beta\delta} \gamma_a{}^\epsilon{}_{\dot{\beta}} \epsilon^{ilmn} \\
& + \left(-\frac{13}{192} \mathcal{D}^\dagger \bar{\mathcal{H}} + \frac{3}{32} \mathcal{D} \bar{\mathcal{L}}\right) \Lambda_{\alpha j} \Lambda_{\beta k} \Lambda^{\dot{\beta}i} \Lambda^{\dot{\gamma}j} \Lambda^{\dot{\delta}k} \Lambda^{\dot{\epsilon}l} \Lambda_{\gamma l} \epsilon^{\alpha\beta} \epsilon_{\dot{\beta}\dot{\epsilon}} \epsilon_{\dot{\gamma}\dot{\delta}} \gamma_a{}^{\dot{\alpha}\gamma} + \left(\frac{13}{192} \mathcal{D}^\dagger \bar{\mathcal{H}} - \frac{3}{32} \mathcal{D} \bar{\mathcal{L}}\right) \Lambda_{\alpha j} \Lambda_{\beta k} \Lambda^{\dot{\beta}i} \Lambda^{\dot{\gamma}j} \Lambda^{\dot{\delta}k} \Lambda^{\dot{\epsilon}l} \Lambda_{\gamma l} \epsilon^{\alpha\beta} \epsilon_{\dot{\beta}\dot{\gamma}} \epsilon_{\dot{\delta}\dot{\epsilon}} \gamma_a{}^{\dot{\alpha}\gamma} \\
& + \frac{1}{11520} \mathcal{D} \mathcal{D} \mathcal{D} \mathcal{D} \mathcal{D} \mathcal{H} \Lambda_{\alpha j} \Lambda_{\beta k} \Lambda_{\gamma l} \Lambda_{\delta m} \Lambda_{\epsilon n} \Lambda_{\epsilon 1p} \Lambda_{\epsilon 2q} \epsilon^{\alpha\beta} \epsilon^{\gamma\delta} \epsilon^{\epsilon 1} \gamma_a{}^{\dot{\alpha}\epsilon 2} \epsilon^{ijln} \epsilon^{kmpq};
\end{aligned}$$



## The $\mathcal{E}$ blocks

$\mathcal{E}^{ij}$

The zero fermion terms are:

$$\begin{aligned}
[\mathcal{E}^{ij}]_0 = & (-\mathcal{D}^\dagger \bar{\mathcal{H}} - 2\mathcal{D}\bar{\mathcal{L}})i\nabla_a \nabla_a E^{ij} + 8iE^{ij}\bar{\mathcal{L}}\nabla_a P_a + 16iP_a\bar{\mathcal{L}}\nabla_a E^{ij} - \frac{1}{3}iE_{kl}E^{kl}E^{ij}\mathcal{D}^\dagger \bar{\mathcal{H}} + 8iE^{ij}P_a P_a \mathcal{D}^\dagger \bar{\mathcal{L}} \\
& + (-\frac{8}{3}\mathcal{D}^\dagger \bar{\mathcal{L}} + 2\mathcal{D}\mathcal{H})iE_{kl}T_{ab}{}^{ki}T_{ab}{}^{lj} + (-\frac{2}{3}\bar{\mathcal{H}} - \frac{4}{3}\mathcal{H})iD^{ki}{}_{lm}E_{kn}\varepsilon^{lmnj} + (\mathcal{D}^\dagger \bar{\mathcal{H}} + \frac{4}{3}\mathcal{D}\bar{\mathcal{L}})iE_{kl}E^{ki}E^{lj} \\
& + (\frac{4}{3}\mathcal{D}^\dagger \bar{\mathcal{H}} + \frac{8}{3}\mathcal{D}\bar{\mathcal{L}})iE^{ij}P_a \bar{P}_a - \frac{4}{3}iE^{ij}T_{abkl}T_{abmn}\bar{\mathcal{L}}\varepsilon^{klmn} - \frac{8}{3}iE^{ki}T_{ablm}T_{abkn}\bar{\mathcal{L}}\varepsilon^{lmnj} + \frac{1}{3}iE^{ij}\mathcal{H}T_{ab}{}^{kl}T_{ab}{}^{mn}\varepsilon_{klmn} \\
& - \frac{1}{6}iE_{kl}E_{mn}E_{pq}\mathcal{D}\mathcal{H}\varepsilon^{kmpi}\varepsilon^{lnqj} + (\frac{2}{9}\mathcal{D}^\dagger \bar{\mathcal{H}} + \frac{4}{9}\mathcal{D}\bar{\mathcal{L}})iE_{kl}T_{abmn}T_{abpq}\varepsilon^{kmpi}\varepsilon^{lnqj} + (\frac{7}{18}\mathcal{D}^\dagger \bar{\mathcal{H}} + \frac{4}{9}\mathcal{D}\bar{\mathcal{L}})iE_{kl}T_{abmn}T_{abpq}\varepsilon^{kmni}\varepsilon^{lpqj} \\
& + (-\frac{1}{12}\mathcal{D}^\dagger \bar{\mathcal{L}} + \frac{1}{24}\mathcal{D}\mathcal{H})iT_{ab}{}^{ki}T_{cd}{}^{lm}T_{ef}{}^{nj}\gamma_{ab\alpha\beta}\gamma_{cd}\gamma^\alpha\gamma_{ef}{}^{\beta\gamma}\varepsilon_{klmn} + \frac{1}{12}iT_{abkl}T_{cdmn}T_{efpq}\bar{\mathcal{L}}\gamma_{ab\dot{\alpha}\dot{\beta}}\gamma_{cd}{}^{\dot{\alpha}}{}_{\dot{\gamma}}\gamma_{ef}{}^{\dot{\beta}\dot{\gamma}}\varepsilon^{klmi}\varepsilon^{npqj}
\end{aligned}$$

The two fermion terms are:

$$\begin{aligned}
[\mathcal{E}^{ij}]_2 = & -4i\Lambda^{\dot{\alpha}i}\bar{\mathcal{L}}\epsilon_{\dot{\alpha}\dot{\beta}}\nabla_a \nabla_a \Lambda^{\dot{\beta}j} - 8i\bar{\mathcal{L}}\epsilon_{\dot{\alpha}\dot{\beta}}\nabla_a \Lambda^{\dot{\alpha}i}\nabla_a \Lambda^{\dot{\beta}j} - 4i\mathcal{H}R(Q)_{ab\alpha}{}^i R(Q)_{ab\beta}{}^j \epsilon^{\alpha\beta} - 8i\mathcal{H}\chi_\alpha{}^{ki}{}_l \chi_\beta{}^{lj}{}_k \epsilon^{\alpha\beta} + 8iE^{ki}\Lambda^{\dot{\alpha}l}\bar{\mathcal{L}}\chi^{\dot{\beta}}{}_{kl}{}^j \epsilon_{\dot{\alpha}\dot{\beta}} \\
& - 16iP_a \mathcal{D}^\dagger \bar{\mathcal{L}} \Lambda^{\dot{\alpha}i} \epsilon_{\dot{\alpha}\dot{\beta}} \nabla_a \Lambda^{\dot{\beta}j} + \frac{4}{3}i\Lambda^{\dot{\alpha}k}\Lambda^{\dot{\beta}i}R(V)_{ab}{}^j{}_k \bar{\mathcal{L}}\gamma_{ab\dot{\alpha}\dot{\beta}} - 4i\mathcal{D}^\dagger \bar{\mathcal{L}} \Lambda^{\dot{\alpha}i} \Lambda^{\dot{\beta}j} \epsilon_{\dot{\alpha}\dot{\beta}} \nabla_a P_a + \frac{4}{3}i\mathcal{D}^\dagger \bar{\mathcal{H}} \Lambda_{\alpha k} \Lambda^{\dot{\alpha}i} \gamma_a{}^\alpha{}_{\dot{\alpha}} \nabla_a E^{kj} \\
& + \frac{8}{3}i\mathcal{D}\bar{\mathcal{L}} \Lambda_{\alpha k} \Lambda^{\dot{\alpha}k} \gamma_a{}^\alpha{}_{\dot{\alpha}} \nabla_a E^{ij} + (-\frac{20}{3}\mathcal{D}^\dagger \bar{\mathcal{H}} - \frac{40}{3}\mathcal{D}\bar{\mathcal{L}})i\Lambda^{\dot{\alpha}i} \bar{P}_a \epsilon_{\dot{\alpha}\dot{\beta}} \nabla_a \Lambda^{\dot{\beta}j} + (-\frac{4}{3}\mathcal{D}^\dagger \bar{\mathcal{H}} - \frac{8}{3}\mathcal{D}\bar{\mathcal{L}})i\Lambda^{\dot{\alpha}i} \bar{P}_a \gamma_{ab\dot{\alpha}\dot{\beta}} \nabla_b \Lambda^{\dot{\beta}j} \\
& + (-\frac{2}{3}\mathcal{D}^\dagger \bar{\mathcal{H}} - \frac{4}{3}\mathcal{D}\bar{\mathcal{L}})i\Lambda^{\dot{\alpha}i} \Lambda^{\dot{\beta}j} \epsilon_{\dot{\alpha}\dot{\beta}} \nabla_a \bar{P}_a + (-\frac{1}{3}\mathcal{D}^\dagger \bar{\mathcal{H}} - \frac{2}{3}\mathcal{D}\bar{\mathcal{L}})iE^{ij} \Lambda^{\dot{\alpha}k} \gamma_a{}^\alpha{}_{\dot{\alpha}} \nabla_a \Lambda_{\alpha k} + (-\frac{1}{3}\mathcal{D}^\dagger \bar{\mathcal{H}} + 2\mathcal{D}\bar{\mathcal{L}})iE^{ij} \Lambda_{\alpha k} \gamma_a{}^\alpha{}_{\dot{\alpha}} \nabla_a \Lambda^{\dot{\alpha}k} \\
& + (\frac{2}{3}\mathcal{D}^\dagger \bar{\mathcal{H}} + \frac{4}{3}\mathcal{D}\bar{\mathcal{L}})iE^{ki} \Lambda^{\dot{\alpha}j} \gamma_a{}^\alpha{}_{\dot{\alpha}} \nabla_a \Lambda_{\alpha k} + (2\mathcal{D}^\dagger \bar{\mathcal{H}} + \frac{4}{3}\mathcal{D}\bar{\mathcal{L}})iE^{ki} \Lambda_{\alpha k} \gamma_a{}^\alpha{}_{\dot{\alpha}} \nabla_a \Lambda^{\dot{\alpha}j} + (\frac{8}{3}\bar{\mathcal{H}} + \frac{4}{3}\mathcal{H})i\Lambda_{\alpha k} \gamma_a{}^\alpha{}_{\dot{\alpha}} \nabla_a \chi^{\dot{\alpha}l}{}_{lm}{}^i \varepsilon^{klmj} \\
& + (4\mathcal{D}^\dagger \bar{\mathcal{H}} + 8\mathcal{D}\bar{\mathcal{L}})i\chi^{\dot{\alpha}}{}_{kl}{}^m \chi^{\dot{\beta}}{}_{mn}{}^i \epsilon_{\dot{\alpha}\dot{\beta}} \varepsilon^{klmj} + (\frac{16}{3}\bar{\mathcal{H}} - \frac{4}{3}\mathcal{H})iE^{ki} \Lambda_{\alpha l} \chi_\beta{}^{lj}{}_k \epsilon^{\alpha\beta} - \frac{4}{3}iD^{ki}{}_{lm} \mathcal{D}^\dagger \bar{\mathcal{L}} \Lambda_{\alpha k} \Lambda_{\beta n} \epsilon^{\alpha\beta} \varepsilon^{lmnj} \\
& + \frac{1}{6}iE_{kl}E^{ij} \mathcal{D}^\dagger \mathcal{D}^\dagger \bar{\mathcal{H}} \Lambda^{\dot{\alpha}k} \Lambda^{\dot{\beta}l} \epsilon_{\dot{\alpha}\dot{\beta}} + \frac{1}{6}iE_{kl}E^{kl} \mathcal{D}^\dagger \mathcal{D}^\dagger \bar{\mathcal{H}} \Lambda^{\dot{\alpha}i} \Lambda^{\dot{\beta}j} \epsilon_{\dot{\alpha}\dot{\beta}} + \frac{2}{3}iE_{kl} \mathcal{D}^\dagger \bar{\mathcal{H}} \Lambda^{\dot{\alpha}i} \chi^{\dot{\beta}}{}_{mn}{}^k \epsilon_{\dot{\alpha}\dot{\beta}} \varepsilon^{lmnj} - \frac{2}{3}iE_{kl} \mathcal{D}^\dagger \bar{\mathcal{H}} \Lambda^{\dot{\alpha}k} \chi^{\dot{\beta}}{}_{mn}{}^i \epsilon_{\dot{\alpha}\dot{\beta}} \varepsilon^{lmnj} \\
& - 4iE_{kl} \mathcal{D}\mathcal{H} \Lambda_{\alpha m} \chi_\beta{}^{ki}{}_n \epsilon^{\alpha\beta} \varepsilon^{lmnj} + \frac{4}{3}iE^{ki} P_a \mathcal{D}^\dagger \mathcal{D}^\dagger \bar{\mathcal{H}} \Lambda_{\alpha k} \Lambda^{\dot{\alpha}j} \gamma_a{}^\alpha{}_{\dot{\alpha}} - 4iP_a P_a \mathcal{D}^\dagger \mathcal{D}^\dagger \bar{\mathcal{L}} \Lambda^{\dot{\alpha}i} \Lambda^{\dot{\beta}j} \epsilon_{\dot{\alpha}\dot{\beta}} + \frac{80}{3}iP_a \Lambda^{\dot{\alpha}i} \Lambda^{\dot{\beta}j} \bar{\mathcal{L}} \bar{P}_a \epsilon_{\dot{\alpha}\dot{\beta}} \\
& + \frac{4}{3}i\mathcal{H} \Lambda^{\dot{\alpha}i} \Lambda^{\dot{\beta}j} \bar{P}_a \bar{P}_a \epsilon_{\dot{\alpha}\dot{\beta}} + (-12\bar{\mathcal{L}} - \frac{4}{3}\mathcal{D}^\dagger \mathcal{D}^\dagger \bar{\mathcal{H}})iE^{ij} P_a \Lambda_{\alpha k} \Lambda^{\dot{\alpha}k} \gamma_a{}^\alpha{}_{\dot{\alpha}} + (-\frac{8}{9}\bar{\mathcal{H}} - \frac{16}{9}\mathcal{H})iE^{ki} \Lambda_{\alpha k} \Lambda^{\dot{\alpha}j} \bar{P}_a \gamma_a{}^\alpha{}_{\dot{\alpha}} \\
& + (-\frac{2}{3}\mathcal{D}^\dagger \bar{\mathcal{L}} - \mathcal{D}\mathcal{H})i\Lambda_{\alpha k} \Lambda_{\beta l} R(V)_{ab}{}^i{}_m \gamma_{ab}{}^{\alpha\beta} \varepsilon^{klmj} + (-\frac{5}{9}\bar{\mathcal{H}} + \frac{2}{9}\mathcal{H})iE^{kl} E^{ij} \Lambda_{\alpha k} \Lambda_{\beta l} \epsilon^{\alpha\beta} + (\frac{1}{6}\mathcal{D}\mathcal{D}\mathcal{H} - \frac{2}{3}\mathcal{L})iT_{ab}{}^{ki}T_{ab}{}^{lj} \Lambda_{\alpha k} \Lambda_{\beta l} \epsilon^{\alpha\beta} \\
& + (\frac{5}{9}\bar{\mathcal{H}} - \frac{5}{9}\mathcal{H})iE^{ki} E^{lj} \Lambda_{\alpha k} \Lambda_{\beta l} \epsilon^{\alpha\beta} + (\frac{8}{9}\bar{\mathcal{H}} + \frac{4}{9}\mathcal{H})iE^{ij} \Lambda_{\alpha k} \Lambda^{\dot{\alpha}k} \bar{P}_a \gamma_a{}^\alpha{}_{\dot{\alpha}} + (\frac{4}{3}\bar{\mathcal{L}} - \frac{1}{3}\mathcal{D}^\dagger \mathcal{D}^\dagger \bar{\mathcal{H}})iE_{kl} E^{ki} \Lambda^{\dot{\alpha}l} \Lambda^{\dot{\beta}j} \epsilon_{\dot{\alpha}\dot{\beta}} \\
& + (\frac{4}{3}\mathcal{D}^\dagger \bar{\mathcal{H}} - \frac{8}{3}\mathcal{D}\bar{\mathcal{L}})iP_a \Lambda_{\alpha k} \chi^{\dot{\alpha}}{}_{lm}{}^i \gamma_a{}^\alpha{}_{\dot{\alpha}} \varepsilon^{klmj} + (-\frac{1}{3}\mathcal{D}^\dagger \bar{\mathcal{H}} - \frac{2}{3}\mathcal{D}\bar{\mathcal{L}})iT_{ab}{}^{kl}T_{ab}{}^{mn} \Lambda^{\dot{\alpha}i} \Lambda^{\dot{\beta}j} \epsilon_{\dot{\alpha}\dot{\beta}} \varepsilon_{klmn} \\
& + (-\frac{1}{48}\mathcal{D}\mathcal{D}\mathcal{H} - \frac{5}{12}\mathcal{L})iT_{ab}{}^{ki}T_{cd}{}^{lj} \Lambda_{\alpha k} \Lambda_{\beta l} \gamma_{ab}\gamma^\alpha\gamma_{cd}{}^{\beta\gamma} + (\frac{7}{16}\mathcal{D}\mathcal{D}\mathcal{H} + \frac{3}{4}\mathcal{L})iT_{ab}{}^{ki}T_{cd}{}^{lj} \Lambda_{\alpha k} \Lambda_{\beta l} \gamma_{ab}\gamma^\beta\gamma_{cd}{}^{\alpha\gamma} \\
& + (\frac{2}{3}\mathcal{D}^\dagger \bar{\mathcal{H}} + \frac{4}{3}\mathcal{D}\bar{\mathcal{L}})iT_{ab}{}^{kl}T_{ab}{}^{mi} \Lambda^{\dot{\alpha}n} \Lambda^{\dot{\beta}j} \epsilon_{\dot{\alpha}\dot{\beta}} \varepsilon_{klmn} + \frac{1}{4}iE_{kl}E_{mn} \mathcal{D}\mathcal{D}\mathcal{H} \Lambda_{\alpha p} \Lambda_{\beta q} \epsilon^{\alpha\beta} \varepsilon^{kmpi} \varepsilon^{lnqj} - \frac{1}{6}iT_{abkl}T_{cdmn} \mathcal{D}^\dagger \bar{\mathcal{L}} \Lambda^{\dot{\alpha}i} \Lambda^{\dot{\beta}j} \gamma_{ab\dot{\alpha}\dot{\gamma}} \gamma_{cd}{}^{\dot{\gamma}}{}_{\dot{\beta}} \varepsilon^{klmn} \\
& - \frac{1}{3}iT_{abkl}T_{cdmn} \mathcal{D}^\dagger \bar{\mathcal{L}} \Lambda^{\dot{\alpha}k} \Lambda^{\dot{\beta}i} \gamma_{ab\dot{\alpha}\dot{\gamma}} \gamma_{cd}{}^{\dot{\gamma}}{}_{\dot{\beta}} \varepsilon^{lmnj} - i\mathcal{H}T_{abkl}T_{abmn} \Lambda_{\alpha p} \Lambda_{\beta q} \epsilon^{\alpha\beta} \varepsilon^{kmpi} \varepsilon^{lnqj} + (-\frac{1}{6}\bar{\mathcal{H}} + \frac{1}{6}\mathcal{H})iT_{abkl}T_{abmn} \Lambda_{\alpha p} \Lambda_{\beta q} \epsilon^{\alpha\beta} \varepsilon^{klpi} \varepsilon^{mnqj}
\end{aligned}$$

The four fermion terms are:

$$\begin{aligned}
[\mathcal{E}^{ij}]_4 = & -\frac{4}{3} i\Lambda_{\alpha k} \Lambda^{\dot{\alpha} k} \Lambda^{\dot{\beta} i} \bar{\mathcal{L}} \epsilon_{\dot{\alpha} \dot{\beta}} \gamma_a{}^\alpha{}_{\dot{\gamma}} \nabla_a \Lambda^{\dot{\gamma} j} + \frac{4}{3} i\Lambda_{\alpha k} \Lambda^{\dot{\alpha} k} \Lambda^{\dot{\beta} i} \bar{\mathcal{L}} \epsilon_{\dot{\alpha} \dot{\gamma}} \gamma_a{}^\alpha{}_{\dot{\beta}} \nabla_a \Lambda^{\dot{\gamma} j} - \frac{2}{3} i\Lambda^{\dot{\alpha} i} \Lambda^{\dot{\beta} j} \Lambda^{\dot{\gamma} k} \bar{\mathcal{L}} \epsilon_{\dot{\alpha} \dot{\beta}} \gamma_a{}^\alpha{}_{\dot{\gamma}} \nabla_a \Lambda_{\alpha k} + 4 i\Lambda^{\dot{\alpha} k} \Lambda^{\dot{\beta} i} \Lambda^{\dot{\gamma} j} \bar{\mathcal{L}} \epsilon_{\dot{\alpha} \dot{\beta}} \gamma_a{}^\alpha{}_{\dot{\gamma}} \nabla_a \Lambda_{\alpha k} \\
& + \frac{8}{3} i\mathcal{D}^\dagger \bar{\mathcal{L}} \Lambda^{\dot{\alpha} k} \Lambda^{\dot{\beta} l} \Lambda^{\dot{\gamma} i} \chi^{\dot{\delta}}{}_{kl} \epsilon_{\dot{\alpha} \dot{\gamma}} \epsilon_{\dot{\beta} \dot{\delta}} + (-\frac{4}{3} \mathcal{D}^\dagger \bar{\mathcal{H}} + \frac{8}{3} \mathcal{D} \bar{\mathcal{L}}) i\Lambda_{\alpha k} \Lambda^{\dot{\alpha} l} \Lambda^{\dot{\beta} i} \chi_{\beta}{}^{kj} \epsilon^{\alpha\beta} \epsilon_{\dot{\alpha} \dot{\beta}} + (\frac{2}{3} \bar{\mathcal{L}} + \frac{1}{2} \mathcal{D}^\dagger \mathcal{D}^\dagger \bar{\mathcal{H}}) i\Lambda_{\alpha k} \Lambda^{\dot{\alpha} i} \Lambda^{\dot{\beta} j} \epsilon_{\dot{\alpha} \dot{\beta}} \gamma_a{}^\alpha{}_{\dot{\gamma}} \nabla_a \Lambda^{\dot{\gamma} k} \\
& + (\frac{20}{3} \bar{\mathcal{L}} + \frac{1}{3} \mathcal{D}^\dagger \mathcal{D}^\dagger \bar{\mathcal{H}}) i\Lambda_{\alpha k} \Lambda^{\dot{\alpha} i} \Lambda^{\dot{\beta} j} \epsilon_{\dot{\alpha} \dot{\gamma}} \gamma_a{}^\alpha{}_{\dot{\beta}} \nabla_a \Lambda^{\dot{\gamma} k} + (12 \bar{\mathcal{L}} + \frac{4}{3} \mathcal{D}^\dagger \mathcal{D}^\dagger \bar{\mathcal{H}}) i\Lambda_{\alpha k} \Lambda^{\dot{\alpha} k} \Lambda^{\dot{\beta} i} \epsilon_{\dot{\beta} \dot{\gamma}} \gamma_a{}^\alpha{}_{\dot{\alpha}} \nabla_a \Lambda^{\dot{\gamma} j} \\
& - \frac{2}{3} i\Lambda_{\alpha k} \Lambda_{\beta l} \Lambda^{\dot{\alpha} i} \bar{\mathcal{H}} \chi^{\dot{\beta}}{}_{mn} \epsilon^{\alpha\beta} \epsilon_{\dot{\alpha} \dot{\beta}} \varepsilon^{lmnj} - 2 i\Lambda_{\alpha k} \Lambda_{\beta l} \Lambda^{\dot{\alpha} k} \bar{\mathcal{H}} \chi^{\dot{\beta}}{}_{mn} \epsilon^{\alpha\beta} \epsilon_{\dot{\alpha} \dot{\beta}} \varepsilon^{lmnj} + (-\frac{56}{9} \mathcal{D}^\dagger \bar{\mathcal{L}} - \frac{4}{9} \mathcal{D}^\dagger \mathcal{D}^\dagger \mathcal{D}^\dagger \bar{\mathcal{H}}) iP_a \Lambda_{\alpha k} \Lambda^{\dot{\alpha} k} \Lambda^{\dot{\beta} i} \Lambda^{\dot{\gamma} j} \epsilon_{\dot{\alpha} \dot{\beta}} \gamma_a{}^\alpha{}_{\dot{\gamma}} \\
& + (-\frac{26}{9} \mathcal{D}^\dagger \bar{\mathcal{H}} - \frac{8}{9} \mathcal{D} \bar{\mathcal{L}}) iE^{ki} \Lambda_{\alpha k} \Lambda_{\beta l} \Lambda^{\dot{\alpha} l} \Lambda^{\dot{\beta} j} \epsilon^{\alpha\beta} \epsilon_{\dot{\alpha} \dot{\beta}} + (-\frac{16}{9} \mathcal{D}^\dagger \bar{\mathcal{H}} - \frac{64}{9} \mathcal{D} \bar{\mathcal{L}}) i\Lambda_{\alpha k} \Lambda^{\dot{\alpha} k} \Lambda^{\dot{\beta} i} \Lambda^{\dot{\gamma} j} \bar{P}_a \epsilon_{\dot{\alpha} \dot{\beta}} \gamma_a{}^\alpha{}_{\dot{\gamma}} \\
& + (-\frac{4}{3} \mathcal{D}^\dagger \bar{\mathcal{L}} - \frac{2}{3} \mathcal{D} \mathcal{H}) i\Lambda_{\alpha k} \Lambda_{\beta l} \Lambda^{\dot{\alpha} i} \epsilon^{\alpha\gamma} \gamma_a{}^\beta{}_{\dot{\alpha}} \nabla_a \Lambda_{\gamma m} \varepsilon^{klmj} + (-\frac{11}{9} \mathcal{D}^\dagger \bar{\mathcal{H}} + \frac{10}{9} \mathcal{D} \bar{\mathcal{L}}) i\Lambda_{\alpha k} \Lambda^{\dot{\alpha} k} \Lambda^{\dot{\beta} i} \Lambda^{\dot{\gamma} j} \bar{P}_a \epsilon_{\dot{\beta} \dot{\gamma}} \gamma_a{}^\alpha{}_{\dot{\alpha}} \\
& + (-\frac{4}{9} \mathcal{D}^\dagger \bar{\mathcal{L}} - \frac{1}{18} \mathcal{D}^\dagger \mathcal{D}^\dagger \mathcal{D}^\dagger \bar{\mathcal{H}}) iE_{kl} \Lambda^{\dot{\alpha} k} \Lambda^{\dot{\beta} l} \Lambda^{\dot{\gamma} i} \Lambda^{\dot{\delta} j} \epsilon_{\dot{\alpha} \dot{\beta}} \epsilon_{\dot{\gamma} \dot{\delta}} + (-\frac{1}{6} \mathcal{D} \mathcal{D} \mathcal{H} + \frac{2}{3} \mathcal{L}) i\Lambda_{\alpha k} \Lambda_{\beta l} \Lambda_{\gamma m} R(Q)_{ab\delta}{}^i \epsilon^{\alpha\delta} \gamma_{ab}{}^{\beta\gamma} \varepsilon^{klmj} \\
& + (-\frac{1}{9} \mathcal{D}^\dagger \bar{\mathcal{H}} - \frac{4}{9} \mathcal{D} \bar{\mathcal{L}}) iE^{kl} \Lambda_{\alpha k} \Lambda_{\beta l} \Lambda^{\dot{\alpha} i} \Lambda^{\dot{\beta} j} \epsilon^{\alpha\beta} \epsilon_{\dot{\alpha} \dot{\beta}} + (\frac{8}{9} \mathcal{D}^\dagger \bar{\mathcal{L}} - \frac{1}{18} \mathcal{D}^\dagger \mathcal{D}^\dagger \mathcal{D}^\dagger \bar{\mathcal{H}}) iE_{kl} \Lambda^{\dot{\alpha} k} \Lambda^{\dot{\beta} l} \Lambda^{\dot{\gamma} i} \Lambda^{\dot{\delta} j} \epsilon_{\dot{\alpha} \dot{\gamma}} \epsilon_{\dot{\beta} \dot{\delta}} \\
& + (\mathcal{D}^\dagger \bar{\mathcal{H}} - \frac{8}{3} \mathcal{D} \bar{\mathcal{L}}) iE^{ij} \Lambda_{\alpha k} \Lambda_{\beta l} \Lambda^{\dot{\alpha} k} \Lambda^{\dot{\beta} l} \epsilon^{\alpha\beta} \epsilon_{\dot{\alpha} \dot{\beta}} + (\frac{4}{3} \mathcal{D} \mathcal{D} \mathcal{H} + \frac{8}{3} \mathcal{L}) i\Lambda_{\alpha k} \Lambda_{\beta l} \Lambda_{\gamma m} \chi_{\delta}{}^{ki} \epsilon^{\alpha\beta} \epsilon^{\gamma\delta} \varepsilon^{lmnj} \\
& + (\frac{62}{9} \mathcal{D}^\dagger \bar{\mathcal{L}} + \frac{4}{9} \mathcal{D}^\dagger \mathcal{D}^\dagger \mathcal{D}^\dagger \bar{\mathcal{H}}) iP_a \Lambda_{\alpha k} \Lambda^{\dot{\alpha} k} \Lambda^{\dot{\beta} i} \Lambda^{\dot{\gamma} j} \epsilon_{\dot{\beta} \dot{\gamma}} \gamma_a{}^\alpha{}_{\dot{\alpha}} - \frac{1}{12} iE_{kl} \mathcal{D} \mathcal{D} \mathcal{D} \mathcal{H} \Lambda_{\alpha m} \Lambda_{\beta n} \Lambda_{\gamma p} \Lambda_{\delta q} \epsilon^{\alpha\beta} \epsilon^{\gamma\delta} \varepsilon^{kmpi} \varepsilon^{lnqj}
\end{aligned}$$

The six fermion terms are:

$$\begin{aligned}
[\mathcal{E}^{ij}]_6 = & (-\frac{20}{3} \bar{\mathcal{L}} - \frac{7}{6} \mathcal{D}^\dagger \mathcal{D}^\dagger \bar{\mathcal{H}}) i\Lambda_{\alpha k} \Lambda_{\beta l} \Lambda^{\dot{\alpha} k} \Lambda^{\dot{\beta} l} \Lambda^{\dot{\gamma} i} \Lambda^{\dot{\delta} j} \epsilon^{\alpha\beta} \epsilon_{\dot{\alpha} \dot{\gamma}} \epsilon_{\dot{\beta} \dot{\delta}} + (-\frac{14}{3} \bar{\mathcal{L}} - \frac{7}{6} \mathcal{D}^\dagger \mathcal{D}^\dagger \bar{\mathcal{H}}) i\Lambda_{\alpha k} \Lambda_{\beta l} \Lambda^{\dot{\alpha} k} \Lambda^{\dot{\beta} l} \Lambda^{\dot{\gamma} i} \Lambda^{\dot{\delta} j} \epsilon^{\alpha\beta} \epsilon_{\dot{\alpha} \dot{\beta}} \epsilon_{\dot{\gamma} \dot{\delta}} \\
& + \frac{1}{144} i\mathcal{D} \mathcal{D} \mathcal{D} \mathcal{D} \mathcal{H} \Lambda_{\alpha k} \Lambda_{\beta l} \Lambda_{\gamma m} \Lambda_{\delta n} \Lambda_{\epsilon p} \Lambda_{\epsilon l q} \epsilon^{\alpha\beta} \epsilon^{\gamma\delta} \epsilon^{\epsilon\zeta} \varepsilon^{kmpi} \varepsilon^{lnqj}
\end{aligned}$$

$\mathcal{E}_a^i{}^j$

We give the terms of  $\mathcal{E}_a^i{}^j$  grouped by number of fermions. Projection onto the **15** is assumed (i.e. SU(4) traces must be removed). The zero fermion terms are:

$$\begin{aligned}
[\mathcal{E}_{aj}^i]_0 = & \left(-\frac{16}{3}\bar{\mathcal{H}} + \frac{16}{3}\mathcal{H}\right)\nabla_b R(V)_{ab}{}^i{}_j + \frac{32}{3}E_{jk}\mathcal{D}^\dagger\mathcal{I}\nabla_b T_{ab}{}^{ik} + \frac{32}{3}E^{ik}\mathcal{D}\bar{\mathcal{I}}\nabla_b T_{abjk} + \frac{32}{3}P_b\mathcal{D}\bar{\mathcal{I}}R(V)_{ab}{}^i{}_j + \frac{32}{3}T_{abjk}\mathcal{D}\bar{\mathcal{I}}\nabla_b E^{ik} \\
& + \frac{32}{3}T_{ab}{}^{ik}\mathcal{D}^\dagger\mathcal{I}\nabla_b E_{jk} - \frac{32}{3}\mathcal{D}^\dagger\mathcal{I}R(V)_{ab}{}^i{}_j\bar{P}_b + \left(-\frac{16}{3}\bar{\mathcal{H}} + \frac{16}{3}\mathcal{H}\right)T_{bcjk}\nabla_b T_{ac}{}^{ik} + \left(-\frac{16}{3}\bar{\mathcal{H}} + \frac{16}{3}\mathcal{H}\right)T_{ab}{}^{ik}\nabla_c T_{bcjk} \\
& + \left(-\frac{8}{3}\bar{\mathcal{H}} + \frac{8}{3}\mathcal{H}\right)T_{bc}{}^{ik}\nabla_a T_{bcjk} + \left(-\frac{4}{3}\bar{\mathcal{H}} + \frac{4}{3}\mathcal{H}\right)E^{ik}\nabla_a E_{jk} + \left(\frac{4}{3}\bar{\mathcal{H}} - \frac{4}{3}\mathcal{H}\right)E_{jk}\nabla_a E^{ik} + \left(\frac{8}{3}\bar{\mathcal{H}} - \frac{8}{3}\mathcal{H}\right)T_{bcjk}\nabla_a T_{bc}{}^{ik} \\
& + (16\bar{\mathcal{H}} - 16\mathcal{H})T_{abjk}\nabla_c T_{bc}{}^{ik} + (16\bar{\mathcal{H}} - 16\mathcal{H})T_{bc}{}^{ik}\nabla_b T_{acjk} - \frac{8}{3}E_{jk}E^{ik}P_a\mathcal{D}\bar{\mathcal{I}} - \frac{8}{3}E_{jk}E^{ik}\mathcal{D}^\dagger\mathcal{I}\bar{P}_a + \frac{16}{3}P_a T_{bcjk}T_{bc}{}^{ik}\mathcal{D}\bar{\mathcal{I}} \\
& - 32P_b T_{acjk}T_{bc}{}^{ik}\mathcal{D}\bar{\mathcal{I}} - \frac{32}{3}P_b T_{bcjk}T_{ac}{}^{ik}\mathcal{D}\bar{\mathcal{I}} + \frac{16}{3}P_b\mathcal{D}\bar{\mathcal{I}}R(V)_{cd}{}^i{}_j\varepsilon_{abcd} + 32T_{abjk}T_{bc}{}^{ik}\mathcal{D}^\dagger\mathcal{I}\bar{P}_c + \frac{32}{3}T_{bcjk}T_{ab}{}^{ik}\mathcal{D}^\dagger\mathcal{I}\bar{P}_c \\
& + \frac{16}{3}T_{bcjk}T_{bc}{}^{ik}\mathcal{D}^\dagger\mathcal{I}\bar{P}_a + \frac{25}{6}T_{abjk}\mathcal{D}\bar{\mathcal{I}}\nabla_c T_{bclm}\varepsilon^{iklm} - \frac{13}{2}T_{abkl}\mathcal{D}\bar{\mathcal{I}}\nabla_c T_{bcjm}\varepsilon^{iklm} + \frac{19}{12}T_{bcjk}\mathcal{D}\bar{\mathcal{I}}\nabla_a T_{bclm}\varepsilon^{iklm} \\
& + \frac{25}{6}T_{bcjk}\mathcal{D}\bar{\mathcal{I}}\nabla_b T_{aclm}\varepsilon^{iklm} + \frac{19}{12}T_{bckl}\mathcal{D}\bar{\mathcal{I}}\nabla_a T_{bcjm}\varepsilon^{iklm} - \frac{13}{2}T_{bckl}\mathcal{D}\bar{\mathcal{I}}\nabla_b T_{acjm}\varepsilon^{iklm} + \frac{25}{6}T_{ab}{}^{ik}\mathcal{D}^\dagger\mathcal{I}\nabla_c T_{bc}{}^{lm}\varepsilon_{jklm} \\
& - \frac{13}{2}T_{ab}{}^{kl}\mathcal{D}^\dagger\mathcal{I}\nabla_c T_{bc}{}^{im}\varepsilon_{jklm} + \frac{19}{12}T_{bc}{}^{ik}\mathcal{D}^\dagger\mathcal{I}\nabla_a T_{bc}{}^{lm}\varepsilon_{jklm} + \frac{25}{6}T_{bc}{}^{ik}\mathcal{D}^\dagger\mathcal{I}\nabla_b T_{ac}{}^{lm}\varepsilon_{jklm} + \frac{19}{12}T_{bc}{}^{kl}\mathcal{D}^\dagger\mathcal{I}\nabla_a T_{bc}{}^{im}\varepsilon_{jklm} \\
& - \frac{13}{2}T_{bc}{}^{kl}\mathcal{D}^\dagger\mathcal{I}\nabla_b T_{ac}{}^{im}\varepsilon_{jklm} + \frac{16}{3}\mathcal{D}^\dagger\mathcal{I}R(V)_{bc}{}^i{}_j\bar{P}_d\varepsilon_{abcd} + \left(-\frac{128}{3}\bar{\mathcal{I}} - \frac{16}{3}\mathcal{D}^\dagger\mathcal{D}^\dagger\bar{\mathcal{H}}\right)E^{ik}P_b T_{abjk} + \left(-\frac{16}{3}\mathcal{D}\mathcal{D}\mathcal{H} - \frac{128}{3}\mathcal{I}\right)E_{jk}T_{ab}{}^{ik}\bar{P}_b
\end{aligned}$$

The two fermion terms are:

$$\begin{aligned}
[\mathcal{E}_{aj}]_2 = & +(-\frac{8}{3}\bar{\mathcal{H}} + \frac{8}{3}\mathcal{H})E^{ik}\nabla_b T_{ab}{}^{lm}\varepsilon_{jklm} + (-\frac{8}{3}\bar{\mathcal{H}} + \frac{8}{3}\mathcal{H})T_{ab}{}^{kl}\nabla_b E^{im}\varepsilon_{jklm} + (\frac{8}{3}\bar{\mathcal{H}} - \frac{8}{3}\mathcal{H})E_{jk}\nabla_b T_{ablm}\varepsilon^{iklm} + (\frac{8}{3}\bar{\mathcal{H}} - \frac{8}{3}\mathcal{H})T_{abkl}\nabla_b E_{jm}\varepsilon^{iklm} \\
& - \frac{16}{3}E_{jk}P_b T_{ablm}\mathcal{D}\bar{\mathcal{L}}\varepsilon^{iklm} + \frac{16}{3}E_{jk}T_{ablm}\mathcal{D}^\dagger\mathcal{I}\bar{P}_b\varepsilon^{iklm} + \frac{16}{3}E^{ik}P_b T_{ab}{}^{lm}\mathcal{D}\bar{\mathcal{L}}\varepsilon_{jklm} - \frac{16}{3}E^{ik}T_{ab}{}^{lm}\mathcal{D}^\dagger\mathcal{I}\bar{P}_b\varepsilon_{jklm} \\
& + (-\frac{64}{3}\bar{\mathcal{L}} - \frac{8}{3}\mathcal{D}^\dagger\mathcal{D}^\dagger\bar{\mathcal{H}})P_b T_{ackl}T_{bcjm}\varepsilon^{iklm} + (-\frac{38}{3}\bar{\mathcal{L}} - \frac{13}{12}\mathcal{D}^\dagger\mathcal{D}^\dagger\bar{\mathcal{H}})P_a T_{bcjk}T_{bclm}\varepsilon^{iklm} + (-\frac{16}{3}\bar{\mathcal{H}} + \frac{16}{3}\mathcal{H})P_b T_{ac}{}^{kl}T_{bc}{}^{im}\varepsilon_{jklm} \\
& + (-\frac{16}{3}\bar{\mathcal{H}} + \frac{16}{3}\mathcal{H})T_{abkl}T_{bcjm}\bar{P}_c\varepsilon^{iklm} + (-\frac{8}{3}\mathcal{D}\mathcal{D}\mathcal{H} - \frac{64}{3}\mathcal{I})T_{ab}{}^{ik}T_{bc}{}^{lm}\bar{P}_c\varepsilon_{jklm} + (-2\bar{\mathcal{H}} + 4\mathcal{H})P_a T_{bc}{}^{ik}T_{bc}{}^{lm}\varepsilon_{jklm} \\
& + (-\frac{13}{12}\mathcal{D}\mathcal{D}\mathcal{H} - \frac{38}{3}\mathcal{I})T_{bc}{}^{ik}T_{bc}{}^{lm}\bar{P}_a\varepsilon_{jklm} + (\frac{8}{3}\mathcal{D}\mathcal{D}\mathcal{H} + \frac{64}{3}\mathcal{I})T_{ab}{}^{kl}T_{bc}{}^{im}\bar{P}_c\varepsilon_{jklm} + (4\bar{\mathcal{H}} - 2\mathcal{H})T_{bcjk}T_{bclm}\bar{P}_a\varepsilon^{iklm} \\
& + (\frac{16}{3}\bar{\mathcal{H}} - \frac{16}{3}\mathcal{H})P_b T_{ac}{}^{ik}T_{bc}{}^{lm}\varepsilon_{jklm} + (\frac{16}{3}\bar{\mathcal{H}} - \frac{16}{3}\mathcal{H})T_{abjk}T_{bclm}\bar{P}_c\varepsilon^{iklm} + (\frac{64}{3}\bar{\mathcal{L}} + \frac{8}{3}\mathcal{D}^\dagger\mathcal{D}^\dagger\bar{\mathcal{H}})P_b T_{ackl}T_{bclm}\varepsilon^{iklm} \\
& - \frac{32}{3}\mathcal{D}^\dagger\mathcal{I}\Lambda_{\alpha j}\epsilon^{\alpha\beta}\nabla_b R(Q)_{ab\beta}{}^i - \frac{32}{3}\mathcal{D}^\dagger\mathcal{I}R(Q)_{ab\alpha}{}^i\epsilon^{\alpha\beta}\nabla_b\Lambda_{\beta j} - \frac{16}{3}\mathcal{D}^\dagger\mathcal{I}\chi_{\alpha}{}^{ik}{}_j\gamma_{ab}{}^{\alpha\beta}\nabla_b\Lambda_{\beta k} - \frac{32}{3}\mathcal{D}\bar{\mathcal{L}}\Lambda^{\dot{\alpha}i}\epsilon_{\dot{\alpha}\dot{\beta}}\nabla_b R(Q)_{ab}{}^{\dot{\beta}}{}_j \\
& - \frac{32}{3}\mathcal{D}\bar{\mathcal{L}}R(Q)_{ab}{}^{\dot{\alpha}}{}_j\epsilon_{\dot{\alpha}\dot{\beta}}\nabla_b\Lambda^{\dot{\beta}i} - \frac{16}{3}\mathcal{D}\bar{\mathcal{L}}\chi^{\dot{\alpha}}{}_{jk}{}_i\gamma_{ab\dot{\alpha}\dot{\beta}}\nabla_b\Lambda^{\dot{\beta}k} + (-8\mathcal{D}^\dagger\mathcal{I} - 4\mathcal{D}\mathcal{H})\Lambda_{\alpha k}\epsilon^{\alpha\beta}\nabla_a\chi_{\beta}{}^{ik}{}_j + (-\frac{16}{3}\bar{\mathcal{H}} + \frac{16}{3}\mathcal{H})\chi_{\alpha}{}^{ik}{}_l\chi^{\dot{\alpha}}{}_{jk}{}_l\gamma_a{}^{\alpha}{}_{\dot{\alpha}} \\
& + (-4\mathcal{D}^\dagger\bar{\mathcal{H}} - 8\mathcal{D}\bar{\mathcal{L}})\Lambda^{\dot{\alpha}k}\epsilon_{\dot{\alpha}\dot{\beta}}\nabla_a\chi^{\dot{\beta}}{}_{jk}{}_i + (-4\mathcal{D}^\dagger\bar{\mathcal{H}} - \frac{8}{3}\mathcal{D}\bar{\mathcal{L}})\Lambda^{\dot{\alpha}k}\gamma_{ab\dot{\alpha}\dot{\beta}}\nabla_b\chi^{\dot{\beta}}{}_{jk}{}_i + (-\frac{8}{3}\mathcal{D}^\dagger\mathcal{I} - 4\mathcal{D}\mathcal{H})\Lambda_{\alpha k}\gamma_{ab}{}^{\alpha\beta}\nabla_b\chi_{\beta}{}^{ik}{}_j \\
& + (-\frac{4}{3}\bar{\mathcal{H}} + \frac{4}{3}\mathcal{H})\Lambda^{\dot{\alpha}i}\gamma_a{}^{\alpha}{}_{\dot{\alpha}}\nabla_b\nabla_b\Lambda_{\alpha j} + (-\frac{4}{3}\bar{\mathcal{H}} + \frac{4}{3}\mathcal{H})\gamma_b{}^{\alpha}{}_{\dot{\alpha}}\nabla_a\Lambda_{\alpha j}\nabla_b\Lambda^{\dot{\alpha}i} + (-\frac{4}{3}\bar{\mathcal{H}} + \frac{4}{3}\mathcal{H})\gamma_b{}^{\alpha}{}_{\dot{\alpha}}\nabla_b\Lambda_{\alpha j}\nabla_a\Lambda^{\dot{\alpha}i} \\
& + (\frac{4}{3}\bar{\mathcal{H}} - \frac{4}{3}\mathcal{H})\Lambda_{\alpha j}\gamma_a{}^{\alpha}{}_{\dot{\alpha}}\nabla_b\nabla_b\Lambda^{\dot{\alpha}i} + (\frac{4}{3}\bar{\mathcal{H}} - \frac{4}{3}\mathcal{H})\gamma_a{}^{\alpha}{}_{\dot{\alpha}}\nabla_b\Lambda_{\alpha j}\nabla_b\Lambda^{\dot{\alpha}i} + (\frac{8}{3}\bar{\mathcal{H}} - \frac{8}{3}\mathcal{H})\chi_{\alpha}{}^{kl}{}_j\chi^{\dot{\alpha}}{}_{kl}{}_i\gamma_a{}^{\alpha}{}_{\dot{\alpha}} + \frac{4}{3}E_{jk}\mathcal{D}\bar{\mathcal{L}}\Lambda^{\dot{\alpha}i}\epsilon_{\dot{\alpha}\dot{\beta}}\nabla_a\Lambda^{\dot{\beta}k} \\
& + \frac{4}{3}E_{jk}\mathcal{D}\bar{\mathcal{L}}\Lambda^{\dot{\alpha}k}\epsilon_{\dot{\alpha}\dot{\beta}}\nabla_a\Lambda^{\dot{\beta}i} + \frac{4}{9}E_{jk}\mathcal{D}\bar{\mathcal{L}}\Lambda^{\dot{\alpha}i}\gamma_{ab\dot{\alpha}\dot{\beta}}\nabla_b\Lambda^{\dot{\beta}k} - \frac{4}{9}E_{jk}\mathcal{D}\bar{\mathcal{L}}\Lambda^{\dot{\alpha}k}\gamma_{ab\dot{\alpha}\dot{\beta}}\nabla_b\Lambda^{\dot{\beta}i} + 4E_{jk}\mathcal{H}\Lambda^{\dot{\alpha}l}\chi_{\alpha}{}^{ik}{}_l\gamma_a{}^{\alpha}{}_{\dot{\alpha}} \\
& - 4E_{kl}\mathcal{H}\Lambda^{\dot{\alpha}k}\chi_{\alpha}{}^{il}{}_j\gamma_a{}^{\alpha}{}_{\dot{\alpha}} + 4E^{ik}\Lambda_{\alpha l}\bar{\mathcal{H}}\chi^{\dot{\alpha}}{}_{jk}{}_l\gamma_a{}^{\alpha}{}_{\dot{\alpha}} - 4E^{kl}\Lambda_{\alpha k}\bar{\mathcal{H}}\chi^{\dot{\alpha}}{}_{jl}{}_i\gamma_a{}^{\alpha}{}_{\dot{\alpha}} + \frac{4}{3}E^{ik}\mathcal{D}^\dagger\mathcal{I}\Lambda_{\alpha j}\epsilon^{\alpha\beta}\nabla_a\Lambda_{\beta k} + \frac{4}{3}E^{ik}\mathcal{D}^\dagger\mathcal{I}\Lambda_{\alpha k}\epsilon^{\alpha\beta}\nabla_a\Lambda_{\beta j} \\
& + \frac{4}{9}E^{ik}\mathcal{D}^\dagger\mathcal{I}\Lambda_{\alpha j}\gamma_{ab}{}^{\alpha\beta}\nabla_b\Lambda_{\beta k} - \frac{4}{9}E^{ik}\mathcal{D}^\dagger\mathcal{I}\Lambda_{\alpha k}\gamma_{ab}{}^{\alpha\beta}\nabla_b\Lambda_{\beta j} - \frac{16}{9}P_a\mathcal{D}\bar{\mathcal{L}}\Lambda_{\alpha j}\gamma_b{}^{\alpha}{}_{\dot{\alpha}}\nabla_b\Lambda^{\dot{\alpha}i} - \frac{32}{9}P_b\mathcal{D}\bar{\mathcal{L}}\Lambda_{\alpha j}\gamma_a{}^{\alpha}{}_{\dot{\alpha}}\nabla_b\Lambda^{\dot{\alpha}i} \\
& - \frac{8}{9}P_a\mathcal{D}\bar{\mathcal{L}}\Lambda^{\dot{\alpha}i}\gamma_b{}^{\alpha}{}_{\dot{\alpha}}\nabla_b\Lambda_{\alpha j} + \frac{8}{9}P_b\mathcal{D}\bar{\mathcal{L}}\Lambda^{\dot{\alpha}i}\gamma_a{}^{\alpha}{}_{\dot{\alpha}}\nabla_b\Lambda_{\alpha j} - \frac{8}{3}P_b\mathcal{D}\bar{\mathcal{L}}\Lambda^{\dot{\alpha}i}\gamma_b{}^{\alpha}{}_{\dot{\alpha}}\nabla_a\Lambda_{\alpha j} - \frac{32}{3}T_{abjk}\mathcal{D}\bar{\mathcal{L}}\Lambda^{\dot{\alpha}l}\chi_{\alpha}{}^{ik}{}_l\gamma_b{}^{\alpha}{}_{\dot{\alpha}} \\
& + \frac{16}{3}T_{abki}\mathcal{D}\bar{\mathcal{L}}\Lambda^{\dot{\alpha}i}\chi_{\alpha}{}^{kl}{}_j\gamma_b{}^{\alpha}{}_{\dot{\alpha}} - \frac{32}{3}T_{ab}{}^{ik}\mathcal{D}^\dagger\mathcal{I}\Lambda_{\alpha l}\chi^{\dot{\alpha}}{}_{jk}{}_l\gamma_b{}^{\alpha}{}_{\dot{\alpha}} + \frac{16}{3}T_{ab}{}^{kl}\mathcal{D}^\dagger\mathcal{I}\Lambda_{\alpha j}\chi^{\dot{\alpha}}{}_{kl}{}_i\gamma_b{}^{\alpha}{}_{\dot{\alpha}} + 16\bar{\mathcal{L}}P_a\Lambda^{\dot{\alpha}k}\chi^{\dot{\beta}}{}_{jk}{}_i\epsilon_{\dot{\alpha}\dot{\beta}} \\
& - \frac{4}{3}\bar{\mathcal{L}}T_{bcjk}\Lambda^{\dot{\alpha}i}\gamma_{bc\dot{\alpha}\dot{\beta}}\nabla_a\Lambda^{\dot{\beta}k} + 4\bar{\mathcal{L}}T_{bcjk}\Lambda^{\dot{\alpha}k}\gamma_{bc\dot{\alpha}\dot{\beta}}\nabla_a\Lambda^{\dot{\beta}i} - \frac{16}{3}\bar{\mathcal{L}}\Lambda^{\dot{\alpha}i}\Lambda^{\dot{\beta}k}\gamma_{bc\dot{\alpha}\dot{\beta}}\nabla_a T_{bcjk} - \frac{4}{3}\mathcal{D}^\dagger\mathcal{D}^\dagger\bar{\mathcal{H}}\Lambda^{\dot{\alpha}i}\Lambda^{\dot{\beta}k}\gamma_{ab\dot{\alpha}\dot{\beta}}\nabla_c T_{bcjk} \\
& - \frac{4}{3}\mathcal{D}^\dagger\mathcal{D}^\dagger\bar{\mathcal{H}}\Lambda^{\dot{\alpha}i}\Lambda^{\dot{\beta}k}\gamma_{bc\dot{\alpha}\dot{\beta}}\nabla_b T_{acjk} - \frac{4}{3}\mathcal{D}^\dagger\mathcal{I}\Lambda_{\alpha j}\Lambda_{\beta k}\epsilon^{\alpha\beta}\nabla_a E^{ik} + \frac{4}{9}\mathcal{D}^\dagger\mathcal{I}\Lambda_{\alpha j}\Lambda_{\beta k}\gamma_{ab}{}^{\alpha\beta}\nabla_b E^{ik} + \frac{8}{9}\mathcal{D}^\dagger\mathcal{I}\Lambda_{\alpha j}\Lambda^{\dot{\alpha}i}\gamma_a{}^{\alpha}{}_{\dot{\alpha}}\nabla_b\bar{P}_b \\
& + \frac{16}{9}\mathcal{D}^\dagger\mathcal{I}\Lambda_{\alpha j}\Lambda^{\dot{\alpha}i}\gamma_b{}^{\alpha}{}_{\dot{\alpha}}\nabla_b\bar{P}_a - \frac{8}{9}\mathcal{D}^\dagger\mathcal{I}\Lambda_{\alpha j}\bar{P}_a\gamma_b{}^{\alpha}{}_{\dot{\alpha}}\nabla_b\Lambda^{\dot{\alpha}i} + \frac{8}{9}\mathcal{D}^\dagger\mathcal{I}\Lambda_{\alpha j}\bar{P}_b\gamma_a{}^{\alpha}{}_{\dot{\alpha}}\nabla_b\Lambda^{\dot{\alpha}i} - \frac{8}{3}\mathcal{D}^\dagger\mathcal{I}\Lambda_{\alpha j}\bar{P}_b\gamma_b{}^{\alpha}{}_{\dot{\alpha}}\nabla_a\Lambda^{\dot{\alpha}i} \\
& - \frac{16}{9}\mathcal{D}^\dagger\mathcal{I}\Lambda^{\dot{\alpha}i}\bar{P}_a\gamma_b{}^{\alpha}{}_{\dot{\alpha}}\nabla_b\Lambda_{\alpha j} - \frac{32}{9}\mathcal{D}^\dagger\mathcal{I}\Lambda^{\dot{\alpha}i}\bar{P}_b\gamma_a{}^{\alpha}{}_{\dot{\alpha}}\nabla_b\Lambda_{\alpha j} - \frac{8}{9}\mathcal{D}\bar{\mathcal{L}}\Lambda_{\alpha j}\Lambda^{\dot{\alpha}i}\gamma_a{}^{\alpha}{}_{\dot{\alpha}}\nabla_b P_b - \frac{16}{9}\mathcal{D}\bar{\mathcal{L}}\Lambda_{\alpha j}\Lambda^{\dot{\alpha}i}\gamma_b{}^{\alpha}{}_{\dot{\alpha}}\nabla_a P_a \\
& - \frac{4}{3}\mathcal{D}\bar{\mathcal{L}}\Lambda^{\dot{\alpha}i}\Lambda^{\dot{\beta}k}\epsilon_{\dot{\alpha}\dot{\beta}}\nabla_a E_{jk} + \frac{4}{9}\mathcal{D}\bar{\mathcal{L}}\Lambda^{\dot{\alpha}i}\Lambda^{\dot{\beta}k}\gamma_{ab\dot{\alpha}\dot{\beta}}\nabla_b E_{jk} - \frac{4}{3}\mathcal{D}\mathcal{D}\mathcal{H}\Lambda_{\alpha j}\Lambda_{\beta k}\gamma_{ab}{}^{\alpha\beta}\nabla_c T_{bc}{}^{ik} - \frac{4}{3}\mathcal{D}\mathcal{D}\mathcal{H}\Lambda_{\alpha j}\Lambda_{\beta k}\gamma_{bc}{}^{\alpha\beta}\nabla_b T_{ac}{}^{ik} + 1\cdots
\end{aligned}$$

$$\begin{aligned}
[\mathcal{E}_{aj}]_{2,cont} = & -\frac{4}{3}\mathcal{I}T_{bc}{}^{ik}\Lambda_{\alpha j}\gamma_{bc}{}^{\alpha\beta}\nabla_a\Lambda_{\beta k} + 4\mathcal{I}T_{bc}{}^{ik}\Lambda_{\alpha k}\gamma_{bc}{}^{\alpha\beta}\nabla_a\Lambda_{\beta j} - \frac{16}{3}\mathcal{I}\Lambda_{\alpha j}\Lambda_{\beta k}\gamma_{bc}{}^{\alpha\beta}\nabla_aT_{bc}{}^{ik} + 16\mathcal{I}\Lambda_{\alpha k}\bar{P}_a\chi_{\beta}{}^{ik}{}_j\epsilon^{\alpha\beta} \\
& + (-8\bar{\mathcal{I}} - \frac{4}{3}\mathcal{D}^\dagger\mathcal{D}^\dagger\bar{\mathcal{H}})T_{bcjk}\Lambda^{\dot{\alpha}i}\gamma_{ab\dot{\alpha}\dot{\beta}}\nabla_c\Lambda^{\dot{\beta}k} + (-\frac{16}{3}\bar{\mathcal{I}} - \frac{8}{3}\mathcal{D}^\dagger\mathcal{D}^\dagger\bar{\mathcal{H}})P_b\Lambda^{\dot{\alpha}k}\chi^{\dot{\beta}}{}_{jk}{}_i\gamma_{ab\dot{\alpha}\dot{\beta}} + (-\frac{16}{3}\bar{\mathcal{H}} + \frac{16}{3}\mathcal{H})\Lambda^{\dot{\alpha}i}R(Q)_{ab}{}^{\dot{\beta}}{}_j\bar{P}_b\epsilon_{\dot{\alpha}\dot{\beta}} \\
& + (-\frac{8}{3}\bar{\mathcal{I}} - \frac{4}{3}\mathcal{D}^\dagger\mathcal{D}^\dagger\bar{\mathcal{H}})T_{abjk}\Lambda^{\dot{\alpha}k}\gamma_{bc\dot{\alpha}\dot{\beta}}\nabla_c\Lambda^{\dot{\beta}i} + (-\frac{8}{3}\bar{\mathcal{H}} - \frac{8}{3}\mathcal{H})\Lambda_{\alpha j}\Lambda^{\dot{\alpha}k}R(V)_{ab}{}^i{}_k\gamma_b{}^\alpha{}_{\dot{\alpha}} + (-\frac{8}{3}\bar{\mathcal{H}} - \frac{8}{3}\mathcal{H})\Lambda_{\alpha k}\Lambda^{\dot{\alpha}i}R(V)_{ab}{}^k{}_j\gamma_b{}^\alpha{}_{\dot{\alpha}} \\
& + (-\frac{8}{3}\mathcal{D}\mathcal{D}\mathcal{H} - \frac{16}{3}\mathcal{I})\Lambda_{\alpha k}\bar{P}_b\chi_{\beta}{}^{ik}{}_j\gamma_{ab}{}^{\alpha\beta} + (-\frac{4}{3}\bar{\mathcal{H}} + \frac{4}{3}\mathcal{H})D^{ik}{}_{jl}\Lambda_{\alpha k}\Lambda^{\dot{\alpha}l}\gamma_a{}^\alpha{}_{\dot{\alpha}} + (-\frac{4}{3}\bar{\mathcal{H}} + \frac{4}{3}\mathcal{H})\gamma_b{}^\alpha{}_{\dot{\alpha}}\nabla_c\Lambda_{\alpha j}\nabla_d\Lambda^{\dot{\alpha}i}\epsilon_{abcd} \\
& + (-\frac{4}{3}\mathcal{D}\mathcal{D}\mathcal{H} - 8\mathcal{I})T_{bc}{}^{ik}\Lambda_{\alpha j}\gamma_{ab}{}^{\alpha\beta}\nabla_c\Lambda_{\beta k} + (-\frac{4}{3}\mathcal{D}\mathcal{D}\mathcal{H} - \frac{8}{3}\mathcal{I})T_{ab}{}^{ik}\Lambda_{\alpha k}\gamma_{bc}{}^{\alpha\beta}\nabla_c\Lambda_{\beta j} + (\frac{4}{3}\mathcal{D}\mathcal{D}\mathcal{H} + \frac{8}{3}\mathcal{I})T_{bc}{}^{ik}\Lambda_{\alpha k}\gamma_{ab}{}^{\alpha\beta}\nabla_c\Lambda_{\beta j} \\
& + (\frac{4}{3}\mathcal{D}\mathcal{D}\mathcal{H} + 8\mathcal{I})T_{ab}{}^{ik}\Lambda_{\alpha j}\gamma_{bc}{}^{\alpha\beta}\nabla_c\Lambda_{\beta k} + (\frac{8}{3}\bar{\mathcal{I}} + \frac{4}{3}\mathcal{D}^\dagger\mathcal{D}^\dagger\bar{\mathcal{H}})T_{bcjk}\Lambda^{\dot{\alpha}k}\gamma_{ab\dot{\alpha}\dot{\beta}}\nabla_c\Lambda^{\dot{\beta}i} + (\frac{8}{3}\mathcal{D}\mathcal{D}\mathcal{H} + \frac{16}{3}\mathcal{I})T_{ab}{}^{ik}\Lambda_{\alpha k}\epsilon^{\alpha\beta}\nabla_b\Lambda_{\beta j} \\
& + (\frac{8}{3}\mathcal{D}\mathcal{D}\mathcal{H} + \frac{32}{3}\mathcal{I})\Lambda_{\alpha j}\Lambda_{\beta k}\epsilon^{\alpha\beta}\nabla_bT_{ab}{}^{ik} + (\frac{8}{3}\mathcal{D}\mathcal{D}\mathcal{H} + \frac{80}{3}\mathcal{I})T_{ab}{}^{ik}\Lambda_{\alpha j}\epsilon^{\alpha\beta}\nabla_b\Lambda_{\beta k} + (4\bar{\mathcal{H}} + 4\mathcal{H})\Lambda_{\alpha k}\Lambda^{\dot{\alpha}k}R(V)_{ab}{}^i{}_j\gamma_b{}^\alpha{}_{\dot{\alpha}} \\
& + (\frac{16}{3}\bar{\mathcal{I}} + \frac{8}{3}\mathcal{D}^\dagger\mathcal{D}^\dagger\bar{\mathcal{H}})T_{abjk}\Lambda^{\dot{\alpha}k}\epsilon_{\dot{\alpha}\dot{\beta}}\nabla_b\Lambda^{\dot{\beta}i} + (\frac{16}{3}\bar{\mathcal{H}} - \frac{16}{3}\mathcal{H})P_b\Lambda_{\alpha j}R(Q)_{ab\beta}{}^i\epsilon^{\alpha\beta} + (\frac{16}{3}\mathcal{D}\mathcal{D}\mathcal{H} + \frac{128}{3}\mathcal{I})\Lambda_{\alpha j}R(Q)_{ab\beta}{}^i\bar{P}_b\epsilon^{\alpha\beta} \\
& + (8\bar{\mathcal{I}} + \frac{4}{3}\mathcal{D}^\dagger\mathcal{D}^\dagger\bar{\mathcal{H}})T_{abjk}\Lambda^{\dot{\alpha}i}\gamma_{bc\dot{\alpha}\dot{\beta}}\nabla_c\Lambda^{\dot{\beta}k} + (\frac{32}{3}\bar{\mathcal{I}} + \frac{8}{3}\mathcal{D}^\dagger\mathcal{D}^\dagger\bar{\mathcal{H}})\Lambda^{\dot{\alpha}i}\Lambda^{\dot{\beta}k}\epsilon_{\dot{\alpha}\dot{\beta}}\nabla_bT_{abjk} + (\frac{80}{3}\bar{\mathcal{I}} + \frac{8}{3}\mathcal{D}^\dagger\mathcal{D}^\dagger\bar{\mathcal{H}})T_{abjk}\Lambda^{\dot{\alpha}i}\epsilon_{\dot{\alpha}\dot{\beta}}\nabla_b\Lambda^{\dot{\beta}k} \\
& + (\frac{128}{3}\bar{\mathcal{I}} + \frac{16}{3}\mathcal{D}^\dagger\mathcal{D}^\dagger\bar{\mathcal{H}})P_b\Lambda^{\dot{\alpha}i}R(Q)_{ab}{}^{\dot{\beta}}{}_j\epsilon_{\dot{\alpha}\dot{\beta}} - \frac{8}{9}E_{jk}T_{ab}{}^{il}\mathcal{D}^\dagger\mathcal{I}\Lambda_{\alpha l}\Lambda^{\dot{\alpha}k}\gamma_b{}^\alpha{}_{\dot{\alpha}} - \frac{1}{48}E_{jk}\mathcal{D}^\dagger\mathcal{I}\Lambda_{\alpha l}\chi^{\dot{\alpha}}{}_{mn}{}_i\gamma_a{}^\alpha{}_{\dot{\alpha}}\epsilon^{klmn} \\
& - \frac{65}{48}E_{jk}\mathcal{D}^\dagger\mathcal{I}\Lambda_{\alpha l}\chi^{\dot{\alpha}}{}_{mn}{}_l\gamma_a{}^\alpha{}_{\dot{\alpha}}\epsilon^{ikmn} - \frac{3}{8}E_{kl}\mathcal{D}^\dagger\mathcal{I}\Lambda_{\alpha m}\chi^{\dot{\alpha}}{}_{jn}{}_k\gamma_a{}^\alpha{}_{\dot{\alpha}}\epsilon^{ilmn} + \frac{8}{9}E^{ik}T_{abjl}\mathcal{D}\bar{\mathcal{I}}\Lambda_{\alpha k}\Lambda^{\dot{\alpha}l}\gamma_b{}^\alpha{}_{\dot{\alpha}} \\
& - \frac{1}{48}E^{ik}\mathcal{D}\bar{\mathcal{I}}\Lambda^{\dot{\alpha}l}\chi_{\alpha}{}^{mn}{}_j\gamma_a{}^\alpha{}_{\dot{\alpha}}\epsilon_{klmn} - \frac{65}{48}E^{ik}\mathcal{D}\bar{\mathcal{I}}\Lambda^{\dot{\alpha}l}\chi_{\alpha}{}^{mn}{}_l\gamma_a{}^\alpha{}_{\dot{\alpha}}\epsilon_{jkln} - \frac{3}{8}E^{kl}\mathcal{D}\bar{\mathcal{I}}\Lambda^{\dot{\alpha}m}\chi_{\alpha}{}^{in}{}_k\gamma_a{}^\alpha{}_{\dot{\alpha}}\epsilon_{jlmn} \\
& - \frac{16}{9}P_b\mathcal{D}\bar{\mathcal{I}}\Lambda_{\alpha j}\gamma_c{}^\alpha{}_{\dot{\alpha}}\nabla_d\Lambda^{\dot{\alpha}i}\epsilon_{abcd} - \frac{8}{9}P_b\mathcal{D}\bar{\mathcal{I}}\Lambda^{\dot{\alpha}i}\gamma_c{}^\alpha{}_{\dot{\alpha}}\nabla_d\Lambda_{\alpha j}\epsilon_{abcd} - \frac{5}{3}T_{abkl}\Lambda_{\alpha j}\bar{\mathcal{H}}\chi^{\dot{\alpha}}{}_{mn}{}_i\gamma_b{}^\alpha{}_{\dot{\alpha}}\epsilon^{klmn} - 4T_{abjk}\mathcal{D}^\dagger\mathcal{I}\Lambda_{\alpha l}\epsilon^{\alpha\beta}\nabla_b\Lambda_{\beta m}\epsilon^{iklm} \\
& + \frac{4}{3}T_{bcjk}\mathcal{D}^\dagger\mathcal{I}\Lambda_{\alpha l}\gamma_{ab}{}^{\alpha\beta}\nabla_c\Lambda_{\beta m}\epsilon^{iklm} - 4T_{ab}{}^{ik}\mathcal{D}\bar{\mathcal{I}}\Lambda^{\dot{\alpha}l}\epsilon_{\dot{\alpha}\dot{\beta}}\nabla_b\Lambda^{\dot{\beta}m}\epsilon_{jklm} + \frac{4}{3}T_{bc}{}^{ik}\mathcal{D}\bar{\mathcal{I}}\Lambda^{\dot{\alpha}l}\gamma_{ab\dot{\alpha}\dot{\beta}}\nabla_c\Lambda^{\dot{\beta}m}\epsilon_{jklm} \\
& - 4\bar{\mathcal{I}}E^{ik}\Lambda^{\dot{\alpha}l}\epsilon_{\dot{\alpha}\dot{\beta}}\nabla_a\Lambda^{\dot{\beta}m}\epsilon_{jklm} - \frac{4}{3}\bar{\mathcal{H}}\Lambda_{\alpha k}\Lambda^{\dot{\alpha}i}R(V)_{bc}{}^k{}_j\gamma_d{}^\alpha{}_{\dot{\alpha}}\epsilon_{abcd} - \frac{16}{3}\mathcal{D}^\dagger\bar{\mathcal{I}}P_aT_{bcjk}\Lambda^{\dot{\alpha}i}\Lambda^{\dot{\beta}k}\gamma_{bc\dot{\alpha}\dot{\beta}} + \frac{4}{3}\mathcal{D}^\dagger\mathcal{I}\Lambda_{\alpha k}\Lambda_{\beta l}\gamma_{ab}{}^{\alpha\beta}\nabla_cT_{bcjm}\epsilon^{iklm} \\
& + \frac{8}{9}\mathcal{D}^\dagger\mathcal{I}\Lambda_{\alpha j}\Lambda^{\dot{\alpha}i}\gamma_b{}^\alpha{}_{\dot{\alpha}}\nabla_c\bar{P}_d\epsilon_{abcd} + \frac{8}{9}\mathcal{D}^\dagger\mathcal{I}\Lambda_{\alpha j}\bar{P}_b\gamma_c{}^\alpha{}_{\dot{\alpha}}\nabla_d\Lambda^{\dot{\alpha}i}\epsilon_{abcd} + \frac{16}{9}\mathcal{D}^\dagger\mathcal{I}\Lambda^{\dot{\alpha}i}\bar{P}_b\gamma_c{}^\alpha{}_{\dot{\alpha}}\nabla_d\Lambda_{\alpha j}\epsilon_{abcd} + \frac{8}{9}\mathcal{D}\bar{\mathcal{I}}\Lambda_{\alpha j}\Lambda^{\dot{\alpha}i}\gamma_b{}^\alpha{}_{\dot{\alpha}}\nabla_cP_d\epsilon_{abcd} \\
& + \frac{4}{3}\mathcal{D}\bar{\mathcal{I}}\Lambda^{\dot{\alpha}k}\Lambda^{\dot{\beta}l}\gamma_{ab\dot{\alpha}\dot{\beta}}\nabla_cT_{bc}{}^{im}\epsilon_{jklm} - \frac{16}{3}\mathcal{D}\bar{\mathcal{I}}T_{bc}{}^{ik}\Lambda_{\alpha j}\Lambda_{\beta k}\bar{P}_a\gamma_{bc}{}^{\alpha\beta} - 4\mathcal{I}E_{jk}\Lambda_{\alpha l}\epsilon^{\alpha\beta}\nabla_a\Lambda_{\beta m}\epsilon^{iklm} - \frac{5}{3}\mathcal{H}T_{ab}{}^{kl}\Lambda^{\dot{\alpha}i}\chi_{\alpha}{}^{mn}{}_j\gamma_b{}^\alpha{}_{\dot{\alpha}}\epsilon_{klmn} \\
& + \frac{4}{3}\mathcal{H}\Lambda_{\alpha j}\Lambda^{\dot{\alpha}k}R(V)_{bc}{}^i{}_k\gamma_d{}^\alpha{}_{\dot{\alpha}}\epsilon_{abcd} + (-6\mathcal{D}^\dagger\mathcal{I} - \frac{2}{3}\mathcal{D}\mathcal{H})T_{abkl}\Lambda_{\alpha j}\epsilon^{\alpha\beta}\nabla_b\Lambda_{\beta m}\epsilon^{iklm} + (-\frac{16}{3}\bar{\mathcal{I}} - \frac{2}{3}\mathcal{D}^\dagger\mathcal{D}^\dagger\bar{\mathcal{H}})E_{jk}P_a\Lambda^{\dot{\alpha}i}\Lambda^{\dot{\beta}k}\epsilon_{\dot{\alpha}\dot{\beta}} \\
& + (-\frac{16}{3}\mathcal{D}^\dagger\bar{\mathcal{I}} - \frac{4}{3}\mathcal{D}^\dagger\mathcal{D}^\dagger\bar{\mathcal{H}})P_bT_{acjk}\Lambda^{\dot{\alpha}i}\Lambda^{\dot{\beta}k}\gamma_{bc\dot{\alpha}\dot{\beta}} + (-\frac{16}{3}\mathcal{D}^\dagger\bar{\mathcal{H}} - \frac{16}{9}\mathcal{D}\bar{\mathcal{I}})T_{abjk}\Lambda^{\dot{\alpha}i}\Lambda^{\dot{\beta}k}\bar{P}_c\gamma_{bc\dot{\alpha}\dot{\beta}} \\
& + (-\frac{16}{3}\mathcal{D}^\dagger\bar{\mathcal{H}} - \frac{16}{9}\mathcal{D}\bar{\mathcal{I}})T_{bcjk}\Lambda^{\dot{\alpha}i}\Lambda^{\dot{\beta}k}\bar{P}_b\gamma_{ac\dot{\alpha}\dot{\beta}} + (-\frac{16}{3}\mathcal{D}^\dagger\bar{\mathcal{H}} + \frac{32}{9}\mathcal{D}\bar{\mathcal{I}})T_{abjk}\Lambda^{\dot{\alpha}i}\Lambda^{\dot{\beta}k}\bar{P}_b\epsilon_{\dot{\alpha}\dot{\beta}} + (-\frac{16}{3}\mathcal{D}^\dagger\mathcal{I} - \frac{4}{3}\mathcal{D}\mathcal{H})\Lambda_{\alpha j}\Lambda_{\beta k}\epsilon^{\alpha\beta}\nabla_bT_{ablm}\epsilon^{iklm} \\
& + (-\frac{16}{3}\mathcal{D}^\dagger\mathcal{I} + 4\mathcal{D}\mathcal{H})E_{kl}T_{ab}{}^{ik}\Lambda_{\alpha j}\Lambda^{\dot{\alpha}l}\gamma_b{}^\alpha{}_{\dot{\alpha}} + (-\frac{40}{9}\mathcal{D}^\dagger\mathcal{I} - \frac{8}{3}\mathcal{D}\mathcal{H})P_aT_{bc}{}^{ik}\Lambda_{\alpha j}\Lambda_{\beta k}\gamma_{bc}{}^{\alpha\beta} + (-4\bar{\mathcal{H}} + 4\mathcal{H})T_{bcjk}T_{ab}{}^{il}\Lambda_{\alpha l}\Lambda^{\dot{\alpha}k}\gamma_c{}^\alpha{}_{\dot{\alpha}} \\
& + (-4\mathcal{D}^\dagger\bar{\mathcal{H}} + \frac{16}{3}\mathcal{D}\bar{\mathcal{I}})E^{kl}T_{abjk}\Lambda_{\alpha l}\Lambda^{\dot{\alpha}i}\gamma_b{}^\alpha{}_{\dot{\alpha}} + (-\frac{10}{3}\bar{\mathcal{H}} - \frac{2}{3}\mathcal{H})T_{bckl}\Lambda_{\alpha m}R(Q)_{bc}{}^{\dot{\alpha}}{}_j\gamma_a{}^\alpha{}_{\dot{\alpha}}\epsilon^{iklm} \\
& + (-3\bar{\mathcal{H}} - 3\mathcal{H})T_{abkl}\Lambda_{\alpha m}\chi^{\dot{\alpha}}{}_{jn}{}_m\gamma_b{}^\alpha{}_{\dot{\alpha}}\epsilon^{ikln} + (-3\bar{\mathcal{H}} - 3\mathcal{H})T_{ab}{}^{kl}\Lambda^{\dot{\alpha}m}\chi_{\alpha}{}^{in}{}_m\gamma_b{}^\alpha{}_{\dot{\alpha}}\epsilon_{jklm} + (-\frac{8}{3}\mathcal{D}^\dagger\bar{\mathcal{H}} - \frac{40}{9}\mathcal{D}\bar{\mathcal{I}})T_{bcjk}\Lambda^{\dot{\alpha}i}\Lambda^{\dot{\beta}k}\bar{P}_a\gamma_{bc\dot{\alpha}\dot{\beta}} \\
& + (-\frac{20}{9}\bar{\mathcal{H}} + \frac{20}{9}\mathcal{H})E^{ik}P_a\Lambda_{\alpha j}\Lambda_{\beta k}\epsilon^{\alpha\beta} + (-2\mathcal{D}^\dagger\bar{\mathcal{H}} - \frac{3}{2}\mathcal{D}\bar{\mathcal{I}})E^{ik}\Lambda^{\dot{\alpha}l}\chi_{\alpha}{}^{mn}{}_k\gamma_a{}^\alpha{}_{\dot{\alpha}}\epsilon_{jlmn} + (-\frac{16}{9}\bar{\mathcal{I}} - \frac{2}{9}\mathcal{D}^\dagger\mathcal{D}^\dagger\bar{\mathcal{H}})E_{jk}P_b\Lambda^{\dot{\alpha}i}\Lambda^{\dot{\beta}k}\gamma_{ab\dot{\alpha}\dot{\beta}} \\
& + (-\frac{16}{9}\bar{\mathcal{H}} + \frac{16}{9}\mathcal{H})P_a\Lambda_{\alpha j}\Lambda^{\dot{\alpha}i}\bar{P}_b\gamma_b{}^\alpha{}_{\dot{\alpha}} + (-\frac{16}{9}\bar{\mathcal{H}} + \frac{16}{9}\mathcal{H})P_b\Lambda_{\alpha j}\Lambda^{\dot{\alpha}i}\bar{P}_a\gamma_b{}^\alpha{}_{\dot{\alpha}} + (-\frac{16}{9}\bar{\mathcal{H}} + \frac{16}{9}\mathcal{H})P_b\Lambda_{\alpha j}\Lambda^{\dot{\alpha}i}\bar{P}_b\gamma_a{}^\alpha{}_{\dot{\alpha}} \\
& + (-\frac{16}{9}\mathcal{D}^\dagger\mathcal{I} - \frac{16}{3}\mathcal{D}\mathcal{H})P_bT_{bc}{}^{ik}\Lambda_{\alpha j}\Lambda_{\beta k}\gamma_{ac}{}^{\alpha\beta} + (-\frac{3}{2}\mathcal{D}^\dagger\mathcal{I} - 2\mathcal{D}\mathcal{H})E_{jk}\Lambda_{\alpha l}\chi^{\dot{\alpha}}{}_{mn}{}_k\gamma_a{}^\alpha{}_{\dot{\alpha}}\epsilon^{ilmn} + 2\cdots
\end{aligned}$$

$$\begin{aligned}
[\mathcal{E}_{aj}]_{2,cont} = & +(-\frac{4}{3}\bar{\mathcal{I}} + \frac{1}{3}\mathcal{D}^\dagger\mathcal{D}^\dagger\bar{\mathcal{H}})\Lambda^{\dot{\alpha}k}\Lambda^{\dot{\beta}l}\gamma_{ab\dot{\alpha}\dot{\beta}}\nabla_b E^{im}\varepsilon_{jklm} + (-\frac{4}{3}\bar{\mathcal{H}} + \frac{4}{3}\mathcal{H})T_{abjk}T_{bc}{}^{il}\Lambda_{\alpha l}\Lambda^{\dot{\alpha}k}\gamma_c{}^\alpha{}_{\dot{\alpha}} \\
& + (-\frac{4}{3}\mathcal{D}^\dagger\bar{\mathcal{H}} - \frac{16}{3}\mathcal{D}\bar{\mathcal{I}})\Lambda^{\dot{\alpha}i}\Lambda^{\dot{\beta}k}\epsilon_{\dot{\alpha}\dot{\beta}}{}^k{}_{\dot{\alpha}}\nabla_b T_{ab}{}^{lm}\varepsilon_{jklm} + (-\frac{5}{4}\bar{\mathcal{H}} + \frac{5}{4}\mathcal{H})T_{ab}{}^{kl}\Lambda^{\dot{\alpha}i}\chi_{\alpha}{}^{mn}{}_k\gamma_b{}^\alpha{}_{\dot{\alpha}}\varepsilon_{jlmn} \\
& + (-\frac{7}{6}\bar{\mathcal{H}} + \frac{7}{6}\mathcal{H})T_{ab}{}^{kl}\Lambda^{\dot{\alpha}m}\chi_{\alpha}{}^{in}{}_k\gamma_b{}^\alpha{}_{\dot{\alpha}}\varepsilon_{jlmn} + (-\bar{\mathcal{H}} + \mathcal{H})E_{jk}E^{ik}\Lambda_{\alpha l}\Lambda^{\dot{\alpha}l}\gamma_a{}^\alpha{}_{\dot{\alpha}} + (-\frac{8}{9}\mathcal{D}\mathcal{D}\mathcal{H} - \frac{64}{9}\mathcal{I})\Lambda_{\alpha j}\Lambda^{\dot{\alpha}i}\bar{P}_a\bar{P}_b\gamma_b{}^\alpha{}_{\dot{\alpha}} \\
& + (-\frac{5}{6}\bar{\mathcal{H}} + \frac{5}{6}\mathcal{H})T_{abjk}\Lambda_{\alpha l}\chi^{\dot{\alpha}}{}_{mn}{}_i\gamma_b{}^\alpha{}_{\dot{\alpha}}\varepsilon^{klmn} + (-\frac{5}{6}\bar{\mathcal{H}} + \frac{41}{6}\mathcal{H})T_{ab}{}^{kl}\Lambda^{\dot{\alpha}m}\chi_{\alpha}{}^{in}{}_j\gamma_b{}^\alpha{}_{\dot{\alpha}}\varepsilon_{klmn} \\
& + (-\frac{2}{3}\bar{\mathcal{H}} - \frac{10}{3}\mathcal{H})T_{bc}{}^{kl}\Lambda^{\dot{\alpha}m}R(Q)_{bc\alpha}{}^i\gamma_a{}^\alpha{}_{\dot{\alpha}}\varepsilon_{jklm} + (-\frac{2}{3}\bar{\mathcal{H}} + 2\mathcal{H})T_{bc}{}^{kl}\Lambda^{\dot{\alpha}i}R(Q)_{bc\alpha}{}^m\gamma_a{}^\alpha{}_{\dot{\alpha}}\varepsilon_{jklm} \\
& + (-\frac{2}{3}\mathcal{D}^\dagger\bar{\mathcal{H}} - 6\mathcal{D}\bar{\mathcal{I}})T_{ab}{}^{kl}\Lambda^{\dot{\alpha}i}\epsilon_{\dot{\alpha}\dot{\beta}}{}^k{}_{\dot{\alpha}}\nabla_b\Lambda^{\dot{\beta}m}\varepsilon_{jklm} + (-\frac{2}{3}\mathcal{D}^\dagger\bar{\mathcal{H}} + 2\mathcal{D}\bar{\mathcal{I}})T_{bc}{}^{kl}\Lambda^{\dot{\alpha}i}\gamma_{ab\dot{\alpha}\dot{\beta}}\nabla_c\Lambda^{\dot{\beta}m}\varepsilon_{jklm} \\
& + (-\frac{2}{3}\mathcal{D}\mathcal{D}\mathcal{H} - \frac{16}{3}\mathcal{I})E^{ik}\Lambda_{\alpha j}\Lambda_{\beta k}\bar{P}_a\epsilon^{\alpha\beta} + (-\frac{4}{9}\bar{\mathcal{H}} + \frac{4}{9}\mathcal{H})E_{jk}E^{il}\Lambda_{\alpha l}\Lambda^{\dot{\alpha}k}\gamma_a{}^\alpha{}_{\dot{\alpha}} + (-\frac{4}{9}\bar{\mathcal{H}} + \frac{4}{9}\mathcal{H})E^{ik}P_b\Lambda_{\alpha j}\Lambda_{\beta k}\gamma_{ab}{}^{\alpha\beta} \\
& + (-\frac{4}{9}\mathcal{D}\mathcal{D}\mathcal{H} - \frac{32}{9}\mathcal{I})\Lambda_{\alpha j}\Lambda^{\dot{\alpha}i}\bar{P}_b\bar{P}_b\gamma_a{}^\alpha{}_{\dot{\alpha}} + (-\frac{1}{3}\bar{\mathcal{H}} - \frac{1}{3}\mathcal{H})E_{kl}E^{ik}\Lambda_{\alpha j}\Lambda^{\dot{\alpha}l}\gamma_a{}^\alpha{}_{\dot{\alpha}} + (-\frac{1}{3}\bar{\mathcal{H}} + \frac{1}{3}\mathcal{H})T_{ab}{}^{ik}\Lambda^{\dot{\alpha}l}\chi_{\alpha}{}^{mn}{}_l\gamma_b{}^\alpha{}_{\dot{\alpha}}\varepsilon_{jkmn} \\
& + (-\frac{2}{9}\mathcal{D}\mathcal{D}\mathcal{H} - \frac{16}{9}\mathcal{I})E^{ik}\Lambda_{\alpha j}\Lambda_{\beta k}\bar{P}_b\gamma_{ab}{}^{\alpha\beta} + (-\frac{1}{9}\bar{\mathcal{H}} + \frac{1}{9}\mathcal{H})E_{kl}E^{kl}\Lambda_{\alpha j}\Lambda^{\dot{\alpha}i}\gamma_a{}^\alpha{}_{\dot{\alpha}} + (\frac{3}{16}\mathcal{D}^\dagger\mathcal{I} + \frac{2}{3}\mathcal{D}\mathcal{H})E_{kl}\Lambda_{\alpha j}\chi^{\dot{\alpha}}{}_{mn}{}_k\gamma_a{}^\alpha{}_{\dot{\alpha}}\varepsilon^{ilmn} \\
& + (\frac{1}{3}\bar{\mathcal{H}} - \frac{1}{3}\mathcal{H})T_{abjk}\Lambda_{\alpha l}\chi^{\dot{\alpha}}{}_{mn}{}_l\gamma_b{}^\alpha{}_{\dot{\alpha}}\varepsilon^{ikmn} + (\frac{1}{3}\bar{\mathcal{H}} + \frac{1}{3}\mathcal{H})E_{jk}E^{kl}\Lambda_{\alpha l}\Lambda^{\dot{\alpha}i}\gamma_a{}^\alpha{}_{\dot{\alpha}} + (\frac{1}{3}\mathcal{D}\mathcal{D}\mathcal{H} - \frac{4}{3}\mathcal{I})\Lambda_{\alpha k}\Lambda_{\beta l}\gamma_{ab}{}^{\alpha\beta}\nabla_b E_{jm}\varepsilon^{iklm} \\
& + (\frac{4}{9}\bar{\mathcal{H}} - \frac{4}{9}\mathcal{H})E_{jk}\Lambda^{\dot{\alpha}i}\Lambda^{\dot{\beta}k}\bar{P}_b\gamma_{ab\dot{\alpha}\dot{\beta}} + (\frac{7}{12}\bar{\mathcal{H}} + \frac{17}{12}\mathcal{H})T_{ab}{}^{ik}\Lambda^{\dot{\alpha}l}\chi_{\alpha}{}^{mn}{}_k\gamma_b{}^\alpha{}_{\dot{\alpha}}\varepsilon_{jlmn} + (\frac{2}{3}\mathcal{D}^\dagger\bar{\mathcal{H}} + \frac{3}{16}\mathcal{D}\bar{\mathcal{I}})E^{kl}\Lambda^{\dot{\alpha}i}\chi_{\alpha}{}^{mn}{}_k\gamma_a{}^\alpha{}_{\dot{\alpha}}\varepsilon_{jlmn} \\
& + (\frac{2}{3}\mathcal{D}^\dagger\mathcal{I} + 2\mathcal{D}\mathcal{H})T_{bckl}\Lambda_{\alpha m}\gamma_{ab}{}^{\alpha\beta}\nabla_c\Lambda_{\beta j}\varepsilon^{iklm} + (\frac{2}{3}\mathcal{D}\mathcal{D}\mathcal{H} + \frac{4}{3}\mathcal{I})E_{jk}\Lambda_{\alpha l}\gamma_{ab}{}^{\alpha\beta}\nabla_b\Lambda_{\beta m}\varepsilon^{iklm} \\
& + (\frac{5}{6}\bar{\mathcal{H}} - \frac{5}{6}\mathcal{H})T_{ab}{}^{ik}\Lambda^{\dot{\alpha}l}\chi_{\alpha}{}^{mn}{}_j\gamma_b{}^\alpha{}_{\dot{\alpha}}\varepsilon_{klmn} + (\frac{7}{6}\bar{\mathcal{H}} - \frac{7}{6}\mathcal{H})T_{abkl}\Lambda_{\alpha m}\chi^{\dot{\alpha}}{}_{jn}{}_k\gamma_b{}^\alpha{}_{\dot{\alpha}}\varepsilon^{ilmn} + (\frac{5}{4}\bar{\mathcal{H}} - \frac{5}{4}\mathcal{H})T_{abkl}\Lambda_{\alpha j}\chi^{\dot{\alpha}}{}_{mn}{}_k\gamma_b{}^\alpha{}_{\dot{\alpha}}\varepsilon^{ilmn} \\
& + (\frac{4}{3}\bar{\mathcal{I}} + \frac{2}{3}\mathcal{D}^\dagger\mathcal{D}^\dagger\bar{\mathcal{H}})E^{ik}\Lambda^{\dot{\alpha}l}\gamma_{ab\dot{\alpha}\dot{\beta}}\nabla_b\Lambda^{\dot{\beta}m}\varepsilon_{jklm} + (\frac{4}{3}\bar{\mathcal{H}} - \frac{4}{3}\mathcal{H})T_{abjk}T_{bc}{}^{kl}\Lambda_{\alpha l}\Lambda^{\dot{\alpha}i}\gamma_c{}^\alpha{}_{\dot{\alpha}} + (\frac{4}{3}\bar{\mathcal{H}} - \frac{4}{3}\mathcal{H})T_{abkl}T_{bc}{}^{ik}\Lambda_{\alpha j}\Lambda^{\dot{\alpha}l}\gamma_c{}^\alpha{}_{\dot{\alpha}} \\
& + (\frac{4}{3}\bar{\mathcal{H}} - \frac{4}{3}\mathcal{H})T_{abkl}T_{bc}{}^{kl}\Lambda_{\alpha j}\Lambda^{\dot{\alpha}i}\gamma_c{}^\alpha{}_{\dot{\alpha}} + (\frac{4}{3}\mathcal{D}^\dagger\bar{\mathcal{H}} - \frac{16}{3}\mathcal{D}\bar{\mathcal{I}})E^{ik}T_{abkl}\Lambda_{\alpha j}\Lambda^{\dot{\alpha}l}\gamma_b{}^\alpha{}_{\dot{\alpha}} + (\frac{4}{3}\mathcal{D}\mathcal{D}\mathcal{D}\mathcal{H} + \frac{16}{3}\mathcal{D}\mathcal{I})T_{ab}{}^{ik}\Lambda_{\alpha j}\Lambda_{\beta k}\bar{P}_c\gamma_{bc}{}^{\alpha\beta} \\
& + (\frac{4}{3}\mathcal{D}\mathcal{D}\mathcal{D}\mathcal{H} + \frac{16}{3}\mathcal{D}\mathcal{I})T_{bc}{}^{ik}\Lambda_{\alpha j}\Lambda_{\beta k}\bar{P}_b\gamma_{ac}{}^{\alpha\beta} + (\frac{17}{12}\bar{\mathcal{H}} + \frac{7}{12}\mathcal{H})T_{abjk}\Lambda_{\alpha l}\chi^{\dot{\alpha}}{}_{mn}{}_k\gamma_b{}^\alpha{}_{\dot{\alpha}}\varepsilon^{ilmn} + (\frac{16}{9}\mathcal{D}^\dagger\mathcal{I} + \frac{16}{3}\mathcal{D}\mathcal{H})P_bT_{ac}{}^{ik}\Lambda_{\alpha j}\Lambda_{\beta k}\gamma_{bc}{}^{\alpha\beta} \\
& + (2\bar{\mathcal{H}} - 2\mathcal{H})\Lambda_{\alpha k}\Lambda^{\dot{\alpha}k}R(V)_{bc}{}^i{}_j\gamma_d{}^\alpha{}_{\dot{\alpha}}\varepsilon_{abcd} + (2\bar{\mathcal{H}} - \frac{2}{3}\mathcal{H})T_{bckl}\Lambda_{\alpha j}R(Q)_{bc}{}^{\dot{\alpha}}{}_m\gamma_a{}^\alpha{}_{\dot{\alpha}}\varepsilon^{iklm} + (2\mathcal{D}^\dagger\bar{\mathcal{H}} + \frac{2}{3}\mathcal{D}\bar{\mathcal{I}})T_{bc}{}^{kl}\Lambda^{\dot{\alpha}m}\gamma_{ab\dot{\alpha}\dot{\beta}}\nabla_c\Lambda^{\dot{\beta}i}\varepsilon_{jklm} \\
& + (2\mathcal{D}^\dagger\bar{\mathcal{H}} + \frac{10}{3}\mathcal{D}\bar{\mathcal{I}})T_{ab}{}^{kl}\Lambda^{\dot{\alpha}m}\epsilon_{\dot{\alpha}\dot{\beta}}{}^k{}_{\dot{\alpha}}\nabla_b\Lambda^{\dot{\beta}i}\varepsilon_{jklm} + (2\mathcal{D}^\dagger\mathcal{I} - \frac{2}{3}\mathcal{D}\mathcal{H})T_{bckl}\Lambda_{\alpha j}\gamma_{ab}{}^{\alpha\beta}\nabla_c\Lambda_{\beta m}\varepsilon^{iklm} \\
& + (\frac{20}{9}\bar{\mathcal{H}} - \frac{20}{9}\mathcal{H})E_{jk}\Lambda^{\dot{\alpha}i}\Lambda^{\dot{\beta}k}\bar{P}_a\epsilon_{\dot{\alpha}\dot{\beta}}{}^k{}_{\dot{\alpha}} + (\frac{8}{3}\bar{\mathcal{H}} - \frac{8}{3}\mathcal{H})T_{abjk}T_{bc}{}^{ik}\Lambda_{\alpha l}\Lambda^{\dot{\alpha}l}\gamma_c{}^\alpha{}_{\dot{\alpha}} + (\frac{8}{3}\mathcal{D}^\dagger\bar{\mathcal{H}} + 4\mathcal{D}\bar{\mathcal{I}})\Lambda^{\dot{\alpha}i}\Lambda^{\dot{\beta}k}\gamma_{ab\dot{\alpha}\dot{\beta}}\nabla_c T_{bc}{}^{lm}\varepsilon_{jklm} \\
& + (\frac{8}{3}\mathcal{D}\mathcal{D}\mathcal{D}\mathcal{H} + \frac{64}{3}\mathcal{D}\mathcal{I})T_{ab}{}^{ik}\Lambda_{\alpha j}\Lambda_{\beta k}\bar{P}_b\epsilon^{\alpha\beta} + (\frac{10}{3}\mathcal{D}^\dagger\mathcal{I} + 2\mathcal{D}\mathcal{H})T_{abkl}\Lambda_{\alpha m}\epsilon^{\alpha\beta}\nabla_b\Lambda_{\beta j}\varepsilon^{iklm} \\
& + (\frac{32}{9}\bar{\mathcal{I}} + \frac{4}{9}\mathcal{D}^\dagger\mathcal{D}^\dagger\bar{\mathcal{H}})P_bP_b\Lambda_{\alpha j}\Lambda^{\dot{\alpha}i}\gamma_a{}^\alpha{}_{\dot{\alpha}} + (\frac{32}{9}\mathcal{D}^\dagger\mathcal{I} - \frac{16}{3}\mathcal{D}\mathcal{H})P_bT_{ab}{}^{ik}\Lambda_{\alpha j}\Lambda_{\beta k}\epsilon^{\alpha\beta} + (4\bar{\mathcal{H}} - 4\mathcal{H})T_{bcjk}T_{ab}{}^{kl}\Lambda_{\alpha l}\Lambda^{\dot{\alpha}i}\gamma_c{}^\alpha{}_{\dot{\alpha}} \\
& + (4\bar{\mathcal{H}} - 4\mathcal{H})T_{bckl}T_{ab}{}^{ik}\Lambda_{\alpha j}\Lambda^{\dot{\alpha}l}\gamma_c{}^\alpha{}_{\dot{\alpha}} + (4\bar{\mathcal{H}} - 4\mathcal{H})T_{bckl}T_{ab}{}^{kl}\Lambda_{\alpha j}\Lambda^{\dot{\alpha}i}\gamma_c{}^\alpha{}_{\dot{\alpha}} + (4\mathcal{D}^\dagger\bar{\mathcal{H}} - \frac{40}{3}\mathcal{D}\bar{\mathcal{I}})E^{ik}T_{abjk}\Lambda_{\alpha l}\Lambda^{\dot{\alpha}l}\gamma_b{}^\alpha{}_{\dot{\alpha}} \\
& + (4\mathcal{D}^\dagger\mathcal{I} + \frac{8}{3}\mathcal{D}\mathcal{H})\Lambda_{\alpha j}\Lambda_{\beta k}\gamma_{ab}{}^{\alpha\beta}\nabla_c T_{bclm}\varepsilon^{iklm} + (\frac{16}{3}\mathcal{D}^\dagger\bar{\mathcal{I}} + \frac{4}{3}\mathcal{D}^\dagger\mathcal{D}^\dagger\mathcal{D}^\dagger\bar{\mathcal{H}})P_bT_{bcjk}\Lambda^{\dot{\alpha}i}\Lambda^{\dot{\beta}k}\gamma_{ac\dot{\alpha}\dot{\beta}} + 3\cdots
\end{aligned}$$

$$\begin{aligned}
[\mathcal{E}_{aj}]_{2,cont} = & + \left( \frac{16}{3} \mathcal{D}^\dagger \mathcal{I} - \frac{4}{3} \mathcal{D} \mathcal{H} \right) E_{jk} T_{ab}{}^{kl} \Lambda_{\alpha l} \Lambda^{\dot{\alpha} i} \gamma_b{}^\alpha{}_{\dot{\alpha}} + \left( \frac{41}{6} \bar{\mathcal{H}} - \frac{5}{6} \mathcal{H} \right) T_{abkl} \Lambda_{\alpha m} \chi^{\dot{\alpha}}{}_{jn}{}^i \gamma_b{}^\alpha{}_{\dot{\alpha}} \varepsilon^{klmn} + \left( \frac{64}{9} \bar{\mathcal{I}} + \frac{8}{9} \mathcal{D}^\dagger \mathcal{D}^\dagger \bar{\mathcal{H}} \right) P_a P_b \Lambda_{\alpha j} \Lambda^{\dot{\alpha} i} \gamma_b{}^\alpha{}_{\dot{\alpha}} \\
& + (8 \bar{\mathcal{H}} - 8 \mathcal{H}) T_{bcjk} T_{ab}{}^{ik} \Lambda_{\alpha l} \Lambda^{\dot{\alpha} l} \gamma_c{}^\alpha{}_{\dot{\alpha}} + \left( \frac{40}{3} \mathcal{D}^\dagger \mathcal{I} - 4 \mathcal{D} \mathcal{H} \right) E_{jk} T_{ab}{}^{ik} \Lambda_{\alpha l} \Lambda^{\dot{\alpha} l} \gamma_b{}^\alpha{}_{\dot{\alpha}} + \left( \frac{64}{3} \mathcal{D}^\dagger \bar{\mathcal{I}} + \frac{8}{3} \mathcal{D}^\dagger \mathcal{D}^\dagger \mathcal{D}^\dagger \bar{\mathcal{H}} \right) P_b T_{abjk} \Lambda^{\dot{\alpha} i} \Lambda^{\dot{\beta} k} \epsilon_{\dot{\alpha} \dot{\beta}} \\
& + \frac{2}{3} \mathcal{D}^\dagger \bar{\mathcal{H}} E^{ik} E^{lm} \Lambda_{\alpha l} \Lambda^{\dot{\alpha} n} \gamma_a{}^\alpha{}_{\dot{\alpha}} \varepsilon_{jkmn} - \frac{2}{3} \mathcal{D}^\dagger \bar{\mathcal{H}} E^{ik} \Lambda^{\dot{\alpha} l} \Lambda^{\dot{\beta} m} \bar{P}_b \gamma_{ab\dot{\alpha}\dot{\beta}} \varepsilon_{jklm} + \frac{1}{3} \mathcal{D}^\dagger \mathcal{D}^\dagger \mathcal{D}^\dagger \bar{\mathcal{H}} E^{ik} P_b \Lambda^{\dot{\alpha} l} \Lambda^{\dot{\beta} m} \gamma_{ab\dot{\alpha}\dot{\beta}} \varepsilon_{jklm} \\
& - \frac{2}{3} \mathcal{D}^\dagger \mathcal{I} T_{bc}{}^{kl} T_{bc}{}^{mn} \Lambda_{\alpha j} \Lambda^{\dot{\alpha} i} \gamma_a{}^\alpha{}_{\dot{\alpha}} \varepsilon_{klmn} + \frac{2}{3} \mathcal{D} \bar{\mathcal{I}} T_{bckl} T_{bcmn} \Lambda_{\alpha j} \Lambda^{\dot{\alpha} i} \gamma_a{}^\alpha{}_{\dot{\alpha}} \varepsilon^{klmn} + \frac{1}{3} \mathcal{D} \mathcal{D} \mathcal{D} \mathcal{H} E_{jk} \Lambda_{\alpha l} \Lambda_{\beta m} \bar{P}_b \gamma_{ab}{}^{\alpha\beta} \varepsilon^{iklm} \\
& - \frac{2}{3} \mathcal{D} \mathcal{H} E_{jk} E_{lm} \Lambda_{\alpha n} \Lambda^{\dot{\alpha} l} \gamma_a{}^\alpha{}_{\dot{\alpha}} \varepsilon^{ikmn} - \frac{2}{3} \mathcal{D} \mathcal{H} E_{jk} P_b \Lambda_{\alpha l} \Lambda_{\beta m} \gamma_{ab}{}^{\alpha\beta} \varepsilon^{iklm} + \left( -\frac{85}{6} \mathcal{D}^\dagger \mathcal{I} + 6 \mathcal{D} \mathcal{H} \right) T_{ab}{}^{kl} T_{bc}{}^{im} \Lambda_{\alpha n} \Lambda^{\dot{\alpha} n} \gamma_c{}^\alpha{}_{\dot{\alpha}} \varepsilon_{jklm} \\
& + \left( -\frac{53}{6} \mathcal{D}^\dagger \mathcal{I} + 6 \mathcal{D} \mathcal{H} \right) T_{ab}{}^{kl} T_{bc}{}^{im} \Lambda_{\alpha j} \Lambda^{\dot{\alpha} n} \gamma_c{}^\alpha{}_{\dot{\alpha}} \varepsilon_{klmn} + \left( -\frac{16}{3} \bar{\mathcal{I}} + \frac{4}{3} \mathcal{D}^\dagger \mathcal{D}^\dagger \bar{\mathcal{H}} \right) P_b T_{bc}{}^{ik} \Lambda^{\dot{\alpha} l} \Lambda^{\dot{\beta} m} \gamma_{ac\dot{\alpha}\dot{\beta}} \varepsilon_{jklm} \\
& + \left( -\frac{16}{3} \bar{\mathcal{I}} + \frac{8}{3} \mathcal{D}^\dagger \mathcal{D}^\dagger \bar{\mathcal{H}} \right) P_b T_{bc}{}^{kl} \Lambda^{\dot{\alpha} i} \Lambda^{\dot{\beta} m} \gamma_{ac\dot{\alpha}\dot{\beta}} \varepsilon_{jklm} + \left( -\frac{10}{3} \mathcal{D}^\dagger \bar{\mathcal{H}} + \frac{7}{2} \mathcal{D} \bar{\mathcal{I}} \right) T_{abkl} T_{bcmn} \Lambda_{\alpha j} \Lambda^{\dot{\alpha} k} \gamma_c{}^\alpha{}_{\dot{\alpha}} \varepsilon^{ilmn} \\
& + \left( -\frac{37}{12} \mathcal{D}^\dagger \mathcal{I} + \frac{7}{3} \mathcal{D} \mathcal{H} \right) T_{ab}{}^{kl} T_{bc}{}^{mn} \Lambda_{\alpha j} \Lambda^{\dot{\alpha} i} \gamma_c{}^\alpha{}_{\dot{\alpha}} \varepsilon_{klmn} + \left( -\frac{107}{36} \bar{\mathcal{H}} + \frac{23}{36} \mathcal{H} \right) E_{jk} T_{ablm} \Lambda_{\alpha n} \Lambda^{\dot{\alpha} n} \gamma_b{}^\alpha{}_{\dot{\alpha}} \varepsilon^{iklm} \\
& + \left( -\frac{26}{9} \bar{\mathcal{H}} + \frac{2}{3} \mathcal{H} \right) T_{bc}{}^{kl} \Lambda^{\dot{\alpha} i} \Lambda^{\dot{\beta} m} \bar{P}_b \gamma_{ac\dot{\alpha}\dot{\beta}} \varepsilon_{jklm} + \left( -\frac{35}{18} \bar{\mathcal{H}} + \frac{23}{18} \mathcal{H} \right) E_{jk} T_{ablm} \Lambda_{\alpha n} \Lambda^{\dot{\alpha} l} \gamma_b{}^\alpha{}_{\dot{\alpha}} \varepsilon^{ikmn} \\
& + \left( -\frac{59}{36} \bar{\mathcal{H}} - \frac{25}{36} \mathcal{H} \right) E_{jk} T_{ablm} \Lambda_{\alpha n} \Lambda^{\dot{\alpha} i} \gamma_b{}^\alpha{}_{\dot{\alpha}} \varepsilon^{klmn} + \left( -\frac{19}{12} \mathcal{D}^\dagger \mathcal{I} + \mathcal{D} \mathcal{H} \right) T_{ab}{}^{ik} T_{bc}{}^{lm} \Lambda_{\alpha k} \Lambda^{\dot{\alpha} n} \gamma_c{}^\alpha{}_{\dot{\alpha}} \varepsilon_{jlmn} \\
& + \left( -\frac{23}{18} \bar{\mathcal{H}} + \frac{35}{18} \mathcal{H} \right) E^{ik} T_{ab}{}^{lm} \Lambda_{\alpha l} \Lambda^{\dot{\alpha} n} \gamma_b{}^\alpha{}_{\dot{\alpha}} \varepsilon_{jkmn} + \left( -\mathcal{D}^\dagger \bar{\mathcal{H}} + \frac{23}{12} \mathcal{D} \bar{\mathcal{I}} \right) T_{abjk} T_{bclm} \Lambda_{\alpha n} \Lambda^{\dot{\alpha} k} \gamma_c{}^\alpha{}_{\dot{\alpha}} \varepsilon^{ilmn} \\
& + \left( -\frac{8}{9} \bar{\mathcal{H}} - \frac{8}{9} \mathcal{H} \right) P_b T_{abkl} \Lambda_{\alpha j} \Lambda_{\beta m} \epsilon^{\alpha\beta} \varepsilon^{iklm} + \left( -\frac{8}{9} \bar{\mathcal{H}} - \frac{8}{9} \mathcal{H} \right) T_{ab}{}^{kl} \Lambda^{\dot{\alpha} i} \Lambda^{\dot{\beta} m} \bar{P}_b \epsilon_{\dot{\alpha}\dot{\beta}} \varepsilon_{jklm} + \left( -\frac{23}{36} \bar{\mathcal{H}} + \frac{107}{36} \mathcal{H} \right) E^{ik} T_{ab}{}^{lm} \Lambda_{\alpha n} \Lambda^{\dot{\alpha} n} \gamma_b{}^\alpha{}_{\dot{\alpha}} \varepsilon_{jklm} \\
& + \left( -\frac{11}{18} \bar{\mathcal{H}} - \frac{1}{2} \mathcal{H} \right) E^{kl} T_{ab}{}^{mn} \Lambda_{\alpha k} \Lambda^{\dot{\alpha} i} \gamma_b{}^\alpha{}_{\dot{\alpha}} \varepsilon_{jlmn} + \left( -\frac{3}{8} \mathcal{D}^\dagger \mathcal{I} - \frac{1}{2} \mathcal{D} \mathcal{H} \right) T_{bc}{}^{ik} T_{bc}{}^{lm} \Lambda_{\alpha k} \Lambda^{\dot{\alpha} n} \gamma_a{}^\alpha{}_{\dot{\alpha}} \varepsilon_{jlmn} \\
& + \left( -\frac{1}{3} \bar{\mathcal{H}} + \frac{1}{3} \mathcal{H} \right) E_{kl} T_{abjm} \Lambda_{\alpha n} \Lambda^{\dot{\alpha} k} \gamma_b{}^\alpha{}_{\dot{\alpha}} \varepsilon^{ilmn} + \left( -\frac{1}{3} \bar{\mathcal{H}} + \frac{1}{3} \mathcal{H} \right) E^{kl} T_{ab}{}^{im} \Lambda_{\alpha k} \Lambda^{\dot{\alpha} n} \gamma_b{}^\alpha{}_{\dot{\alpha}} \varepsilon_{jlmn} + \left( -\frac{2}{9} \bar{\mathcal{H}} + \frac{14}{9} \mathcal{H} \right) T_{bc}{}^{ik} \Lambda^{\dot{\alpha} l} \Lambda^{\dot{\beta} m} \bar{P}_b \gamma_{ac\dot{\alpha}\dot{\beta}} \varepsilon_{jklm} \\
& + \left( \frac{4}{9} \bar{\mathcal{H}} - \frac{4}{9} \mathcal{H} \right) P_b \Lambda_{\alpha j} \Lambda^{\dot{\alpha} i} \bar{P}_c \gamma_d{}^\alpha{}_{\dot{\alpha}} \varepsilon_{abcd} + \left( \frac{1}{2} \bar{\mathcal{H}} + \frac{11}{18} \mathcal{H} \right) E_{kl} T_{abmn} \Lambda_{\alpha j} \Lambda^{\dot{\alpha} k} \gamma_b{}^\alpha{}_{\dot{\alpha}} \varepsilon^{ilmn} + \left( \frac{1}{2} \mathcal{D}^\dagger \bar{\mathcal{H}} + \frac{13}{24} \mathcal{D} \bar{\mathcal{I}} \right) T_{bcjk} T_{bclm} \Lambda_{\alpha n} \Lambda^{\dot{\alpha} k} \gamma_a{}^\alpha{}_{\dot{\alpha}} \varepsilon^{ilmn} \\
& + \left( \frac{2}{3} \bar{\mathcal{H}} - \frac{26}{9} \mathcal{H} \right) P_b T_{bckl} \Lambda_{\alpha j} \Lambda_{\beta m} \gamma_{ac}{}^{\alpha\beta} \varepsilon^{iklm} + \left( \frac{25}{36} \bar{\mathcal{H}} - \frac{61}{36} \mathcal{H} \right) E_{jk} T_{ablm} \Lambda_{\alpha n} \Lambda^{\dot{\alpha} k} \gamma_b{}^\alpha{}_{\dot{\alpha}} \varepsilon^{ilmn} \\
& + \left( \frac{25}{36} \bar{\mathcal{H}} + \frac{59}{36} \mathcal{H} \right) E^{ik} T_{ab}{}^{lm} \Lambda_{\alpha j} \Lambda^{\dot{\alpha} n} \gamma_b{}^\alpha{}_{\dot{\alpha}} \varepsilon_{klmn} + \left( \frac{4}{3} \mathcal{D} \mathcal{D} \mathcal{H} - \frac{16}{3} \mathcal{I} \right) T_{bcjk} \Lambda_{\alpha l} \Lambda_{\beta m} \bar{P}_b \gamma_{ac}{}^{\alpha\beta} \varepsilon^{iklm} \\
& + \left( \frac{4}{3} \mathcal{D} \mathcal{D} \mathcal{H} + \frac{16}{3} \mathcal{I} \right) T_{abkl} \Lambda_{\alpha j} \Lambda_{\beta m} \bar{P}_b \epsilon^{\alpha\beta} \varepsilon^{iklm} + \left( \frac{14}{9} \bar{\mathcal{H}} - \frac{2}{9} \mathcal{H} \right) P_b T_{bcjk} \Lambda_{\alpha l} \Lambda_{\beta m} \gamma_{ac}{}^{\alpha\beta} \varepsilon^{iklm} + \left( \frac{61}{36} \bar{\mathcal{H}} - \frac{25}{36} \mathcal{H} \right) E^{ik} T_{ab}{}^{lm} \Lambda_{\alpha k} \Lambda^{\dot{\alpha} n} \gamma_b{}^\alpha{}_{\dot{\alpha}} \varepsilon_{jlmn} \\
& + \left( \frac{7}{3} \mathcal{D}^\dagger \bar{\mathcal{H}} - \frac{37}{12} \mathcal{D} \bar{\mathcal{I}} \right) T_{abkl} T_{bcmn} \Lambda_{\alpha j} \Lambda^{\dot{\alpha} i} \gamma_c{}^\alpha{}_{\dot{\alpha}} \varepsilon^{klmn} + \left( \frac{8}{3} \mathcal{D} \mathcal{D} \mathcal{H} - \frac{16}{3} \mathcal{I} \right) T_{bckl} \Lambda_{\alpha j} \Lambda_{\beta m} \bar{P}_b \gamma_{ac}{}^{\alpha\beta} \varepsilon^{iklm} \\
& + \left( 3 \mathcal{D}^\dagger \bar{\mathcal{H}} - \frac{61}{12} \mathcal{D} \bar{\mathcal{I}} \right) T_{abkl} T_{bcjm} \Lambda_{\alpha n} \Lambda^{\dot{\alpha} m} \gamma_c{}^\alpha{}_{\dot{\alpha}} \varepsilon^{ikln} + \left( \frac{7}{2} \mathcal{D}^\dagger \mathcal{I} - \frac{10}{3} \mathcal{D} \mathcal{H} \right) T_{ab}{}^{kl} T_{bc}{}^{mn} \Lambda_{\alpha m} \Lambda^{\dot{\alpha} i} \gamma_c{}^\alpha{}_{\dot{\alpha}} \varepsilon_{jklm} \\
& + \left( \frac{16}{3} \bar{\mathcal{I}} + \frac{4}{3} \mathcal{D}^\dagger \mathcal{D}^\dagger \bar{\mathcal{H}} \right) P_b T_{ab}{}^{kl} \Lambda^{\dot{\alpha} i} \Lambda^{\dot{\beta} m} \epsilon_{\dot{\alpha}\dot{\beta}} \varepsilon_{jklm} + \left( \frac{65}{12} \mathcal{D}^\dagger \mathcal{I} - 3 \mathcal{D} \mathcal{H} \right) T_{ab}{}^{kl} T_{bc}{}^{im} \Lambda_{\alpha m} \Lambda^{\dot{\alpha} n} \gamma_c{}^\alpha{}_{\dot{\alpha}} \varepsilon_{jklm} \\
& + \left( 6 \mathcal{D}^\dagger \bar{\mathcal{H}} - \frac{85}{6} \mathcal{D} \bar{\mathcal{I}} \right) T_{abjk} T_{bclm} \Lambda_{\alpha n} \Lambda^{\dot{\alpha} n} \gamma_c{}^\alpha{}_{\dot{\alpha}} \varepsilon^{iklm} + \left( 6 \mathcal{D}^\dagger \bar{\mathcal{H}} - \frac{53}{6} \mathcal{D} \bar{\mathcal{I}} \right) T_{abjk} T_{bclm} \Lambda_{\alpha n} \Lambda^{\dot{\alpha} i} \gamma_c{}^\alpha{}_{\dot{\alpha}} \varepsilon^{klmn}
\end{aligned}$$

$$\begin{aligned}
[\mathcal{E}_{aj}^i]_4 = & -\frac{2}{3}\Lambda_{\alpha j}\Lambda_{\beta k}\Lambda^{\dot{\alpha}k}\bar{\mathcal{H}}\gamma_a^\alpha{}_\beta\gamma_b^\beta{}_\alpha\nabla_b\Lambda^{\dot{\beta}i}-2\Lambda_{\alpha j}\Lambda_{\beta k}\Lambda^{\dot{\alpha}k}\bar{\mathcal{H}}\gamma_a^\beta{}_\beta\gamma_b^\alpha{}_\alpha\nabla_b\Lambda^{\dot{\beta}i}-\frac{2}{3}\mathcal{H}\Lambda_{\alpha k}\Lambda^{\dot{\alpha}i}\Lambda^{\dot{\beta}k}\gamma_a^\beta{}_\beta\gamma_b^\alpha{}_\alpha\nabla_b\Lambda_{\beta j}\\
& -2\mathcal{H}\Lambda_{\alpha k}\Lambda^{\dot{\alpha}i}\Lambda^{\dot{\beta}k}\gamma_a^\beta{}_\beta\gamma_b^\alpha{}_\alpha\nabla_b\Lambda_{\beta j}+(-\frac{32}{3}\mathcal{D}^\dagger\mathcal{I}+4\mathcal{DH})\Lambda_{\alpha j}\Lambda_{\beta k}\Lambda^{\dot{\alpha}k}R(Q)_{ab\gamma}{}^i\epsilon^{\alpha\gamma}\gamma_b^\beta{}_\alpha+(-\frac{73}{12}\mathcal{D}^\dagger\mathcal{I}+\frac{3}{2}\mathcal{DH})\Lambda_{\alpha k}\Lambda_{\beta l}\Lambda^{\dot{\alpha}k}\chi_{\gamma}{}^{il}{}_j\epsilon^{\alpha\beta}\gamma_a^\gamma{}_\alpha\\
& +(-\frac{8}{3}\mathcal{D}^\dagger\mathcal{I}-\frac{4}{3}\mathcal{DH})\Lambda_{\alpha k}\Lambda_{\beta l}\Lambda^{\dot{\alpha}i}\chi_{\gamma}{}^{kl}{}_j\epsilon^{\alpha\gamma}\gamma_a^\beta{}_\alpha+(-\frac{4}{3}\mathcal{D}^\dagger\bar{\mathcal{H}}-\frac{8}{3}\mathcal{D}\bar{\mathcal{L}})\Lambda_{\alpha j}\Lambda^{\dot{\alpha}k}\Lambda^{\dot{\beta}l}\chi^{\dot{\gamma}}{}_{kl}{}^i\epsilon^{\dot{\alpha}\dot{\gamma}}\gamma_a^\alpha{}_\beta\\
& +(-\frac{4}{3}\mathcal{D}^\dagger\bar{\mathcal{H}}+4\mathcal{D}\bar{\mathcal{L}})\Lambda_{\alpha j}\Lambda^{\dot{\alpha}i}\Lambda^{\dot{\beta}k}R(Q)_{ab}{}^{\dot{\gamma}}{}_k\epsilon^{\dot{\alpha}\dot{\gamma}}\gamma_b^\alpha{}_\beta+(-\frac{7}{6}\mathcal{D}^\dagger\mathcal{I}+\frac{1}{3}\mathcal{DH})\Lambda_{\alpha j}\Lambda_{\beta k}\Lambda^{\dot{\alpha}l}\chi_{\gamma}{}^{ik}{}_l\epsilon^{\beta\gamma}\gamma_a^\alpha{}_\alpha\\
& +(-\frac{37}{36}\bar{\mathcal{H}}+\frac{23}{18}\mathcal{H})\Lambda_{\alpha j}\Lambda_{\beta k}\Lambda^{\dot{\alpha}k}\epsilon^{\alpha\beta}\epsilon_{\dot{\alpha}\dot{\beta}}\nabla_a\Lambda^{\dot{\beta}i}+(-\mathcal{D}^\dagger\bar{\mathcal{H}}+\frac{3}{2}\mathcal{D}\bar{\mathcal{L}})\Lambda_{\alpha k}\Lambda^{\dot{\alpha}i}\Lambda^{\dot{\beta}l}\chi^{\dot{\gamma}}{}_{jl}{}^k\epsilon^{\dot{\alpha}\dot{\beta}}\gamma_a^\alpha{}_\gamma+(-\frac{11}{36}\bar{\mathcal{H}}+\frac{1}{18}\mathcal{H})\Lambda_{\alpha j}\Lambda_{\beta k}\Lambda^{\dot{\alpha}k}\gamma_a^\beta{}_\alpha\gamma_b^\alpha{}_\beta\nabla_b\Lambda^{\dot{\beta}i}\\
& +(-\frac{5}{18}\bar{\mathcal{H}}+\frac{7}{36}\mathcal{H})\Lambda_{\alpha j}\Lambda^{\dot{\alpha}i}\Lambda^{\dot{\beta}k}\gamma_a^\alpha{}_\beta\gamma_b^\beta{}_\alpha\nabla_b\Lambda_{\beta k}+(-\frac{1}{12}\bar{\mathcal{H}}+\frac{1}{6}\mathcal{H})\Lambda_{\alpha j}\Lambda_{\beta k}\Lambda^{\dot{\alpha}i}\gamma_a^\alpha{}_\alpha\gamma_b^\beta{}_\beta\nabla_b\Lambda^{\dot{\beta}k}\\
& +(-\frac{1}{18}\bar{\mathcal{H}}+\frac{5}{36}\mathcal{H})\Lambda_{\alpha j}\Lambda^{\dot{\alpha}i}\Lambda^{\dot{\beta}k}\epsilon^{\alpha\beta}\epsilon_{\dot{\alpha}\dot{\beta}}\nabla_a\Lambda_{\beta k}+(-\frac{1}{18}\bar{\mathcal{H}}+\frac{5}{36}\mathcal{H})\Lambda_{\alpha j}\Lambda^{\dot{\alpha}i}\Lambda^{\dot{\beta}k}\epsilon_{\dot{\alpha}\dot{\beta}}\gamma_{ab}{}^{\alpha\beta}\nabla_b\Lambda_{\beta k}+(-\frac{1}{18}\bar{\mathcal{H}}+\frac{11}{36}\mathcal{H})\Lambda_{\alpha k}\Lambda^{\dot{\alpha}i}\Lambda^{\dot{\beta}k}\epsilon_{\dot{\alpha}\dot{\beta}}\gamma_{ab}{}^{\alpha\beta}\nabla_b\Lambda_{\beta j}\\
& +(-\frac{1}{18}\bar{\mathcal{H}}+\frac{11}{36}\mathcal{H})\Lambda_{\alpha k}\Lambda^{\dot{\alpha}i}\Lambda^{\dot{\beta}k}\gamma_a^\alpha{}_\alpha\gamma_b^\beta{}_\beta\nabla_b\Lambda_{\beta j}+(\frac{1}{18}\bar{\mathcal{H}}-\frac{11}{36}\mathcal{H})\Lambda_{\alpha k}\Lambda^{\dot{\alpha}i}\Lambda^{\dot{\beta}k}\gamma_a^\alpha{}_\beta\gamma_b^\beta{}_\alpha\nabla_b\Lambda_{\beta j}\\
& +(\frac{5}{36}\bar{\mathcal{H}}-\frac{1}{18}\mathcal{H})\Lambda_{\alpha j}\Lambda_{\beta k}\Lambda^{\dot{\alpha}i}\epsilon^{\alpha\beta}\epsilon_{\dot{\alpha}\dot{\beta}}\nabla_a\Lambda^{\dot{\beta}k}+(\frac{5}{36}\bar{\mathcal{H}}-\frac{1}{18}\mathcal{H})\Lambda_{\alpha j}\Lambda_{\beta k}\Lambda^{\dot{\alpha}i}\epsilon^{\alpha\beta}\gamma_{ab\dot{\alpha}\dot{\beta}}\nabla_b\Lambda^{\dot{\beta}k}+(\frac{1}{6}\bar{\mathcal{H}}-\frac{1}{12}\mathcal{H})\Lambda_{\alpha j}\Lambda^{\dot{\alpha}i}\Lambda^{\dot{\beta}k}\gamma_a^\alpha{}_\alpha\gamma_b^\beta{}_\beta\nabla_b\Lambda_{\beta k}\\
& +(\frac{7}{36}\bar{\mathcal{H}}-\frac{5}{18}\mathcal{H})\Lambda_{\alpha j}\Lambda_{\beta k}\Lambda^{\dot{\alpha}i}\gamma_a^\beta{}_\alpha\gamma_b^\alpha{}_\beta\nabla_b\Lambda^{\dot{\beta}k}+(\frac{11}{36}\bar{\mathcal{H}}-\frac{1}{18}\mathcal{H})\Lambda_{\alpha j}\Lambda_{\beta k}\Lambda^{\dot{\alpha}k}\epsilon^{\alpha\beta}\gamma_{ab\dot{\alpha}\dot{\beta}}\nabla_b\Lambda^{\dot{\beta}i}+(\frac{11}{36}\bar{\mathcal{H}}-\frac{1}{18}\mathcal{H})\Lambda_{\alpha j}\Lambda_{\beta k}\Lambda^{\dot{\alpha}k}\gamma_a^\alpha{}_\alpha\gamma_b^\beta{}_\beta\nabla_b\Lambda^{\dot{\beta}i}\\
& +(\frac{1}{3}\bar{\mathcal{H}}+\frac{1}{3}\mathcal{H})\Lambda_{\alpha j}\Lambda_{\beta k}\Lambda^{\dot{\alpha}i}\gamma_a^\alpha{}_\beta\gamma_b^\beta{}_\alpha\nabla_b\Lambda^{\dot{\beta}k}+(\frac{1}{3}\bar{\mathcal{H}}+\frac{1}{3}\mathcal{H})\Lambda_{\alpha j}\Lambda^{\dot{\alpha}i}\Lambda^{\dot{\beta}k}\gamma_a^\beta{}_\alpha\gamma_b^\alpha{}_\beta\nabla_b\Lambda_{\beta k}+(\frac{1}{3}\mathcal{D}^\dagger\bar{\mathcal{H}}-\frac{7}{6}\mathcal{D}\bar{\mathcal{L}})\Lambda_{\alpha k}\Lambda^{\dot{\alpha}i}\Lambda^{\dot{\beta}l}\chi^{\dot{\gamma}}{}_{jl}{}^k\epsilon^{\dot{\beta}\dot{\gamma}}\gamma_a^\alpha{}_\alpha\\
& +(\frac{2}{3}\bar{\mathcal{H}}+\frac{4}{3}\mathcal{H})\Lambda_{\alpha j}\Lambda^{\dot{\alpha}i}\Lambda^{\dot{\beta}k}\gamma_a^\beta{}_\beta\gamma_b^\alpha{}_\alpha\nabla_b\Lambda_{\beta k}+(\mathcal{D}^\dagger\bar{\mathcal{H}}+\frac{7}{6}\mathcal{D}\bar{\mathcal{L}})\Lambda_{\alpha k}\Lambda^{\dot{\alpha}i}\Lambda^{\dot{\beta}l}\chi^{\dot{\gamma}}{}_{jl}{}^k\epsilon^{\dot{\alpha}\dot{\gamma}}\gamma_a^\alpha{}_\beta+(\frac{7}{6}\mathcal{D}^\dagger\mathcal{I}+\mathcal{DH})\Lambda_{\alpha j}\Lambda_{\beta k}\Lambda^{\dot{\alpha}l}\chi_{\gamma}{}^{ik}{}_l\epsilon^{\alpha\gamma}\gamma_a^\beta{}_\alpha\\
& +(\frac{23}{18}\bar{\mathcal{H}}-\frac{37}{36}\mathcal{H})\Lambda_{\alpha k}\Lambda^{\dot{\alpha}i}\Lambda^{\dot{\beta}k}\epsilon^{\alpha\beta}\epsilon_{\dot{\alpha}\dot{\beta}}\nabla_a\Lambda_{\beta j}+(\frac{4}{3}\bar{\mathcal{H}}+\frac{2}{3}\mathcal{H})\Lambda_{\alpha j}\Lambda_{\beta k}\Lambda^{\dot{\alpha}i}\gamma_a^\beta{}_\beta\gamma_b^\alpha{}_\alpha\nabla_b\Lambda^{\dot{\beta}k}+(\frac{3}{2}\mathcal{D}^\dagger\bar{\mathcal{H}}-\frac{73}{12}\mathcal{D}\bar{\mathcal{L}})\Lambda_{\alpha k}\Lambda^{\dot{\alpha}k}\Lambda^{\dot{\beta}l}\chi^{\dot{\gamma}}{}_{jl}{}^i\epsilon^{\dot{\alpha}\dot{\beta}}\gamma_a^\alpha{}_\gamma\\
& +(\frac{3}{2}\mathcal{D}^\dagger\bar{\mathcal{H}}+\frac{23}{12}\mathcal{D}\bar{\mathcal{L}})\Lambda_{\alpha k}\Lambda^{\dot{\alpha}k}\Lambda^{\dot{\beta}l}\chi^{\dot{\gamma}}{}_{jl}{}^i\epsilon^{\dot{\beta}\dot{\gamma}}\gamma_a^\alpha{}_\alpha+(\frac{3}{2}\mathcal{D}^\dagger\mathcal{I}-\mathcal{DH})\Lambda_{\alpha j}\Lambda_{\beta k}\Lambda^{\dot{\alpha}l}\chi_{\gamma}{}^{ik}{}_l\epsilon^{\alpha\beta}\gamma_a^\gamma{}_\alpha+(\frac{23}{12}\mathcal{D}^\dagger\mathcal{I}+\frac{3}{2}\mathcal{DH})\Lambda_{\alpha k}\Lambda_{\beta l}\Lambda^{\dot{\alpha}k}\chi_{\gamma}{}^{il}{}_j\epsilon^{\beta\gamma}\gamma_a^\alpha{}_\alpha\\
& +(\frac{5}{2}\mathcal{D}^\dagger\bar{\mathcal{H}}+\frac{41}{12}\mathcal{D}\bar{\mathcal{L}})\Lambda_{\alpha k}\Lambda^{\dot{\alpha}k}\Lambda^{\dot{\beta}l}\chi^{\dot{\gamma}}{}_{jl}{}^i\epsilon^{\dot{\alpha}\dot{\gamma}}\gamma_a^\alpha{}_\beta+(\frac{41}{12}\mathcal{D}^\dagger\mathcal{I}+\frac{5}{2}\mathcal{DH})\Lambda_{\alpha k}\Lambda_{\beta l}\Lambda^{\dot{\alpha}k}\chi_{\gamma}{}^{il}{}_j\epsilon^{\alpha\gamma}\gamma_a^\beta{}_\alpha\\
& +(4\mathcal{D}^\dagger\bar{\mathcal{H}}-\frac{32}{3}\mathcal{D}\bar{\mathcal{L}})\Lambda_{\alpha k}\Lambda^{\dot{\alpha}i}\Lambda^{\dot{\beta}k}R(Q)_{ab}{}^{\dot{\gamma}}{}_j\epsilon^{\dot{\alpha}\dot{\gamma}}\gamma_b^\alpha{}_\beta+(4\mathcal{D}^\dagger\mathcal{I}-\frac{4}{3}\mathcal{DH})\Lambda_{\alpha j}\Lambda_{\beta k}\Lambda^{\dot{\alpha}i}R(Q)_{ab\gamma}{}^k\epsilon^{\alpha\gamma}\gamma_b^\beta{}_\alpha\\
& +\frac{4}{3}\mathcal{D}^\dagger\bar{\mathcal{L}}\Lambda^{\dot{\alpha}i}\Lambda^{\dot{\beta}k}\Lambda^{\dot{\gamma}l}\epsilon_{\dot{\alpha}\dot{\beta}}\epsilon_{\dot{\gamma}\dot{\delta}}\nabla_a\Lambda^{\dot{\delta}m}\varepsilon_{jklm}+\frac{4}{3}\mathcal{DL}\Lambda_{\alpha j}\Lambda_{\beta k}\Lambda_{\gamma l}\epsilon^{\alpha\beta}\epsilon^{\gamma\delta}\nabla_a\Lambda_{\delta m}\varepsilon^{iklm}+(-\frac{28}{3}\bar{\mathcal{L}}-\frac{8}{3}\mathcal{D}^\dagger\mathcal{D}^\dagger\bar{\mathcal{H}})T_{bcjk}\Lambda_{\alpha l}\Lambda^{\dot{\alpha}i}\Lambda^{\dot{\beta}k}\Lambda^{\dot{\gamma}l}\gamma_a^\alpha{}_\beta\gamma_{bc\dot{\alpha}\dot{\gamma}}\\
& +(-\frac{8}{3}\mathcal{DDH}-\frac{28}{3}\mathcal{I})T_{bc}{}^{ik}\Lambda_{\alpha j}\Lambda_{\beta k}\Lambda^{\dot{\alpha}l}\Lambda_{\gamma l}\gamma_a^\beta{}_\alpha\gamma_{bc}{}^{\alpha\gamma}+(-\frac{13}{6}\bar{\mathcal{L}}+\frac{23}{48}\mathcal{D}^\dagger\mathcal{D}^\dagger\bar{\mathcal{H}})\Lambda^{\dot{\alpha}k}\Lambda^{\dot{\beta}l}\Lambda^{\dot{\gamma}m}\chi_{\alpha}{}^{in}{}_k\epsilon_{\dot{\alpha}\dot{\beta}}\gamma_a^\alpha{}_\gamma\varepsilon_{jlmn}\\
& +(-\frac{13}{8}\mathcal{D}$$





$\mathcal{E}_{ab}^{ij}$

We give the block  $\mathcal{E}_{ab}^{ij}$  with anti-symmetrizations assumed and with factors of  $\gamma_{ab}$  to emphasize which terms are self-dual and which are anti-self-dual. The zero fermion terms are

$$\begin{aligned}
[\mathcal{E}_{ab}^{ij}]_0 = & \left( \frac{2}{3} \mathcal{H} - \frac{2}{3} \bar{\mathcal{H}} \right) i \gamma_{ab\dot{\alpha}\dot{\beta}} \gamma_{cd}^{\dot{\alpha}\dot{\beta}} \nabla_c \nabla_e T_{de}^{ij} + \left( \frac{2}{3} \mathcal{H} - \frac{2}{3} \bar{\mathcal{H}} \right) i \gamma_{ab\dot{\alpha}\dot{\beta}} \gamma_{cd}^{\dot{\alpha}\dot{\beta}} \nabla_e \nabla_c T_{de}^{ij} - \frac{1}{3} i E^{ik} \mathcal{D} \bar{\mathcal{L}} R(V)_{cd}{}^j{}_k \gamma_{ab\dot{\alpha}\dot{\beta}} \gamma_{cd}^{\dot{\alpha}\dot{\beta}} \\
& + \frac{1}{3} i E^{jk} \mathcal{D} \bar{\mathcal{L}} R(V)_{cd}{}^i{}_k \gamma_{ab\dot{\alpha}\dot{\beta}} \gamma_{cd}^{\dot{\alpha}\dot{\beta}} + i \mathcal{H} T_{cd}{}^{ij} R(M)_{cdef} \gamma_{ef\alpha\beta} \gamma_{ab}^{\alpha\beta} - 2 i \mathcal{H} T_{cd}{}^{ik} R(V)_{ce}{}^j{}_k \gamma_{de\alpha\beta} \gamma_{ab}^{\alpha\beta} + 2 i \mathcal{H} T_{cd}{}^{jk} R(V)_{ce}{}^i{}_k \gamma_{de\alpha\beta} \gamma_{ab}^{\alpha\beta} \\
& + \frac{4}{3} i T_{cd}{}^{ij} \mathcal{D}^\dagger \mathcal{I} \gamma_{ab\dot{\alpha}\dot{\beta}} \gamma_{ce}^{\dot{\alpha}\dot{\beta}} \nabla_d \bar{P}_e + \frac{4}{3} i T_{cd}{}^{ij} \mathcal{D}^\dagger \mathcal{I} \gamma_{ab\dot{\alpha}\dot{\beta}} \gamma_{ce}^{\dot{\alpha}\dot{\beta}} \nabla_e \bar{P}_d - \frac{8}{3} i \mathcal{D}^\dagger \mathcal{I} \bar{P}_c \gamma_{ab\dot{\alpha}\dot{\beta}} \gamma_{cd}^{\dot{\alpha}\dot{\beta}} \nabla_e T_{de}^{ij} + \frac{8}{3} i \mathcal{D}^\dagger \mathcal{I} \bar{P}_c \gamma_{ab\dot{\alpha}\dot{\beta}} \gamma_{de}^{\dot{\alpha}\dot{\beta}} \nabla_d T_{ce}^{ij} \\
& - \frac{1}{2} i \bar{\mathcal{H}} D^{ij}{}_{kl} T_{cd}{}^{kl} \gamma_{cd\alpha\beta} \gamma_{ab}^{\alpha\beta} + (-2 \mathcal{D}^\dagger \bar{\mathcal{H}} - 4 \mathcal{D} \bar{\mathcal{L}}) i P_c \gamma_{cd\alpha\beta} \gamma_{ab}^{\alpha\beta} \nabla_e T_{de}^{ij} + (-2 \mathcal{D}^\dagger \bar{\mathcal{H}} - 4 \mathcal{D} \bar{\mathcal{L}}) i P_c \gamma_{de\alpha\beta} \gamma_{ab}^{\alpha\beta} \nabla_d T_{ce}^{ij} \\
& + (-\mathcal{D}^\dagger \bar{\mathcal{H}} - 2 \mathcal{D} \bar{\mathcal{L}}) i T_{cd}{}^{ij} \gamma_{cd\alpha\beta} \gamma_{ab}^{\alpha\beta} \nabla_e P_e + (-\frac{1}{4} \mathcal{D}^\dagger \bar{\mathcal{H}} - \frac{1}{2} \mathcal{D} \bar{\mathcal{L}}) i E^{ik} R(V)_{cd}{}^j{}_k \gamma_{cd\alpha\beta} \gamma_{ab}^{\alpha\beta} + (\frac{1}{4} \mathcal{D}^\dagger \bar{\mathcal{H}} + \frac{1}{2} \mathcal{D} \bar{\mathcal{L}}) i E^{jk} R(V)_{cd}{}^i{}_k \gamma_{cd\alpha\beta} \gamma_{ab}^{\alpha\beta} \\
& + (\frac{1}{2} \mathcal{D}^\dagger \bar{\mathcal{H}} + \mathcal{D} \bar{\mathcal{L}}) i \gamma_{cd\alpha\beta} \gamma_{ab}^{\alpha\beta} \nabla_c \nabla_e T_{dekl} \varepsilon^{ijkl} + (\frac{1}{2} \mathcal{D}^\dagger \bar{\mathcal{H}} + \mathcal{D} \bar{\mathcal{L}}) i \gamma_{cd\alpha\beta} \gamma_{ab}^{\alpha\beta} \nabla_e \nabla_c T_{dekl} \varepsilon^{ijkl} - \frac{1}{6} i E_{kl} E^{kl} \mathcal{H} T_{cd}{}^{ij} \gamma_{cd\alpha\beta} \gamma_{ab}^{\alpha\beta} \\
& + \frac{1}{2} i E_{kl} \mathcal{H} R(V)_{cd}{}^k{}_m \gamma_{cd\alpha\beta} \gamma_{ab}^{\alpha\beta} \varepsilon^{ijlm} + 2 i \mathcal{H} P_c T_{cd}{}^{ij} \bar{P}_e \gamma_{de\alpha\beta} \gamma_{ab}^{\alpha\beta} + \frac{2}{3} i \mathcal{H} P_c T_{de}{}^{ij} \bar{P}_c \gamma_{de\alpha\beta} \gamma_{ab}^{\alpha\beta} + 2 i \mathcal{H} P_c T_{de}{}^{ij} \bar{P}_d \gamma_{ce\alpha\beta} \gamma_{ab}^{\alpha\beta} \\
& + \frac{1}{3} i T_{cdkl} \mathcal{D} \bar{\mathcal{L}} R(M)_{cdef} \gamma_{ab\dot{\alpha}\dot{\beta}} \gamma_{ef}^{\dot{\alpha}\dot{\beta}} \varepsilon^{ijkl} + \frac{2}{3} i T_{cdkl} \mathcal{D} \bar{\mathcal{L}} R(V)_{ce}{}^i{}_m \gamma_{ab\dot{\alpha}\dot{\beta}} \gamma_{de}^{\dot{\alpha}\dot{\beta}} \varepsilon^{jklm} - \frac{2}{3} i T_{cdkl} \mathcal{D} \bar{\mathcal{L}} R(V)_{ce}{}^j{}_m \gamma_{ab\dot{\alpha}\dot{\beta}} \gamma_{de}^{\dot{\alpha}\dot{\beta}} \varepsilon^{iklm} \\
& - 4 i \bar{\mathcal{L}} P_c \gamma_{cd\alpha\beta} \gamma_{ab}^{\alpha\beta} \nabla_e T_{dekl} \varepsilon^{ijkl} + (-2 \mathcal{D}^\dagger \mathcal{I} + \mathcal{D} \mathcal{H}) i E_{kl} T_{cd}{}^{ik} T_{ce}{}^{jl} \gamma_{de\alpha\beta} \gamma_{ab}^{\alpha\beta} + 2 i \bar{\mathcal{L}} T_{cdkl} \gamma_{ce\alpha\beta} \gamma_{ab}^{\alpha\beta} \nabla_d P_e \varepsilon^{ijkl} \\
& + 2 i \bar{\mathcal{L}} T_{cdkl} \gamma_{ce\alpha\beta} \gamma_{ab}^{\alpha\beta} \nabla_e P_d \varepsilon^{ijkl} - \frac{2}{3} i \bar{\mathcal{H}} T_{cdkl} T_{ef}{}^{ij} T_{ef}{}^{kl} \gamma_{ab\dot{\alpha}\dot{\beta}} \gamma_{cd}^{\dot{\alpha}\dot{\beta}} + 4 i \bar{\mathcal{L}} P_c P_c T_{de}{}^{ij} \gamma_{de\alpha\beta} \gamma_{ab}^{\alpha\beta} + 4 i \bar{\mathcal{L}} P_c \gamma_{de\alpha\beta} \gamma_{ab}^{\alpha\beta} \nabla_d T_{cekl} \varepsilon^{ijkl} \\
& + (-\frac{4}{3} \mathcal{H} + \frac{4}{3} \bar{\mathcal{H}}) i P_c T_{cd}{}^{ij} \bar{P}_e \gamma_{ab\dot{\alpha}\dot{\beta}} \gamma_{de}^{\dot{\alpha}\dot{\beta}} + (\frac{4}{3} \mathcal{D} \mathcal{D} \mathcal{H} + \frac{32}{3} \mathcal{I}) i T_{cd}{}^{ij} \bar{P}_c \bar{P}_e \gamma_{ab\dot{\alpha}\dot{\beta}} \gamma_{de}^{\dot{\alpha}\dot{\beta}} + (-\frac{2}{3} \mathcal{H} + \frac{2}{3} \bar{\mathcal{H}}) i \bar{P}_c \gamma_{ab\dot{\alpha}\dot{\beta}} \gamma_{cd}^{\dot{\alpha}\dot{\beta}} \nabla_e T_{dekl} \varepsilon^{ijkl} \\
& + (-\frac{2}{3} \mathcal{H} + \frac{2}{3} \bar{\mathcal{H}}) i \bar{P}_c \gamma_{ab\dot{\alpha}\dot{\beta}} \gamma_{de}^{\dot{\alpha}\dot{\beta}} \nabla_d T_{cekl} \varepsilon^{ijkl} + (-\frac{4}{3} \mathcal{H} + \frac{2}{3} \bar{\mathcal{H}}) i T_{cdkl} T_{ef}{}^{ik} T_{ef}{}^{jl} \gamma_{ab\dot{\alpha}\dot{\beta}} \gamma_{cd}^{\dot{\alpha}\dot{\beta}} + (-\frac{1}{3} \mathcal{H} + \frac{1}{3} \bar{\mathcal{H}}) i T_{cdkl} \gamma_{ab\dot{\alpha}\dot{\beta}} \gamma_{cd}^{\dot{\alpha}\dot{\beta}} \nabla_e \bar{P}_e \varepsilon^{ijkl} \\
& + (\frac{1}{12} \mathcal{D}^\dagger \mathcal{D}^\dagger \bar{\mathcal{H}} - \frac{1}{3} \bar{\mathcal{L}}) i E^{ik} E^{jl} T_{cdkl} \gamma_{ab\dot{\alpha}\dot{\beta}} \gamma_{cd}^{\dot{\alpha}\dot{\beta}} + (\frac{1}{6} \mathcal{H} - \frac{1}{6} \bar{\mathcal{H}}) i E_{kl} R(V)_{cd}{}^k{}_m \gamma_{ab\dot{\alpha}\dot{\beta}} \gamma_{cd}^{\dot{\alpha}\dot{\beta}} \varepsilon^{ijlm} \\
& + (\frac{1}{4} \mathcal{D}^\dagger \bar{\mathcal{H}} + \frac{1}{3} \mathcal{D} \bar{\mathcal{L}}) i D^{ij}{}_{kl} T_{cdmn} \gamma_{ab\dot{\alpha}\dot{\beta}} \gamma_{cd}^{\dot{\alpha}\dot{\beta}} \varepsilon^{klmn} + (\frac{4}{3} \mathcal{H} - \frac{4}{3} \bar{\mathcal{H}}) i P_c T_{de}{}^{ij} \bar{P}_d \gamma_{ab\dot{\alpha}\dot{\beta}} \gamma_{ce}^{\dot{\alpha}\dot{\beta}} - \frac{1}{8} i E_{kl} E_{mn} T_{cd}{}^{km} \mathcal{D} \mathcal{H} \gamma_{cd\alpha\beta} \gamma_{ab}^{\alpha\beta} \varepsilon^{ijln} \\
& - \frac{1}{18} i E_{kl} E^{kl} T_{cdmn} \mathcal{D} \bar{\mathcal{L}} \gamma_{ab\dot{\alpha}\dot{\beta}} \gamma_{cd}^{\dot{\alpha}\dot{\beta}} \varepsilon^{ijmn} - \frac{1}{2} i E^{ik} \mathcal{H} T_{cd}{}^{jl} T_{ce}{}^{mn} \gamma_{de\alpha\beta} \gamma_{ab}^{\alpha\beta} \varepsilon_{klmn} + \frac{1}{2} i E^{jk} \mathcal{H} T_{cd}{}^{il} T_{ce}{}^{mn} \gamma_{de\alpha\beta} \gamma_{ab}^{\alpha\beta} \varepsilon_{klmn} \\
& - \frac{2}{3} i P_c T_{cdkl} \mathcal{D} \bar{\mathcal{L}} \bar{P}_e \gamma_{ab\dot{\alpha}\dot{\beta}} \gamma_{de}^{\dot{\alpha}\dot{\beta}} \varepsilon^{ijkl} + \frac{2}{9} i P_c T_{dekl} \mathcal{D} \bar{\mathcal{L}} \bar{P}_c \gamma_{ab\dot{\alpha}\dot{\beta}} \gamma_{de}^{\dot{\alpha}\dot{\beta}} \varepsilon^{ijkl} - \frac{2}{3} i P_c T_{dekl} \mathcal{D} \bar{\mathcal{L}} \bar{P}_d \gamma_{ab\dot{\alpha}\dot{\beta}} \gamma_{ce}^{\dot{\alpha}\dot{\beta}} \varepsilon^{ijkl} \\
& + \frac{2}{3} i T_{cdkl} \mathcal{D}^\dagger \mathcal{I} \bar{P}_e \bar{P}_c \gamma_{ab\dot{\alpha}\dot{\beta}} \gamma_{cd}^{\dot{\alpha}\dot{\beta}} \varepsilon^{ijkl} + \frac{1}{4} i T_{cd}{}^{ij} T_{cd}{}^{kl} T_{ef}{}^{mn} \mathcal{D} \mathcal{H} \gamma_{ef\alpha\beta} \gamma_{ab}^{\alpha\beta} \varepsilon_{klmn} + 4 i \mathcal{D}^\dagger \bar{\mathcal{L}} P_c P_d T_{cekl} \gamma_{de\alpha\beta} \gamma_{ab}^{\alpha\beta} \varepsilon^{ijkl} \\
& - \frac{1}{8} i \mathcal{D}^\dagger \bar{\mathcal{H}} E^{ik} E^{jl} T_{cd}{}^{mn} \gamma_{cd\alpha\beta} \gamma_{ab}^{\alpha\beta} \varepsilon_{klmn} + (\frac{1}{6} \mathcal{D}^\dagger \mathcal{I} - \frac{1}{8} \mathcal{D} \mathcal{H}) i T_{cd}{}^{ij} T_{ef}{}^{kl} T_{ef}{}^{mn} \gamma_{cd\alpha\beta} \gamma_{ab}^{\alpha\beta} \varepsilon_{klmn} \\
& + \frac{1}{4} i \mathcal{D}^\dagger \bar{\mathcal{H}} T_{cdkl} T_{cdmn} T_{ef}{}^{mn} \gamma_{ef\alpha\beta} \gamma_{ab}^{\alpha\beta} \varepsilon^{ijkl} + (-\mathcal{D}^\dagger \bar{\mathcal{H}} - 2 \mathcal{D} \bar{\mathcal{L}}) i P_c T_{cdkl} \bar{P}_e \gamma_{de\alpha\beta} \gamma_{ab}^{\alpha\beta} \varepsilon^{ijkl} \\
& + (-\frac{1}{24} \mathcal{D}^\dagger \mathcal{D}^\dagger \bar{\mathcal{H}} - \frac{1}{3} \bar{\mathcal{L}}) i E^{ik} T_{cdkl} T_{cemn} \gamma_{ab\dot{\alpha}\dot{\beta}} \gamma_{de}^{\dot{\alpha}\dot{\beta}} \varepsilon^{jlmn} + (-\frac{1}{24} \mathcal{D}^\dagger \mathcal{D}^\dagger \bar{\mathcal{H}} - \frac{1}{3} \bar{\mathcal{L}}) i E^{jk} T_{cdlm} T_{cekn} \gamma_{ab\dot{\alpha}\dot{\beta}} \gamma_{de}^{\dot{\alpha}\dot{\beta}} \varepsilon^{ilmn} \\
& + (\frac{1}{24} \mathcal{D}^\dagger \mathcal{D}^\dagger \bar{\mathcal{H}} + \frac{1}{3} \bar{\mathcal{L}}) i E^{ik} T_{cdlm} T_{cekn} \gamma_{ab\dot{\alpha}\dot{\beta}} \gamma_{de}^{\dot{\alpha}\dot{\beta}} \varepsilon^{jlmn} + (\frac{1}{24} \mathcal{D}^\dagger \mathcal{D}^\dagger \bar{\mathcal{H}} + \frac{1}{3} \bar{\mathcal{L}}) i E^{jk} T_{cdkl} T_{cemn} \gamma_{ab\dot{\alpha}\dot{\beta}} \gamma_{de}^{\dot{\alpha}\dot{\beta}} \varepsilon^{ilmn} \\
& + (\frac{1}{8} \mathcal{D}^\dagger \bar{\mathcal{H}} + \frac{1}{3} \mathcal{D} \bar{\mathcal{L}}) i T_{cdkl} T_{cdmn} T_{ef}{}^{ij} \gamma_{ef\alpha\beta} \gamma_{ab}^{\alpha\beta} \varepsilon^{klmn} + (\mathcal{D}^\dagger \bar{\mathcal{H}} + 2 \mathcal{D} \bar{\mathcal{L}}) i P_c T_{dekl} \bar{P}_d \gamma_{ce\alpha\beta} \gamma_{ab}^{\alpha\beta} \varepsilon^{ijkl} \\
& + \frac{1}{180} i E_{kl} T_{cdmn} T_{cepq} \mathcal{D} \bar{\mathcal{L}} \gamma_{ab\dot{\alpha}\dot{\beta}} \gamma_{de}^{\dot{\alpha}\dot{\beta}} \varepsilon^{ijkm} \varepsilon^{lnpq} - \frac{1}{180} i E_{kl} T_{cdmn} T_{cepq} \mathcal{D} \bar{\mathcal{L}} \gamma_{ab\dot{\alpha}\dot{\beta}} \gamma_{de}^{\dot{\alpha}\dot{\beta}} \varepsilon^{ijkp} \varepsilon^{lmnq} \\
& + \frac{31}{360} i E_{kl} T_{cdmn} T_{cepq} \mathcal{D} \bar{\mathcal{L}} \gamma_{ab\dot{\alpha}\dot{\beta}} \gamma_{de}^{\dot{\alpha}\dot{\beta}} \varepsilon^{ikmn} \varepsilon^{jlpq} - \frac{31}{120} i E_{kl} T_{cdmn} T_{cepq} \mathcal{D} \bar{\mathcal{L}} \gamma_{ab\dot{\alpha}\dot{\beta}} \gamma_{de}^{\dot{\alpha}\dot{\beta}} \varepsilon^{ikpq} \varepsilon^{jlmn} \\
& + (\frac{1}{12} \mathcal{H} + \frac{1}{24} \bar{\mathcal{H}}) i E_{kl} E_{mn} T_{cdpq} \gamma_{ab\dot{\alpha}\dot{\beta}} \gamma_{cd}^{\dot{\alpha}\dot{\beta}} \varepsilon^{ijkm} \varepsilon^{lnpq} + (-\frac{1}{30} \mathcal{D}^\dagger \mathcal{D}^\dagger \bar{\mathcal{H}} - \frac{4}{15} \bar{\mathcal{L}}) i T_{cdkl} T_{cemn} T_{efpq} \gamma_{ab\dot{\alpha}\dot{\beta}} \gamma_{df}^{\dot{\alpha}\dot{\beta}} \varepsilon^{ijmn} \varepsilon^{klpq} \\
& + (\frac{1}{80} \mathcal{D}^\dagger \mathcal{D}^\dagger \bar{\mathcal{H}} + \frac{1}{60} \bar{\mathcal{L}}) i T_{cdkl} T_{cdmn} T_{efpq} \gamma_{ab\dot{\alpha}\dot{\beta}} \gamma_{ef}^{\dot{\alpha}\dot{\beta}} \varepsilon^{ijpq} \varepsilon^{klmn} + (-\frac{1}{40} \mathcal{D}^\dagger \mathcal{D}^\dagger \bar{\mathcal{H}} + \frac{3}{10} \bar{\mathcal{L}}) i T_{cdkl} T_{cdmn} T_{efpq} \gamma_{ab\dot{\alpha}\dot{\beta}} \gamma_{ef}^{\dot{\alpha}\dot{\beta}} \varepsilon^{ijmn} \varepsilon^{klpq}
\end{aligned}$$

The two fermion terms are

$$\begin{aligned}
[\mathcal{E}_{ab}^{ij}]_2 = & -2i\mathcal{H}R(Q)_{cd\alpha}{}^i R(Q)_{cd\beta}{}^j \gamma_{ab}{}^{\alpha\beta} - 4i\mathcal{H}\chi_{\alpha}{}^{ik}{}_l \chi_{\beta}{}^{jl}{}_k \gamma_{ab}{}^{\alpha\beta} - i\mathcal{H}R(Q)_{cd\alpha}{}^k \chi_{\beta}{}^{ij}{}_k \gamma_{cd\gamma}{}^{\beta} \gamma_{ab}{}^{\alpha\gamma} + \frac{1}{3}i\mathcal{D}\bar{\mathcal{L}}\Lambda^{\dot{\alpha}i}R(S)_{cd}{}^{\dot{\beta}j} \gamma_{ab\dot{\beta}\dot{\gamma}} \gamma_{cd}{}^{\dot{\gamma}}{}_{\dot{\alpha}} \\
& - \frac{1}{3}i\mathcal{D}\bar{\mathcal{L}}\Lambda^{\dot{\alpha}j}R(S)_{cd}{}^{\dot{\beta}i} \gamma_{ab\dot{\beta}\dot{\gamma}} \gamma_{cd}{}^{\dot{\gamma}}{}_{\dot{\alpha}} - \frac{2}{3}i\mathcal{D}\bar{\mathcal{L}}R(Q)_{cd}{}^{\dot{\alpha}}{}_k R(Q)_{cd}{}^{\dot{\beta}}{}_l \gamma_{ab\dot{\alpha}\dot{\beta}} \varepsilon^{ijkl} - \frac{19}{60}i\mathcal{D}\bar{\mathcal{L}}\chi^{\dot{\alpha}}{}_{kl} \chi^{\dot{\beta}}{}_{mn} \gamma_{ab\dot{\alpha}\dot{\beta}} \varepsilon^{klmn} \\
& - \frac{7}{20}i\mathcal{D}\bar{\mathcal{L}}\chi^{\dot{\alpha}}{}_{kl} \chi^{\dot{\beta}}{}_{mn} \gamma_{ab\dot{\alpha}\dot{\beta}} \varepsilon^{jlmn} + \frac{7}{20}i\mathcal{D}\bar{\mathcal{L}}\chi^{\dot{\alpha}}{}_{kl} \chi^{\dot{\beta}}{}_{mn} \gamma_{ab\dot{\alpha}\dot{\beta}} \varepsilon^{ilmn} + (-\frac{2}{3}\mathcal{D}^{\dagger}\mathcal{I} - \mathcal{D}\mathcal{H})iT_{cd}{}^{ij} \Lambda_{\alpha k}R(Q)_{cd\beta}{}^k \gamma_{ab}{}^{\alpha\beta} \\
& + (-\frac{2}{3}\mathcal{D}^{\dagger}\mathcal{I} + \mathcal{D}\mathcal{H})iT_{cd}{}^{jk} \Lambda_{\alpha k}R(Q)_{cd\beta}{}^i \gamma_{ab}{}^{\alpha\beta} + (\frac{2}{3}\mathcal{D}^{\dagger}\mathcal{I} - \mathcal{D}\mathcal{H})iT_{cd}{}^{ik} \Lambda_{\alpha k}R(Q)_{cd\beta}{}^j \gamma_{ab}{}^{\alpha\beta} + (-2\mathcal{D}^{\dagger}\bar{\mathcal{H}} - 4\mathcal{D}\bar{\mathcal{L}})i\chi_{\alpha}{}^{ij}{}_k \gamma_{c\beta\dot{\alpha}} \gamma_{ab}{}^{\alpha\beta} \nabla_c \Lambda^{\dot{\alpha}k} \\
& + (\frac{1}{3}\mathcal{H} + \frac{2}{3}\bar{\mathcal{H}})iE^{ik} \Lambda_{\alpha l} \chi_{\beta}{}^{jl}{}_k \gamma_{ab}{}^{\alpha\beta} + (\frac{1}{3}\mathcal{D}^{\dagger}\mathcal{D}^{\dagger}\bar{\mathcal{H}} + \frac{2}{3}\bar{\mathcal{L}})iE^{ik} \Lambda^{\dot{\alpha}l} \chi^{\dot{\beta}}{}_{kl} \gamma_{ab\dot{\alpha}\dot{\beta}} + (-\frac{1}{3}\mathcal{D}^{\dagger}\mathcal{D}^{\dagger}\bar{\mathcal{H}} - \frac{2}{3}\bar{\mathcal{L}})iE^{jk} \Lambda^{\dot{\alpha}l} \chi^{\dot{\beta}}{}_{kl} \gamma_{ab\dot{\alpha}\dot{\beta}} \\
& + (-\frac{1}{6}\mathcal{D}^{\dagger}\mathcal{D}^{\dagger}\bar{\mathcal{H}} + \frac{2}{3}\bar{\mathcal{L}})iD^{ij}{}_{kl} \Lambda^{\dot{\alpha}k} \Lambda^{\dot{\beta}l} \gamma_{ab\dot{\alpha}\dot{\beta}} + (-\frac{1}{3}\mathcal{H} - \frac{2}{3}\bar{\mathcal{H}})iE^{jk} \Lambda_{\alpha l} \chi_{\beta}{}^{il}{}_k \gamma_{ab}{}^{\alpha\beta} + (\mathcal{D}^{\dagger}\bar{\mathcal{H}} + 2\mathcal{D}\bar{\mathcal{L}})i\Lambda^{\dot{\alpha}k} \gamma_{c\alpha\dot{\alpha}} \gamma_{ab}{}^{\alpha\beta} \nabla_c \chi_{\beta}{}^{ij}{}_k \\
& + (\mathcal{D}^{\dagger}\bar{\mathcal{H}} + \frac{2}{3}\mathcal{D}\bar{\mathcal{L}})i\Lambda^{\dot{\alpha}k} \gamma_c{}^{\dot{\beta}\alpha} \gamma_{ab\dot{\alpha}\dot{\beta}} \nabla_c \chi_{\alpha}{}^{ij}{}_k + (\frac{2}{3}\mathcal{H} - \frac{4}{3}\bar{\mathcal{H}})iE^{kl} \Lambda_{\alpha k} \chi_{\beta}{}^{ij}{}_l \gamma_{ab}{}^{\alpha\beta} + \frac{9}{20}iE_{kl}\mathcal{D}\mathcal{H} \Lambda_{\alpha m} \chi_{\beta}{}^{ik}{}_n \gamma_{ab}{}^{\alpha\beta} \varepsilon^{jlmn} \\
& - \frac{9}{20}iE_{kl}\mathcal{D}\mathcal{H} \Lambda_{\alpha m} \chi_{\beta}{}^{jk}{}_n \gamma_{ab}{}^{\alpha\beta} \varepsilon^{ilmn} - \frac{11}{20}iE_{kl}\mathcal{D}\mathcal{H} \Lambda_{\alpha m} \chi_{\beta}{}^{km}{}_n \gamma_{ab}{}^{\alpha\beta} \varepsilon^{ijln} - \frac{7}{360}iE_{kl}\mathcal{D}\bar{\mathcal{L}}\Lambda^{\dot{\alpha}k} \chi^{\dot{\beta}}{}_{mn} \gamma_{ab\dot{\alpha}\dot{\beta}} \varepsilon^{jlmn} \\
& + \frac{7}{360}iE_{kl}\mathcal{D}\bar{\mathcal{L}}\Lambda^{\dot{\alpha}k} \chi^{\dot{\beta}}{}_{mn} \gamma_{ab\dot{\alpha}\dot{\beta}} \varepsilon^{ilmn} + \frac{1}{60}iE_{kl}\mathcal{D}\bar{\mathcal{L}}\Lambda^{\dot{\alpha}m} \chi^{\dot{\beta}}{}_{mn} \gamma_{ab\dot{\alpha}\dot{\beta}} \varepsilon^{ijln} - \frac{1}{6}iE^{ik} \mathcal{H} \Lambda_{\alpha k} R(Q)_{cd\beta}{}^j \gamma_{cd\gamma}{}^{\alpha} \gamma_{ab}{}^{\beta\gamma} \\
& + \frac{1}{6}iE^{jk} \mathcal{H} \Lambda_{\alpha k} R(Q)_{cd\beta}{}^i \gamma_{cd\gamma}{}^{\alpha} \gamma_{ab}{}^{\beta\gamma} + \frac{1}{3}iE^{ik} \mathcal{D}\bar{\mathcal{L}} \Lambda_{\alpha k} \gamma_c{}^{\dot{\alpha}\alpha} \gamma_{ab\dot{\alpha}\dot{\beta}} \nabla_c \Lambda^{\dot{\beta}j} - \frac{1}{3}iE^{jk} \mathcal{D}\bar{\mathcal{L}} \Lambda_{\alpha k} \gamma_c{}^{\dot{\alpha}\alpha} \gamma_{ab\dot{\alpha}\dot{\beta}} \nabla_c \Lambda^{\dot{\beta}i} \\
& - \frac{4}{9}iE^{ik} \mathcal{D}\bar{\mathcal{L}} \Lambda^{\dot{\alpha}j} \gamma_c{}^{\dot{\beta}\alpha} \gamma_{ab\dot{\alpha}\dot{\beta}} \nabla_c \Lambda_{\alpha k} + \frac{4}{9}iE^{jk} \mathcal{D}\bar{\mathcal{L}} \Lambda^{\dot{\alpha}i} \gamma_c{}^{\dot{\beta}\alpha} \gamma_{ab\dot{\alpha}\dot{\beta}} \nabla_c \Lambda_{\alpha k} - \frac{2}{3}i\mathcal{H}T_{cd}{}^{ij} \Lambda^{\dot{\alpha}k} \gamma_{c\alpha\dot{\alpha}} \gamma_{ab}{}^{\alpha\beta} \nabla_d \Lambda_{\beta k} \\
& + 2i\mathcal{H}T_{cd}{}^{ik} \Lambda^{\dot{\alpha}j} \gamma_{c\alpha\dot{\alpha}} \gamma_{ab}{}^{\alpha\beta} \nabla_d \Lambda_{\beta k} - 2i\mathcal{H}T_{cd}{}^{jk} \Lambda^{\dot{\alpha}i} \gamma_{c\alpha\dot{\alpha}} \gamma_{ab}{}^{\alpha\beta} \nabla_d \Lambda_{\beta k} - 2i\mathcal{H}T_{cd}{}^{ij} \Lambda^{\dot{\alpha}k} \gamma_c{}^{\dot{\beta}\alpha} \gamma_{ab\dot{\alpha}\dot{\beta}} \nabla_d \Lambda_{\alpha k} \\
& + \frac{2}{3}i\mathcal{H}T_{cd}{}^{ik} \Lambda^{\dot{\alpha}j} \gamma_c{}^{\dot{\beta}\alpha} \gamma_{ab\dot{\alpha}\dot{\beta}} \nabla_d \Lambda_{\alpha k} - \frac{2}{3}i\mathcal{H}T_{cd}{}^{jk} \Lambda^{\dot{\alpha}i} \gamma_c{}^{\dot{\beta}\alpha} \gamma_{ab\dot{\alpha}\dot{\beta}} \nabla_d \Lambda_{\alpha k} + \frac{1}{2}i\mathcal{H} \Lambda_{\alpha k} R(S)_{cd\beta l} \gamma_{cd\gamma}{}^{\alpha} \gamma_{ab}{}^{\beta\gamma} \varepsilon^{ijkl} + \frac{2}{3}i\mathcal{H} \Lambda^{\dot{\alpha}k} \bar{P}_c \chi_{\alpha}{}^{ij}{}_k \gamma_{c\beta\dot{\alpha}} \gamma_{ab}{}^{\alpha\beta} \\
& - \frac{1}{15}iT_{cd}{}^{ik} \mathcal{D}^{\dagger}\mathcal{I} \Lambda_{\alpha l} \chi_{\beta}{}^{jl}{}_k \gamma_{cd\gamma}{}^{\beta} \gamma_{ab}{}^{\alpha\gamma} + \frac{1}{15}iT_{cd}{}^{jk} \mathcal{D}^{\dagger}\mathcal{I} \Lambda_{\alpha l} \chi_{\beta}{}^{il}{}_k \gamma_{cd\gamma}{}^{\beta} \gamma_{ab}{}^{\alpha\gamma} - \frac{1}{9}i\mathcal{D}\bar{\mathcal{L}} \Lambda_{\alpha k} \Lambda^{\dot{\alpha}i} \gamma_c{}^{\dot{\beta}\alpha} \gamma_{ab\dot{\alpha}\dot{\beta}} \nabla_c E^{jk} \\
& + \frac{1}{9}i\mathcal{D}\bar{\mathcal{L}} \Lambda_{\alpha k} \Lambda^{\dot{\alpha}j} \gamma_c{}^{\dot{\beta}\alpha} \gamma_{ab\dot{\alpha}\dot{\beta}} \nabla_c E^{ik} + \frac{11}{60}i\mathcal{D}\bar{\mathcal{L}}R(Q)_{cd}{}^{\dot{\alpha}}{}_k \chi^{\dot{\beta}}{}_{lm} \gamma_{ab\dot{\alpha}\dot{\beta}} \gamma_{cd}{}^{\dot{\gamma}}{}_{\dot{\beta}} \varepsilon^{jklm} - \frac{11}{60}i\mathcal{D}\bar{\mathcal{L}}R(Q)_{cd}{}^{\dot{\alpha}}{}_k \chi^{\dot{\beta}}{}_{lm} \gamma_{ab\dot{\alpha}\dot{\beta}} \gamma_{cd}{}^{\dot{\gamma}}{}_{\dot{\beta}} \varepsilon^{iklm} \\
& - \frac{3}{20}i\mathcal{D}\bar{\mathcal{L}}R(Q)_{cd}{}^{\dot{\alpha}}{}_k \chi^{\dot{\beta}}{}_{lm} \gamma_{ab\dot{\alpha}\dot{\beta}} \gamma_{cd}{}^{\dot{\gamma}}{}_{\dot{\beta}} \varepsilon^{ijlm} - 8i\bar{\mathcal{L}}P_c \Lambda^{\dot{\alpha}k} \chi_{\alpha}{}^{ij}{}_k \gamma_{c\beta\dot{\alpha}} \gamma_{ab}{}^{\alpha\beta} + (-2\mathcal{D}^{\dagger}\mathcal{I} + \mathcal{D}\mathcal{H})iT_{cd}{}^{ij} \Lambda_{\alpha k} R(Q)_{ce\beta}{}^k \gamma_{de\gamma}{}^{\alpha} \gamma_{ab}{}^{\beta\gamma} \\
& + (-2\mathcal{D}^{\dagger}\mathcal{I} + \mathcal{D}\mathcal{H})iT_{cd}{}^{jk} \Lambda_{\alpha k} R(Q)_{ce\beta}{}^i \gamma_{de\gamma}{}^{\alpha} \gamma_{ab}{}^{\beta\gamma} + (-\frac{7}{5}\mathcal{D}^{\dagger}\mathcal{I} + \mathcal{D}\mathcal{H})iT_{cd}{}^{jk} \Lambda_{\alpha l} \chi_{\beta}{}^{il}{}_k \gamma_{cd\gamma}{}^{\alpha} \gamma_{ab}{}^{\beta\gamma} - 2i\bar{\mathcal{L}} \gamma_{c\alpha\dot{\alpha}} \gamma_{d\beta\dot{\beta}} \gamma_{ab}{}^{\alpha\beta} \nabla_c \Lambda^{\dot{\alpha}i} \nabla_d \Lambda^{\dot{\beta}j} \\
& - 2i\bar{\mathcal{L}} \gamma_{c\alpha\dot{\alpha}} \gamma_{d\beta\dot{\beta}} \gamma_{ab}{}^{\alpha\beta} \nabla_c \Lambda^{\dot{\beta}i} \nabla_d \Lambda^{\dot{\alpha}j} - \frac{3}{2}i\bar{\mathcal{L}} \Lambda^{\dot{\alpha}i} \gamma_{c\alpha\dot{\alpha}} \gamma_{d\beta\dot{\beta}} \gamma_{ab}{}^{\alpha\beta} \nabla_c \nabla_d \Lambda^{\dot{\beta}j} - \frac{1}{2}i\bar{\mathcal{L}} \Lambda^{\dot{\alpha}i} \gamma_{c\alpha\dot{\alpha}} \gamma_{d\beta\dot{\beta}} \gamma_{ab}{}^{\alpha\beta} \nabla_d \nabla_c \Lambda^{\dot{\beta}j} \\
& - \frac{1}{3}i\bar{\mathcal{L}} \Lambda^{\dot{\alpha}j} \Lambda^{\dot{\beta}k} R(V)_{cd}{}^i{}_k \gamma_{ab\dot{\alpha}\dot{\gamma}} \gamma_{cd}{}^{\dot{\gamma}}{}_{\dot{\beta}} + (-\frac{1}{6}\mathcal{D}^{\dagger}\mathcal{D}^{\dagger}\bar{\mathcal{H}} - \frac{2}{3}\bar{\mathcal{L}})iT_{cdkl} \Lambda^{\dot{\alpha}j} R(Q)_{cd}{}^{\dot{\beta}}{}_m \gamma_{ab\dot{\alpha}\dot{\beta}} \varepsilon^{iklm} + \frac{1}{3}i\bar{\mathcal{L}} \Lambda^{\dot{\alpha}i} \Lambda^{\dot{\beta}k} R(V)_{cd}{}^j{}_k \gamma_{ab\dot{\alpha}\dot{\gamma}} \gamma_{cd}{}^{\dot{\gamma}}{}_{\dot{\beta}} \\
& + (\frac{1}{6}\mathcal{D}^{\dagger}\mathcal{D}^{\dagger}\bar{\mathcal{H}} + \frac{2}{3}\bar{\mathcal{L}})iT_{cdkl} \Lambda^{\dot{\alpha}i} R(Q)_{cd}{}^{\dot{\beta}}{}_m \gamma_{ab\dot{\alpha}\dot{\beta}} \varepsilon^{jklm} + \frac{1}{2}i\bar{\mathcal{L}} \Lambda^{\dot{\alpha}j} \gamma_{c\alpha\dot{\alpha}} \gamma_{d\beta\dot{\beta}} \gamma_{ab}{}^{\alpha\beta} \nabla_d \nabla_c \Lambda^{\dot{\beta}i} + (\frac{8}{15}\mathcal{D}^{\dagger}\mathcal{I} + \mathcal{D}\mathcal{H})iT_{cd}{}^{kl} \Lambda_{\alpha k} \chi_{\beta}{}^{ij}{}_l \gamma_{cd\gamma}{}^{\beta} \gamma_{ab}{}^{\alpha\gamma} \\
& + \frac{3}{2}i\bar{\mathcal{L}} \Lambda^{\dot{\alpha}j} \gamma_{c\alpha\dot{\alpha}} \gamma_{d\beta\dot{\beta}} \gamma_{ab}{}^{\alpha\beta} \nabla_c \nabla_d \Lambda^{\dot{\beta}i} + (\frac{4}{5}\mathcal{D}^{\dagger}\mathcal{I} - \mathcal{D}\mathcal{H})iT_{cd}{}^{kl} \Lambda_{\alpha k} \chi_{\beta}{}^{ij}{}_l \gamma_{cd\gamma}{}^{\alpha} \gamma_{ab}{}^{\beta\gamma} + (\frac{7}{5}\mathcal{D}^{\dagger}\mathcal{I} - \mathcal{D}\mathcal{H})iT_{cd}{}^{ik} \Lambda_{\alpha l} \chi_{\beta}{}^{jl}{}_k \gamma_{cd\gamma}{}^{\alpha} \gamma_{ab}{}^{\beta\gamma} \\
& - i\bar{\mathcal{H}} \Lambda_{\alpha k} \gamma_{c\beta\dot{\alpha}} \gamma_{ab}{}^{\alpha\beta} \nabla_c \chi^{\dot{\alpha}}{}_{lm}{}^k \varepsilon^{ijlm} + (2\mathcal{D}^{\dagger}\mathcal{I} - \mathcal{D}\mathcal{H})iT_{cd}{}^{ik} \Lambda_{\alpha k} R(Q)_{ce\beta}{}^j \gamma_{de\gamma}{}^{\alpha} \gamma_{ab}{}^{\beta\gamma} + (\frac{2}{3}\mathcal{H} + \frac{4}{3}\bar{\mathcal{H}})i\Lambda^{\dot{\alpha}k} \bar{P}_c \chi_{\alpha}{}^{ij}{}_k \gamma_c{}^{\dot{\beta}\alpha} \gamma_{ab\dot{\alpha}\dot{\beta}} \\
& + (-\frac{8}{3}\mathcal{H} + \frac{4}{3}\bar{\mathcal{H}})iT_{cd}{}^{ij} \Lambda_{\alpha k} \gamma_{c\beta\dot{\alpha}} \gamma_{ab}{}^{\alpha\beta} \nabla_d \Lambda^{\dot{\alpha}k} + (-\frac{43}{60}\mathcal{H} + \frac{43}{60}\bar{\mathcal{H}})i\chi^{\dot{\alpha}}{}_{kl}{}^m \gamma_c{}^{\dot{\beta}\alpha} \gamma_{ab\dot{\alpha}\dot{\beta}} \nabla_c \Lambda_{\alpha m} \varepsilon^{ijkl} + (\frac{4}{3}\mathcal{H} + \frac{2}{3}\bar{\mathcal{H}})iT_{cd}{}^{ik} \Lambda_{\alpha k} \gamma_{c\beta\dot{\alpha}} \gamma_{ab}{}^{\alpha\beta} \nabla_d \Lambda^{\dot{\alpha}j} \\
& + (-\frac{2}{3}\mathcal{H} + \frac{2}{3}\bar{\mathcal{H}})iT_{cd}{}^{ik} \Lambda_{\alpha k} \gamma_c{}^{\dot{\alpha}\alpha} \gamma_{ab\dot{\alpha}\dot{\beta}} \nabla_d \Lambda^{\dot{\beta}j} + (-\frac{2}{3}\mathcal{H} + \frac{2}{3}\bar{\mathcal{H}})i\Lambda_{\alpha k} \Lambda^{\dot{\alpha}i} \gamma_{c\beta\dot{\alpha}} \gamma_{ab}{}^{\alpha\beta} \nabla_d T_{cd}{}^{jk} + (-\frac{4}{3}\mathcal{H} + \frac{2}{3}\bar{\mathcal{H}})i\Lambda_{\alpha k} \Lambda^{\dot{\alpha}j} \gamma_c{}^{\dot{\beta}\alpha} \gamma_{ab\dot{\alpha}\dot{\beta}} \nabla_d T_{cd}{}^{ik} \\
& + (\frac{1}{18}\mathcal{H} - \frac{1}{6}\bar{\mathcal{H}})iE^{ik} E^{jl} \Lambda_{\alpha k} \Lambda_{\beta l} \gamma_{ab}{}^{\alpha\beta} + (-\frac{1}{3}\mathcal{D}^{\dagger}\bar{\mathcal{H}} + \frac{1}{3}\mathcal{D}\bar{\mathcal{L}})i\Lambda_{\alpha k} \Lambda^{\dot{\alpha}j} \gamma_{c\beta\dot{\alpha}} \gamma_{ab}{}^{\alpha\beta} \nabla_c E^{ik} + (\frac{2}{3}\mathcal{D}\mathcal{D}\mathcal{H} + 4\mathcal{I})iT_{cd}{}^{ij} T_{cd}{}^{kl} \Lambda_{\alpha k} \Lambda_{\beta l} \gamma_{ab}{}^{\alpha\beta} \\
& + (-\frac{1}{6}\mathcal{D}^{\dagger}\bar{\mathcal{H}} + \frac{2}{3}\mathcal{D}\bar{\mathcal{L}})iE^{ik} \Lambda_{\alpha k} \gamma_{c\beta\dot{\alpha}} \gamma_{ab}{}^{\alpha\beta} \nabla_c \Lambda^{\dot{\alpha}j} + (-\frac{1}{6}\mathcal{D}^{\dagger}\bar{\mathcal{H}} + \frac{1}{120}\mathcal{D}\bar{\mathcal{L}})iE_{kl} \Lambda^{\dot{\alpha}j} \chi^{\dot{\beta}}{}_{mn} \gamma_{ab\dot{\alpha}\dot{\beta}} \varepsilon^{ilmn} + 1 \dots
\end{aligned}$$

$$\begin{aligned}
[\mathcal{E}_{ab}{}^{ij}]_{2,cont} = & +(-\frac{1}{6}\mathcal{D}^\dagger\bar{\mathcal{H}} - \frac{1}{3}\mathcal{D}\bar{\mathcal{I}})\mathrm{i}E^{ik}\Lambda^{\dot{\alpha}j}\gamma_{c\alpha\dot{\alpha}}\gamma_{ab}{}^{\alpha\beta}\nabla_c\Lambda_{\beta k} + (\frac{1}{3}\mathcal{D}^\dagger\mathcal{D}^\dagger\bar{\mathcal{H}} + \frac{2}{3}\bar{\mathcal{I}})\mathrm{i}T_{cdkl}\Lambda^{\dot{\alpha}m}R(Q)_{cd}{}^{\dot{\beta}}{}_m\gamma_{ab\dot{\alpha}\dot{\beta}}\varepsilon^{ijkl} \\
& + (-\frac{1}{8}\mathcal{D}^\dagger\bar{\mathcal{H}} - \frac{1}{4}\mathcal{D}\bar{\mathcal{I}})\mathrm{i}\Lambda^{\dot{\alpha}i}\gamma_{c\alpha\dot{\alpha}}\gamma_{de\beta}{}^{\alpha}\gamma_{ab}{}^{\beta\gamma}\nabla_c R(Q)_{de\gamma}{}^j + (-\frac{1}{8}\mathcal{D}^\dagger\bar{\mathcal{H}} - \frac{1}{4}\mathcal{D}\bar{\mathcal{I}})\mathrm{i}R(Q)_{cd\alpha}{}^j\gamma_{e\beta\dot{\alpha}}\gamma_{cd\gamma}{}^{\beta}\gamma_{ab}{}^{\alpha\gamma}\nabla_e\Lambda^{\dot{\alpha}i} \\
& + (\frac{1}{18}\mathcal{D}^\dagger\mathcal{D}^\dagger\bar{\mathcal{H}} - \frac{2}{9}\bar{\mathcal{I}})\mathrm{i}E_{kl}E^{jk}\Lambda^{\dot{\alpha}i}\Lambda^{\dot{\beta}l}\gamma_{ab\dot{\alpha}\dot{\beta}} + (-\frac{1}{10}\mathcal{H} + \frac{1}{10}\bar{\mathcal{H}})\mathrm{i}\Lambda_{\alpha k}\gamma_c{}^{\dot{\alpha}\alpha}\gamma_{ab\dot{\alpha}\dot{\beta}}\nabla_c\chi^{\dot{\beta}}{}_{lm}{}^l\varepsilon^{ijkm} \\
& + (-\frac{1}{12}\mathcal{D}^\dagger\mathcal{D}^\dagger\bar{\mathcal{H}} - \frac{2}{3}\bar{\mathcal{I}})\mathrm{i}E^{ik}\Lambda^{\dot{\alpha}j}R(Q)_{cd}{}^{\dot{\beta}}{}_k\gamma_{ab\dot{\beta}\dot{\gamma}}\gamma_{cd}{}^{\dot{\gamma}}{}_{\dot{\alpha}} + (\frac{1}{6}\mathcal{D}^\dagger\mathcal{D}^\dagger\bar{\mathcal{H}} + \frac{1}{3}\bar{\mathcal{I}})\mathrm{i}\Lambda^{\dot{\alpha}j}\Lambda^{\dot{\beta}k}R(V)_{cd}{}^i{}_k\gamma_{ab\dot{\beta}\dot{\gamma}}\gamma_{cd}{}^{\dot{\gamma}}{}_{\dot{\alpha}} \\
& + (-\frac{1}{20}\mathcal{H} + \frac{1}{20}\bar{\mathcal{H}})\mathrm{i}\Lambda_{\alpha k}\gamma_c{}^{\dot{\alpha}\alpha}\gamma_{ab\dot{\alpha}\dot{\beta}}\nabla_c\chi^{\dot{\beta}}{}_{lm}{}^j\varepsilon^{iklm} + (-\frac{1}{20}\mathcal{H} + \frac{1}{20}\bar{\mathcal{H}})\mathrm{i}\chi^{\dot{\alpha}}{}_{kl}{}^i\gamma_c{}^{\dot{\beta}\alpha}\gamma_{ab\dot{\alpha}\dot{\beta}}\nabla_c\Lambda_{\alpha m}\varepsilon^{jklm} \\
& + (-\frac{1}{18}\mathcal{D}^\dagger\mathcal{D}^\dagger\bar{\mathcal{H}} - \frac{1}{9}\bar{\mathcal{I}})\mathrm{i}E_{kl}E^{kl}\Lambda^{\dot{\alpha}i}\Lambda^{\dot{\beta}j}\gamma_{ab\dot{\alpha}\dot{\beta}} + (\frac{1}{20}\mathcal{H} - \frac{1}{20}\bar{\mathcal{H}})\mathrm{i}\Lambda_{\alpha k}\gamma_c{}^{\dot{\alpha}\alpha}\gamma_{ab\dot{\alpha}\dot{\beta}}\nabla_c\chi^{\dot{\beta}}{}_{lm}{}^i\varepsilon^{jklm} \\
& + (\frac{1}{20}\mathcal{H} - \frac{1}{20}\bar{\mathcal{H}})\mathrm{i}\chi^{\dot{\alpha}}{}_{kl}{}^j\gamma_c{}^{\dot{\beta}\alpha}\gamma_{ab\dot{\alpha}\dot{\beta}}\nabla_c\Lambda_{\alpha m}\varepsilon^{iklm} + (-\frac{1}{6}\mathcal{D}^\dagger\mathcal{D}^\dagger\bar{\mathcal{H}} - \frac{1}{3}\bar{\mathcal{I}})\mathrm{i}\Lambda^{\dot{\alpha}i}\Lambda^{\dot{\beta}k}R(V)_{cd}{}^j{}_k\gamma_{ab\dot{\beta}\dot{\gamma}}\gamma_{cd}{}^{\dot{\gamma}}{}_{\dot{\alpha}} \\
& + (\frac{1}{12}\mathcal{D}^\dagger\mathcal{D}^\dagger\bar{\mathcal{H}} + \frac{2}{3}\bar{\mathcal{I}})\mathrm{i}E^{jk}\Lambda^{\dot{\alpha}i}R(Q)_{cd}{}^{\dot{\beta}}{}_k\gamma_{ab\dot{\beta}\dot{\gamma}}\gamma_{cd}{}^{\dot{\gamma}}{}_{\dot{\alpha}} + (-\frac{1}{18}\mathcal{D}^\dagger\mathcal{D}^\dagger\bar{\mathcal{H}} + \frac{2}{9}\bar{\mathcal{I}})\mathrm{i}E_{kl}E^{ik}\Lambda^{\dot{\alpha}j}\Lambda^{\dot{\beta}l}\gamma_{ab\dot{\alpha}\dot{\beta}} \\
& + (\frac{1}{8}\mathcal{D}^\dagger\bar{\mathcal{H}} + \frac{1}{4}\mathcal{D}\bar{\mathcal{I}})\mathrm{i}\Lambda^{\dot{\alpha}j}\gamma_{c\alpha\dot{\alpha}}\gamma_{de\beta}{}^{\alpha}\gamma_{ab}{}^{\beta\gamma}\nabla_c R(Q)_{de\gamma}{}^i + (\frac{1}{8}\mathcal{D}^\dagger\bar{\mathcal{H}} + \frac{1}{4}\mathcal{D}\bar{\mathcal{I}})\mathrm{i}R(Q)_{cd\alpha}{}^i\gamma_{e\beta\dot{\alpha}}\gamma_{cd\gamma}{}^{\beta}\gamma_{ab}{}^{\alpha\gamma}\nabla_e\Lambda^{\dot{\alpha}j} \\
& + (\frac{1}{6}\mathcal{D}^\dagger\bar{\mathcal{H}} + \frac{1}{3}\mathcal{D}\bar{\mathcal{I}})\mathrm{i}E^{jk}\Lambda^{\dot{\alpha}i}\gamma_{c\alpha\dot{\alpha}}\gamma_{ab}{}^{\alpha\beta}\nabla_c\Lambda_{\beta k} + (\frac{1}{6}\mathcal{D}^\dagger\bar{\mathcal{H}} - \frac{1}{120}\mathcal{D}\bar{\mathcal{I}})\mathrm{i}E_{kl}\Lambda^{\dot{\alpha}i}\chi^{\dot{\beta}}{}_{mn}{}^k\gamma_{ab\dot{\alpha}\dot{\beta}}\varepsilon^{jlmn} \\
& + (\frac{1}{6}\mathcal{D}^\dagger\bar{\mathcal{H}} - \frac{2}{3}\mathcal{D}\bar{\mathcal{I}})\mathrm{i}E^{jk}\Lambda_{\alpha k}\gamma_{c\beta\dot{\alpha}}\gamma_{ab}{}^{\alpha\beta}\nabla_c\Lambda^{\dot{\alpha}i} + (\frac{3}{10}\mathcal{H} - \frac{3}{10}\bar{\mathcal{H}})\mathrm{i}\Lambda_{\alpha k}\gamma_{c\beta\dot{\alpha}}\gamma_{ab}{}^{\alpha\beta}\nabla_c\chi^{\dot{\beta}}{}_{lm}{}^l\varepsilon^{ijkm} \\
& + (\frac{1}{3}\mathcal{D}^\dagger\bar{\mathcal{H}} - \frac{1}{3}\mathcal{D}\bar{\mathcal{I}})\mathrm{i}\Lambda_{\alpha k}\Lambda^{\dot{\alpha}i}\gamma_{c\beta\dot{\alpha}}\gamma_{ab}{}^{\alpha\beta}\nabla_c E^{jk} + (\frac{23}{60}\mathcal{H} - \frac{23}{60}\bar{\mathcal{H}})\mathrm{i}\Lambda_{\alpha k}\gamma_c{}^{\dot{\alpha}\alpha}\gamma_{ab\dot{\alpha}\dot{\beta}}\nabla_c\chi^{\dot{\beta}}{}_{lm}{}^k\varepsilon^{ijlm} \\
& + (\frac{1}{2}\mathcal{D}^\dagger\bar{\mathcal{H}} + \frac{5}{12}\mathcal{D}\bar{\mathcal{I}})\mathrm{i}E_{kl}\Lambda^{\dot{\alpha}k}\chi^{\dot{\beta}}{}_{mn}{}^l\gamma_{ab\dot{\alpha}\dot{\beta}}\varepsilon^{ijmn} + (\frac{4}{3}\mathcal{H} - \frac{2}{3}\bar{\mathcal{H}})\mathrm{i}\Lambda_{\alpha k}\Lambda^{\dot{\alpha}i}\gamma_c{}^{\dot{\beta}\alpha}\gamma_{ab\dot{\alpha}\dot{\beta}}\nabla_d T_{cd}{}^{jk} \\
& + (\frac{2}{3}\mathcal{H} - \frac{2}{3}\bar{\mathcal{H}})\mathrm{i}T_{cd}{}^{jk}\Lambda_{\alpha k}\gamma_c{}^{\dot{\alpha}\alpha}\gamma_{ab\dot{\alpha}\dot{\beta}}\nabla_d\Lambda^{\dot{\beta}i} + (\frac{2}{3}\mathcal{H} - \frac{2}{3}\bar{\mathcal{H}})\mathrm{i}\Lambda_{\alpha k}\Lambda^{\dot{\alpha}j}\gamma_{c\beta\dot{\alpha}}\gamma_{ab}{}^{\alpha\beta}\nabla_d T_{cd}{}^{ik} + (-\frac{4}{3}\mathcal{H} - \frac{2}{3}\bar{\mathcal{H}})\mathrm{i}T_{cd}{}^{jk}\Lambda_{\alpha k}\gamma_{c\beta\dot{\alpha}}\gamma_{ab}{}^{\alpha\beta}\nabla_d\Lambda^{\dot{\alpha}i} \\
& + (-\frac{7}{3}\mathcal{D}\mathcal{D}\mathcal{H} - 8\mathcal{I})\mathrm{i}T_{cd}{}^{ik}T_{cd}{}^{jl}\Lambda_{\alpha k}\Lambda_{\beta l}\gamma_{ab}{}^{\alpha\beta} + (\frac{10}{3}\mathcal{H} - \frac{4}{3}\bar{\mathcal{H}})\mathrm{i}\Lambda_{\alpha k}\Lambda^{\dot{\alpha}k}\gamma_c{}^{\dot{\beta}\alpha}\gamma_{ab\dot{\alpha}\dot{\beta}}\nabla_d T_{cd}{}^{ij} + (\frac{4}{3}\mathcal{H} - \frac{4}{3}\bar{\mathcal{H}})\mathrm{i}T_{cd}{}^{ij}\Lambda_{\alpha k}\gamma_c{}^{\dot{\alpha}\alpha}\gamma_{ab\dot{\alpha}\dot{\beta}}\nabla_d\Lambda^{\dot{\beta}k} \\
& + (-\frac{2}{3}\mathcal{H} - \frac{4}{3}\bar{\mathcal{H}})\mathrm{i}\Lambda_{\alpha k}\Lambda^{\dot{\alpha}k}\gamma_{c\beta\dot{\alpha}}\gamma_{ab}{}^{\alpha\beta}\nabla_d T_{cd}{}^{ij} + \frac{1}{12}\mathrm{i}E_{kl}E^{kl}\mathcal{D}\mathcal{H}\Lambda_{\alpha m}\Lambda_{\beta n}\gamma_{ab}{}^{\alpha\beta}\varepsilon^{ijmn} - \frac{2}{3}\mathrm{i}E_{kl}\mathcal{H}\Lambda_{\alpha m}\gamma_{c\beta\dot{\alpha}}\gamma_{ab}{}^{\alpha\beta}\nabla_c\Lambda^{\dot{\alpha}k}\varepsilon^{ijlm} \\
& + \frac{1}{2}\mathrm{i}E_{kl}\mathcal{H}\Lambda^{\dot{\alpha}k}\gamma_{c\alpha\dot{\alpha}}\gamma_{ab}{}^{\alpha\beta}\nabla_c\Lambda_{\beta m}\varepsilon^{ijlm} - \frac{1}{9}\mathrm{i}E_{kl}\mathcal{D}\bar{\mathcal{I}}\Lambda^{\dot{\alpha}k}R(Q)_{cd}{}^{\dot{\beta}}{}_m\gamma_{ab\dot{\beta}\dot{\gamma}}\gamma_{cd}{}^{\dot{\gamma}}{}_{\dot{\alpha}}\varepsilon^{ijlm} + \frac{1}{6}\mathrm{i}\mathcal{H}T_{cd}{}^{ij}\Lambda_{\alpha k}\gamma_c{}^{\alpha}\gamma_{de\beta\gamma}\gamma_{ab}{}^{\beta\gamma}\nabla_e\Lambda^{\dot{\alpha}k} \\
& - \frac{5}{6}\mathrm{i}\mathcal{H}T_{cd}{}^{ij}\Lambda_{\alpha k}\gamma_e{}^{\alpha}\gamma_{cd\beta\gamma}\gamma_{ab}{}^{\beta\gamma}\nabla_e\Lambda^{\dot{\alpha}k} + \frac{1}{6}\mathrm{i}\mathcal{H}T_{cd}{}^{ij}\Lambda_{\alpha k}\gamma_e{}^{\alpha}\gamma_{ce\beta\gamma}\gamma_{ab}{}^{\beta\gamma}\nabla_d\Lambda^{\dot{\alpha}k} + \frac{1}{2}\mathrm{i}\mathcal{H}T_{cd}{}^{ik}\Lambda_{\alpha k}\gamma_e{}^{\alpha}\gamma_{cd\beta\gamma}\gamma_{ab}{}^{\beta\gamma}\nabla_e\Lambda^{\dot{\alpha}j} \\
& - \frac{1}{2}\mathrm{i}\mathcal{H}T_{cd}{}^{jk}\Lambda_{\alpha k}\gamma_e{}^{\alpha}\gamma_{cd\beta\gamma}\gamma_{ab}{}^{\beta\gamma}\nabla_e\Lambda^{\dot{\alpha}i} - \frac{1}{6}\mathrm{i}\mathcal{H}T_{cd}{}^{ij}\Lambda^{\dot{\alpha}k}\gamma_c{}^{\alpha}\gamma_{de\beta\gamma}\gamma_{ab}{}^{\beta\gamma}\nabla_e\Lambda_{\alpha k} - \frac{1}{6}\mathrm{i}\mathcal{H}T_{cd}{}^{ij}\Lambda^{\dot{\alpha}k}\gamma_e{}^{\alpha}\gamma_{ce\beta\gamma}\gamma_{ab}{}^{\beta\gamma}\nabla_d\Lambda_{\alpha k} \\
& + \frac{1}{6}\mathrm{i}\mathcal{H}\Lambda_{\alpha k}\Lambda^{\dot{\alpha}l}\gamma_{c\beta\dot{\alpha}}\gamma_{ab}{}^{\alpha\beta}\nabla_c E_{lm}\varepsilon^{ijkm} + \frac{1}{2}\mathrm{i}\mathcal{H}\$$

$$\begin{aligned}
[\mathcal{E}_{ab}^{ij}]_{2,cont} = & -\frac{2}{3}i\mathcal{D}\bar{\mathcal{L}}\Lambda^{\dot{\alpha}j}\bar{P}_c\gamma_{c\dot{\alpha}}^{\dot{\beta}}\gamma_d^{\dot{\alpha}}\gamma_{ab\dot{\beta}\dot{\gamma}}\nabla_d\Lambda^{\dot{\gamma}i} - i\mathcal{D}^\dagger\bar{\mathcal{H}}P_c\Lambda_{\alpha k}\chi^{\dot{\alpha}}{}_{lm}{}^k\gamma_{c\beta\dot{\alpha}}\gamma_{ab}{}^{\alpha\beta}\varepsilon^{ijlm} - \frac{2}{3}i\mathcal{D}^\dagger\bar{\mathcal{H}}P_cT_{cd}{}^{ik}\Lambda_{\alpha k}\Lambda^{\dot{\alpha}j}\gamma_d^{\dot{\beta}\alpha}\gamma_{ab\dot{\alpha}\dot{\beta}} \\
& + (-\frac{4}{3}\mathcal{D}^\dagger\mathcal{I} + \frac{2}{3}\mathcal{D}\mathcal{H})iT_{cd}{}^{ik}\Lambda_{\alpha k}\Lambda^{\dot{\alpha}j}\bar{P}_c\gamma_d^{\dot{\beta}\alpha}\gamma_{ab\dot{\alpha}\dot{\beta}} - \frac{1}{2}i\mathcal{D}^\dagger\bar{\mathcal{H}}T_{cd}{}^{ik}\Lambda^{\dot{\alpha}l}\chi^{\dot{\beta}}{}_{kl}{}^j\epsilon_{\dot{\alpha}\dot{\beta}}\gamma_{cd\alpha\beta}\gamma_{ab}{}^{\alpha\beta} \\
& - \frac{1}{2}i\mathcal{D}^\dagger\bar{\mathcal{H}}T_{cd}{}^{kl}\Lambda^{\dot{\alpha}i}\chi^{\dot{\beta}}{}_{kl}{}^j\epsilon_{\dot{\alpha}\dot{\beta}}\gamma_{cd\alpha\beta}\gamma_{ab}{}^{\alpha\beta} + 2i\mathcal{D}^\dagger\bar{\mathcal{L}}P_c\Lambda^{\dot{\alpha}j}\gamma_{c\alpha\dot{\alpha}}\gamma_{d\beta\dot{\beta}}\gamma_{ab}{}^{\alpha\beta}\nabla_d\Lambda^{\dot{\beta}i} + 2i\mathcal{D}^\dagger\bar{\mathcal{L}}P_c\Lambda^{\dot{\alpha}j}\gamma_{c\alpha\dot{\alpha}}\gamma_{d\beta\dot{\beta}}\gamma_{ab}{}^{\alpha\beta}\nabla_d\Lambda^{\dot{\beta}i} \\
& + (-\frac{1}{2}\mathcal{D}^\dagger\mathcal{I} + \frac{1}{4}\mathcal{D}\mathcal{H})iE_{kl}\Lambda_{\alpha m}R(Q)_{cd\beta}{}^k\gamma_{cd\gamma}{}^{\alpha\gamma}\gamma_{ab}{}^{\beta\gamma}\varepsilon^{ijlm} + (-\frac{4}{9}\mathcal{D}^\dagger\mathcal{I} + \frac{2}{3}\mathcal{D}\mathcal{H})iT_{cd}{}^{ik}\Lambda_{\alpha k}\Lambda^{\dot{\alpha}j}\bar{P}_c\gamma_{d\beta\dot{\alpha}}\gamma_{ab}{}^{\alpha\beta} \\
& + (-\frac{1}{3}\mathcal{D}^\dagger\mathcal{I} - \frac{1}{6}\mathcal{D}\mathcal{H})iE_{kl}E^{km}\Lambda_{\alpha m}\Lambda_{\beta n}\gamma_{ab}{}^{\alpha\beta}\varepsilon^{ijnl} - \frac{1}{2}i\bar{\mathcal{L}}P_c\Lambda^{\dot{\alpha}i}R(Q)_{de\alpha}{}^i\gamma_{c\beta\dot{\alpha}}\gamma_{de\gamma}{}^{\beta\gamma}\gamma_{ab}{}^{\alpha\gamma} - \frac{1}{2}i\bar{\mathcal{L}}\Lambda^{\dot{\alpha}i}\Lambda^{\dot{\beta}k}R(V)_{cd}{}^j{}^k\epsilon_{\dot{\alpha}\dot{\beta}}\gamma_{cd\alpha\beta}\gamma_{ab}{}^{\alpha\beta} \\
& - \frac{1}{2}i\bar{\mathcal{L}}\Lambda^{\dot{\alpha}j}\epsilon_{\dot{\alpha}\dot{\beta}}\gamma_{c\alpha\dot{\gamma}}\gamma_{d\beta}{}^{\dot{\gamma}}\gamma_{ab}{}^{\alpha\beta}\nabla_d\nabla_c\Lambda^{\dot{\beta}i} - \frac{2}{5}i\bar{\mathcal{L}}T_{cdkl}\Lambda^{\dot{\alpha}m}\chi^{\dot{\beta}}{}_{mn}{}^i\gamma_{ab\dot{\beta}\dot{\gamma}}\gamma_{cd}{}^{\dot{\gamma}}{}_{\dot{\alpha}}\varepsilon^{ijkln} + (-\frac{1}{6}\mathcal{D}^\dagger\mathcal{I} - \frac{1}{6}\mathcal{D}\mathcal{H})iE^{ik}T_{cd}{}^{jl}\Lambda_{\alpha k}\Lambda_{\beta l}\gamma_{cd\gamma}{}^{\beta\gamma}\gamma_{ab}{}^{\alpha\gamma} \\
& - \frac{1}{24}i\mathcal{D}^\dagger\mathcal{D}^\dagger\mathcal{D}^\dagger\bar{\mathcal{H}}E^{ik}E^{jl}\Lambda^{\dot{\alpha}m}\Lambda^{\dot{\beta}n}\gamma_{ab\dot{\alpha}\dot{\beta}}\varepsilon_{klmn} + (-\frac{1}{18}\mathcal{D}^\dagger\mathcal{I} + \frac{1}{6}\mathcal{D}\mathcal{H})iE^{jk}T_{cd}{}^{il}\Lambda_{\alpha k}\Lambda_{\beta l}\gamma_{cd\gamma}{}^{\alpha\gamma}\gamma_{ab}{}^{\beta\gamma} \\
& + \frac{1}{30}i\mathcal{D}^\dagger\bar{\mathcal{L}}E^{jk}T_{cdkl}\Lambda^{\dot{\alpha}i}\Lambda^{\dot{\beta}l}\gamma_{ab\dot{\alpha}\dot{\gamma}}\gamma_{cd}{}^{\dot{\gamma}}{}_{\dot{\beta}} - \frac{1}{30}i\mathcal{D}^\dagger\bar{\mathcal{L}}E^{ik}T_{cdkl}\Lambda^{\dot{\alpha}j}\Lambda^{\dot{\beta}l}\gamma_{ab\dot{\alpha}\dot{\gamma}}\gamma_{cd}{}^{\dot{\gamma}}{}_{\dot{\beta}} + (\frac{1}{18}\mathcal{D}^\dagger\mathcal{I} - \frac{1}{6}\mathcal{D}\mathcal{H})iE^{ik}T_{cd}{}^{jl}\Lambda_{\alpha k}\Lambda_{\beta l}\gamma_{cd\gamma}{}^{\alpha\gamma}\gamma_{ab}{}^{\beta\gamma} \\
& + \frac{1}{12}i\mathcal{D}^\dagger\mathcal{D}^\dagger\mathcal{D}^\dagger\bar{\mathcal{H}}T_{cdkl}T_{cdmn}\Lambda^{\dot{\alpha}m}\Lambda^{\dot{\beta}n}\gamma_{ab\dot{\alpha}\dot{\beta}}\varepsilon^{ijkl} + (\frac{1}{6}\mathcal{D}^\dagger\mathcal{I} + \frac{1}{6}\mathcal{D}\mathcal{H})iE^{jk}T_{cd}{}^{il}\Lambda_{\alpha k}\Lambda_{\beta l}\gamma_{cd\gamma}{}^{\beta\gamma}\gamma_{ab}{}^{\alpha\gamma} \\
& + \frac{2}{5}i\bar{\mathcal{L}}T_{cdkl}\Lambda^{\dot{\alpha}m}\chi^{\dot{\beta}}{}_{mn}{}^j\gamma_{ab\dot{\beta}\dot{\gamma}}\gamma_{cd}{}^{\dot{\gamma}}{}_{\dot{\alpha}}\varepsilon^{ikln} + (\frac{2}{9}\mathcal{D}^\dagger\mathcal{I} + \frac{1}{6}\mathcal{D}\mathcal{H})iE^{kl}T_{cd}{}^{ij}\Lambda_{\alpha k}\Lambda_{\beta l}\gamma_{cd\gamma}{}^{\alpha\gamma}\gamma_{ab}{}^{\beta\gamma} + \frac{1}{2}i\bar{\mathcal{L}}P_c\Lambda^{\dot{\alpha}j}R(Q)_{de\alpha}{}^i\gamma_{c\beta\dot{\alpha}}\gamma_{de\gamma}{}^{\beta\gamma}\gamma_{ab}{}^{\alpha\gamma} \\
& + \frac{1}{2}i\bar{\mathcal{L}}\Lambda^{\dot{\alpha}j}\Lambda^{\dot{\beta}k}R(V)_{cd}{}^i{}^k\epsilon_{\dot{\alpha}\dot{\beta}}\gamma_{cd\alpha\beta}\gamma_{ab}{}^{\alpha\beta} + \frac{1}{2}i\bar{\mathcal{L}}\Lambda^{\dot{\alpha}i}\epsilon_{\dot{\alpha}\dot{\beta}}\gamma_{c\alpha\dot{\gamma}}\gamma_{d\beta}{}^{\dot{\gamma}}\gamma_{ab}{}^{\alpha\beta}\nabla_d\nabla_c\Lambda^{\dot{\beta}j} + (\frac{4}{9}\mathcal{D}^\dagger\mathcal{I} - \frac{2}{3}\mathcal{D}\mathcal{H})iT_{cd}{}^{jk}\Lambda_{\alpha k}\Lambda^{\dot{\alpha}i}\bar{P}_c\gamma_{d\beta\dot{\alpha}}\gamma_{ab}{}^{\alpha\beta} \\
& + (\frac{4}{9}\mathcal{D}^\dagger\mathcal{I} + \frac{2}{3}\mathcal{D}\mathcal{H})iT_{cd}{}^{ij}\Lambda_{\alpha k}\Lambda^{\dot{\alpha}k}\bar{P}_c\gamma_{d\beta\dot{\alpha}}\gamma_{ab}{}^{\alpha\beta} - i\mathcal{D}^\dagger\bar{\mathcal{L}}\Lambda^{\dot{\alpha}i}\Lambda^{\dot{\beta}j}\gamma_{c\alpha\dot{\alpha}}\gamma_{d\beta\dot{\beta}}\gamma_{ab}{}^{\alpha\beta}\nabla_cP_d - i\mathcal{D}^\dagger\bar{\mathcal{L}}\Lambda^{\dot{\alpha}i}\Lambda^{\dot{\beta}j}\gamma_{c\alpha\dot{\alpha}}\gamma_{d\beta\dot{\beta}}\gamma_{ab}{}^{\alpha\beta}\nabla_dP_c \\
& + \frac{1}{2}i\mathcal{D}^\dagger\bar{\mathcal{H}}T_{cd}{}^{jk}\Lambda^{\dot{\alpha}l}\chi^{\dot{\beta}}{}_{kl}{}^i\epsilon_{\dot{\alpha}\dot{\beta}}\gamma_{cd\alpha\beta}\gamma_{ab}{}^{\alpha\beta} + \frac{1}{2}i\mathcal{D}^\dagger\bar{\mathcal{H}}T_{cd}{}^{kl}\Lambda^{\dot{\alpha}j}\chi^{\dot{\beta}}{}_{kl}{}^i\epsilon_{\dot{\alpha}\dot{\beta}}\gamma_{cd\alpha\beta}\gamma_{ab}{}^{\alpha\beta} - 2i\mathcal{D}^\dagger\bar{\mathcal{L}}P_c\Lambda^{\dot{\alpha}i}\gamma_{c\alpha\dot{\alpha}}\gamma_{d\beta\dot{\beta}}\gamma_{ab}{}^{\alpha\beta}\nabla_d\Lambda^{\dot{\beta}j} \\
& - 2i\mathcal{D}^\dagger\bar{\mathcal{L}}P_c\Lambda^{\dot{\alpha}i}\gamma_{c\alpha\dot{\alpha}}\gamma_{d\beta\dot{\beta}}\gamma_{ab}{}^{\alpha\beta}\nabla_d\Lambda^{\dot{\beta}j} + \frac{2}{3}i\mathcal{D}^\dagger\bar{\mathcal{H}}P_cT_{cd}{}^{jk}\Lambda_{\alpha k}\Lambda^{\dot{\alpha}i}\gamma_d^{\dot{\beta}\alpha}\gamma_{ab\dot{\alpha}\dot{\beta}} + (\frac{4}{3}\mathcal{D}^\dagger\mathcal{I} - \frac{2}{3}\mathcal{D}\mathcal{H})iT_{cd}{}^{jk}\Lambda_{\alpha k}\Lambda^{\dot{\alpha}i}\bar{P}_c\gamma_d^{\dot{\beta}\alpha}\gamma_{ab\dot{\alpha}\dot{\beta}} \\
& + (\frac{20}{3}\mathcal{D}^\dagger\mathcal{I} - 2\mathcal{D}\mathcal{H})iT_{cd}{}^{ij}\Lambda_{\alpha k}\Lambda^{\dot{\alpha}k}\bar{P}_c\gamma_d^{\dot{\beta}\alpha}\gamma_{ab\dot{\alpha}\dot{\beta}} + (-2\mathcal{D}^\dagger\bar{\mathcal{H}} - \frac{4}{3}\mathcal{D}\bar{\mathcal{L}})iP_cT_{cd}{}^{ij}\Lambda_{\alpha k}\Lambda^{\dot{\alpha}k}\gamma_{d\beta\dot{\alpha}}\gamma_{ab}{}^{\alpha\beta} \\
& + (-\frac{5}{6}\mathcal{D}^\dagger\bar{\mathcal{H}} - \frac{5}{3}\mathcal{D}\bar{\mathcal{L}})i\Lambda^{\dot{\alpha}i}\bar{P}_c\gamma_{c\alpha\dot{\alpha}}\gamma_{d\beta\dot{\beta}}\gamma_{ab}{}^{\alpha\beta}\nabla_d\Lambda^{\dot{\beta}j} + (-\frac{1}{2}\mathcal{D}^\dagger\bar{\mathcal{H}} - \frac{31}{90}\mathcal{D}\bar{\mathcal{L}})iT_{cdkl}\Lambda^{\dot{\alpha}m}\gamma_c^{\dot{\beta}\alpha}\gamma_{ab\dot{\alpha}\dot{\beta}}\nabla_d\Lambda_{\alpha m}\varepsilon^{ijkl} \\
& + (-\frac{1}{2}\mathcal{D}^\dagger\bar{\mathcal{H}} - \frac{7}{15}\mathcal{D}\bar{\mathcal{L}})i\Lambda_{\alpha k}\Lambda^{\dot{\alpha}k}\gamma_c^{\dot{\beta}\alpha}\gamma_{ab\dot{\alpha}\dot{\beta}}\nabla_dT_{cdlm}\varepsilon^{ijlm} + (-\frac{1}{2}\mathcal{D}^\dagger\bar{\mathcal{H}} - \mathcal{D}\bar{\mathcal{L}})iT_{cdkl}\Lambda^{\dot{\alpha}i}\gamma_{c\alpha\dot{\alpha}}\gamma_{ab}{}^{\alpha\beta}\nabla_d\Lambda_{\beta m}\varepsilon^{jklm} \\
& + (-\frac{1}{2}\mathcal{D}^\dagger\bar{\mathcal{H}} - \frac{5}{3}\mathcal{D}\bar{\mathcal{L}})i\Lambda_{\alpha k}\Lambda^{\dot{\alpha}j}\gamma_{c\beta\dot{\alpha}}\gamma_{ab}{}^{\alpha\beta}\nabla_dT_{cdlm}\varepsilon^{iklm} + (-\frac{1}{2}\mathcal{D}^\dagger\bar{\mathcal{H}} - \frac{7}{3}\mathcal{D}\bar{\mathcal{L}})i\Lambda_{\alpha k}\Lambda^{\dot{\alpha}k}\gamma_{c\beta\dot{\alpha}}\gamma_{ab}{}^{\alpha\beta}\nabla_dT_{cdlm}\varepsilon^{ijlm} \\
& + (\frac{1}{9}\mathcal{H} + \frac{1}{3}\bar{\mathcal{H}})iE^{ik}\Lambda_{\alpha k}\Lambda^{\dot{\alpha}j}\bar{P}_c\gamma_{c\beta\dot{\alpha}}\gamma_{ab}{}^{\alpha\beta} + (\frac{5}{18}\mathcal{H} + \frac{2}{9}\bar{\mathcal{H}})i\Lambda_{\alpha k}\Lambda^{\dot{\alpha}l}\gamma_c^{\dot{\beta}\alpha}\gamma_{ab\dot{\alpha}\dot{\beta}}\nabla_cE_{lm}\varepsilon^{ijkm} \\
& + (-\frac{1}{5}\mathcal{D}^\dagger\bar{\mathcal{H}} - \frac{2}{5}\mathcal{D}\bar{\mathcal{L}})iT_{cd}{}^{ij}\Lambda^{\dot{\alpha}k}R(Q)_{ce}{}^{\dot{\beta}}{}^k\epsilon_{\dot{\alpha}\dot{\beta}}\gamma_{de\alpha\beta}\gamma_{ab}{}^{\alpha\beta} + (\frac{1}{6}\mathcal{D}^\dagger\mathcal{D}^\dagger\bar{\mathcal{H}} - \frac{1}{15}\bar{\mathcal{L}})iT_{cdkl}\Lambda^{\dot{\alpha}m}\chi^{\dot{\beta}}{}_{mn}{}^j\gamma_{ab\dot{\beta}\dot{\gamma}}\gamma_{cd}{}^{\dot{\gamma}}{}_{\dot{\beta}}\varepsilon^{ikln} \\
& + (-\frac{1}{6}\mathcal{D}^\dagger\bar{\mathcal{H}} + \frac{1}{15}\mathcal{D}\bar{\mathcal{L}})i\Lambda_{\alpha k}\Lambda^{\dot{\alpha}i}\gamma_c^{\dot{\beta}\alpha}\gamma_{ab\dot{\alpha}\dot{\beta}}\nabla_dT_{cdlm}\varepsilon^{jklm} + (-\frac{1}{6}\mathcal{D}^\dagger\bar{\mathcal{H}} - \frac{1}{3}\mathcal{D}\bar{\mathcal{L}})i\Lambda^{\dot{\alpha}i}\Lambda^{\dot{\beta}j}\gamma_{c\alpha\dot{\alpha}}\gamma_{d\beta\dot{\beta}}\gamma_{ab}{}^{\alpha\beta}\nabla_c\bar{P}_d \\
& + (-\frac{1}{6}\mathcal{D}^\dagger\bar{\mathcal{H}} - \frac{1}{3}\mathcal{D}\bar{\mathcal{L}})i\Lambda^{\dot{\alpha}i}\Lambda^{\dot{\beta}j}\gamma_{c\alpha\dot{\alpha}}\gamma_{d\beta\dot{\beta}}\gamma_{ab}{}^{\alpha\beta}\nabla_d\bar{P}_c + (-\frac{1}{6}\mathcal{D}^\dagger\bar{\mathcal{H}} - \frac{1}{3}\mathcal{D}\bar{\mathcal{L}})i\Lambda^{\dot{\alpha}i}\bar{P}_c\gamma_{c\alpha\dot{\alpha}}\gamma_{d\beta\dot{\beta}}\gamma_{ab}{}^{\alpha\beta}\nabla_d\Lambda^{\dot{\beta}j} \\
& + (-\frac{1}{6}\mathcal{D}^\dagger\bar{\mathcal{H}} - \frac{22}{45}\mathcal{D}\bar{\mathcal{L}})iT_{cdkl}\Lambda^{\dot{\alpha}i}\gamma_c^{\dot{\beta}\alpha}\gamma_{ab\dot{\alpha}\dot{\beta}}\nabla_d\Lambda_{\alpha m}\varepsilon^{jklm} + (-\frac{1}{6}\mathcal{D}^\dagger\mathcal{D}^\dagger\bar{\mathcal{H}} - \frac{4}{3}\bar{\mathcal{L}})iT_{cdkl}\Lambda^{\dot{\alpha}j}R(Q)_{ce}{}^{\dot{\beta}}{}^m\gamma_{ab\dot{\beta}\dot{\gamma}}\gamma_{de}{}^{\dot{\gamma}}{}_{\dot{\alpha}}\varepsilon^{iklm} \\
& + (\frac{1}{2}\mathcal{D}^\dagger\mathcal{D}^\dagger\bar{\mathcal{H}} + \frac{4}{3}\bar{\mathcal{L}})iE^{jk}P_c\Lambda_{\alpha k}\Lambda^{\dot{\alpha}i}\gamma_{c\beta\dot{\alpha}}\gamma_{ab}{}^{\alpha\beta} + (\frac{7}{6}\mathcal{D}\mathcal{D}\mathcal{H} + \frac{10}{3}\mathcal{I})iT_{cd}{}^{ik}T_{ce}{}^{jl}\Lambda_{\alpha k}\Lambda_{\beta l}\gamma_{de\gamma}{}^{\beta\gamma}\gamma_{ab}{}^{\alpha\gamma} \\
& + (\frac{7}{18}\mathcal{H} + \frac{1}{9}\bar{\mathcal{H}})iE_{kl}\Lambda^{\dot{\alpha}k}\gamma_c^{\dot{\beta}\alpha}\gamma_{ab\dot{\alpha}\dot{\beta}}\nabla_c\Lambda_{\alpha m}\varepsilon^{ijlm} + (-\frac{1}{9}\mathcal{H} + \frac{1}{9}\bar{\mathcal{H}})iE_{kl}\Lambda_{\alpha m}\gamma_c^{\dot{\alpha}\alpha}\gamma_{ab\dot{\alpha}\dot{\beta}}\nabla_c\Lambda^{\dot{\beta}k}\varepsilon^{ijlm} + 3\cdots
\end{aligned}$$

$$\begin{aligned}
[\mathcal{E}_{ab}{}^{ij}]_{2,cont} = & +(-\frac{1}{9}\mathcal{H} + \frac{1}{9}\bar{\mathcal{H}})iE^{jk}\Lambda_{\alpha k}\Lambda^{\dot{\alpha}k}\bar{P}_c\gamma_c{}^{\dot{\beta}\alpha}\gamma_{ab\dot{\alpha}\dot{\beta}} + (-\frac{1}{10}\mathcal{D}^\dagger\bar{\mathcal{H}} - \frac{1}{5}\mathcal{D}\bar{\mathcal{L}})iT_{cd}{}^{ik}\Lambda^{\dot{\alpha}j}R(Q)_{ce}{}^{\dot{\beta}}{}_{k\epsilon\dot{\alpha}\dot{\beta}}\gamma_{de\alpha\beta}\gamma_{ab}{}^{\alpha\beta} \\
& + (\frac{1}{12}\mathcal{D}^\dagger\mathcal{D}^\dagger\bar{\mathcal{H}} - \frac{1}{15}\bar{\mathcal{L}})iT_{cdkl}\Lambda^{\dot{\alpha}j}\chi^{\dot{\beta}}{}_{mn}{}^i\gamma_{ab\dot{\alpha}\dot{\gamma}}\gamma_{cd}{}^{\dot{\gamma}}{}_{\dot{\beta}}\epsilon^{klmn} + (-\frac{1}{12}\mathcal{H} + \frac{1}{12}\bar{\mathcal{H}})i\Lambda_{\alpha k}\gamma_c{}^{\dot{\alpha}\alpha}\gamma_{ab\dot{\beta}\dot{\gamma}}\gamma_{de}{}^{\dot{\beta}}{}_{\dot{\alpha}}\nabla_e R(Q)_{de}{}^{\dot{\gamma}}{}_{\dot{l}}\epsilon^{ijkl} \\
& + (-\frac{1}{12}\mathcal{D}^\dagger\bar{\mathcal{H}} - \frac{1}{27}\mathcal{D}\bar{\mathcal{L}})iE_{kl}E_{mn}\Lambda^{\dot{\alpha}k}\Lambda^{\dot{\beta}m}\gamma_{ab\dot{\alpha}\dot{\beta}}\epsilon^{ijnl} + (-\frac{1}{12}\mathcal{D}^\dagger\bar{\mathcal{H}} - \frac{1}{6}\mathcal{D}\bar{\mathcal{L}})iT_{cd}{}^{kl}T_{cd}{}^{mn}\Lambda^{\dot{\alpha}i}\Lambda^{\dot{\beta}j}\gamma_{ab\dot{\alpha}\dot{\beta}}\epsilon_{klmn} \\
& + (-\frac{1}{18}\mathcal{D}^\dagger\mathcal{D}^\dagger\bar{\mathcal{H}} - \frac{4}{9}\bar{\mathcal{L}})iE^{ik}P_c\Lambda_{\alpha k}\Lambda^{\dot{\alpha}j}\gamma_c{}^{\dot{\beta}\alpha}\gamma_{ab\dot{\alpha}\dot{\beta}} + (-\frac{1}{18}\mathcal{D}^\dagger\mathcal{D}^\dagger\bar{\mathcal{H}} - \frac{4}{9}\bar{\mathcal{L}})iP_c\Lambda^{\dot{\alpha}i}\Lambda^{\dot{\beta}j}\bar{P}_d\gamma_{ab\dot{\alpha}\dot{\gamma}}\gamma_{cd}{}^{\dot{\gamma}}{}_{\dot{\beta}} \\
& + (-\frac{1}{18}\mathcal{D}^\dagger\mathcal{D}^\dagger\bar{\mathcal{H}} - \frac{4}{9}\bar{\mathcal{L}})iP_c\Lambda^{\dot{\alpha}i}\Lambda^{\dot{\beta}j}\bar{P}_d\gamma_{ab\dot{\beta}\dot{\gamma}}\gamma_{cd}{}^{\dot{\gamma}}{}_{\dot{\alpha}} + (\frac{1}{12}\mathcal{D}^\dagger\mathcal{D}^\dagger\bar{\mathcal{H}} + \frac{4}{15}\bar{\mathcal{L}})iT_{cdkl}\Lambda^{\dot{\alpha}i}\chi^{\dot{\beta}}{}_{mn}{}^j\gamma_{ab\dot{\beta}\dot{\gamma}}\gamma_{cd}{}^{\dot{\gamma}}{}_{\dot{\alpha}}\epsilon^{klmn} \\
& + (-\frac{1}{12}\mathcal{D}^\dagger\mathcal{D}^\dagger\mathcal{D}^\dagger\bar{\mathcal{H}} - \frac{3}{10}\mathcal{D}^\dagger\bar{\mathcal{L}})iE^{ik}T_{cdkl}\Lambda^{\dot{\alpha}j}\Lambda^{\dot{\beta}l}\gamma_{ab\dot{\beta}\dot{\gamma}}\gamma_{cd}{}^{\dot{\gamma}}{}_{\dot{\alpha}} + (\frac{1}{12}\mathcal{D}^\dagger\mathcal{D}^\dagger\mathcal{D}^\dagger\bar{\mathcal{H}} + \frac{3}{10}\mathcal{D}^\dagger\bar{\mathcal{L}})iE^{jk}T_{cdkl}\Lambda^{\dot{\alpha}i}\Lambda^{\dot{\beta}l}\gamma_{ab\dot{\beta}\dot{\gamma}}\gamma_{cd}{}^{\dot{\gamma}}{}_{\dot{\alpha}} \\
& + (-\frac{1}{12}\mathcal{D}^\dagger\mathcal{D}^\dagger\bar{\mathcal{H}} - \frac{4}{15}\bar{\mathcal{L}})iT_{cdkl}\Lambda^{\dot{\alpha}j}\chi^{\dot{\beta}}{}_{mn}{}^i\gamma_{ab\dot{\beta}\dot{\gamma}}\gamma_{cd}{}^{\dot{\gamma}}{}_{\dot{\alpha}}\epsilon^{klmn} + (\frac{1}{24}\mathcal{D}^\dagger\mathcal{D}^\dagger\bar{\mathcal{H}} + \frac{1}{3}\bar{\mathcal{L}})i\Lambda^{\dot{\alpha}i}\Lambda^{\dot{\beta}j}R(M)_{cdef}\gamma_{ab\dot{\gamma}\dot{\delta}}\gamma_{cd\dot{\alpha}\dot{\beta}}\gamma_{ef}{}^{\dot{\gamma}\dot{\delta}} \\
& + (-\frac{1}{24}\mathcal{D}^\dagger\mathcal{D}^\dagger\mathcal{D}^\dagger\bar{\mathcal{H}} - \frac{1}{3}\mathcal{D}^\dagger\bar{\mathcal{L}})iT_{cdkl}T_{cdmn}\Lambda^{\dot{\alpha}i}\Lambda^{\dot{\beta}j}\gamma_{ab\dot{\alpha}\dot{\beta}}\epsilon^{klmn} + (\frac{1}{18}\mathcal{D}^\dagger\mathcal{D}^\dagger\bar{\mathcal{H}} + \frac{4}{9}\bar{\mathcal{L}})iE^{jk}P_c\Lambda_{\alpha k}\Lambda^{\dot{\alpha}i}\gamma_c{}^{\dot{\beta}\alpha}\gamma_{ab\dot{\alpha}\dot{\beta}} \\
& + (\frac{1}{12}\mathcal{H} - \frac{1}{12}\bar{\mathcal{H}})iR(Q)_{cd}{}^{\dot{\alpha}}{}_{k\gamma_e}{}^{\dot{\beta}\alpha}\gamma_{ab\dot{\alpha}\dot{\gamma}}\gamma_{cd}{}^{\dot{\gamma}}{}_{\dot{\beta}}\nabla_e\Lambda_{\alpha l}\epsilon^{ijkl} + (\frac{1}{10}\mathcal{D}^\dagger\bar{\mathcal{H}} + \frac{1}{5}\mathcal{D}\bar{\mathcal{L}})iT_{cd}{}^{jk}\Lambda^{\dot{\alpha}i}R(Q)_{ce}{}^{\dot{\beta}}{}_{k\epsilon\dot{\alpha}\dot{\beta}}\gamma_{de\alpha\beta}\gamma_{ab}{}^{\alpha\beta} \\
& + (-\frac{1}{12}\mathcal{D}^\dagger\mathcal{D}^\dagger\bar{\mathcal{H}} + \frac{1}{15}\bar{\mathcal{L}})iT_{cdkl}\Lambda^{\dot{\alpha}i}\chi^{\dot{\beta}}{}_{mn}{}^j\gamma_{ab\dot{\alpha}\dot{\gamma}}\gamma_{cd}{}^{\dot{\gamma}}{}_{\dot{\beta}}\epsilon^{klmn} + (\frac{1}{9}\mathcal{H} - \frac{1}{9}\bar{\mathcal{H}})iE^{ik}\Lambda_{\alpha k}\Lambda^{\dot{\alpha}j}\bar{P}_c\gamma_c{}^{\dot{\beta}\alpha}\gamma_{ab\dot{\alpha}\dot{\beta}} \\
& + (\frac{1}{6}\mathcal{D}^\dagger\bar{\mathcal{H}} + \frac{7}{18}\mathcal{D}\bar{\mathcal{L}})iT_{cdkl}\Lambda^{\dot{\alpha}j}\gamma_c{}^{\dot{\beta}\alpha}\gamma_{ab\dot{\alpha}\dot{\beta}}\nabla_d\Lambda_{\alpha m}\epsilon^{iklm} + (\frac{1}{6}\mathcal{D}^\dagger\bar{\mathcal{H}} + \frac{1}{3}\mathcal{D}\bar{\mathcal{L}})i\Lambda^{\dot{\alpha}j}\bar{P}_c\gamma_{c\alpha\dot{\beta}}\gamma_{d\dot{\beta}\dot{\alpha}}\gamma_{ab}{}^{\alpha\beta}\nabla_d\Lambda^{\dot{\beta}i} \\
& + (\frac{1}{6}\mathcal{D}^\dagger\bar{\mathcal{H}} - \frac{1}{15}\mathcal{D}\bar{\mathcal{L}})i\Lambda_{\alpha k}\Lambda^{\dot{\alpha}j}\gamma_c{}^{\dot{\beta}\alpha}\gamma_{ab\dot{\alpha}\dot{\beta}}\nabla_dT_{cdlm}\epsilon^{iklm} + (-\frac{1}{2}\mathcal{D}^\dagger\mathcal{D}^\dagger\bar{\mathcal{H}} - \frac{4}{3}\bar{\mathcal{L}})iE^{ik}P_c\Lambda_{\alpha k}\Lambda^{\dot{\alpha}j}\gamma_{c\beta\dot{\alpha}}\gamma_{ab}{}^{\alpha\beta} \\
& + (\frac{1}{6}\mathcal{D}^\dagger\mathcal{D}^\dagger\bar{\mathcal{H}} + \frac{4}{3}\bar{\mathcal{L}})iT_{cdkl}\Lambda^{\dot{\alpha}i}R(Q)_{ce}{}^{\dot{\beta}}{}_{m\gamma_{ab\dot{\beta}\dot{\gamma}}\gamma_{de}{}^{\dot{\gamma}}{}_{\dot{\alpha}}\epsilon^{jklm}} + (-\frac{7}{6}\mathcal{D}\mathcal{D}\mathcal{H} - \frac{10}{3}\mathcal{I})iT_{cd}{}^{ik}T_{ce}{}^{jl}\Lambda_{\alpha k}\Lambda_{\beta l}\gamma_{de\gamma}{}^{\alpha}\gamma_{ab}{}^{\beta\gamma} \\
& + (-\frac{1}{6}\mathcal{D}^\dagger\mathcal{D}^\dagger\bar{\mathcal{H}} + \frac{1}{15}\bar{\mathcal{L}})iT_{cdkl}\Lambda^{\dot{\alpha}m}\chi^{\dot{\beta}}{}_{mn}{}^i\gamma_{ab\dot{\alpha}\dot{\gamma}}\gamma_{cd}{}^{\dot{\gamma}}{}_{\dot{\beta}}\epsilon^{jklm} + (\frac{8}{15}\mathcal{D}\mathcal{D}\mathcal{H} - \frac{8}{15}\mathcal{I})iT_{cd}{}^{ij}T_{ce}{}^{kl}\Lambda_{\alpha k}\Lambda_{\beta l}\gamma_{de\gamma}{}^{\alpha}\gamma_{ab}{}^{\beta\gamma} \\
& + (-\frac{1}{9}\mathcal{H} - \frac{1}{3}\bar{\mathcal{H}})iE^{jk}\Lambda_{\alpha k}\Lambda^{\dot{\alpha}i}\bar{P}_c\gamma_{c\beta\dot{\alpha}}\gamma_{ab}{}^{\alpha\beta} + (\frac{1}{2}\mathcal{D}^\dagger\bar{\mathcal{H}} + \frac{5}{3}\mathcal{D}\bar{\mathcal{L}})i\Lambda_{\alpha k}\Lambda^{\dot{\alpha}i}\gamma_{c\beta\dot{\alpha}}\gamma_{ab}{}^{\alpha\beta}\nabla_dT_{cdlm}\epsilon^{jklm} \\
& + (\frac{1}{2}\mathcal{D}^\dagger\bar{\mathcal{H}} + \mathcal{D}\bar{\mathcal{L}})iT_{cdkl}\Lambda^{\dot{\alpha}j}\gamma_{c\alpha\dot{\gamma}}\gamma_{ab}{}^{\alpha\beta}\nabla_d\Lambda_{\beta m}\epsilon^{iklm} + (\frac{1}{2}\mathcal{D}^\dagger\bar{\mathcal{H}} + \mathcal{D}\bar{\mathcal{L}})iT_{cdkl}\Lambda^{\dot{\alpha}m}\gamma_{c\alpha\dot{\gamma}}\gamma_{ab}{}^{\alpha\beta}\nabla_d\Lambda_{\beta m}\epsilon^{ijkl} \\
& + (\frac{1}{2}\mathcal{D}^\dagger\bar{\mathcal{H}} + \frac{1}{3}\mathcal{D}\bar{\mathcal{L}})iT_{cd}{}^{ij}T_{cd}{}^{kl}\Lambda^{\dot{\alpha}m}\Lambda^{\dot{\beta}n}\gamma_{ab\dot{\alpha}\dot{\beta}}\epsilon_{klmn} + (\frac{5}{6}\mathcal{D}^\dagger\bar{\mathcal{H}} + \frac{5}{3}\mathcal{D}\bar{\mathcal{L}})i\Lambda^{\dot{\alpha}j}\bar{P}_c\gamma_{c\alpha\dot{\gamma}}\gamma_{d\dot{\beta}\dot{\gamma}}\gamma_{ab}{}^{\alpha\beta}\nabla_d\Lambda^{\dot{\beta}i} \\
& + (2\mathcal{D}^\dagger\bar{\mathcal{H}} + \frac{4}{3}\mathcal{D}\bar{\mathcal{L}})iP_cT_{cd}{}^{ij}\Lambda_{\alpha k}\Lambda^{\dot{\alpha}k}\gamma_d{}^{\dot{\beta}\alpha}\gamma_{ab\dot{\alpha}\dot{\beta}} + \frac{1}{16}iE_{kl}E_{mn}\mathcal{D}\mathcal{D}\mathcal{H}\Lambda_{\alpha p}\Lambda_{\beta q}\gamma_{ab}{}^{\alpha\beta}\epsilon^{ijkm}\epsilon^{lnpq} \\
& + \frac{1}{3}i\mathcal{H}P_c\Lambda_{\alpha k}\gamma_{d\beta\dot{\alpha}}\gamma_c{}^{\dot{\alpha}\gamma}\gamma_{ab}{}^{\alpha\beta}\nabla_d\Lambda_{\gamma l}\epsilon^{ijkl} + i\mathcal{H}P_c\Lambda_{\alpha k}\gamma_{c\beta}{}^{\dot{\alpha}}\gamma_d{}^{\dot{\alpha}}{}_{\dot{\alpha}}\gamma_{ab}{}^{\beta\gamma}\nabla_d\Lambda_{\gamma l}\epsilon^{ijkl} - \frac{1}{10}i\mathcal{H}T_{cdkl}T_{cdmn}\Lambda_{\alpha p}\Lambda_{\beta q}\gamma_{ab}{}^{\alpha\beta}\epsilon^{ijkm}\epsilon^{lnpq} \\
& + \frac{1}{3}i\mathcal{H}\Lambda_{\alpha k}\Lambda_{\beta l}\gamma_{c\gamma\dot{\alpha}}\gamma_d{}^{\dot{\alpha}\alpha}\gamma_{ab}{}^{\beta\gamma}\nabla_cP_d\epsilon^{ijkl} + \frac{2}{9$$

$$\begin{aligned}
[\mathcal{E}_{ab}^{ij}]_{2,cont} = & -\frac{1}{6}i\mathcal{D}^\dagger\mathcal{I}\Lambda_{\alpha k}R(Q)_{cd}{}^{\dot{\alpha}}{}_l\bar{P}_e\gamma_e{}^{\dot{\beta}\alpha}\gamma_{ab\dot{\alpha}\dot{\gamma}}\gamma_{cd}{}^{\dot{\gamma}}{}_{\dot{\beta}}\varepsilon^{ijkl} + \frac{1}{6}i\mathcal{D}^\dagger\mathcal{I}\Lambda_{\alpha k}\epsilon^{\alpha\beta}\gamma_c{}^{\dot{\alpha}\gamma}\gamma_{d\dot{\gamma}}{}^{\dot{\beta}}\gamma_{ab\dot{\alpha}\dot{\beta}}\nabla_d\nabla_c\Lambda_{\beta l}\varepsilon^{ijkl} \\
& -\frac{1}{15}i\mathcal{D}\bar{\mathcal{I}}\Lambda_{\alpha k}\Lambda^{\dot{\alpha}i}\gamma_c{}^{\alpha}{}_{\dot{\alpha}}\gamma_{ab\dot{\beta}\dot{\gamma}}\gamma_{de}{}^{\dot{\beta}\dot{\gamma}}\nabla_cT_{delm}\varepsilon^{ijklm} + \frac{1}{15}i\mathcal{D}\bar{\mathcal{I}}\Lambda_{\alpha k}\Lambda^{\dot{\alpha}j}\gamma_c{}^{\alpha}{}_{\dot{\alpha}}\gamma_{ab\dot{\beta}\dot{\gamma}}\gamma_{de}{}^{\dot{\beta}\dot{\gamma}}\nabla_cT_{delm}\varepsilon^{iklm} \\
& -\frac{1}{30}i\mathcal{D}\bar{\mathcal{I}}\Lambda_{\alpha k}\Lambda^{\dot{\alpha}k}\gamma_c{}^{\alpha}{}_{\dot{\alpha}}\gamma_{ab\dot{\beta}\dot{\gamma}}\gamma_{de}{}^{\dot{\beta}\dot{\gamma}}\nabla_cT_{delm}\varepsilon^{ijlm} - \frac{1}{10}i\mathcal{D}\bar{\mathcal{I}}\Lambda_{\alpha k}\Lambda^{\dot{\alpha}i}\gamma_c{}^{\beta\alpha}{}_{\dot{\alpha}}\gamma_{ab\dot{\beta}\dot{\gamma}}\gamma_{de}{}^{\dot{\gamma}}{}_{\dot{\beta}}\nabla_cT_{delm}\varepsilon^{ijklm} \\
& + \frac{1}{10}i\mathcal{D}\bar{\mathcal{I}}\Lambda_{\alpha k}\Lambda^{\dot{\alpha}j}\gamma_c{}^{\beta\alpha}{}_{\dot{\alpha}}\gamma_{ab\dot{\beta}\dot{\gamma}}\gamma_{de}{}^{\dot{\gamma}}{}_{\dot{\beta}}\nabla_cT_{delm}\varepsilon^{iklm} + \frac{1}{30}i\mathcal{D}\bar{\mathcal{I}}\Lambda_{\alpha k}\Lambda^{\dot{\alpha}k}\gamma_c{}^{\beta\alpha}{}_{\dot{\alpha}}\gamma_{ab\dot{\beta}\dot{\gamma}}\gamma_{de}{}^{\dot{\gamma}}{}_{\dot{\beta}}\nabla_cT_{delm}\varepsilon^{ijlm} \\
& + \frac{1}{5}i\mathcal{D}\bar{\mathcal{I}}\Lambda^{\dot{\alpha}i}\Lambda^{\dot{\beta}j}\epsilon_{\dot{\alpha}\dot{\beta}}\gamma_{c\alpha}{}^{\dot{\gamma}}\gamma_d{}^{\dot{\delta}\alpha}\gamma_{ab\dot{\gamma}\dot{\delta}}\nabla_d\bar{P}_c - 2i\mathcal{D}^\dagger\mathcal{D}^\dagger\bar{\mathcal{I}}P_cP_d\Lambda^{\dot{\alpha}i}\Lambda^{\dot{\beta}j}\gamma_{c\alpha\dot{\alpha}}\gamma_{d\beta\dot{\beta}}\gamma_{ab}{}^{\alpha\beta} \\
& + (-\frac{1}{3}\mathcal{D}^\dagger\mathcal{I} + \frac{1}{6}\mathcal{D}\mathcal{H})iT_{cd}{}^{ij}\Lambda^{\dot{\alpha}k}\Lambda_{\alpha k}\bar{P}_e\gamma_e{}^{\alpha}{}_{\dot{\alpha}}\gamma_{cd\beta\dot{\gamma}}\gamma_{ab}{}^{\beta\gamma} + (-\frac{1}{3}\mathcal{D}^\dagger\mathcal{I} + \frac{1}{6}\mathcal{D}\mathcal{H})iT_{cd}{}^{jk}\Lambda^{\dot{\alpha}i}\Lambda_{\alpha k}\bar{P}_e\gamma_e{}^{\alpha}{}_{\dot{\alpha}}\gamma_{cd\beta\dot{\gamma}}\gamma_{ab}{}^{\beta\gamma} \\
& -\frac{3}{5}i\bar{\mathcal{I}}T_{cdkl}\Lambda^{\dot{\alpha}i}\chi^{\dot{\beta}}{}_{mn}{}^j\epsilon_{\dot{\alpha}\dot{\beta}}\gamma_{ab\dot{\gamma}\dot{\delta}}\gamma_{cd}{}^{\dot{\gamma}\dot{\delta}}\varepsilon^{klmn} - \frac{3}{5}i\bar{\mathcal{I}}T_{cdkl}\Lambda^{\dot{\alpha}m}\chi^{\dot{\beta}}{}_{mn}{}^i\epsilon_{\dot{\alpha}\dot{\beta}}\gamma_{ab\dot{\gamma}\dot{\delta}}\gamma_{cd}{}^{\dot{\gamma}\dot{\delta}}\varepsilon^{jklm} + \frac{1}{8}i\mathcal{D}^\dagger\mathcal{D}^\dagger\bar{\mathcal{H}}T_{cdkl}T_{ef}{}^{ik}\Lambda^{\dot{\alpha}j}\Lambda^{\dot{\beta}l}\gamma_{ef\alpha\beta}\gamma_{ab}{}^{\alpha\beta}\gamma_{cd\dot{\alpha}\dot{\beta}} \\
& + (\frac{1}{4}\mathcal{D}\mathcal{D}\mathcal{H} + \frac{1}{2}\mathcal{I})iT_{cd}{}^{ik}T_{ef}{}^{jl}\Lambda_{\alpha k}\Lambda_{\beta l}\gamma_{cd\gamma\delta}\gamma_{ab}{}^{\gamma\delta}\gamma_{ef}{}^{\alpha\beta} + (\frac{1}{4}\mathcal{D}\mathcal{D}\mathcal{H} + \frac{1}{2}\mathcal{I})iT_{cd}{}^{ik}T_{ef}{}^{jl}\Lambda_{\alpha k}\Lambda_{\beta l}\gamma_{ef\gamma\delta}\gamma_{ab}{}^{\gamma\delta}\gamma_{cd}{}^{\alpha\beta} \\
& + (\frac{1}{5}\mathcal{D}\mathcal{D}\mathcal{H} + \frac{2}{5}\mathcal{I})iE_{kl}T_{cd}{}^{km}\Lambda_{\alpha m}\Lambda_{\beta n}\gamma_{cd\gamma}{}^{\alpha}\gamma_{ab}{}^{\beta\gamma}\varepsilon^{ijln} + \frac{3}{10}i\mathcal{D}^\dagger\bar{\mathcal{I}}E^{ik}T_{cdkl}\Lambda^{\dot{\alpha}j}\Lambda^{\dot{\beta}l}\epsilon_{\dot{\alpha}\dot{\beta}}\gamma_{ab\dot{\gamma}\dot{\delta}}\gamma_{cd}{}^{\dot{\gamma}\dot{\delta}} \\
& + (\frac{1}{9}\mathcal{D}^\dagger\mathcal{D}^\dagger\bar{\mathcal{H}} + \frac{4}{9}\bar{\mathcal{I}})iP_cT_{cdkl}\Lambda_{\alpha m}\Lambda^{\dot{\alpha}i}\gamma_d{}^{\beta\alpha}{}_{\dot{\alpha}}\gamma_{ab\dot{\beta}\dot{\gamma}}\varepsilon^{ijklm} + (\frac{1}{9}\mathcal{D}^\dagger\mathcal{I} - \frac{1}{2}\mathcal{D}\mathcal{H})iE_{kl}\Lambda_{\alpha m}\Lambda^{\dot{\alpha}k}\bar{P}_c\gamma_c{}^{\beta\alpha}{}_{\dot{\alpha}}\gamma_{ab\dot{\beta}\dot{\gamma}}\varepsilon^{ijlm} \\
& + (\frac{1}{8}\mathcal{D}^\dagger\mathcal{I} - \frac{1}{16}\mathcal{D}\mathcal{H})i\Lambda_{\alpha k}\Lambda_{\beta l}R(M)_{cdef}\gamma_{cd\gamma\delta}\gamma_{ab}{}^{\gamma\delta}\gamma_{ef}{}^{\alpha\beta}\varepsilon^{ijkl} - \frac{3}{10}i\mathcal{D}^\dagger\bar{\mathcal{I}}E^{jk}T_{cdkl}\Lambda^{\dot{\alpha}i}\Lambda^{\dot{\beta}l}\epsilon_{\dot{\alpha}\dot{\beta}}\gamma_{ab\dot{\gamma}\dot{\delta}}\gamma_{cd}{}^{\dot{\gamma}\dot{\delta}} \\
& - \frac{1}{8}i\mathcal{D}^\dagger\mathcal{D}^\dagger\bar{\mathcal{H}}T_{cdkl}T_{ef}{}^{jk}\Lambda^{\dot{\alpha}i}\Lambda^{\dot{\beta}l}\gamma_{ef\alpha\beta}\gamma_{ab}{}^{\alpha\beta}\gamma_{cd\dot{\alpha}\dot{\beta}} - \frac{1}{8}i\mathcal{D}^\dagger\mathcal{D}^\dagger\bar{\mathcal{H}}T_{cdkl}T_{ef}{}^{kl}\Lambda^{\dot{\alpha}i}\Lambda^{\dot{\beta}j}\gamma_{ef\alpha\beta}\gamma_{ab}{}^{\alpha\beta}\gamma_{cd\dot{\alpha}\dot{\beta}} \\
& + \frac{3}{5}i\bar{\mathcal{I}}T_{cdkl}\Lambda^{\dot{\alpha}j}\chi^{\dot{\beta}}{}_{mn}{}^i\epsilon_{\dot{\alpha}\dot{\beta}}\gamma_{ab\dot{\gamma}\dot{\delta}}\gamma_{cd}{}^{\dot{\gamma}\dot{\delta}}\varepsilon^{klmn} + \frac{3}{5}i\bar{\mathcal{I}}T_{cdkl}\Lambda^{\dot{\alpha}m}\chi^{\dot{\beta}}{}_{mn}{}^j\epsilon_{\dot{\alpha}\dot{\beta}}\gamma_{ab\dot{\gamma}\dot{\delta}}\gamma_{cd}{}^{\dot{\gamma}\dot{\delta}}\varepsilon^{ikln} \\
& + (\frac{1}{3}\mathcal{D}^\dagger\mathcal{I} - \frac{1}{6}\mathcal{D}\mathcal{H})iE_{kl}\Lambda_{\alpha m}\Lambda^{\dot{\alpha}k}\bar{P}_c\gamma_{c\beta\dot{\alpha}}\gamma_{ab}{}^{\alpha\beta}\varepsilon^{ijlm} + (\frac{1}{3}\mathcal{D}^\dagger\mathcal{I} - \frac{1}{6}\mathcal{D}\mathcal{H})iP_c\Lambda_{\alpha k}\Lambda_{\beta l}\bar{P}_d\gamma_{cd\gamma}{}^{\alpha}\gamma_{ab}{}^{\beta\gamma}\varepsilon^{ijkl} \\
& + (\frac{1}{3}\mathcal{D}^\dagger\mathcal{I} - \frac{1}{6}\mathcal{D}\mathcal{H})iT_{cd}{}^{ik}\Lambda^{\dot{\alpha}j}\Lambda_{\alpha k}\bar{P}_e\gamma_e{}^{\alpha}{}_{\dot{\alpha}}\gamma_{cd\beta\dot{\gamma}}\gamma_{ab}{}^{\beta\gamma} + \frac{16}{3}i\bar{\mathcal{I}}P_c\Lambda^{\dot{\alpha}i}\Lambda^{\dot{\beta}j}\bar{P}_d\gamma_{c\alpha\dot{\alpha}}\gamma_{d\beta\dot{\beta}}\gamma_{ab}{}^{\alpha\beta} + \frac{16}{3}i\bar{\mathcal{I}}P_c\Lambda^{\dot{\alpha}i}\Lambda^{\dot{\beta}j}\bar{P}_d\gamma_{c\alpha\dot{\alpha}}\gamma_{d\beta\dot{\beta}}\gamma_{ab}{}^{\alpha\beta} \\
& + (-\frac{2}{3}\mathcal{D}^\dagger\mathcal{D}^\dagger\bar{\mathcal{H}} - \frac{28}{3}\bar{\mathcal{I}})iP_cT_{cdkl}\Lambda_{\alpha m}\Lambda^{\dot{\alpha}m}\gamma_{d\beta\dot{\alpha}}\gamma_{ab}{}^{\alpha\beta}\varepsilon^{ijkl} + (-\frac{1}{3}\mathcal{H} + \frac{4}{3}\bar{\mathcal{H}})iT_{cdkl}\Lambda_{\alpha m}\Lambda^{\dot{\alpha}m}\bar{P}_c\gamma_{d\beta\dot{\alpha}}\gamma_{ab}{}^{\alpha\beta}\varepsilon^{ijkl} \\
& + (\frac{1}{3}\mathcal{H} + \frac{2}{3}\bar{\mathcal{H}})iT_{cdkl}\Lambda_{\alpha m}\Lambda^{\dot{\alpha}j}\bar{P}_c\gamma_{d\beta\dot{\alpha}}\gamma_{ab}{}^{\alpha\beta}\varepsilon^{iklm} + (-\frac{5}{9}\mathcal{H} + \frac{5}{9}\bar{\mathcal{H}})iP_c\Lambda_{\alpha k}\gamma_c{}^{\dot{\alpha}\alpha}{}_{\dot{\alpha}}\gamma_d{}^{\dot{\beta}\beta}{}_{\dot{\beta}}\gamma_{ab\dot{\alpha}\dot{\beta}}\nabla_d\Lambda_{\beta l}\varepsilon^{ijkl} \\
& + (-\frac{1}{2}\mathcal{D}^\dagger\bar{\mathcal{H}} - \mathcal{D}\bar{\mathcal{I}})i\Lambda^{\dot{\alpha}j}\bar{P}_c\epsilon_{\dot{\alpha}\dot{\beta}}\gamma_{d\alpha\dot{\gamma}}\gamma_{c\beta}{}^{\dot{\gamma}}\gamma_{ab}{}^{\alpha\beta}\nabla_d\Lambda^{\dot{\beta}i} + (-\frac{3}{10}\mathcal{H} + \frac{7}{20}\bar{\mathcal{H}})iT_{cdkl}T_{cdmn}\Lambda_{\alpha p}\Lambda_{\beta q}\gamma_{ab}{}^{\alpha\beta}\varepsilon^{ijmp}\varepsilon^{klmq} \\
& + (\frac{2}{3}\mathcal{H} + \frac{1}{3}\bar{\mathcal{H}})iT_{cdkl}\Lambda_{\alpha m}\chi_{\beta}{}^{ij}{}_n\epsilon^{\alpha\beta}\gamma_{ab\dot{\alpha}\dot{\beta}}\gamma_{cd}{}^{\dot{\alpha}\dot{\beta}}\varepsilon^{klmn} + (-\frac{1}{3}\mathcal{D}^\dagger\bar{\mathcal{H}} - \frac{2}{3}\mathcal{D}\bar{\mathcal{I}})iP_cT_{de}{}^{ij}\Lambda^{\dot{\alpha}k}\Lambda_{\alpha k}\gamma_c{}^{\alpha}{}_{\dot{\alpha}}\gamma_{de\beta\dot{\gamma}}\gamma_{ab}{}^{\beta\gamma} \\
& + (-\frac{1}{3}\mathcal{D}^\dagger\mathcal{D}^\dagger\bar{\mathcal{H}} - \frac{8}{3}\bar{\mathcal{I}})iP_cT_{cdkl}\Lambda_{\alpha m}\Lambda^{\dot{\alpha}j}\gamma_{d\beta\dot{\alpha}}\gamma_{ab}{}^{\alpha\beta}\varepsilon^{iklm} + (\frac{1}{3}\mathcal{D}\mathcal{D}\mathcal{H} + \frac{8}{3}\mathcal{I})i\Lambda_{\alpha k}\bar{P}_c\gamma_c{}^{\dot{\alpha}\alpha}{}_{\dot{\alpha}}\gamma_d{}^{\dot{\beta}\beta}{}_{\dot{\beta}}\gamma_{ab\dot{\alpha}\dot{\beta}}\nabla_d\Lambda_{\beta l}\varepsilon^{ijkl} \\
& + (\frac{1}{3}\mathcal{D}\mathcal{D}\mathcal{H} + \frac{8}{3}\mathcal{I})i\Lambda_{\alpha k}\bar{P}_c\gamma_c{}^{\dot{\alpha}\beta}{}_{\dot{\alpha}}\gamma_d{}^{\dot{\beta}\alpha}{}_{\dot{\beta}}\gamma_{ab\dot{\alpha}\dot{\beta}}\nabla_d\Lambda_{\beta l}\varepsilon^{ijkl} + (-\frac{14}{45}\mathcal{D}^\dagger\mathcal{D}^\dagger\bar{\mathcal{H}} - \frac{112}{45}\bar{\mathcal{I}})iP_c\Lambda^{\dot{\alpha}i}\Lambda^{\dot{\beta}j}\bar{P}_d\gamma_{d\alpha}{}^{\dot{\gamma}}\gamma_c{}^{\alpha}{}_{\dot{\alpha}}\gamma_{ab\dot{\beta}\dot{\gamma}} \\
& + (-\frac{2}{9}\mathcal{H} + \frac{2}{9}\bar{\mathcal{H}})i\Lambda^{\dot{\alpha}i}\Lambda^{\dot{\beta}j}\bar{P}_c\bar{P}_d\gamma_{c\alpha}{}^{\dot{\gamma}}\gamma_d{}^{\alpha}{}_{\dot{\alpha}}\gamma_{ab\dot{\beta}\dot{\gamma}} + (-\frac{2}{9}\mathcal{H} + \frac{2}{9}\bar{\mathcal{H}})i\Lambda^{\dot{\alpha}i}\Lambda^{\dot{\beta}j}\bar{P}_c\bar{P}_d\gamma_{c\alpha}{}^{\dot{\gamma}}\gamma_d{}^{\alpha}{}_{\dot{\alpha}}\gamma_{ab\dot{\beta}\dot{\gamma}} \\
& + (-\frac{6}{5}\mathcal{H} + \frac{1}{5}\bar{\mathcal{H}})iT_{cdkl}\Lambda_{\alpha m}\Lambda^{\dot{\alpha}m}\bar{P}_c\gamma_d{}^{\dot{\beta}\alpha}{}_{\dot{\beta}}\gamma_{ab\dot{\alpha}\dot{\beta}}\varepsilon^{ijkl} + (-\frac{1}{5}\mathcal{D}^\dagger\mathcal{D}^\dagger\bar{\mathcal{H}} - \frac{8}{5}\bar{\mathcal{I}})iP_c\Lambda^{\dot{\alpha}i}\Lambda^{\dot{\beta}j}\bar{P}_d\gamma_{d\alpha\dot{\beta}}\gamma_c{}^{\dot{\gamma}\alpha}{}_{\dot{\beta}}\gamma_{ab\dot{\alpha}\dot{\gamma}} \\
& + (\frac{1}{3}\mathcal{H} + \frac{1}{6}\bar{\mathcal{H}})iT_{cdkl}\Lambda_{\alpha m}\chi_{\beta}{}^{jm}{}_n\epsilon^{\alpha\beta}\gamma_{ab\dot{\alpha}\dot{\beta}}\gamma_{cd}{}^{\dot{\alpha}\dot{\beta}}\varepsilon^{ikln} + (-\frac{1}{6}\mathcal{D}^\dagger\bar{\mathcal{H}} - \frac{1}{3}\mathcal{D}\bar{\mathcal{I}})iE_{kl}P_c\Lambda_{\alpha m}\Lambda^{\dot{\alpha}k}\gamma_{c\beta\dot{\alpha}}\gamma_{ab}{}^{\alpha\beta}\varepsilon^{ijlm} \\
& + (\frac{1}{6}\mathcal{D}\mathcal{D}\mathcal{H} + \frac{4}{3}\mathcal{I})i\Lambda_{\alpha k}\Lambda_{\beta l}\gamma_c{}^{\dot{\alpha}\alpha}{}_{\dot{\alpha}}\gamma_d{}^{\dot{\beta}\beta}{}_{\dot{\beta}}\gamma_{ab\dot{\alpha}\dot{\beta}}\nabla_c\bar{P}_d\varepsilon^{ijkl} + (-\frac{1}{9}\mathcal{H} + \frac{1}{9}\bar{\mathcal{H}})iP_c\Lambda_{\alpha k}\gamma_c{}^{\dot{\alpha}\beta}{}_{\dot{\alpha}}\gamma_d{}^{\dot{\beta}\alpha}{}_{\dot{\beta}}\gamma_{ab\dot{\alpha}\dot{\beta}}\nabla_d\Lambda_{\beta l}\varepsilon^{ijkl} \\
& + (-\frac{1}{9}\mathcal{H} + \frac{1}{9}\bar{\mathcal{H}})i\Lambda_{\alpha k}\Lambda_{\beta l}\gamma_c{}^{\dot{\alpha}\alpha}{}_{\dot{\alpha}}\gamma_d{}^{\dot{\beta}\beta}{}_{\dot{\beta}}\gamma_{ab\dot{\alpha}\dot{\beta}}\nabla_cP_d\varepsilon^{ijkl} + (-\frac{1}{10}\mathcal{H} + \frac{1}{10}\bar{\mathcal{H}})iT_{cdkl}\Lambda_{\alpha m}R(Q)_{ce\beta}{}^m\epsilon^{\alpha\beta}\gamma_{ab\dot{\alpha}\dot{\beta}}\gamma_{de}{}^{\dot{\alpha}\dot{\beta}}\varepsilon^{ijkl} \\
& + (-\frac{19}{90}\mathcal{D}^\dagger\mathcal{D}^\dagger\bar{\mathcal{H}} - \frac{56}{45}\bar{\mathcal{I}})iP_cT_{cdkl}\Lambda_{\alpha m}\Lambda^{\dot{\alpha}j}\gamma_d{}^{\dot{\beta}\alpha}{}_{\dot{\beta}}\gamma_{ab\dot{\alpha}\dot{\beta}}\varepsilon^{iklm} + (\frac{7}{30}\mathcal{D}^\dagger\mathcal{D}^\dagger\bar{\mathcal{H}} + \frac{8}{15}\bar{\mathcal{I}})iP_cT_{cdkl}\Lambda_{\alpha m}\Lambda^{\dot{\alpha}m}\gamma_d{}^{\dot{\beta}\alpha}{}_{\dot{\beta}}\gamma_{ab\dot{\alpha}\dot{\beta}}\varepsilon^{ijkl} \\
& + (-\frac{2}{5}\mathcal{H} + \frac{1}{15}\bar{\mathcal{H}})iT_{cdkl}\Lambda_{\alpha m}\Lambda^{\dot{\alpha}i}\bar{P}_c\gamma_d{}^{\dot{\beta}\alpha}{}_{\dot{\beta}}\gamma_{ab\dot{\alpha}\dot{\beta}}\varepsilon^{ijklm} + (-\frac{7}{30}\mathcal{D}\mathcal{D}\mathcal{H} - \frac{1}{15}\mathcal{I})iE_{kl}T_{cd}{}^{km}\Lambda_{\alpha m}\Lambda_{\beta n}\gamma_{cd\gamma}{}^{\beta}\gamma_{ab}{}^{\alpha\gamma}\varepsilon^{ijln} \\
& + (-\frac{1}{10}\mathcal{D}\mathcal{D}\mathcal{H} + \frac{1}{10}\mathcal{I})iT_{cd}{}^{ij}T_{ef}{}^{kl}\Lambda_{\alpha k}\Lambda_{\beta l}\gamma_{ef\gamma\delta}\gamma_{ab}{}^{\gamma\delta}\gamma_{cd}{}^{\alpha\beta} + (\frac{1}{36}\mathcal{D}^\dagger\mathcal{D}^\dagger\bar{\mathcal{H}} - \frac{1}{36}\bar{\mathcal{I}})iE_{kl}T_{cdmn}\Lambda^{\dot{\alpha}i}\Lambda^{\dot{\beta}k}\gamma_{ab\dot{\beta}\dot{\gamma}}\gamma_{cd}{}^{\dot{\gamma}}{}_{\dot{\alpha}}\varepsilon^{jlmn} + 5\cdots
\end{aligned}$$

$$\begin{aligned}
[\mathcal{E}_{ab}{}^{ij}]_{2,cont} = & +(-\frac{1}{30}\mathcal{H} + \frac{1}{30}\bar{\mathcal{H}})iT_{cdkl}\Lambda_{\alpha m}R(Q)_{ce\beta}{}^j\epsilon^{\alpha\beta}\gamma_{ab\dot{\alpha}\dot{\beta}}\gamma_{de}{}^{\dot{\alpha}\dot{\beta}}\epsilon^{ijklm} + (-\frac{1}{96}\mathcal{D}^\dagger\mathcal{D}^\dagger\mathcal{D}^\dagger\bar{\mathcal{H}} + \frac{1}{12}\mathcal{D}^\dagger\bar{\mathcal{I}})iT_{cdkl}T_{cemn}\Lambda^{\dot{\alpha}i}\Lambda^{\dot{\beta}m}\gamma_{ab\dot{\alpha}\dot{\gamma}}\gamma_{de}{}^{\dot{\gamma}}\epsilon^{ilmn} \\
& + (-\frac{1}{96}\mathcal{D}^\dagger\mathcal{D}^\dagger\mathcal{D}^\dagger\bar{\mathcal{H}} + \frac{1}{12}\mathcal{D}^\dagger\bar{\mathcal{I}})iT_{cdkl}T_{cemn}\Lambda^{\dot{\alpha}j}\Lambda^{\dot{\beta}k}\gamma_{ab\dot{\alpha}\dot{\gamma}}\gamma_{de}{}^{\dot{\gamma}}\epsilon^{ilmn} + (\frac{1}{36}\mathcal{D}^\dagger\mathcal{D}^\dagger\bar{\mathcal{H}} + \frac{1}{18}\bar{\mathcal{I}})iE_{kl}T_{cdmn}\Lambda^{\dot{\alpha}k}\Lambda^{\dot{\beta}l}\gamma_{ab\dot{\alpha}\dot{\gamma}}\gamma_{cd}{}^{\dot{\gamma}}\epsilon^{ijmn} \\
& + (\frac{5}{96}\mathcal{D}^\dagger\mathcal{D}^\dagger\mathcal{D}^\dagger\bar{\mathcal{H}} + \frac{1}{4}\mathcal{D}^\dagger\bar{\mathcal{I}})iT_{cdkl}T_{cemn}\Lambda^{\dot{\alpha}i}\Lambda^{\dot{\beta}k}\gamma_{ab\dot{\beta}\dot{\gamma}}\gamma_{de}{}^{\dot{\gamma}}\epsilon^{jlmn} + (\frac{5}{96}\mathcal{D}^\dagger\mathcal{D}^\dagger\mathcal{D}^\dagger\bar{\mathcal{H}} + \frac{1}{4}\mathcal{D}^\dagger\bar{\mathcal{I}})iT_{cdkl}T_{cemn}\Lambda^{\dot{\alpha}j}\Lambda^{\dot{\beta}m}\gamma_{ab\dot{\beta}\dot{\gamma}}\gamma_{de}{}^{\dot{\gamma}}\epsilon^{ikln} \\
& + (-\frac{23}{120}\mathcal{D}\mathcal{D}\mathcal{H} - \frac{1}{3}\mathcal{I})iE_{kl}T_{cd}{}^{jk}\Lambda_{\alpha m}\Lambda_{\beta n}\gamma_{cd\gamma}{}^{\alpha}\gamma_{ab}{}^{\beta\gamma}\epsilon^{ilmn} + (\frac{1}{36}\mathcal{D}^\dagger\mathcal{D}^\dagger\bar{\mathcal{H}} + \frac{1}{12}\bar{\mathcal{I}})iE_{kl}T_{cdmn}\Lambda^{\dot{\alpha}i}\Lambda^{\dot{\beta}k}\gamma_{ab\dot{\alpha}\dot{\gamma}}\gamma_{cd}{}^{\dot{\gamma}}\epsilon^{jlmn} \\
& + (-\frac{7}{480}\mathcal{D}^\dagger\mathcal{D}^\dagger\mathcal{D}^\dagger\bar{\mathcal{H}} - \frac{1}{20}\mathcal{D}^\dagger\bar{\mathcal{I}})iT_{cdkl}T_{cemn}\Lambda^{\dot{\alpha}k}\Lambda^{\dot{\beta}l}\gamma_{ab\dot{\alpha}\dot{\gamma}}\gamma_{de}{}^{\dot{\gamma}}\epsilon^{ijmn} \\
& + (\frac{7}{160}\mathcal{D}^\dagger\mathcal{D}^\dagger\mathcal{D}^\dagger\bar{\mathcal{H}} + \frac{3}{20}\mathcal{D}^\dagger\bar{\mathcal{I}})iT_{cdkl}T_{cemn}\Lambda^{\dot{\alpha}m}\Lambda^{\dot{\beta}n}\gamma_{ab\dot{\alpha}\dot{\gamma}}\gamma_{de}{}^{\dot{\gamma}}\epsilon^{ijkl} + (-\frac{1}{36}\mathcal{D}^\dagger\mathcal{D}^\dagger\bar{\mathcal{H}} - \frac{1}{12}\bar{\mathcal{I}})iE_{kl}T_{cdmn}\Lambda^{\dot{\alpha}j}\Lambda^{\dot{\beta}k}\gamma_{ab\dot{\alpha}\dot{\gamma}}\gamma_{cd}{}^{\dot{\gamma}}\epsilon^{ilmn} \\
& + (\frac{23}{120}\mathcal{D}\mathcal{D}\mathcal{H} + \frac{1}{3}\mathcal{I})iE_{kl}T_{cd}{}^{ik}\Lambda_{\alpha m}\Lambda_{\beta n}\gamma_{cd\gamma}{}^{\alpha}\gamma_{ab}{}^{\beta\gamma}\epsilon^{jlmn} + (-\frac{13}{120}\mathcal{D}\mathcal{D}\mathcal{H} - \frac{4}{15}\mathcal{I})iT_{cd}{}^{ij}T_{ef}{}^{kl}\Lambda_{\alpha k}\Lambda_{\beta l}\gamma_{cd\gamma\delta}\gamma_{ab}{}^{\gamma\delta}\gamma_{ef}{}^{\alpha\beta} \\
& + (-\frac{5}{96}\mathcal{D}^\dagger\mathcal{D}^\dagger\mathcal{D}^\dagger\bar{\mathcal{H}} - \frac{1}{4}\mathcal{D}^\dagger\bar{\mathcal{I}})iT_{cdkl}T_{cemn}\Lambda^{\dot{\alpha}i}\Lambda^{\dot{\beta}m}\gamma_{ab\dot{\beta}\dot{\gamma}}\gamma_{de}{}^{\dot{\gamma}}\epsilon^{jklm} + (-\frac{5}{96}\mathcal{D}^\dagger\mathcal{D}^\dagger\mathcal{D}^\dagger\bar{\mathcal{H}} - \frac{1}{4}\mathcal{D}^\dagger\bar{\mathcal{I}})iT_{cdkl}T_{cemn}\Lambda^{\dot{\alpha}j}\Lambda^{\dot{\beta}k}\gamma_{ab\dot{\beta}\dot{\gamma}}\gamma_{de}{}^{\dot{\gamma}}\epsilon^{ilmn} \\
& + (-\frac{2}{15}\mathcal{H} - \frac{1}{60}\bar{\mathcal{H}})iT_{cdkl}T_{cdmn}\Lambda_{\alpha p}\Lambda_{\beta q}\gamma_{ab}{}^{\alpha\beta}\epsilon^{ijkp}\epsilon^{lmnq} + (\frac{1}{96}\mathcal{D}^\dagger\mathcal{D}^\dagger\mathcal{D}^\dagger\bar{\mathcal{H}} - \frac{1}{12}\mathcal{D}^\dagger\bar{\mathcal{I}})iT_{cdkl}T_{cemn}\Lambda^{\dot{\alpha}i}\Lambda^{\dot{\beta}k}\gamma_{ab\dot{\alpha}\dot{\gamma}}\gamma_{de}{}^{\dot{\gamma}}\epsilon^{jlmn} \\
& + (\frac{1}{96}\mathcal{D}^\dagger\mathcal{D}^\dagger\mathcal{D}^\dagger\bar{\mathcal{H}} - \frac{1}{12}\mathcal{D}^\dagger\bar{\mathcal{I}})iT_{cdkl}T_{cemn}\Lambda^{\dot{\alpha}j}\Lambda^{\dot{\beta}m}\gamma_{ab\dot{\alpha}\dot{\gamma}}\gamma_{de}{}^{\dot{\gamma}}\epsilon^{ikln} + (\frac{1}{30}\mathcal{H} - \frac{1}{30}\bar{\mathcal{H}})iT_{cdkl}\Lambda_{\alpha m}R(Q)_{ce\beta}{}^j\epsilon^{\alpha\beta}\gamma_{ab\dot{\alpha}\dot{\beta}}\gamma_{de}{}^{\dot{\alpha}\dot{\beta}}\epsilon^{iklm} \\
& + (-\frac{1}{36}\mathcal{D}^\dagger\mathcal{D}^\dagger\bar{\mathcal{H}} + \frac{1}{36}\bar{\mathcal{I}})iE_{kl}T_{cdmn}\Lambda^{\dot{\alpha}j}\Lambda^{\dot{\beta}k}\gamma_{ab\dot{\beta}\dot{\gamma}}\gamma_{cd}{}^{\dot{\gamma}}\epsilon^{ilmn} + (\frac{2}{5}\mathcal{H} - \frac{1}{15}\bar{\mathcal{H}})iT_{cdkl}\Lambda_{\alpha m}\Lambda^{\dot{\alpha}j}\bar{P}_c\gamma_d{}^{\dot{\beta}\alpha}\gamma_{ab\dot{\alpha}\dot{\beta}}\epsilon^{iklm} \\
& + (\frac{1}{12}\mathcal{D}^\dagger\bar{\mathcal{H}} + \frac{1}{6}\mathcal{D}\bar{\mathcal{I}})iE_{kl}T_{cd}{}^{ij}\Lambda^{\dot{\alpha}k}\Lambda^{\dot{\beta}l}\epsilon_{\dot{\alpha}\dot{\beta}}\gamma_{cd\alpha\beta}\gamma_{ab}{}^{\alpha\beta} + (-\frac{1}{24}\mathcal{D}^\dagger\mathcal{D}^\dagger\bar{\mathcal{H}} + \frac{1}{6}\bar{\mathcal{I}})iT_{cdkl}T_{ef}{}^{ij}\Lambda^{\dot{\alpha}k}\Lambda^{\dot{\beta}l}\gamma_{ef\alpha\beta}\gamma_{ab}{}^{\alpha\beta}\gamma_{cd\dot{\alpha}\dot{\beta}} \\
& + (\frac{4}{45}\mathcal{D}^\dagger\mathcal{D}^\dagger\bar{\mathcal{H}} + \frac{32}{45}\bar{\mathcal{I}})iP_c\Lambda^{\dot{\alpha}i}\Lambda^{\dot{\beta}j}\bar{P}_d\gamma_{d\alpha}{}^{\dot{\gamma}}\gamma_c{}^{\alpha}{}_{\dot{\beta}}\gamma_{ab\dot{\alpha}\dot{\gamma}} + (-\frac{1}{3}\mathcal{H} - \frac{1}{6}\bar{\mathcal{H}})iT_{cdkl}\Lambda_{\alpha m}\chi_{\beta}{}^{im}n\epsilon^{\alpha\beta}\gamma_{ab\dot{\alpha}\dot{\beta}}\gamma_{cd}{}^{\dot{\alpha}\dot{\beta}}\epsilon^{jklm} \\
& + (\frac{1}{6}\mathcal{D}^\dagger\bar{\mathcal{H}} + \frac{1}{27}\mathcal{D}\bar{\mathcal{I}})iE_{kl}P_c\Lambda_{\alpha m}\Lambda^{\dot{\alpha}k}\gamma_c{}^{\dot{\beta}\alpha}\gamma_{ab\dot{\alpha}\dot{\beta}}\epsilon^{ijlm} + (\frac{1}{5}\mathcal{D}^\dagger\mathcal{D}^\dagger\bar{\mathcal{H}} + \frac{8}{5}\bar{\mathcal{I}})iP_c\Lambda^{\dot{\alpha}i}\Lambda^{\dot{\beta}j}\bar{P}_d\gamma_{d\alpha\dot{\alpha}}\gamma_c{}^{\dot{\gamma}}\gamma_{ab\dot{\beta}\dot{\gamma}} \\
& + (\frac{1}{3}\mathcal{D}^\dagger\mathcal{D}^\dagger\bar{\mathcal{H}} + \frac{8}{3}\bar{\mathcal{I}})iP_cT_{cdkl}\Lambda_{\alpha m}\Lambda^{\dot{\alpha}i}\gamma_{d\beta\dot{\alpha}}\gamma_{ab}{}^{\alpha\beta}\epsilon^{jklm} + (\frac{1}{20}\mathcal{H} - \frac{1}{4}\bar{\mathcal{H}})iT_{cdkl}T_{cdmn}\Lambda_{\alpha p}\Lambda_{\beta q}\gamma_{ab}{}^{\alpha\beta}\epsilon^{ijkl}\epsilon^{mnpq} \\
& + (\frac{1}{2}\mathcal{D}^\dagger\bar{\mathcal{H}} + \mathcal{D}\bar{\mathcal{I}})i\Lambda^{\dot{\alpha}i}\bar{P}_c\epsilon_{\dot{\alpha}\dot{\beta}}\gamma_{d\alpha\dot{\gamma}}\gamma_{c\beta}{}^{\dot{\gamma}}\gamma_{ab}{}^{\alpha\beta}\nabla_d\Lambda^{\dot{\beta}j} + (-\frac{1}{3}\mathcal{H} - \frac{2}{3}\bar{\mathcal{H}})iT_{cdkl}\Lambda_{\alpha m}\Lambda^{\dot{\alpha}i}\bar{P}_c\gamma_{d\beta\dot{\alpha}}\gamma_{ab}{}^{\alpha\beta}\epsilon^{jklm} \\
& + \frac{2}{27}iP_cP_d\mathcal{D}\bar{\mathcal{I}}\Lambda_{\alpha k}\Lambda_{\beta l}\gamma_c{}^{\dot{\alpha}\alpha}\gamma_d{}^{\dot{\beta}\beta}\gamma_{ab\dot{\alpha}\dot{\beta}}\epsilon^{ijkl} + \frac{16}{9}iP_c\mathcal{D}^\dagger\mathcal{I}\Lambda_{\alpha k}\Lambda_{\beta l}\bar{P}_d\gamma_c{}^{\dot{\alpha}\alpha}\gamma_d{}^{\dot{\beta}\beta}\gamma_{ab\dot{\alpha}\dot{\beta}}\epsilon^{ijkl} \\
& + \frac{1}{24}iT_{cdkl}T_{ef}{}^{ik}\mathcal{D}^\dagger\mathcal{I}\Lambda_{\alpha m}\Lambda_{\beta n}\gamma_{ef}{}^{\alpha\beta}\gamma_{ab\dot{\alpha}\dot{\beta}}\gamma_{cd}{}^{\dot{\alpha}\dot{\beta}}\epsilon^{jlmn} - \frac{1}{48}iT_{cdkl}T_{ef}{}^{jk}\mathcal{D}^\dagger\mathcal{I}\Lambda_{\alpha m}\Lambda_{\beta n}\gamma_{ef}{}^{\alpha\beta}\gamma_{ab\dot{\alpha}\dot{\beta}}\gamma_{cd}{}^{\dot{\alpha}\dot{\beta}}\epsilon^{ilmn} \\
& + \frac{1}{32}iT_{cdkl}T_{ef}{}^{kl}\mathcal{D}^\dagger\mathcal{I}\Lambda_{\alpha m}\Lambda_{\beta n}\gamma_{ef}{}^{\alpha\beta}\gamma_{ab\dot{\alpha}\dot{\beta}}\gamma_{cd}{}^{\dot{\alpha}\dot{\beta}}\epsilon^{ijmn} - \frac{1}{120}iT_{cdkl}T_{ef}{}^{km}\mathcal{D}^\dagger\mathcal{I}\Lambda_{\alpha m}\Lambda_{\beta n}\gamma_{ef}{}^{\alpha\beta}\gamma_{ab\dot{\alpha}\dot{\beta}}\gamma_{cd}{}^{\dot{\alpha}\dot{\beta}}\epsilon^{ijln} \\
& + (-\frac{2}{3}\mathcal{D}^\dagger\mathcal{I} + \frac{1}{3}\mathcal{D}\mathcal{H})iP_c\Lambda_{\alpha k}\Lambda_{\beta l}\bar{P}_d\gamma_{c\gamma}{}^{\dot{\alpha}}\gamma_d{}^$$



The four fermion terms are:

[illegible]

$$\begin{aligned}
[\mathcal{E}_{ab}^{ij}]_{4,cont} = & +(-\frac{1}{40} \mathcal{D}^\dagger \mathcal{D}^\dagger \bar{\mathcal{H}} - \frac{13}{60} \bar{\mathcal{I}}) i \Lambda^{\dot{\alpha} i} \Lambda^{\dot{\beta} j} \Lambda^{\dot{\gamma} k} \epsilon_{\dot{\beta} \dot{\gamma} \dot{\gamma} c}^{\delta \alpha} \gamma_{ab \dot{\alpha} \dot{\beta}} \nabla_c \Lambda_{\alpha k} + (-\frac{49}{720} \mathcal{D}^\dagger \mathcal{D}^\dagger \mathcal{D}^\dagger \bar{\mathcal{H}} - \frac{8}{45} \mathcal{D}^\dagger \bar{\mathcal{I}}) i E_{kl} \Lambda^{\dot{\alpha} i} \Lambda^{\dot{\beta} j} \Lambda^{\dot{\gamma} k} \Lambda^{\dot{\delta} l} \epsilon_{\dot{\alpha} \dot{\gamma} \dot{\gamma} ab \dot{\beta} \dot{\delta}} \\
& + (-\frac{1}{72} \mathcal{D}^\dagger \mathcal{D}^\dagger \bar{\mathcal{H}} - \frac{1}{9} \bar{\mathcal{I}}) i \Lambda_{\alpha k} \Lambda^{\dot{\alpha} i} \Lambda^{\dot{\beta} j} \gamma_c^{\alpha} \gamma_{ab \dot{\alpha} \dot{\beta}} \gamma_{cd}^{\dot{\delta}} \nabla_d \Lambda^{\dot{\gamma} k} + (-\frac{1}{72} \mathcal{D}^\dagger \mathcal{D}^\dagger \bar{\mathcal{H}} - \frac{1}{9} \bar{\mathcal{I}}) i \Lambda_{\alpha k} \Lambda^{\dot{\alpha} i} \Lambda^{\dot{\beta} j} \gamma_c^{\alpha} \gamma_{ab \dot{\beta} \dot{\delta}} \gamma_{cd}^{\dot{\delta}} \nabla_d \Lambda^{\dot{\gamma} k} \\
& + (-\frac{49}{360} \mathcal{H} + \frac{1}{90} \bar{\mathcal{H}}) i \Lambda_{\alpha k} \Lambda_{\beta l} \Lambda^{\dot{\alpha} k} \chi^{\dot{\beta}}_{mn} \epsilon^{\alpha \beta} \gamma_{ab \dot{\alpha} \dot{\beta}} \epsilon^{ijlmn} + (-\frac{2}{15} \mathcal{D}^\dagger \mathcal{D}^\dagger \mathcal{D}^\dagger \bar{\mathcal{H}} - \frac{22}{45} \mathcal{D}^\dagger \bar{\mathcal{I}}) i P_c \Lambda_{\alpha k} \Lambda^{\dot{\alpha} i} \Lambda^{\dot{\beta} j} \Lambda^{\dot{\gamma} k} \gamma_c^{\alpha} \gamma_{ab \dot{\beta} \dot{\gamma}} \\
& + (-\frac{1}{120} \mathcal{D}^\dagger \mathcal{D}^\dagger \bar{\mathcal{H}} - \frac{1}{15} \bar{\mathcal{I}}) i \Lambda_{\alpha k} \Lambda^{\dot{\alpha} i} \Lambda^{\dot{\beta} k} \epsilon_{\dot{\alpha} \dot{\beta}} \gamma_c^{\dot{\gamma} \alpha} \gamma_{ab \dot{\gamma} \dot{\delta}} \nabla_c \Lambda^{\dot{\delta} j} + (-\frac{1}{360} \mathcal{D}^\dagger \mathcal{D}^\dagger \mathcal{D}^\dagger \bar{\mathcal{H}} + \frac{1}{45} \mathcal{D}^\dagger \bar{\mathcal{I}}) i E_{kl} \Lambda^{\dot{\alpha} i} \Lambda^{\dot{\beta} j} \Lambda^{\dot{\gamma} k} \Lambda^{\dot{\delta} l} \epsilon_{\dot{\gamma} \dot{\delta}} \gamma_{ab \dot{\alpha} \dot{\beta}} \\
& + (\frac{1}{120} \mathcal{D}^\dagger \mathcal{D}^\dagger \bar{\mathcal{H}} + \frac{1}{15} \bar{\mathcal{I}}) i \Lambda_{\alpha k} \Lambda^{\dot{\alpha} j} \Lambda^{\dot{\beta} k} \epsilon_{\dot{\alpha} \dot{\beta}} \gamma_c^{\dot{\gamma} \alpha} \gamma_{ab \dot{\gamma} \dot{\delta}} \nabla_c \Lambda^{\dot{\delta} i} + (\frac{49}{360} \mathcal{H} - \frac{1}{90} \bar{\mathcal{H}}) i \Lambda_{\alpha k} \Lambda_{\beta l} \Lambda^{\dot{\alpha} k} \chi^{\dot{\beta}}_{mn} \epsilon^{\alpha \beta} \gamma_{ab \dot{\alpha} \dot{\beta}} \epsilon^{ilmn} \\
& + (\frac{1}{72} \mathcal{D}^\dagger \mathcal{D}^\dagger \bar{\mathcal{H}} + \frac{1}{9} \bar{\mathcal{I}}) i \Lambda^{\dot{\alpha} i} \Lambda^{\dot{\beta} j} \Lambda^{\dot{\gamma} k} \gamma_c^{\alpha} \gamma_{ab \dot{\alpha} \dot{\beta}} \gamma_{cd}^{\dot{\delta}} \nabla_d \Lambda_{\alpha k} + (\frac{1}{72} \mathcal{D}^\dagger \mathcal{D}^\dagger \bar{\mathcal{H}} + \frac{1}{9} \bar{\mathcal{I}}) i \Lambda^{\dot{\alpha} i} \Lambda^{\dot{\beta} j} \Lambda^{\dot{\gamma} k} \gamma_c^{\alpha} \gamma_{ab \dot{\beta} \dot{\delta}} \gamma_{cd}^{\dot{\delta}} \nabla_d \Lambda_{\alpha k} \\
& + (\frac{1}{180} \mathcal{D}^\dagger \mathcal{D}^\dagger \mathcal{D}^\dagger \bar{\mathcal{H}} - \frac{2}{45} \mathcal{D}^\dagger \bar{\mathcal{I}}) i P_c \Lambda_{\alpha k} \Lambda^{\dot{\alpha} i} \Lambda^{\dot{\beta} j} \Lambda^{\dot{\gamma} k} \gamma_c^{\alpha} \gamma_{ab \dot{\alpha} \dot{\beta}} + (-\frac{1}{24} \mathcal{D}^\dagger \mathcal{D}^\dagger \mathcal{D}^\dagger \mathcal{D}^\dagger \bar{\mathcal{H}} - \frac{1}{10} \mathcal{D}^\dagger \mathcal{D}^\dagger \bar{\mathcal{I}}) i T_{cdkl} \Lambda^{\dot{\alpha} i} \Lambda^{\dot{\beta} j} \Lambda^{\dot{\gamma} k} \Lambda^{\dot{\delta} l} \gamma_{ab \dot{\gamma} \dot{\delta}} \gamma_{cd \dot{\alpha} \dot{\beta}} \\
& + (\frac{1}{40} \mathcal{D}^\dagger \mathcal{D}^\dagger \bar{\mathcal{H}} + \frac{1}{5} \bar{\mathcal{I}}) i \Lambda_{\alpha k} \Lambda^{\dot{\alpha} i} \Lambda^{\dot{\beta} j} \epsilon_{\dot{\alpha} \dot{\beta}} \gamma_c^{\dot{\gamma} \alpha} \gamma_{ab \dot{\gamma} \dot{\delta}} \nabla_c \Lambda^{\dot{\delta} k} + (\frac{1}{3} \mathcal{D}^\dagger \bar{\mathcal{H}} - \frac{2}{3} \mathcal{D} \bar{\mathcal{I}}) i E^{ik} \Lambda_{\alpha k} \Lambda_{\beta l} \Lambda^{\dot{\alpha} j} \Lambda^{\dot{\beta} l} \epsilon_{\dot{\alpha} \dot{\beta}} \gamma_{ab}^{\alpha \beta} \\
& + (-\frac{1}{12} \mathcal{D} \mathcal{D} \mathcal{H} - \frac{2}{3} \mathcal{I}) i \Lambda_{\alpha k} \Lambda_{\beta l} \Lambda_{\gamma m} R(Q)_{cd\delta}^k \gamma_{ab}^{\beta \delta} \gamma_{cd}^{\alpha \gamma} \epsilon^{ijlm} + (\frac{1}{10} \mathcal{D}^\dagger \mathcal{D}^\dagger \bar{\mathcal{H}} + \frac{47}{60} \bar{\mathcal{I}}) i \Lambda^{\dot{\alpha} i} \Lambda^{\dot{\beta} j} \Lambda^{\dot{\gamma} k} \epsilon_{\dot{\alpha} \dot{\gamma} \dot{\gamma} c}^{\delta \alpha} \gamma_{ab \dot{\beta} \dot{\delta}} \nabla_c \Lambda_{\alpha k} \\
& + (\frac{1}{9} \mathcal{D}^\dagger \bar{\mathcal{H}} + \frac{2}{3} \mathcal{D} \bar{\mathcal{I}}) i \Lambda_{\alpha k} \Lambda^{\dot{\alpha} i} \Lambda^{\dot{\beta} j} \Lambda^{\dot{\gamma} k} \bar{P}_c \gamma_c^{\alpha} \gamma_{ab \dot{\alpha} \dot{\beta}} + (\frac{1}{9} \mathcal{D}^\dagger \bar{\mathcal{H}} + \frac{2}{9} \mathcal{D} \bar{\mathcal{I}}) i E^{ik} \Lambda_{\alpha k} \Lambda_{\beta l} \Lambda^{\dot{\alpha} j} \Lambda^{\dot{\beta} l} \epsilon^{\alpha \beta} \gamma_{ab \dot{\alpha} \dot{\beta}} \\
& + (-\frac{17}{40} \mathcal{H} - \frac{7}{60} \bar{\mathcal{H}}) i \Lambda_{\alpha k} \Lambda_{\beta l} \Lambda^{\dot{\alpha} i} \chi^{\dot{\beta}}_{mn} \epsilon^{\alpha \beta} \gamma_{ab \dot{\alpha} \dot{\beta}} \epsilon^{ijlmn} + (\frac{1}{8} \mathcal{D}^\dagger \bar{\mathcal{H}} + \frac{1}{4} \mathcal{D} \bar{\mathcal{I}}) i \Lambda^{\dot{\alpha} j} \Lambda^{\dot{\beta} k} \Lambda_{\alpha k} R(Q)_{cd\beta}^i \epsilon_{\dot{\alpha} \dot{\beta}} \gamma_{cd \gamma}^{\alpha} \gamma_{ab}^{\beta \gamma} \\
& + (\frac{2}{15} \mathcal{D}^\dagger \mathcal{D}^\dagger \bar{\mathcal{H}} + \frac{16}{15} \bar{\mathcal{I}}) i \Lambda_{\alpha k} \Lambda^{\dot{\alpha} j} \Lambda^{\dot{\beta} k} \epsilon_{\dot{\alpha} \dot{\gamma}} \gamma_{c \dot{\beta} \dot{\delta}} \gamma_{ab}^{\alpha \beta} \nabla_c \Lambda^{\dot{\gamma} i} + (\frac{1}{6} \mathcal{H} - \frac{1}{6} \bar{\mathcal{H}}) i T_{cd}^{ij} \Lambda_{\alpha k} \Lambda_{\beta l} \Lambda^{\dot{\alpha} k} \Lambda^{\dot{\beta} l} \gamma_{cd}^{\alpha \beta} \gamma_{ab \dot{\alpha} \dot{\beta}} \\
& + (\frac{2}{9} \mathcal{D}^\dagger \bar{\mathcal{H}} - \frac{2}{9} \mathcal{D} \bar{\mathcal{I}}) i \Lambda_{\alpha k} \Lambda^{\dot{\alpha} i} \Lambda^{\dot{\beta} j} \Lambda^{\dot{\gamma} k} \bar{P}_c \gamma_c^{\alpha} \gamma_{ab \dot{\beta} \dot{\gamma}} + (\frac{2}{9} \mathcal{D}^\dagger \bar{\mathcal{H}} - \frac{2}{9} \mathcal{D} \bar{\mathcal{I}}) i \Lambda_{\alpha k} \Lambda^{\dot{\alpha} i} \Lambda^{\dot{\beta} j} \Lambda^{\dot{\gamma} k} \bar{P}_c \gamma_c^{\alpha} \gamma_{ab \dot{\beta} \dot{\gamma}} \\
& + (\frac{1}{30} \mathcal{D}^\dagger \mathcal{D}^\dagger \bar{\mathcal{H}} + \frac{34}{15} \bar{\mathcal{I}}) i \Lambda_{\alpha k} \Lambda^{\dot{\alpha} j} \Lambda^{\dot{\beta} k} \epsilon_{\dot{\beta} \dot{\gamma}} \gamma_{c \dot{\beta} \dot{\delta}} \gamma_{ab}^{\alpha \beta} \nabla_c \Lambda^{\dot{\gamma} i} + (\frac{3}{10} \mathcal{D}^\dagger \mathcal{D}^\dagger \bar{\mathcal{H}} + \frac{27}{5} \bar{\mathcal{I}}) i \Lambda_{\alpha k} \Lambda^{\dot{\alpha} i} \Lambda^{\dot{\beta} k} \epsilon_{\dot{\alpha} \dot{\beta}} \gamma_{c \dot{\beta} \dot{\gamma}} \gamma_{ab}^{\alpha \beta} \nabla_c \Lambda^{\dot{\gamma} j} \\
& - \frac{2}{5} i \mathcal{D}^\dagger \mathcal{I} \Lambda_{\alpha k} \Lambda_{\beta l} \Lambda^{\dot{\alpha} m} \epsilon^{\alpha \gamma} \gamma_c^{\dot{\beta} \beta} \gamma_{ab \dot{\alpha} \dot{\beta}} \nabla_c \Lambda_{\gamma m} \epsilon^{ijkl} - \frac{2}{3} i \mathcal{D}^\dagger \mathcal{I} \Lambda_{\alpha k} \Lambda_{\beta l} \Lambda_{\gamma m} \epsilon^{\alpha \beta} \gamma_c^{\dot{\alpha} \gamma} \gamma_{ab \dot{\alpha} \dot{\beta}} \nabla_c \Lambda^{\dot{\beta} k} \epsilon^{ijlm} \\
& + (-\frac{7}{24} \mathcal{D}^\dagger \mathcal{I} + \frac{13}{80} \mathcal{D} \mathcal{H}) i \Lambda_{\alpha k} \Lambda_{\beta l} \Lambda_{\gamma m} \epsilon^{\alpha \beta} \gamma_{cd \dot{\alpha}} \gamma_{ab}^{\gamma \delta} \nabla_c \Lambda^{\dot{\alpha} k} \epsilon^{ijlm} + (-\frac{4}{15} \mathcal{D}^\dagger \mathcal{I} + \frac{1}{6} \mathcal{D} \mathcal{H}) i \Lambda_{\alpha k} \Lambda_{\beta l} \Lambda^{\dot{\alpha} j} \epsilon^{\alpha \gamma} \gamma_c^{\dot{\beta} \beta} \gamma_{ab \dot{\alpha} \dot{\beta}} \nabla_c \Lambda_{\gamma m} \epsilon^{iklm} \\
& + (-\frac{1}{5} \mathcal{D}^\dagger \mathcal{I} + \frac{1}{10} \mathcal{D} \mathcal{H}) i \Lambda_{\alpha k} \Lambda^{\dot{\alpha} k} \Lambda_{\beta l} \epsilon^{\alpha \gamma} \gamma_{cd \dot{\alpha}} \gamma_{ab}^{\beta \delta} \nabla_c \Lambda_{\gamma m} \epsilon^{ijlm} + (-\frac{1}{20} \mathcal{D}^\dagger \mathcal{I} + \frac{1}{40} \mathcal{D} \mathcal{H}) i \Lambda^{\dot{\alpha} k} \Lambda_{\alpha k} \Lambda_{\beta l} \epsilon^{\alpha \beta} \gamma_{c \dot{\gamma}} \gamma_{ab}^{\gamma \delta} \nabla_c \Lambda_{\delta m} \epsilon^{ijlm} \\
& + (\frac{1}{24} \mathcal{D}^\dagger \bar{\mathcal{H}} - \frac{1}{12} \mathcal{D} \bar{\mathcal{I}}) i T_{cdkl} \Lambda_{\alpha m} \Lambda_{\beta n} \Lambda^{\dot{\alpha} j} \Lambda^{\dot{\beta} m} \gamma_{ab}^{\alpha \beta} \gamma_{cd \dot{\alpha} \dot{\beta}} \epsilon^{ikln} + \frac{1}{96} i \mathcal{D}^\dagger \mathcal{D}^\dagger \mathcal{D}^\dagger \mathcal{D}^\dagger \bar{\mathcal{H}} E^{ik} \Lambda^{\dot{\alpha} j} \Lambda^{\dot{\beta} l} \Lambda^{\dot{\gamma} m} \Lambda^{\dot{\delta} n} \epsilon_{\dot{\alpha} \dot{\beta}} \gamma_{ab \dot{\gamma} \dot{\delta}} \epsilon^{klmn} \\
& + \frac{11}{120} i \mathcal{D} \mathcal{D} \mathcal{D} \mathcal{H} T_{cd}^{jk} \Lambda_{\alpha k} \Lambda_{\beta l} \Lambda_{\gamma m} \Lambda_{\delta n} \gamma_{ab}^{\beta \gamma} \gamma_{cd}^{\alpha \delta} \epsilon^{ilmn} - \frac{11}{120} i \mathcal{D} \mathcal{D} \mathcal{D} \mathcal{H} T_{cd}^{ik} \Lambda_{\alpha k} \Lambda_{\beta l} \Lambda_{\gamma m} \Lambda_{\delta n} \gamma_{ab}^{\beta \gamma} \gamma_{cd}^{\alpha \delta} \epsilon^{jlmn} \\
& - \frac{1}{96} i \mathcal{D}^\dagger \mathcal{D}^\dagger \mathcal{D}^\dagger \mathcal{D}^\dagger \bar{\mathcal{H}} E^{jk} \Lambda^{\dot{\alpha} i} \Lambda^{\dot{\beta} l} \Lambda^{\dot{\gamma} m} \Lambda^{\dot{\delta} n} \epsilon_{\dot{\alpha} \dot{\beta}} \gamma_{ab \dot{\gamma} \dot{\delta}} \epsilon^{klmn} + (-\frac{1}{24} \mathcal{D}^\dagger \bar{\mathcal{H}} + \frac{1}{4} \mathcal{D} \bar{\mathcal{I}}) i T_{cdkl} \Lambda_{\alpha m} \Lambda_{\beta n} \Lambda^{\dot{\alpha} m} \Lambda^{\dot{\beta} n} \gamma_{ab}^{\alpha \beta} \gamma_{cd \dot{\alpha} \dot{\beta}} \epsilon^{ijkl} + 2 \dots
\end{aligned}$$

$$\begin{aligned}
[\mathcal{E}_{ab}^{ij}]_{4,cont} = & +(-\frac{1}{24} \mathcal{D}^\dagger \bar{\mathcal{H}} + \frac{1}{12} \mathcal{D} \bar{\mathcal{I}}) i T_{cdkl} \Lambda_{\alpha m} \Lambda_{\beta n} \Lambda^{\dot{\alpha} i} \Lambda^{\dot{\beta} m} \gamma_{ab}^{\alpha \beta} \gamma_{cd \dot{\alpha} \dot{\beta}} \varepsilon^{ijkln} + (\frac{1}{12} \mathcal{D}^\dagger \bar{\mathcal{I}} - \frac{1}{24} \mathcal{D} \mathcal{H}) i \Lambda_{\alpha k} \Lambda_{\beta l} \Lambda_{\gamma m} \gamma_c^{\alpha} \gamma_{cd \dot{\delta}}^{\beta} \gamma_{ab}^{\gamma \delta} \nabla_d \Lambda^{\dot{\alpha} k} \varepsilon^{ijlm} \\
& + (\frac{1}{12} \mathcal{D}^\dagger \bar{\mathcal{I}} - \frac{1}{24} \mathcal{D} \mathcal{H}) i \Lambda_{\alpha k} \Lambda^{\dot{\alpha} l} \Lambda_{\beta m} \gamma_c^{\gamma} \gamma_{cd \dot{\delta}}^{\alpha} \gamma_{ab}^{\beta \delta} \nabla_d \Lambda_{\gamma l} \varepsilon^{ijkm} + (\frac{1}{5} \mathcal{D}^\dagger \bar{\mathcal{I}} - \frac{1}{10} \mathcal{D} \mathcal{H}) i \Lambda_{\alpha k} \Lambda^{\dot{\alpha} k} \Lambda_{\beta l} \varepsilon^{\beta \gamma} \gamma_{cd \dot{\alpha}} \gamma_{ab}^{\alpha \delta} \nabla_c \Lambda_{\gamma m} \varepsilon^{ijlm} \\
& + (\frac{4}{15} \mathcal{D}^\dagger \bar{\mathcal{I}} - \frac{1}{6} \mathcal{D} \mathcal{H}) i \Lambda_{\alpha k} \Lambda_{\beta l} \Lambda^{\dot{\alpha} i} \varepsilon^{\alpha \gamma} \gamma_c^{\dot{\beta} \beta} \gamma_{ab \dot{\alpha} \dot{\beta}} \nabla_c \Lambda_{\gamma m} \varepsilon^{ijklm} + (\frac{11}{15} \mathcal{D}^\dagger \bar{\mathcal{I}} - \frac{2}{5} \mathcal{D} \mathcal{H}) i \Lambda_{\alpha k} \Lambda_{\beta l} \Lambda^{\dot{\alpha} k} \varepsilon^{\beta \gamma} \gamma_c^{\dot{\beta} \alpha} \gamma_{ab \dot{\alpha} \dot{\beta}} \nabla_c \Lambda_{\gamma m} \varepsilon^{ijlm} \\
& + (\frac{4}{5} \mathcal{D}^\dagger \bar{\mathcal{I}} - \frac{1}{10} \mathcal{D} \mathcal{H}) i \Lambda_{\alpha k} \Lambda_{\beta l} \Lambda^{\dot{\alpha} k} \varepsilon^{\alpha \gamma} \gamma_c^{\dot{\beta} \beta} \gamma_{ab \dot{\alpha} \dot{\beta}} \nabla_c \Lambda_{\gamma m} \varepsilon^{ijlm} + (\frac{9}{5} \mathcal{D}^\dagger \bar{\mathcal{I}} - \frac{2}{5} \mathcal{D} \mathcal{H}) i \Lambda_{\alpha k} \Lambda_{\beta l} \Lambda^{\dot{\alpha} k} \varepsilon^{\alpha \beta} \gamma_c^{\dot{\beta} \gamma} \gamma_{ab \dot{\alpha} \dot{\beta}} \nabla_c \Lambda_{\gamma m} \varepsilon^{ijlm} \\
& + (\frac{1}{6} \mathcal{H} + \frac{1}{3} \bar{\mathcal{H}}) i T_{cd}^{ij} \Lambda_{\alpha k} \Lambda^{\dot{\alpha} k} \Lambda^{\dot{\beta} l} \Lambda_{\beta l} \varepsilon_{\dot{\alpha} \dot{\beta}} \gamma_{cd \gamma}^{\alpha} \gamma_{ab}^{\beta \gamma} + (-\frac{2}{9} \mathcal{H} + \frac{2}{9} \bar{\mathcal{H}}) i E_{kl} \Lambda_{\alpha m} \Lambda_{\beta n} \Lambda^{\dot{\alpha} k} \Lambda^{\dot{\beta} m} \varepsilon_{\dot{\alpha} \dot{\beta}} \gamma_{ab}^{\alpha \beta} \varepsilon^{ijn} \\
& + (\frac{1}{3} \mathcal{H} + \frac{1}{6} \bar{\mathcal{H}}) i T_{cd}^{jk} \Lambda_{\alpha k} \Lambda^{\dot{\alpha} i} \Lambda^{\dot{\beta} l} \Lambda_{\beta l} \varepsilon_{\dot{\alpha} \dot{\beta}} \gamma_{cd \gamma}^{\beta} \gamma_{ab}^{\alpha \gamma} + (-\frac{1}{6} \mathcal{D}^\dagger \bar{\mathcal{H}} - \frac{5}{3} \mathcal{D} \bar{\mathcal{I}}) i \Lambda_{\alpha k} \Lambda^{\dot{\alpha} i} \Lambda^{\dot{\beta} j} \Lambda^{\dot{\gamma} k} \bar{P}_c \varepsilon_{\dot{\alpha} \dot{\gamma}} \gamma_{c \beta \dot{\beta}} \gamma_{ab}^{\alpha \beta} \\
& + (-\frac{1}{6} \mathcal{D}^\dagger \bar{\mathcal{H}} - \frac{5}{3} \mathcal{D} \bar{\mathcal{I}}) i \Lambda_{\alpha k} \Lambda^{\dot{\alpha} i} \Lambda^{\dot{\beta} j} \Lambda^{\dot{\gamma} k} \bar{P}_c \varepsilon_{\dot{\beta} \dot{\gamma}} \gamma_{c \beta \dot{\alpha}} \gamma_{ab}^{\alpha \beta} + (-\frac{1}{12} \mathcal{H} + \frac{1}{12} \bar{\mathcal{H}}) i \Lambda_{\alpha k} \Lambda_{\beta l} \Lambda^{\dot{\alpha} k} R(Q)_{cd}^{\dot{\beta}} \varepsilon^{\alpha \beta} \gamma_{ab \dot{\beta} \dot{\gamma}} \gamma_{cd}^{\dot{\gamma}} \varepsilon^{ijlm} \\
& + (\frac{71}{720} \mathcal{D} \mathcal{D} \mathcal{H} + \frac{97}{180} \mathcal{I}) i E^{kl} \Lambda_{\alpha k} \Lambda_{\beta l} \Lambda_{\gamma m} \Lambda_{\delta n} \varepsilon^{\alpha \beta} \gamma_{ab}^{\gamma \delta} \varepsilon^{ijmn} + (\frac{1}{16} \mathcal{D} \mathcal{D} \mathcal{D} \mathcal{H} - \frac{1}{15} \mathcal{D} \mathcal{I}) i T_{cd}^{kl} \Lambda_{\alpha k} \Lambda_{\beta l} \Lambda_{\gamma m} \Lambda_{\delta n} \gamma_{ab}^{\alpha \beta} \gamma_{cd}^{\gamma \delta} \varepsilon^{ijmn} \\
& + (-\frac{1}{120} \mathcal{D} \mathcal{D} \mathcal{D} \mathcal{H} - \frac{1}{3} \mathcal{D} \mathcal{I}) i T_{cd}^{jk} \Lambda_{\alpha k} \Lambda_{\beta l} \Lambda_{\gamma m} \Lambda_{\delta n} \gamma_{ab}^{\alpha \beta} \gamma_{cd}^{\gamma \delta} \varepsilon^{ilmn} + (\frac{3}{40} \mathcal{D}^\dagger \mathcal{D}^\dagger \mathcal{D}^\dagger \bar{\mathcal{H}} + \frac{2}{5} \mathcal{D}^\dagger \bar{\mathcal{I}}) i P_c \Lambda_{\alpha k} \Lambda^{\dot{\alpha} i} \Lambda^{\dot{\beta} j} \Lambda^{\dot{\gamma} k} \varepsilon_{\dot{\alpha} \dot{\beta}} \gamma_c^{\dot{\delta} \alpha} \gamma_{ab \dot{\gamma} \dot{\delta}} \\
& + (\frac{1}{24} \mathcal{D} \mathcal{D} \mathcal{D} \mathcal{H} - \frac{1}{6} \mathcal{D} \mathcal{I}) i T_{cd}^{ij} \Lambda_{\alpha k} \Lambda_{\beta l} \Lambda_{\gamma m} \Lambda_{\delta n} \gamma_{ab}^{\alpha \beta} \gamma_{cd}^{\gamma \delta} \varepsilon^{klmn} + (\frac{151}{360} \mathcal{D} \mathcal{D} \mathcal{H} + \frac{77}{90} \mathcal{I}) i \Lambda_{\alpha k} \Lambda_{\beta l} \Lambda^{\dot{\alpha} k} \Lambda_{\gamma m} \bar{P}_c \gamma_c^{\beta} \gamma_{ab}^{\alpha \gamma} \varepsilon^{ijlm} \\
& + (-\frac{7}{120} \mathcal{D} \mathcal{D} \mathcal{D} \mathcal{H} - \frac{1}{5} \mathcal{D} \mathcal{I}) i T_{cd}^{kl} \Lambda_{\alpha k} \Lambda_{\beta l} \Lambda_{\gamma m} \Lambda_{\delta n} \gamma_{ab}^{\alpha \gamma} \gamma_{cd}^{\beta \delta} \varepsilon^{ijmn} + (\frac{3}{80} \mathcal{D} \mathcal{D} \mathcal{D} \mathcal{H} + \frac{1}{10} \mathcal{D} \mathcal{I}) i T_{cd}^{kl} \Lambda_{\alpha k} \Lambda_{\beta l} \Lambda_{\gamma m} \Lambda_{\delta n} \gamma_{ab}^{\gamma \delta} \gamma_{cd}^{\alpha \beta} \varepsilon^{ijmn} \\
& + (-\frac{101}{360} \mathcal{D} \mathcal{D} \mathcal{H} - \frac{67}{90} \mathcal{I}) i E^{kl} \Lambda_{\alpha k} \Lambda_{\beta l} \Lambda_{\gamma m} \Lambda_{\delta n} \varepsilon^{\alpha \gamma} \gamma_{ab}^{\beta \delta} \varepsilon^{ijmn} + (\frac{1}{360} \mathcal{D}^\dagger \mathcal{D}^\dagger \mathcal{D}^\dagger \bar{\mathcal{H}} - \frac{2}{15} \mathcal{D}^\dagger \bar{\mathcal{I}}) i P_c \Lambda_{\alpha k} \Lambda^{\dot{\alpha} i} \Lambda^{\dot{\beta} j} \Lambda^{\dot{\gamma} k} \varepsilon_{\dot{\beta} \dot{\gamma}} \gamma_c^{\dot{\delta} \alpha} \gamma_{ab \dot{\delta}} \\
& + (\frac{1}{360} \mathcal{D}^\dagger \mathcal{D}^\dagger \mathcal{D}^\dagger \bar{\mathcal{H}} - \frac{2}{15} \mathcal{D}^\dagger \bar{\mathcal{I}}) i P_c \Lambda_{\alpha k} \Lambda^{\dot{\alpha} i} \Lambda^{\dot{\beta} j} \Lambda^{\dot{\gamma} k} \varepsilon_{\dot{\beta} \dot{\gamma}} \gamma_c^{\dot{\delta} \alpha} \gamma_{ab \dot{\delta}} + (\frac{1}{120} \mathcal{D} \mathcal{D} \mathcal{D} \mathcal{H} + \frac{1}{3} \mathcal{D} \mathcal{I}) i T_{cd}^{ik} \Lambda_{\alpha k} \Lambda_{\beta l} \Lambda_{\gamma m} \Lambda_{\delta n} \gamma_{ab}^{\alpha \beta} \gamma_{cd}^{\gamma \delta} \varepsilon^{jlmn} \\
& + (-\frac{1}{36} \mathcal{H} - \frac{1}{18} \bar{\mathcal{H}}) i E_{kl} \Lambda_{\alpha m} \Lambda_{\beta n} \Lambda^{\dot{\alpha} k} \Lambda^{\dot{\beta} l} \varepsilon_{\dot{\alpha} \dot{\beta}} \gamma_{ab}^{\alpha \beta} \varepsilon^{ijmn} + (-\frac{1}{9} \mathcal{H} - \frac{1}{18} \bar{\mathcal{H}}) i E_{kl} \Lambda_{\alpha m} \Lambda_{\beta n} \Lambda^{\dot{\alpha} k} \Lambda^{\dot{\beta} m} \varepsilon^{\alpha \beta} \gamma_{ab \dot{\alpha} \dot{\beta}} \varepsilon^{ijn} \\
& + (\frac{4}{9} \mathcal{H} - \frac{1}{9} \bar{\mathcal{H}}) i P_c \Lambda_{\alpha k} \Lambda_{\beta l} \Lambda^{\dot{\alpha} k} \Lambda_{\gamma m} \gamma_c^{\alpha} \gamma_{ab}^{\beta \gamma} \varepsilon^{ijlm} + (-\frac{71}{360} \mathcal{D} \mathcal{D} \mathcal{H} - \frac{97}{90} \mathcal{I}) i \Lambda_{\alpha k} \Lambda_{\beta l} \Lambda^{\dot{\alpha} k} \Lambda_{\gamma m} \bar{P}_c \gamma_c^{\alpha} \gamma_{ab}^{\beta \gamma} \varepsilon^{ijlm} \\
& + (\frac{1}{12} \mathcal{D}^\dagger \bar{\mathcal{H}} + \frac{1}{6} \mathcal{D} \bar{\mathcal{I}}) i T_{cdkl} \Lambda_{\alpha m} \Lambda_{\beta n} \Lambda^{\dot{\alpha} i} \Lambda^{\dot{\beta} j} \gamma_{ab}^{\alpha \beta} \gamma_{cd \dot{\alpha} \dot{\beta}} \varepsilon^{klmn} + (-\frac{1}{3} \mathcal{H} - \frac{1}{6} \bar{\mathcal{H}}) i T_{cd}^{ik} \Lambda_{\alpha k} \Lambda^{\dot{\alpha} j} \Lambda^{\dot{\beta} l} \Lambda_{\beta l} \varepsilon_{\dot{\alpha} \dot{\beta}} \gamma_{cd \gamma}^{\beta} \gamma_{ab}^{\alpha \gamma} \\
& + (-\frac{5}{9} \mathcal{H} - \frac{4}{9} \bar{\mathcal{H}}) i P_c \Lambda_{\alpha k} \Lambda_{\beta l} \Lambda^{\dot{\alpha} k} \Lambda_{\gamma m} \gamma_c^{\beta} \gamma_{ab}^{\alpha \gamma} \varepsilon^{ijlm} + (-\frac{1}{6} \mathcal{D}^\dagger \mathcal{D}^\dagger \mathcal{D}^\dagger \bar{\mathcal{H}} - 5 \mathcal{D}^\dagger \bar{\mathcal{I}}) i P_c \Lambda$$

The six fermion terms are:

$$\begin{aligned}
[\mathcal{E}_{ab}{}^{ij}]_6 = & \left( \frac{1}{40} \mathcal{D}^\dagger \mathcal{D}^\dagger \bar{\mathcal{H}} - \frac{2}{15} \bar{\mathcal{I}} \right) i \Lambda_{\alpha k} \Lambda_{\beta l} \Lambda^{\dot{\alpha} i} \Lambda^{\dot{\beta} j} \Lambda^{\dot{\gamma} k} \Lambda^{\dot{\delta} l} \epsilon^{\alpha \beta} \epsilon_{\dot{\gamma} \dot{\delta}} \gamma_{ab \dot{\alpha} \dot{\beta}} + \left( -\frac{13}{60} \mathcal{D}^\dagger \mathcal{D}^\dagger \bar{\mathcal{H}} - \frac{16}{15} \bar{\mathcal{I}} \right) i \Lambda_{\alpha k} \Lambda_{\beta l} \Lambda^{\dot{\alpha} i} \Lambda^{\dot{\beta} j} \Lambda^{\dot{\gamma} k} \Lambda^{\dot{\delta} l} \epsilon^{\alpha \beta} \epsilon_{\dot{\alpha} \dot{\gamma}} \gamma_{ab \dot{\beta} \dot{\delta}} \\
& + \left( -\frac{1}{15} \mathcal{D}^\dagger \mathcal{D}^\dagger \bar{\mathcal{H}} + \frac{2}{15} \bar{\mathcal{I}} \right) i \Lambda_{\alpha k} \Lambda_{\beta l} \Lambda^{\dot{\alpha} i} \Lambda^{\dot{\beta} j} \Lambda^{\dot{\gamma} k} \Lambda^{\dot{\delta} l} \epsilon^{\alpha \beta} \epsilon_{\dot{\beta} \dot{\gamma}} \gamma_{ab \dot{\alpha} \dot{\delta}} + \left( \frac{3}{4} \mathcal{D}^\dagger \mathcal{D}^\dagger \bar{\mathcal{H}} + 8 \bar{\mathcal{I}} \right) i \Lambda_{\alpha k} \Lambda_{\beta l} \Lambda^{\dot{\alpha} i} \Lambda^{\dot{\beta} j} \Lambda^{\dot{\gamma} k} \Lambda^{\dot{\delta} l} \epsilon_{\dot{\alpha} \dot{\gamma}} \epsilon^{\dot{\beta} \dot{\delta}} \gamma_{ab}{}^{\alpha \beta} \\
& + \frac{1}{480} i \mathcal{D}^\dagger \mathcal{D}^\dagger \mathcal{D}^\dagger \mathcal{D}^\dagger \bar{\mathcal{H}} \Lambda^{\dot{\alpha} i} \Lambda^{\dot{\beta} j} \Lambda^{\dot{\gamma} k} \Lambda^{\dot{\delta} l} \Lambda^{\dot{e} m} \Lambda^{\sigma 1 n} \epsilon_{\dot{\alpha} \dot{\gamma}} \epsilon_{\dot{\beta} \dot{\delta}} \gamma_{ab \dot{e} \sigma 1} \varepsilon_{klmn} + \left( -\frac{11}{120} \mathcal{D}^\dagger \mathcal{I} - \frac{3}{80} \mathcal{D} \mathcal{H} \right) i \Lambda_{\alpha k} \Lambda_{\beta l} \Lambda^{\dot{\alpha} k} \Lambda^{\dot{\beta} l} \Lambda_{\gamma m} \Lambda_{\delta n} \epsilon_{\dot{\alpha} \dot{\beta}} \epsilon^{\alpha \beta} \gamma_{ab}{}^{\gamma \delta} \varepsilon^{ijmn} \\
& + \left( \frac{11}{60} \mathcal{D}^\dagger \mathcal{I} - \frac{17}{40} \mathcal{D} \mathcal{H} \right) i \Lambda_{\alpha k} \Lambda_{\beta l} \Lambda^{\dot{\alpha} k} \Lambda^{\dot{\beta} l} \Lambda_{\gamma m} \Lambda_{\delta n} \epsilon_{\dot{\alpha} \dot{\beta}} \epsilon^{\alpha \gamma} \gamma_{ab}{}^{\beta \delta} \varepsilon^{ijmn} + \left( \mathcal{D}^\dagger \mathcal{I} - \frac{1}{4} \mathcal{D} \mathcal{H} \right) i \Lambda_{\alpha k} \Lambda_{\beta l} \Lambda^{\dot{\alpha} k} \Lambda^{\dot{\beta} l} \Lambda_{\gamma m} \Lambda_{\delta n} \epsilon^{\alpha \gamma} \epsilon^{\beta \delta} \gamma_{ab \dot{\alpha} \dot{\beta}} \varepsilon^{ijmn} \\
& + \frac{1}{192} i \mathcal{D} \mathcal{D} \mathcal{D} \mathcal{D} \mathcal{H} \Lambda_{\alpha k} \Lambda_{\beta l} \Lambda_{\gamma m} \Lambda_{\delta n} \Lambda_{\epsilon p} \Lambda_{\epsilon 1 q} \epsilon^{\alpha \beta} \epsilon^{\gamma \delta} \gamma_{ab}{}^{\epsilon \epsilon 1} \varepsilon^{ijkm} \varepsilon^{lnpq}
\end{aligned}$$

## $\rho$ and $\kappa$

We give the expressions for  $\rho_{\alpha ij}{}^k$  and  $\kappa_{\alpha ij}{}^k$  with projection onto the  $\overline{\mathbf{20}}$  assumed (i.e. antisymmetrized with trace removed).

$$\begin{aligned}
\rho_{\alpha ij}{}^k &= iD^{kl}{}_{ij}\Lambda_{\alpha l}\bar{\mathcal{H}} + 2iE_{il}\chi_{\alpha}{}^{kl}{}_j\mathcal{H} + (-\mathcal{D}^\dagger\bar{\mathcal{H}} - 2\mathcal{D}\bar{\mathcal{I}})i\gamma_{a\alpha\dot{\alpha}}\nabla_a\chi^{\dot{\alpha}}{}_{ij}{}^k - \frac{1}{2}iE_{il}E^{kl}\Lambda_{\alpha j}\mathcal{H} + 4iP_a\bar{\mathcal{I}}\chi^{\dot{\alpha}}{}_{ij}{}^k\gamma_{a\alpha\dot{\alpha}} + \frac{1}{2}iT_{ab}{}^{kl}R(Q)_{ab\alpha}{}^m\mathcal{H}\varepsilon_{ijlm} \\
&- \frac{3}{4}iT_{ab}{}^{lm}R(Q)_{ab\alpha}{}^k\mathcal{H}\varepsilon_{ijlm} + i\Lambda_{\beta i}R(V)_{ab}{}^k{}_j\gamma_{ab\alpha}{}^\beta\mathcal{H} + (-\frac{1}{2}\mathcal{D}^\dagger\bar{\mathcal{H}} - \mathcal{D}\bar{\mathcal{I}})iE^{kl}\chi_{\alpha}{}^{mn}{}_l\varepsilon_{ijmn} + \frac{1}{4}iE_{il}E_{jm}\Lambda_{\alpha n}\mathcal{D}\mathcal{H}\varepsilon^{klmn} \\
&+ iE^{kl}\bar{\mathcal{I}}\gamma_{a\alpha\dot{\alpha}}\nabla_a\Lambda^{\dot{\alpha}m}\varepsilon_{ijlm} - \frac{1}{2}iT_{ablm}T_{abij}\Lambda_{\alpha n}\mathcal{D}^\dagger\bar{\mathcal{H}}\varepsilon^{klmn} - iT_{abij}\bar{\mathcal{I}}\gamma_{c\alpha}{}^{\dot{\alpha}}\gamma_{ab\dot{\alpha}\dot{\beta}}\nabla_c\Lambda^{\dot{\beta}k} + \frac{1}{8}iT_{ab}{}^{kl}\chi_{\beta}{}^{mn}{}_l\gamma_{ab\alpha}{}^\beta\mathcal{H}\varepsilon_{ijmn} \\
&+ \frac{3}{4}iT_{ab}{}^{lm}\chi_{\beta}{}^{kn}{}_i\gamma_{ab\alpha}{}^\beta\mathcal{H}\varepsilon_{jlmn} + i\Lambda_{\alpha l}\Lambda^{\dot{\alpha}k}\chi^{\dot{\beta}}{}_{ij}{}^l\epsilon_{\dot{\alpha}\dot{\beta}}\mathcal{D}^\dagger\bar{\mathcal{H}} + 2i\Lambda_{\alpha i}\Lambda^{\dot{\alpha}l}\chi^{\dot{\beta}}{}_{jl}{}^k\epsilon_{\dot{\alpha}\dot{\beta}}\mathcal{D}\bar{\mathcal{I}} + 2i\Lambda_{\alpha l}\Lambda^{\dot{\alpha}l}\chi^{\dot{\beta}}{}_{ij}{}^k\epsilon_{\dot{\alpha}\dot{\beta}}\mathcal{D}\bar{\mathcal{I}} \\
&+ i\Lambda_{\beta i}\Lambda^{\dot{\alpha}k}\gamma_a{}^\beta{}_{\dot{\alpha}}\mathcal{H}\nabla_a\Lambda_{\alpha j} - i\Lambda^{\dot{\alpha}l}\bar{\mathcal{I}}\gamma_{a\alpha\dot{\alpha}}\nabla_aE^{km}\varepsilon_{ijlm} - i\Lambda^{\dot{\alpha}k}\bar{\mathcal{I}}\gamma_{a\alpha}{}^{\dot{\beta}}\gamma_{bc\dot{\alpha}\dot{\beta}}\nabla_aT_{bcij} + (-\mathcal{D}^\dagger\mathcal{I} - \frac{1}{2}\mathcal{D}\mathcal{H})i\Lambda_{\alpha i}\Lambda_{\beta l}\chi_{\gamma}{}^{kl}{}_j\epsilon^{\beta\gamma} \\
&+ (-\mathcal{D}^\dagger\mathcal{I} + \frac{1}{2}\mathcal{D}\mathcal{H})iE_{il}T_{ab}{}^{kl}\Lambda_{\beta j}\gamma_{ab\alpha}{}^\beta + (-\frac{1}{2}\mathcal{D}^\dagger\mathcal{I} - \frac{1}{4}\mathcal{D}\mathcal{H})iT_{ab}{}^{lm}T_{ab}{}^{kn}\Lambda_{\alpha n}\varepsilon_{ijlm} + (-\frac{1}{2}\mathcal{D}^\dagger\mathcal{I} + \frac{1}{4}\mathcal{D}\mathcal{H})i\Lambda_{\beta i}\Lambda_{\gamma j}R(Q)_{ab\alpha}{}^k\gamma_{ab}{}^{\beta\gamma} \\
&+ (\frac{1}{12}\mathcal{D}^\dagger\bar{\mathcal{H}} - \frac{1}{3}\mathcal{D}\bar{\mathcal{I}})iE^{kl}E^{mn}\Lambda_{\alpha m}\varepsilon_{ijln} + (\mathcal{D}^\dagger\mathcal{I} - \frac{1}{2}\mathcal{D}\mathcal{H})i\Lambda_{\beta i}\Lambda_{\gamma l}\chi_{\alpha}{}^{kl}{}_j\epsilon^{\beta\gamma} + (\mathcal{D}^\dagger\mathcal{I} + \frac{3}{2}\mathcal{D}\mathcal{H})i\Lambda_{\alpha l}\Lambda_{\beta i}\chi_{\gamma}{}^{kl}{}_j\epsilon^{\beta\gamma} \\
&+ iE^{kl}P_a\Lambda^{\dot{\alpha}m}\gamma_{a\alpha\dot{\alpha}}\mathcal{D}^\dagger\bar{\mathcal{I}}\varepsilon_{ijlm} + \frac{7}{24}iE^{kl}T_{ab}{}^{mn}\Lambda_{\beta i}\gamma_{ab\alpha}{}^\beta\mathcal{H}\varepsilon_{jlmn} - \frac{1}{16}iE^{kl}T_{ab}{}^{mn}\Lambda_{\beta l}\gamma_{ab\alpha}{}^\beta\mathcal{H}\varepsilon_{ijmn} - \frac{1}{24}iE^{kl}T_{ab}{}^{mn}\Lambda_{\beta m}\gamma_{ab\alpha}{}^\beta\mathcal{H}\varepsilon_{ijln} \\
&- iP_aT_{bcij}\Lambda^{\dot{\alpha}k}\gamma_{a\alpha}{}^{\dot{\beta}}\gamma_{bc\dot{\alpha}\dot{\beta}}\mathcal{D}^\dagger\bar{\mathcal{I}} - \frac{1}{2}i\Lambda^{\dot{\alpha}k}\Lambda^{\dot{\beta}l}\bar{\mathcal{I}}\chi_{\alpha}{}^{mn}{}_l\epsilon_{\dot{\alpha}\dot{\beta}}\varepsilon_{jlmn} - 2i\Lambda^{\dot{\alpha}k}\Lambda^{\dot{\beta}l}\bar{\mathcal{I}}\chi_{\alpha}{}^{mn}{}_l\epsilon_{\dot{\alpha}\dot{\beta}}\varepsilon_{ijmn} + \frac{3}{2}i\Lambda^{\dot{\alpha}l}\Lambda^{\dot{\beta}m}\bar{\mathcal{I}}\chi_{\alpha}{}^{kn}{}_l\epsilon_{\dot{\alpha}\dot{\beta}}\varepsilon_{ijmn} \\
&+ (-\bar{\mathcal{I}} - \frac{1}{4}\mathcal{D}^\dagger\mathcal{D}^\dagger\bar{\mathcal{H}})iT_{ab il}\Lambda_{\alpha j}\Lambda^{\dot{\alpha}k}\Lambda^{\dot{\beta}l}\gamma_{ab\dot{\alpha}\dot{\beta}} + (-\frac{1}{2}\mathcal{D}^\dagger\bar{\mathcal{H}} - \mathcal{D}\bar{\mathcal{I}})iT_{abij}\Lambda^{\dot{\alpha}k}\bar{P}_c\gamma_{c\alpha}{}^{\dot{\beta}}\gamma_{ab\dot{\alpha}\dot{\beta}} + (-\frac{1}{4}\mathcal{D}\mathcal{D}\mathcal{H} - 2\mathcal{I})iT_{ab}{}^{kl}\Lambda_{\alpha i}\Lambda_{\beta j}\Lambda_{\gamma l}\gamma_{ab}{}^{\beta\gamma} \\
&+ (-\frac{1}{8}\mathcal{D}^\dagger\bar{\mathcal{H}} - \frac{1}{4}\mathcal{D}\bar{\mathcal{I}})i\Lambda^{\dot{\alpha}k}\gamma_{a\beta\dot{\alpha}}\gamma_{bc\alpha}{}^\beta\nabla_aT_{bc}{}^{lm}\varepsilon_{ijlm} + (\frac{1}{8}\mathcal{D}^\dagger\bar{\mathcal{H}} + \frac{1}{4}\mathcal{D}\bar{\mathcal{I}})iT_{ab}{}^{lm}\gamma_{c\beta\dot{\alpha}}\gamma_{ab\alpha}{}^\beta\nabla_c\Lambda^{\dot{\alpha}k}\varepsilon_{ijlm} + (\frac{1}{6}\mathcal{D}^\dagger\bar{\mathcal{H}} + \frac{1}{3}\mathcal{D}\bar{\mathcal{I}})iE_{il}\Lambda_{\alpha j}\Lambda^{\dot{\alpha}k}\Lambda^{\dot{\beta}l}\epsilon_{\dot{\alpha}\dot{\beta}} \\
&+ (\frac{1}{6}\mathcal{D}^\dagger\bar{\mathcal{H}} + \frac{1}{3}\mathcal{D}\bar{\mathcal{I}})iE^{kl}\Lambda^{\dot{\alpha}m}\bar{P}_a\gamma_{a\alpha\dot{\alpha}}\varepsilon_{ijlm} + (\frac{1}{3}\mathcal{D}^\dagger\bar{\mathcal{H}} + \frac{2}{3}\mathcal{D}\bar{\mathcal{I}})iP_a\Lambda_{\alpha i}\Lambda_{\beta j}\Lambda^{\dot{\alpha}k}\gamma_a{}^\beta{}_{\dot{\alpha}} + (\frac{1}{3}\mathcal{D}^\dagger\mathcal{I} - \frac{1}{6}\mathcal{D}\mathcal{H})iE^{kl}\Lambda_{\alpha i}\Lambda_{\beta j}\Lambda_{\gamma l}\epsilon^{\beta\gamma} \\
&+ (\frac{1}{2}\mathcal{D}\mathcal{D}\mathcal{H} + \mathcal{I})iT_{ab}{}^{kl}\Lambda_{\alpha l}\Lambda_{\beta i}\Lambda_{\gamma j}\gamma_{ab}{}^{\beta\gamma} + (\frac{2}{3}\mathcal{D}^\dagger\mathcal{I} - \frac{1}{3}\mathcal{D}\mathcal{H})i\Lambda_{\alpha i}\Lambda_{\beta j}\Lambda^{\dot{\alpha}k}\bar{P}_a\gamma_a{}^\beta{}_{\dot{\alpha}} + (2\bar{\mathcal{I}} + \frac{1}{4}\mathcal{D}^\dagger\mathcal{D}^\dagger\bar{\mathcal{H}})iT_{abij}\Lambda_{\alpha l}\Lambda^{\dot{\alpha}k}\Lambda^{\dot{\beta}l}\gamma_{ab\dot{\alpha}\dot{\beta}} \\
&+ \frac{1}{4}iE_{il}\Lambda_{\alpha m}\Lambda_{\beta j}\Lambda_{\gamma n}\epsilon^{\beta\gamma}\mathcal{D}\mathcal{D}\mathcal{H}\varepsilon^{klmn} - iP_aT_{bc}{}^{kl}\Lambda^{\dot{\alpha}m}\bar{\mathcal{I}}\gamma_{a\beta\dot{\alpha}}\gamma_{bc\alpha}{}^\beta\varepsilon_{ijlm} - iP_aT_{bc}{}^{lm}\Lambda^{\dot{\alpha}k}\bar{\mathcal{I}}\gamma_{a\beta\dot{\alpha}}\gamma_{bc\alpha}{}^\beta\varepsilon_{ijlm} + \frac{1}{12}iT_{ab}{}^{kl}\Lambda^{\dot{\alpha}m}\bar{P}_c\gamma_{c\beta\dot{\alpha}}\gamma_{ab\alpha}{}^\beta\mathcal{H}\varepsilon_{ijlm} \\
&- \frac{1}{8}iT_{ab}{}^{lm}\Lambda^{\dot{\alpha}k}\bar{P}_c\gamma_{c\beta\dot{\alpha}}\gamma_{ab\alpha}{}^\beta\mathcal{H}\varepsilon_{ijlm} - i\Lambda^{\dot{\alpha}k}\Lambda^{\dot{\beta}l}\epsilon_{\dot{\alpha}\dot{\gamma}}\gamma_{a\alpha\dot{\beta}}\mathcal{D}^\dagger\bar{\mathcal{I}}\nabla_a\Lambda^{\dot{\gamma}m}\varepsilon_{ijlm} + (-2\bar{\mathcal{I}} - \frac{1}{8}\mathcal{D}^\dagger\mathcal{D}^\dagger\bar{\mathcal{H}})iE^{kl}\Lambda_{\alpha m}\Lambda^{\dot{\alpha}m}\Lambda^{\dot{\beta}n}\epsilon_{\dot{\alpha}\dot{\beta}}\varepsilon_{ijln} \\
&+ (\frac{1}{8}\mathcal{D}^\dagger\mathcal{I} - \frac{1}{16}\mathcal{D}\mathcal{H})iT_{ab}{}^{kl}T_{cd}{}^{mn}\Lambda_{\beta l}\gamma_{cd\alpha\gamma}\gamma_{ab}{}^{\beta\gamma}\varepsilon_{ijmn} + (\frac{1}{3}\bar{\mathcal{I}} + \frac{1}{8}\mathcal{D}^\dagger\mathcal{D}^\dagger\bar{\mathcal{H}})iE^{lm}\Lambda_{\alpha l}\Lambda^{\dot{\alpha}k}\Lambda^{\dot{\beta}n}\epsilon_{\dot{\alpha}\dot{\beta}}\varepsilon_{ijmn} \\
&+ (\frac{3}{8}\mathcal{D}^\dagger\mathcal{I} - \frac{3}{16}\mathcal{D}\mathcal{H})iT_{ab}{}^{kl}T_{cd}{}^{mn}\Lambda_{\beta i}\gamma_{cd\alpha\gamma}\gamma_{ab}{}^{\beta\gamma}\varepsilon_{jlmn} - \frac{1}{3}iP_a\Lambda^{\dot{\alpha}k}\Lambda^{\dot{\beta}l}\Lambda^{\dot{\gamma}m}\epsilon_{\dot{\alpha}\dot{\beta}}\gamma_{a\alpha\dot{\gamma}}\mathcal{D}^\dagger\mathcal{D}^\dagger\bar{\mathcal{I}}\varepsilon_{ijlm} \\
&- \frac{1}{2}i\Lambda_{\alpha i}\Lambda_{\beta j}\Lambda^{\dot{\alpha}k}\Lambda^{\dot{\beta}l}\Lambda_{\gamma l}\epsilon^{\beta\gamma}\epsilon_{\dot{\alpha}\dot{\beta}}\mathcal{H} + \frac{4}{3}i\Lambda^{\dot{\alpha}k}\Lambda^{\dot{\beta}l}\Lambda^{\dot{\gamma}m}\bar{P}_a\bar{\mathcal{I}}\epsilon_{\dot{\alpha}\dot{\beta}}\gamma_{a\alpha\dot{\gamma}}\varepsilon_{ijlm} + (-\frac{1}{8}\mathcal{D}^\dagger\bar{\mathcal{H}} - \frac{1}{4}\mathcal{D}\bar{\mathcal{I}})iT_{ab}{}^{lm}\Lambda_{\beta n}\Lambda^{\dot{\alpha}k}\Lambda^{\dot{\beta}n}\epsilon_{\dot{\alpha}\dot{\beta}}\gamma_{ab\alpha}{}^\beta\varepsilon_{ijlm} \\
&- \frac{1}{24}i\Lambda_{\alpha l}\Lambda_{\beta i}\Lambda_{\gamma j}\Lambda_{\delta m}\Lambda_{\epsilon n}\epsilon^{\beta\delta}\epsilon^{\gamma\epsilon}\mathcal{D}\mathcal{D}\mathcal{D}\mathcal{H}\varepsilon^{klmn} + (-\mathcal{D}^\dagger\bar{\mathcal{I}} - \frac{1}{24}\mathcal{D}^\dagger\mathcal{D}^\dagger\bar{\mathcal{H}})i\Lambda_{\alpha l}\Lambda^{\dot{\alpha}k}\Lambda^{\dot{\beta}l}\Lambda^{\dot{\gamma}m}\Lambda^{\dot{\delta}n}\epsilon_{\dot{\alpha}\dot{\gamma}}\epsilon_{\dot{\beta}\dot{\delta}}\varepsilon_{ijmn}
\end{aligned}$$

$$\begin{aligned}
\kappa_{\alpha ij}{}^k = & -2iE_{il}\chi_{\alpha}{}^{kl}{}_j\mathcal{D}^{\dagger}\mathcal{I} + (\bar{\mathcal{H}} - \mathcal{H})i\gamma_{a\alpha\dot{\alpha}}\nabla_a\chi^{\dot{\alpha}}{}_{ij}{}^k + (\mathcal{D}^{\dagger}\mathcal{I} + \mathcal{D}\mathcal{H})i\mathcal{D}^{kl}{}_{ij}\Lambda_{\alpha l} + \frac{1}{2}iE_{il}E^{kl}\Lambda_{\alpha j}\mathcal{D}^{\dagger}\mathcal{I} - 2iP_a\chi^{\dot{\alpha}}{}_{ij}{}^k\gamma_{a\alpha\dot{\alpha}}\mathcal{D}\bar{\mathcal{I}} \\
& - \frac{1}{2}iT_{ab}{}^{kl}R(Q)_{ab\alpha}{}^m\mathcal{D}^{\dagger}\mathcal{I}\varepsilon_{ijlm} + \frac{3}{4}iT_{ab}{}^{lm}R(Q)_{ab\alpha}{}^k\mathcal{D}^{\dagger}\mathcal{I}\varepsilon_{ijlm} - i\Lambda_{\beta i}R(V)_{ab}{}^k{}_j\gamma_{ab\alpha}{}^{\beta}\mathcal{D}^{\dagger}\mathcal{I} + (\frac{1}{2}\bar{\mathcal{H}} - \frac{1}{2}\mathcal{H})iE^{kl}\chi_{\alpha}{}^{mn}{}_l\varepsilon_{ijmn} \\
& + \frac{1}{8}iE_{il}E_{jm}\Lambda_{\alpha n}\mathcal{D}\mathcal{D}\mathcal{H}\varepsilon^{klmn} - \frac{1}{2}iE^{kl}\gamma_{a\alpha\dot{\alpha}}\mathcal{D}\bar{\mathcal{I}}\nabla_a\Lambda^{\dot{\alpha}m}\varepsilon_{ijlm} + \frac{1}{2}iT_{abij}\gamma_{c\alpha}{}^{\dot{\alpha}}\gamma_{ab\dot{\alpha}\beta}\mathcal{D}\bar{\mathcal{I}}\nabla_c\Lambda^{\dot{\beta}k} - \frac{1}{8}iT_{ab}{}^{kl}\chi_{\beta}{}^{mn}{}_l\gamma_{ab\alpha}{}^{\beta}\mathcal{D}^{\dagger}\mathcal{I}\varepsilon_{ijmn} \\
& - \frac{3}{4}iT_{ab}{}^{lm}\chi_{\beta}{}^{kn}{}_i\gamma_{ab\alpha}{}^{\beta}\mathcal{D}^{\dagger}\mathcal{I}\varepsilon_{jlmn} - 2i\Lambda_{\alpha i}\Lambda^{\dot{\alpha}l}\bar{\mathcal{H}}\chi^{\dot{\beta}}{}_{jl}{}^k\epsilon_{\dot{\alpha}\dot{\beta}} - 2i\Lambda_{\alpha l}\Lambda^{\dot{\alpha}l}\bar{\mathcal{H}}\chi^{\dot{\beta}}{}_{ij}{}^k\epsilon_{\dot{\alpha}\dot{\beta}} - i\Lambda_{\beta i}\Lambda^{\dot{\alpha}k}\gamma_a{}^{\beta}{}_{\dot{\alpha}}\mathcal{D}^{\dagger}\mathcal{I}\nabla_a\Lambda_{\alpha j} \\
& + \frac{1}{2}i\Lambda^{\dot{\alpha}l}\gamma_{a\alpha\dot{\alpha}}\mathcal{D}\bar{\mathcal{I}}\nabla_aE^{km}\varepsilon_{ijlm} + \frac{1}{2}i\Lambda^{\dot{\alpha}k}\gamma_{a\alpha}{}^{\dot{\beta}}\gamma_{bc\dot{\alpha}\dot{\beta}}\mathcal{D}\bar{\mathcal{I}}\nabla_aT_{bcij} + (-\frac{1}{2}\bar{\mathcal{H}} - \frac{1}{2}\mathcal{H})iT_{ablm}T_{abij}\Lambda_{\alpha n}\varepsilon^{klmn} \\
& + (-\frac{1}{4}\mathcal{D}\mathcal{D}\mathcal{H} - 2\mathcal{I})i\Lambda_{\beta i}\Lambda_{\gamma l}\chi_{\alpha}{}^{kl}{}_j\epsilon^{\beta\gamma} + (-\frac{1}{4}\mathcal{D}\mathcal{D}\mathcal{H} + 2\mathcal{I})i\Lambda_{\alpha i}\Lambda_{\beta l}\chi_{\gamma}{}^{kl}{}_j\epsilon^{\beta\gamma} + (-\frac{1}{8}\mathcal{D}\mathcal{D}\mathcal{H} + \mathcal{I})iT_{ab}{}^{lm}T_{ab}{}^{kn}\Lambda_{\alpha n}\varepsilon_{ijlm} \\
& + (\frac{1}{8}\mathcal{D}\mathcal{D}\mathcal{H} + \mathcal{I})i\Lambda_{\beta i}\Lambda_{\gamma j}R(Q)_{ab\alpha}{}^k\gamma_{ab}{}^{\beta\gamma} + (\frac{1}{4}\mathcal{D}\mathcal{D}\mathcal{H} + 2\mathcal{I})iE_{il}T_{ab}{}^{kl}\Lambda_{\beta j}\gamma_{ab\alpha}{}^{\beta} + (\frac{5}{12}\bar{\mathcal{H}} + \frac{1}{12}\mathcal{H})iE^{kl}E^{mn}\Lambda_{\alpha m}\varepsilon_{ijln} \\
& + (\frac{3}{4}\mathcal{D}\mathcal{D}\mathcal{H} - 2\mathcal{I})i\Lambda_{\alpha l}\Lambda_{\beta i}\chi_{\gamma}{}^{kl}{}_j\epsilon^{\beta\gamma} + (\bar{\mathcal{H}} + \mathcal{H})i\Lambda_{\alpha l}\Lambda^{\dot{\alpha}k}\chi^{\dot{\beta}}{}_{ij}{}^l\epsilon_{\dot{\alpha}\dot{\beta}} - \frac{7}{24}iE^{kl}T_{ab}{}^{mn}\Lambda_{\beta i}\gamma_{ab\alpha}{}^{\beta}\mathcal{D}^{\dagger}\mathcal{I}\varepsilon_{jlmn} + \frac{1}{16}iE^{kl}T_{ab}{}^{mn}\Lambda_{\beta l}\gamma_{ab\alpha}{}^{\beta}\mathcal{D}^{\dagger}\mathcal{I}\varepsilon_{ijmn} \\
& + \frac{1}{24}iE^{kl}T_{ab}{}^{mn}\Lambda_{\beta m}\gamma_{ab\alpha}{}^{\beta}\mathcal{D}^{\dagger}\mathcal{I}\varepsilon_{ijln} - iT_{ab}{}^{kl}\Lambda_{\alpha i}\Lambda_{\beta j}\Lambda_{\gamma l}\gamma_{ab}{}^{\beta\gamma}\mathcal{D}\bar{\mathcal{I}} + \frac{1}{4}i\Lambda^{\dot{\alpha}k}\Lambda^{\dot{\beta}l}\chi_{\alpha}{}^{mn}{}_i\epsilon_{\dot{\alpha}\dot{\beta}}\mathcal{D}\bar{\mathcal{I}}\varepsilon_{jlmn} + i\Lambda^{\dot{\alpha}k}\Lambda^{\dot{\beta}l}\chi_{\alpha}{}^{mn}{}_l\epsilon_{\dot{\alpha}\dot{\beta}}\mathcal{D}\bar{\mathcal{I}}\varepsilon_{ijmn} \\
& - \frac{3}{4}i\Lambda^{\dot{\alpha}l}\Lambda^{\dot{\beta}m}\chi_{\alpha}{}^{kn}{}_l\epsilon_{\dot{\alpha}\dot{\beta}}\mathcal{D}\bar{\mathcal{I}}\varepsilon_{ijmn} + (-2\bar{\mathcal{I}} - \frac{1}{4}\mathcal{D}^{\dagger}\mathcal{D}^{\dagger}\bar{\mathcal{H}})iP_aT_{bcij}\Lambda^{\dot{\alpha}k}\gamma_{a\alpha}{}^{\dot{\beta}}\gamma_{bc\dot{\alpha}\dot{\beta}} + (-\frac{1}{2}\mathcal{D}^{\dagger}\bar{\mathcal{H}} + \frac{1}{2}\mathcal{D}\bar{\mathcal{I}})iT_{ab}{}^{kl}\Lambda_{\alpha j}\Lambda^{\dot{\alpha}k}\Lambda^{\dot{\beta}l}\gamma_{ab\dot{\alpha}\dot{\beta}} \\
& + (-\frac{1}{3}\bar{\mathcal{H}} + \frac{1}{3}\mathcal{H})iP_a\Lambda_{\alpha i}\Lambda_{\beta j}\Lambda^{\dot{\alpha}k}\gamma_a{}^{\beta}{}_{\dot{\alpha}} + (-\frac{1}{6}\bar{\mathcal{H}} + \frac{1}{6}\mathcal{H})iE_{il}\Lambda_{\alpha j}\Lambda^{\dot{\alpha}k}\Lambda^{\dot{\beta}l}\epsilon_{\dot{\alpha}\dot{\beta}} + (-\frac{1}{6}\bar{\mathcal{H}} + \frac{1}{6}\mathcal{H})iE^{kl}\Lambda^{\dot{\alpha}m}\bar{P}_a\gamma_{a\alpha\dot{\alpha}}\varepsilon_{ijlm} \\
& + (-\frac{1}{6}\mathcal{D}\mathcal{D}\mathcal{H} - \frac{4}{3}\mathcal{I})i\Lambda_{\alpha i}\Lambda_{\beta j}\Lambda^{\dot{\alpha}k}\bar{P}_a\gamma_a{}^{\beta}{}_{\dot{\alpha}} + (-\frac{1}{8}\bar{\mathcal{H}} + \frac{1}{8}\mathcal{H})iT_{ab}{}^{lm}\gamma_{c\beta\dot{\alpha}}\gamma_{ab\alpha}{}^{\beta}\nabla_c\Lambda^{\dot{\alpha}k}\varepsilon_{ijlm} + (-\frac{1}{12}\mathcal{D}\mathcal{D}\mathcal{H} - \frac{2}{3}\mathcal{I})iE^{kl}\Lambda_{\alpha i}\Lambda_{\beta j}\Lambda_{\gamma l}\epsilon^{\beta\gamma} \\
& + (\frac{1}{8}\bar{\mathcal{H}} - \frac{1}{8}\mathcal{H})i\Lambda^{\dot{\alpha}k}\gamma_{a\beta\dot{\alpha}}\gamma_{b\alpha}{}^{\beta}\nabla_aT_{bc}{}^{lm}\varepsilon_{ijlm} + (\frac{1}{8}\mathcal{D}\mathcal{D}\mathcal{D}\mathcal{H} + \frac{1}{2}\mathcal{D}\mathcal{I})iT_{ab}{}^{kl}\Lambda_{\alpha l}\Lambda_{\beta i}\Lambda_{\gamma j}\gamma_{ab}{}^{\beta\gamma} + (\frac{1}{2}\bar{\mathcal{H}} - \frac{1}{2}\mathcal{H})iT_{abij}\Lambda^{\dot{\alpha}k}\bar{P}_c\gamma_{c\alpha}{}^{\dot{\beta}}\gamma_{ab\dot{\alpha}\dot{\beta}} \\
& + (\frac{1}{2}\mathcal{D}^{\dagger}\bar{\mathcal{H}} - \mathcal{D}\bar{\mathcal{I}})iT_{abij}\Lambda_{\alpha l}\Lambda^{\dot{\alpha}k}\Lambda^{\dot{\beta}l}\gamma_{ab\dot{\alpha}\dot{\beta}} + (2\bar{\mathcal{I}} + \frac{1}{4}\mathcal{D}^{\dagger}\mathcal{D}^{\dagger}\bar{\mathcal{H}})iE^{kl}P_a\Lambda^{\dot{\alpha}m}\gamma_{a\alpha\dot{\alpha}}\varepsilon_{ijlm} + \frac{1}{12}iE_{il}\Lambda_{\alpha m}\Lambda_{\beta j}\Lambda_{\gamma n}\epsilon^{\beta\gamma}\mathcal{D}\mathcal{D}\mathcal{D}\mathcal{H}\varepsilon^{klmn} \\
& + \frac{1}{2}iP_aT_{bc}{}^{kl}\Lambda^{\dot{\alpha}m}\gamma_{a\beta\dot{\alpha}}\gamma_{b\alpha}{}^{\beta}\mathcal{D}\bar{\mathcal{I}}\varepsilon_{ijlm} + \frac{1}{2}iP_aT_{bc}{}^{lm}\Lambda^{\dot{\alpha}k}\gamma_{a\beta\dot{\alpha}}\gamma_{b\alpha}{}^{\beta}\mathcal{D}\bar{\mathcal{I}}\varepsilon_{ijlm} - \frac{1}{12}iT_{ab}{}^{kl}\Lambda^{\dot{\alpha}m}\bar{P}_c\gamma_{c\beta\dot{\alpha}}\gamma_{ab\alpha}{}^{\beta}\mathcal{D}^{\dagger}\mathcal{I}\varepsilon_{ijlm} \\
& + \frac{1}{8}iT_{ab}{}^{lm}\Lambda^{\dot{\alpha}k}\bar{P}_c\gamma_{c\beta\dot{\alpha}}\gamma_{ab\alpha}{}^{\beta}\mathcal{D}^{\dagger}\mathcal{I}\varepsilon_{ijlm} + (-2\bar{\mathcal{I}} - \frac{1}{4}\mathcal{D}^{\dagger}\mathcal{D}^{\dagger}\bar{\mathcal{H}})i\Lambda^{\dot{\alpha}k}\Lambda^{\dot{\beta}l}\epsilon_{\dot{\alpha}\dot{\gamma}}\gamma_{a\alpha\dot{\gamma}}\nabla_a\Lambda^{\dot{\gamma}m}\varepsilon_{ijlm} + (-\frac{1}{4}\mathcal{D}^{\dagger}\bar{\mathcal{H}} + \mathcal{D}\bar{\mathcal{I}})iE^{kl}\Lambda_{\alpha m}\Lambda^{\dot{\alpha}m}\Lambda^{\dot{\beta}n}\epsilon_{\dot{\alpha}\dot{\beta}}\varepsilon_{ijln} \\
& + (-\frac{3}{32}\mathcal{D}\mathcal{D}\mathcal{H} - \frac{3}{4}\mathcal{I})iT_{ab}{}^{kl}T_{cd}{}^{mn}\Lambda_{\beta i}\gamma_{cd\alpha\gamma}\gamma_{ab}{}^{\beta\gamma}\varepsilon_{jlmn} + (-\frac{1}{32}\mathcal{D}\mathcal{D}\mathcal{H} - \frac{1}{4}\mathcal{I})iT_{ab}{}^{kl}T_{cd}{}^{mn}\Lambda_{\beta l}\gamma_{cd\alpha\gamma}\gamma_{ab}{}^{\beta\gamma}\varepsilon_{ijmn} \\
& + (\frac{1}{4}\mathcal{D}^{\dagger}\bar{\mathcal{H}} - \frac{1}{6}\mathcal{D}\bar{\mathcal{I}})iE^{lm}\Lambda_{\alpha l}\Lambda^{\dot{\alpha}k}\Lambda^{\dot{\beta}n}\epsilon_{\dot{\alpha}\dot{\beta}}\varepsilon_{ijmn} + \frac{1}{2}i\Lambda_{\alpha i}\Lambda_{\beta j}\Lambda^{\dot{\alpha}k}\Lambda^{\dot{\beta}l}\Lambda_{\gamma l}\epsilon^{\beta\gamma}\epsilon_{\dot{\alpha}\dot{\beta}}\mathcal{D}^{\dagger}\mathcal{I} - \frac{2}{3}i\Lambda^{\dot{\alpha}k}\Lambda^{\dot{\beta}l}\Lambda^{\dot{\gamma}m}\bar{P}_a\epsilon_{\dot{\alpha}\dot{\beta}}\gamma_{a\alpha\dot{\gamma}}\mathcal{D}\bar{\mathcal{I}}\varepsilon_{ijlm} \\
& + (-\mathcal{D}^{\dagger}\bar{\mathcal{I}} - \frac{1}{12}\mathcal{D}^{\dagger}\mathcal{D}^{\dagger}\bar{\mathcal{H}})iP_a\Lambda^{\dot{\alpha}k}\Lambda^{\dot{\beta}l}\Lambda^{\dot{\gamma}m}\epsilon_{\dot{\alpha}\dot{\beta}}\gamma_{a\alpha\dot{\gamma}}\varepsilon_{ijlm} + (\frac{1}{8}\bar{\mathcal{H}} - \frac{1}{8}\mathcal{H})iT_{ab}{}^{lm}\Lambda_{\beta n}\Lambda^{\dot{\alpha}k}\Lambda^{\dot{\beta}n}\epsilon_{\dot{\alpha}\dot{\beta}}\gamma_{ab\alpha}{}^{\beta}\varepsilon_{ijlm} \\
& - \frac{1}{96}i\Lambda_{\alpha l}\Lambda_{\beta i}\Lambda_{\gamma j}\Lambda_{\delta m}\Lambda_{\epsilon n}\epsilon^{\beta\delta}\epsilon^{\gamma\epsilon}\mathcal{D}\mathcal{D}\mathcal{D}\mathcal{D}\mathcal{H}\varepsilon^{klmn} + (-2\bar{\mathcal{I}} - \frac{3}{8}\mathcal{D}^{\dagger}\mathcal{D}^{\dagger}\bar{\mathcal{H}})i\Lambda_{\alpha l}\Lambda^{\dot{\alpha}k}\Lambda^{\dot{\beta}l}\Lambda^{\dot{\gamma}m}\Lambda^{\dot{\delta}n}\epsilon_{\dot{\alpha}\dot{\gamma}}\epsilon_{\dot{\beta}\dot{\delta}}\varepsilon_{ijmn}
\end{aligned}$$
